# Supplementary material for: A search for cool molecular gas in GK Persei and other classical novae
Source: arXiv:2201.10332 source file (2022-01-25)

1;1 CG-CMA CO(3-2) AP-F302-XF0- O:24-AUG-2014 R:12-AUG-2020
RA: 07:04:05.05 DEC: -23:45:34.6 Eq 2000.0 Rad. 0.0° Offs: +0.0 -0.2
Unknown tau: 0.115 Tsys: 180. Time: 23.3min El: 47.3
N: 116 I0: 58.7548 V0: 0.000 Dv: -29.77 LSR
F0: 345796.000 Df: 34.33 Fi: 333795.769

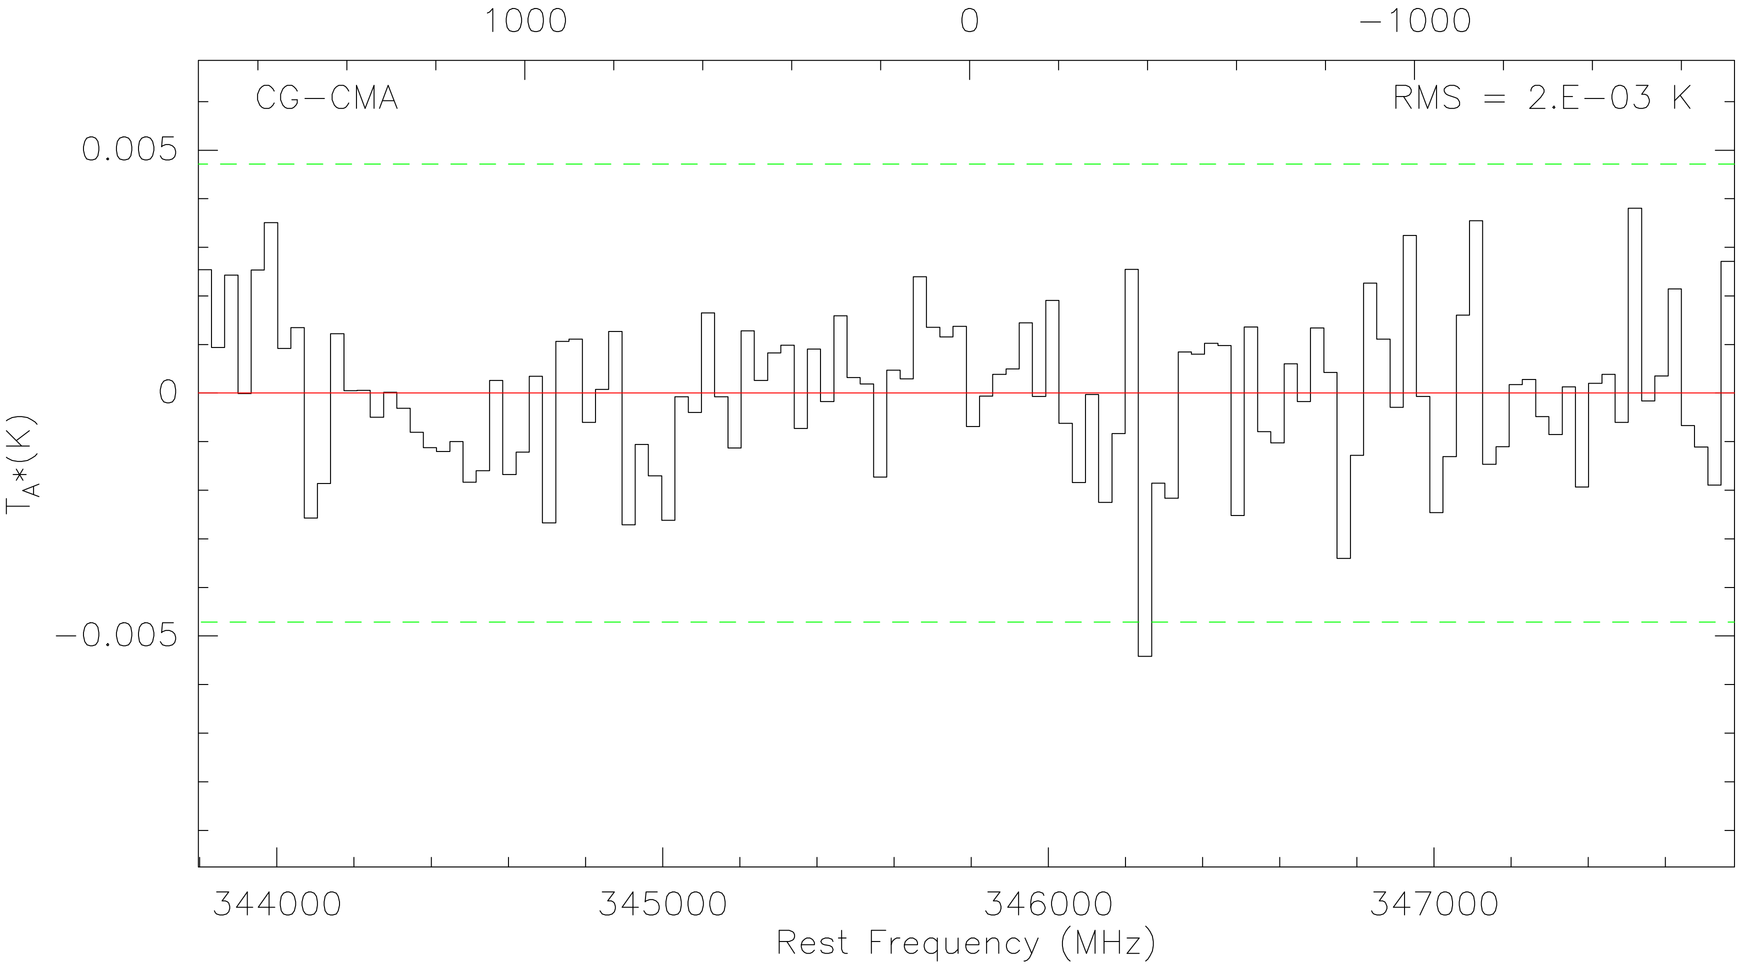

1;1 CN-VEL CO(3-2) AP-F302-XF0- O:24-AUG-2014 R:12-AUG-2020
RA: 11:02:38.57 DEC: -54:23:09.5 Eq 2000.0 Rad. 0.0° Offs: -0.1 -0.5
Unknown tau: 0.158 Tsys: 199. Time: 23.4min El: 50.6
N: 116 I0: 58.7552 V0: 0.000 Dv: 29.77 LSR
F0: 345795.990 Df: -34.33 Fi: 333795.043

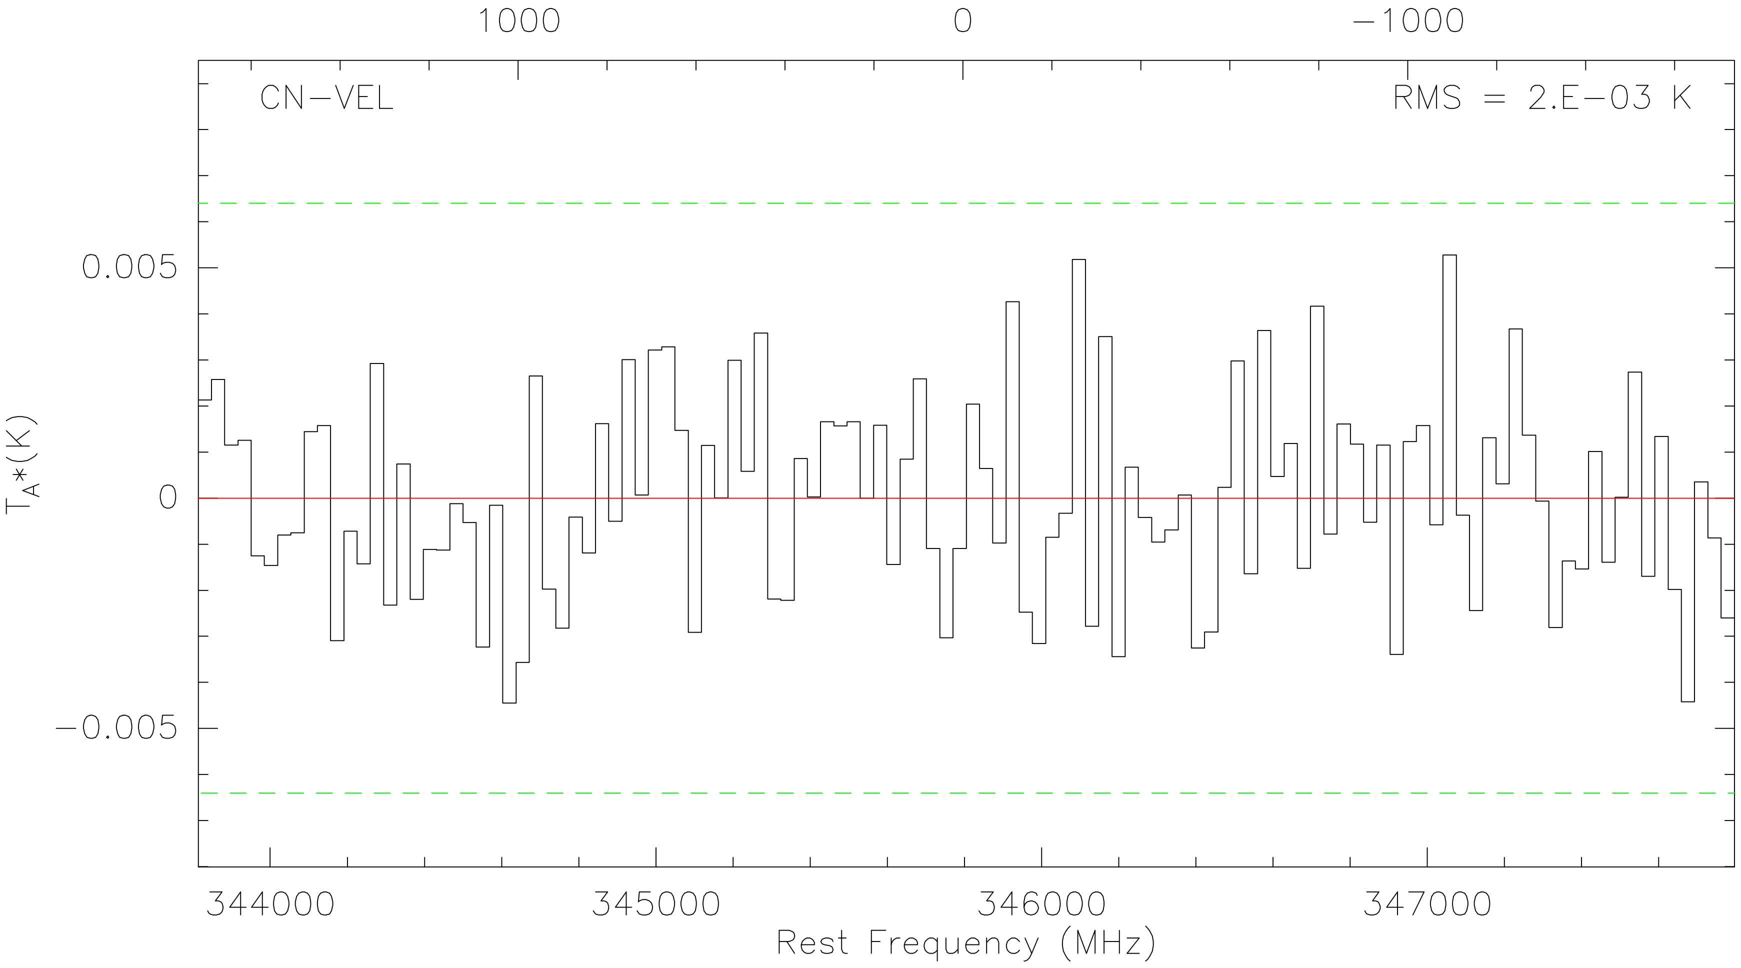

1;1 CQ-VEL CO(3-2) AP-F302-XF0- O:26-AUG-2014 R:12-AUG-2020
RA: 08:58:50.99 DEC: -53:20:17.8 Eq 2000.0 Rad. 0.0° Offs: +0.1 -0.5
Unknown tau: 0.104 Tsys: 176. Time: 23.4min El: 58.6
N: 116 I0: 58.7552 V0: 0.000 Dv: 29.77 LSR
F0: 345795.990 Df: -34.33 Fi: 333795.226

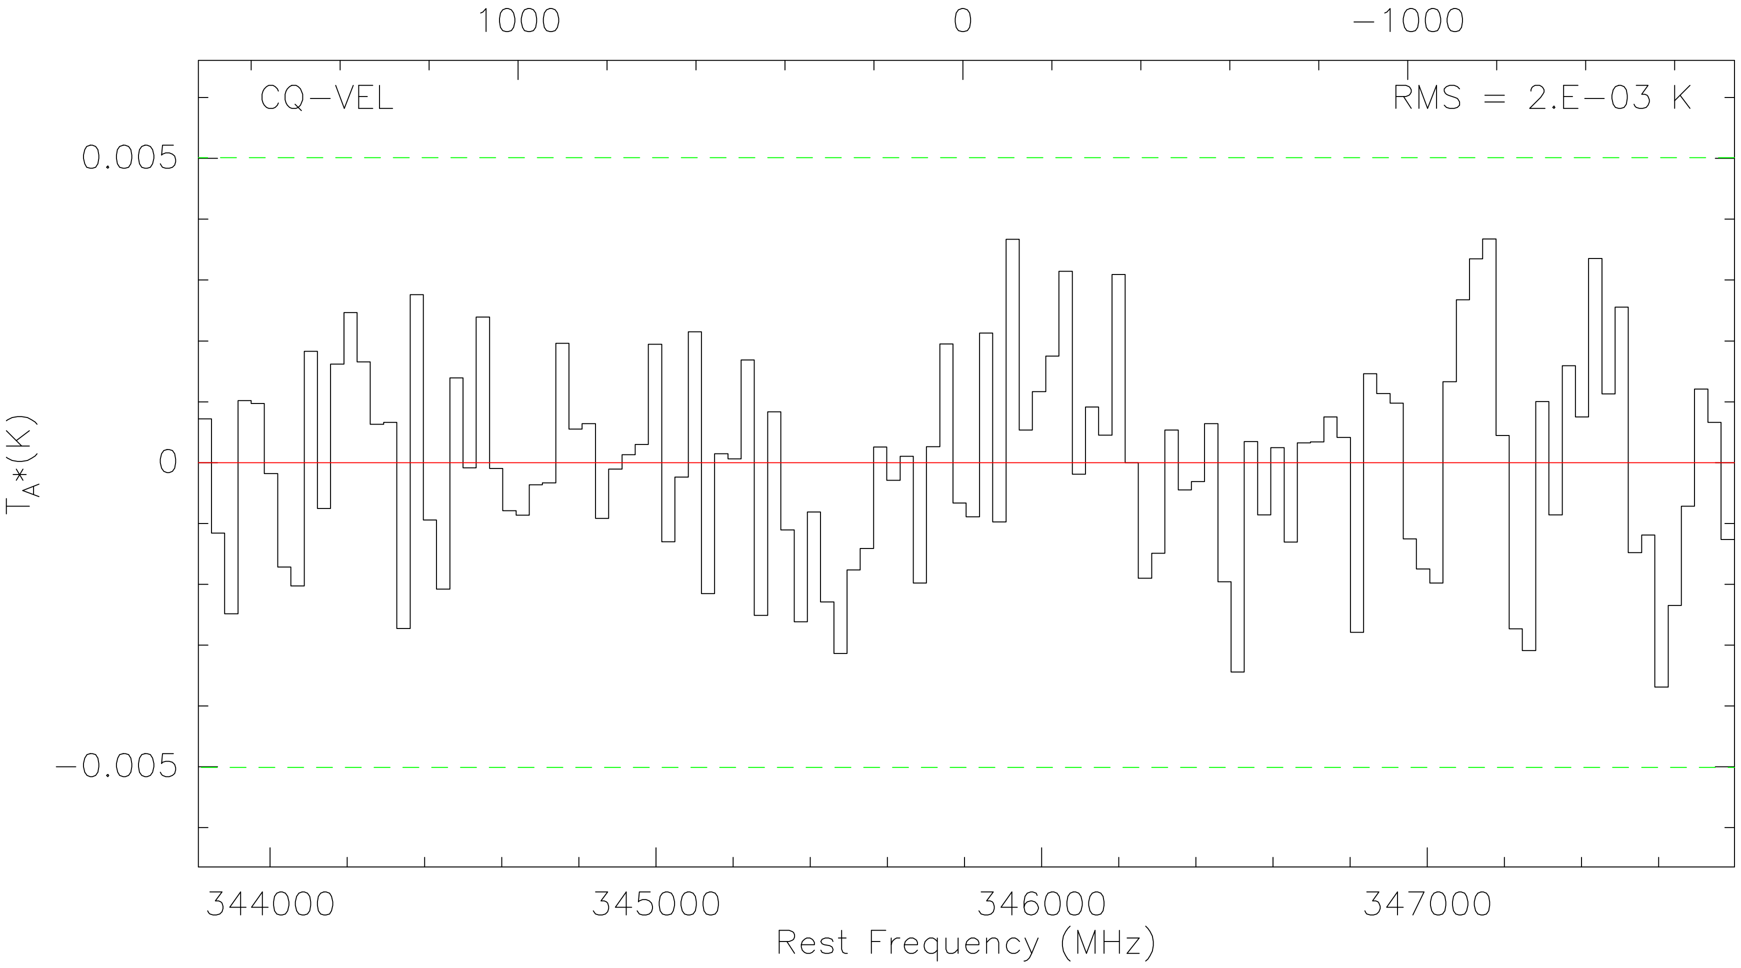

1;1 DY-PUP CO(3-2) AP-F302-XF0- O:25-AUG-2014 R:12-AUG-2020
RA: 08:13:48.51 DEC: -26:33:56.5 Eq 2000.0 Rad. 0.0° Offs: +0.2 -0.2
Unknown tau: 0.096 Tsys: 162. Time: 23.5min El: 65.1
N: 116 I0: 58.7552 V0: 0.000 Dv: 29.77 LSR
F0: 345795.990 Df: -34.33 Fi: 333795.562

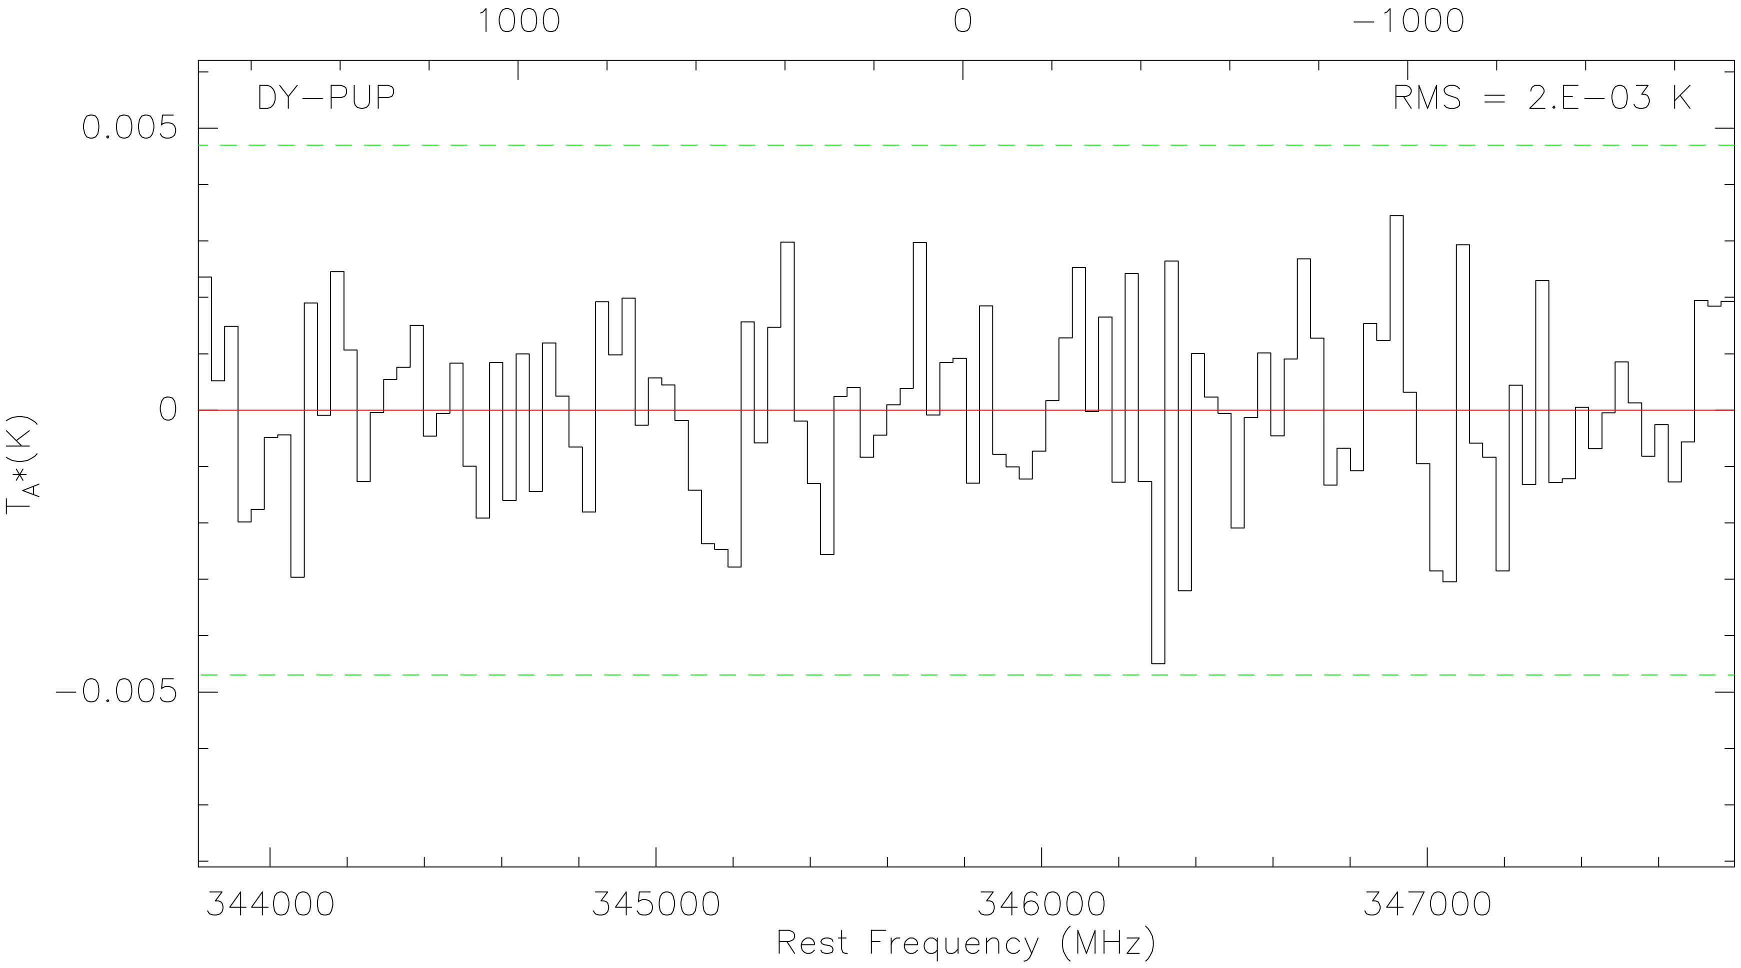

1;1 GQ–MUS CO(3–2) AP–F302–XF0– 0:28–AUG–2014 R:12–AUG–2020
RA: 11:52:02.35 DEC: –67:12:20.2 Eq 2000.0 Rad. 0.0° Offs: +0.1 –0.4
Unknown tau: 0.182 Tsys: 230. Time: 20.4min El: 45.6
N: 116 I0: 58.7548 V0: 0.000 Dv: –29.77 LSR
F0: 345796.000 Df: 34.33 Fi: 333795.049

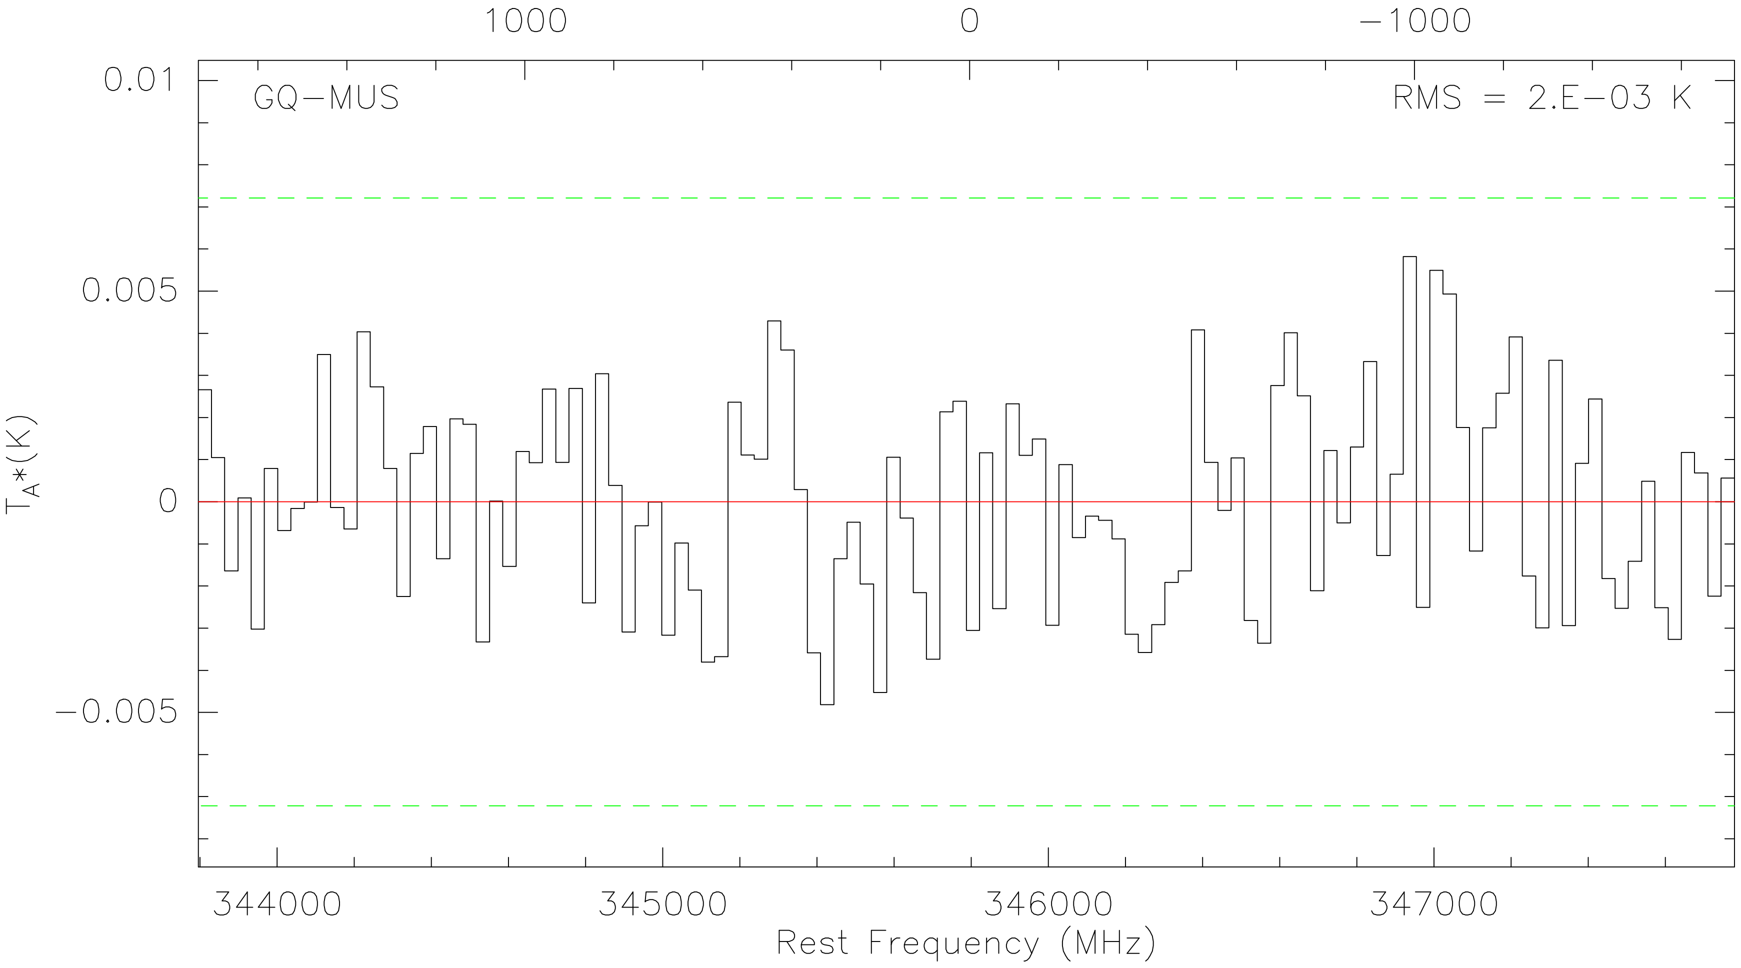

1;1 GU-MUS CO(3-2) AP-F302-XF0- O:24-AUG-2014 R:12-AUG-2020
RA: 11:26:26.60 DEC: -68:40:32.3 Eq 2000.0 Rad. 0.0° Offs: -0.2 -0.4
Unknown tau: 0.146 Tsys: 230. Time: 23.3min El: 37.6
N: 116 I0: 58.7552 V0: 0.000 Dv: 29.77 LSR
F0: 345795.990 Df: -34.34 Fi: 333795.038

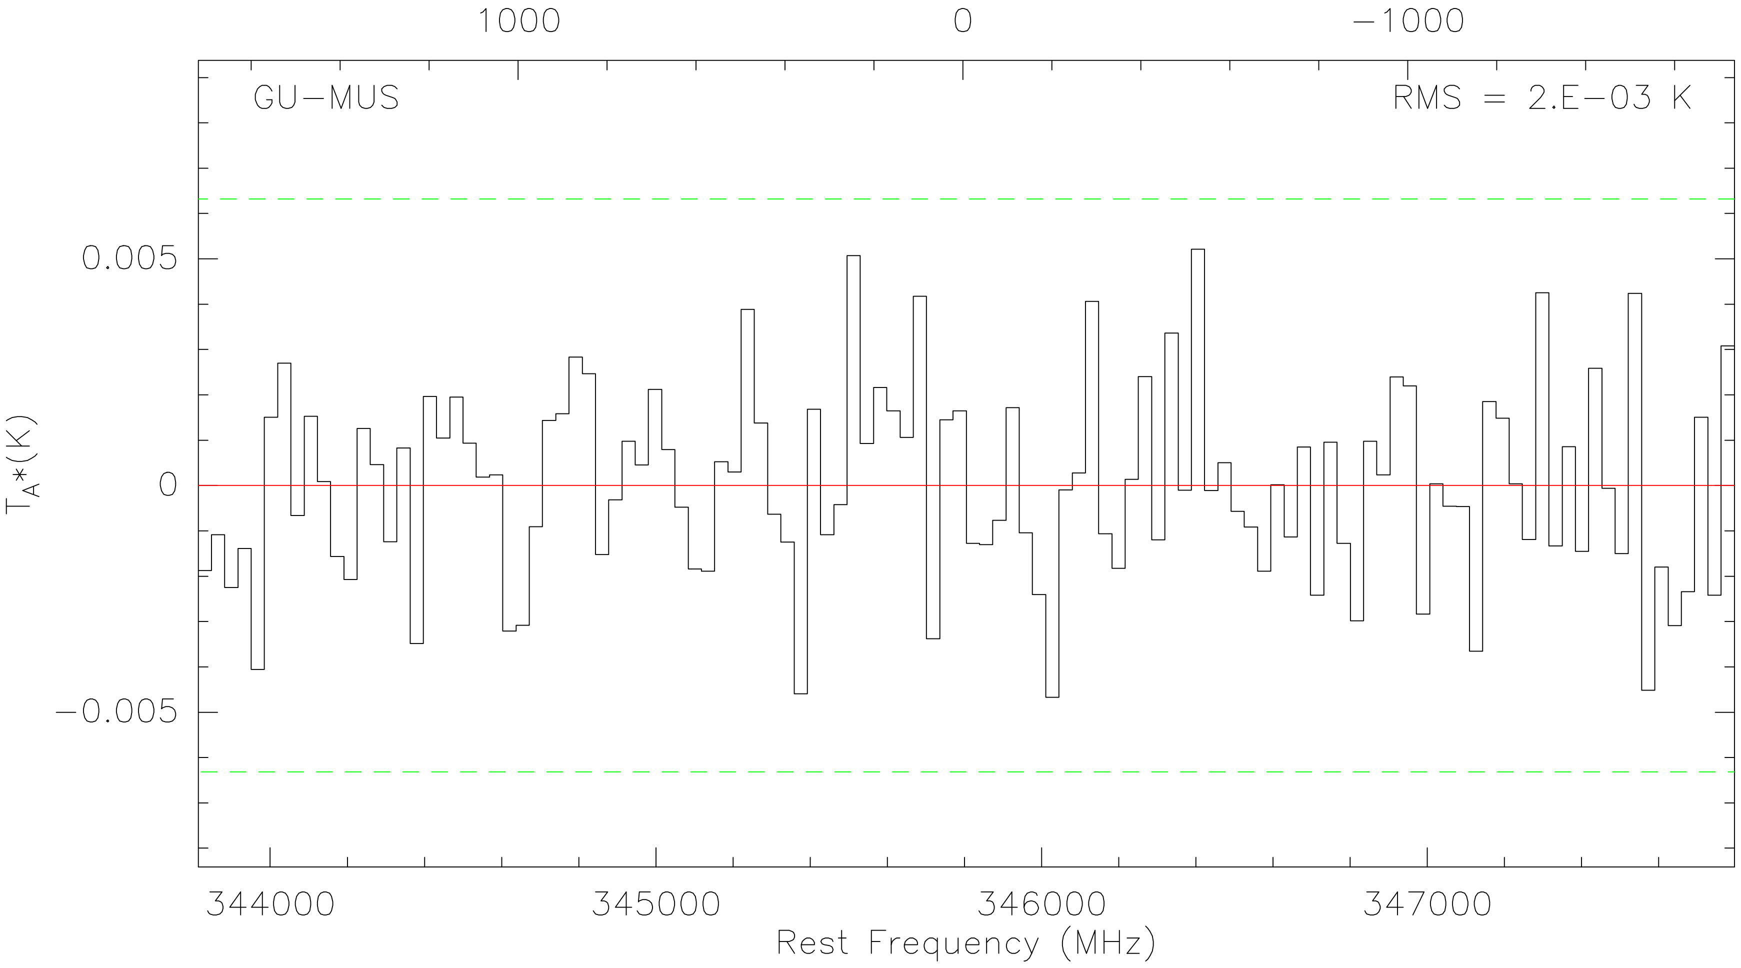

1;1 LZ-MUS CO(3-2) AP-F302-XF0- O:24-AUG-2014 R:12-AUG-2020
RA: 11:56:09.27 DEC: -65:34:20.1 Eq 2000.0 Rad. 0.0° Offs: -0.2 -0.4
Unknown tau: 0.186 Tsys: 254. Time: 23.4min El: 36.6
N: 116 I0: 58.7552 V0: 0.000 Dv: 29.77 LSR
F0: 345795.990 Df: -34.34 Fi: 333795.012

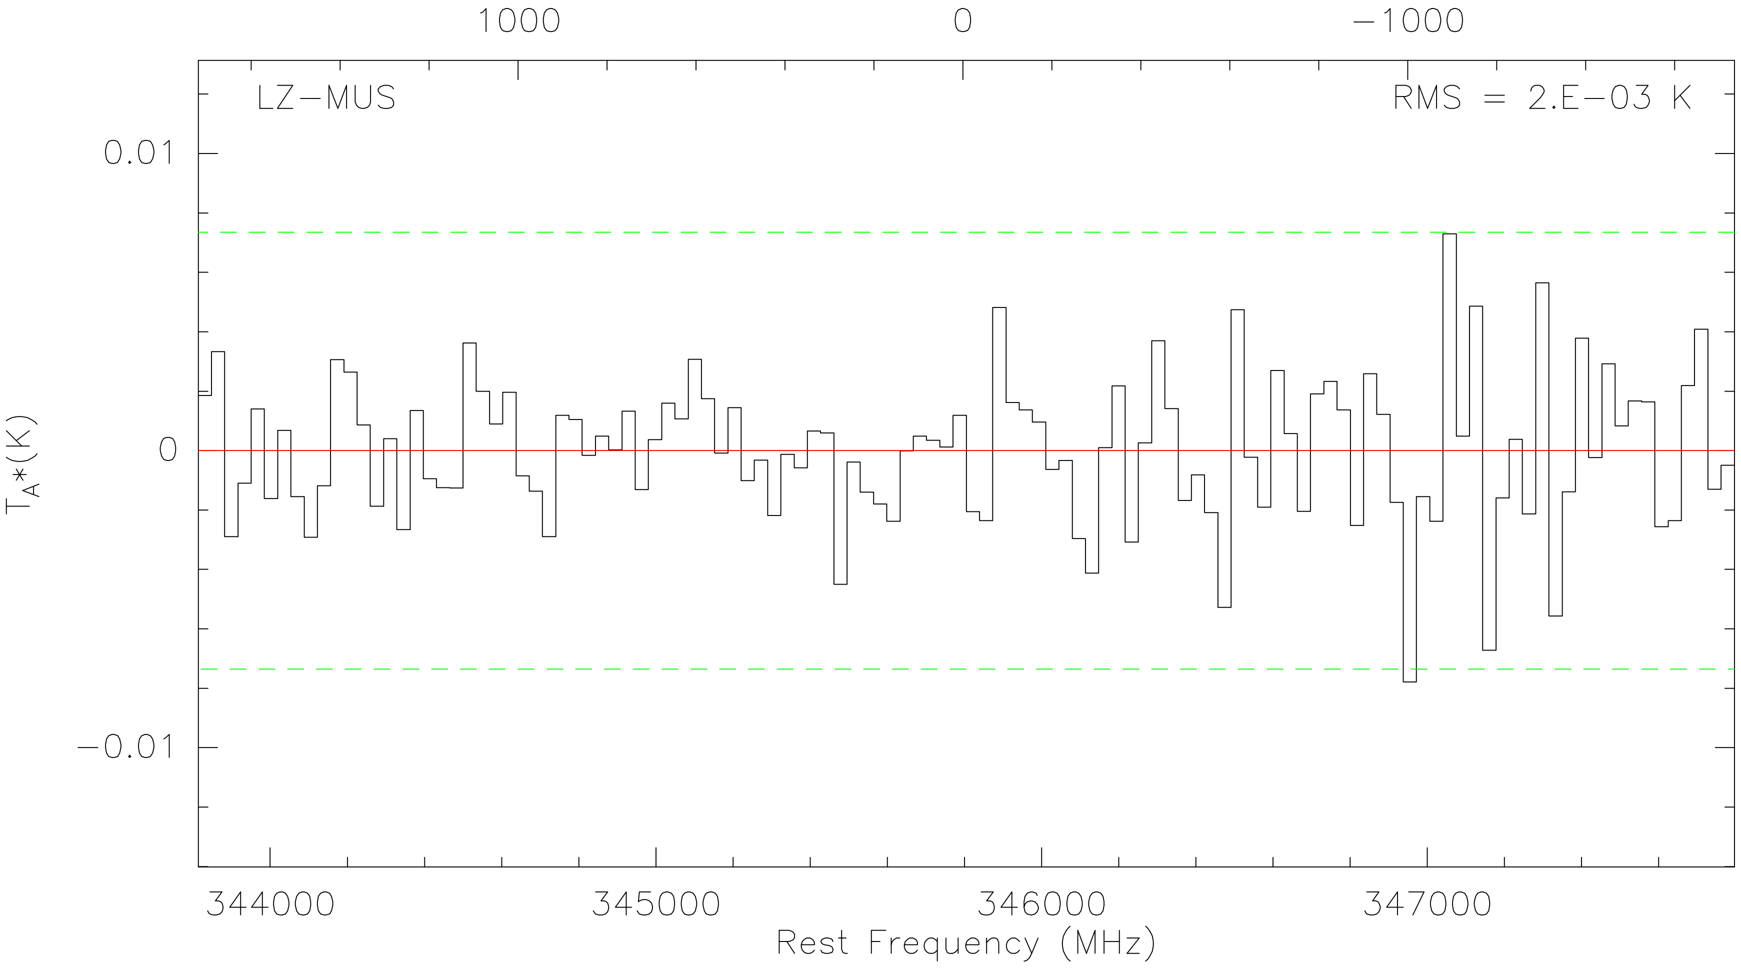

1;1 RR–PIC CO(3–2) AP–F302–XF0– O:25–AUG–2014 R:12–AUG–2020
RA: 06:35:36.06 DEC: –62:38:24.3 Eq 2000.0 Rad. 0.0° Offs: +0.3 –0.2
Unknown tau: 0.107 Tsys: 182. Time: 23.3min El: 42.4
N: 116 I0: 58.7552 V0: 0.000 Dv: 29.77 LSR
F0: 345795.990 Df: –34.33 Fi: 333795.352

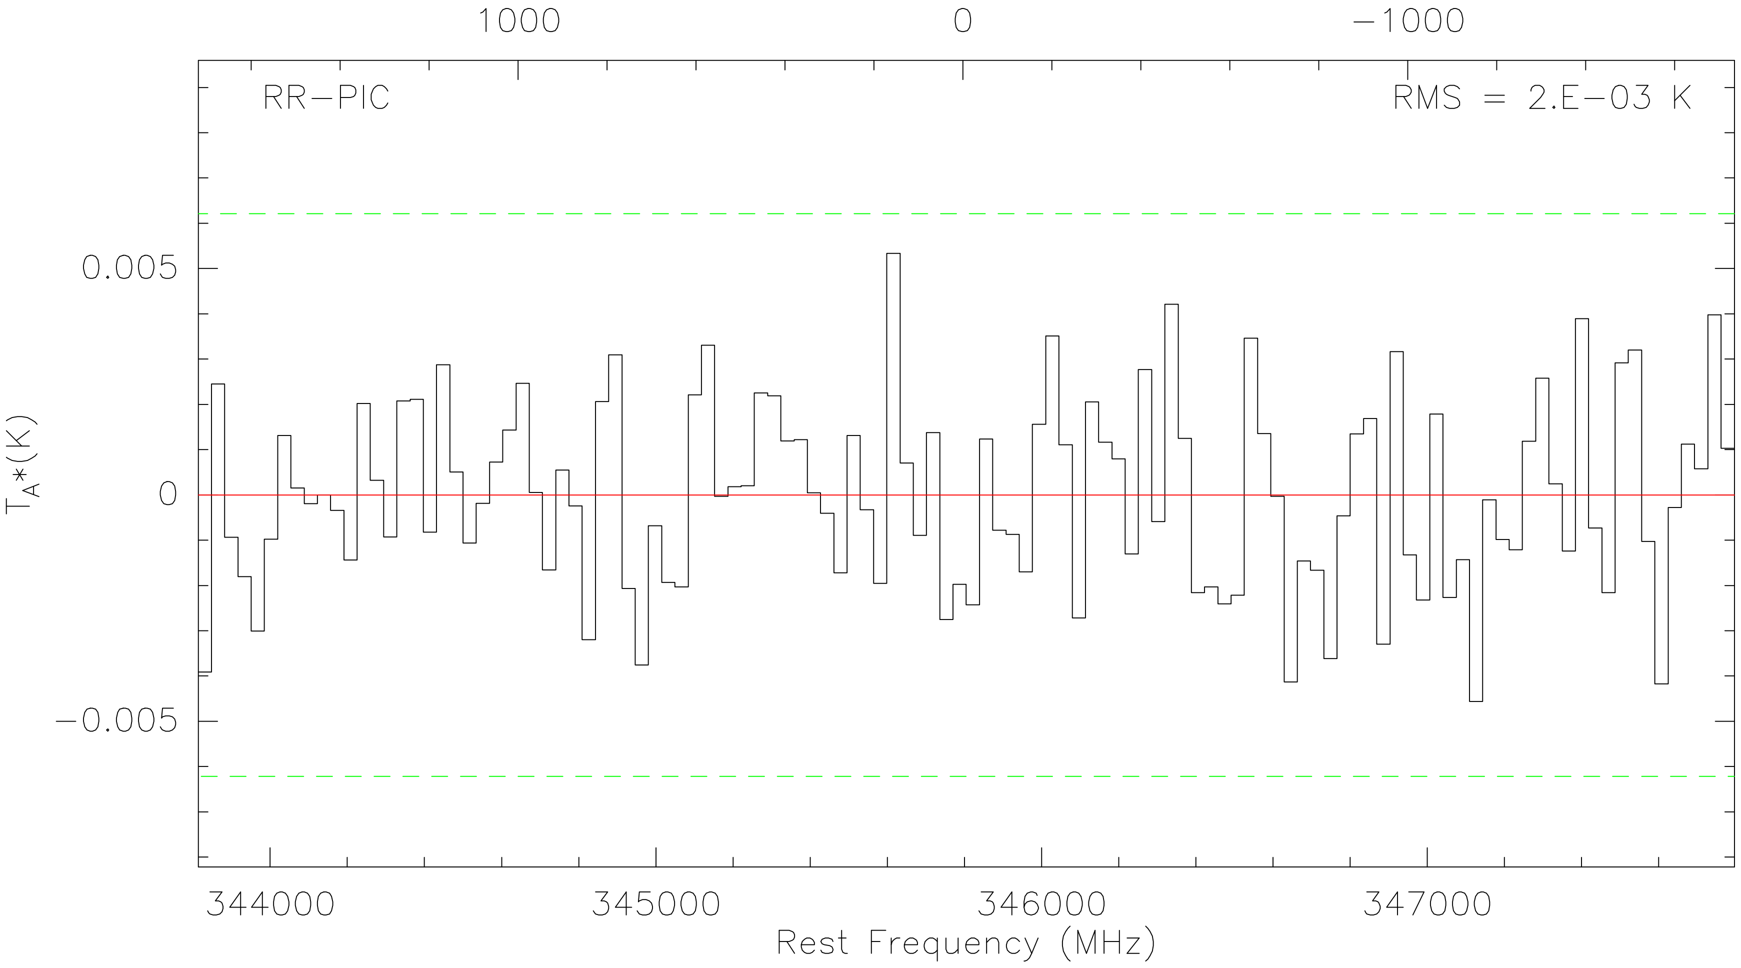

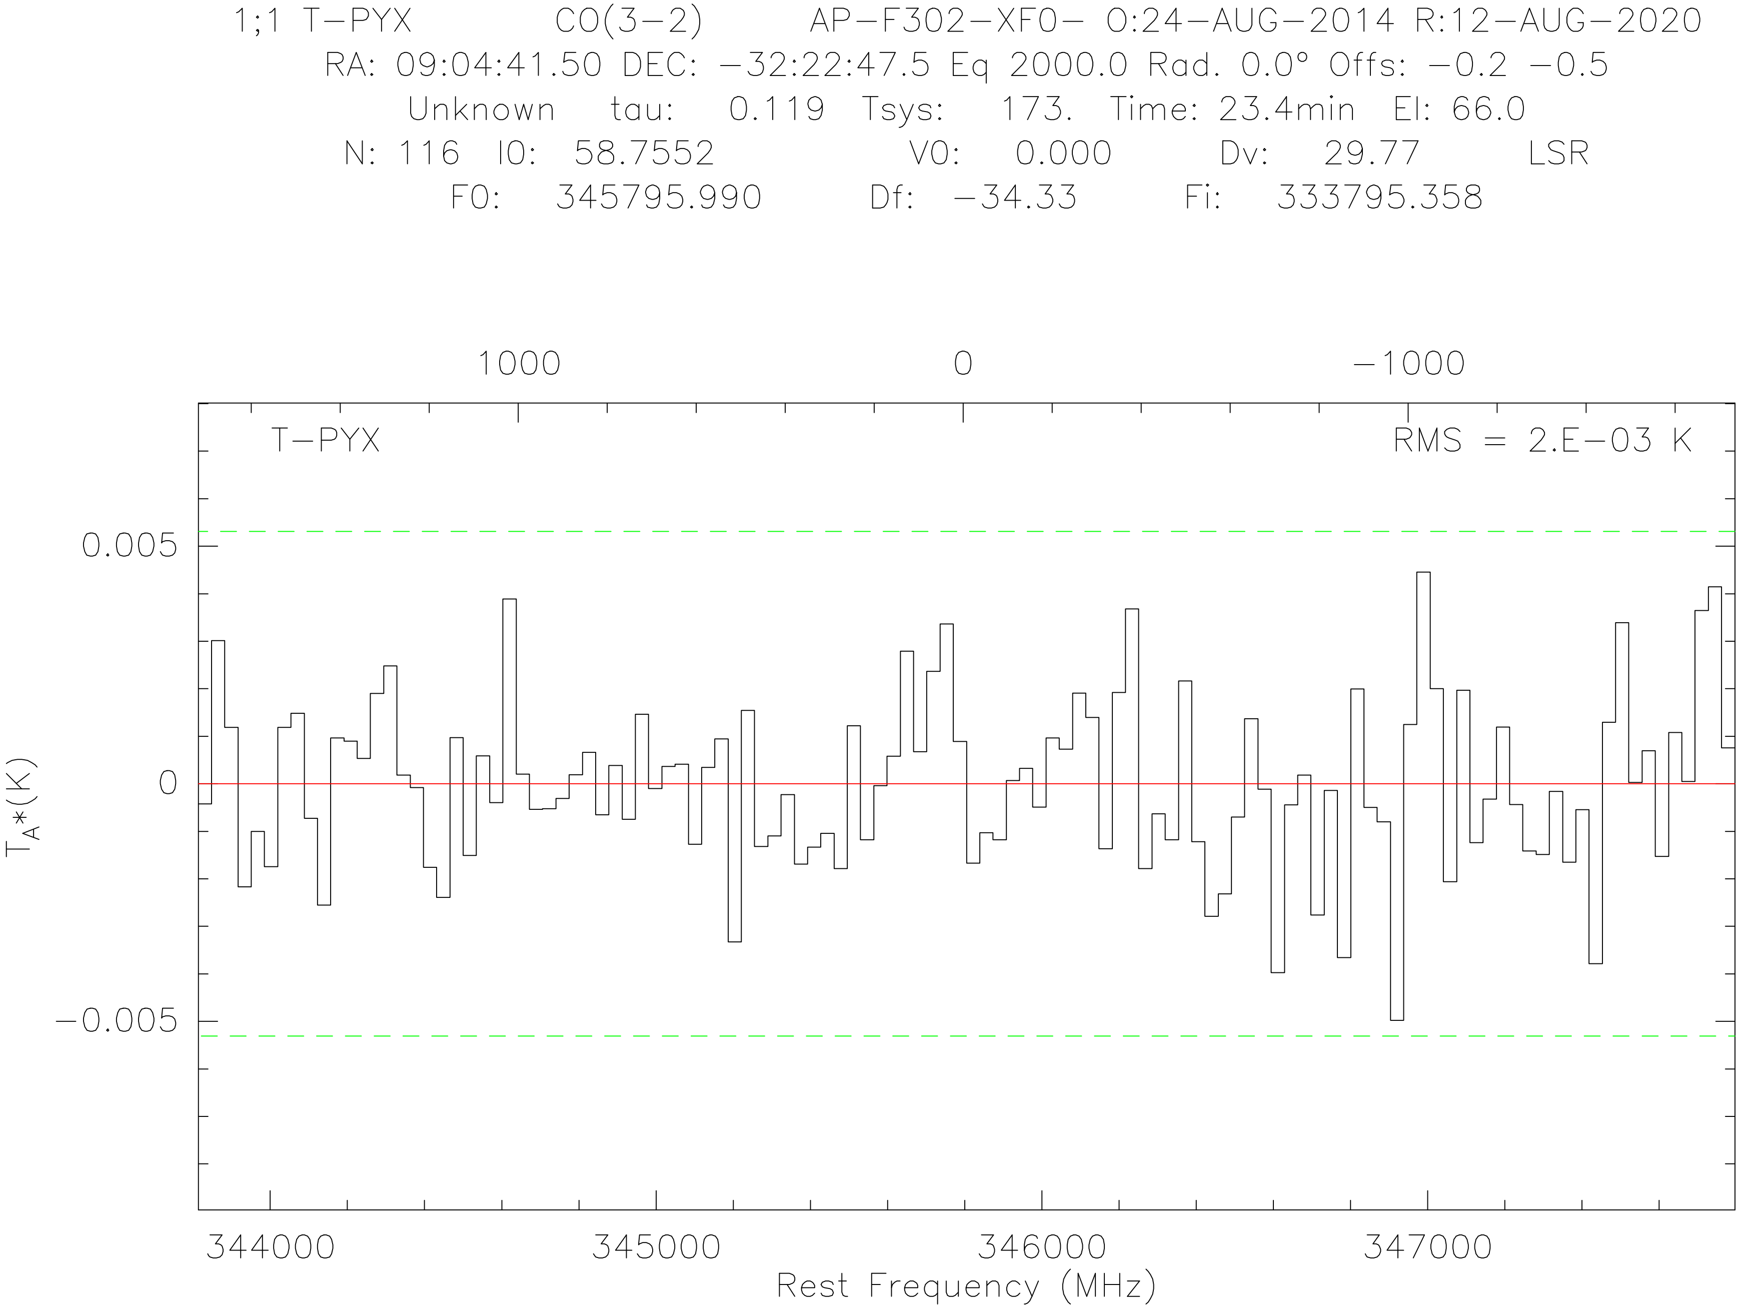

1;1 T-PYX CO(3-2) AP-F302-XF0- O:24-AUG-2014 R:12-AUG-2020
RA: 09:04:41.50 DEC: -32:22:47.5 Eq 2000.0 Rad. 0.0° Offs: -0.2 -0.5
Unknown tau: 0.119 Tsys: 173. Time: 23.4min El: 66.0
N: 116 I0: 58.7552 V0: 0.000 Dv: 29.77 LSR
F0: 345795.990 Df: -34.33 Fi: 333795.358
1000
0
-1000
T-PYX
RMS = 2.E-03 K
0.005
0
-0.005
$T_A$*(K)
344000
345000
346000
347000
Rest Frequency (MHz)

1;1 TV-CRV CO(3-2) AP-F302-XF0- O:24-AUG-2014 R:12-AUG-2020
RA: 12:20:24.15 DEC: −18:27:02.0 Eq 2000.0 Rad. 0.0° Offs: +0.2 −0.3
Unknown tau: 0.117 Tsys: 180. Time: 23.3min El: 51.8
N: 116 I0: 58.7552 V0: 0.000 Dv: 29.77 LSR
F0: 345795.990 Df: −34.33 Fi: 333795.186

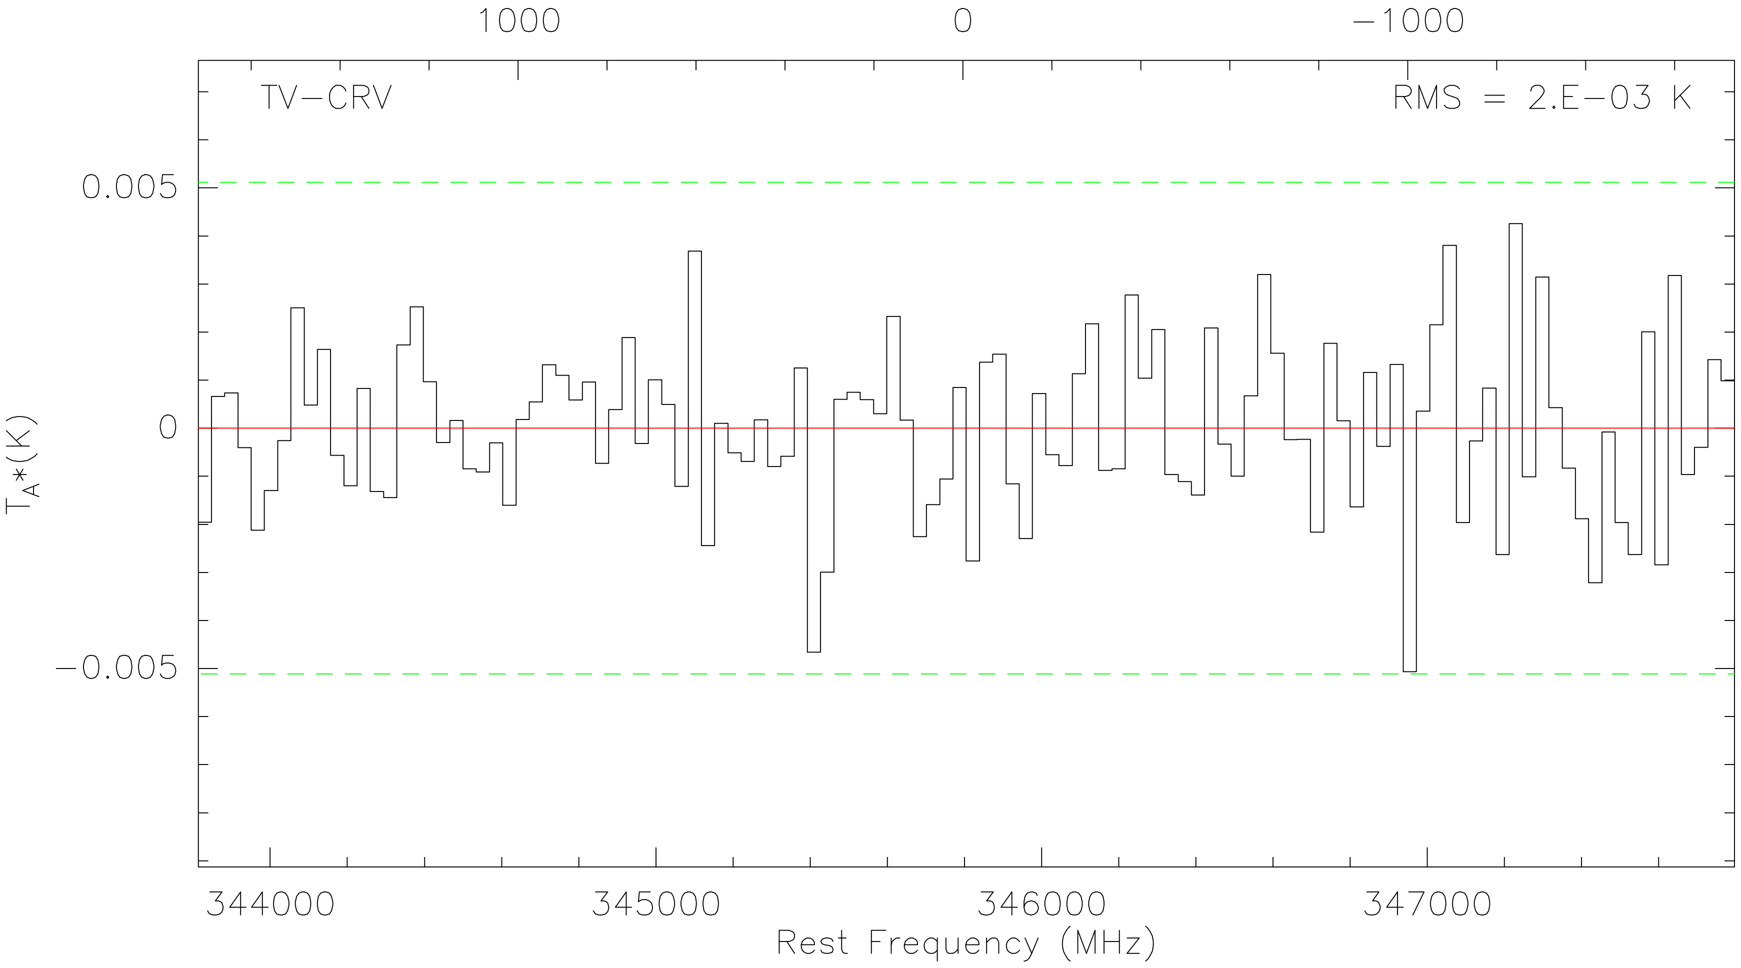

1;1 V1065-CEN    CO(3-2)    AP-F302-XF0- O:24-AUG-2014 R:12-AUG-2020
RA: 11:43:10.33 DEC: -58:04:04.3 Eq 2000.0 Rad. 0.0° Offs: -0.4 -0.3
Unknown  tau:  0.196  Tsys:  299.  Time: 23.3min  El: 30.0
N: 116  I0:  58.7552    V0:  0.000    Dv:  29.77    LSR
F0:  345795.990    Df:  -34.34    Fi:  333795.004

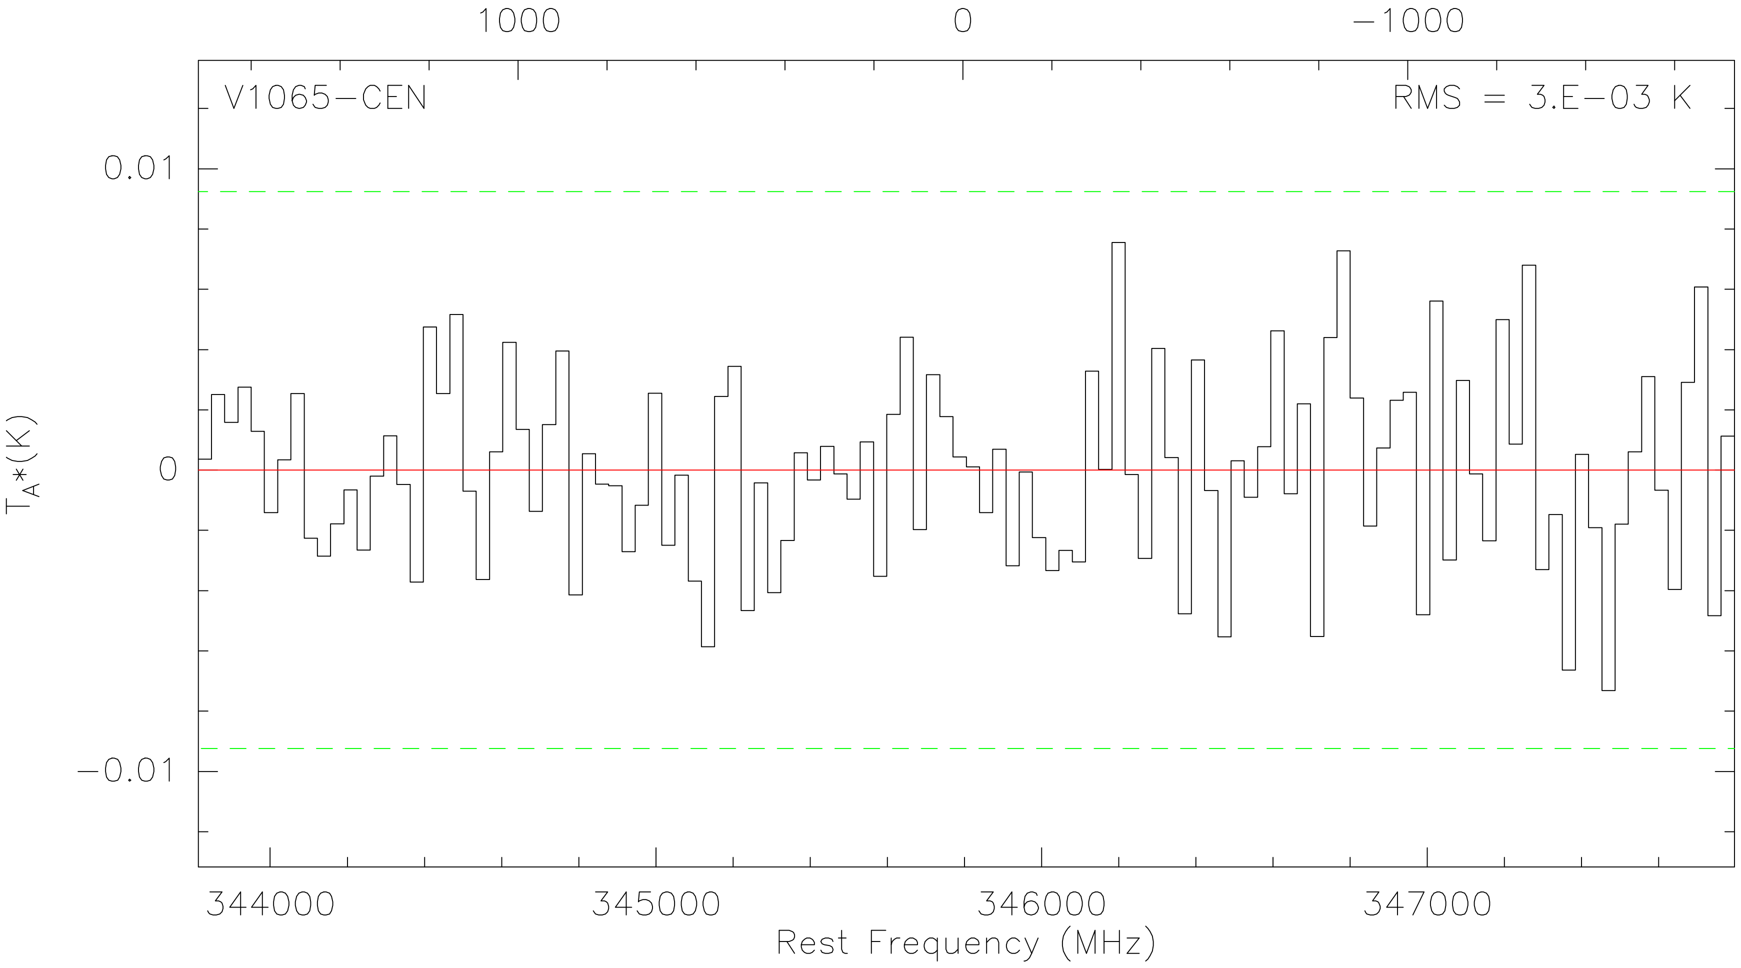

1;1 V351-CAR CO(3-2) AP-F302-XF0- O:28-AUG-2014 R:12-AUG-2020
RA: 10:45:19.14 DEC: -72:03:56.0 Eq 2000.0 Rad. 0.0° Offs: +0.2 -0.4
Unknown tau: 0.173 Tsys: 234. Time: 23.4min El: 40.8
N: 116 I0: 58.7552 V0: 0.000 Dv: 29.77 LSR
F0: 345795.990 Df: -34.33 Fi: 333795.087

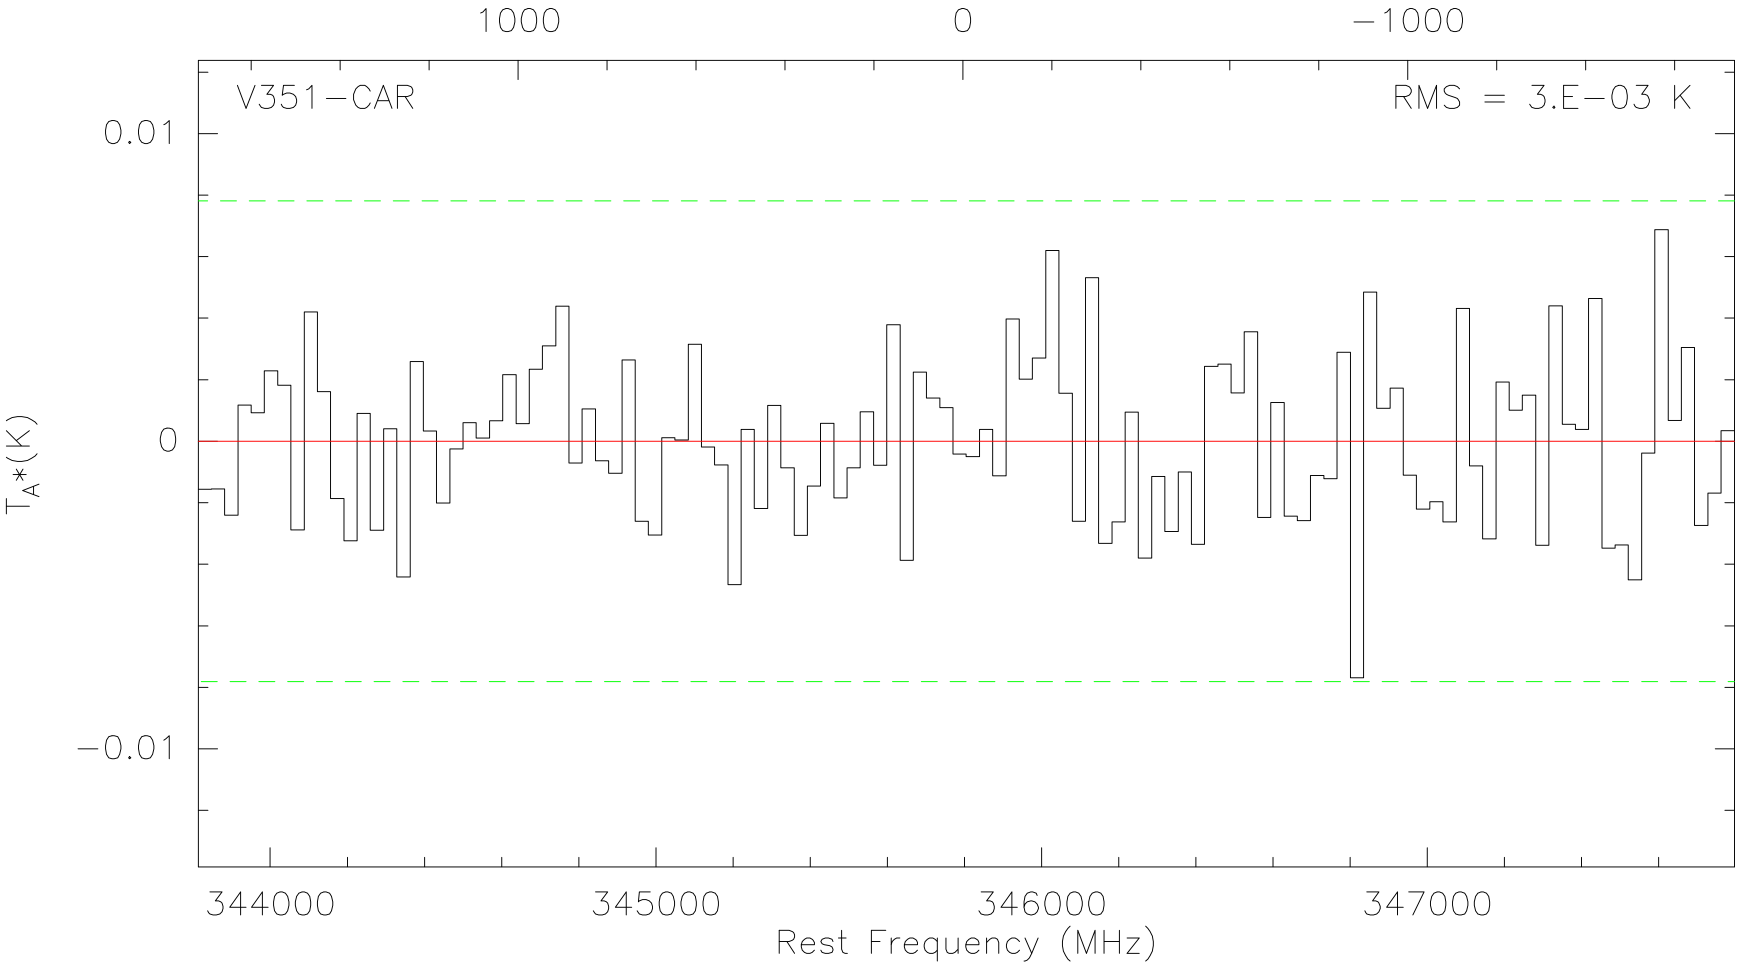

1;1 V359-CEN CO(3-2) AP-F302-XF0- O:24-AUG-2014 R:12-AUG-2020
RA: 11:58:15.33 DEC: −41:46:08.4 Eq 2000.0 Rad. 0.0° Offs: +0.2 −0.4
Unknown tau: 0.117 Tsys: 172. Time: 23.4min El: 70.8
N: 116 I0: 58.7552 V0: 0.000 Dv: 29.77 LSR
F0: 345795.990 Df: −34.34 Fi: 333795.029

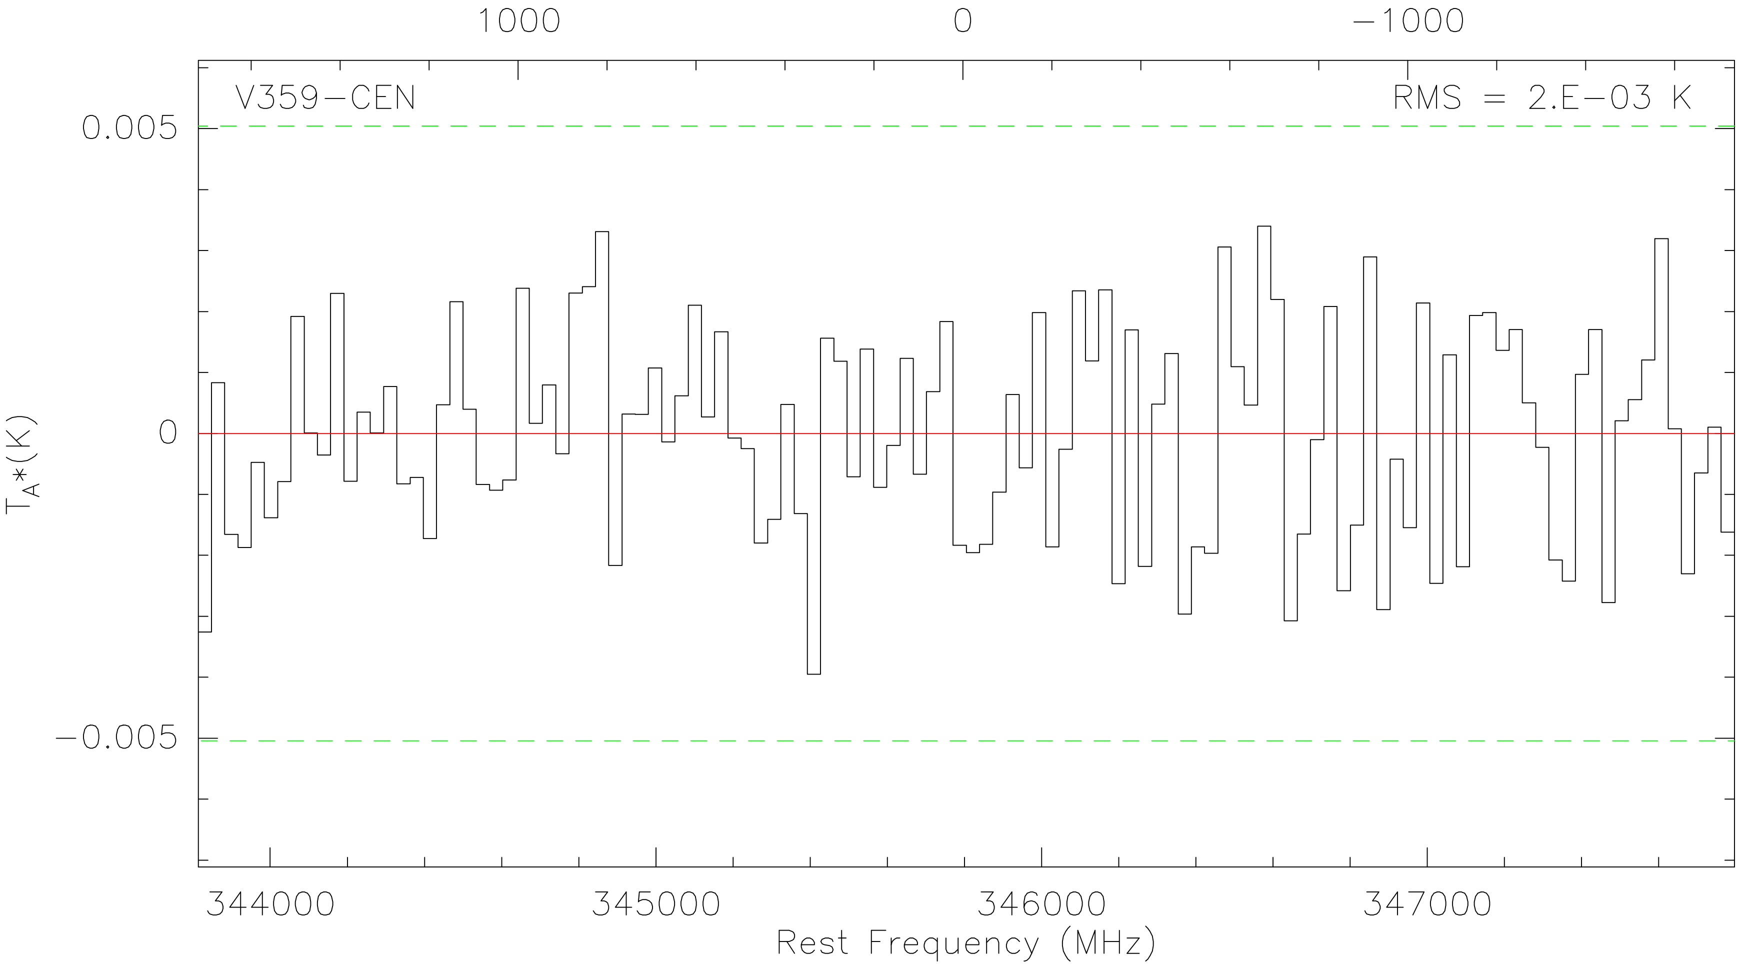

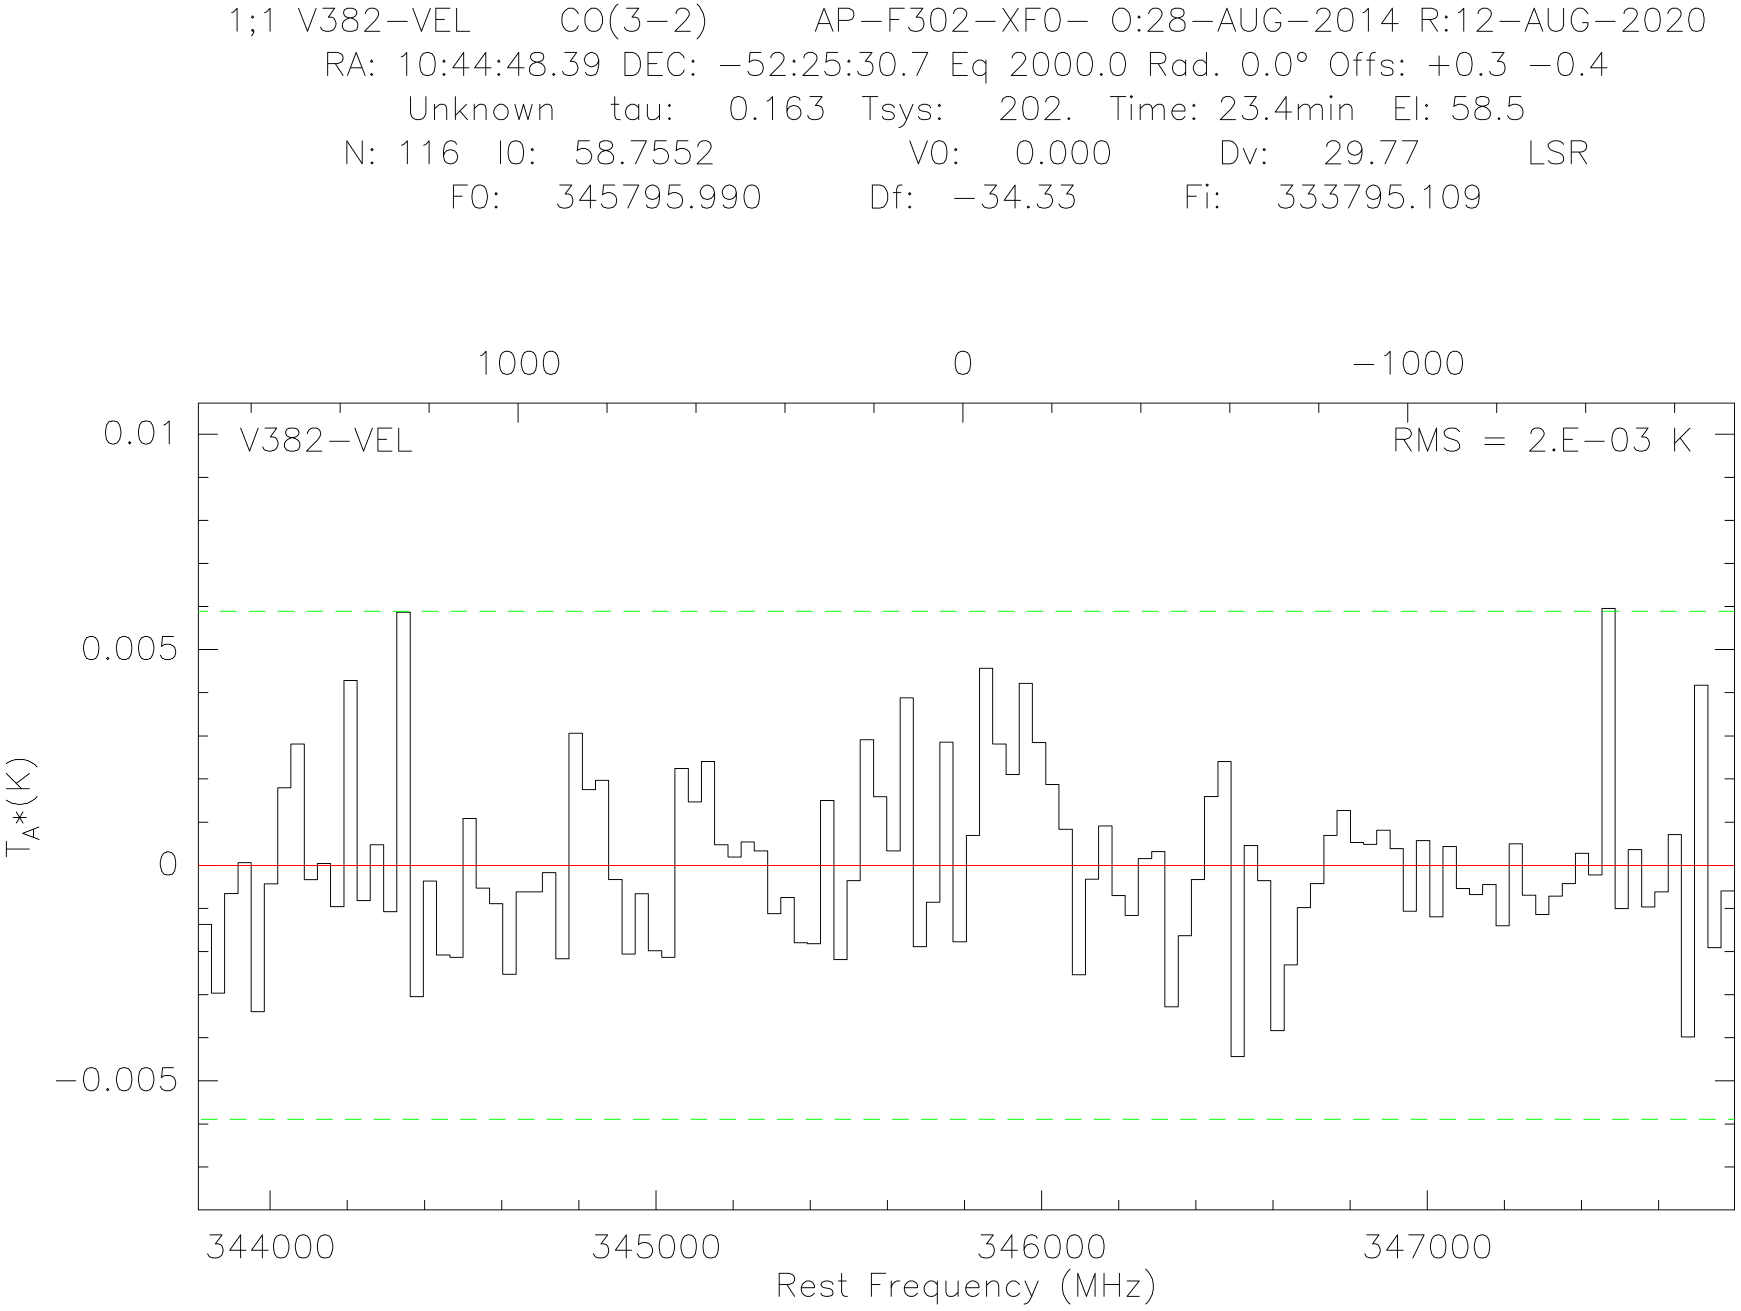
1;1 V382-VEL CO(3-2) AP-F302-XF0- O:28-AUG-2014 R:12-AUG-2020
RA: 10:44:48.39 DEC: -52:25:30.7 Eq 2000.0 Rad. 0.0° Offs: +0.3 -0.4
Unknown tau: 0.163 Tsys: 202. Time: 23.4min El: 58.5
N: 116 I0: 58.7552 V0: 0.000 Dv: 29.77 LSR
F0: 345795.990 Df: -34.33 Fi: 333795.109
1000
0
-1000
V382-VEL
RMS = 2.E-03 K
0.01
0.005
0
-0.005
TA*(K)
344000
345000
346000
347000
Rest Frequency (MHz)

1;1 V382-VEL CO(3-2) AP-F302-XF0- O:08-SEP-2014 R:14-AUG-2020
RA: 10:44:48.39 DEC: -52:25:30.7 Eq 2000.0 Rad. 0.0° Offs: +0.2 -0.3
Unknown tau: 0.159 Tsys: 209. Time: 61.4min El: 57.9
N: 117 I0: 58.7552 V0: 0.000 Dv: 29.77 LSR
F0: 345795.990 Df: -34.33 Fi: 333795.220

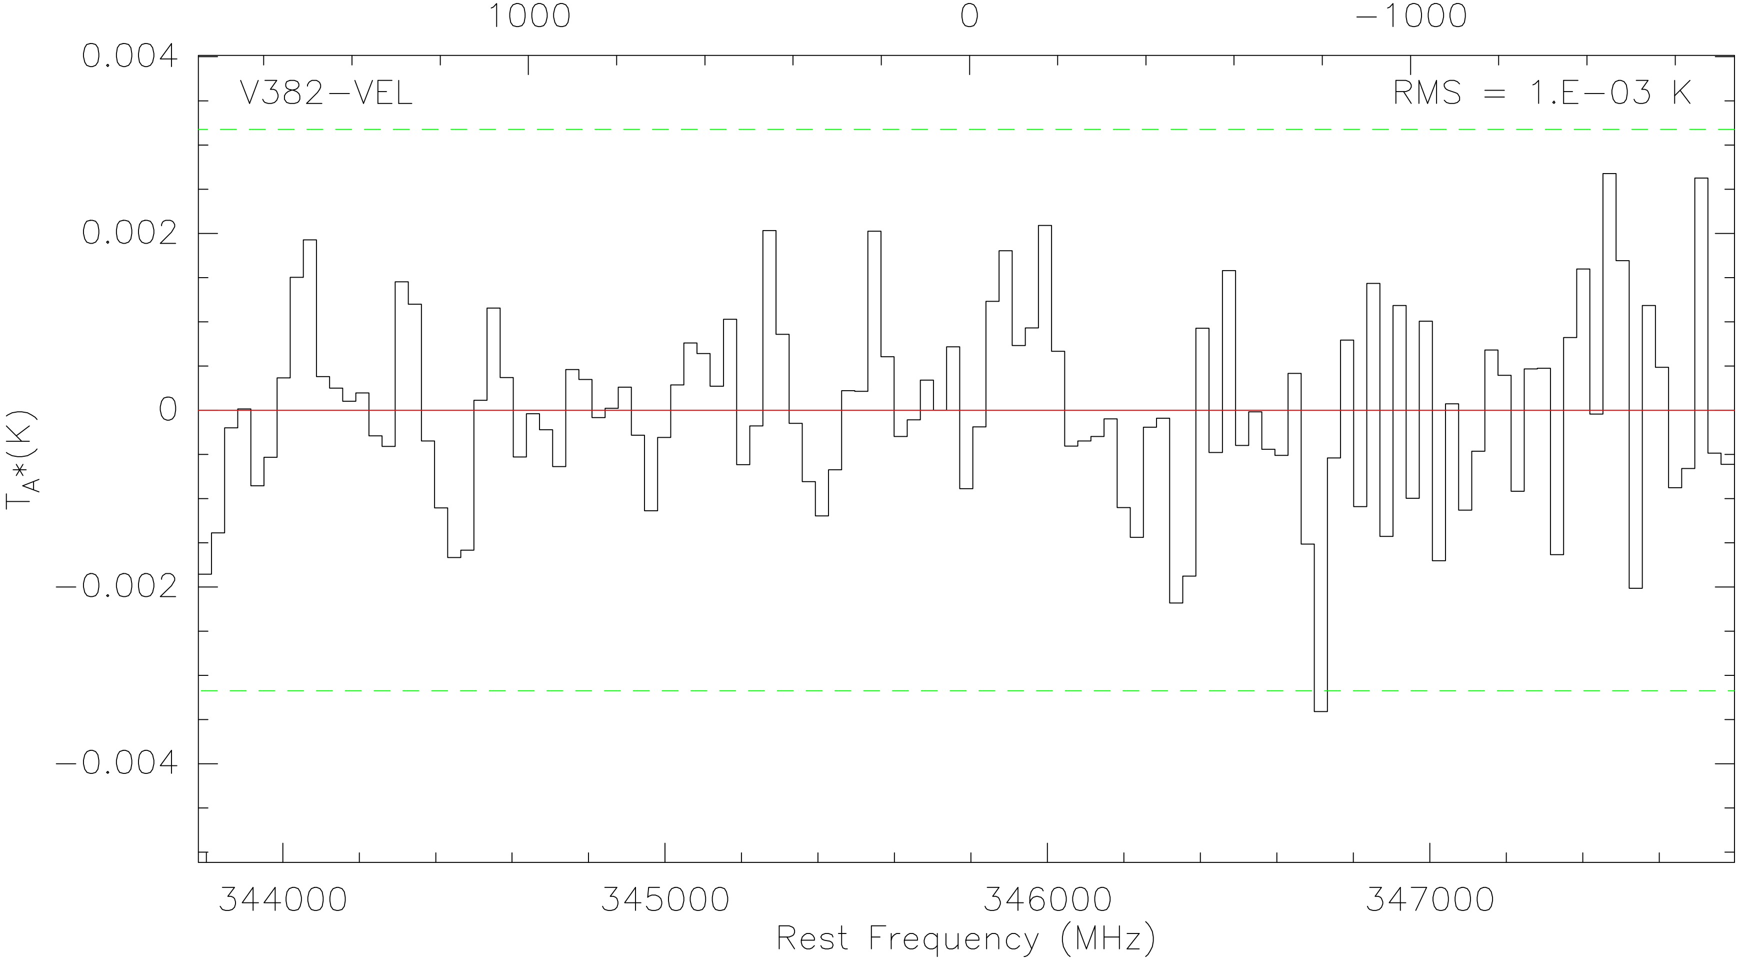

1;1 V598-PUP CO(3-2) AP-F302-XF0- O:25-AUG-2014 R:12-AUG-2020
RA: 07:05:42.50 DEC: -38:14:39.4 Eq 2000.0 Rad. 0.0° Offs: +0.2 -0.3
Unknown tau: 0.100 Tsys: 165. Time: 23.4min El: 59.6
N: 116 I0: 58.7552 V0: 0.000 Dv: 29.77 LSR
F0: 345795.990 Df: -34.33 Fi: 333795.572

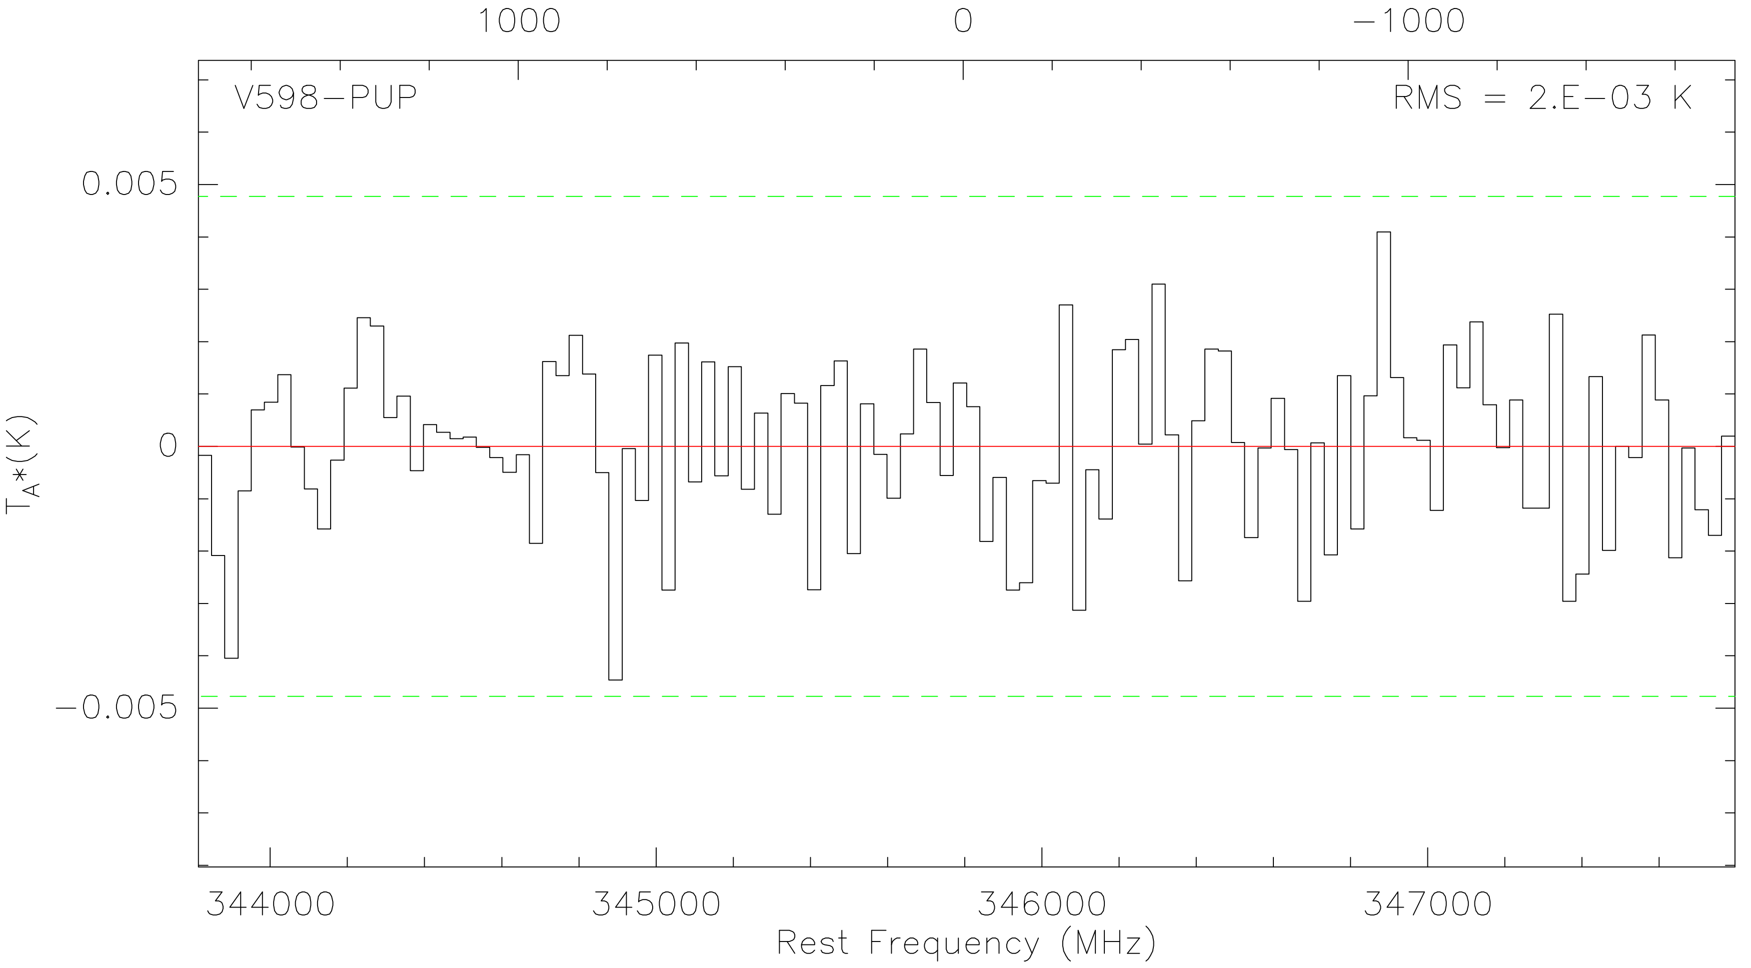

1;1 VX-FOR CO(3-2) AP-F302-XF0- O:24-AUG-2014 R:12-AUG-2020
RA: 03:26:45.71 DEC: -34:26:25.2 Eq 2000.0 Rad. 0.0° Offs: +0.2 -0.2
Unknown tau: 0.180 Tsys: 205. Time: 23.3min El: 53.4
N: 116 I0: 58.7552 V0: 0.000 Dv: 29.76 LSR
F0: 345795.990 Df: -34.33 Fi: 333796.001

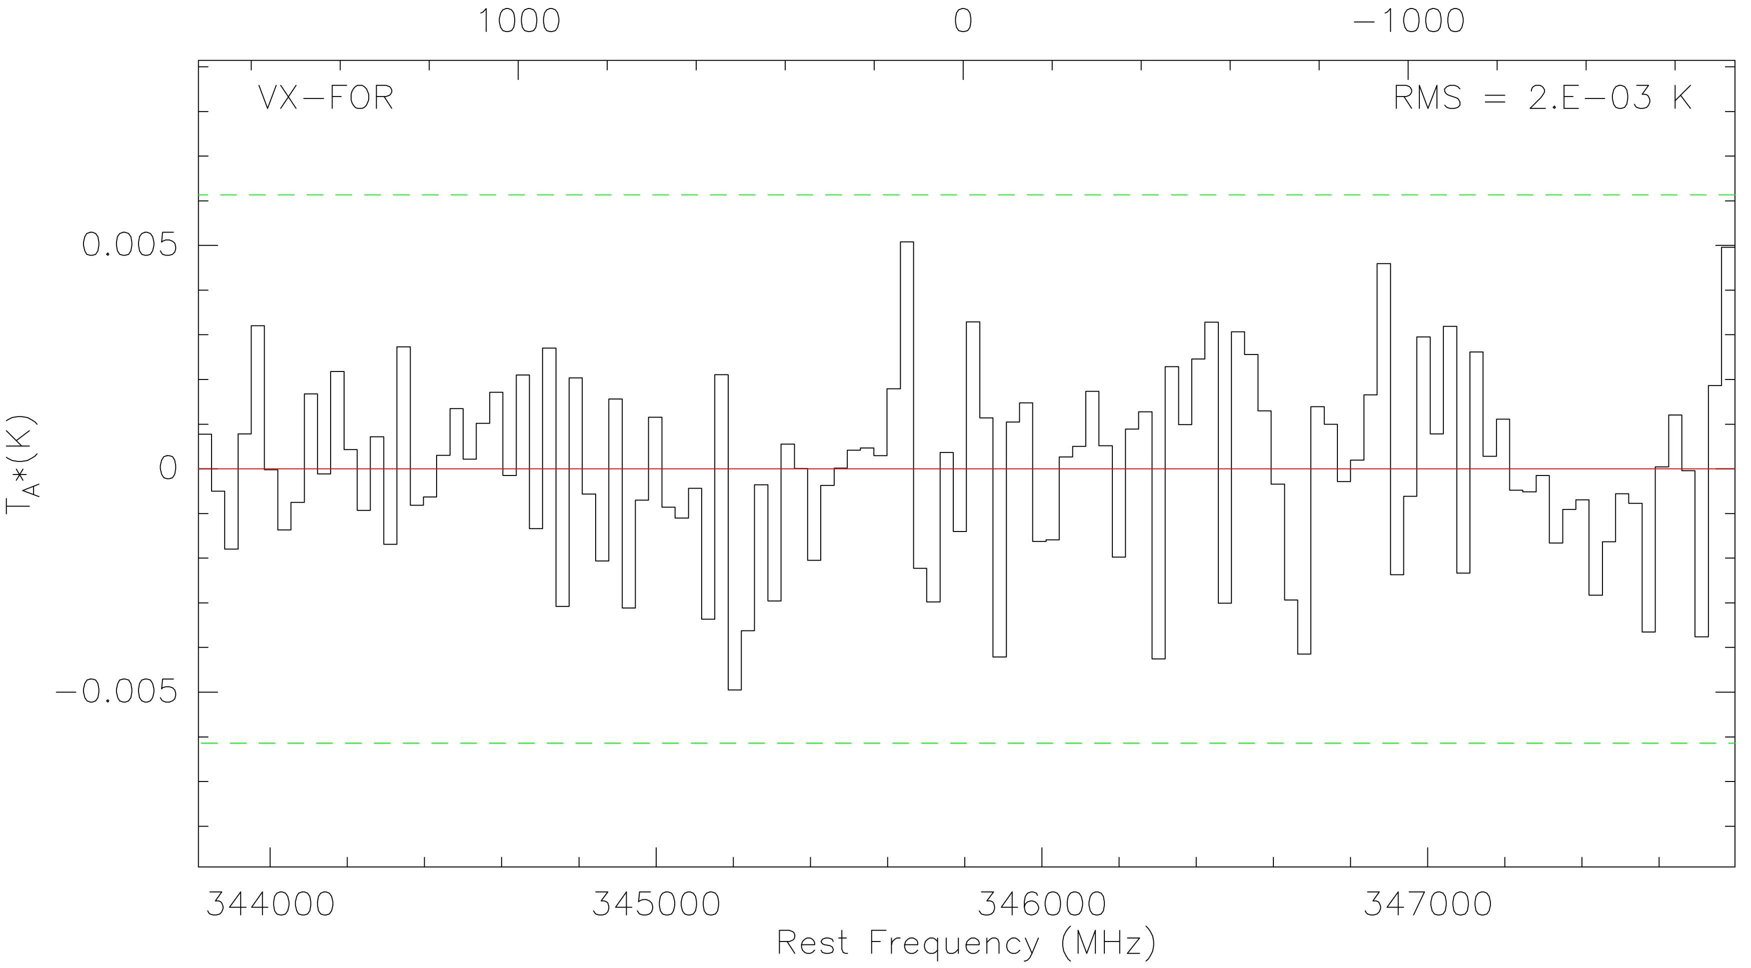

1;1 WX-CET CO(3-2) AP-F302-XF0- O:24-AUG-2014 R:12-AUG-2020
RA: 01:17:04.17 DEC: -17:56:23.0 Eq 2000.0 Rad. 0.0° Offs: -0.2 -0.3
Unknown tau: 0.119 Tsys: 171. Time: 23.3min El: 67.5
N: 116 I0: 58.7552 V0: 0.000 Dv: 29.76 LSR
F0: 345795.990 Df: -34.33 Fi: 333796.330

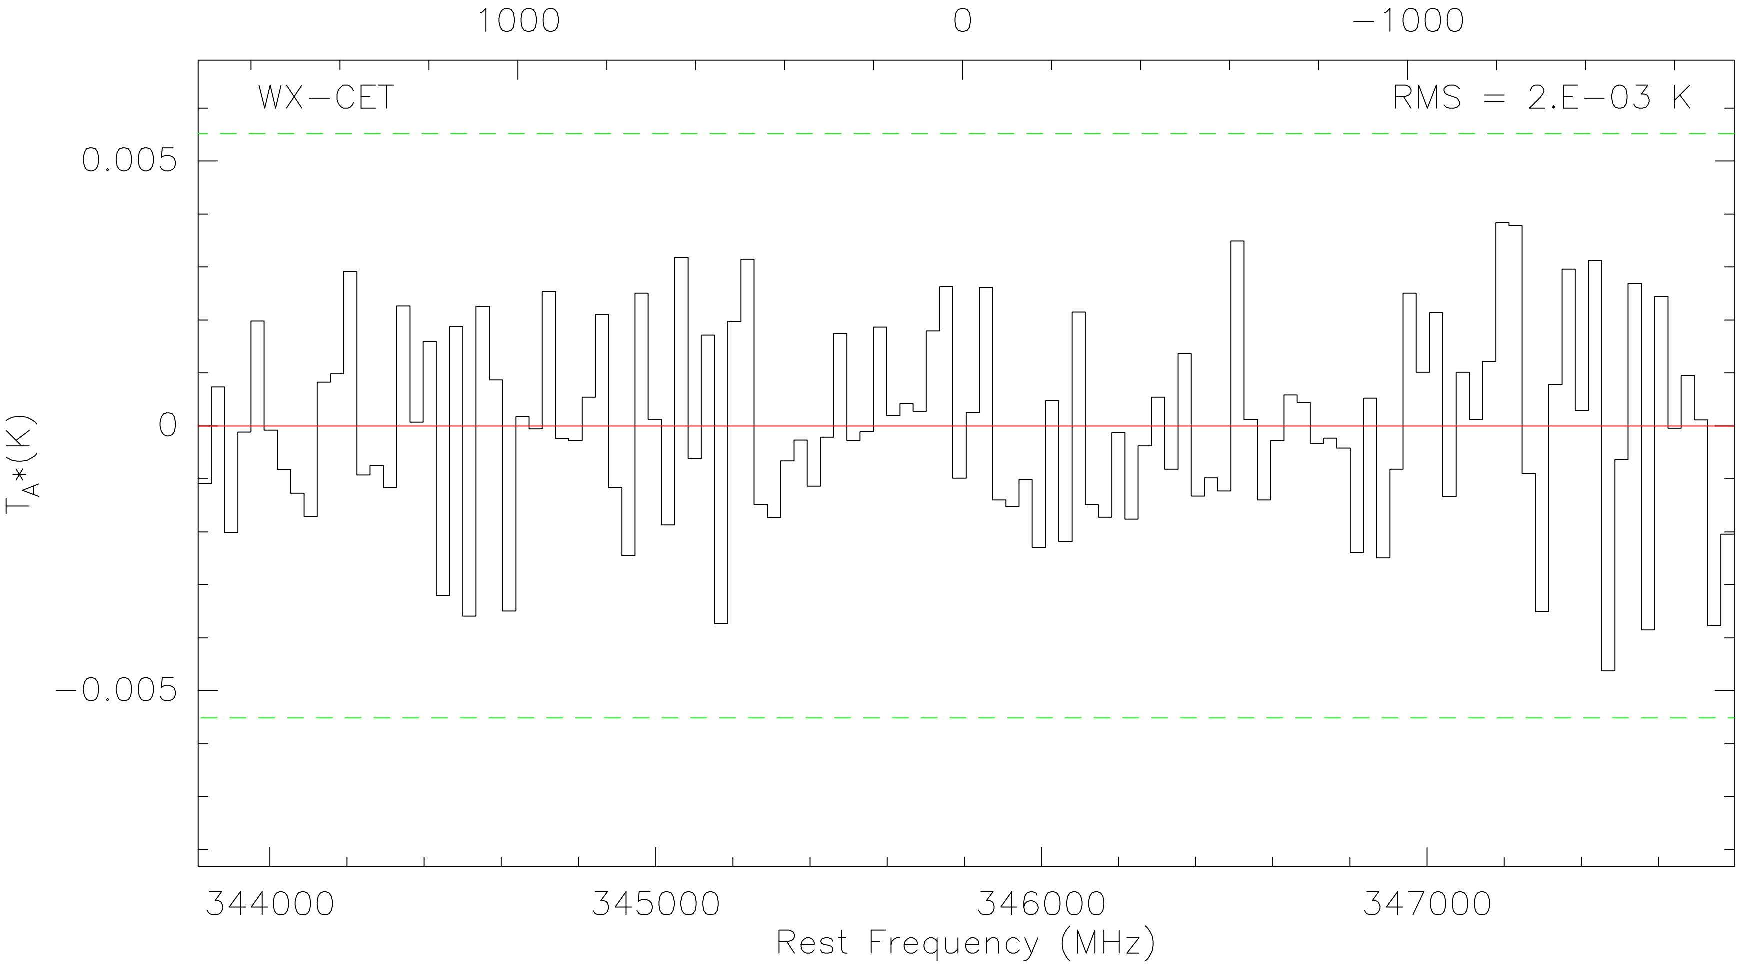

1;1 AICIR CO(3-2) AP-F302-XF0- O:13-JUL-2016 R:07-AUG-2020
RA: 14:49:31.29 DEC: -68:51:35.9 Eq 2000.0 Rad. 0.0° Offs: +0.5 -0.2
Unknown tau: 0.237 Tsys: 294. Time: 5.0min El: 33.7
N: 116 I0: 58.7552 V0: 0.000 Dv: 29.77 LSR
F0: 345795.990 Df: -34.33 Fi: 333795.239

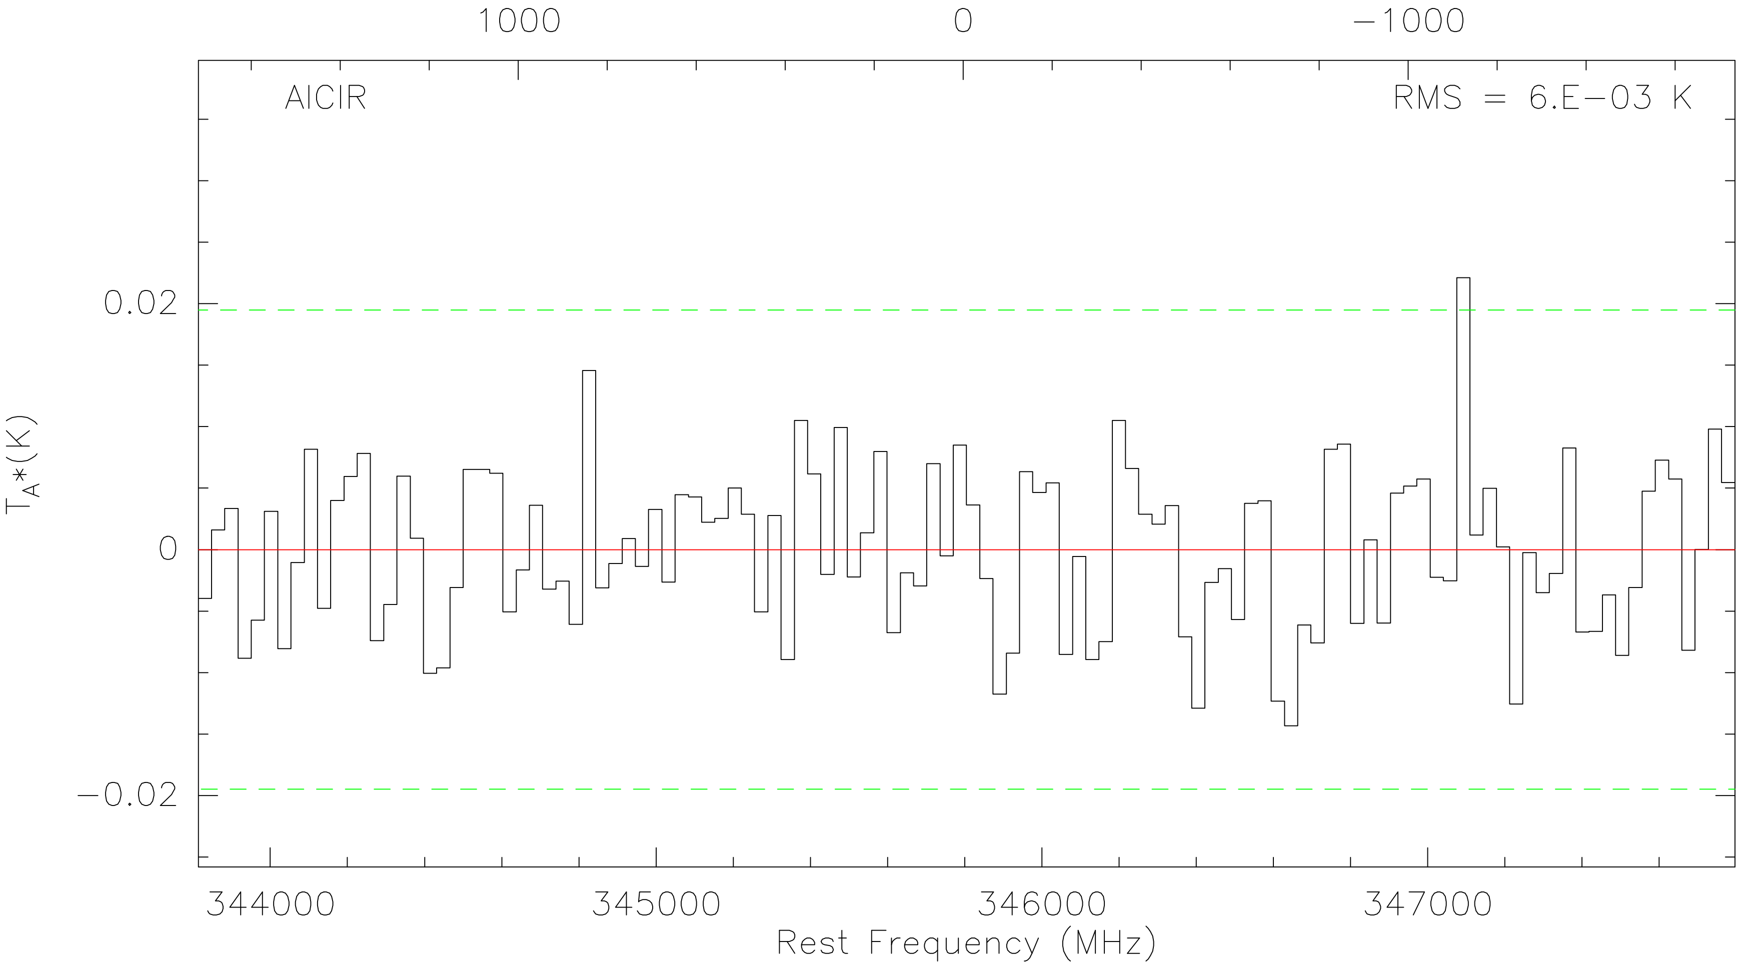

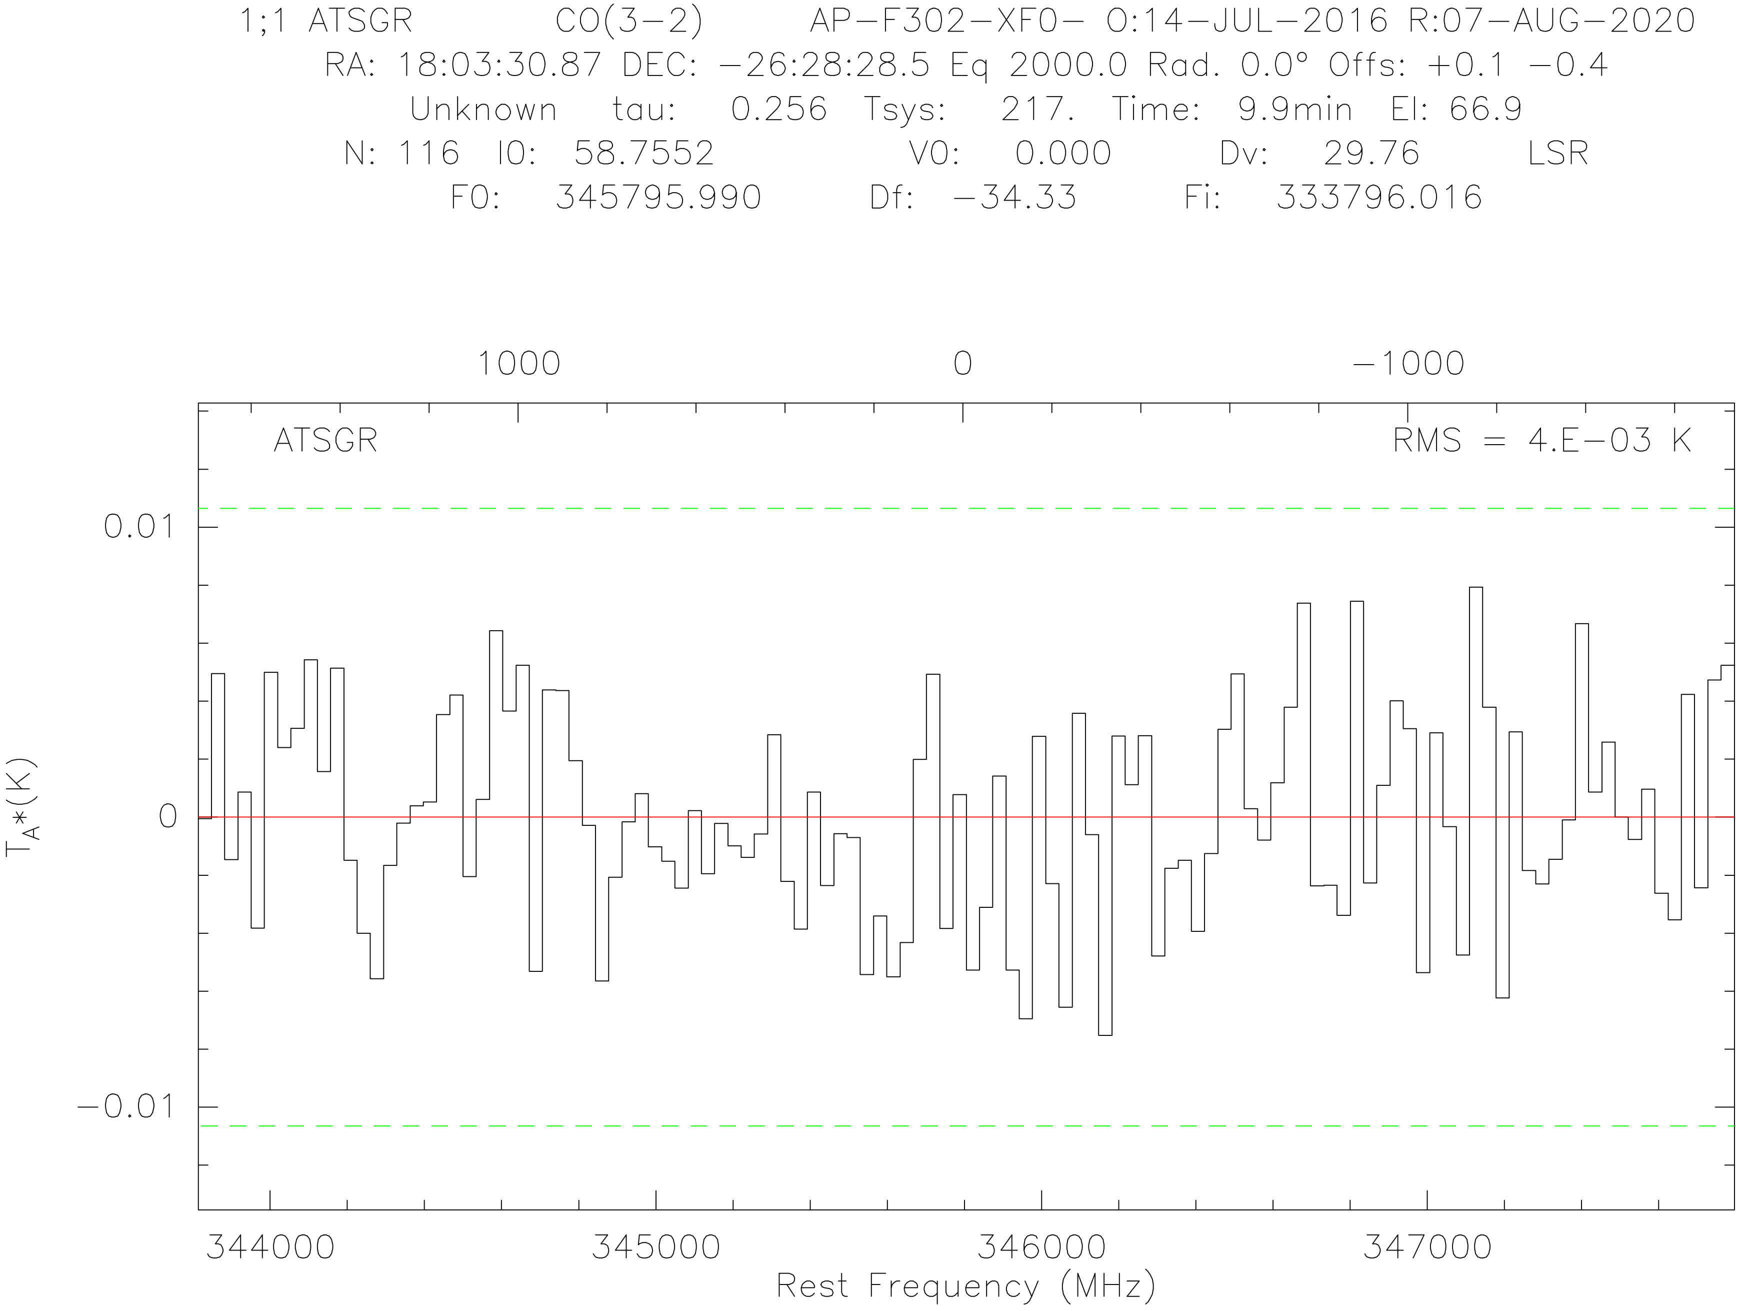

1;1 ATSGR CO(3−2) AP−F302−XF0− O:14−JUL−2016 R:07−AUG−2020
RA: 18:03:30.87 DEC: −26:28:28.5 Eq 2000.0 Rad. 0.0° Offs: +0.1 −0.4
Unknown tau: 0.256 Tsys: 217. Time: 9.9min El: 66.9
N: 116 I0: 58.7552 V0: 0.000 Dv: 29.76 LSR
F0: 345795.990 Df: −34.33 Fi: 333796.016
1000
0
−1000
ATSGR
RMS = 4.E−03 K
0.01
0
−0.01
T_A*(K)
344000
345000
346000
347000
Rest Frequency (MHz)

1;1 FMSGR CO(3-2) AP-F302-XF0- O:13-JUL-2016 R:07-AUG-2020
RA: 18:17:18.10 DEC: -23:38:27.0 Eq 2000.0 Rad. 0.0° Offs: -0.1 -0.4
Unknown tau: 0.175 Tsys: 221. Time: 9.9min El: 35.9
N: 116 I0: 58.7552 V0: 0.000 Dv: 29.76 LSR
F0: 345795.990 Df: -34.33 Fi: 333796.102

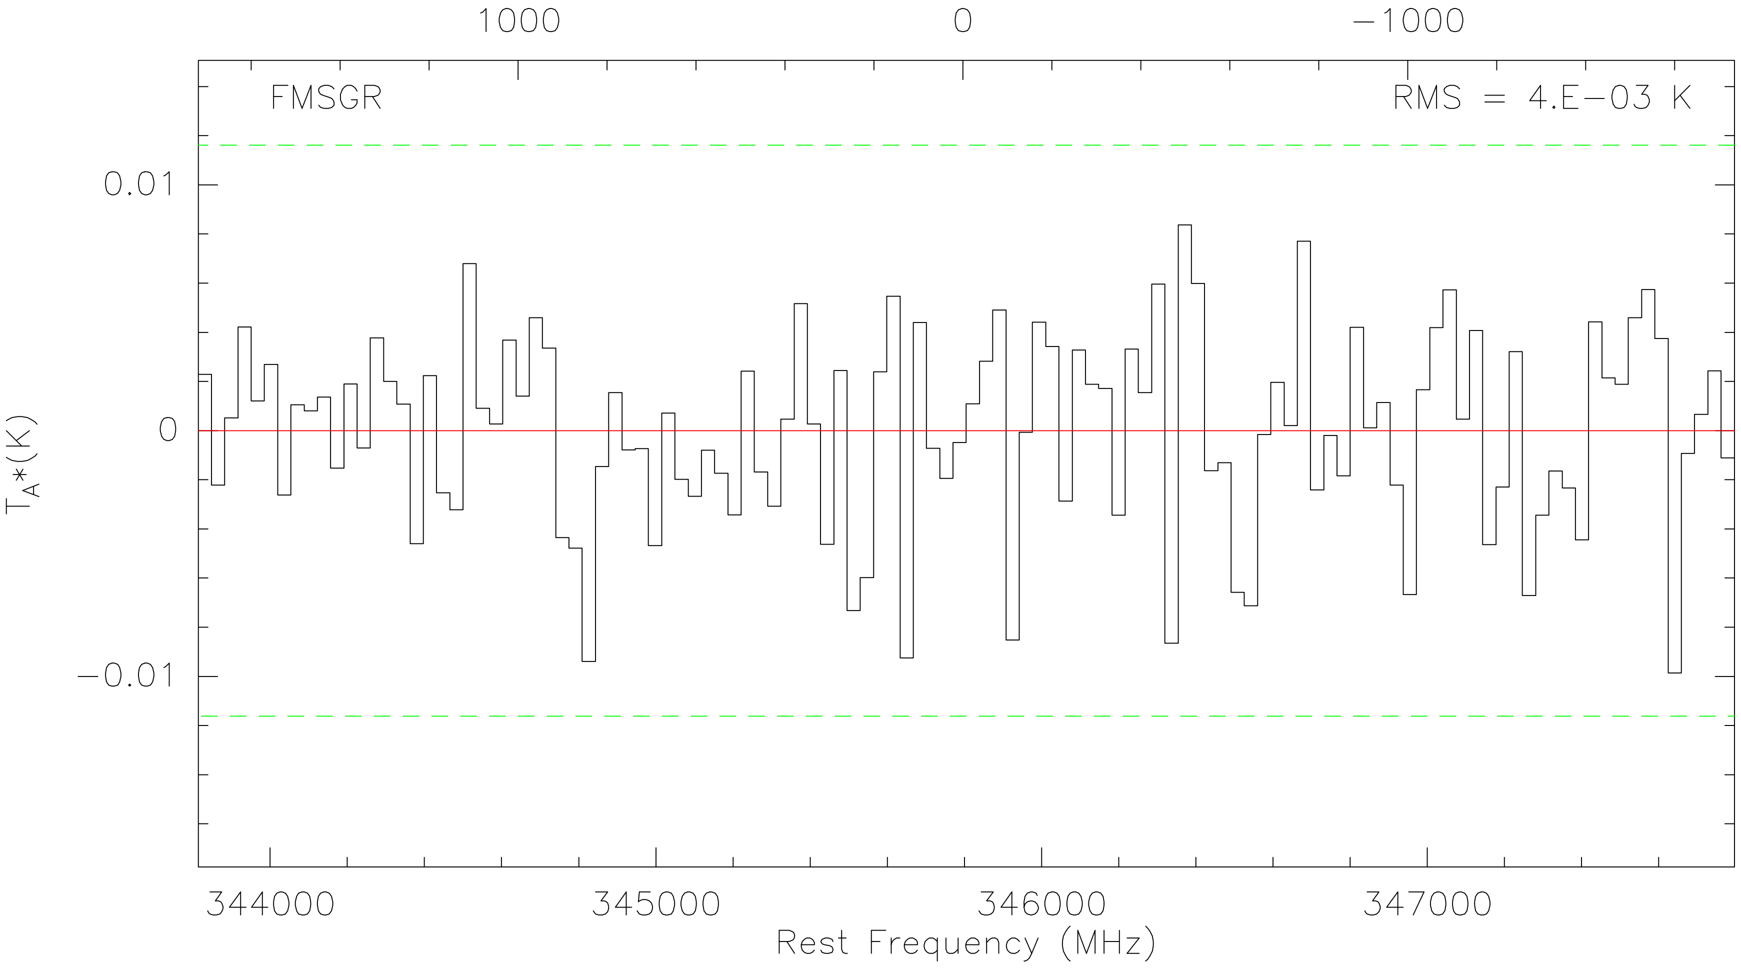

1;1 GRSGR CO(3-2) AP-F302-XF0- O:13-JUL-2016 R:07-AUG-2020
RA: 18:22:58.50 DEC: -25:34:47.3 Eq 2000.0 Rad. 0.0° Offs: -0.1 -0.5
Unknown tau: 0.195 Tsys: 192. Time: 9.9min El: 58.2
N: 116 I0: 58.7552 V0: 0.000 Dv: 29.76 LSR
F0: 345795.990 Df: -34.33 Fi: 333796.109

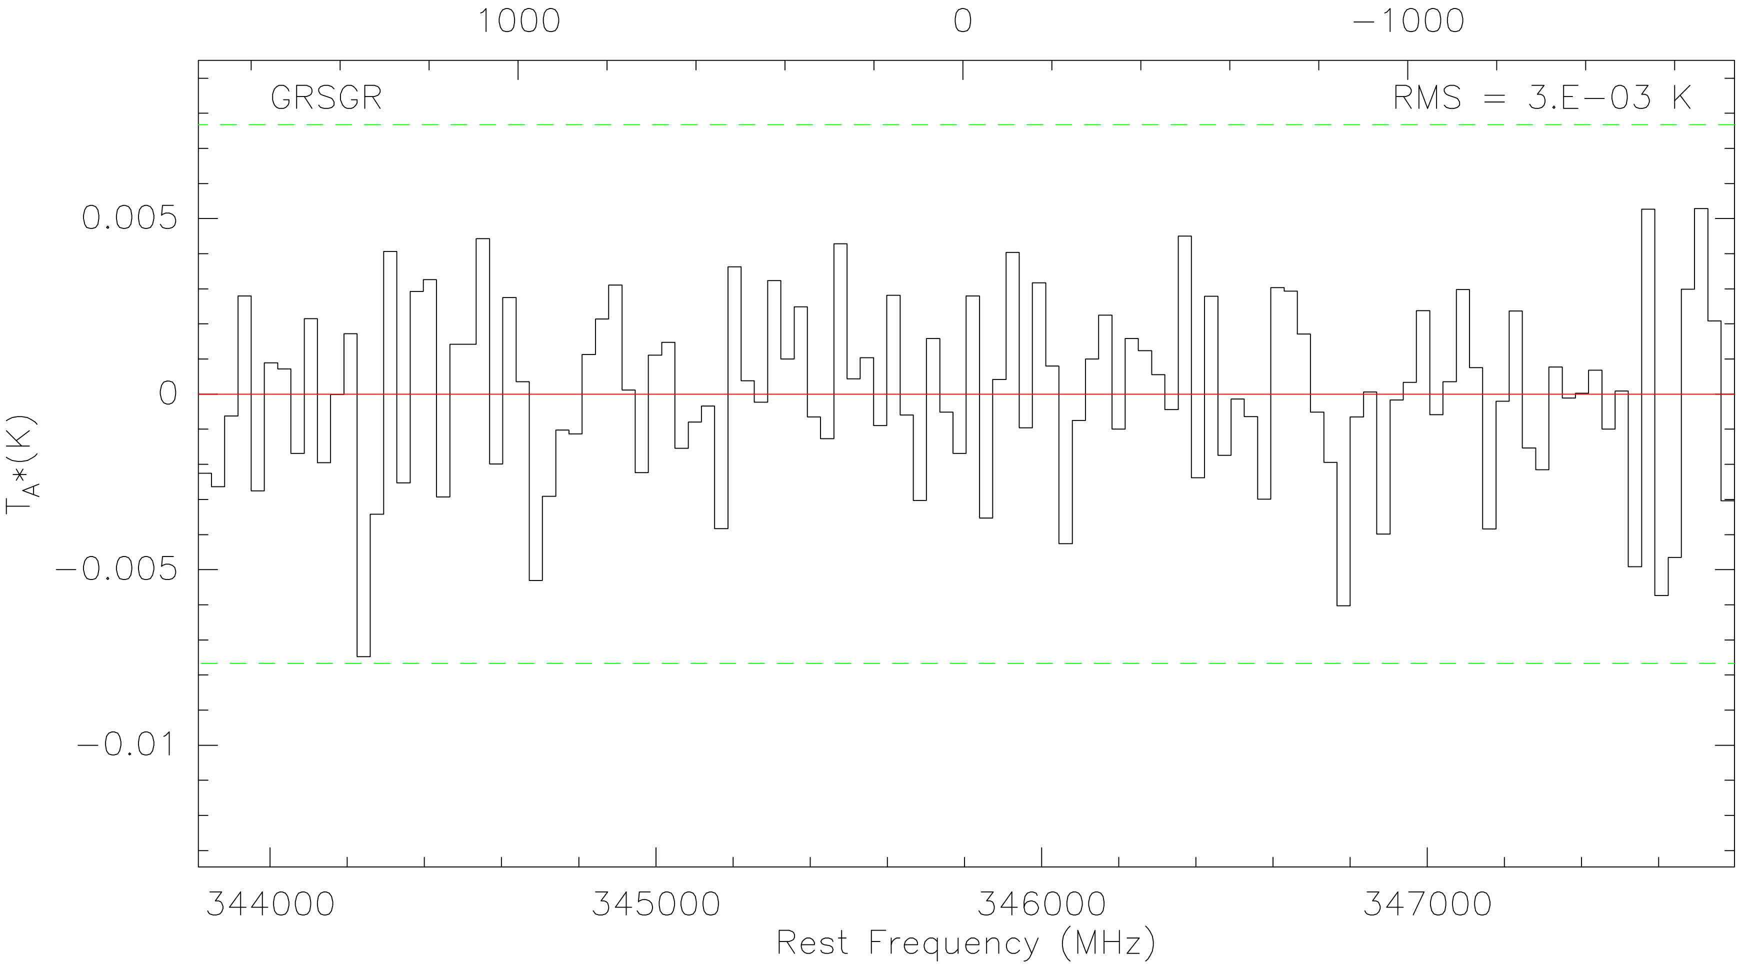

1;1 HSSGR CO(3-2) AP-F302-XF0- O:13-JUL-2016 R:07-AUG-2020
RA: 18:28:03.44 DEC: -21:34:24.7 Eq 2000.0 Rad. 0.0° Offs: -0.3 -0.3
Unknown tau: 0.162 Tsys: 243. Time: 9.9min El: 27.0
N: 116 I0: 58.7552 V0: 0.000 Dv: 29.76 LSR
F0: 345795.990 Df: -34.33 Fi: 333796.170

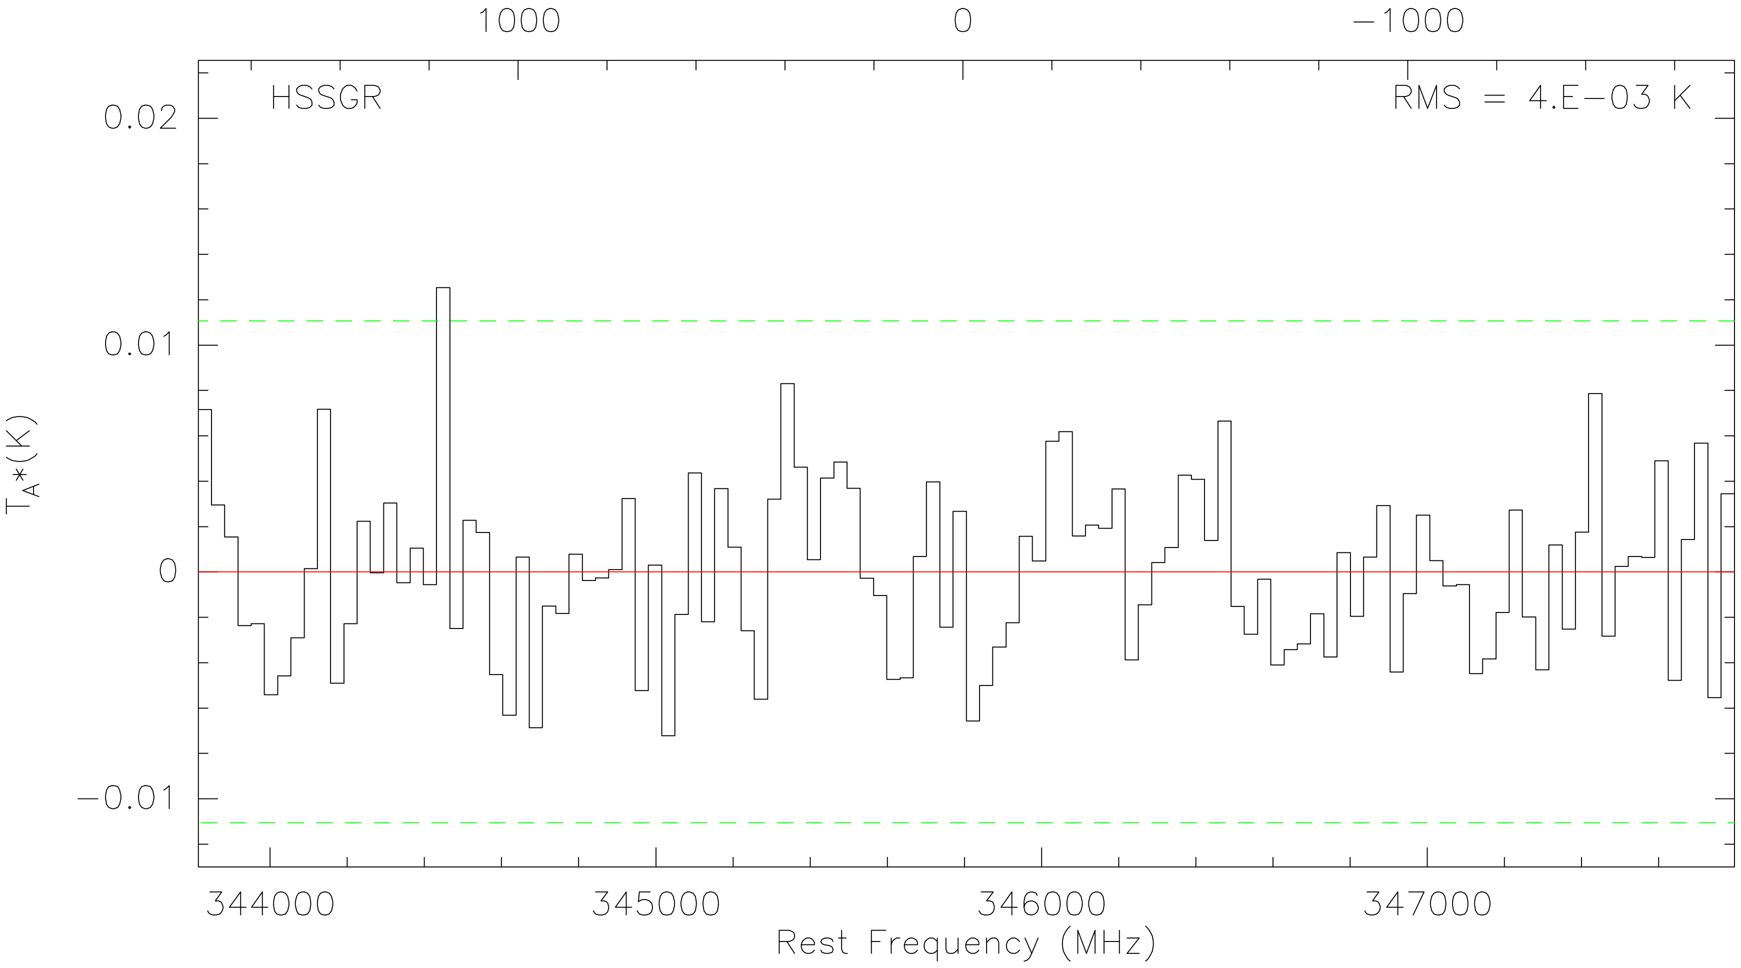

1;1 ILNOR CO(3-2) AP-F302-XF0- O:07-JUL-2016 R:07-AUG-2020
RA: 15:29:23.18 DEC: -50:35:00.7 Eq 2000.0 Rad. 0.0° Offs: -0.2 -0.5
Unknown tau: 0.253 Tsys: 235. Time: 9.9min El: 52.2
N: 116 I0: 58.7552 V0: 0.000 Dv: 29.77 LSR
F0: 345795.990 Df: -34.33 Fi: 333795.343

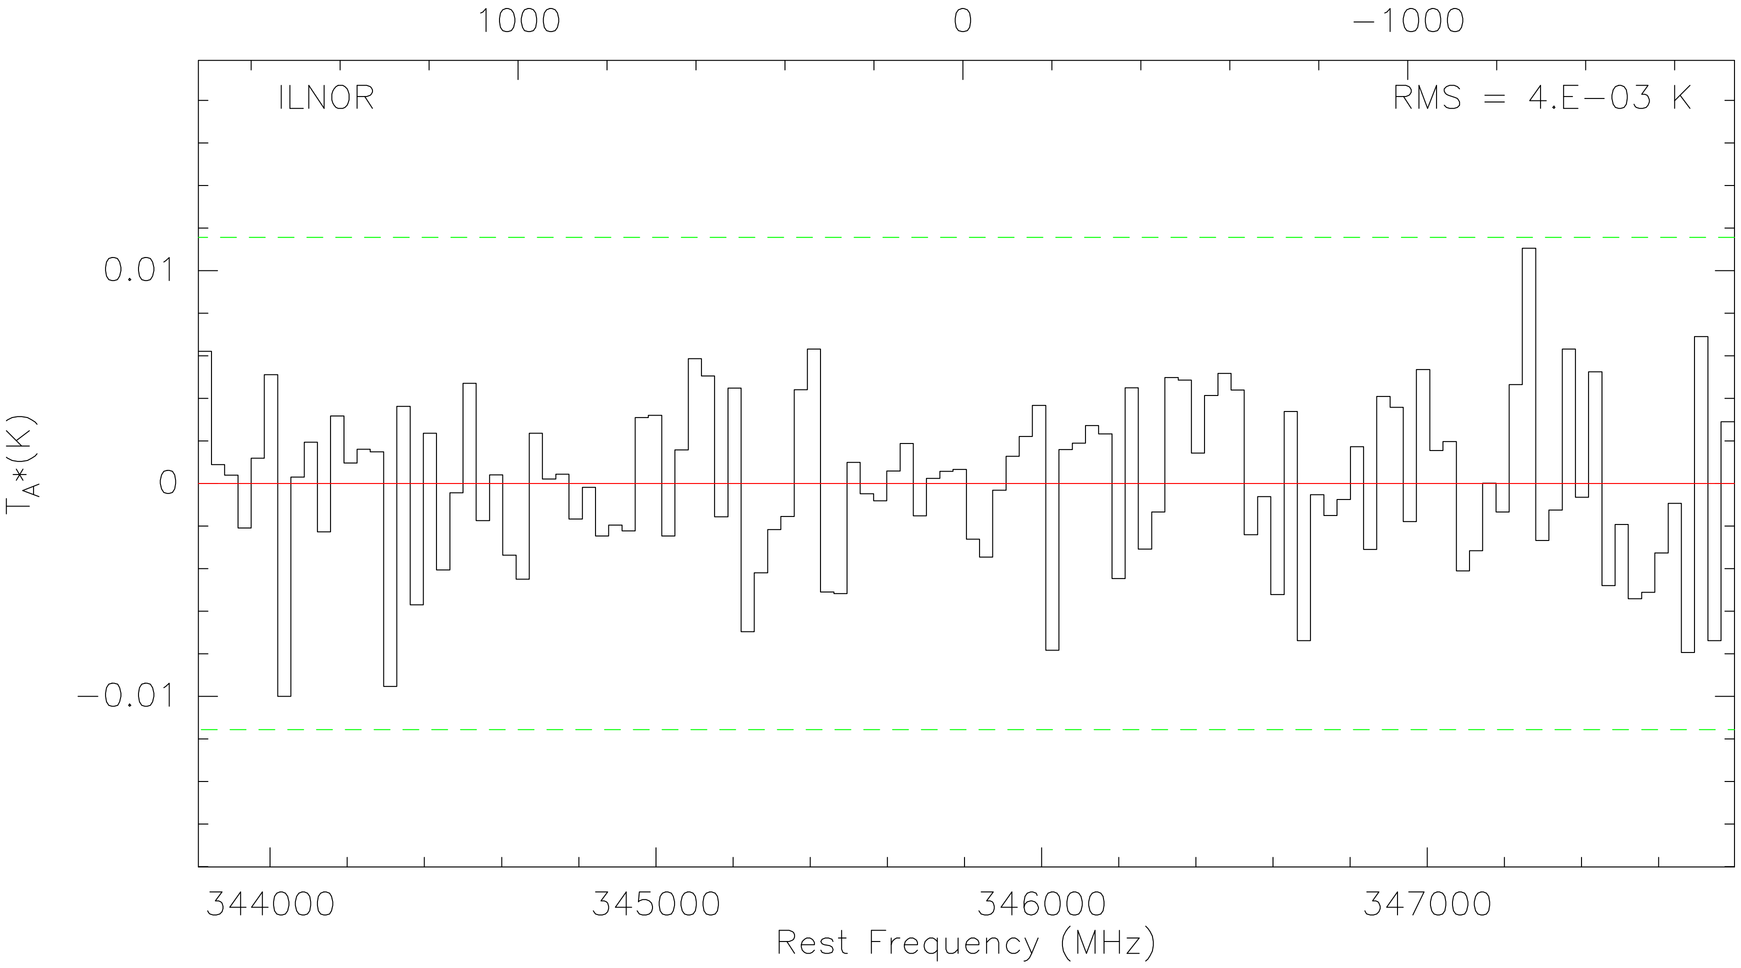

1;1 IMNOR CO(3-2) AP-F302-XF0- O:07-JUL-2016 R:07-AUG-2020
RA: 15:39:26.46 DEC: -52:19:17.9 Eq 2000.0 Rad. 0.0° Offs: -0.2 -0.5
Unknown tau: 0.250 Tsys: 227. Time: 9.9min El: 54.7
N: 116 I0: 58.7552 V0: 0.000 Dv: 29.77 LSR
F0: 345795.990 Df: -34.33 Fi: 333795.375

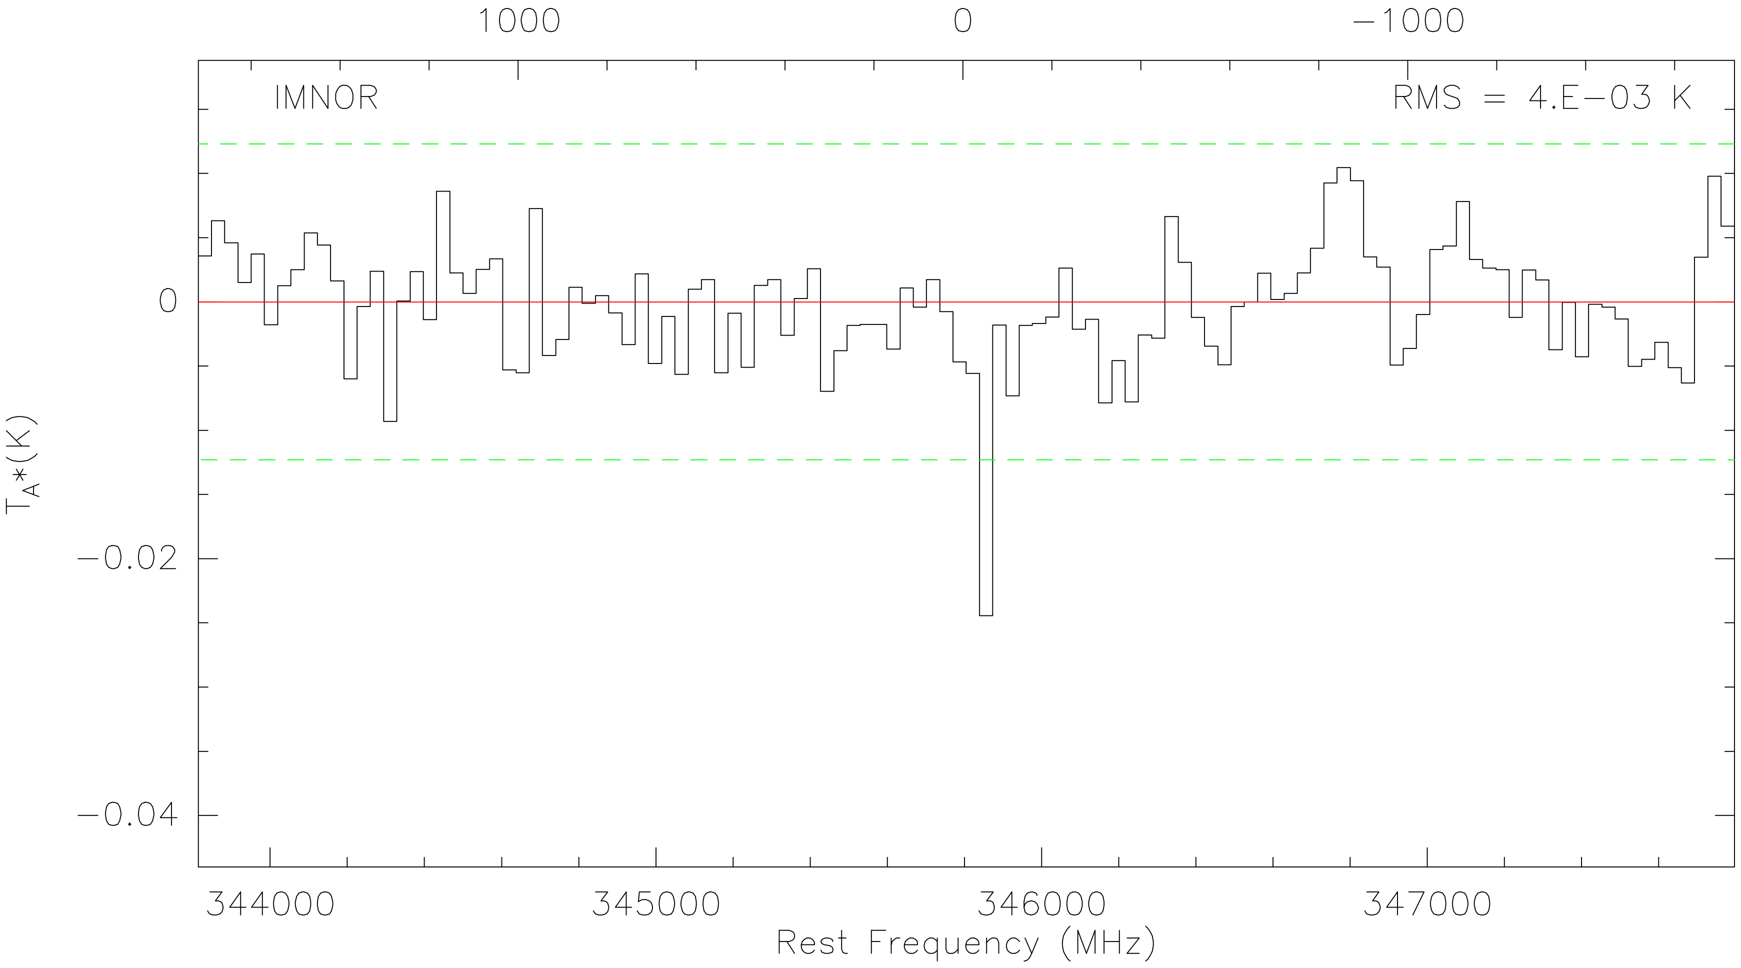

1;1 MTCEN CO(3−2) AP−F302−XF0− O:01−JUL−2016 R:07−AUG−2020
RA: 11:44:00.80 DEC: −60:33:39.5 Eq 2000.0 Rad. 0.0° Offs: +0.3 −0.5
Unknown tau: 0.236 Tsys: 255. Time: 24.8min El: 46.2
N: 116 I0: 58.7552 V0: 0.000 Dv: 29.77 LSR
F0: 345795.990 Df: −34.34 Fi: 333794.986

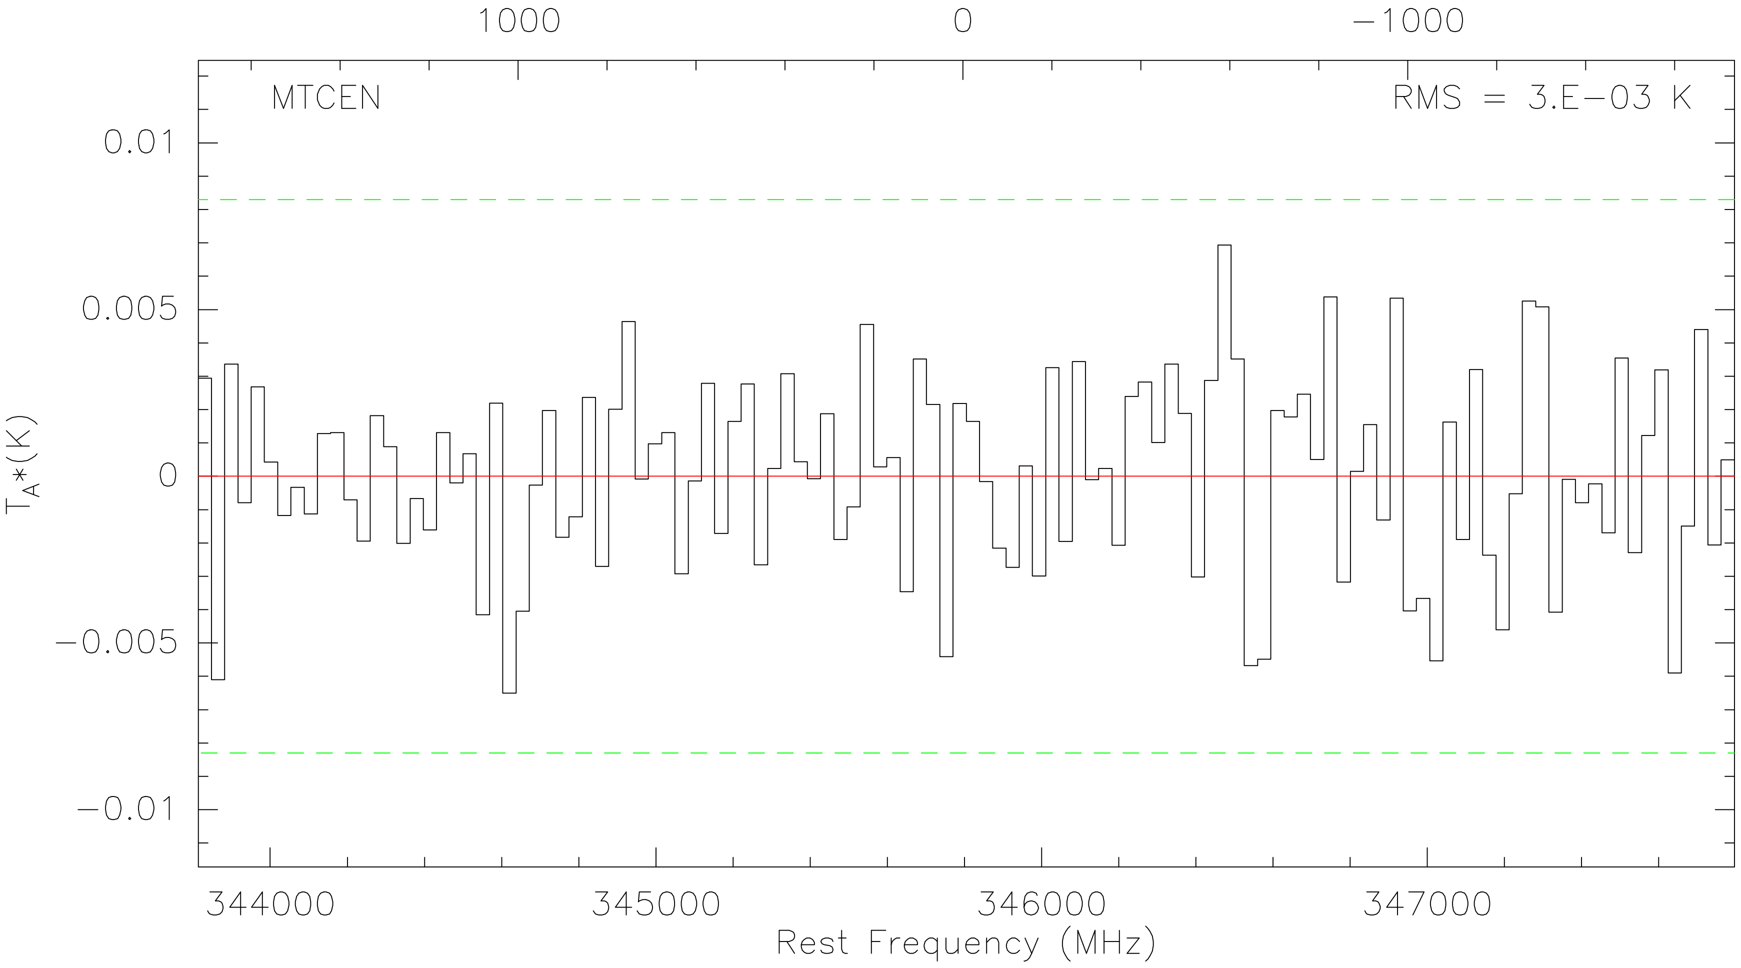

1;1 RSCAR CO(3-2) AP-F302-XF0- O:30-JUN-2016 R:07-AUG-2020
RA: 11:08:06.63 DEC: -61:56:04.6 Eq 2000.0 Rad. 0.0° Offs: +0.3 -0.6
Unknown tau: 0.238 Tsys: 242. Time: 19.8min El: 47.6
N: 116 I0: 58.7552 V0: 0.000 Dv: 29.77 LSR
F0: 345795.990 Df: -34.34 Fi: 333794.980

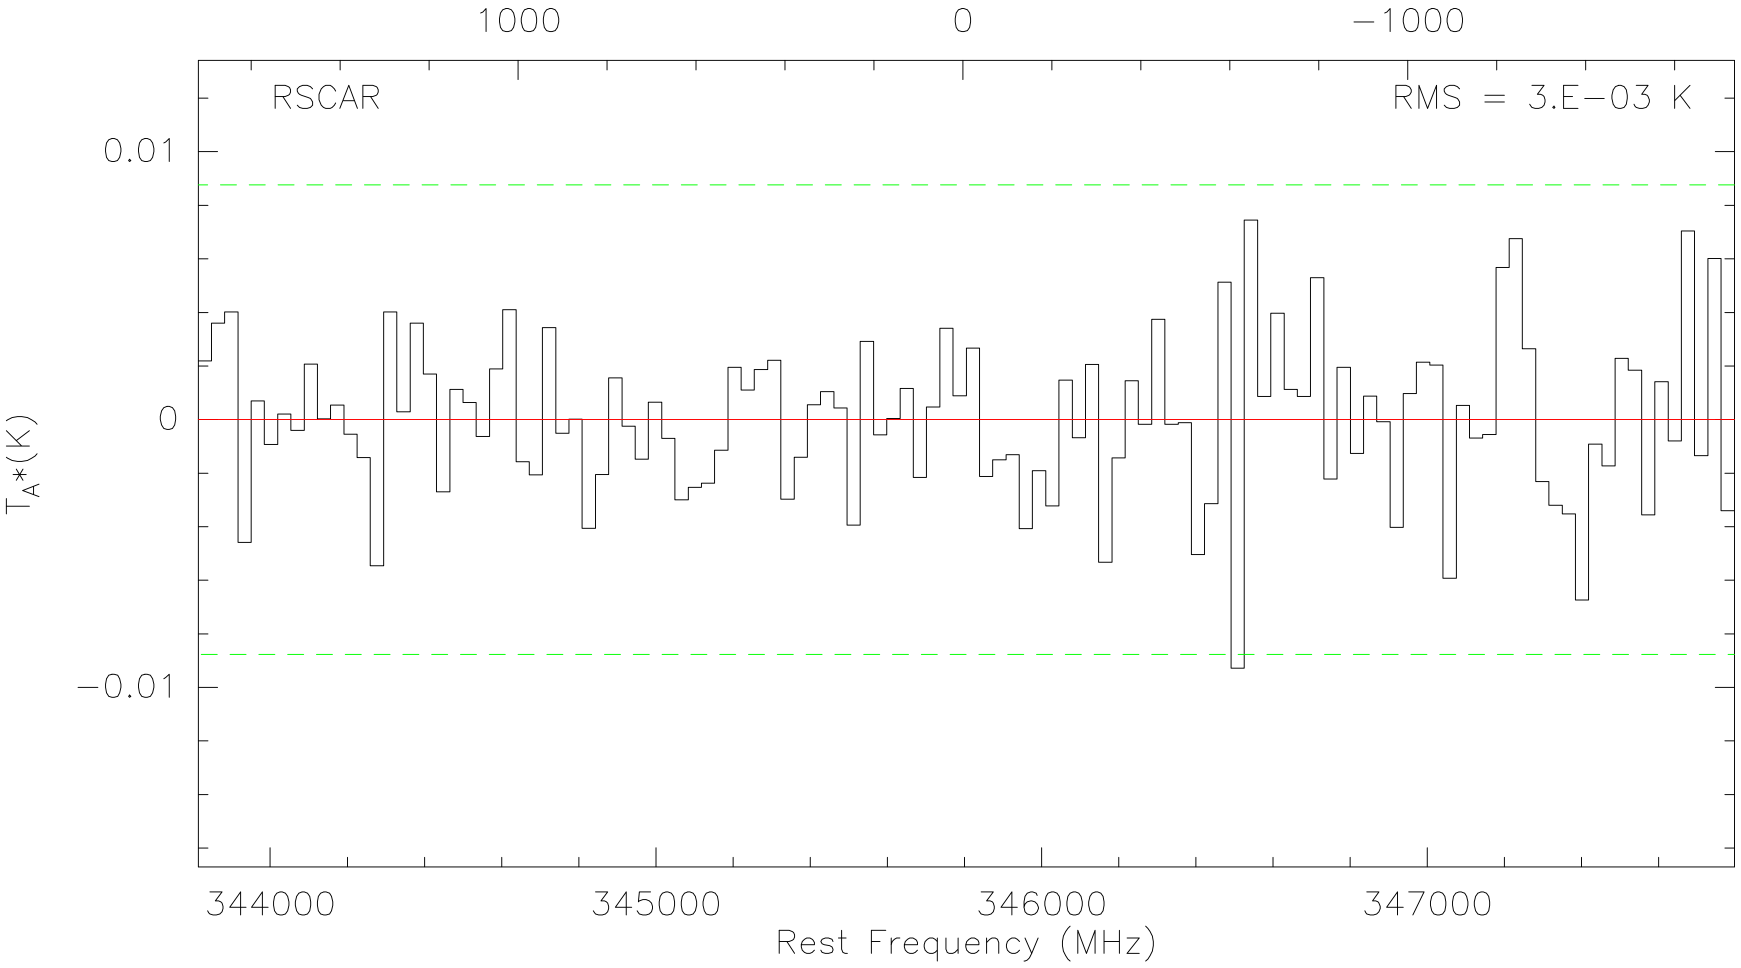

1;1 V1015SGR CO(3-2) AP-F302-XF0- O:13-JUL-2016 R:07-AUG-2020
RA: 18:09:02.00 DEC: -32:28:32.0 Eq 2000.0 Rad. 0.0° Offs: +0.3 -0.3
Unknown tau: 0.233 Tsys: 253. Time: 19.8min El: 45.6
N: 116 I0: 58.7552 V0: 0.000 Dv: 29.76 LSR
F0: 345795.990 Df: -34.33 Fi: 333796.108

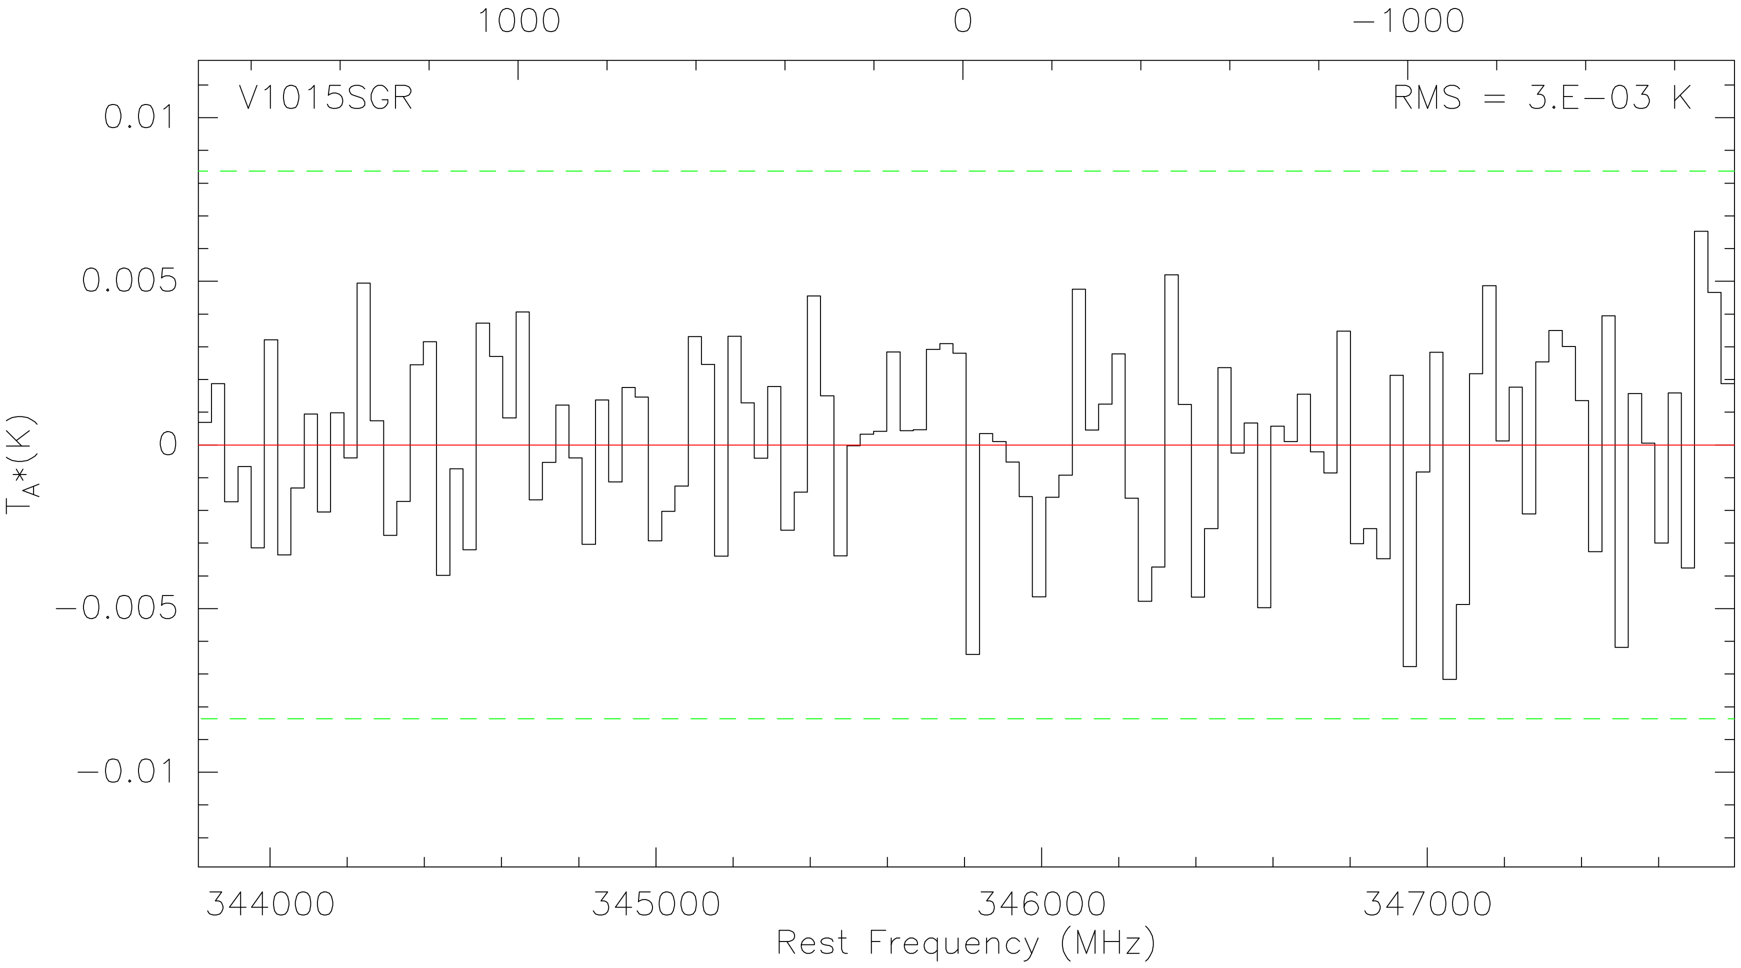

1;1 V1016SGR CO(3-2) AP-F302-XF0- O:13-JUL-2016 R:07-AUG-2020
RA: 18:19:57.63 DEC: -25:11:14.6 Eq 2000.0 Rad. 0.0° Offs: -0.2 -0.3
Unknown tau: 0.168 Tsys: 228. Time: 9.9min El: 32.1
N: 116 I0: 58.7552 V0: 0.000 Dv: 29.76 LSR
F0: 345795.990 Df: -34.33 Fi: 333796.094

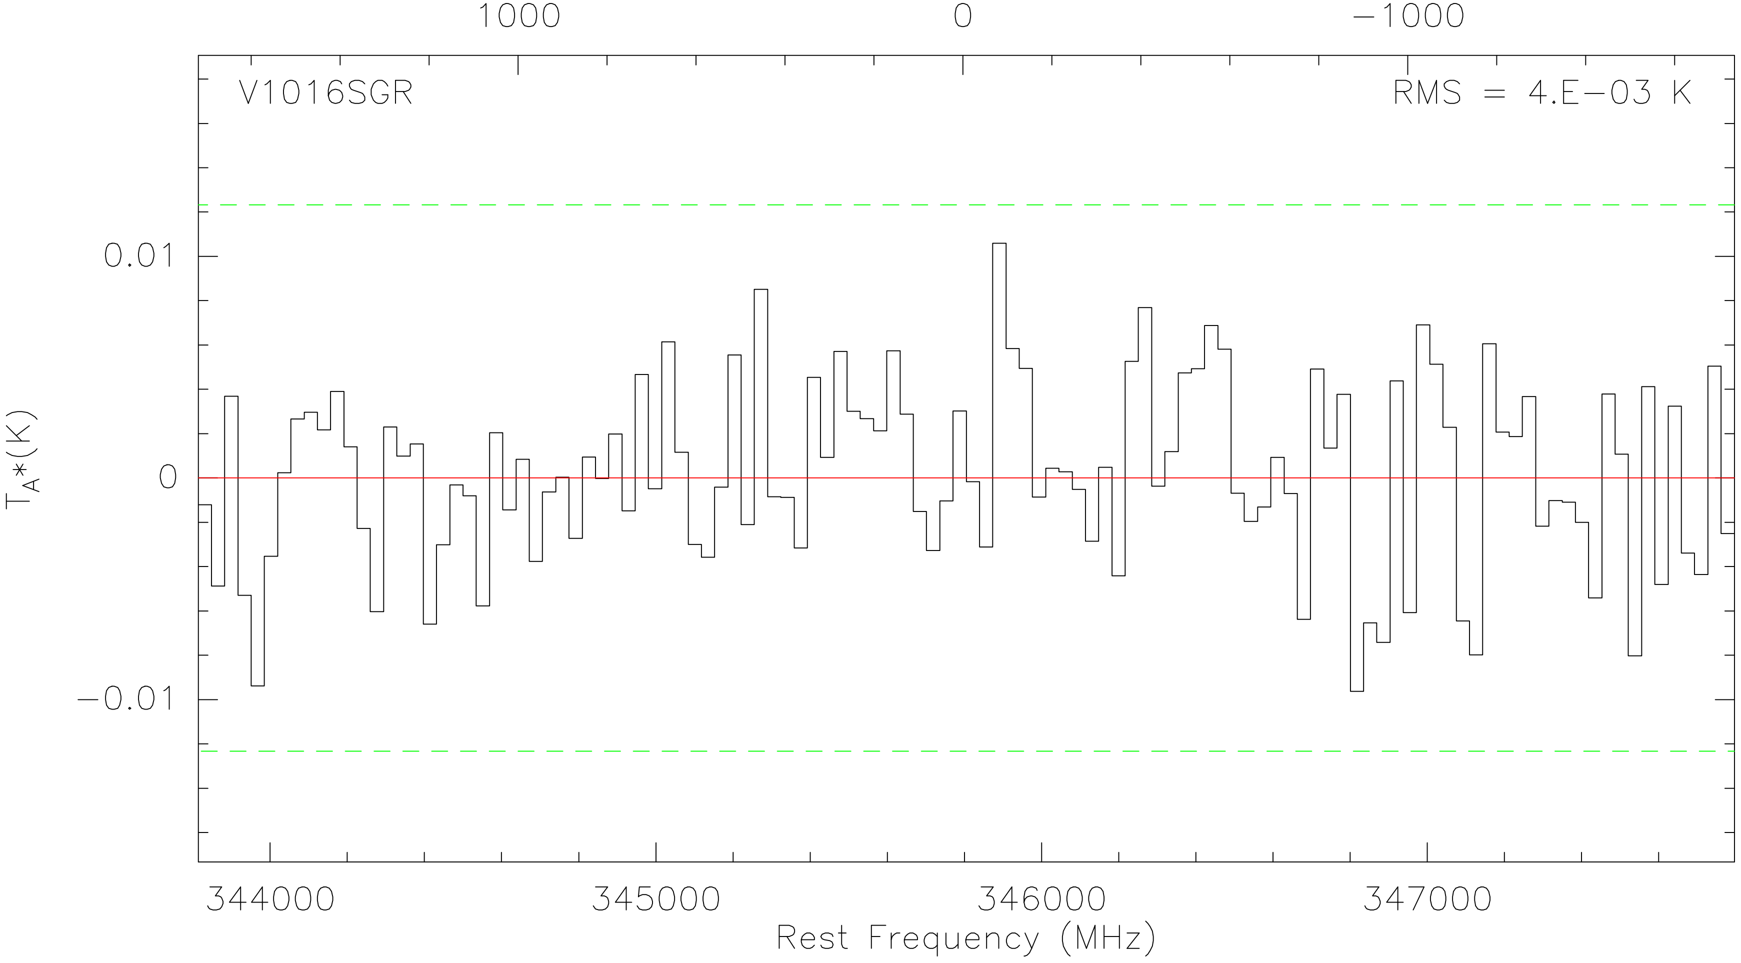

1;1 V1017SGR CO(3-2) AP-F302-XF0- O:13-JUL-2016 R:07-AUG-2020
RA: 18:32:04.47 DEC: -29:23:12.5 Eq 2000.0 Rad. 0.0° Offs: +0.4 -0.4
Unknown tau: 0.239 Tsys: 201. Time: 14.9min El: 75.2
N: 116 I0: 58.7552 V0: 0.000 Dv: 29.76 LSR
F0: 345795.990 Df: -34.33 Fi: 333796.115

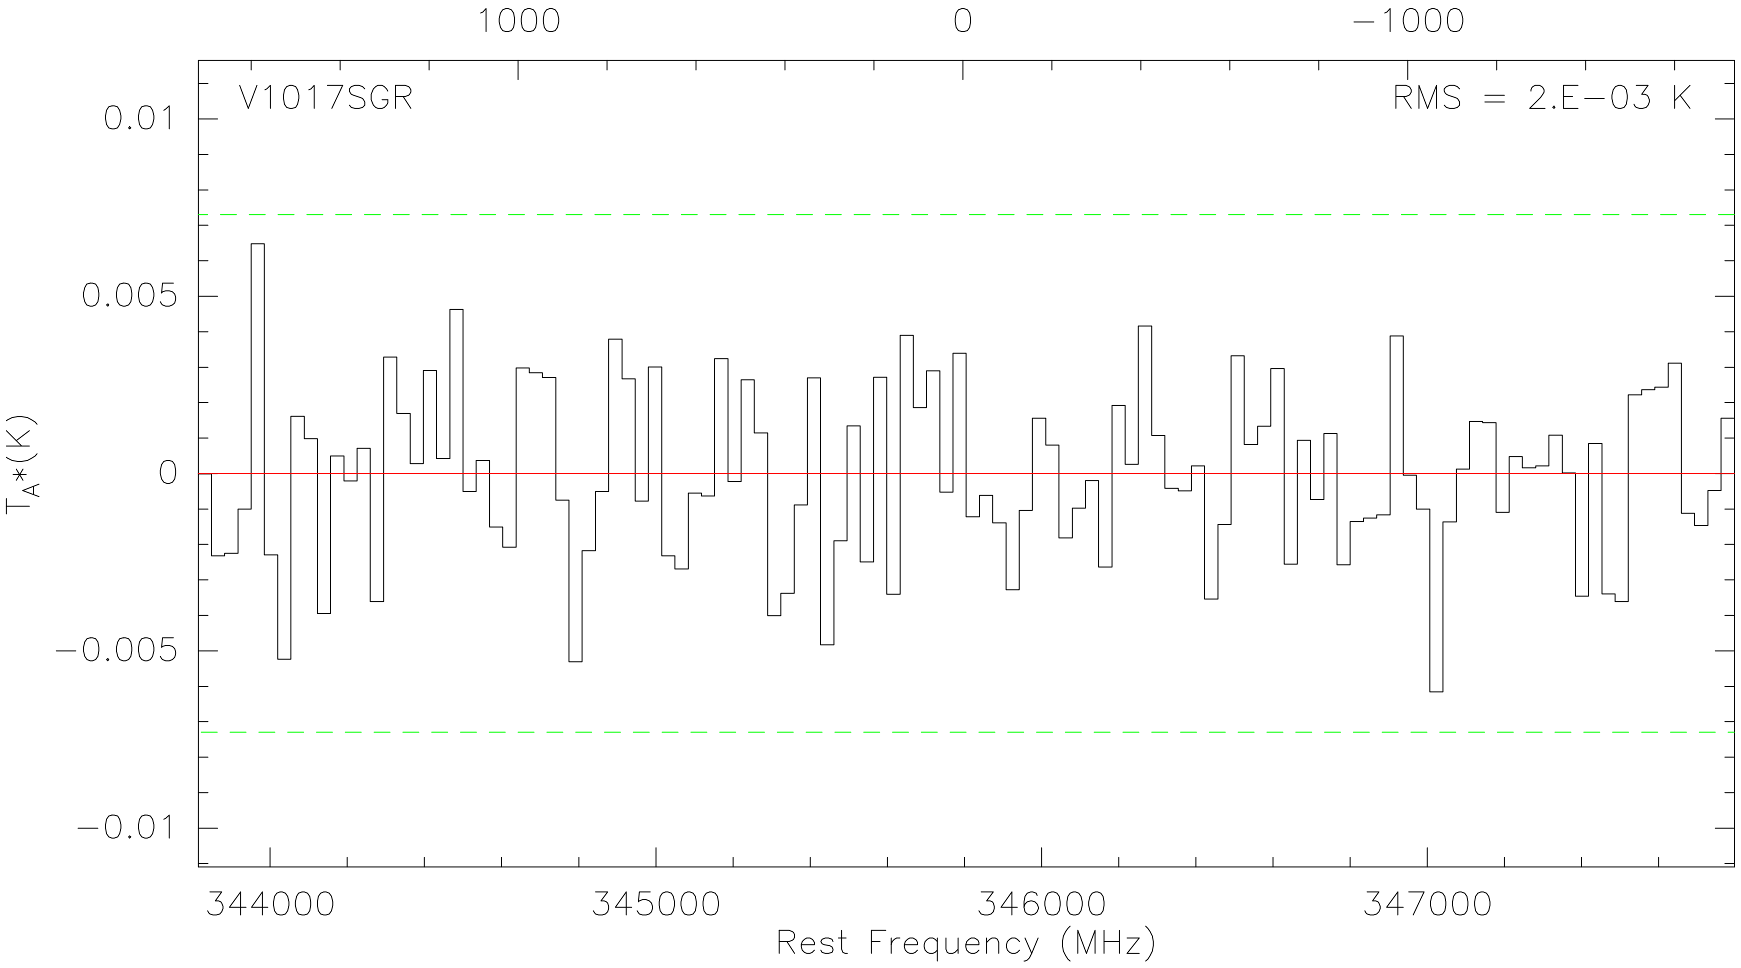

1;1 V1149SGR CO(3−2) AP−F302−XF0− O:13−JUL−2016 R:07−AUG−2020
RA: 18:18:30.40 DEC: −28:17:17.0 Eq 2000.0 Rad. 0.0° Offs: −0.2 −0.6
Unknown tau: 0.190 Tsys: 188. Time: 9.9min El: 61.7
N: 116 I0: 58.7552 V0: 0.000 Dv: 29.76 LSR
F0: 345795.990 Df: −34.33 Fi: 333796.059

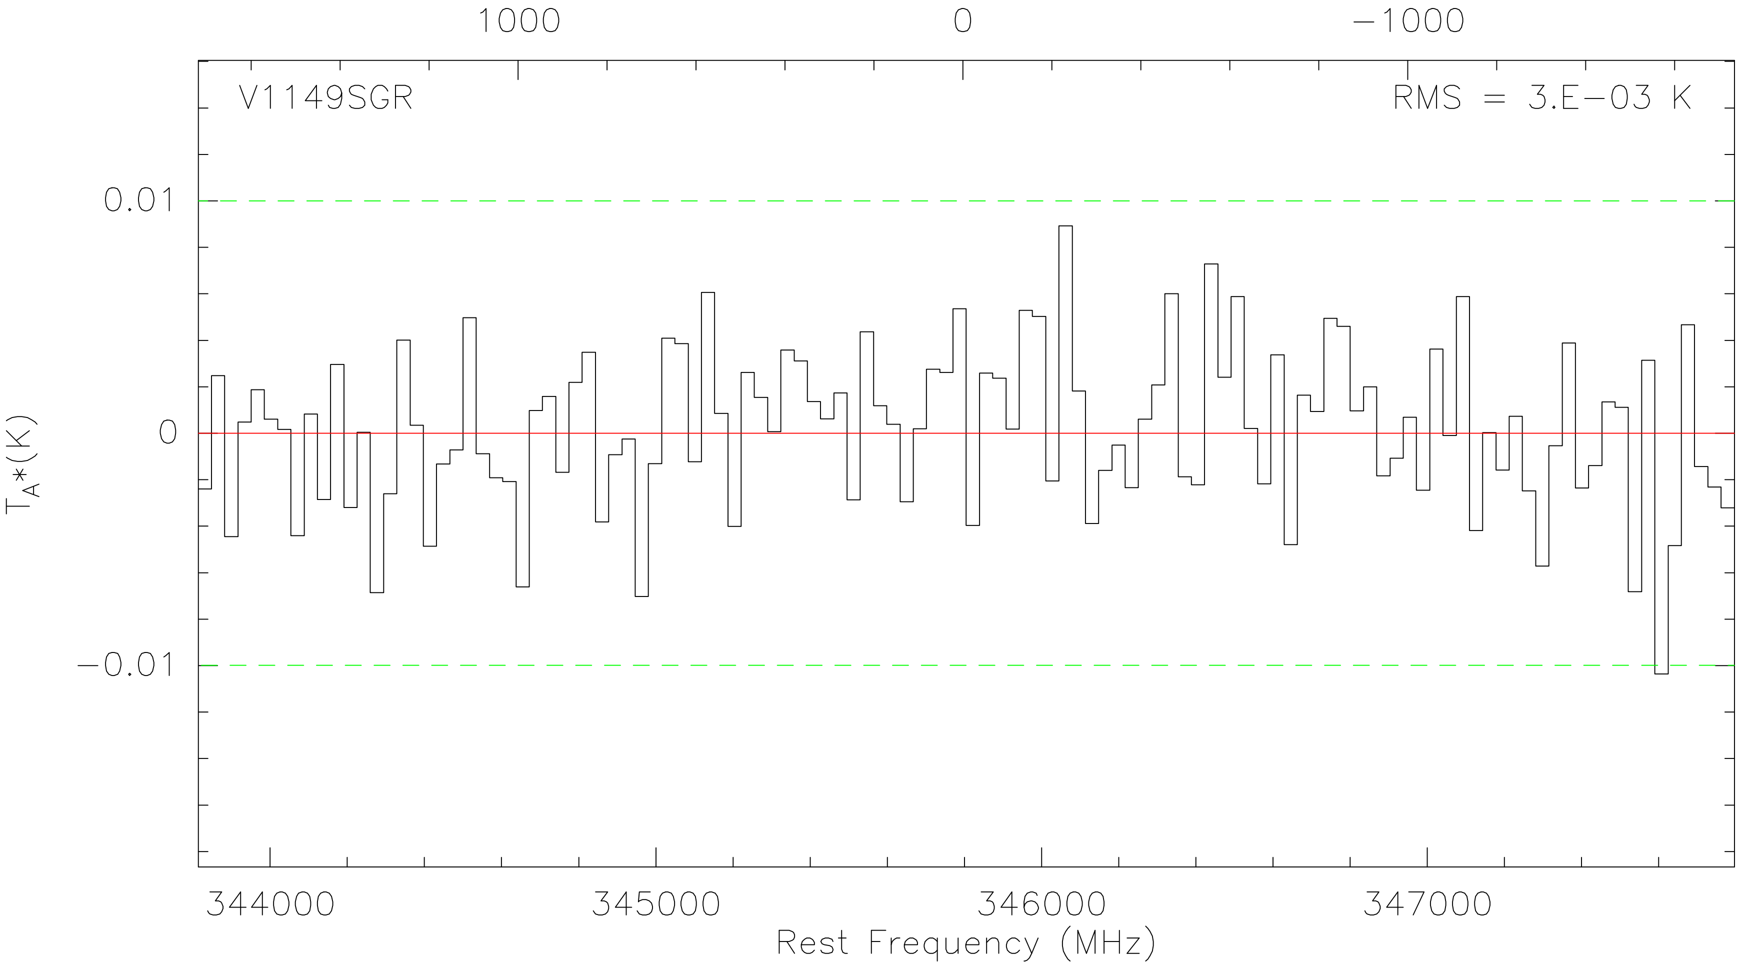

1;1 V1151SGR CO(3-2) AP-F302-XF0- O:14-JUL-2016 R:07-AUG-2020
RA: 18:25:23.75 DEC: -20:11:59.3 Eq 2000.0 Rad. 0.0° Offs: -0.2 -0.3
Unknown tau: 0.180 Tsys: 264. Time: 9.9min El: 26.8
N: 116 I0: 58.7552 V0: 0.000 Dv: 29.76 LSR
F0: 345795.990 Df: -34.33 Fi: 333796.156

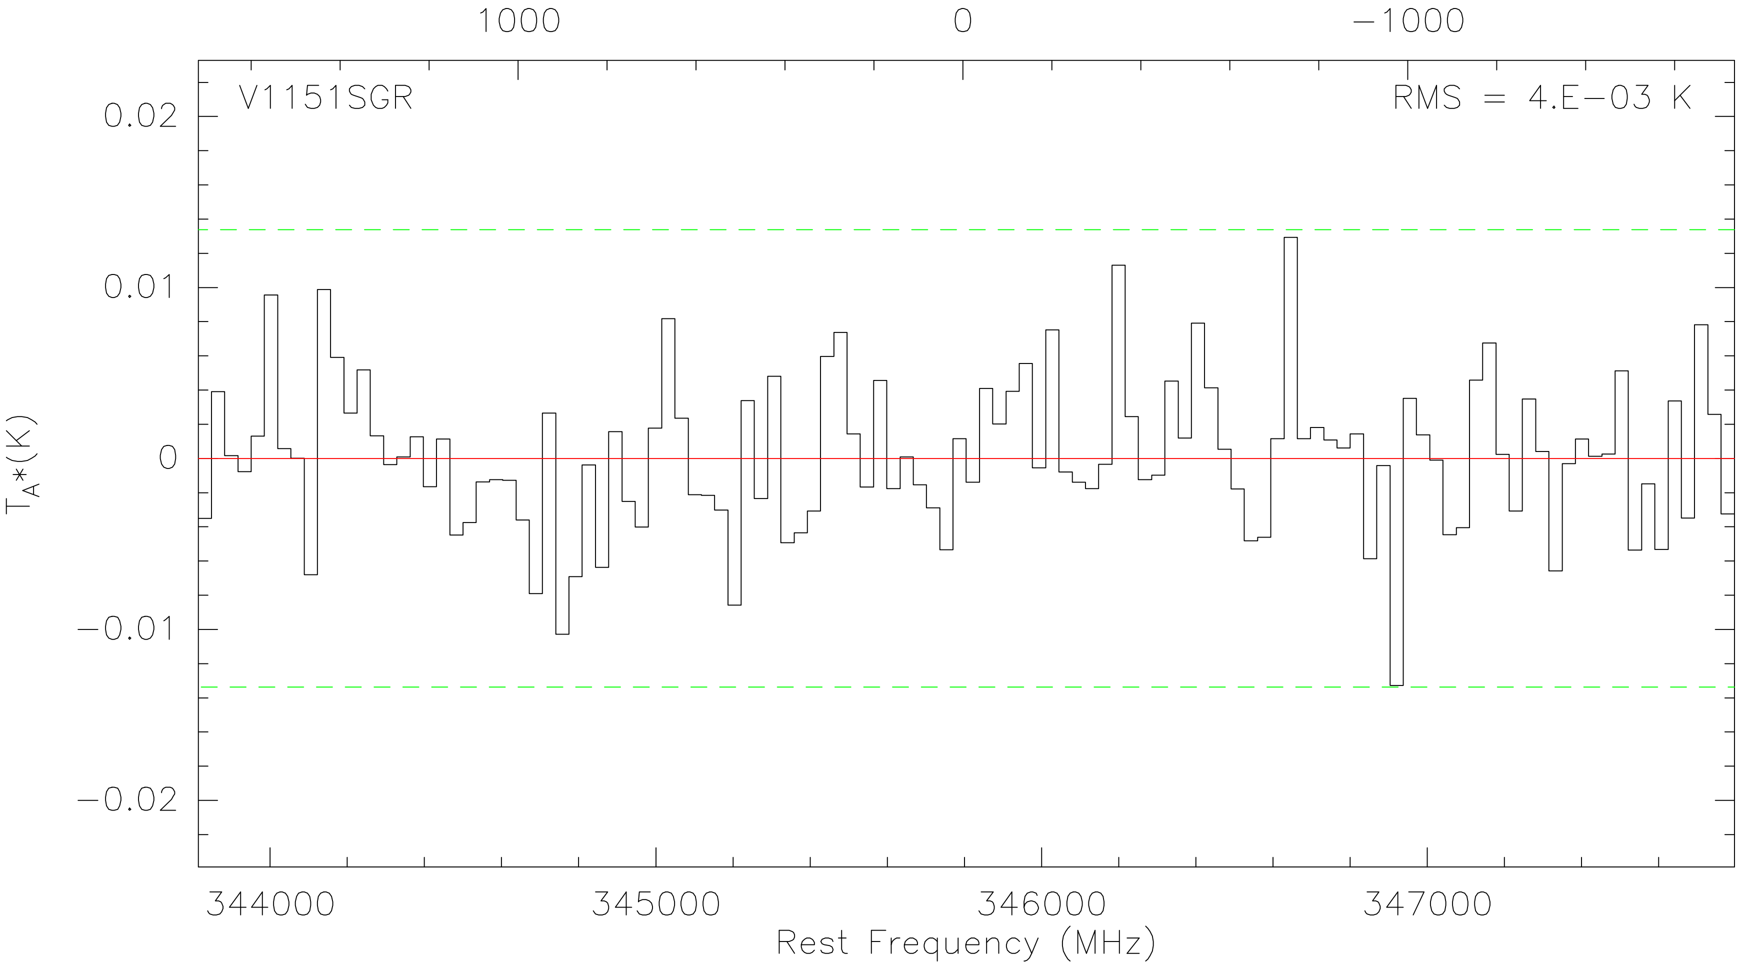

1;1 V1583SGR CO(3-2) AP-F302-XF0- O:14-JUL-2016 R:07-AUG-2020
RA: 18:15:26.30 DEC: -23:23:18.0 Eq 2000.0 Rad. 0.0° Offs: -0.2 -0.3
Unknown tau: 0.187 Tsys: 253. Time: 9.9min El: 30.0
N: 116 I0: 58.7552 V0: 0.000 Dv: 29.76 LSR
F0: 345795.990 Df: -34.33 Fi: 333796.076

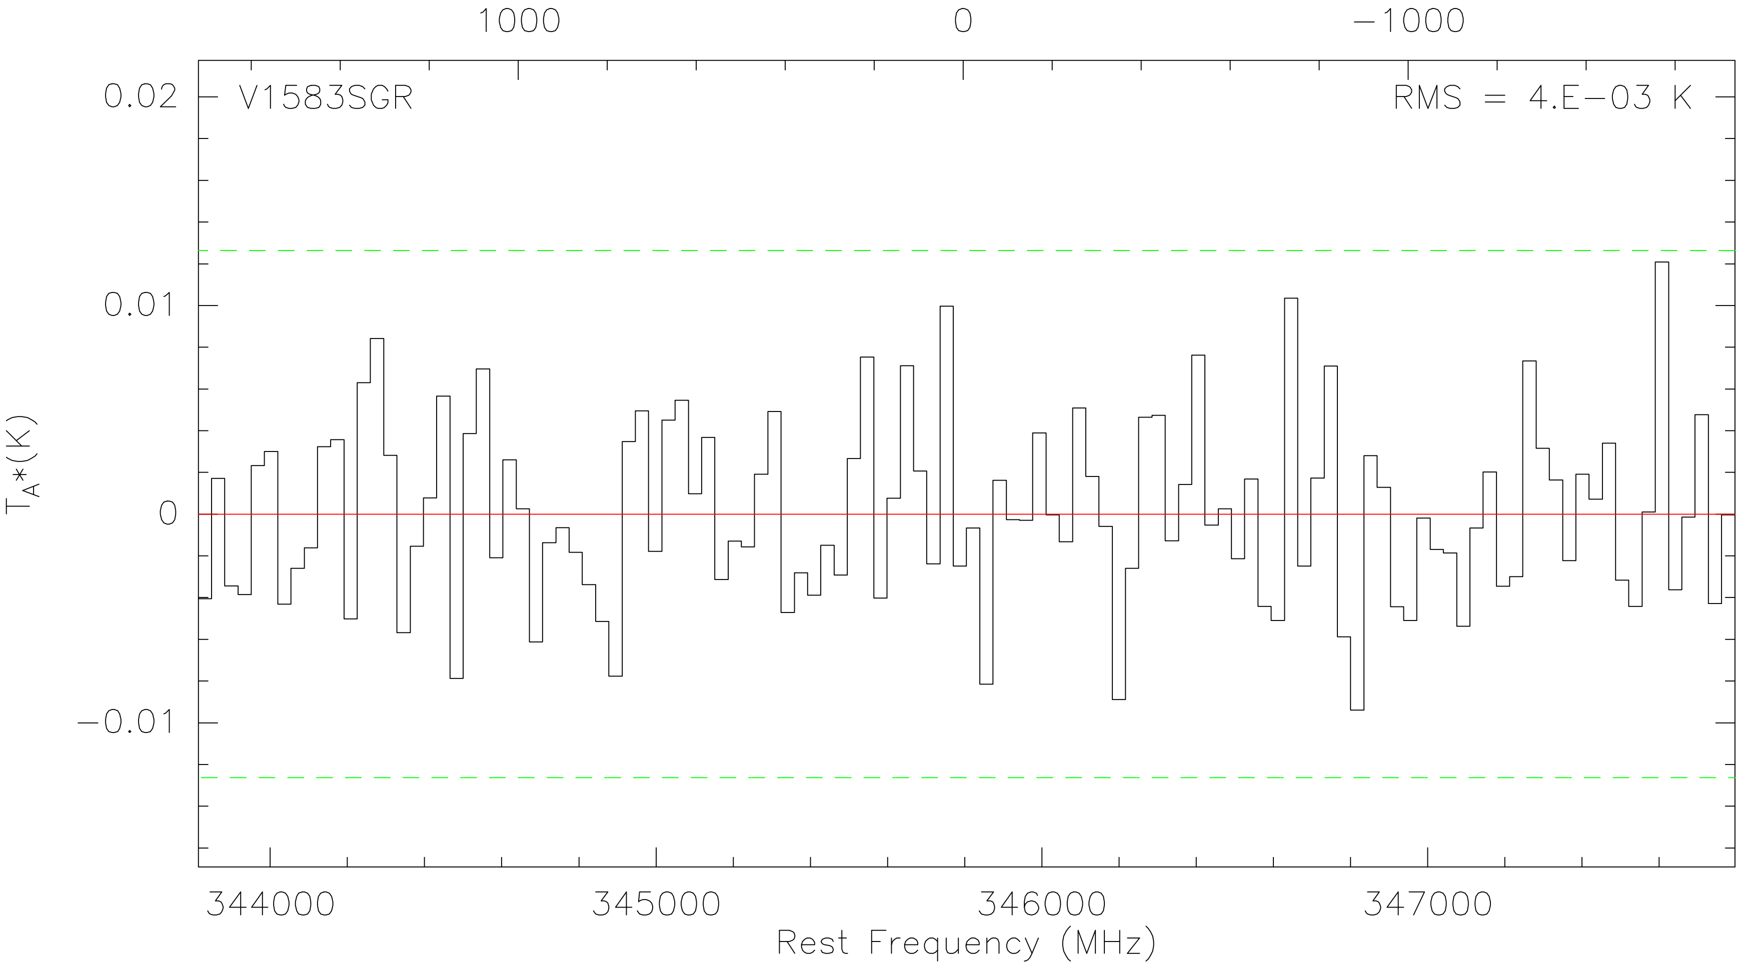

1;1 V363SGR CO(3-2) AP-F302-XF0- O:01-JUL-2016 R:07-AUG-2020
RA: 19:11:16.30 DEC: -29:50:00.0 Eq 2000.0 Rad. 0.0° Offs: -0.2 -0.6
Unknown tau: 0.381 Tsys: 350. Time: 19.9min El: 42.0
N: 116 I0: 58.7552 V0: 0.000 Dv: 29.76 LSR
F0: 345795.990 Df: -34.33 Fi: 333796.475

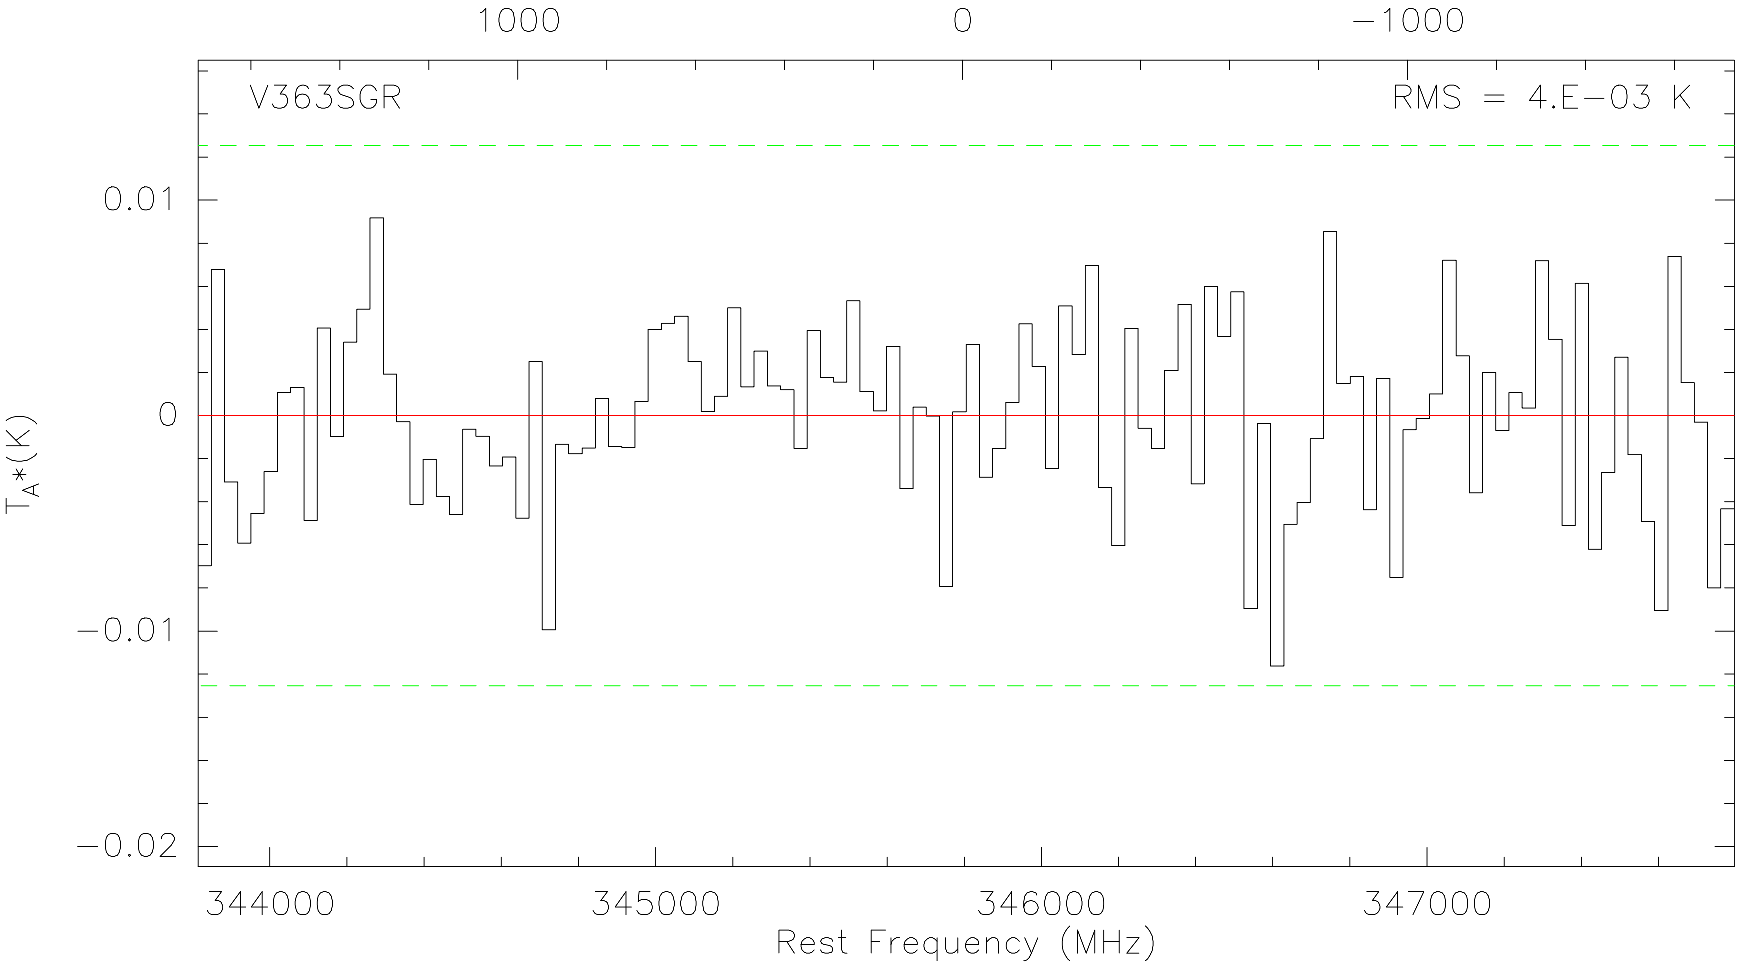

1;1 V365CAR CO(3-2) AP-F302-XF0- O:30-JUN-2016 R:07-AUG-2020
RA: 11:03:16.77 DEC: -58:27:24.9 Eq 2000.0 Rad. 0.0° Offs: +0.3 -0.5
Unknown tau: 0.232 Tsys: 233. Time: 19.8min El: 51.3
N: 116 I0: 58.7552 V0: 0.000 Dv: 29.77 LSR
F0: 345795.990 Df: -34.34 Fi: 333794.926

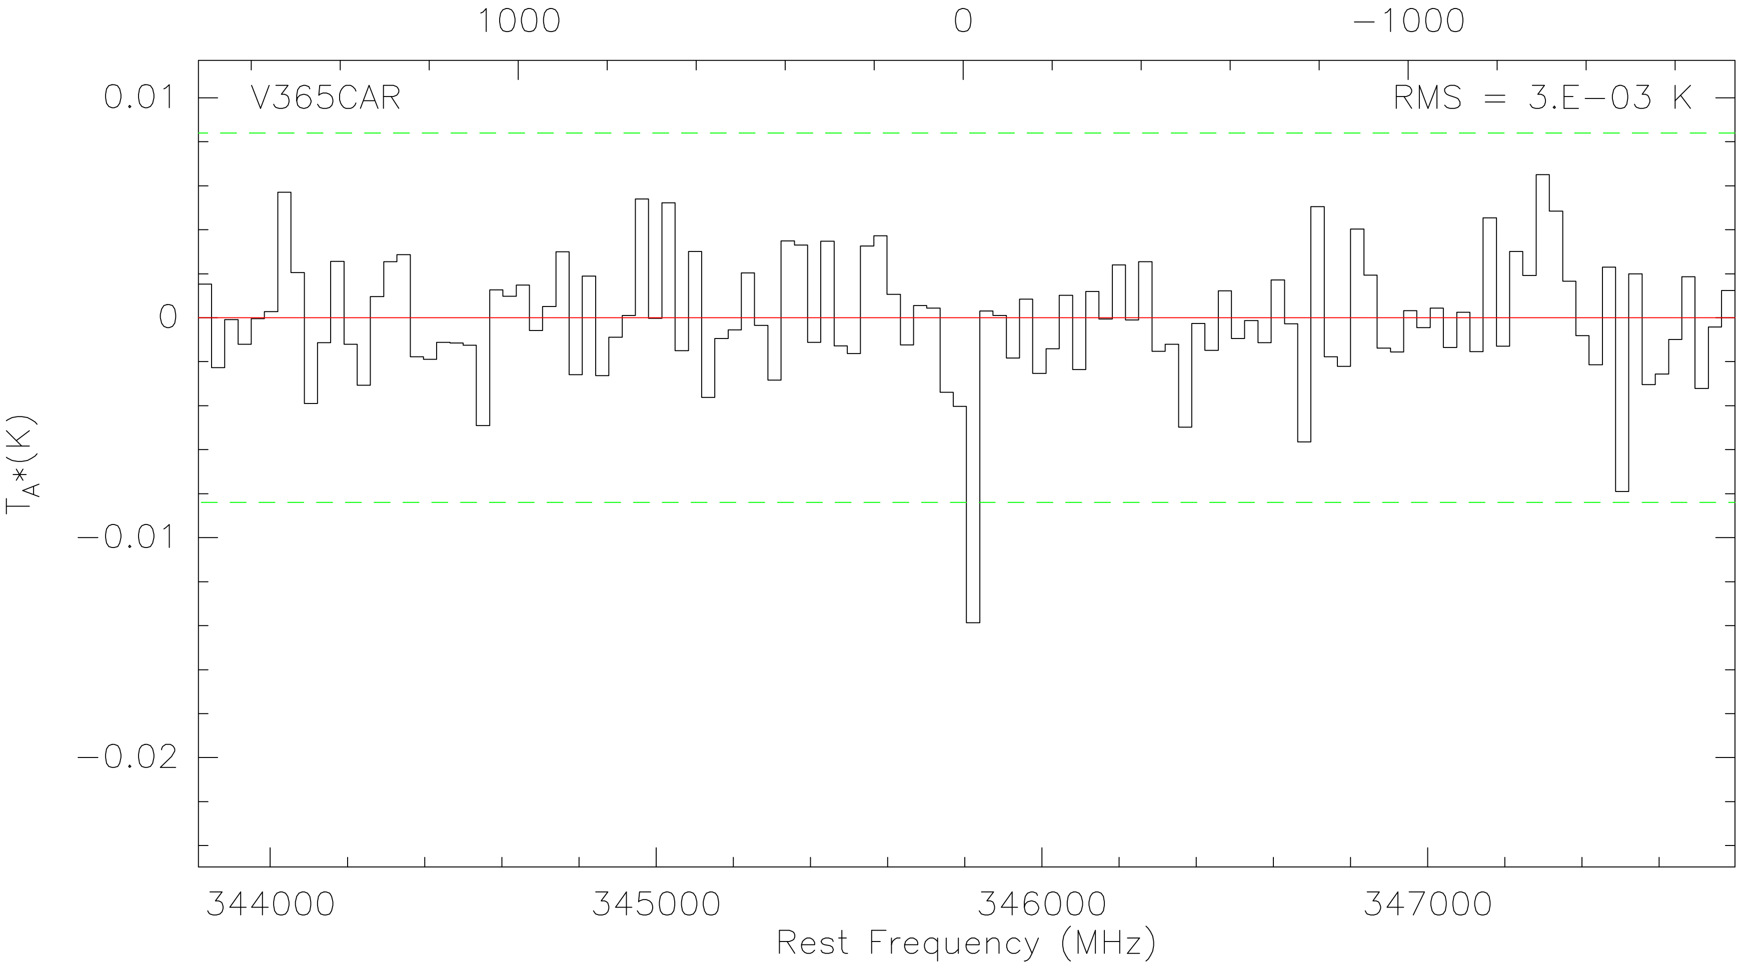

1;1 V382SCO CO(3-2) AP-F302-XF0- O:13-JUL-2016 R:07-AUG-2020
RA: 17:51:56.13 DEC: −35:25:05.4 Eq 2000.0 Rad. 0.0° Offs: +0.1 −0.6
Unknown tau: 0.193 Tsys: 181. Time: 9.9min El: 72.8
N: 116 I0: 58.7552 V0: 0.000 Dv: 29.77 LSR
F0: 345795.990 Df: −34.33 Fi: 333795.875

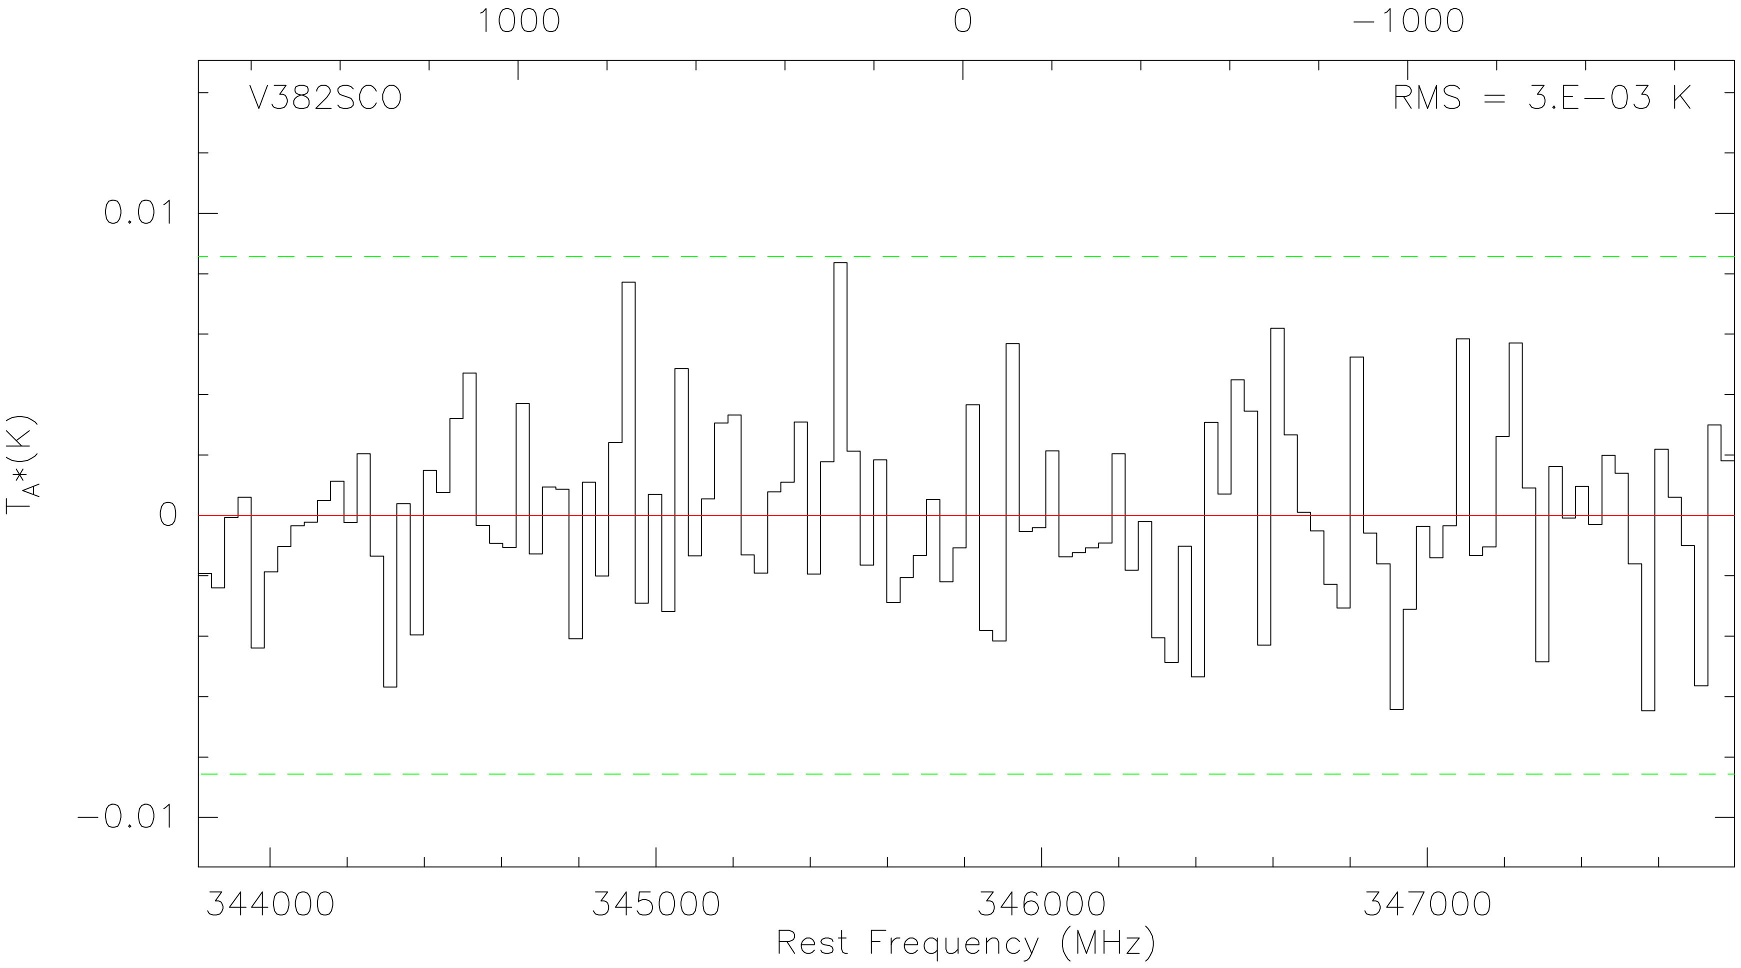

1;1 V384SCO CO(3-2) AP-F302-XF0- O:14-JUL-2016 R:07-AUG-2020
RA: 18:01:43.15 DEC: −35:39:27.8 Eq 2000.0 Rad. 0.0° Offs: +0.3 −0.3
Unknown tau: 0.271 Tsys: 251. Time: 9.9min El: 52.1
N: 116 I0: 58.7552 V0: 0.000 Dv: 29.77 LSR
F0: 345795.990 Df: −34.33 Fi: 333795.908

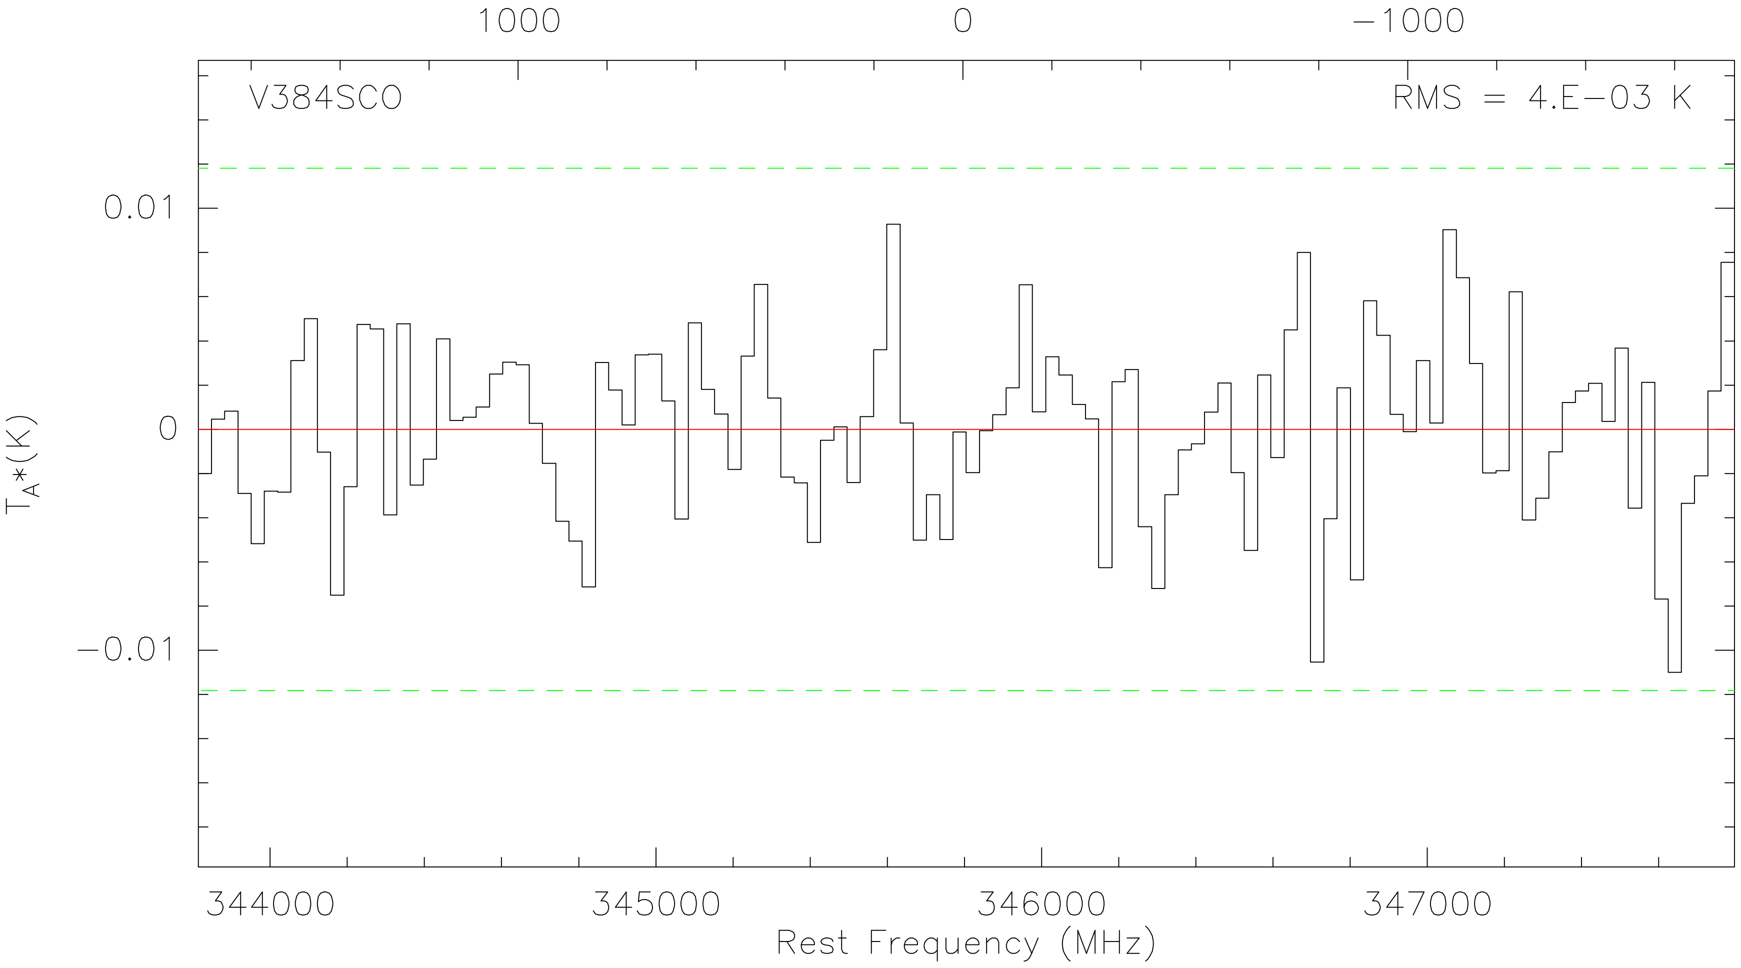

1;1 V522SGR CO(3-2) AP-F302-XF0- O:01-JUL-2016 R:07-AUG-2020
RA: 18:48:00.47 DEC: -25:22:21.9 Eq 2000.0 Rad. 0.0° Offs: -0.2 -0.5
Unknown tau: 0.369 Tsys: 406. Time: 19.8min El: 31.8
N: 116 I0: 58.7552 V0: 0.000 Dv: 29.76 LSR
F0: 345795.990 Df: -34.33 Fi: 333796.445

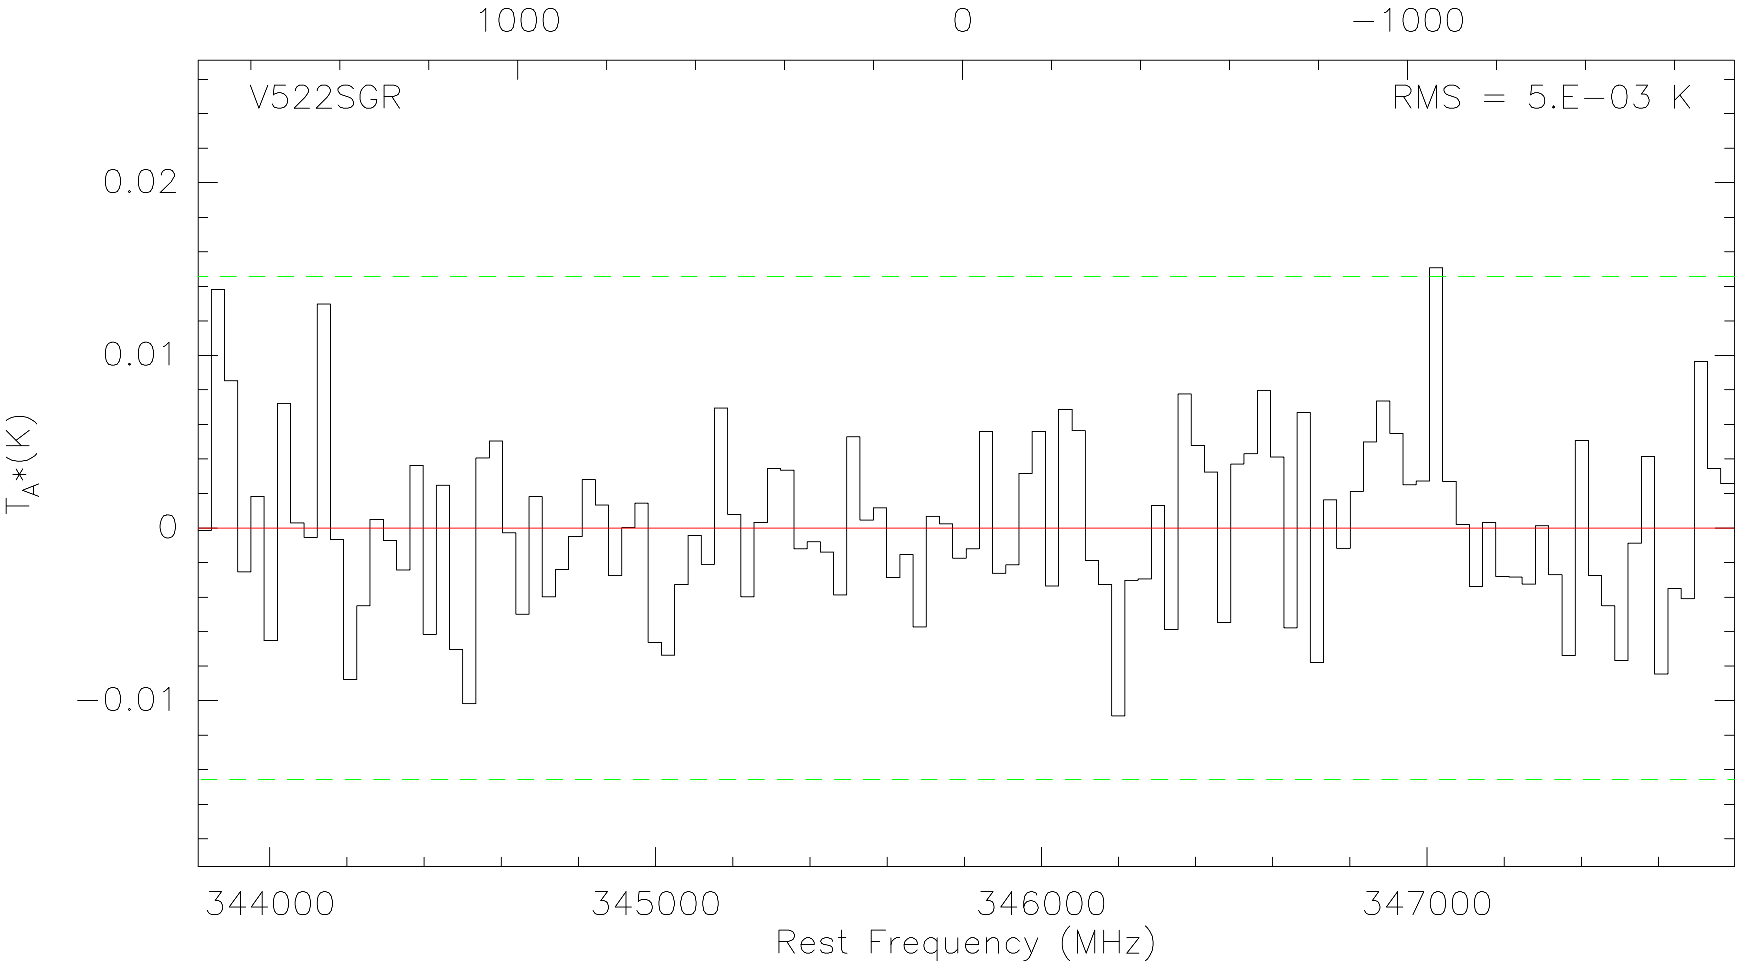

1;1 V5530PH CO(3-2) AP-F302-XF0- O:01-JUL-2016 R:07-AUG-2020
RA: 17:42:53.50 DEC: -24:51:26.2 Eq 2000.0 Rad. 0.0° Offs: -0.4 -0.5
Unknown tau: 0.379 Tsys: 378. Time: 9.9min El: 38.8
N: 116 I0: 58.7552 V0: 0.000 Dv: 29.76 LSR
F0: 345795.990 Df: -34.33 Fi: 333796.162

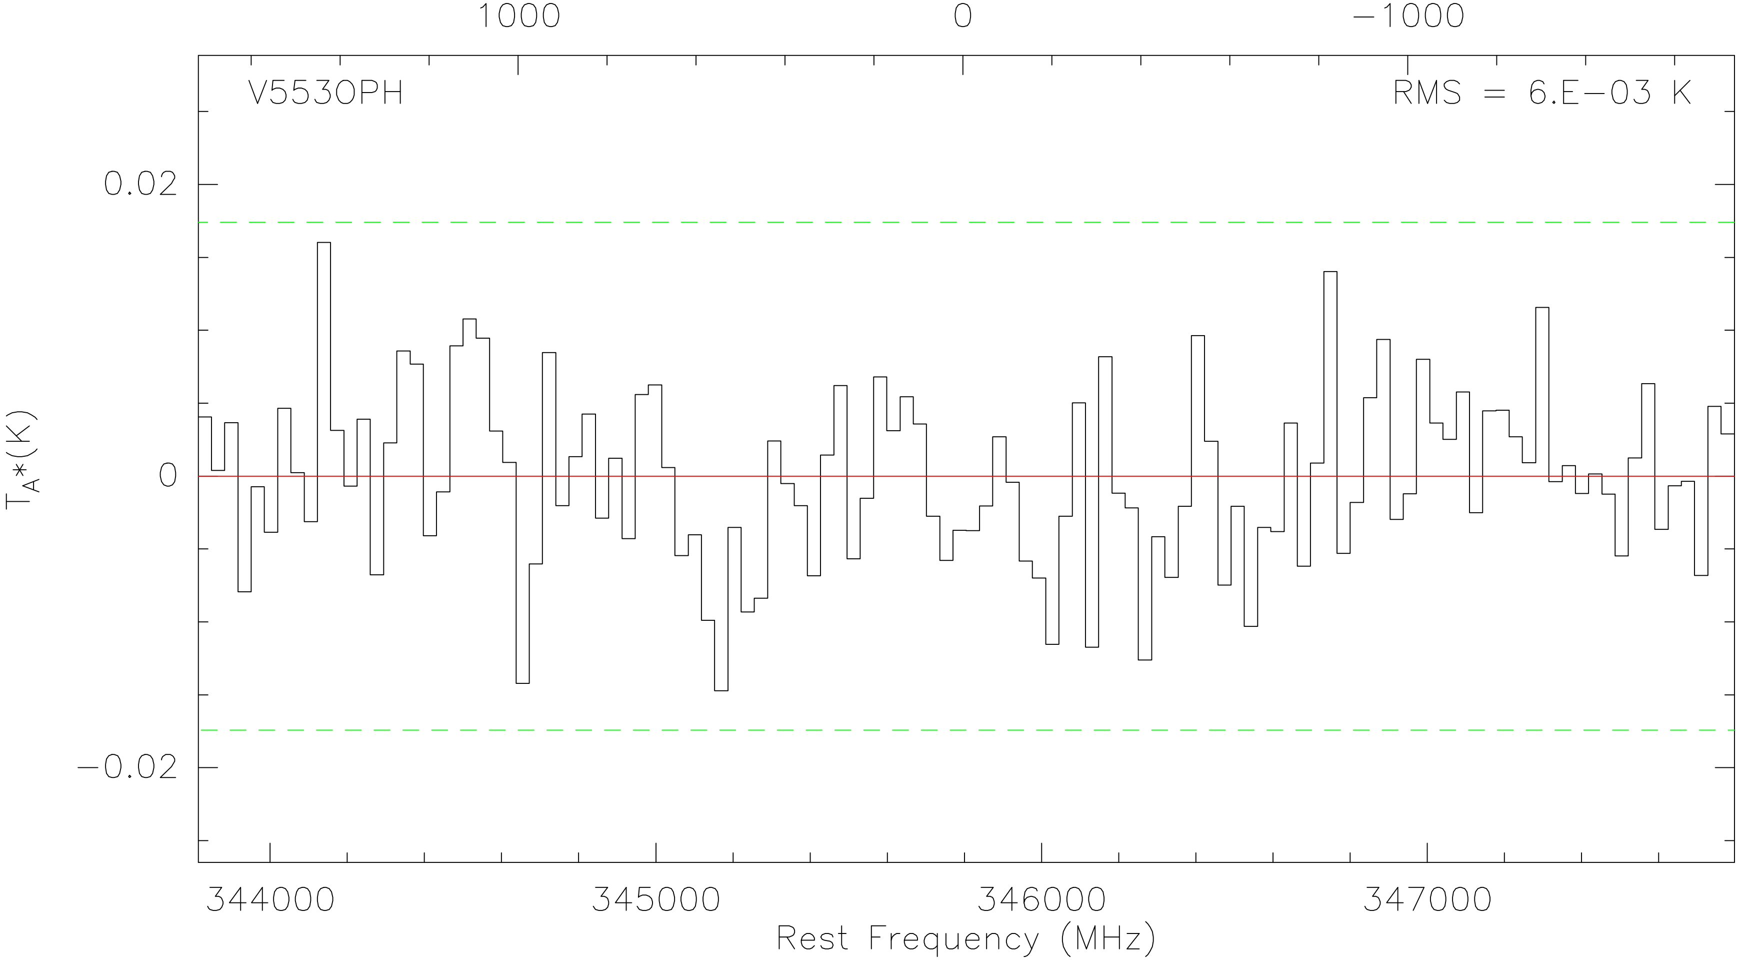

1;1 V696SCO CO(3-2) AP-F302-XF0- O:13-JUL-2016 R:07-AUG-2020
RA: 17:53:11.55 DEC: −35:50:14.4 Eq 2000.0 Rad. 0.0° Offs: +0.2 −0.6
Unknown tau: 0.223 Tsys: 192. Time: 9.9min El: 77.1
N: 116 I0: 58.7552 V0: 0.000 Dv: 29.77 LSR
F0: 345795.990 Df: −34.33 Fi: 333795.879

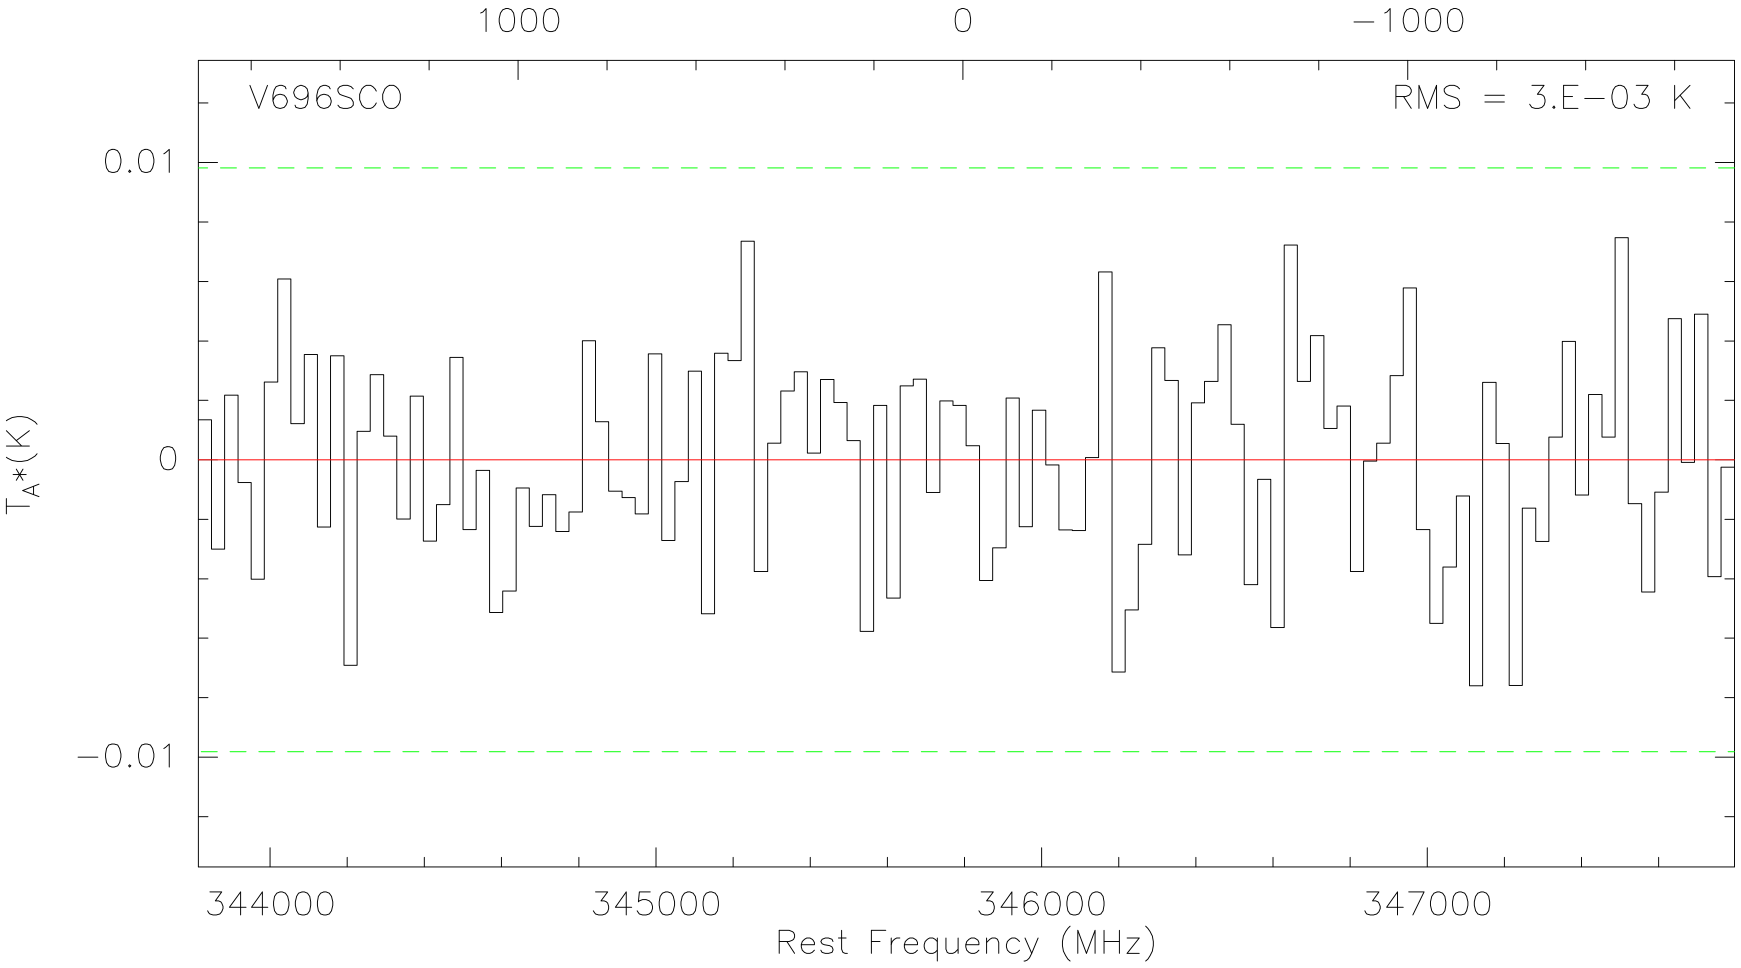

1;1 V697SCO CO(3-2) AP-F302-XF0- O:13-JUL-2016 R:07-AUG-2020
RA: 17:51:21.83 DEC: -37:24:55.2 Eq 2000.0 Rad. 0.0° Offs: -0.2 -0.5
Unknown tau: 0.187 Tsys: 211. Time: 14.9min El: 43.3
N: 116 I0: 58.7552 V0: 0.000 Dv: 29.77 LSR
F0: 345795.990 Df: -34.33 Fi: 333795.842

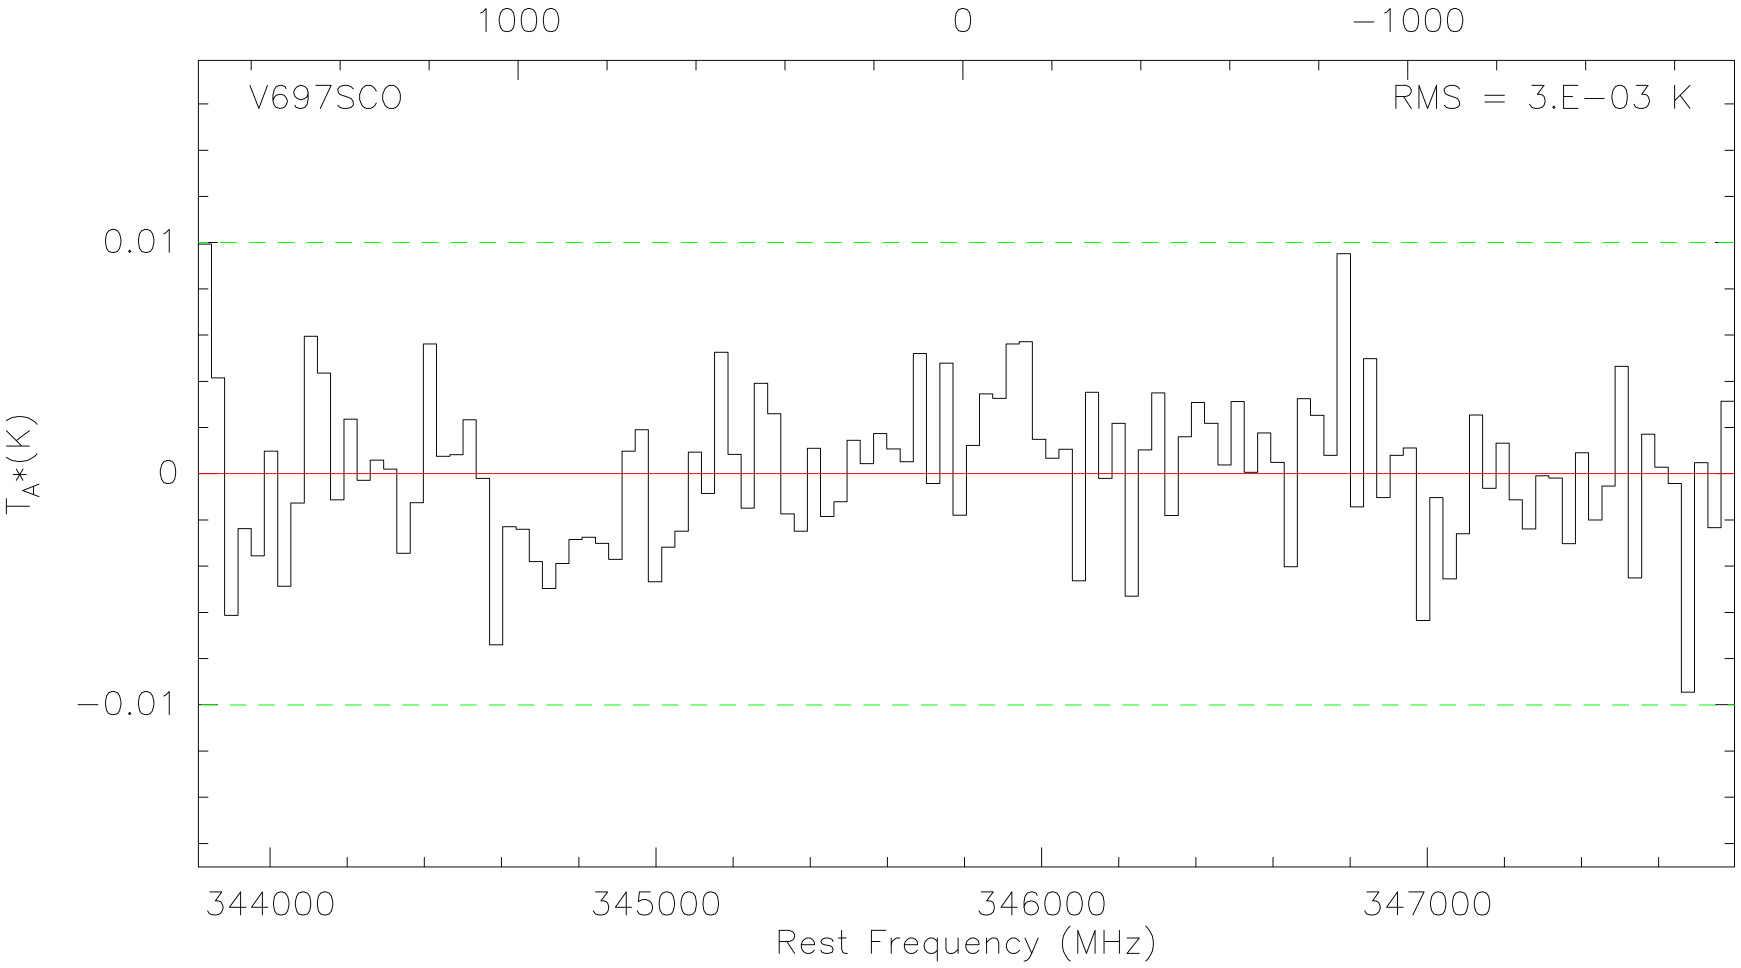

1;1 V707SCO CO(3-2) AP-F302-XF0- O:06-JUL-2016 R:07-AUG-2020
RA: 17:48:26.38 DEC: -36:37:54.9 Eq 2000.0 Rad. 0.0° Offs: +0.3 -0.3
Unknown tau: 0.237 Tsys: 265. Time: 9.9min El: 40.0
N: 116 I0: 58.7552 V0: 0.000 Dv: 29.76 LSR
F0: 345795.990 Df: -34.33 Fi: 333795.975

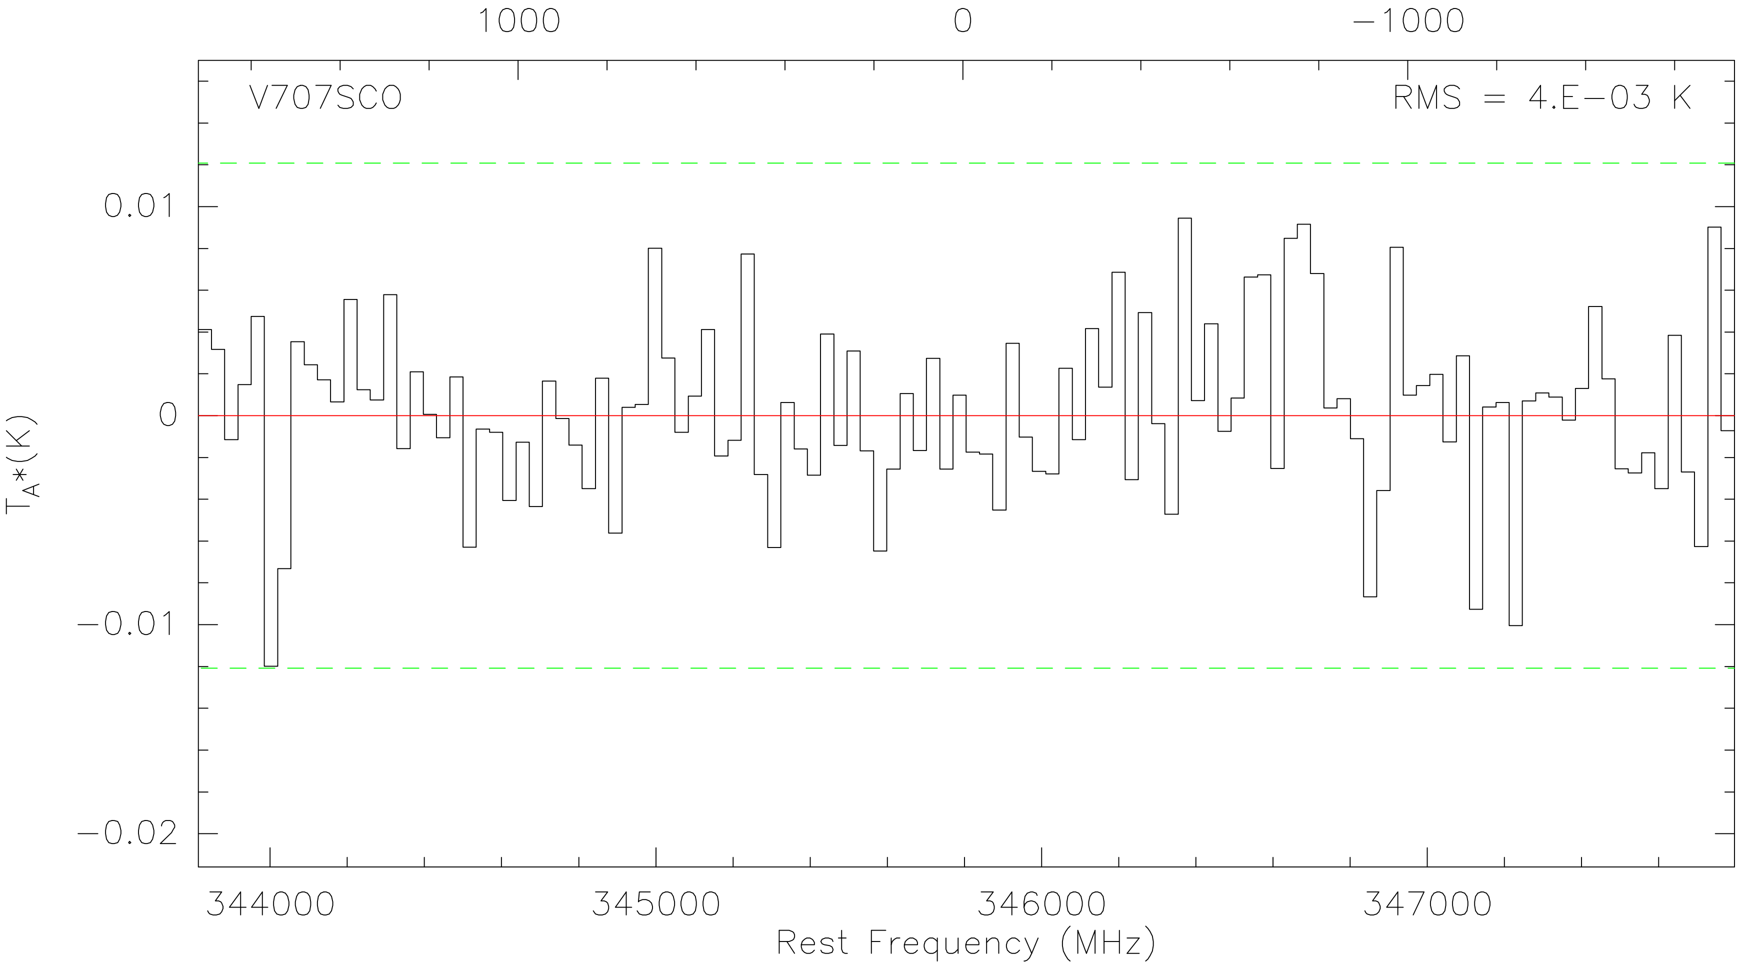

1;1 V711SCO CO(3−2) AP−F302−XF0− O:14−JUL−2016 R:07−AUG−2020
RA: 17:54:06.16 DEC: −34:21:15.5 Eq 2000.0 Rad. 0.0° Offs: +0.3 −0.3
Unknown tau: 0.261 Tsys: 232. Time: 9.9min El: 58.0
N: 116 I0: 58.7552 V0: 0.000 Dv: 29.77 LSR
F0: 345795.990 Df: −34.33 Fi: 333795.891

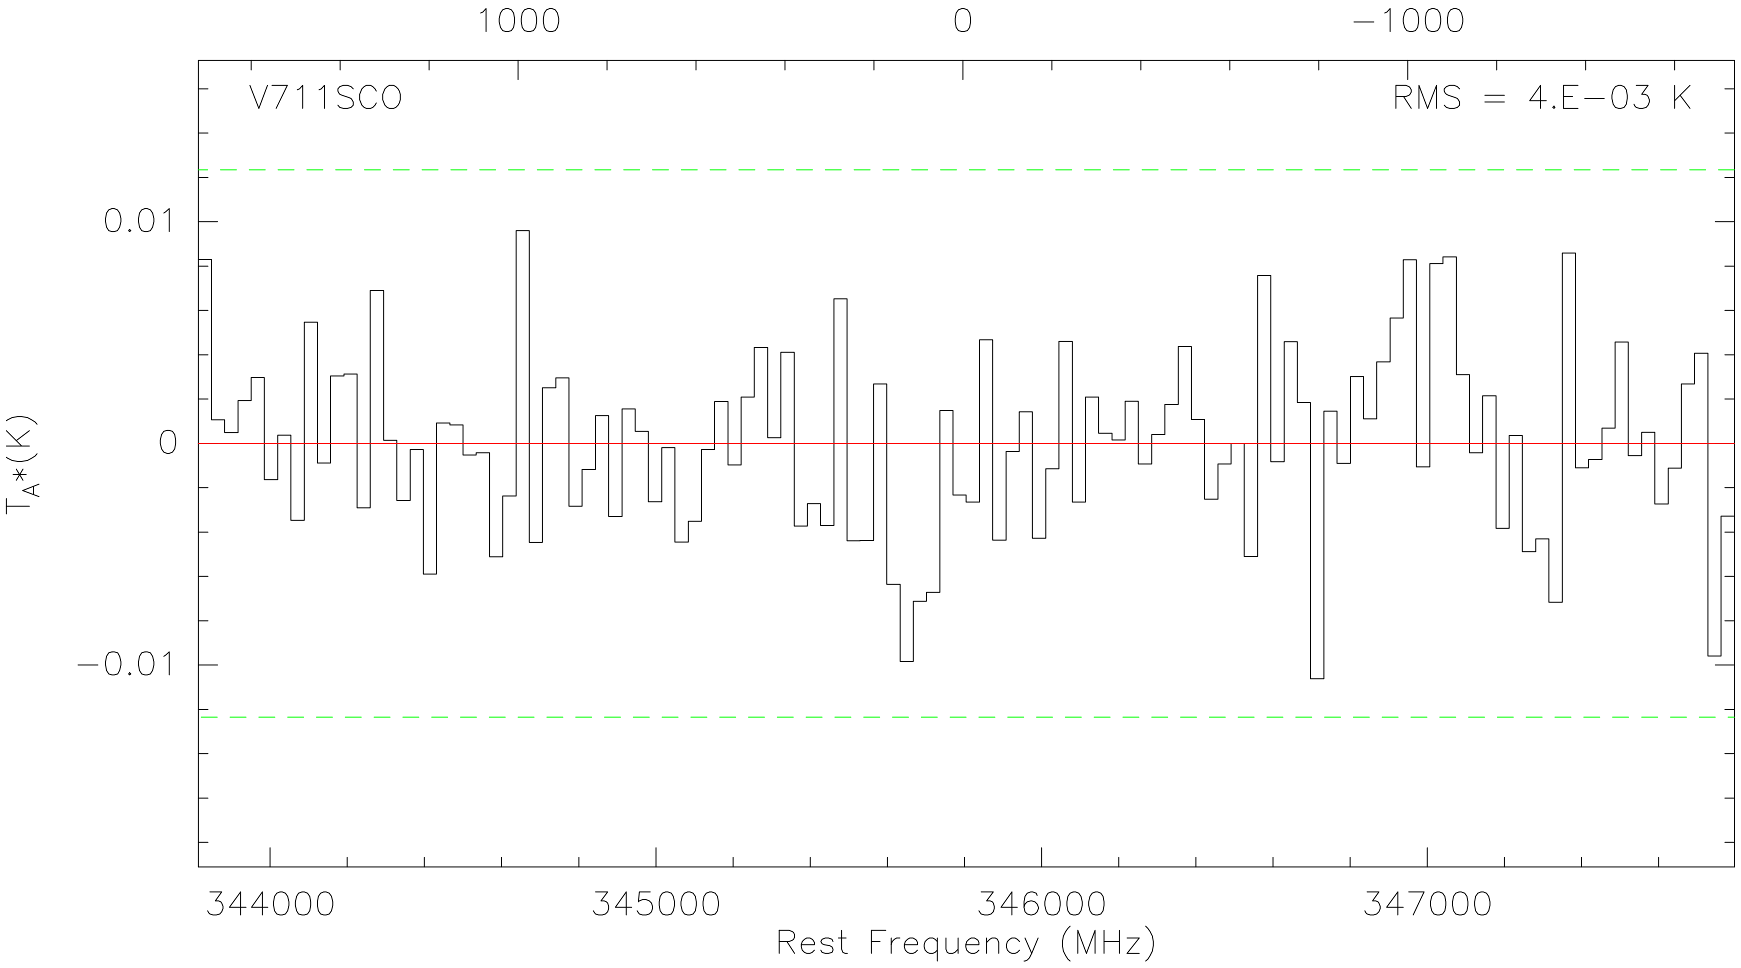

1;1 V729SCO CO(3-2) AP-F302-XF0- O:01-JUL-2016 R:07-AUG-2020
RA: 17:22:02.66 DEC: −32:05:48.8 Eq 2000.0 Rad. 0.0° Offs: −0.2 −0.5
Unknown tau: 0.362 Tsys: 441. Time: 14.9min El: 30.0
N: 116 I0: 58.7552 V0: 0.000 Dv: 29.76 LSR
F0: 345795.990 Df: −34.33 Fi: 333795.989

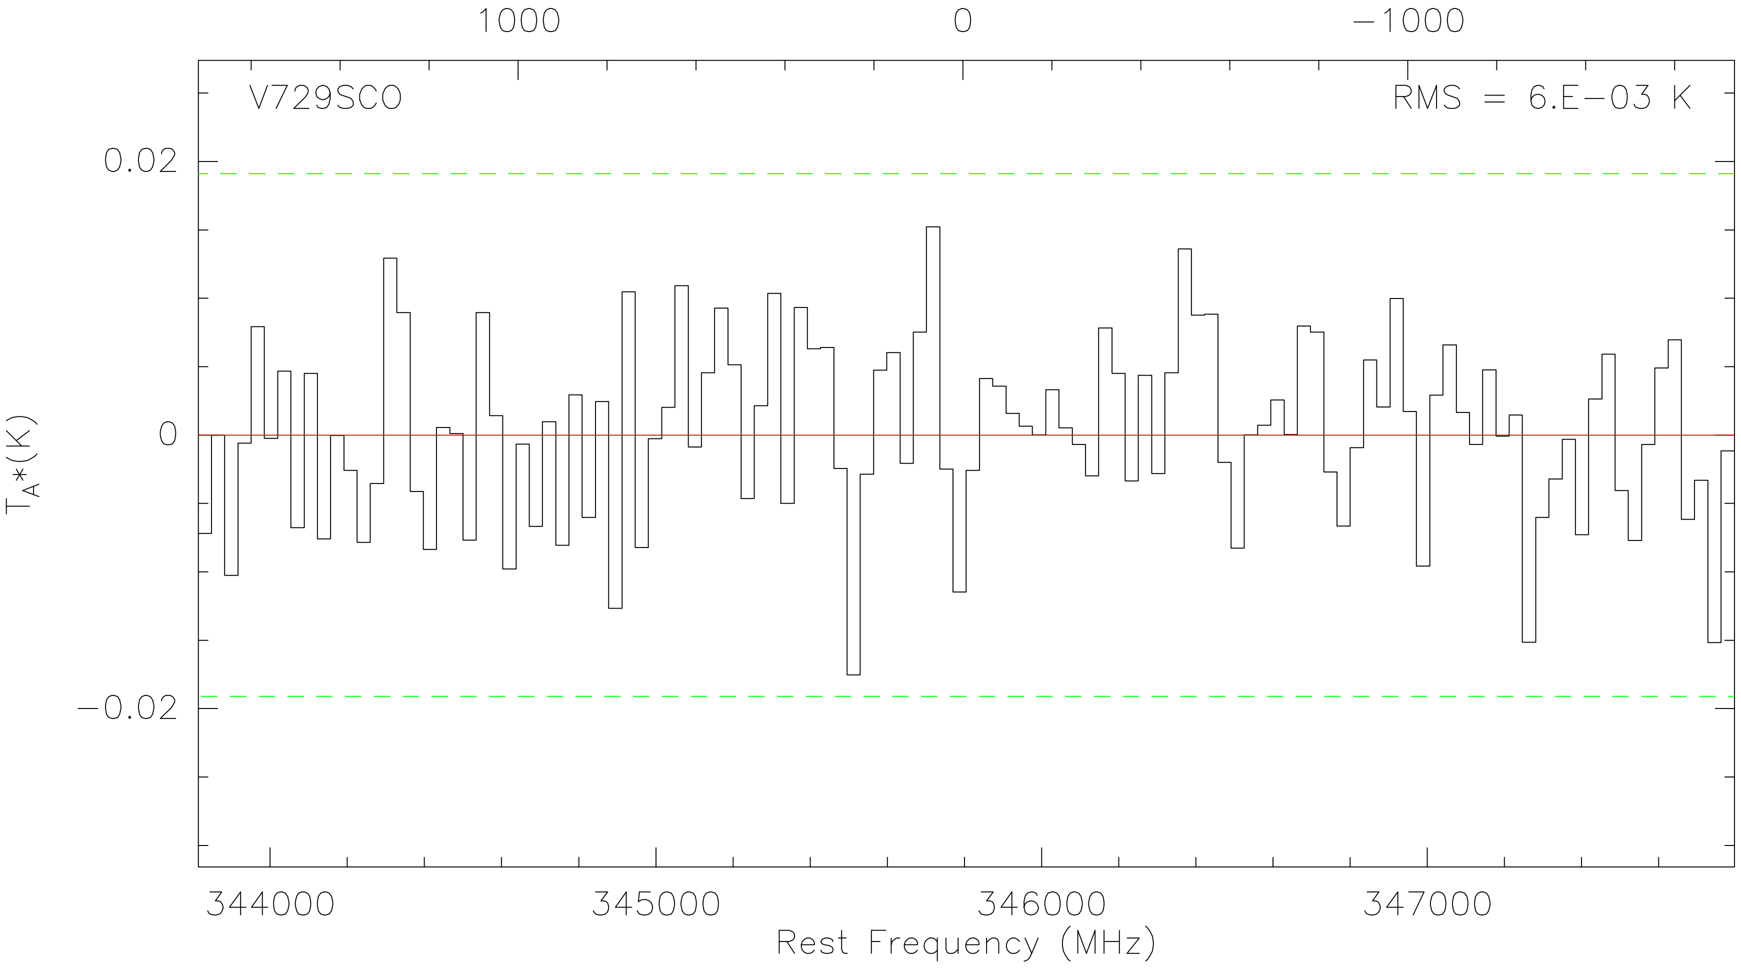

1;1 V732SGR CO(3−2) AP−F302−XF0− O:13−JUL−2016 R:07−AUG−2020
RA: 17:56:07.51 DEC: −27:22:16.1 Eq 2000.0 Rad. 0.0° Offs: +0.2 −0.4
Unknown tau: 0.236 Tsys: 205. Time: 9.9min El: 71.8
N: 116 I0: 58.7552 V0: 0.000 Dv: 29.76 LSR
F0: 345795.990 Df: −34.33 Fi: 333795.991

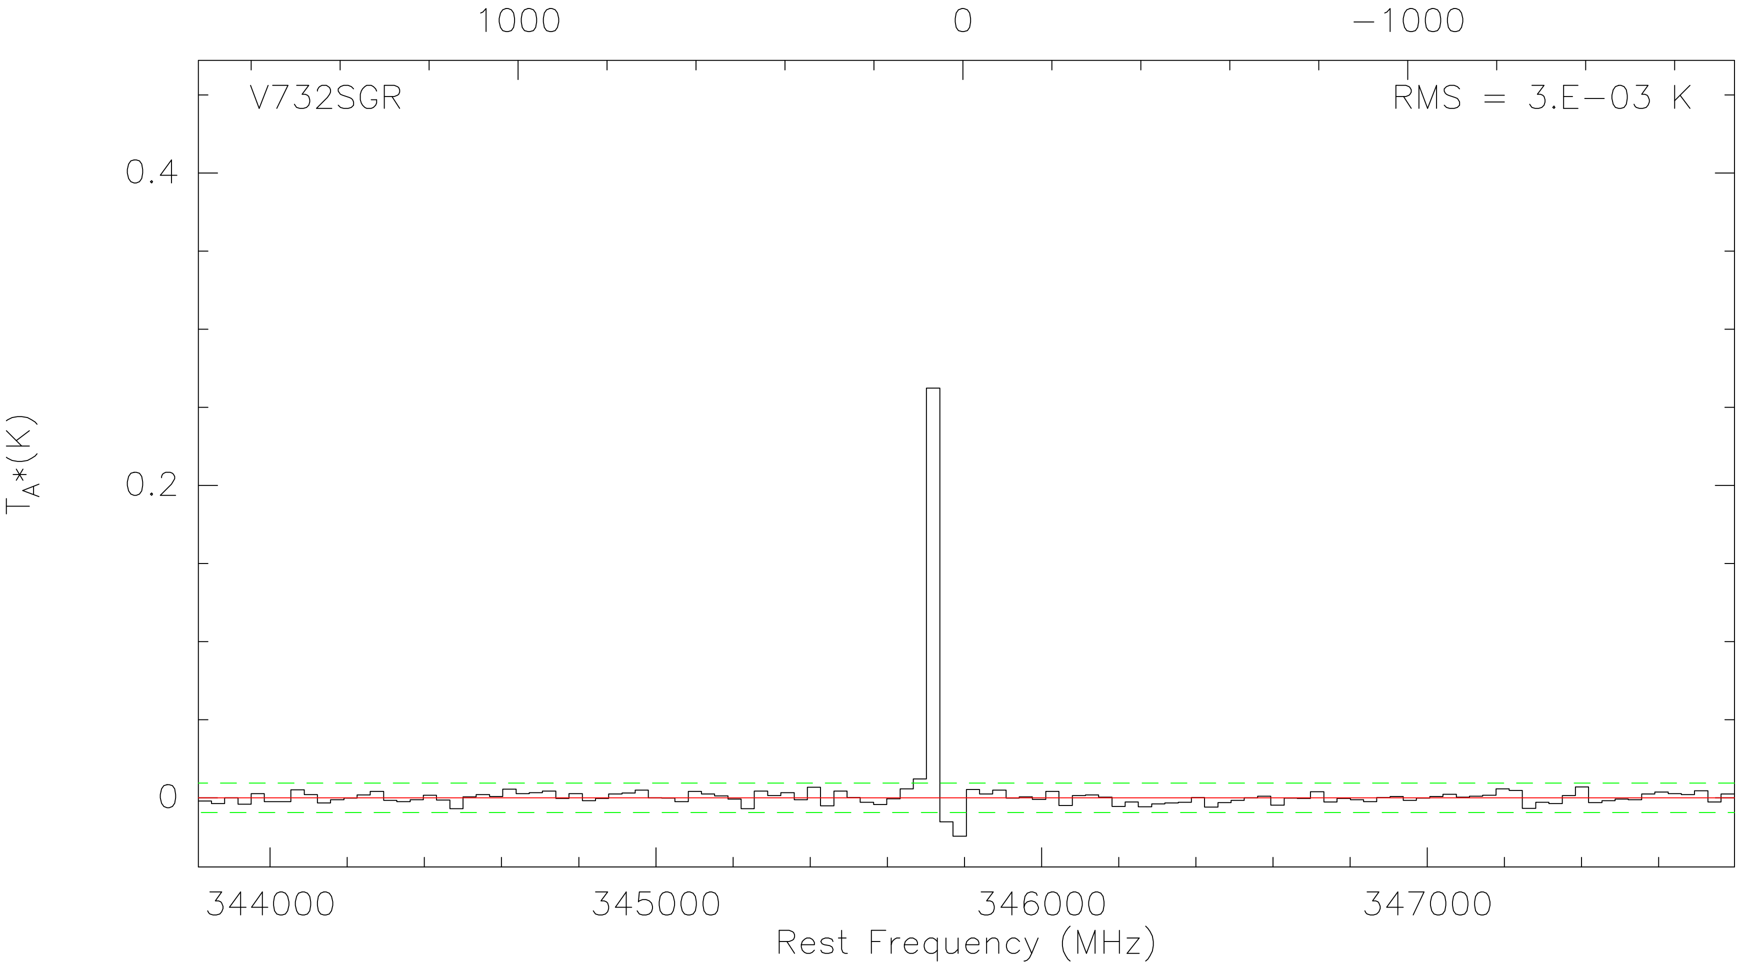

1;1 V733SCO CO(3-2) AP-F302-XF0- 0:06-JUL-2016 R:07-AUG-2020
RA: 17:39:42.88 DEC: -35:52:38.4 Eq 2000.0 Rad. 0.0° Offs: +0.3 -0.3
Unknown tau: 0.225 Tsys: 267. Time: 9.9min El: 37.6
N: 116 I0: 58.7552 V0: 0.000 Dv: 29.76 LSR
F0: 345795.990 Df: -34.33 Fi: 333795.948

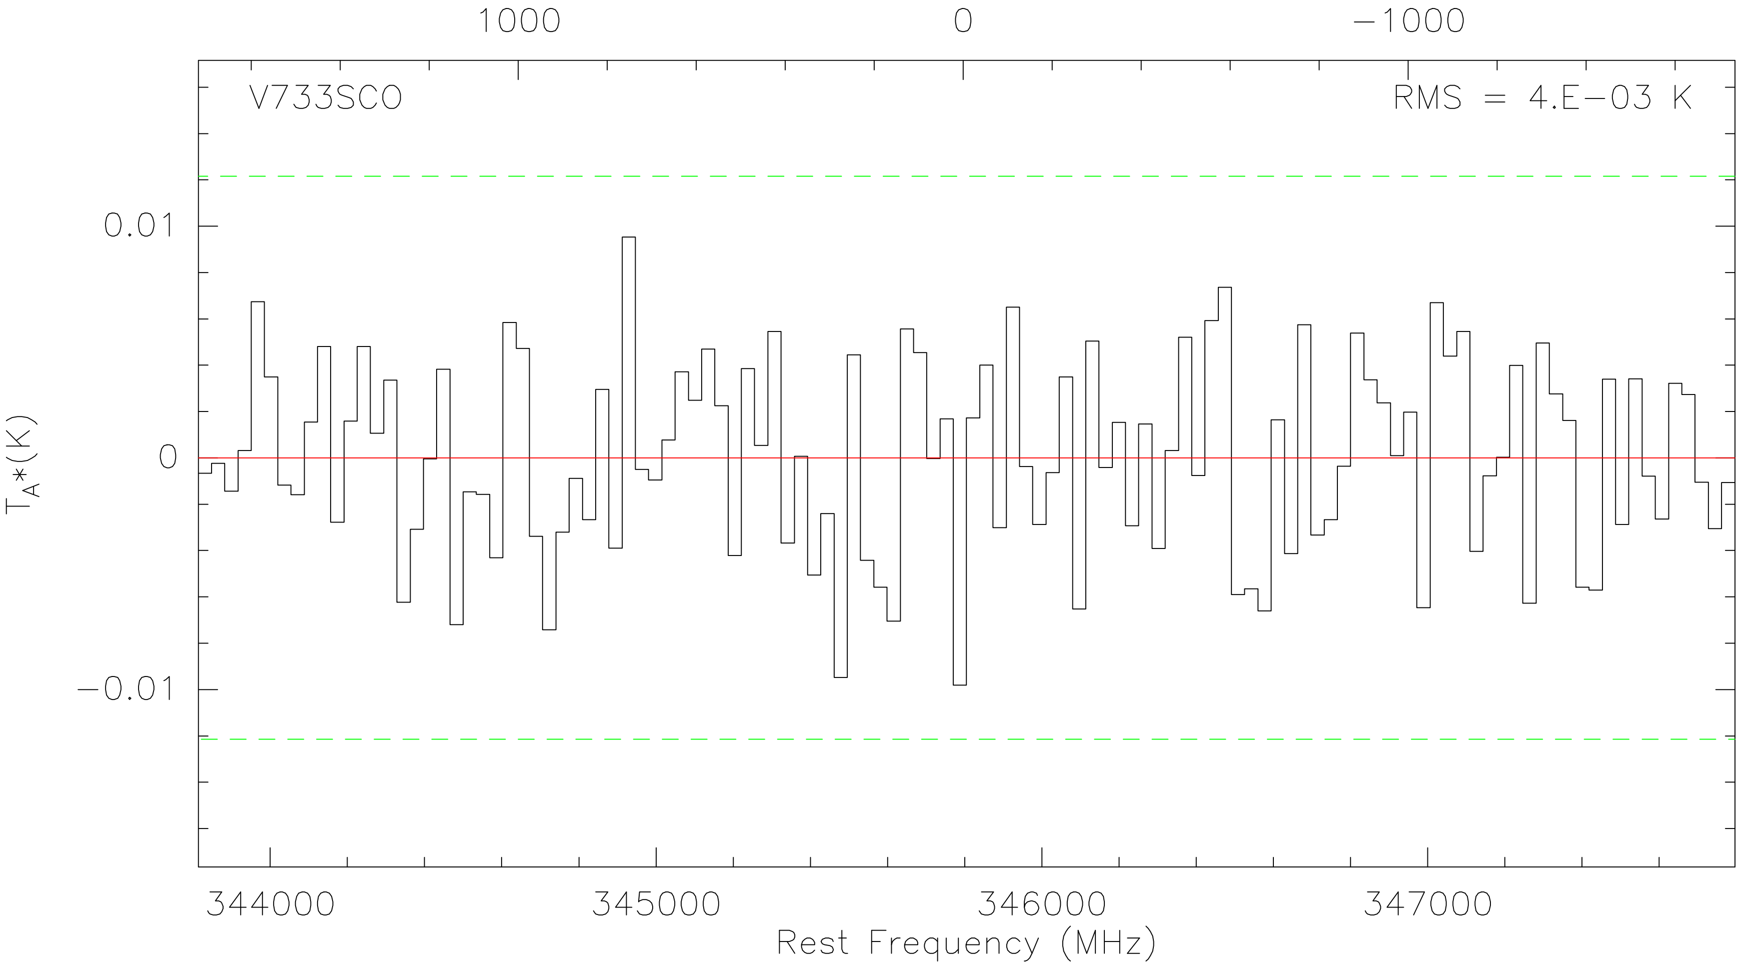

1;1 V737SGR CO(3-2) AP-F302-XF0- O:14-JUL-2016 R:07-AUG-2020
RA: 18:07:08.66 DEC: -28:44:52.3 Eq 2000.0 Rad. 0.0° Offs: +0.2 -0.4
Unknown tau: 0.250 Tsys: 214. Time: 9.9min El: 70.3
N: 116 I0: 58.7552 V0: 0.000 Dv: 29.76 LSR
F0: 345795.990 Df: -34.33 Fi: 333796.004

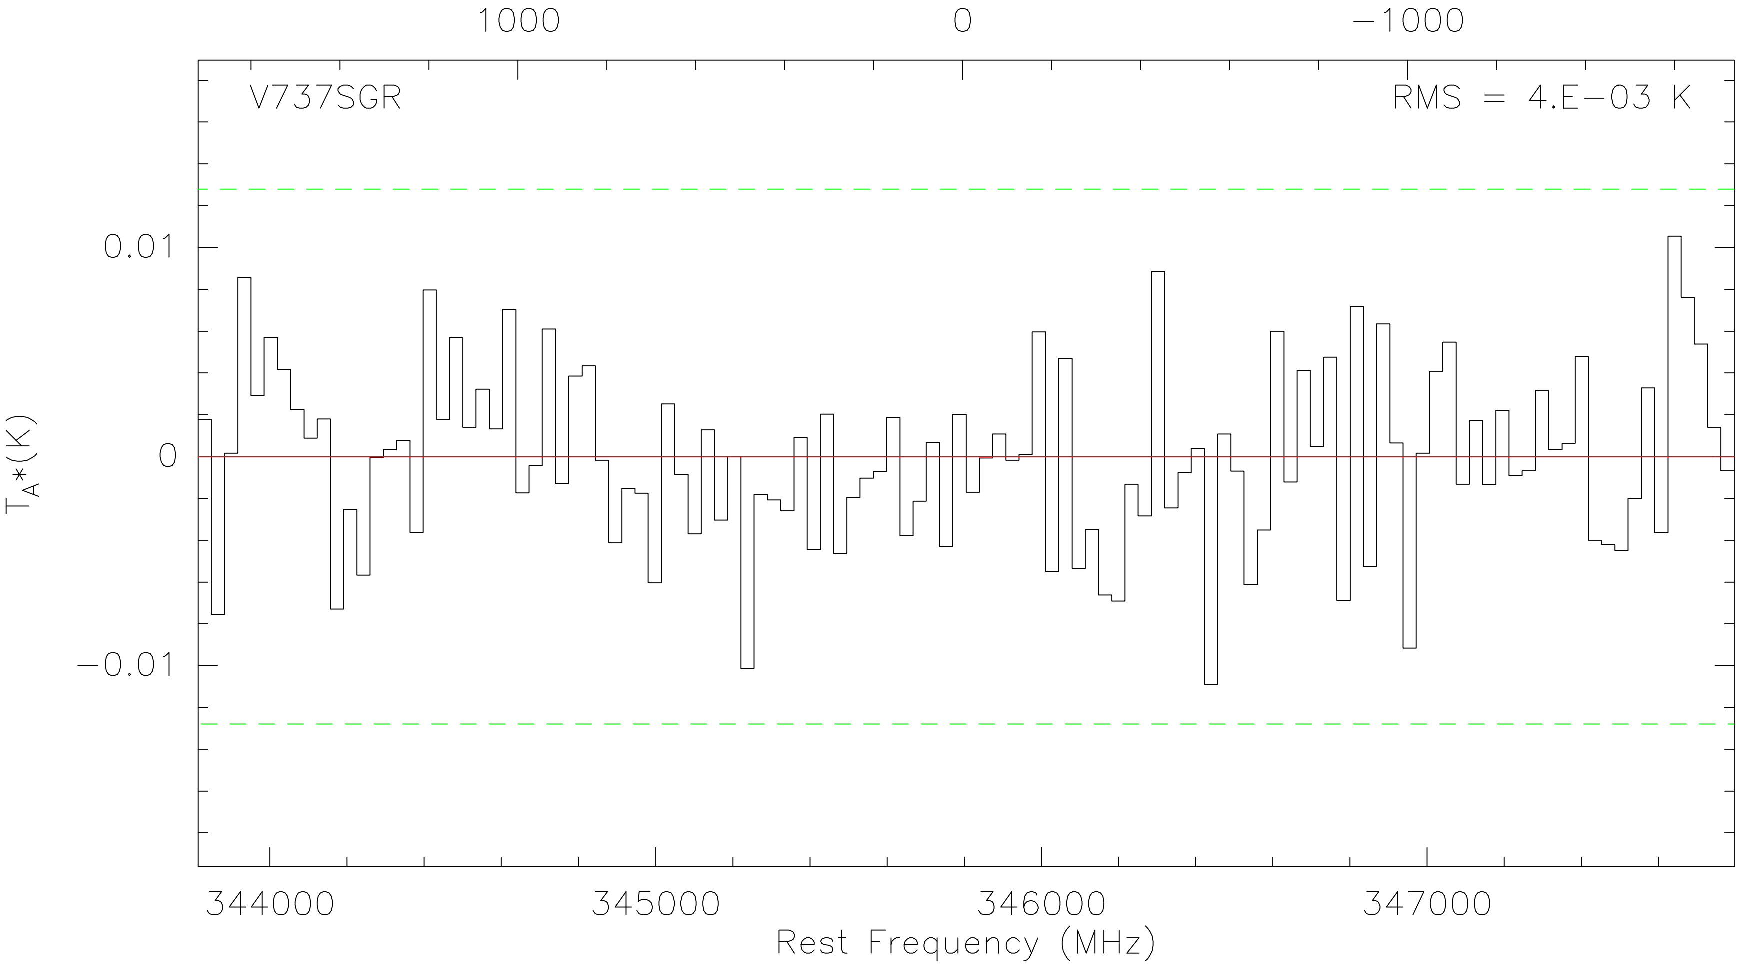

1;1 V745SCO CO(3-2) AP-F302-XF0- O:13-JUL-2016 R:07-AUG-2020
RA: 17:55:22.27 DEC: -33:14:58.5 Eq 2000.0 Rad. 0.0° Offs: +0.0 -0.7
Unknown tau: 0.202 Tsys: 183. Time: 9.9min El: 77.6
N: 116 I0: 58.7552 V0: 0.000 Dv: 29.77 LSR
F0: 345795.990 Df: -34.33 Fi: 333795.914

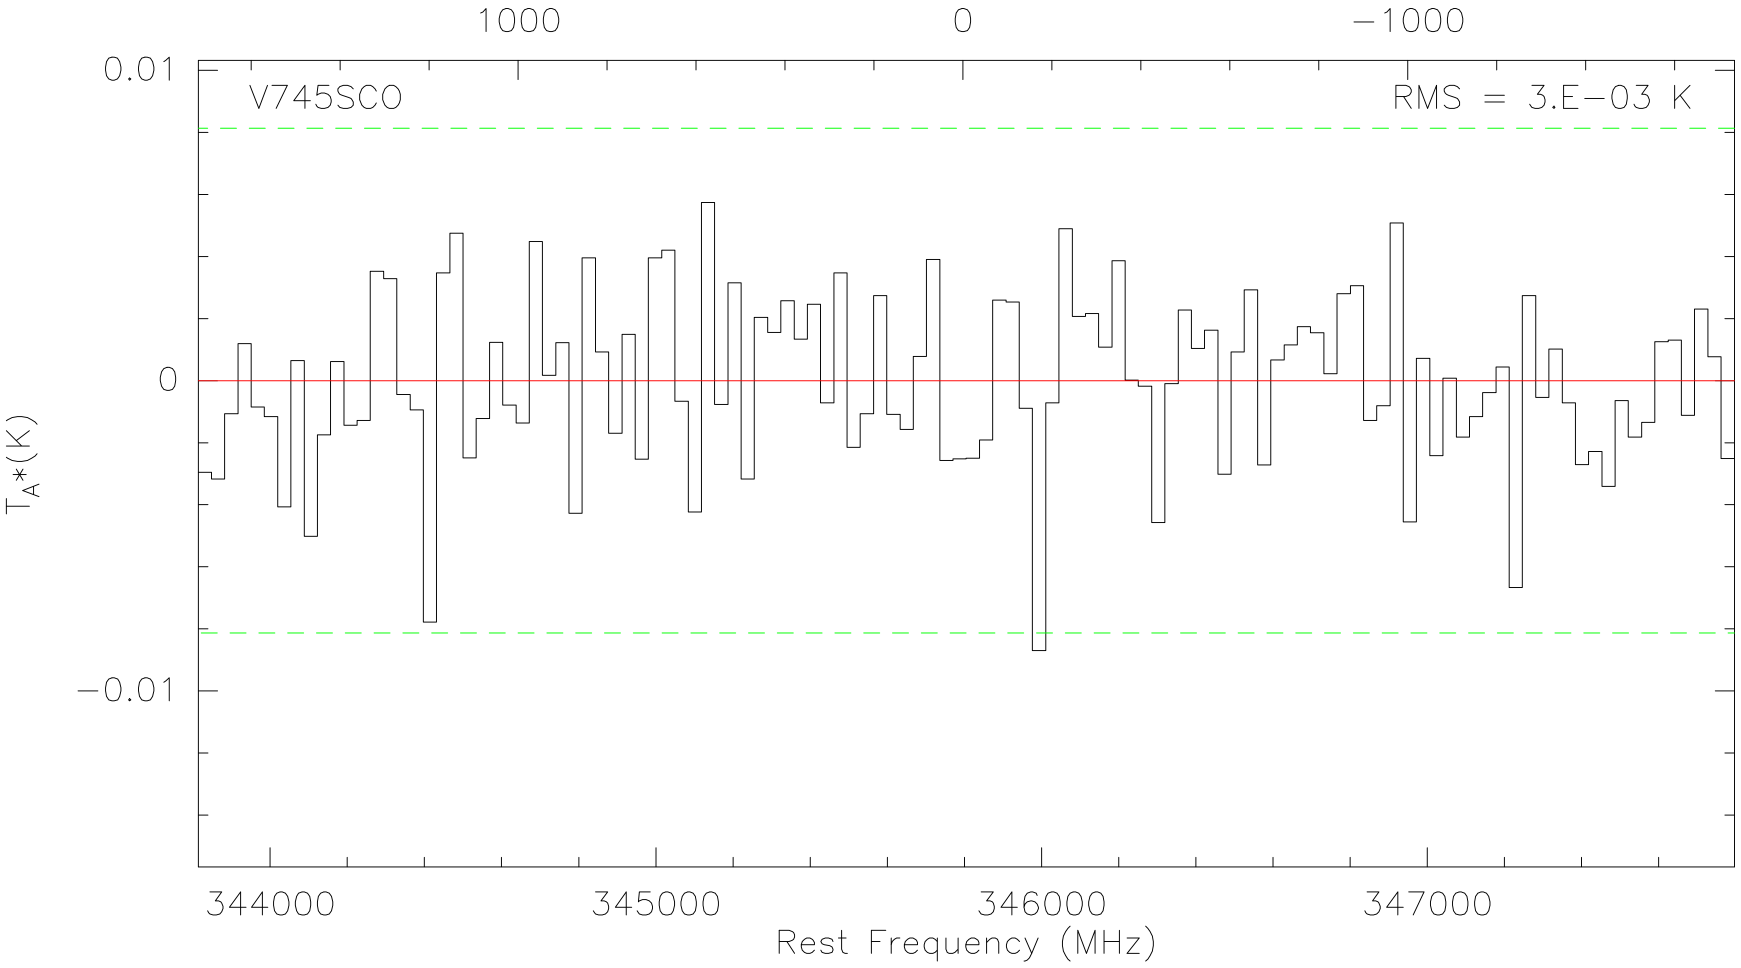

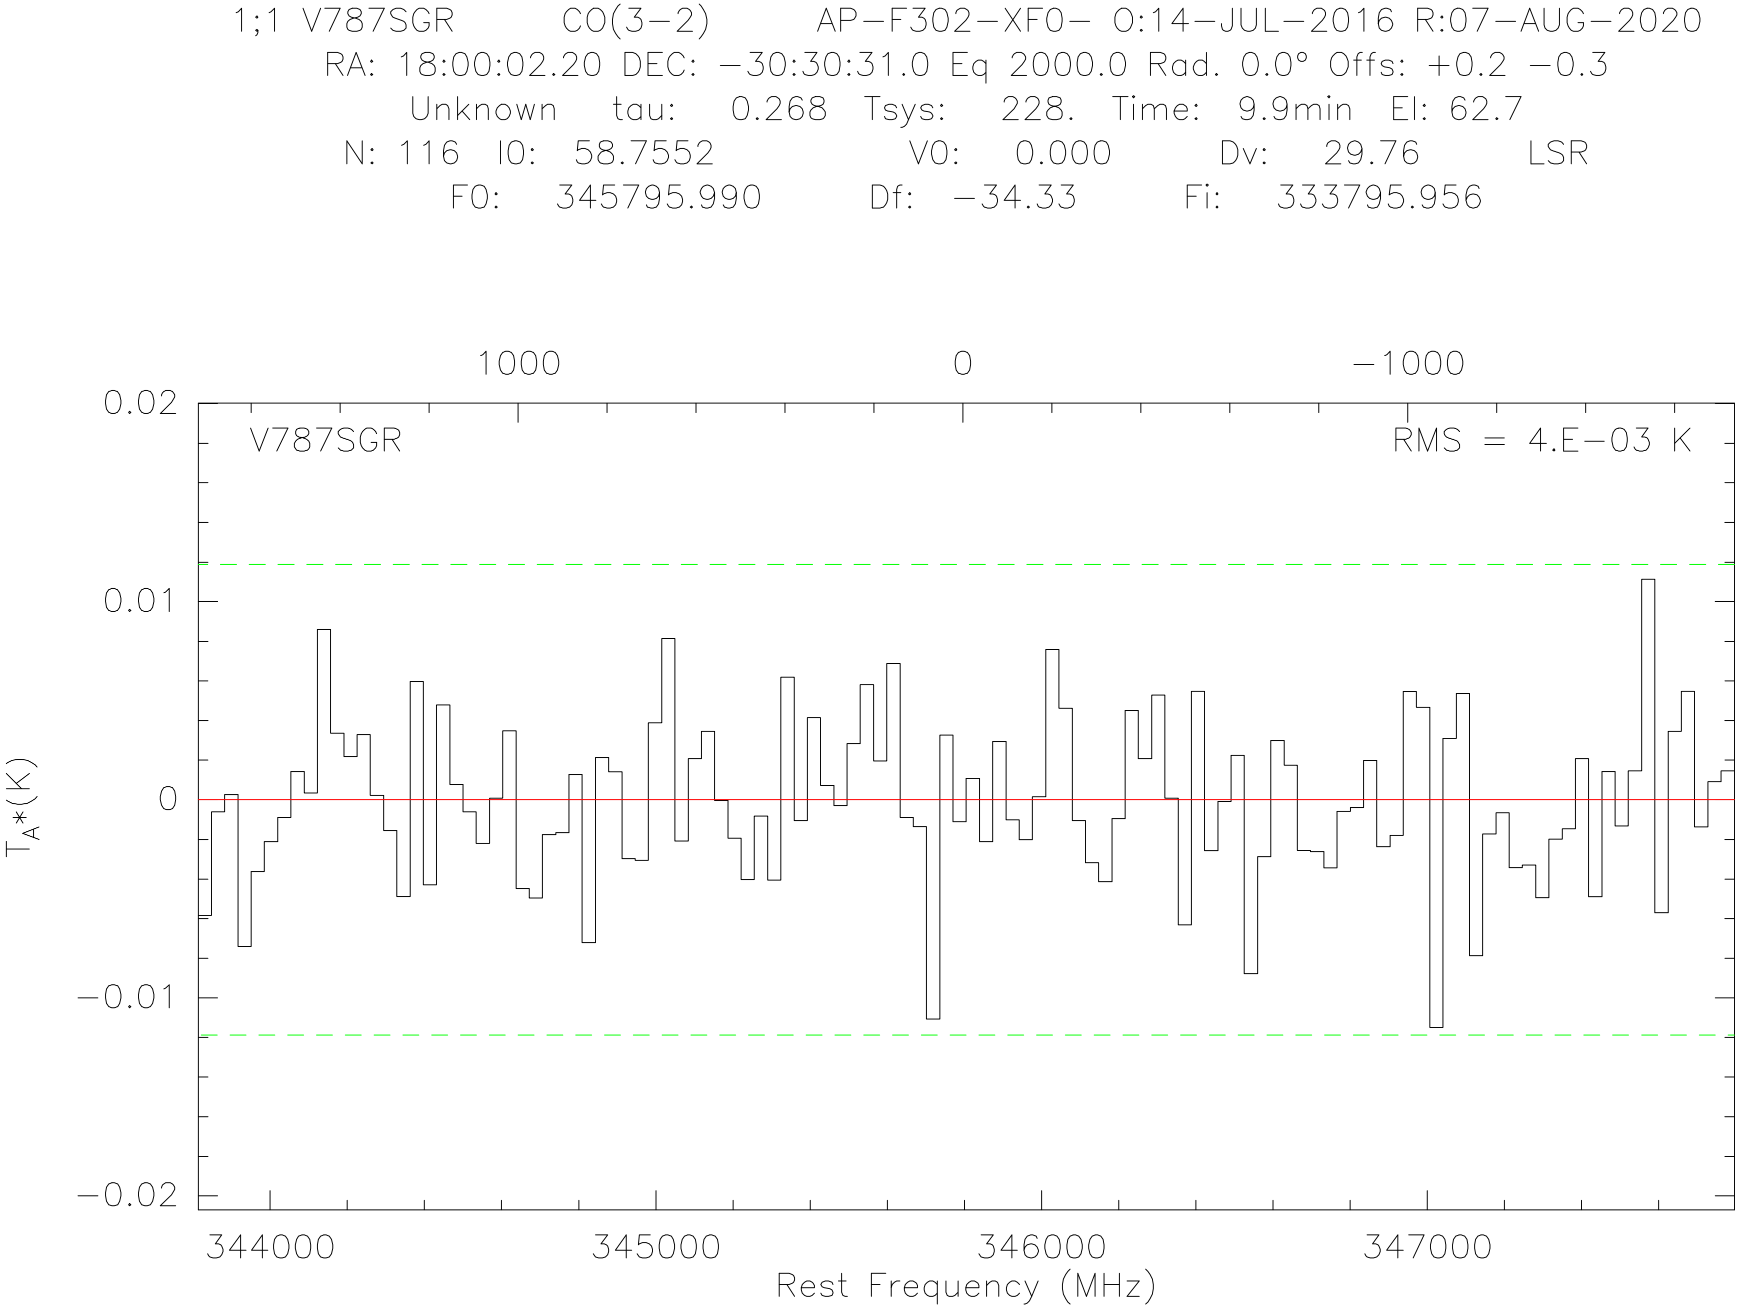
1;1 V787SGR CO(3-2) AP-F302-XF0- O:14-JUL-2016 R:07-AUG-2020
RA: 18:00:02.20 DEC: -30:30:31.0 Eq 2000.0 Rad. 0.0° Offs: +0.2 -0.3
Unknown tau: 0.268 Tsys: 228. Time: 9.9min El: 62.7
N: 116 I0: 58.7552 V0: 0.000 Dv: 29.76 LSR
F0: 345795.990 Df: -34.33 Fi: 333795.956
1000
0
-1000
V787SGR
RMS = 4.E-03 K
0.02
0.01
0
-0.01
-0.02
T_A*(K)
344000
345000
346000
347000
Rest Frequency (MHz)

1;1 V794OPH CO(3-2) AP-F302-XF0- O:01-JUL-2016 R:07-AUG-2020
RA: 17:38:49.25 DEC: -22:50:48.9 Eq 2000.0 Rad. 0.0° Offs: -0.2 -0.5
Unknown tau: 0.365 Tsys: 353. Time: 9.9min El: 42.1
N: 116 I0: 58.7552 V0: 0.000 Dv: 29.76 LSR
F0: 345795.990 Df: -34.33 Fi: 333796.165

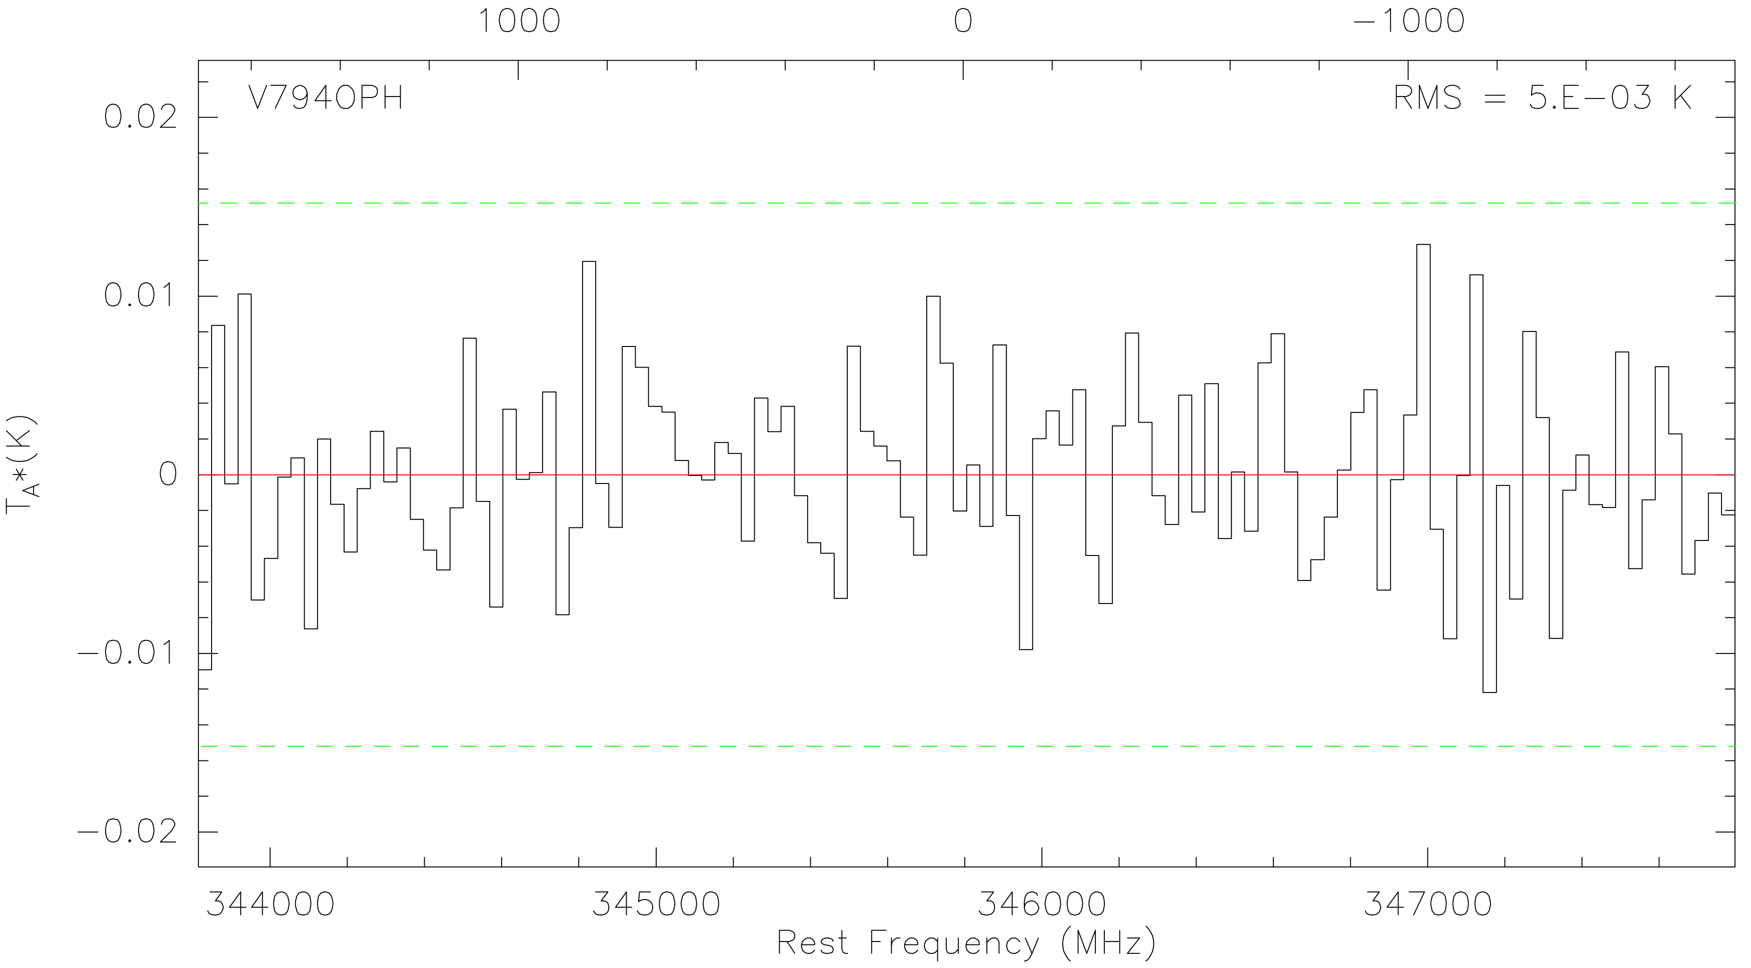

1;1 V909SGR CO(3−2) AP−F302−XF0− O:13−JUL−2016 R:07−AUG−2020
RA: 18:25:52.30 DEC: −35:01:27.0 Eq 2000.0 Rad. 0.0° Offs: +0.2 −0.4
Unknown tau: 0.235 Tsys: 208. Time: 9.9min El: 67.4
N: 116 I0: 58.7552 V0: 0.000 Dv: 29.76 LSR
F0: 345795.990 Df: −34.33 Fi: 333796.021

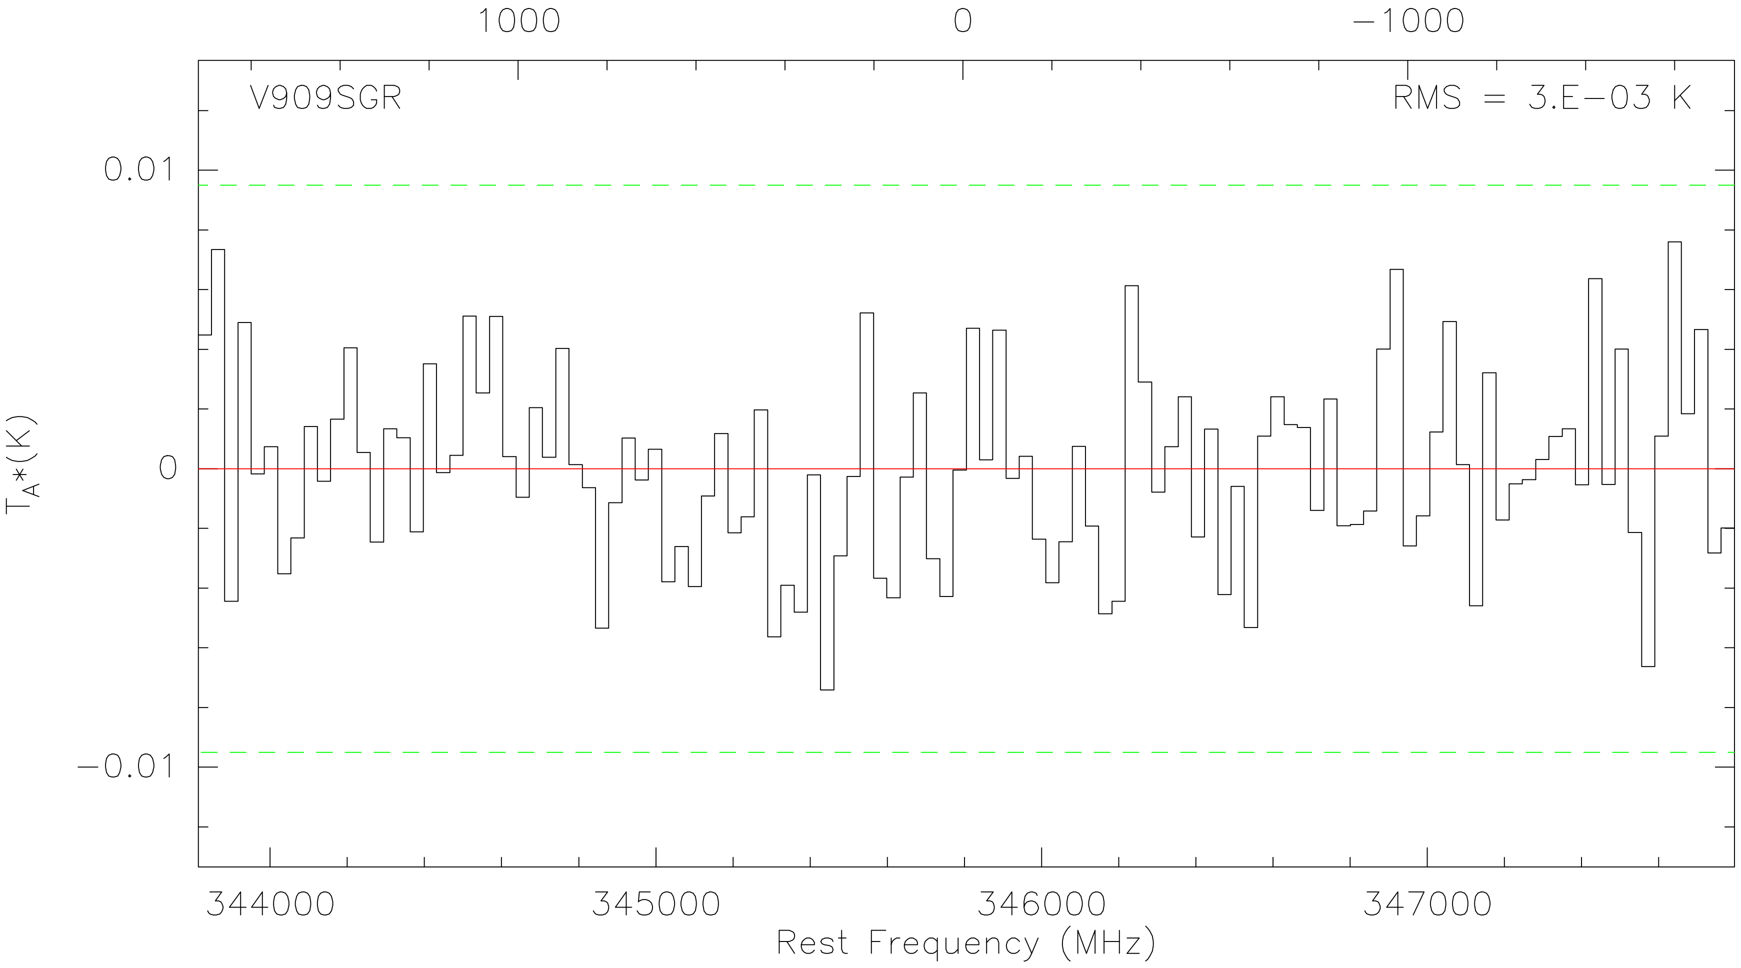

1;1 V941SGR CO(3-2) AP-F302-XF0- O:13-JUL-2016 R:07-AUG-2020
RA: 18:34:43.46 DEC: -29:34:49.1 Eq 2000.0 Rad. 0.0° Offs: -0.2 -0.3
Unknown tau: 0.161 Tsys: 248. Time: 9.9min El: 25.8
N: 116 I0: 58.7552 V0: 0.000 Dv: 29.76 LSR
F0: 345795.990 Df: -34.33 Fi: 333796.099

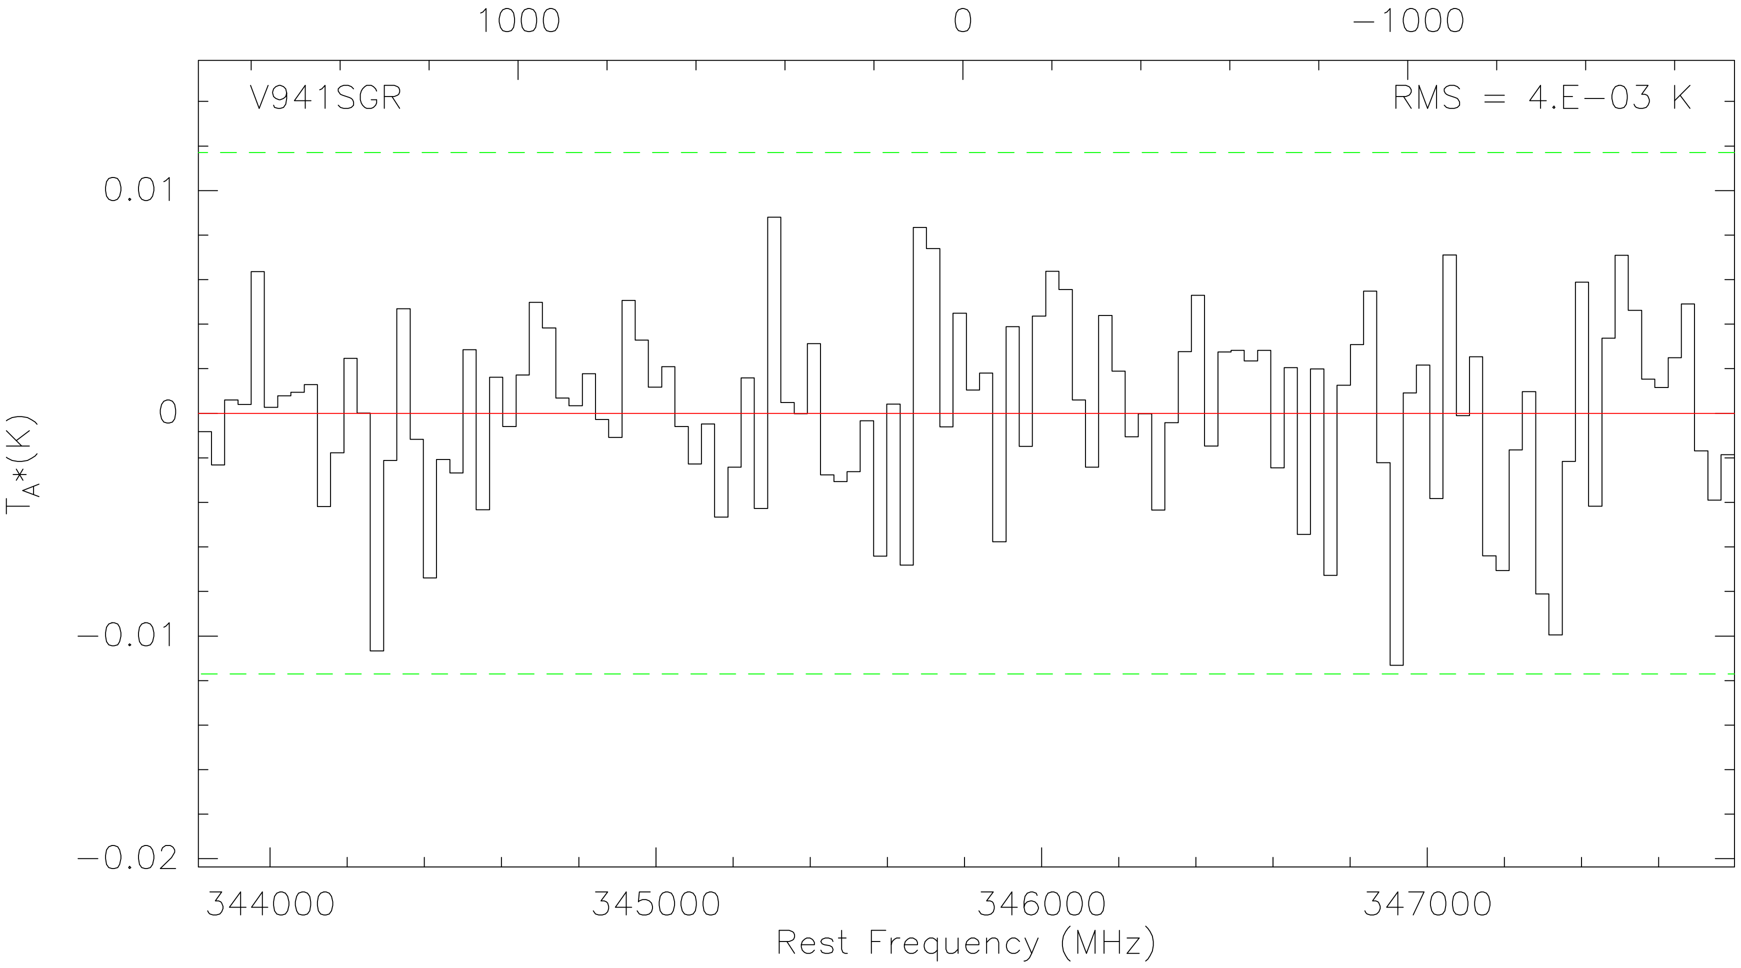

1;1 V999SGR CO(3-2) AP-F302-XF0- O:13-JUL-2016 R:07-AUG-2020
RA: 18:00:05.59 DEC: -27:33:14.0 Eq 2000.0 Rad. 0.0° Offs: -0.2 -0.4
Unknown tau: 0.182 Tsys: 216. Time: 9.9min El: 38.9
N: 116 I0: 58.7552 V0: 0.000 Dv: 29.76 LSR
F0: 345795.990 Df: -34.33 Fi: 333795.984

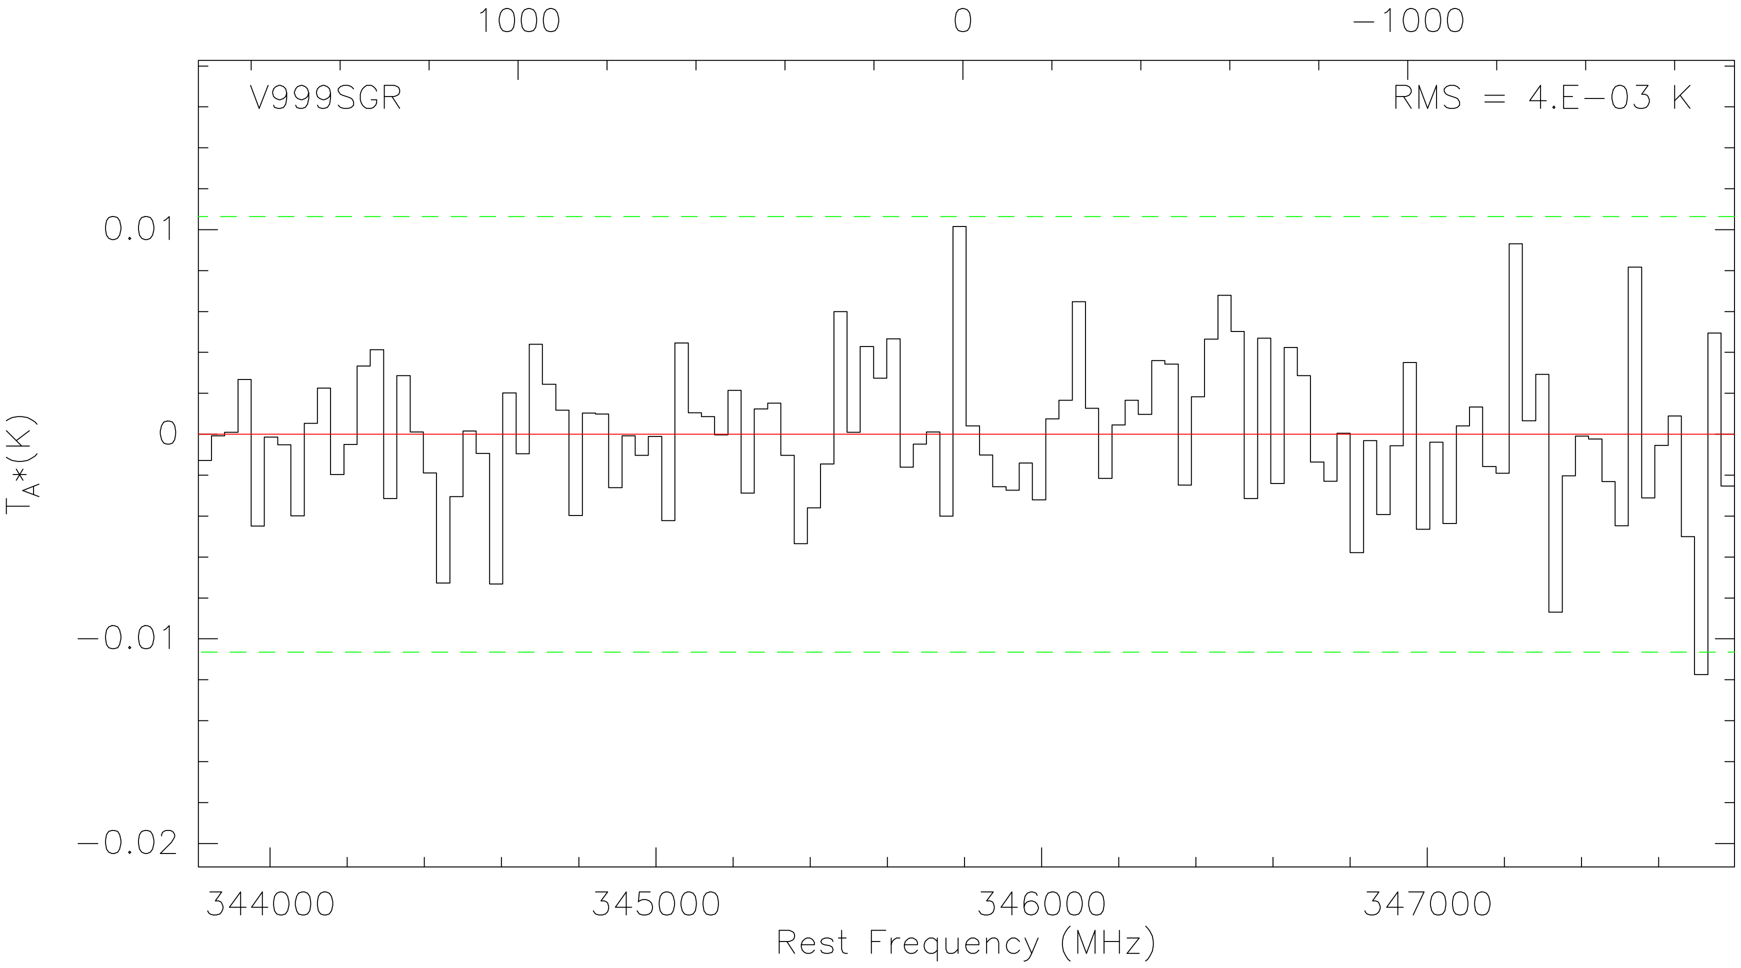

1;1 V1148-SGR CO(3-2) AP-F302-XF0- O:03-JUN-2015 R:13-AUG-2020
RA: 18:09:05.85 DEC: -25:59:08.0 Eq 2000.0 Rad. 0.0° Offs: +0.2 -0.4
Unknown tau: 0.206 Tsys: 209. Time: 44.6min El: 48.5
N: 116 I0: 58.7552 V0: 0.000 Dv: 29.76 LSR
F0: 345795.990 Df: -34.33 Fi: 333797.613

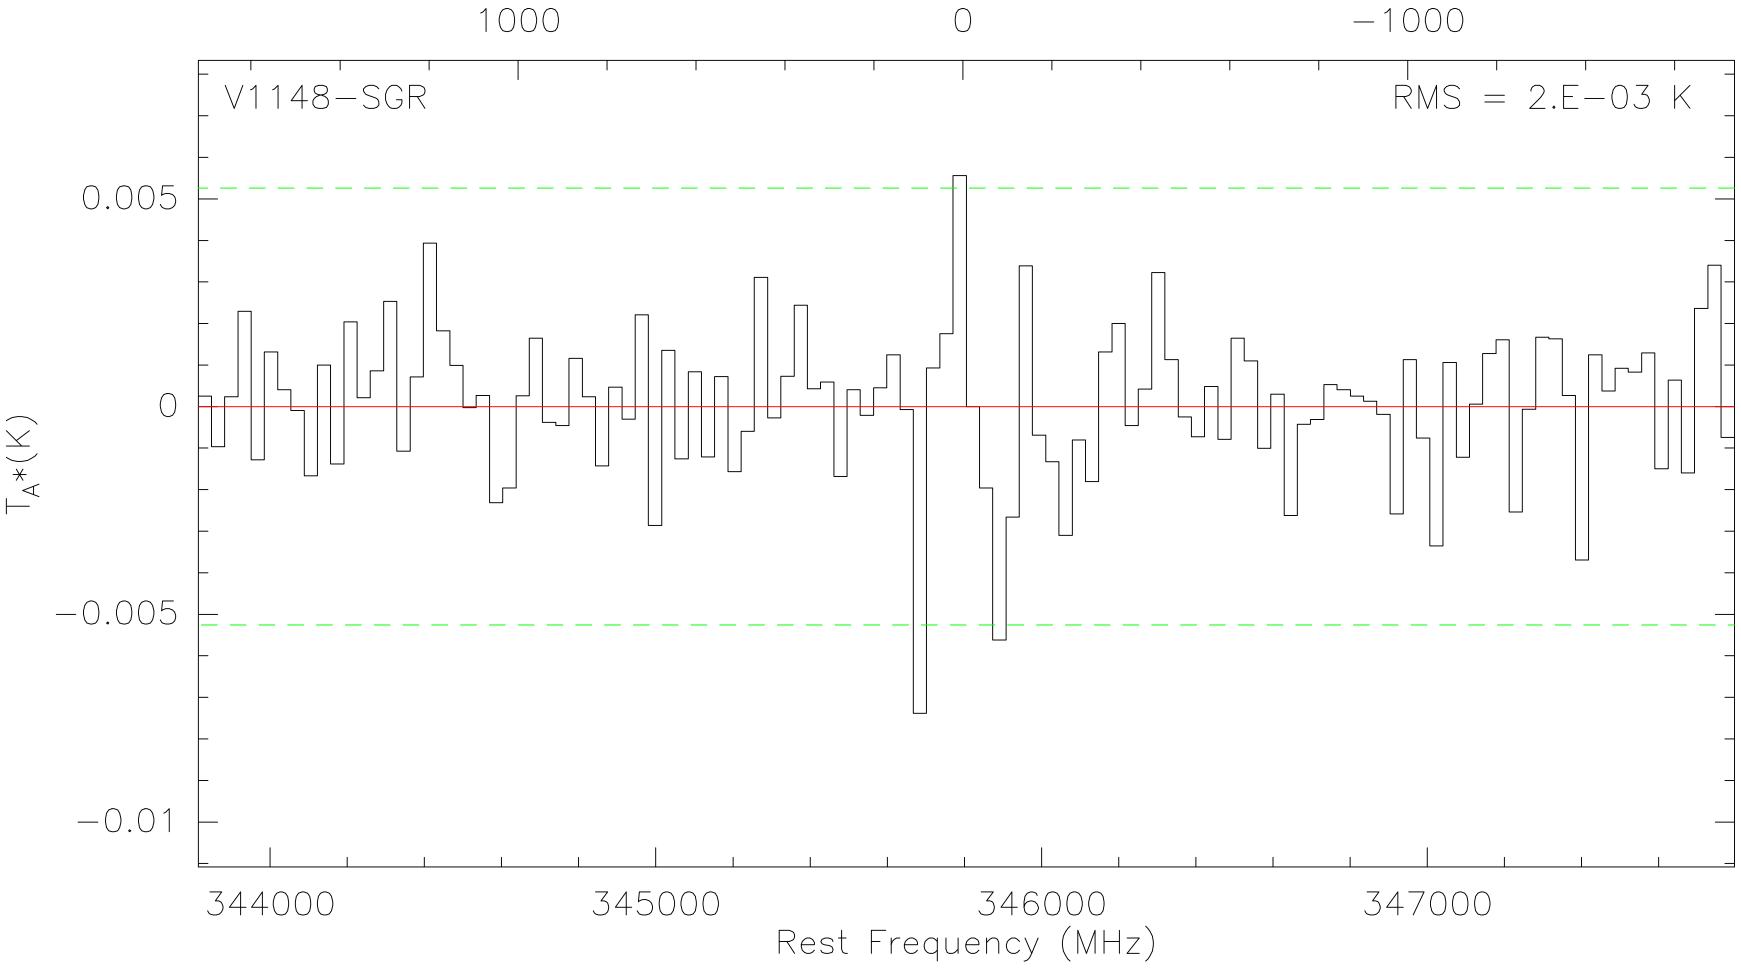

Supplement: Supplementary file 1 [file all_sm_CO32.pdf]
