# Supplementary material for: A search for cool molecular gas in GK Persei and other classical novae
Source: arXiv:2201.10332 source file (2022-01-25)

1;1 CG-CMA CO(3-2) OSB AP-F301-XF0- 0:24-AUG-2014 R:12-AUG-2020  
RA: 07:04:05.05 DEC: -23:45:34.6 Eq 2000.0 Rad. 0.0° Offs: +0.0 -0.2  
Unknown tau: 0.127 Tsys: 184. Time: 23.3min El: 47.3  
N: 116 IO: 58.7548 V0: 0.000 Dv: 30.84 LSR  
FO: 333795.769 Df: -34.33 Fi: 345796.000

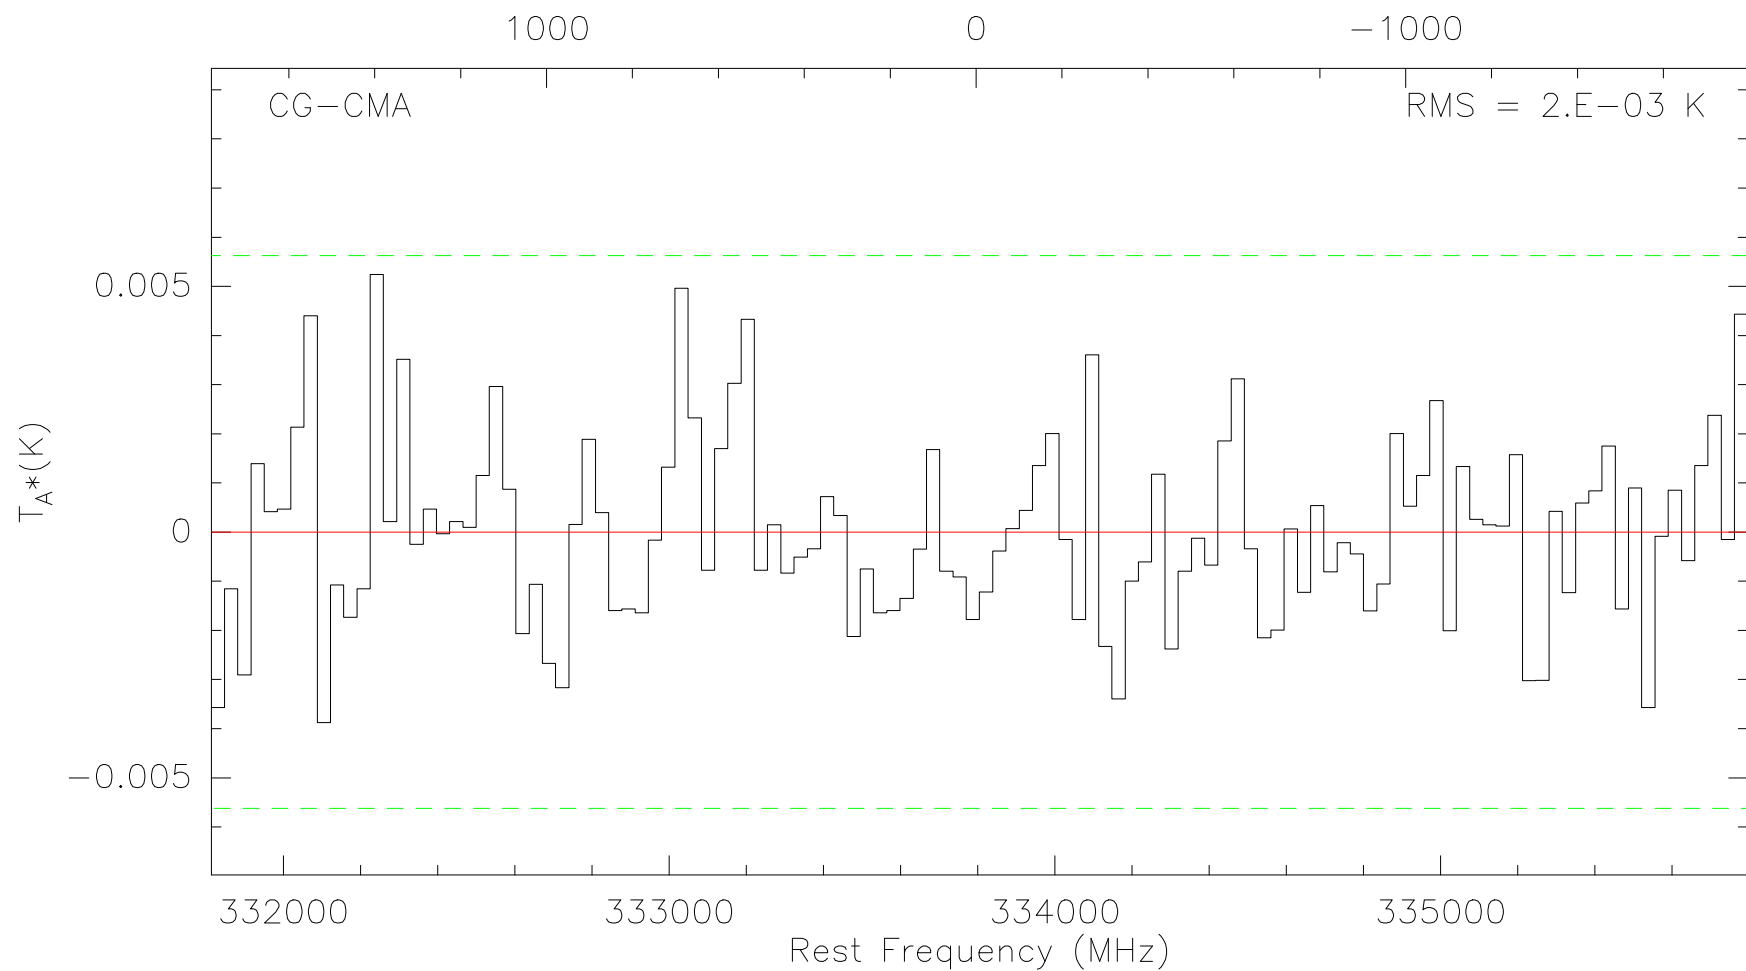

1;1 CN-VEL CO(3-2) OSB AP-F301-XF0- O:24-AUG-2014 R:12-AUG-2020  
RA: 11:02:38.57 DEC: -54:23:09.5 Eq 2000.0 Rad. 0.0° Offs: -0.1 -0.5  
Unknown tau: 0.181 Tsys: 208. Time: 23.4min El: 50.6  
N: 116 IO: 58.7548 V0: 0.000 Dv: 30.84 LSR  
FO: 333795.043 Df: -34.33 Fi: 345795.990

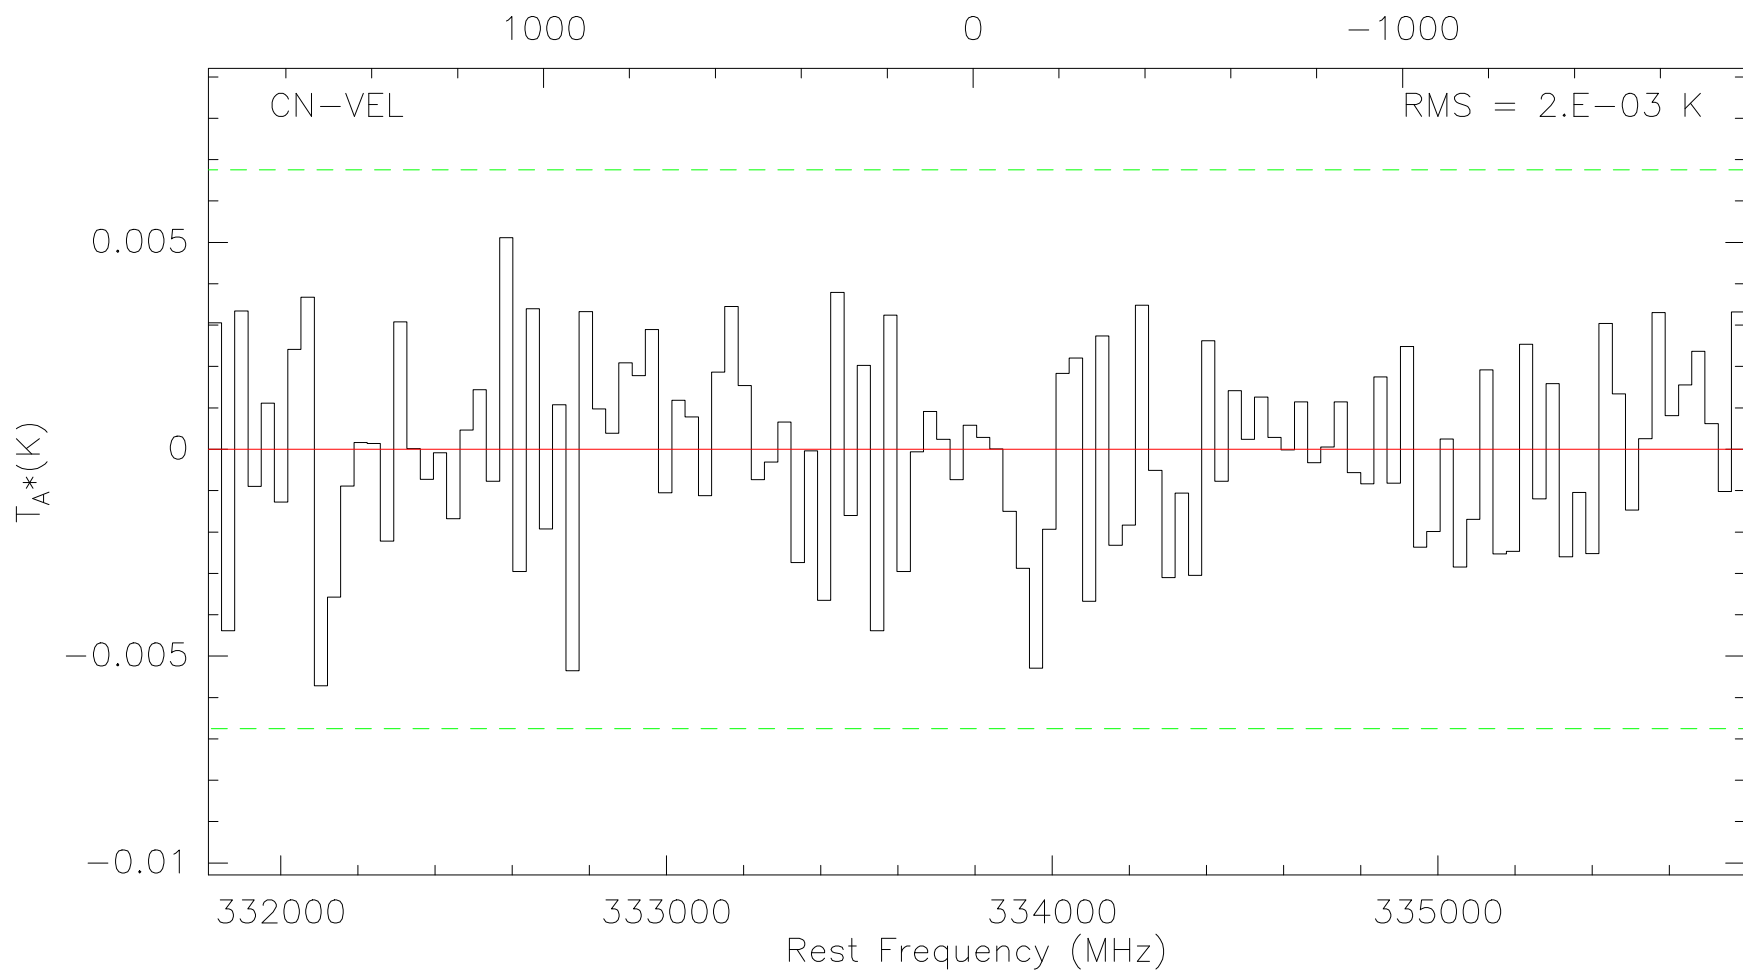

1;1 CQ-VEL CO(3-2) OSB AP-F301-XF0- 0:26-AUG-2014 R:12-AUG-2020  
RA: 08:58:50.99 DEC: -53:20:17.8 Eq 2000.0 Rad. 0.0° Offs: +0.1 -0.5  
Unknown tau: 0.119 Tsys: 180. Time: 23.4min El: 58.6  
N: 116 IO: 58.7548 V0: 0.000 Dv: 30.84 LSR  
FO: 333795.226 Df: -34.33 Fi: 345795.990

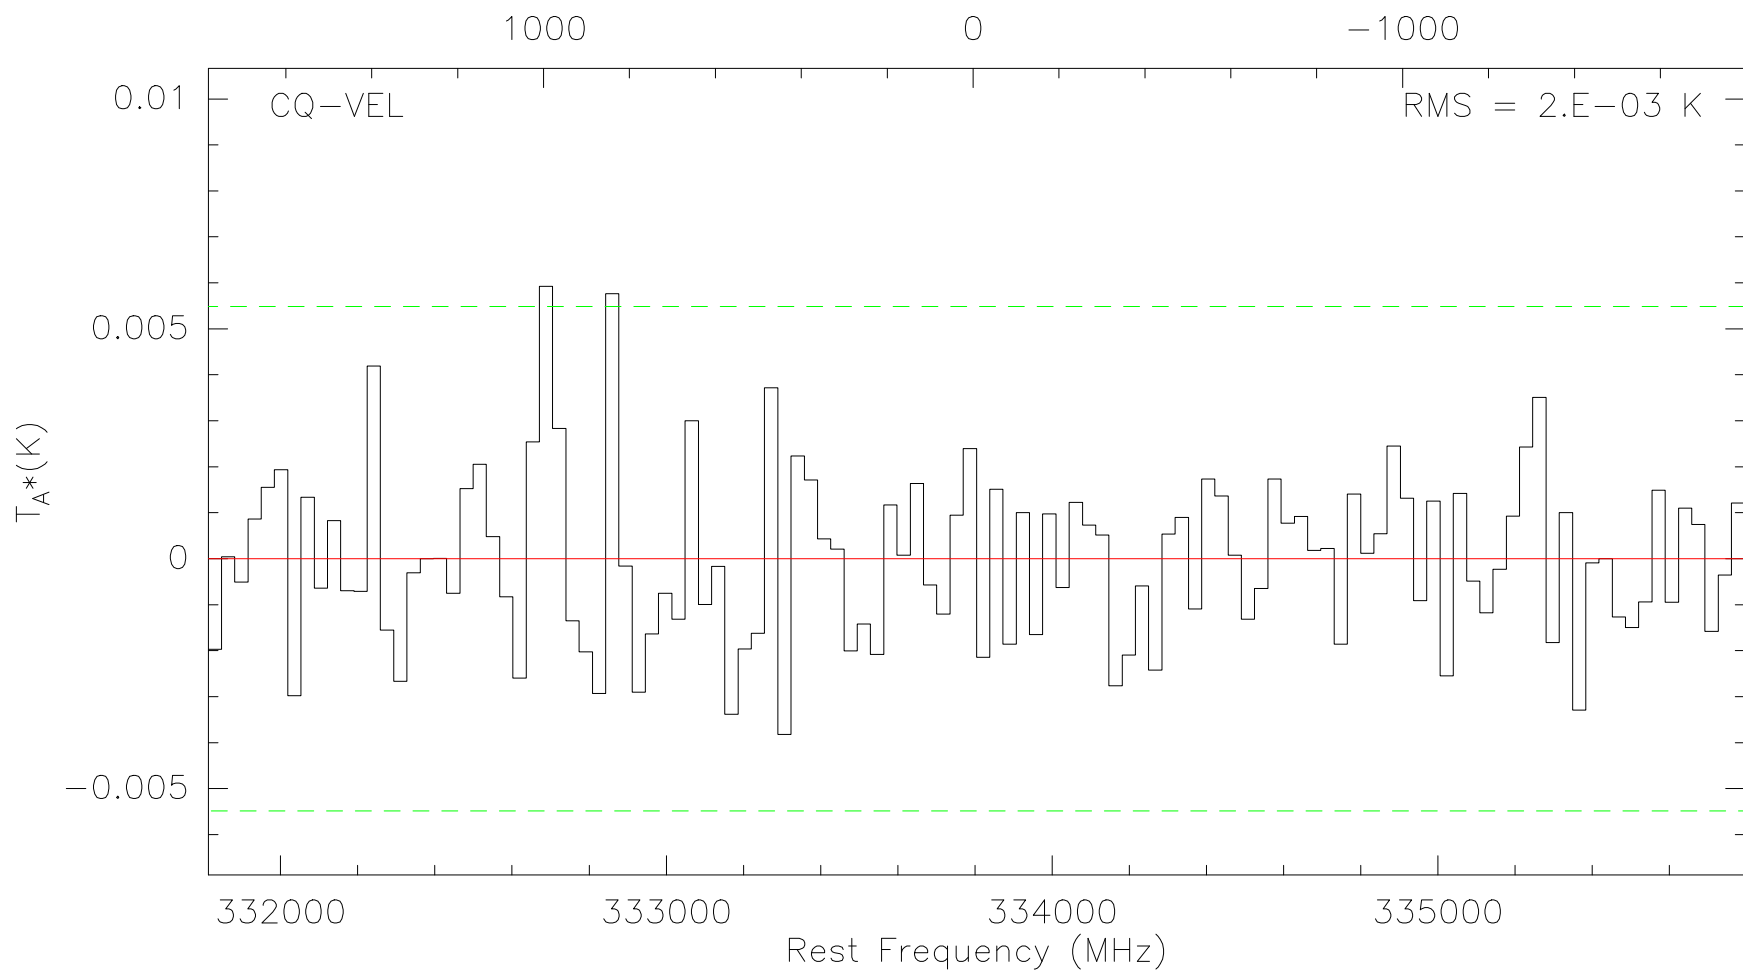

1;1 DY-PUP CO(3-2) OSB AP-F301-XF0- O:25-AUG-2014 R:12-AUG-2020  
RA: 08:13:48.51 DEC: -26:33:56.5 Eq 2000.0 Rad. 0.0° Offs: +0.2 -0.2  
Unknown tau: 0.109 Tsys: 163. Time: 23.5min El: 65.1  
N: 116 IO: 58.7548 V0: 0.000 Dv: 30.84 LSR  
FO: 333795.562 Df: -34.33 Fi: 345795.990

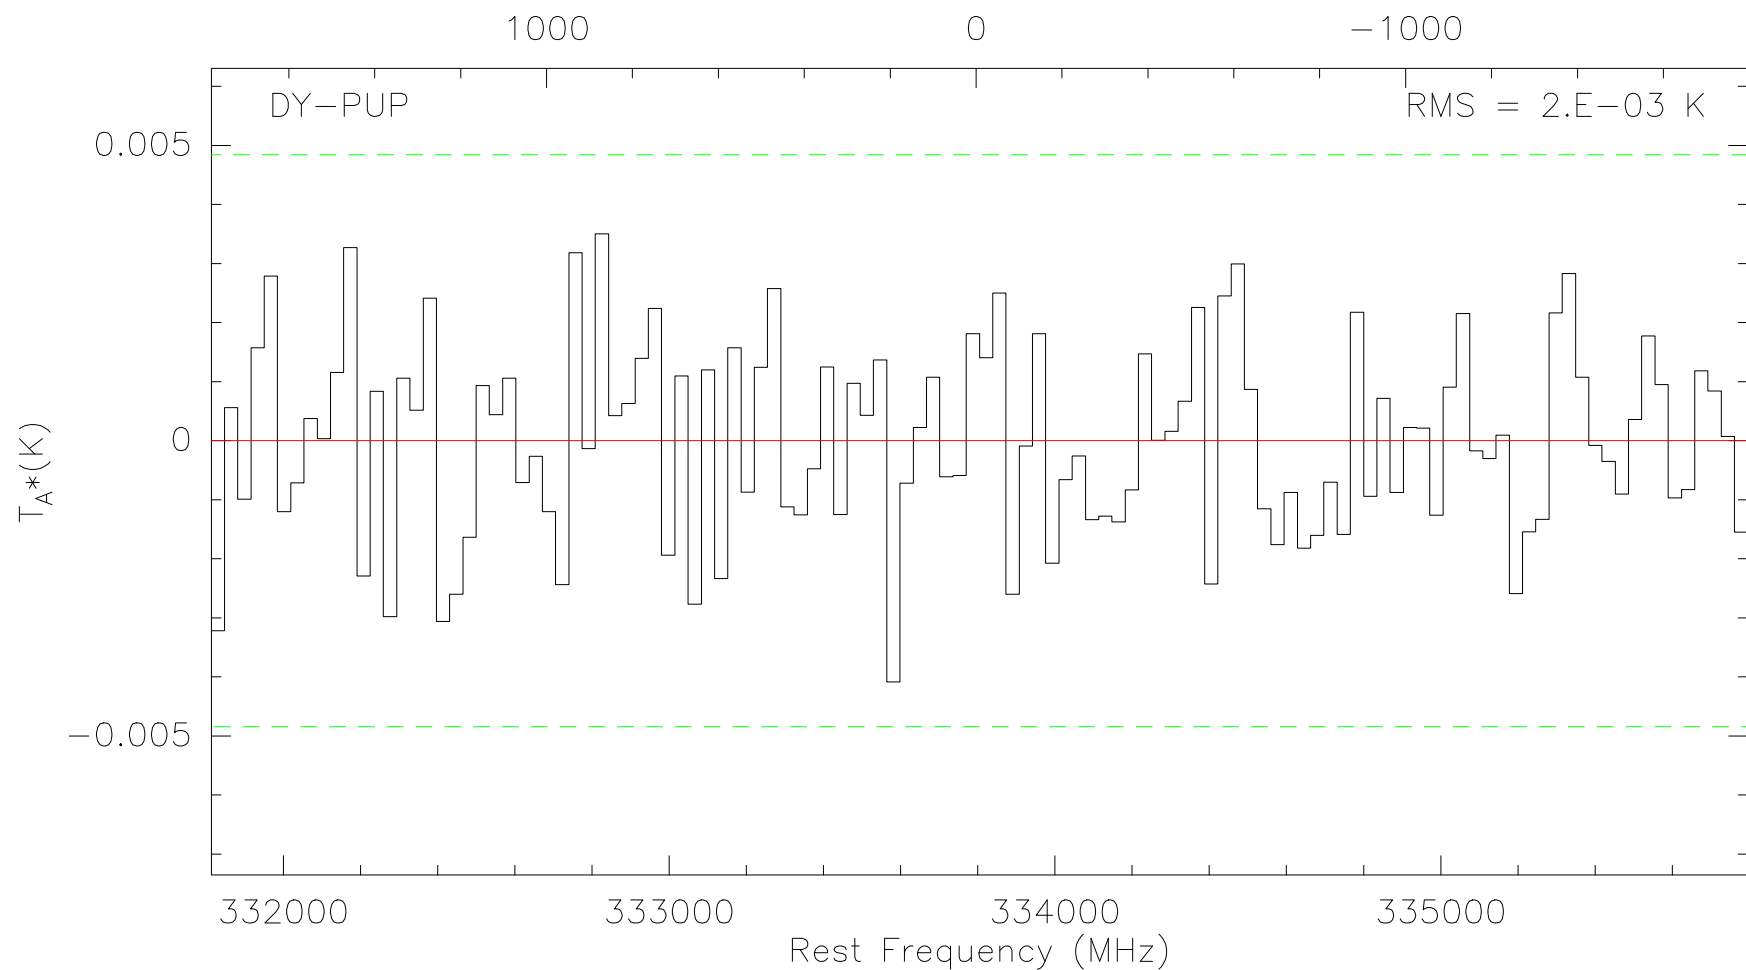

1;1 GQ-MUS CO(3-2) OSB AP-F301-XF0- 0:28-AUG-2014 R:12-AUG-2020  
RA: 11:52:02.35 DEC: -67:12:20.2 Eq 2000.0 Rad. 0.0° Offs: +0.1 -0.4  
Unknown tau: 0.205 Tsys: 246. Time: 20.4min El: 45.6  
N: 116 IO: 58.7548 V0: 0.000 Dv: 30.84 LSR  
FO: 333795.049 Df: -34.33 Fi: 345796.000

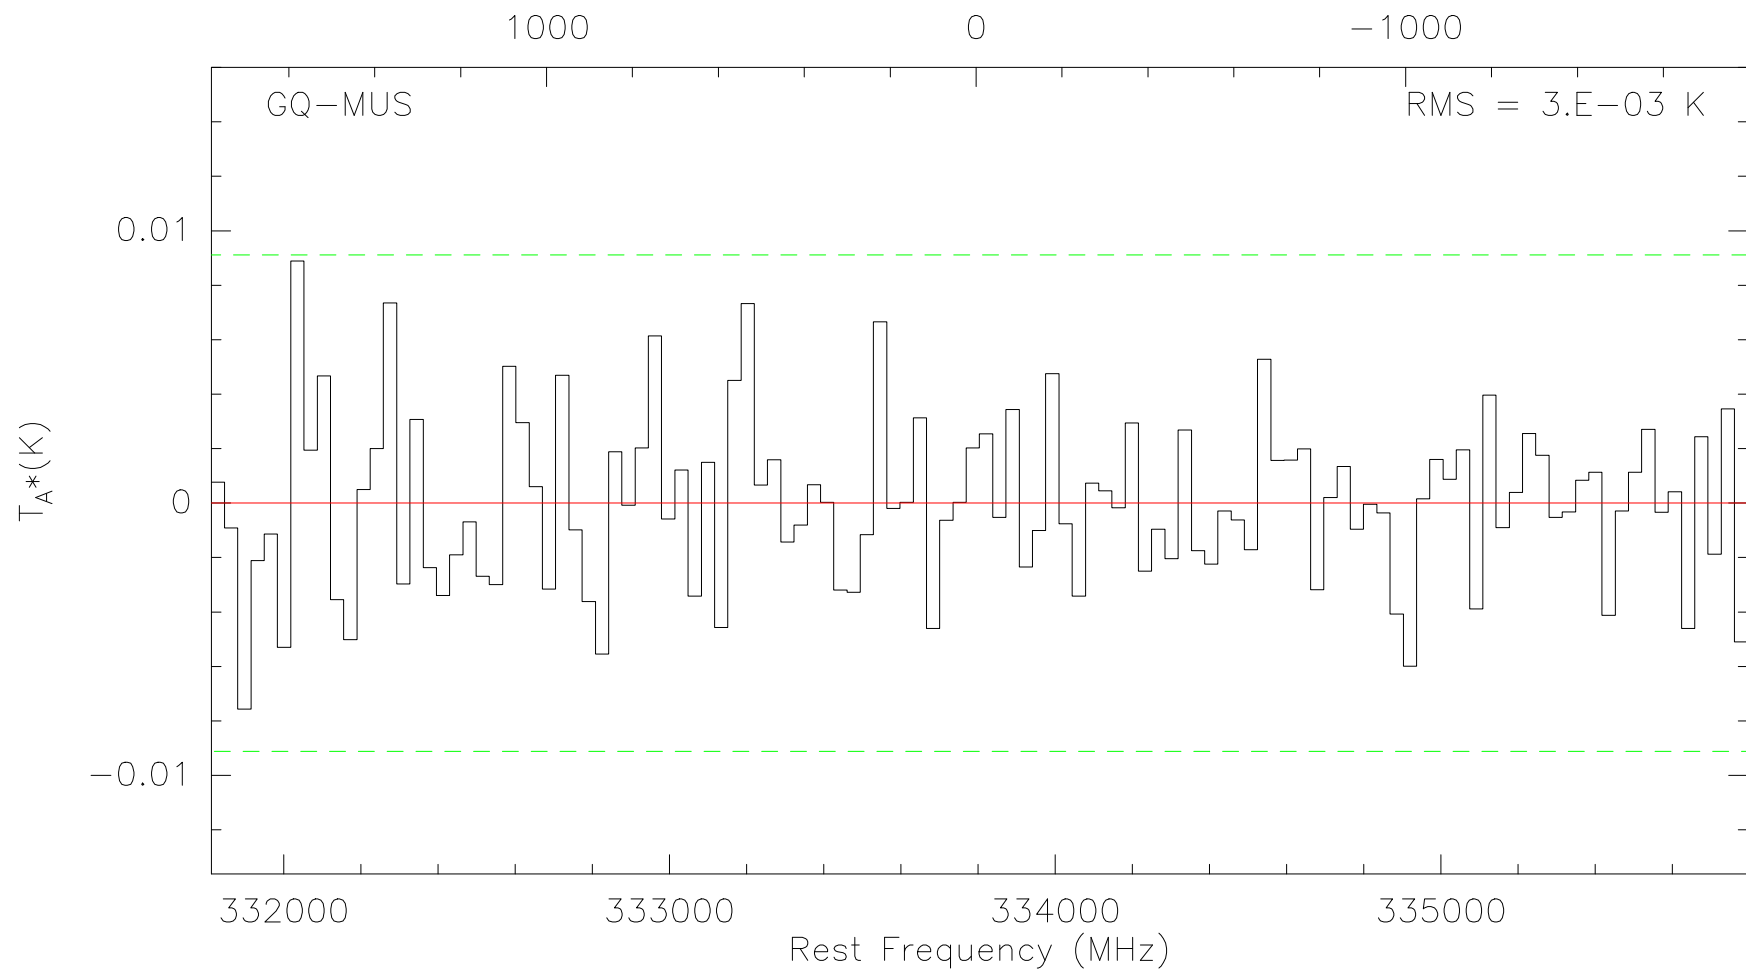

1;1 GU-MUS CO(3-2) OSB AP-F301-XF0- O:24-AUG-2014 R:12-AUG-2020  
RA: 11:26:26.60 DEC: -68:40:32.3 Eq 2000.0 Rad. 0.0° Offs: -0.2 -0.4  
Unknown tau: 0.166 Tsys: 245. Time: 23.3min El: 37.6  
N: 116 IO: 58.7548 V0: 0.000 Dv: 30.84 LSR  
FO: 333795.038 Df: -34.34 Fi: 345795.990

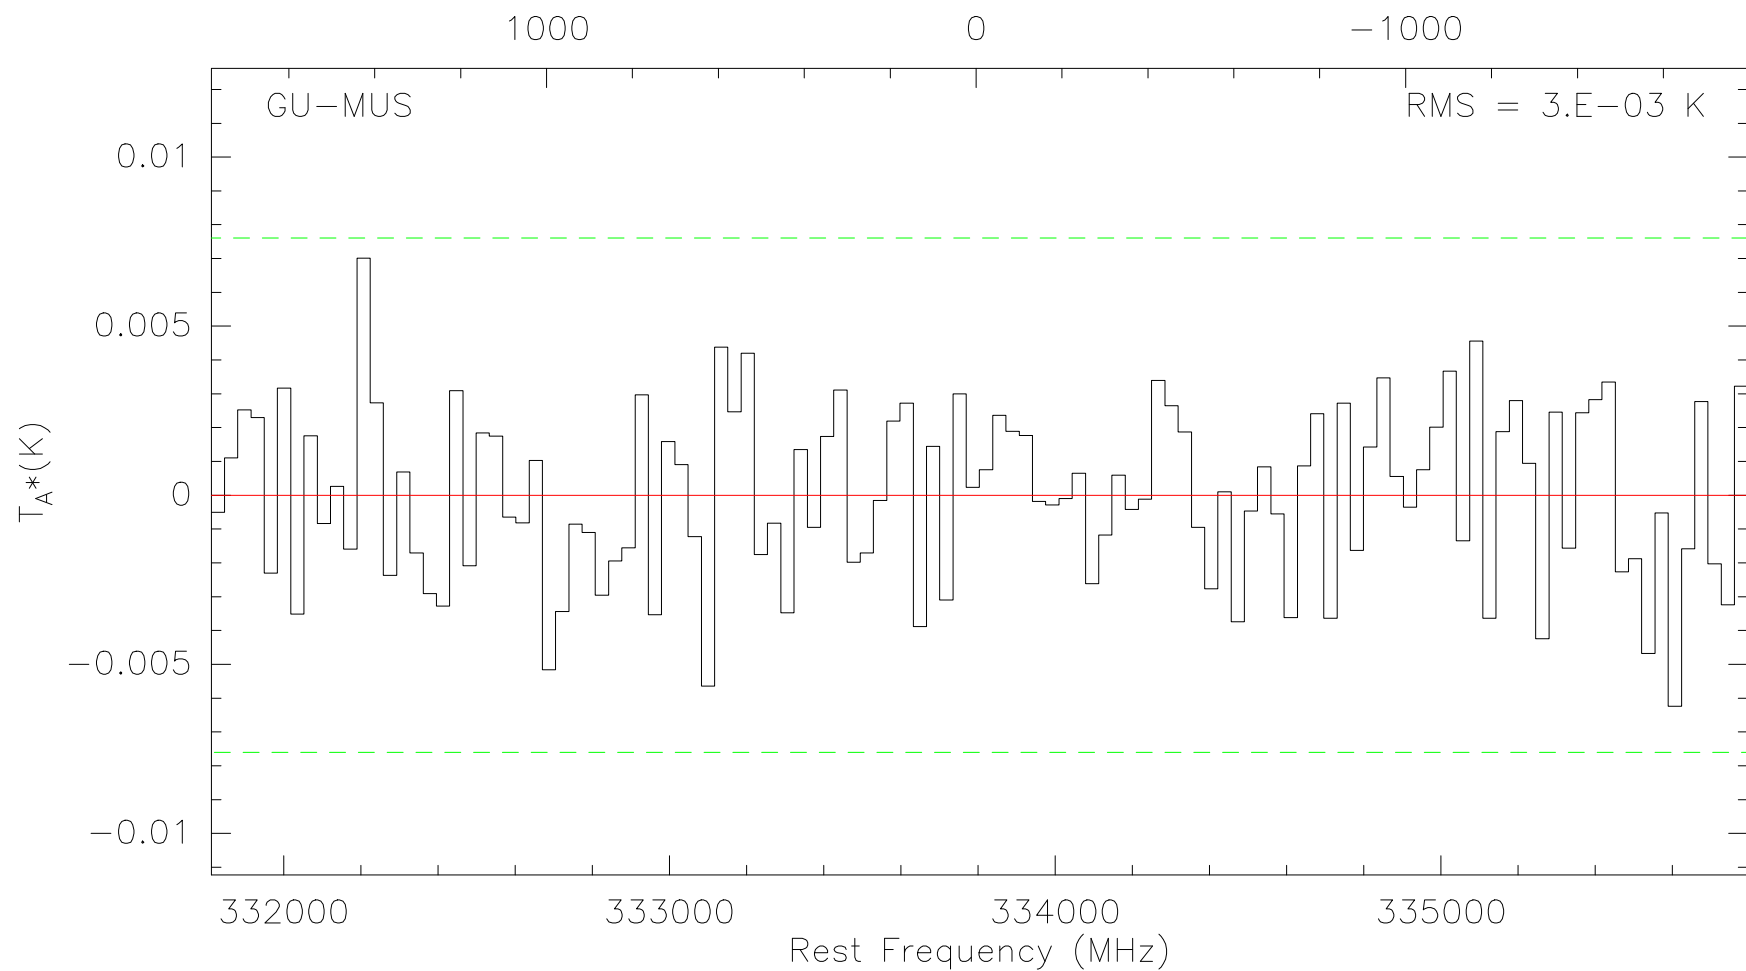

1;1 LZ-MUS CO(3-2) OSB AP-F301-XF0- O:24-AUG-2014 R:12-AUG-2020  
RA: 11:56:09.27 DEC: -65:34:20.1 Eq 2000.0 Rad. 0.0° Offs: -0.2 -0.4  
Unknown tau: 0.212 Tsys: 274. Time: 23.4min El: 36.6  
N: 116 IO: 58.7548 V0: 0.000 Dv: 30.84 LSR  
FO: 333795.012 Df: -34.34 Fi: 345795.990

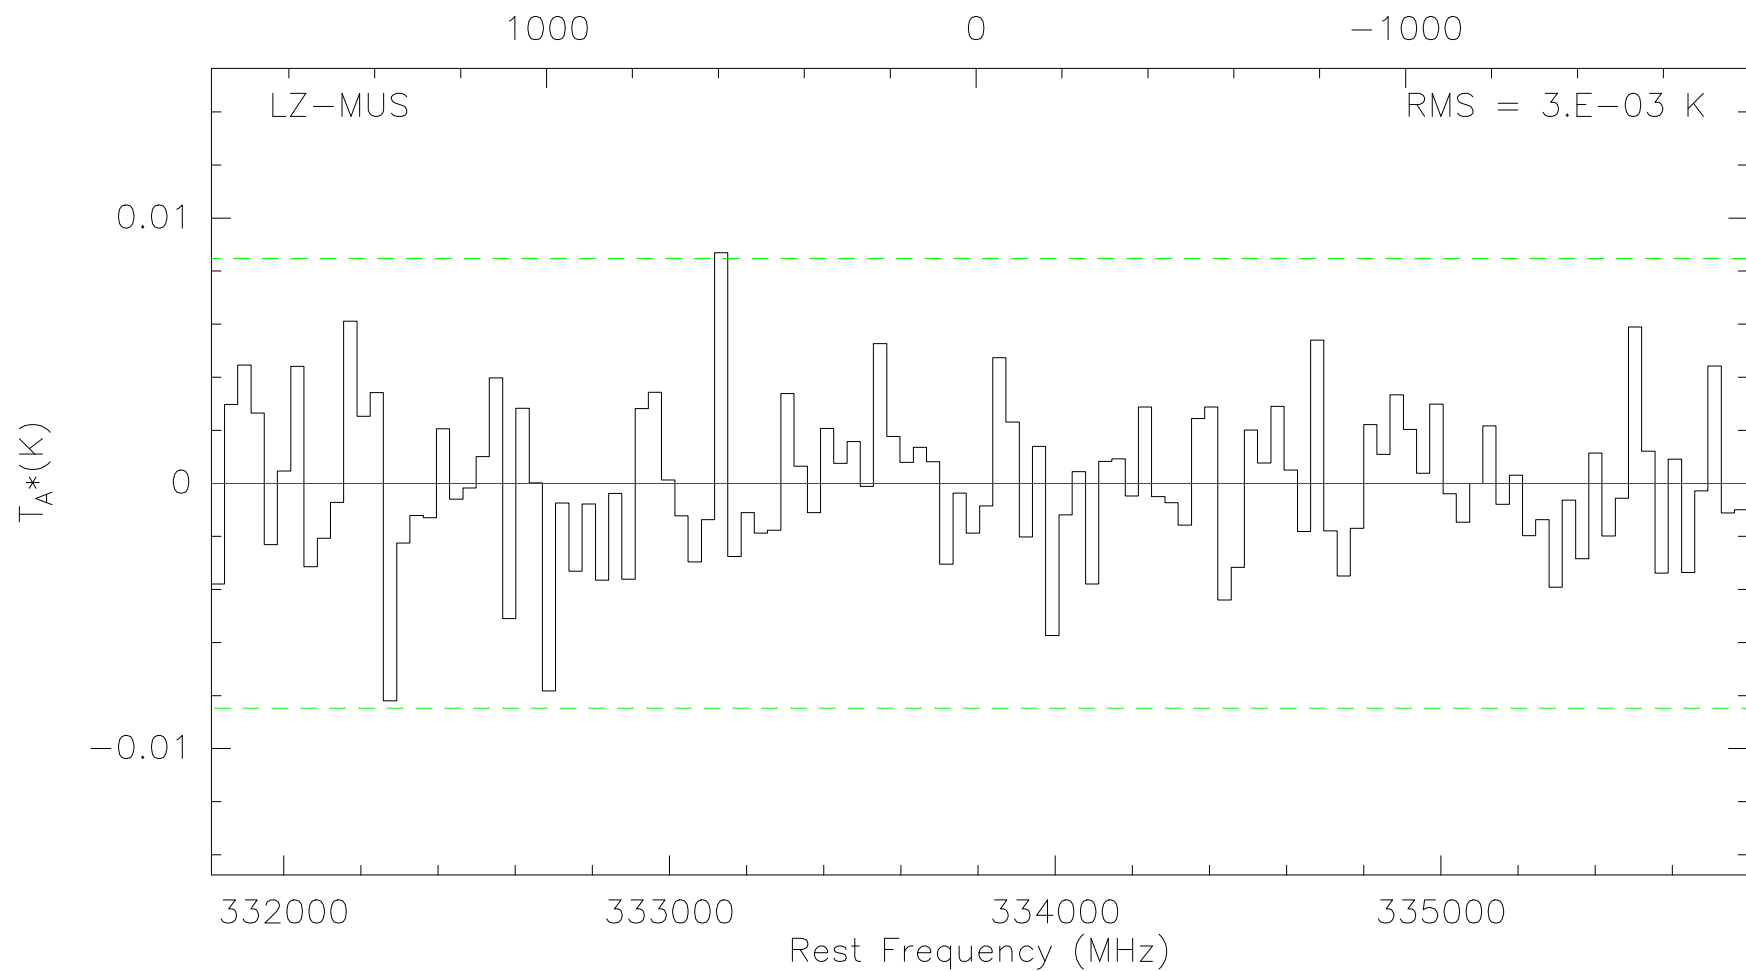

1;1 RR-PIC CO(3-2) OSB AP-F301-XF0- O:25-AUG-2014 R:12-AUG-2020  
RA: 06:35:36.06 DEC: -62:38:24.3 Eq 2000.0 Rad. 0.0° Offs: +0.3 -0.2  
Unknown tau: 0.122 Tsys: 186. Time: 23.3min El: 42.4  
N: 116 I0: 58.7548 V0: 0.000 Dv: 30.84 LSR  
F0: 333795.352 Df: -34.33 Fi: 345795.990

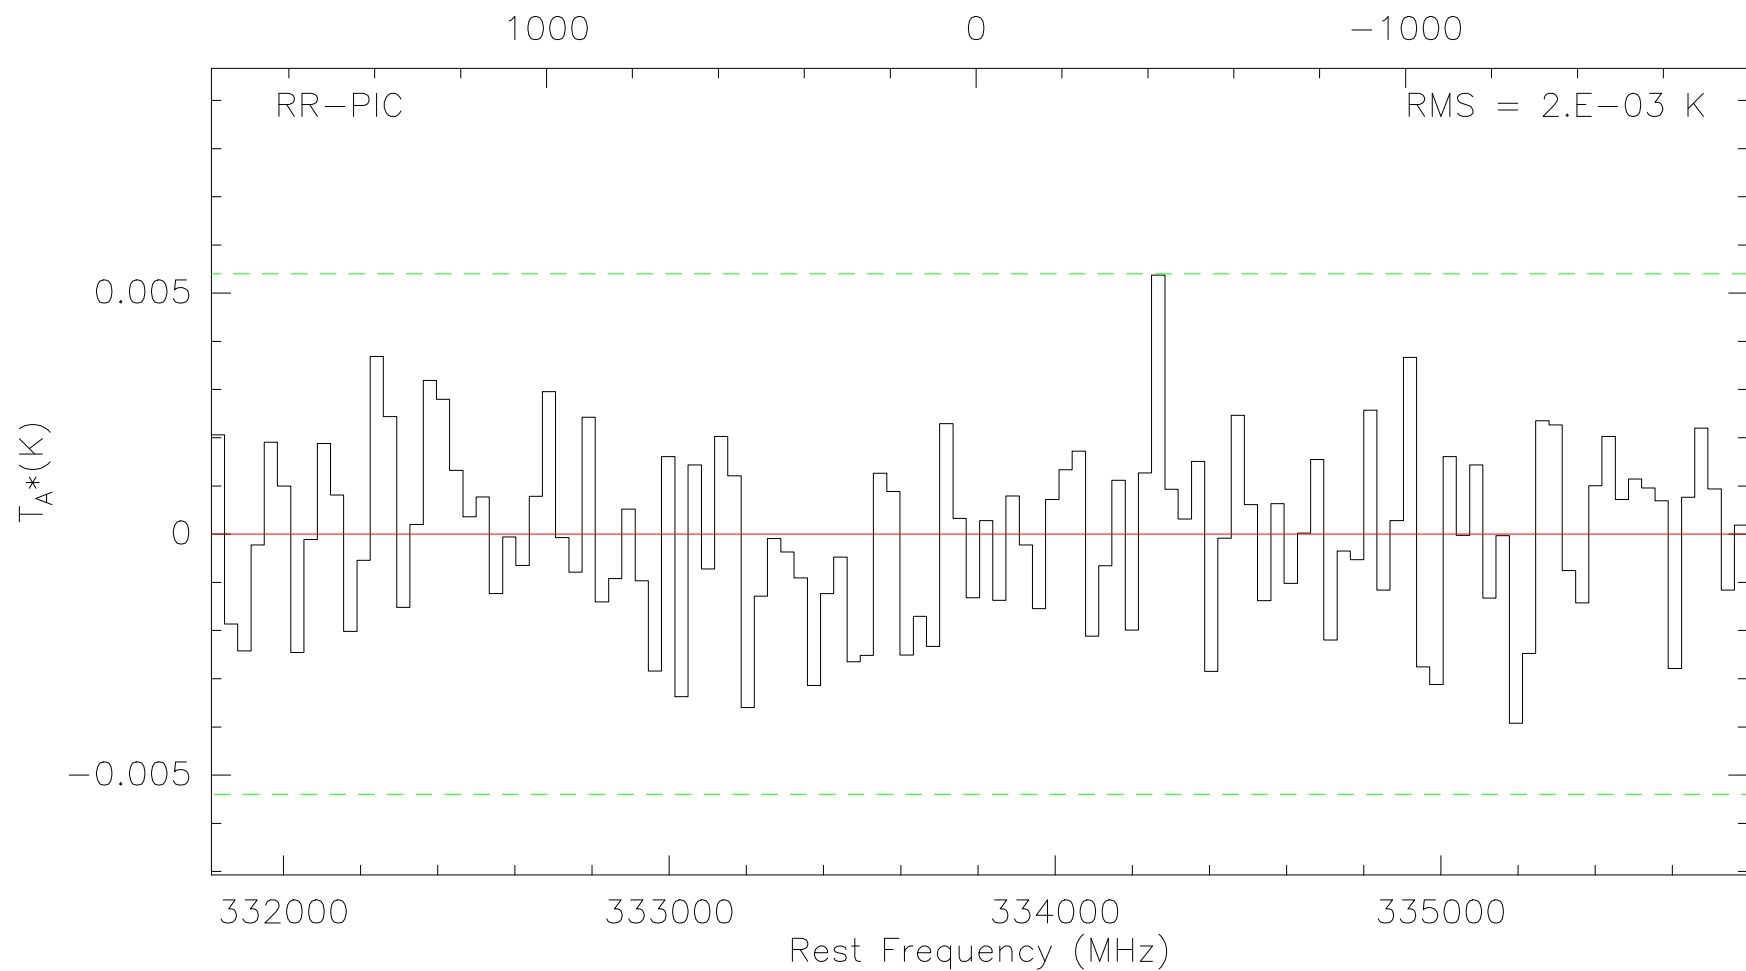

1;1 T-PYX CO(3-2) OSB AP-F301-XF0- O:24-AUG-2014 R:12-AUG-2020  
RA: 09:04:41.50 DEC: -32:22:47.5 Eq 2000.0 Rad. 0.0° Offs: -0.2 -0.5  
Unknown tau: 0.135 Tsys: 176. Time: 23.4min El: 66.0  
N: 116 IO: 58.7548 V0: 0.000 Dv: 30.84 LSR  
FO: 333795.358 Df: -34.33 Fi: 345795.990

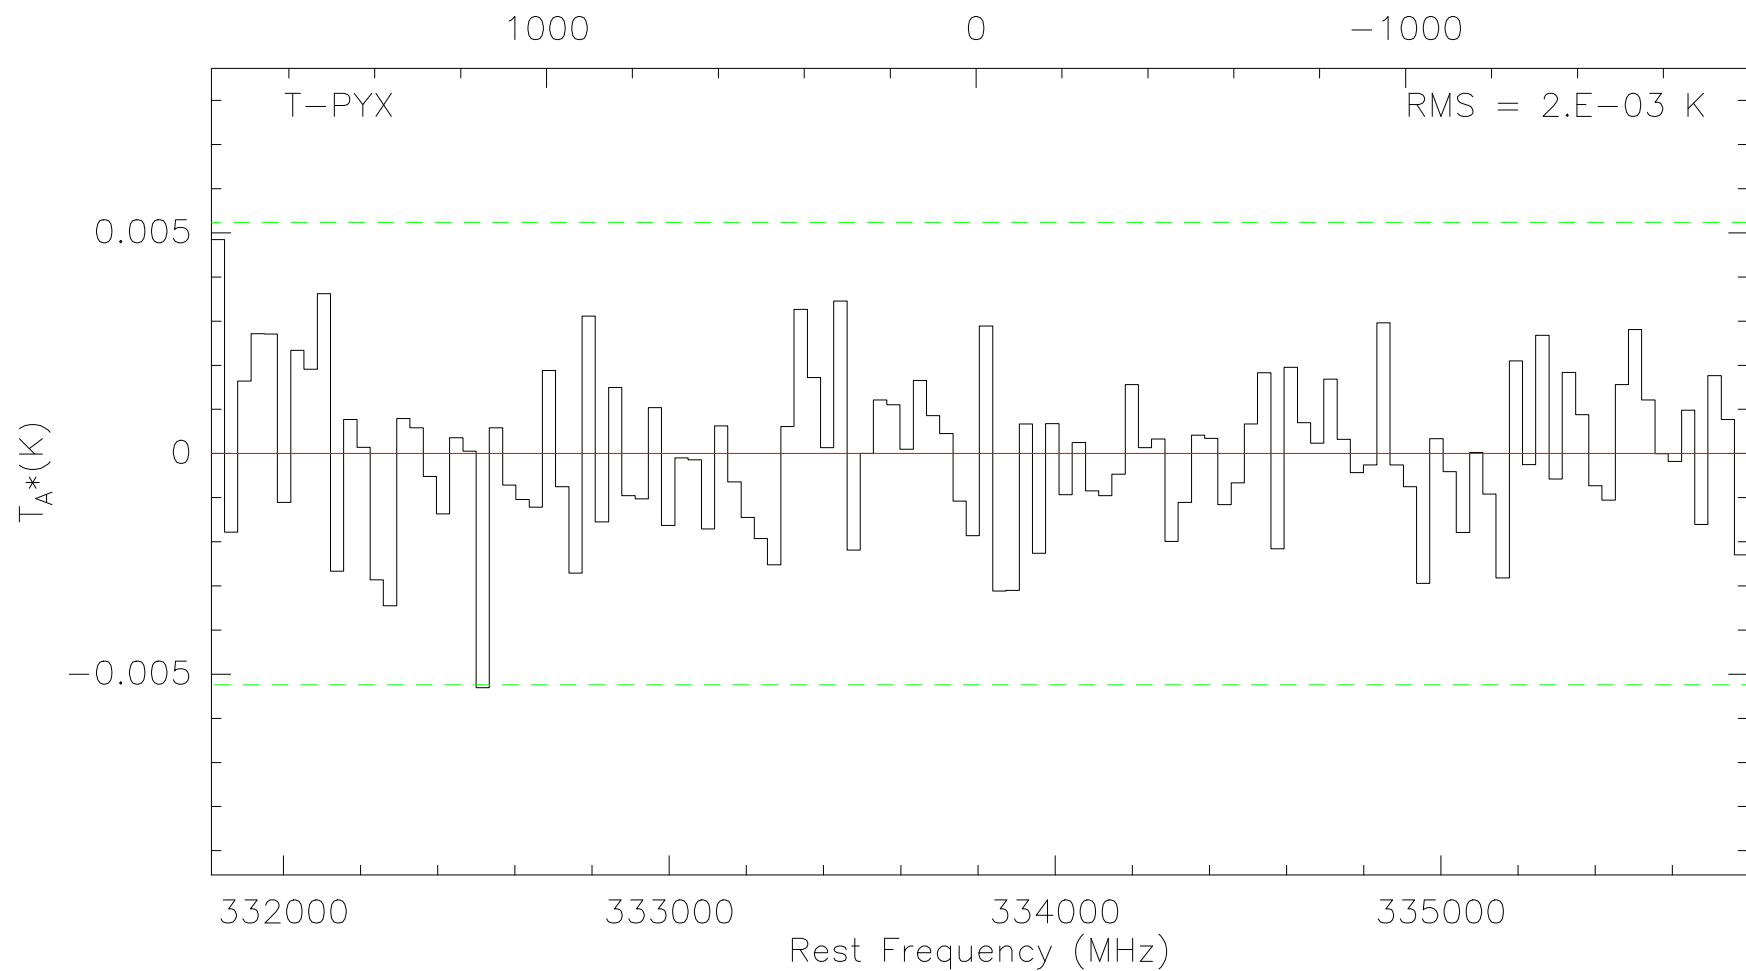

1;1 TV-CRV CO(3-2) OSB AP-F301-XF0- 0:24-AUG-2014 R:12-AUG-2020  
RA: 12:20:24.15 DEC: -18:27:02.0 Eq 2000.0 Rad. 0.0° Offs: +0.2 -0.3  
Unknown tau: 0.133 Tsys: 184. Time: 23.3min El: 51.8  
N: 116 IO: 58.7548 V0: 0.000 Dv: 30.84 LSR  
FO: 333795.186 Df: -34.33 Fi: 345795.990

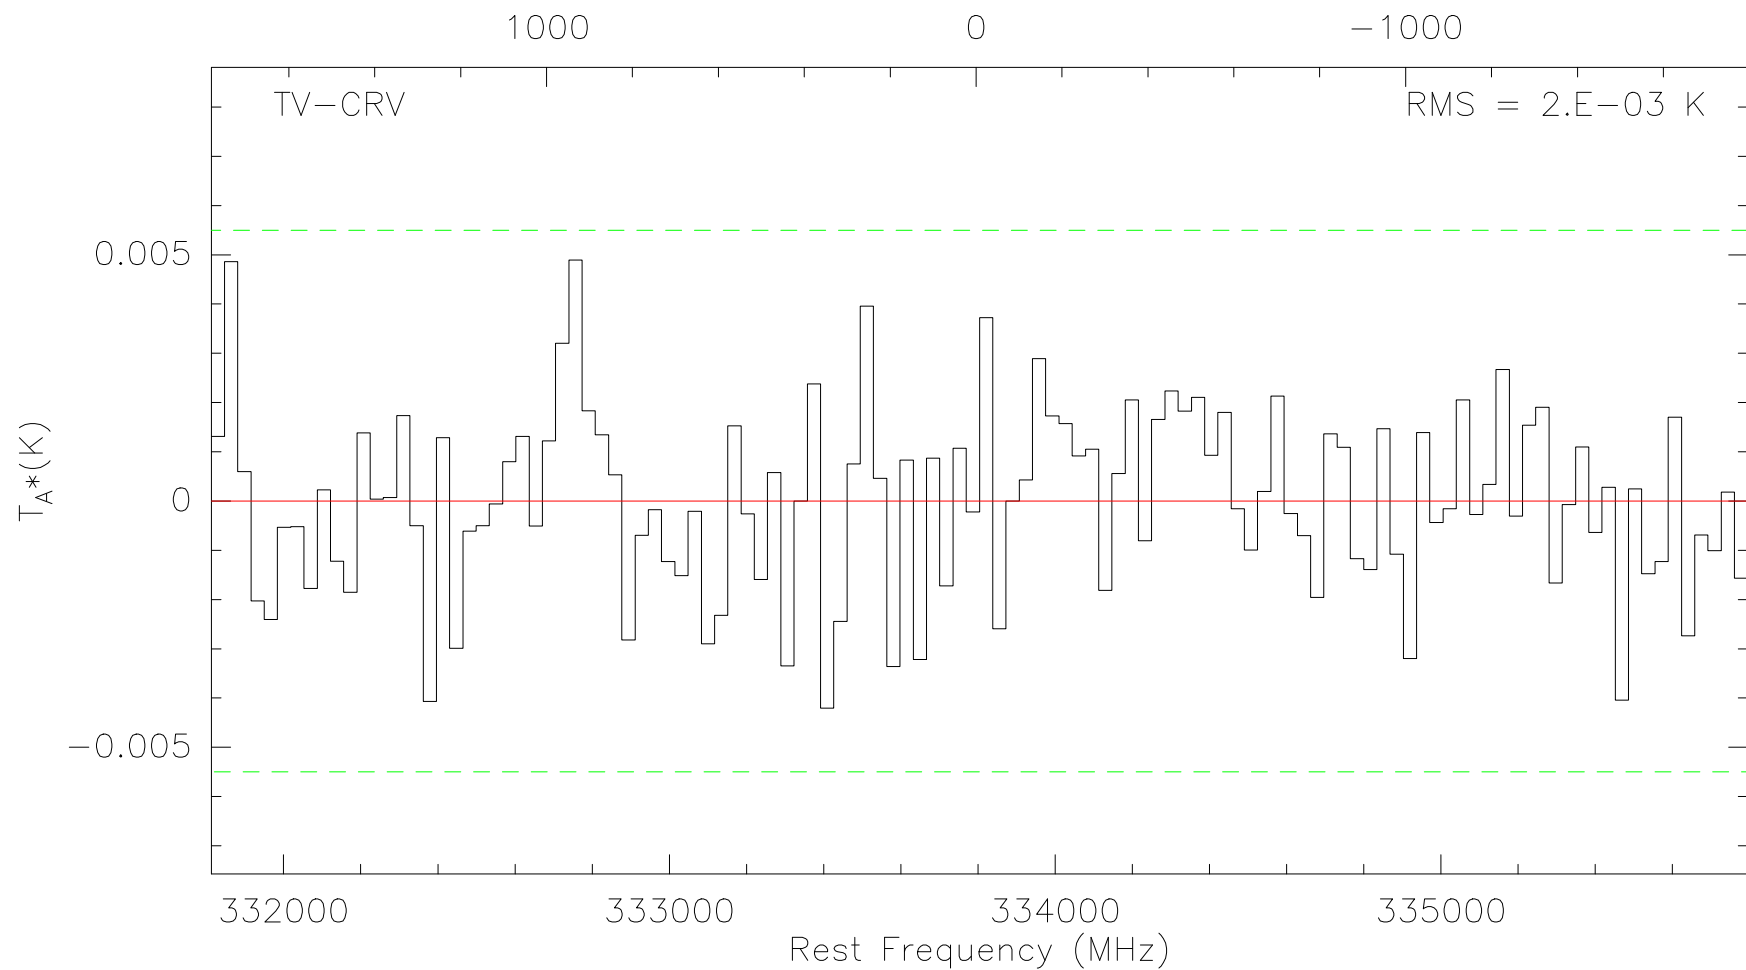

1;1 V1065-CEN CO(3-2) OSB AP-F301-XF0- O:24-AUG-2014 R:12-AUG-2020  
RA: 11:43:10.33 DEC: -58:04:04.3 Eq 2000.0 Rad. 0.0° Offs: -0.4 -0.3  
Unknown tau: 0.221 Tsys: 329. Time: 23.3min El: 30.0  
N: 116 IO: 58.7548 V0: 0.000 Dv: 30.84 LSR  
FO: 333795.004 Df: -34.34 Fi: 345795.990

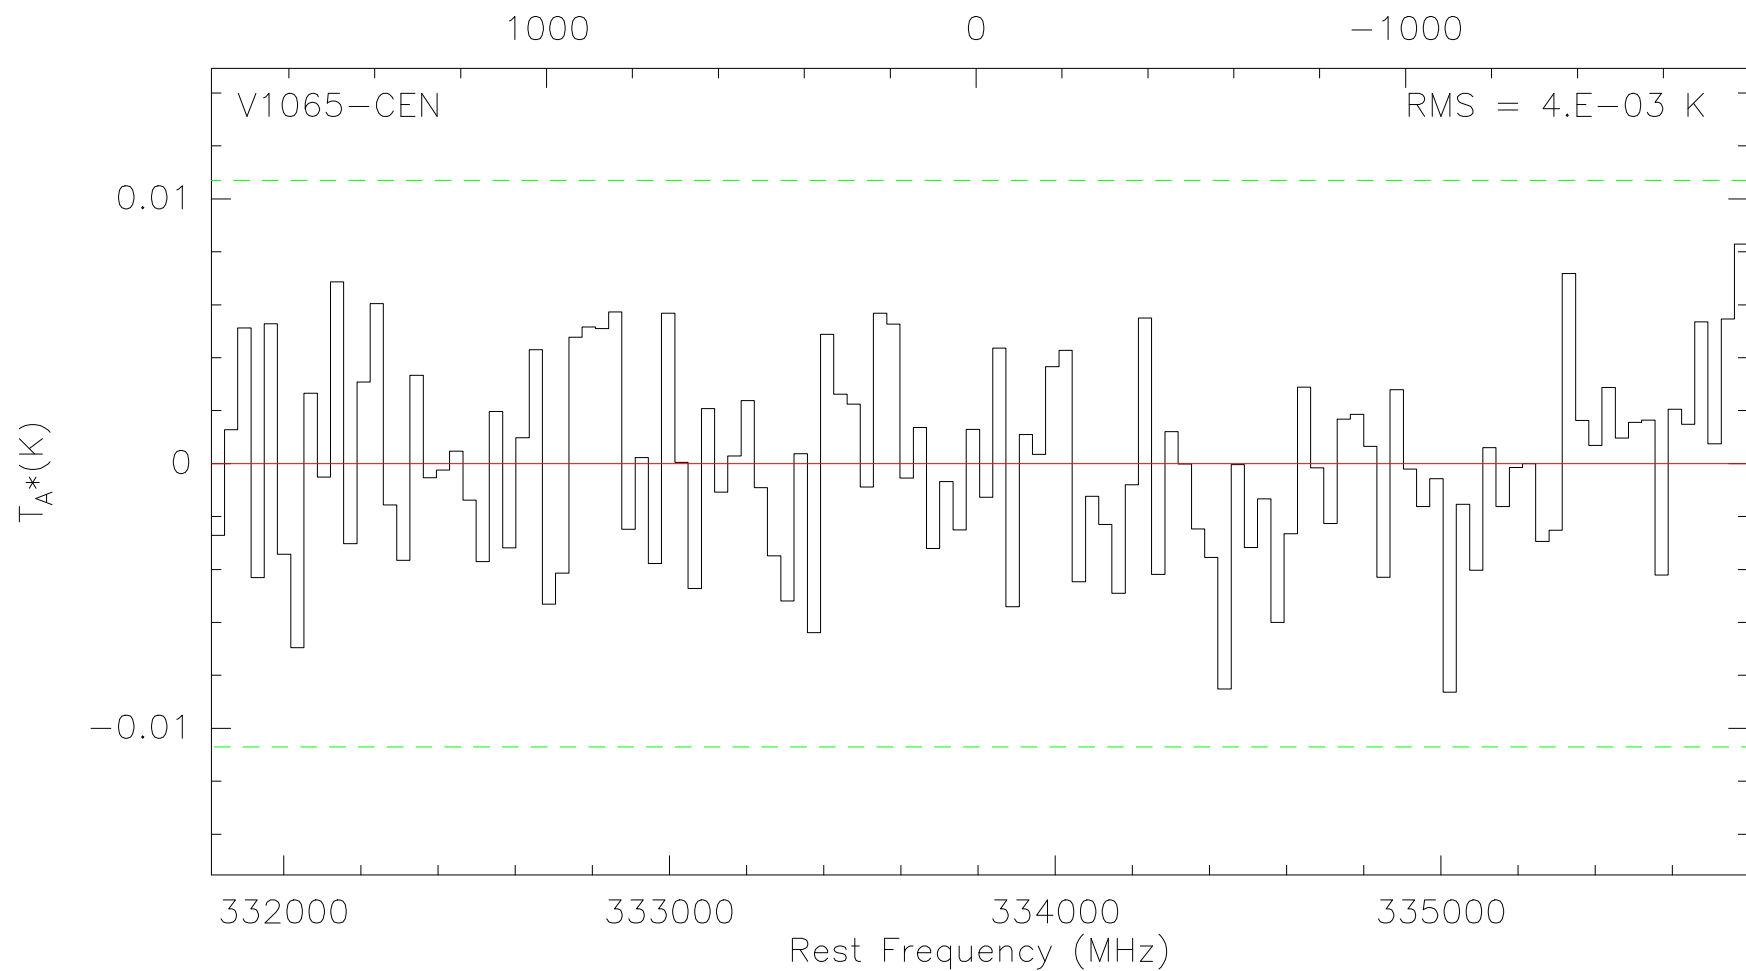

1;1 V351-CAR CO(3-2) OSB AP-F301-XF0- O:28-AUG-2014 R:12-AUG-2020  
RA: 10:45:19.14 DEC: -72:03:56.0 Eq 2000.0 Rad. 0.0° Offs: +0.2 -0.4  
Unknown tau: 0.197 Tsys: 251. Time: 23.4min El: 40.8  
N: 116 IO: 58.7548 V0: 0.000 Dv: 30.84 LSR  
FO: 333795.087 Df: -34.33 Fi: 345795.990

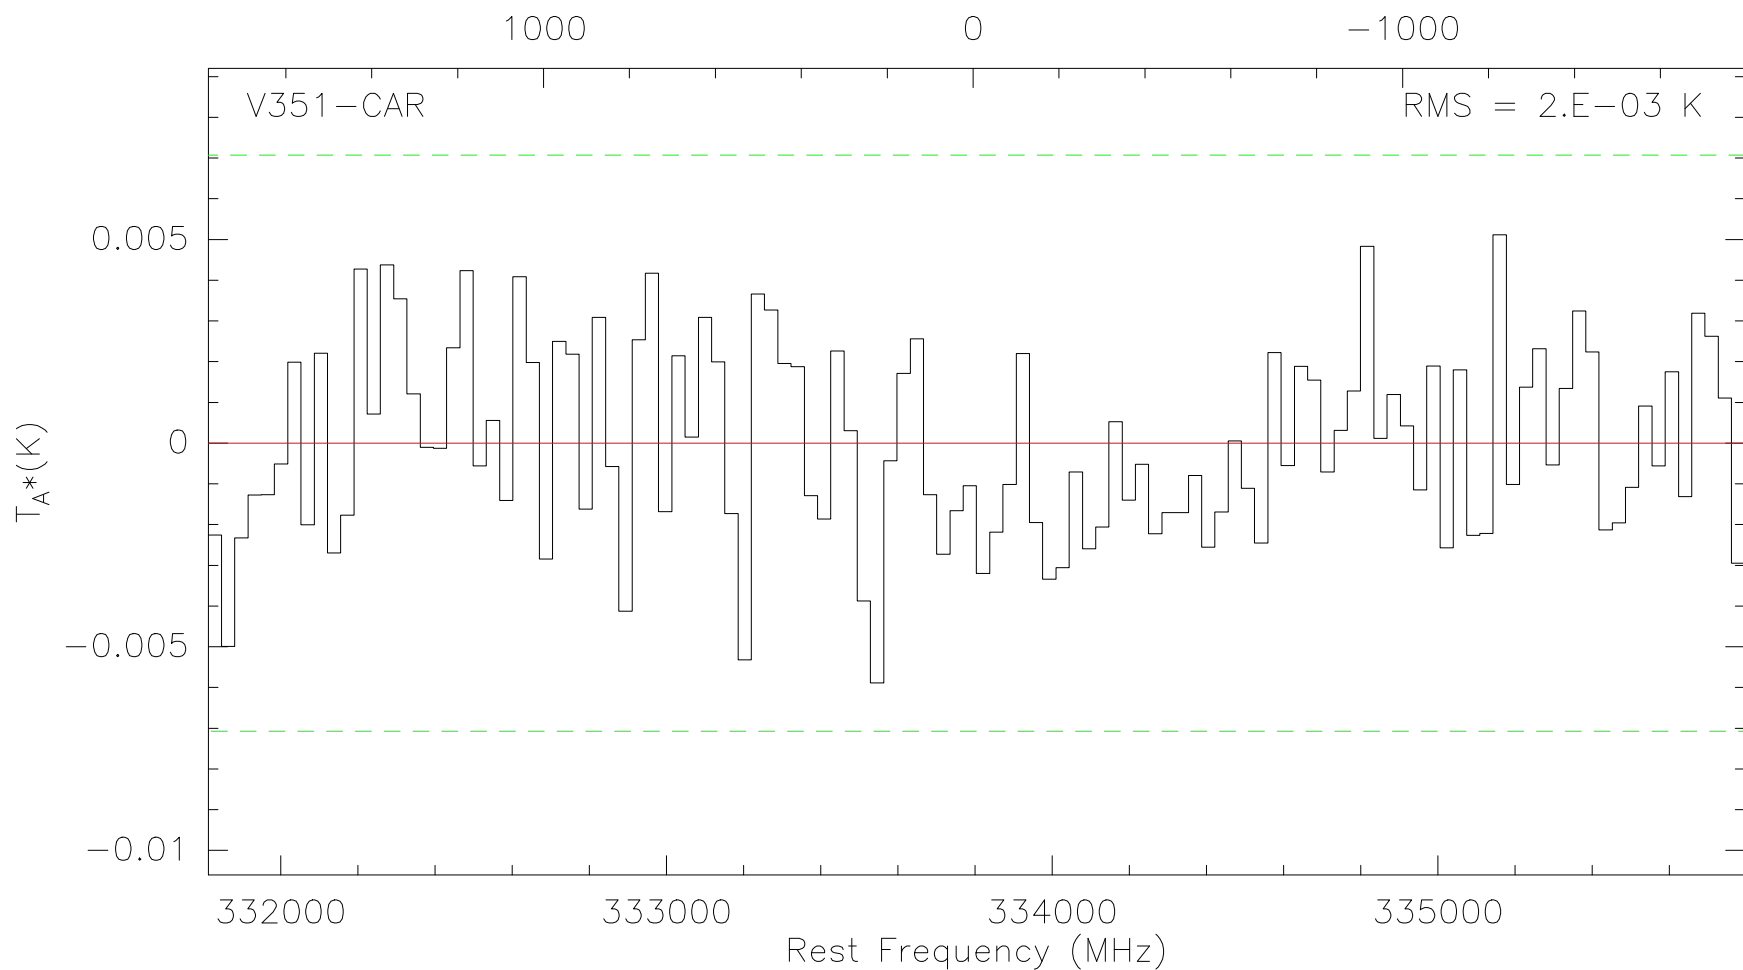

1;1 V359-CEN CO(3-2) OSB AP-F301-XF0- O:24-AUG-2014 R:12-AUG-2020  
RA: 11:58:15.33 DEC: -41:46:08.4 Eq 2000.0 Rad. 0.0° Offs: +0.2 -0.4  
Unknown tau: 0.134 Tsys: 176. Time: 23.4min El: 70.8  
N: 116 IO: 58.7548 V0: 0.000 Dv: 30.84 LSR  
FO: 333795.029 Df: -34.34 Fi: 345795.990

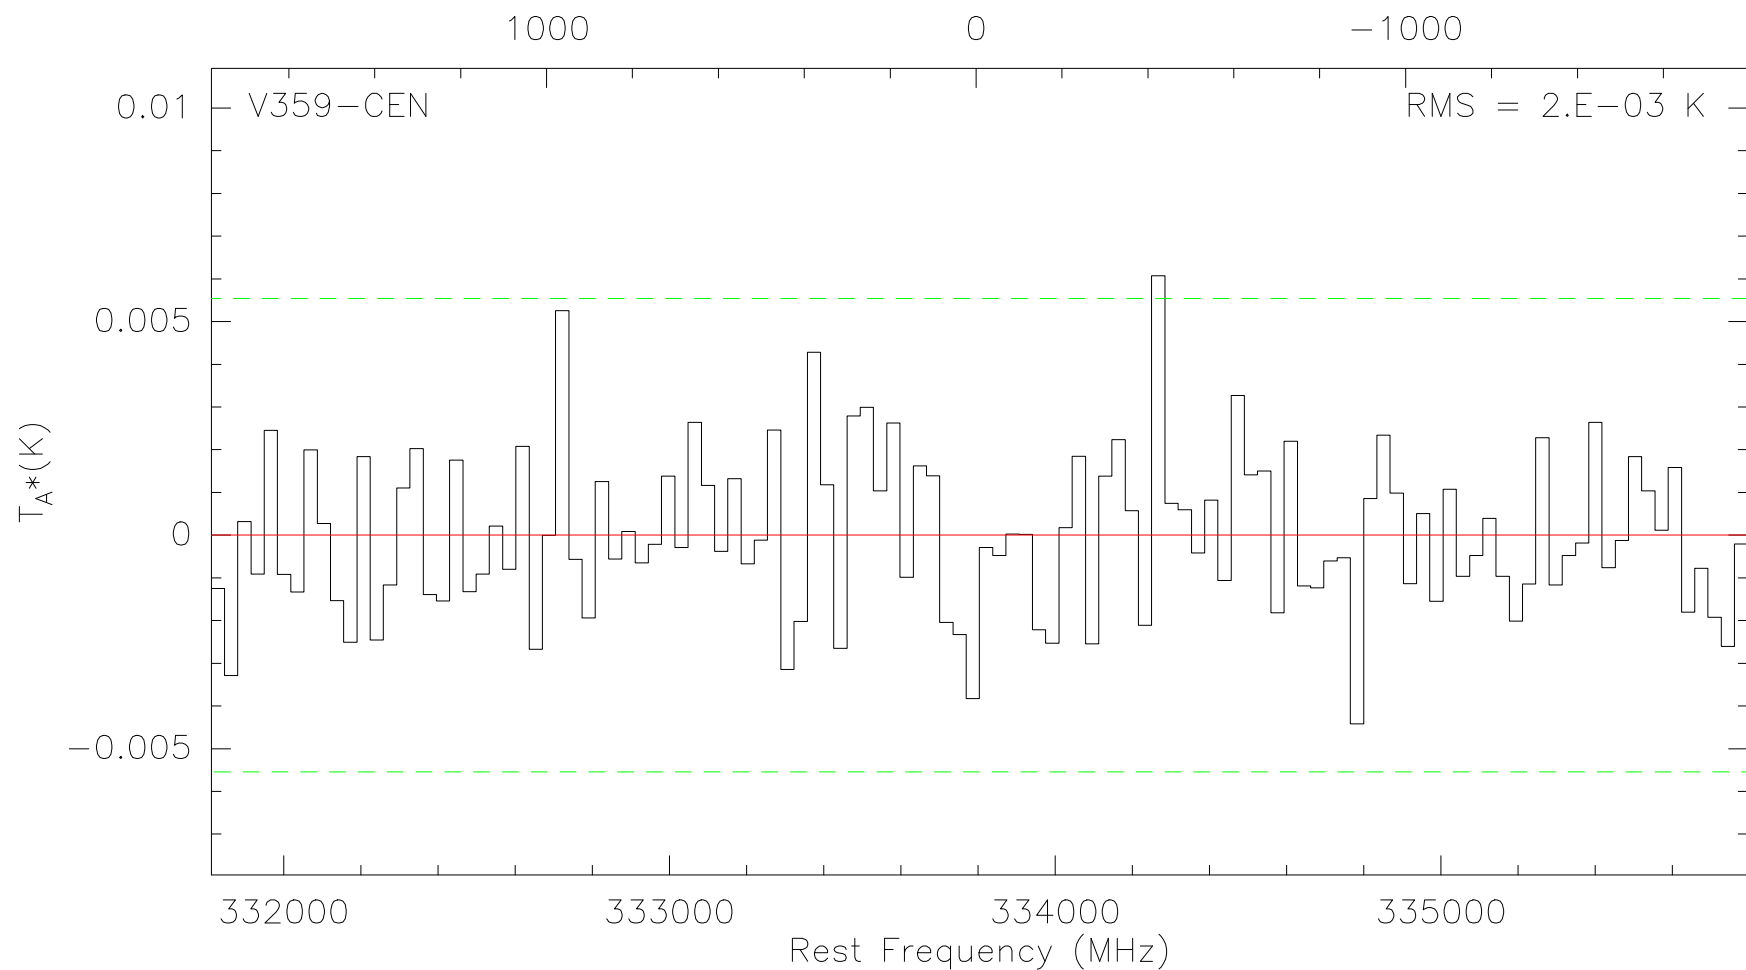

1;1 V382-VEL CO(3-2) OSB AP-F301-XF0- 0:28-AUG-2014 R:12-AUG-2020  
RA: 10:44:48.39 DEC: -52:25:30.7 Eq 2000.0 Rad. 0.0° Offs: +0.3 -0.4  
Unknown tau: 0.186 Tsys: 212. Time: 23.4min El: 58.5  
N: 116 IO: 58.7548 V0: 0.000 Dv: 30.84 LSR  
FO: 333795.109 Df: -34.33 Fi: 345795.990

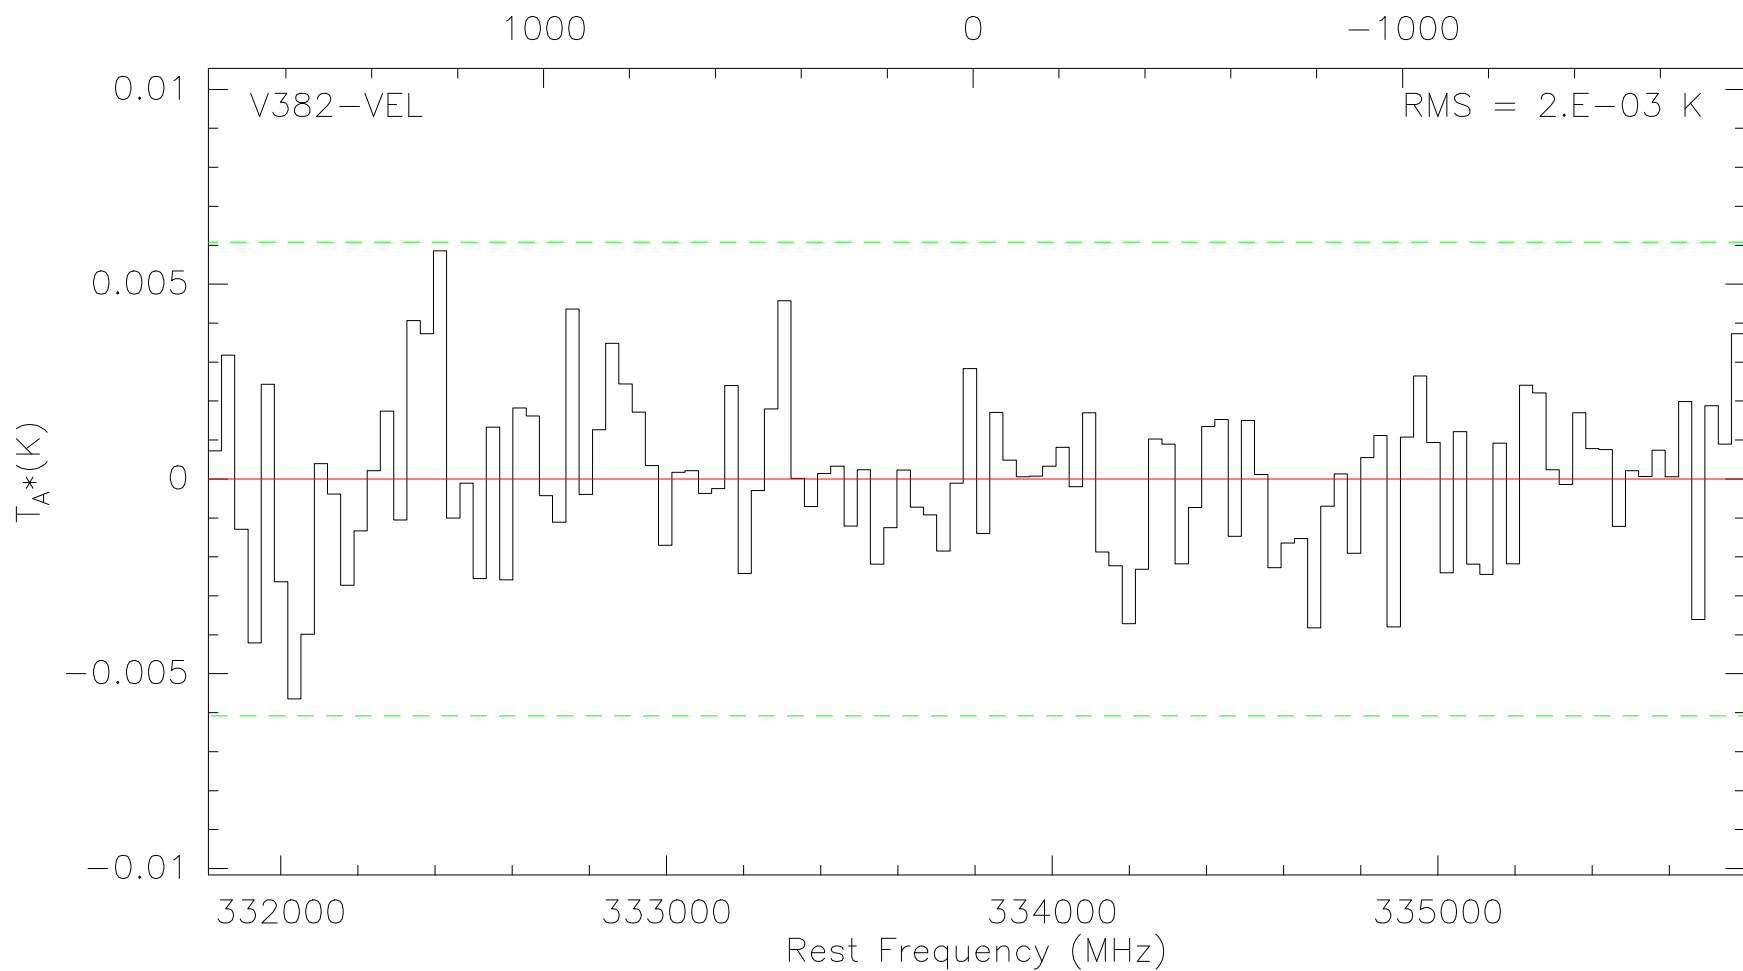

1;1 V598-PUP CO(3-2) OSB AP-F301-XF0- O:25-AUG-2014 R:12-AUG-2020  
RA: 07:05:42.50 DEC: -38:14:39.4 Eq 2000.0 Rad. 0.0° Offs: +0.2 -0.3  
Unknown tau: 0.113 Tsys: 167. Time: 23.4min El: 59.6  
N: 116 IO: 58.7548 V0: 0.000 Dv: 30.84 LSR  
FO: 333795.572 Df: -34.33 Fi: 345795.990

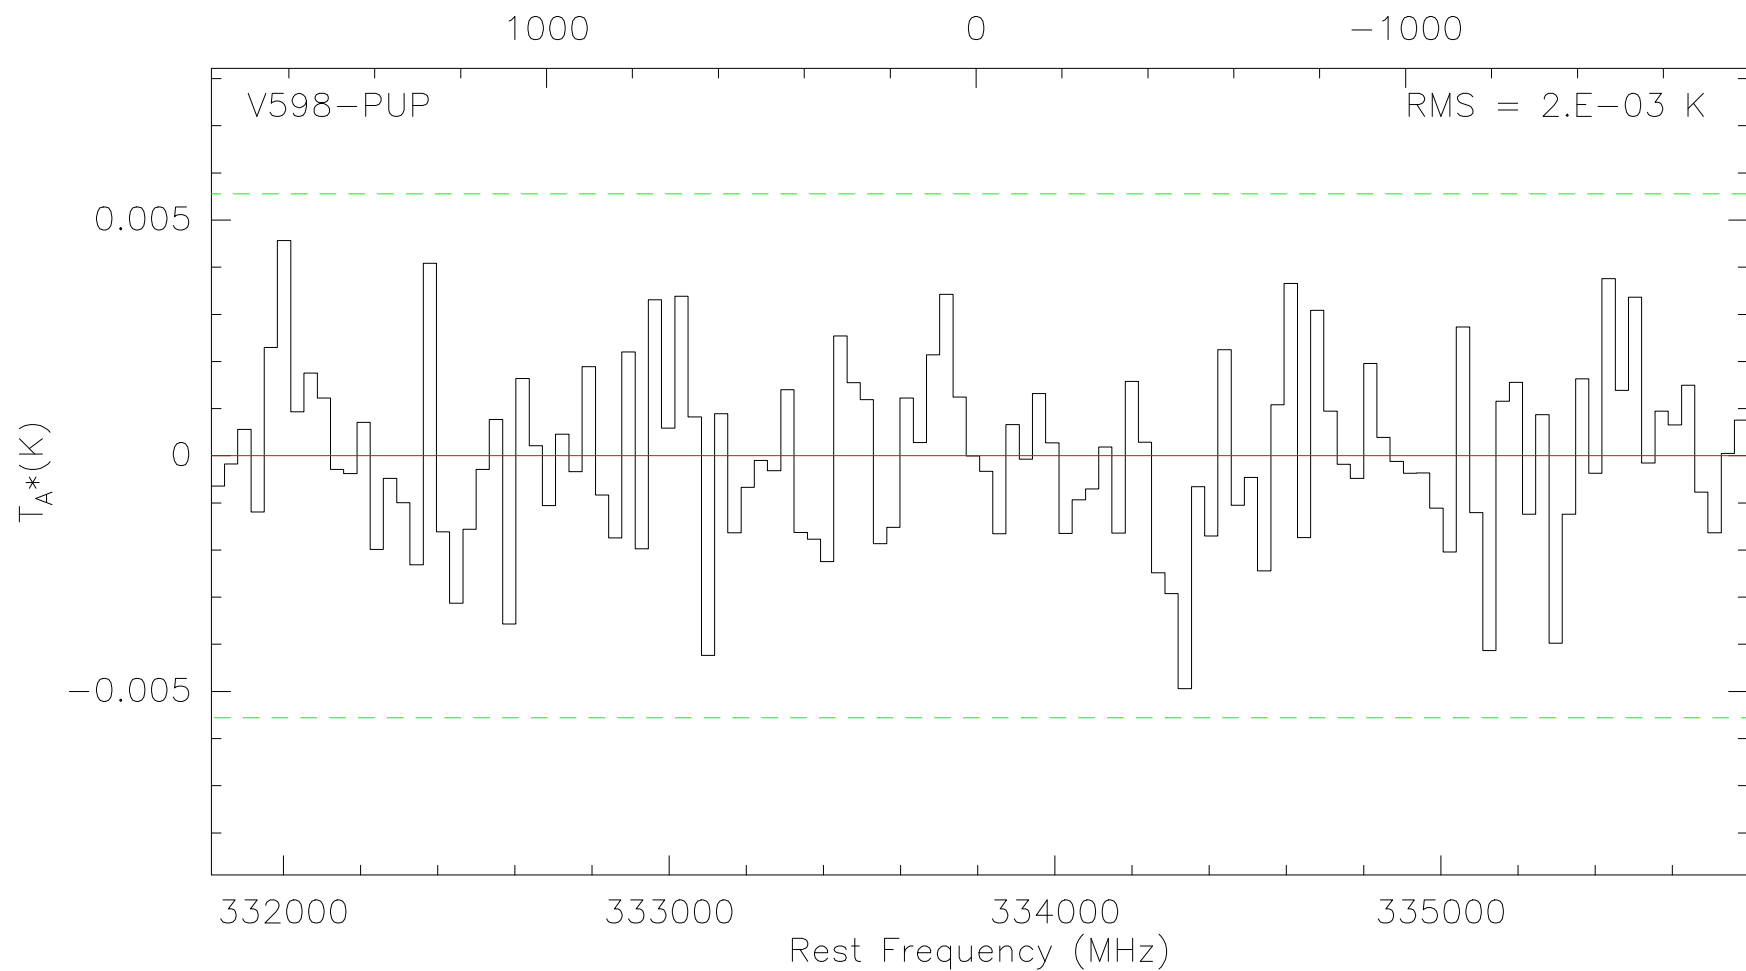

1;1 VX-FOR CO(3-2) OSB AP-F301-XF0- 0:24-AUG-2014 R:12-AUG-2020  
RA: 03:26:45.71 DEC: -34:26:25.2 Eq 2000.0 Rad. 0.0° Offs: +0.2 -0.2  
Unknown tau: 0.203 Tsys: 214. Time: 23.3min El: 53.4  
N: 116 IO: 58.7548 V0: 0.000 Dv: 30.83 LSR  
FO: 333796.001 Df: -34.33 Fi: 345795.990

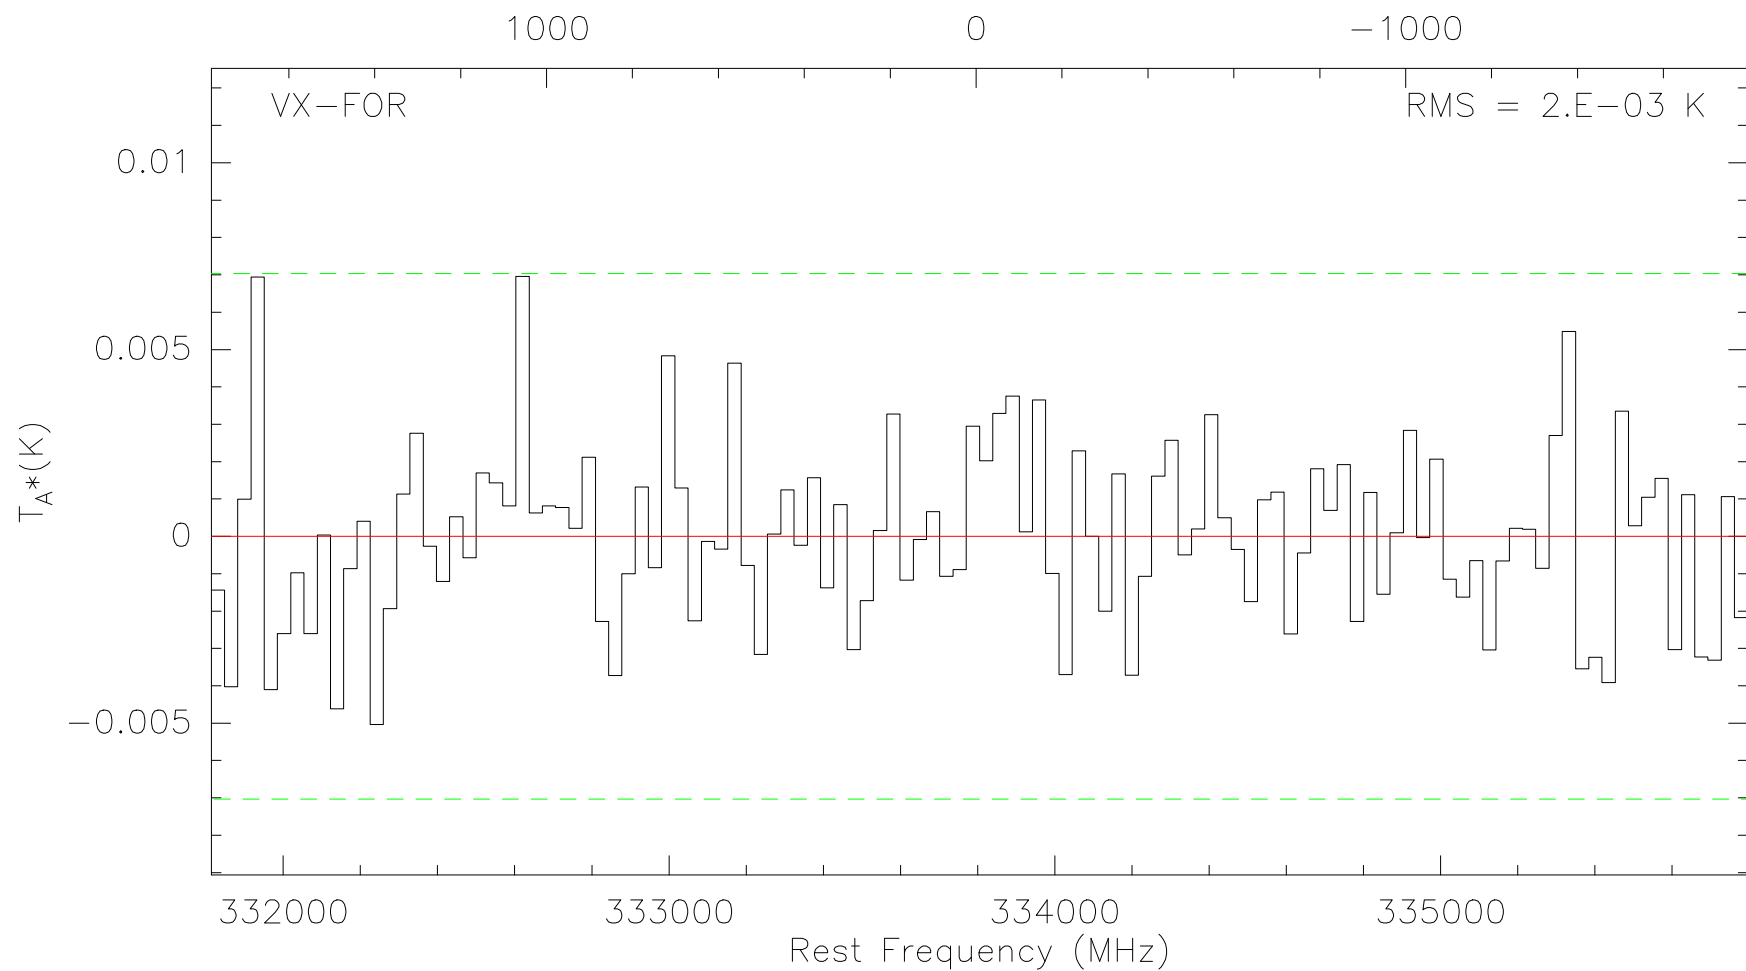

1;1 WX-CET CO(3-2) OSB AP-F301-XF0- O:24-AUG-2014 R:12-AUG-2020  
RA: 01:17:04.17 DEC: -17:56:23.0 Eq 2000.0 Rad. 0.0° Offs: -0.2 -0.3  
Unknown tau: 0.137 Tsys: 174. Time: 23.3min El: 67.5  
N: 116 IO: 58.7548 V0: 0.000 Dv: 30.83 LSR  
FO: 333796.330 Df: -34.33 Fi: 345795.990

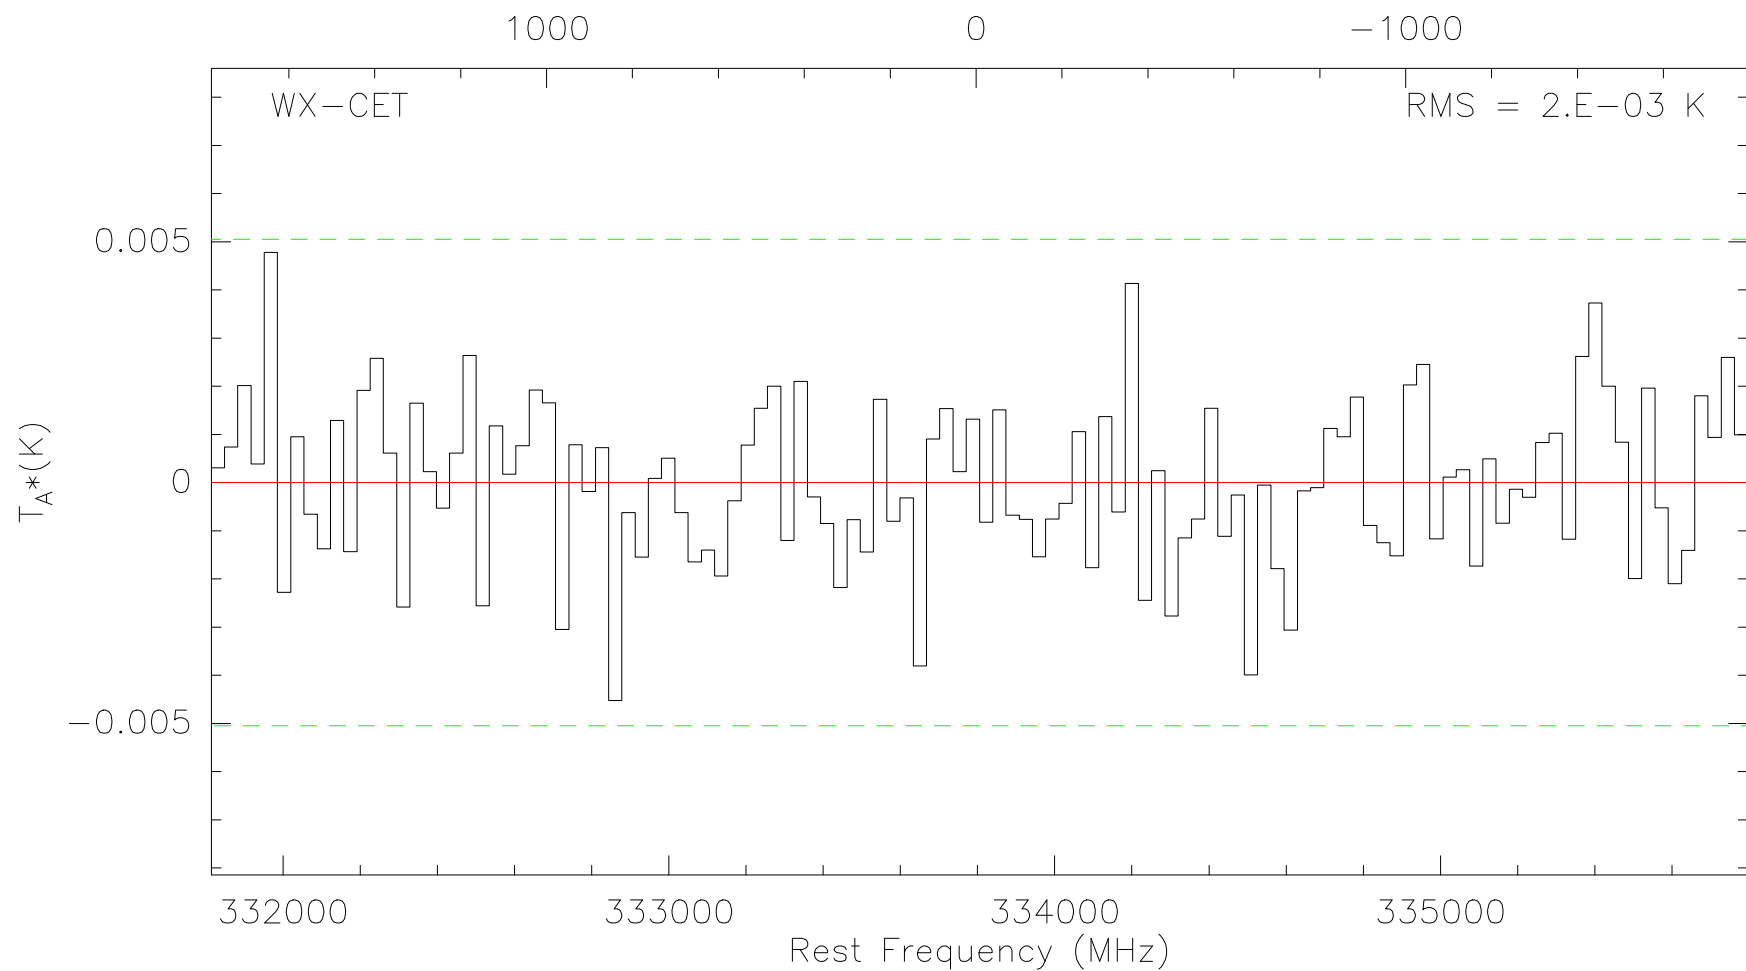

1;1 AICIR CO(3-2) OSB AP-F301-XF0- O:13-JUL-2016 R:07-AUG-2020  
RA: 14:49:31.29 DEC: -68:51:35.9 Eq 2000.0 Rad. 0.0° Offs: +0.5 -0.2  
Unknown tau: 0.260 Tsys: 322. Time: 5.0min El: 33.7  
N: 116 IO: 58.7548 V0: 0.000 Dv: 30.84 LSR  
FO: 333795.239 Df: -34.33 Fi: 345795.990

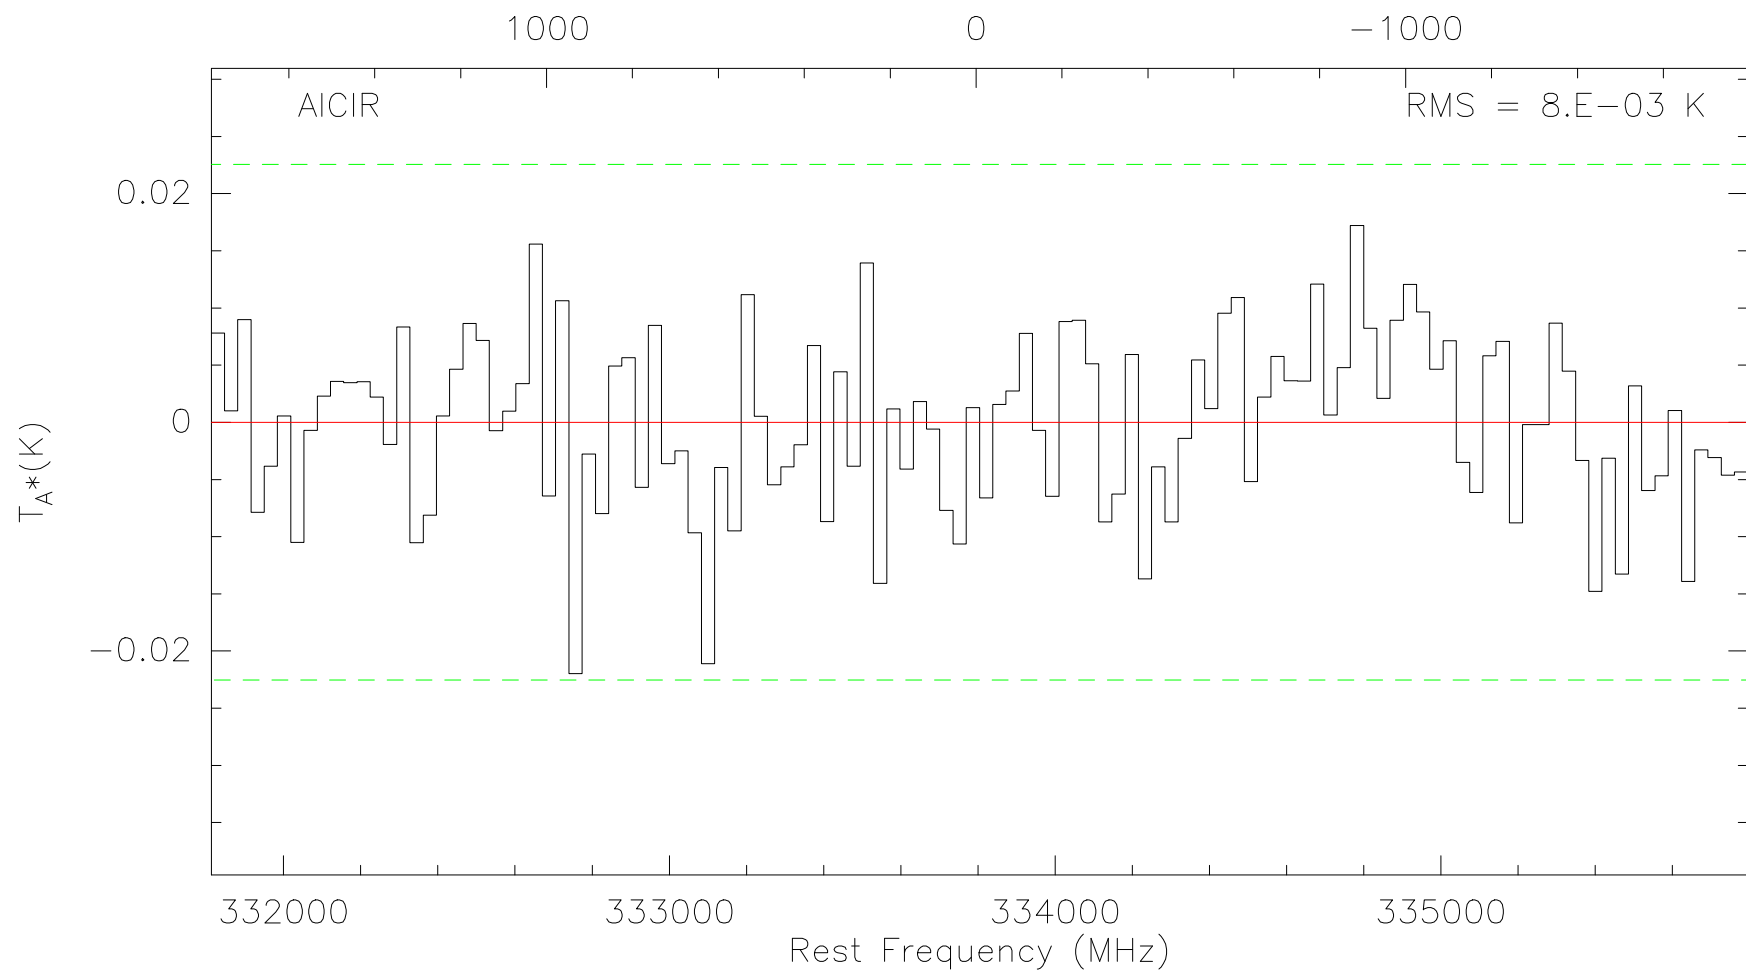

1;1 ATSGR CO(3-2) OSB AP-F301-XF0- O:14-JUL-2016 R:07-AUG-2020  
RA: 18:03:30.87 DEC: -26:28:28.5 Eq 2000.0 Rad. 0.0° Offs: +0.1 -0.4  
Unknown tau: 0.277 Tsys: 229. Time: 9.9min El: 66.9  
N: 116 IO: 58.7548 V0: 0.000 Dv: 30.83 LSR  
FO: 333796.016 Df: -34.33 Fi: 345795.990

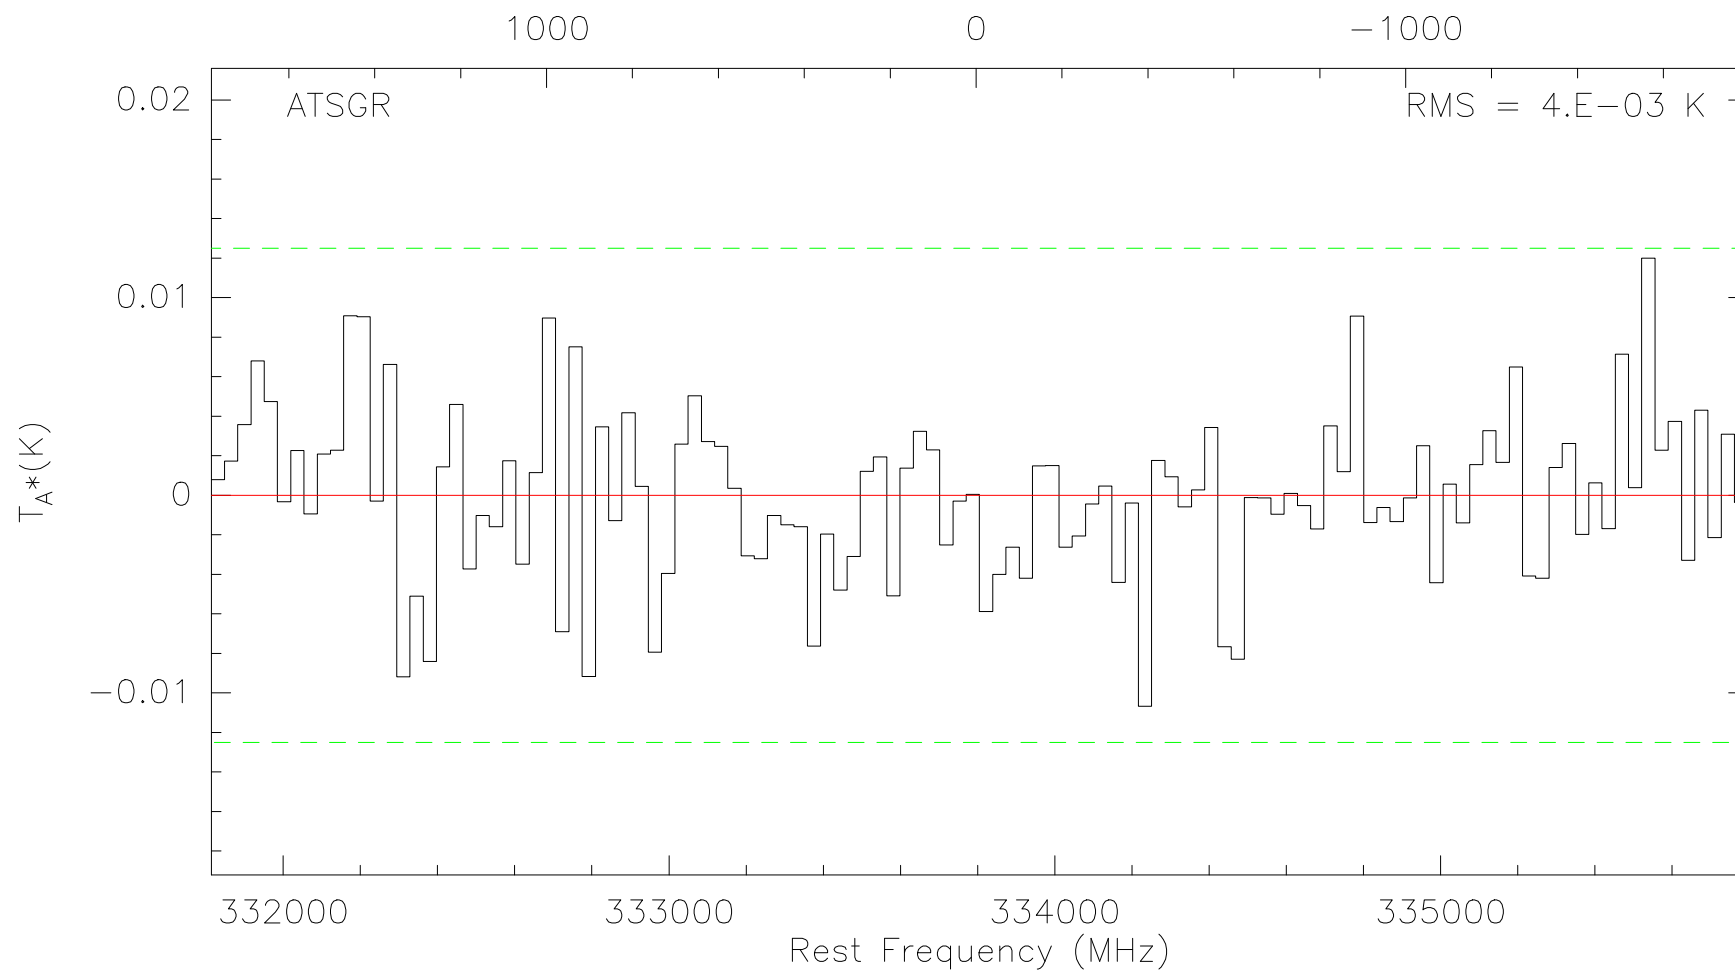

1;1 FMSG R CO(3-2) OSB AP-F301-XF0- O:13-JUL-2016 R:07-AUG-2020  
RA: 18:17:18.10 DEC: -23:38:27.0 Eq 2000.0 Rad. 0.0° Offs: -0.1 -0.4  
Unknown tau: 0.188 Tsys: 232. Time: 9.9min El: 35.9  
N: 116 IO: 58.7548 V0: 0.000 Dv: 30.83 LSR  
FO: 333796.102 Df: -34.33 Fi: 345795.990

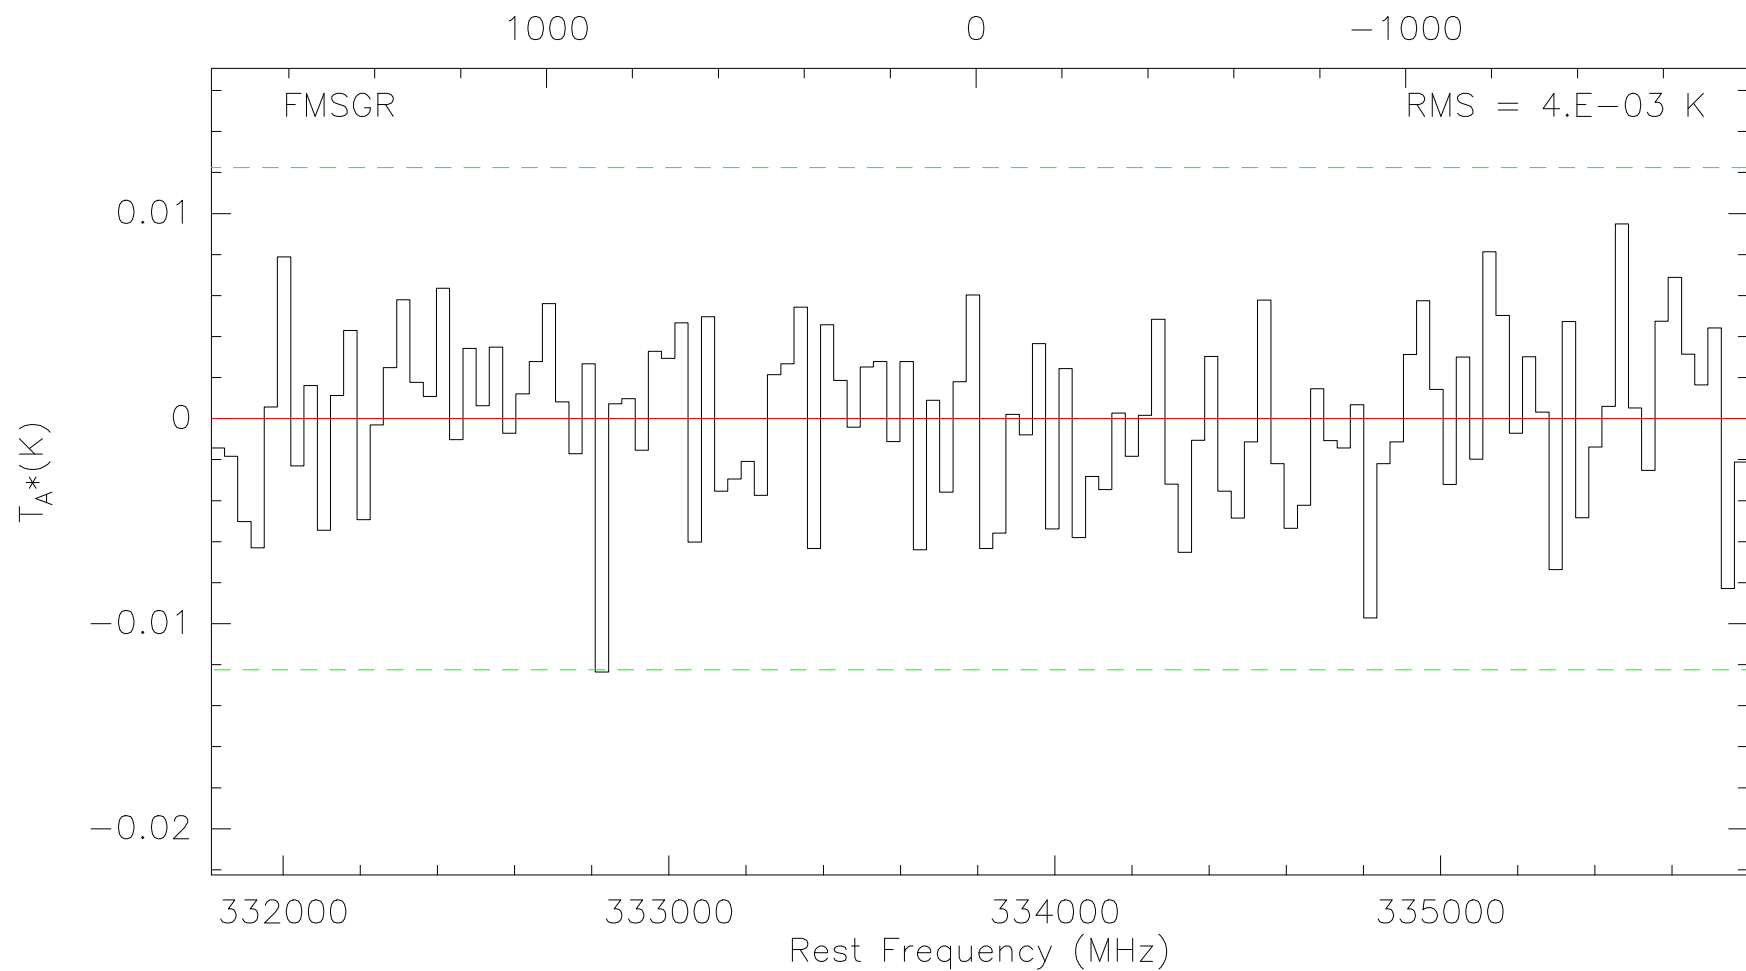

1;1 GRSGR CO(3-2) OSB AP-F301-XF0- O:13-JUL-2016 R:07-AUG-2020  
RA: 18:22:58.50 DEC: -25:34:47.3 Eq 2000.0 Rad. 0.0° Offs: -0.1 -0.5  
Unknown tau: 0.207 Tsys: 199. Time: 9.9min El: 58.2  
N: 116 IO: 58.7548 V0: 0.000 Dv: 30.83 LSR  
FO: 333796.109 Df: -34.33 Fi: 345795.990

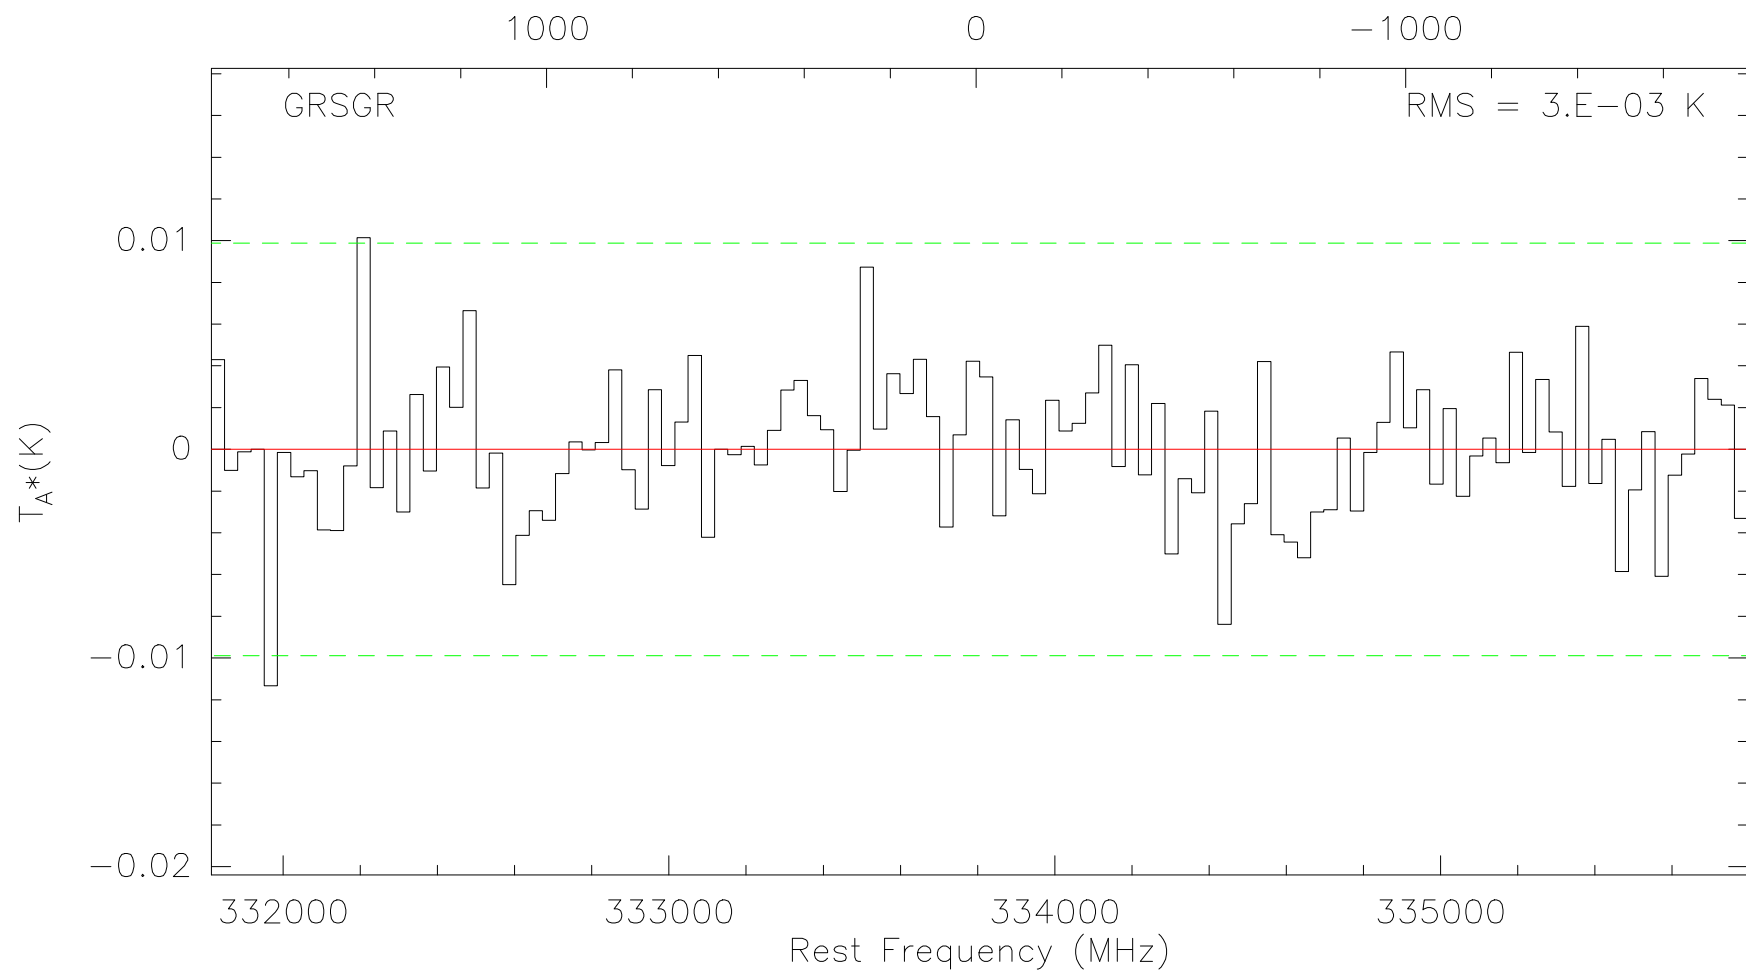

1;1 HSSGR CO(3-2) OSB AP-F301-XF0- O:13-JUL-2016 R:07-AUG-2020  
RA: 18:28:03.44 DEC: -21:34:24.7 Eq 2000.0 Rad. 0.0° Offs: -0.3 -0.3  
Unknown tau: 0.175 Tsys: 257. Time: 9.9min El: 27.0  
N: 116 IO: 58.7548 V0: 0.000 Dv: 30.83 LSR  
FO: 333796.170 Df: -34.33 Fi: 345795.990

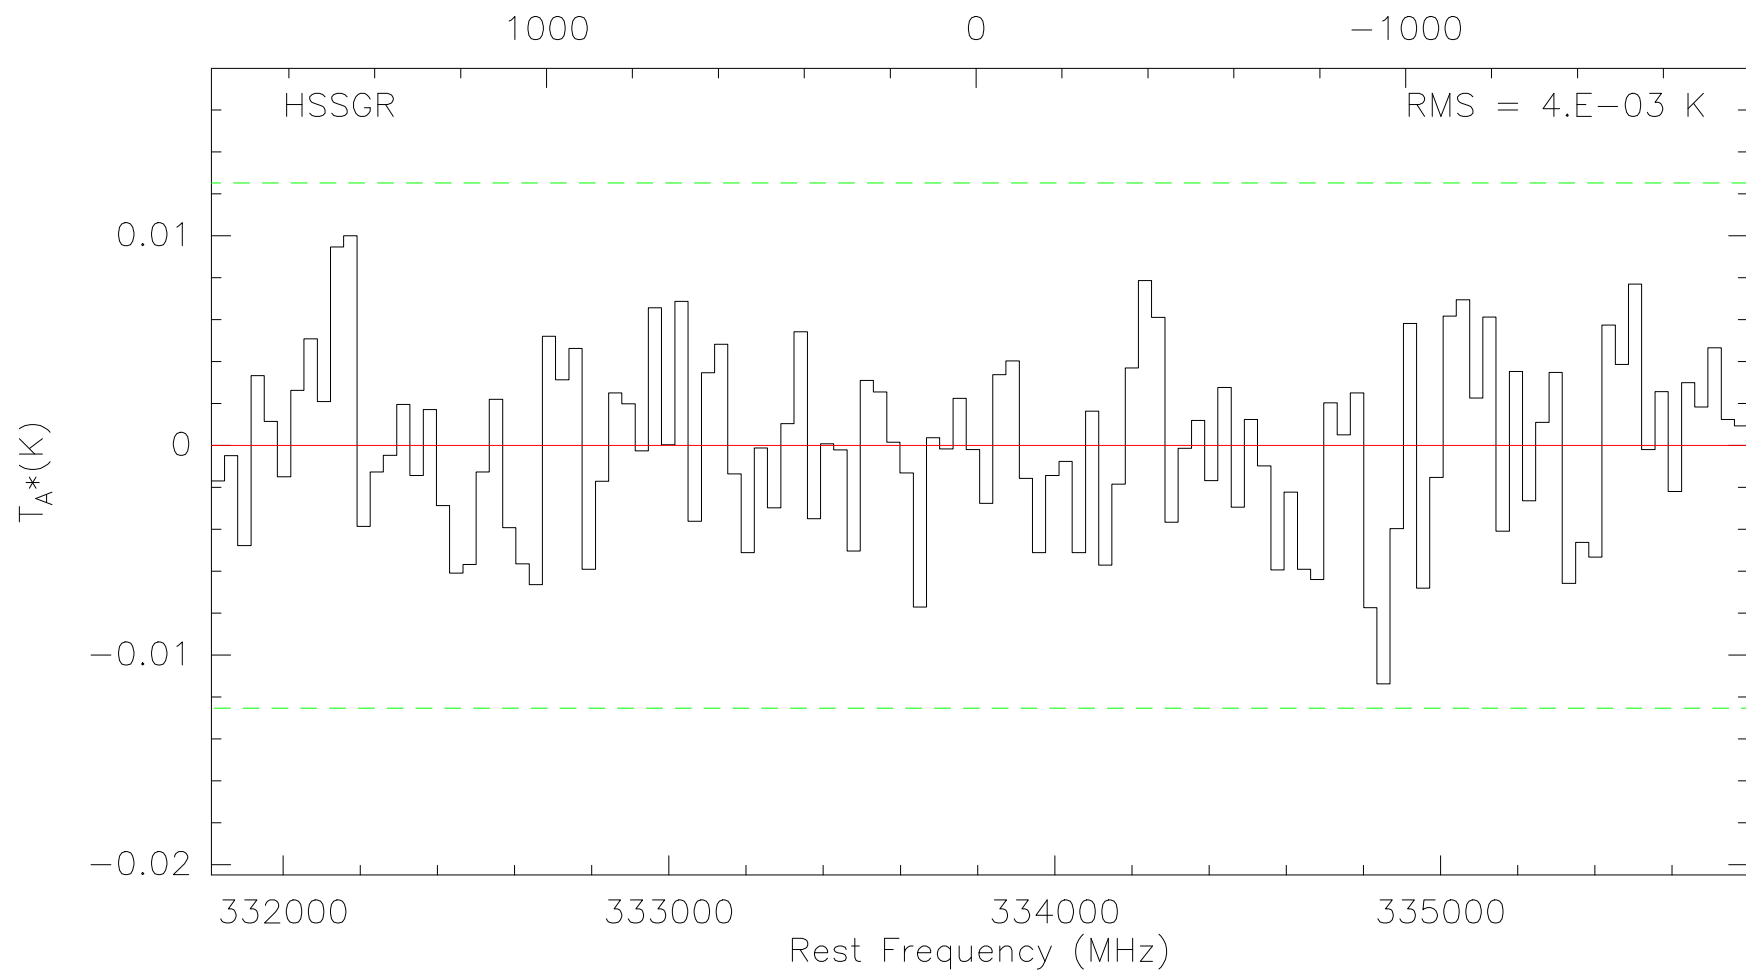

1;1 ILNOR CO(3-2) OSB AP-F301-XF0- O:07-JUL-2016 R:07-AUG-2020  
RA: 15:29:23.18 DEC: -50:35:00.7 Eq 2000.0 Rad. 0.0° Offs: -0.2 -0.5  
Unknown tau: 0.275 Tsys: 251. Time: 9.9min El: 52.2  
N: 116 IO: 58.7548 V0: 0.000 Dv: 30.84 LSR  
FO: 333795.343 Df: -34.33 Fi: 345795.990

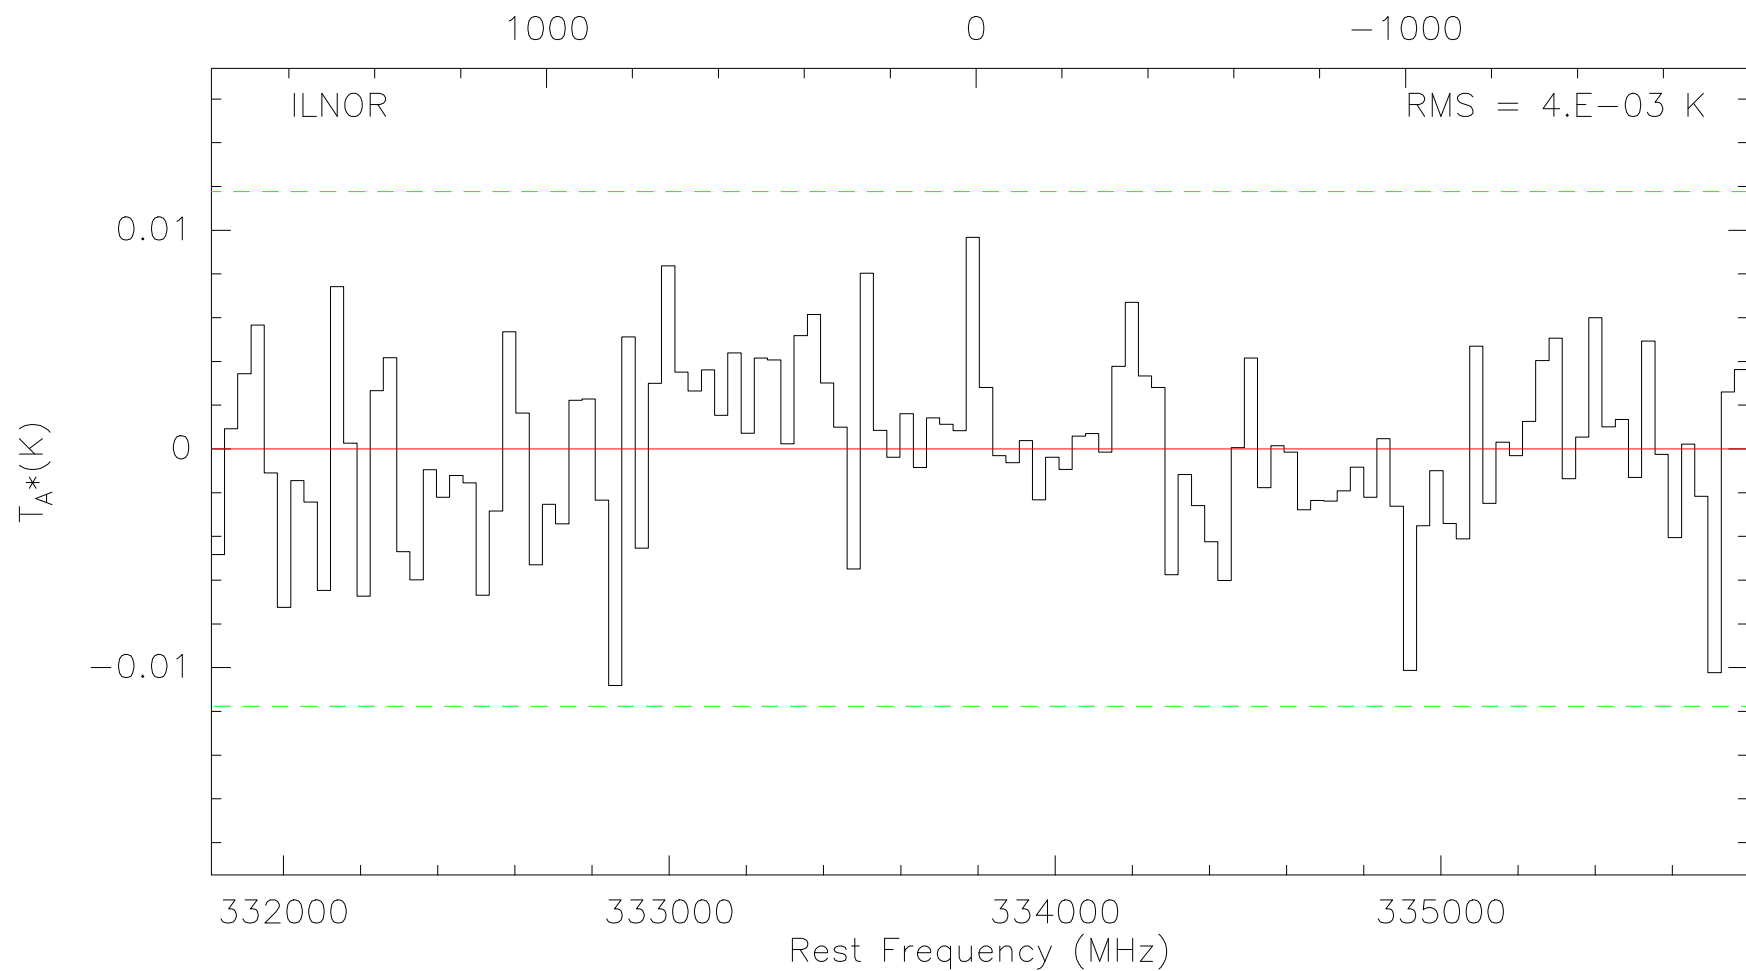

1;1 IMNOR CO(3-2) OSB AP-F301-XF0- 0:07-JUL-2016 R:07-AUG-2020  
RA: 15:39:26.46 DEC: -52:19:17.9 Eq 2000.0 Rad. 0.0° Offs: -0.2 -0.5  
Unknown tau: 0.271 Tsys: 241. Time: 9.9min El: 54.7  
N: 116 IO: 58.7548 V0: 0.000 Dv: 30.84 LSR  
FO: 333795.375 Df: -34.33 Fi: 345795.990

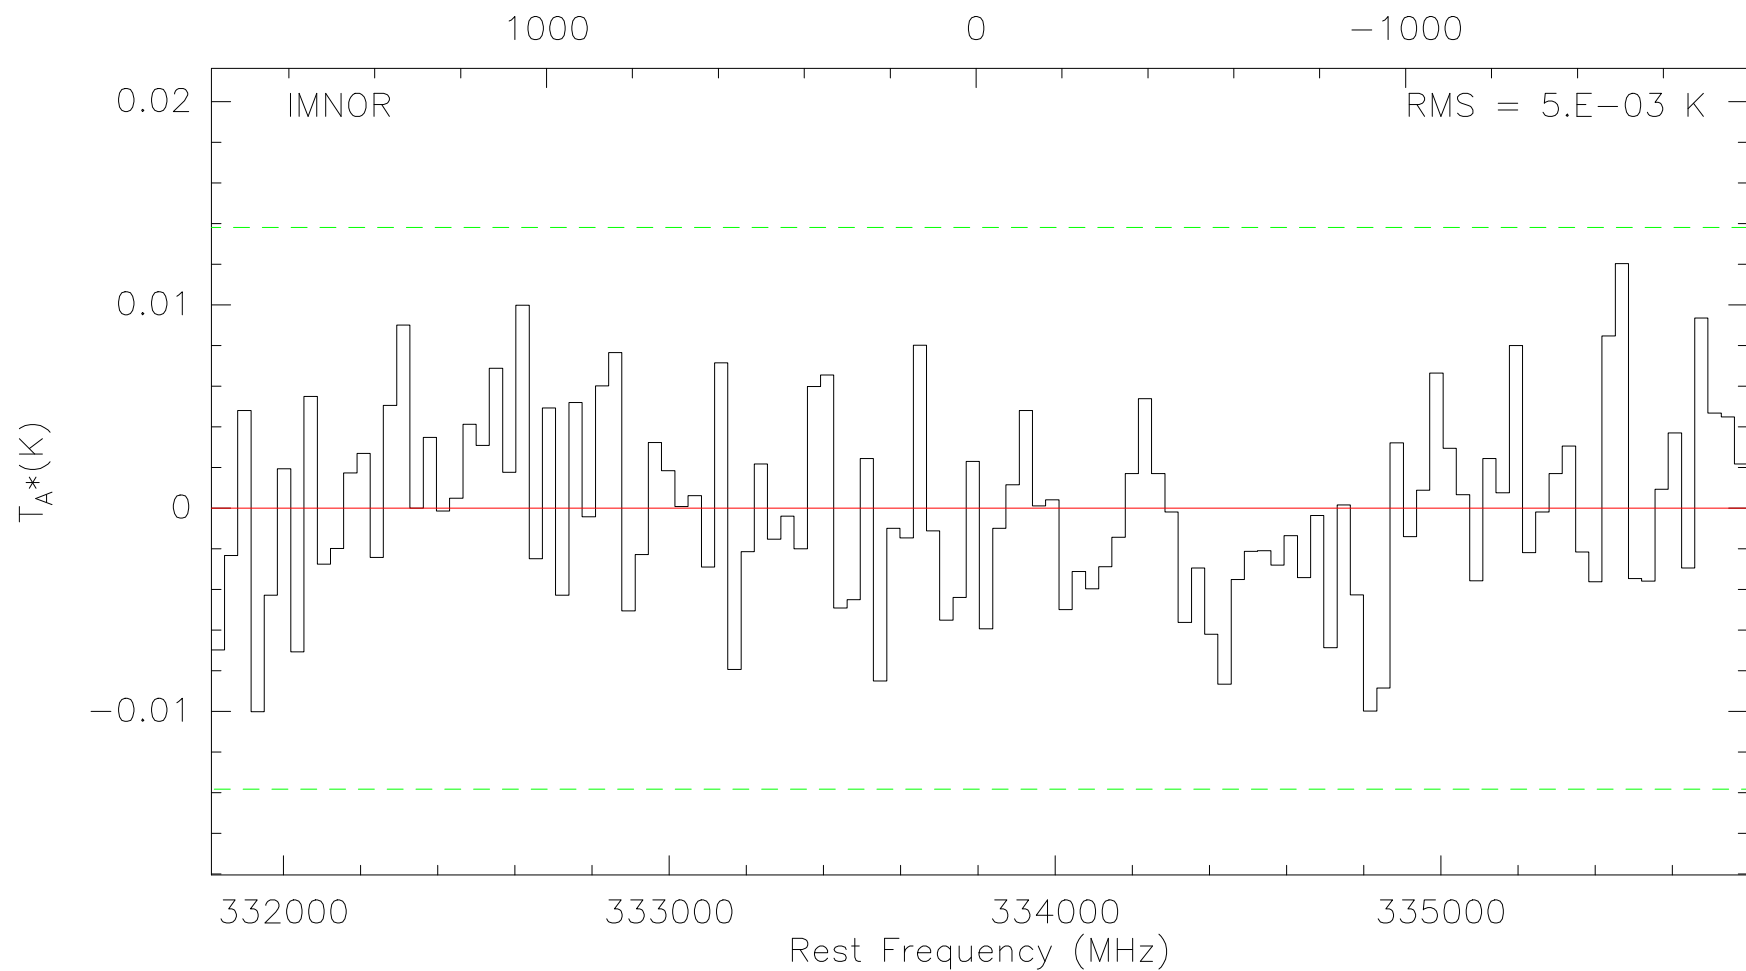

1;1 MTCEN CO(3-2) OSB AP-F301-XF0- O:01-JUL-2016 R:07-AUG-2020  
RA: 11:44:00.80 DEC: -60:33:39.5 Eq 2000.0 Rad. 0.0° Offs: +0.3 -0.5  
Unknown tau: 0.256 Tsys: 275. Time: 24.8min El: 46.2  
N: 116 IO: 58.7547 V0: 0.000 Dv: 30.84 LSR  
FO: 333794.986 Df: -34.34 Fi: 345795.990

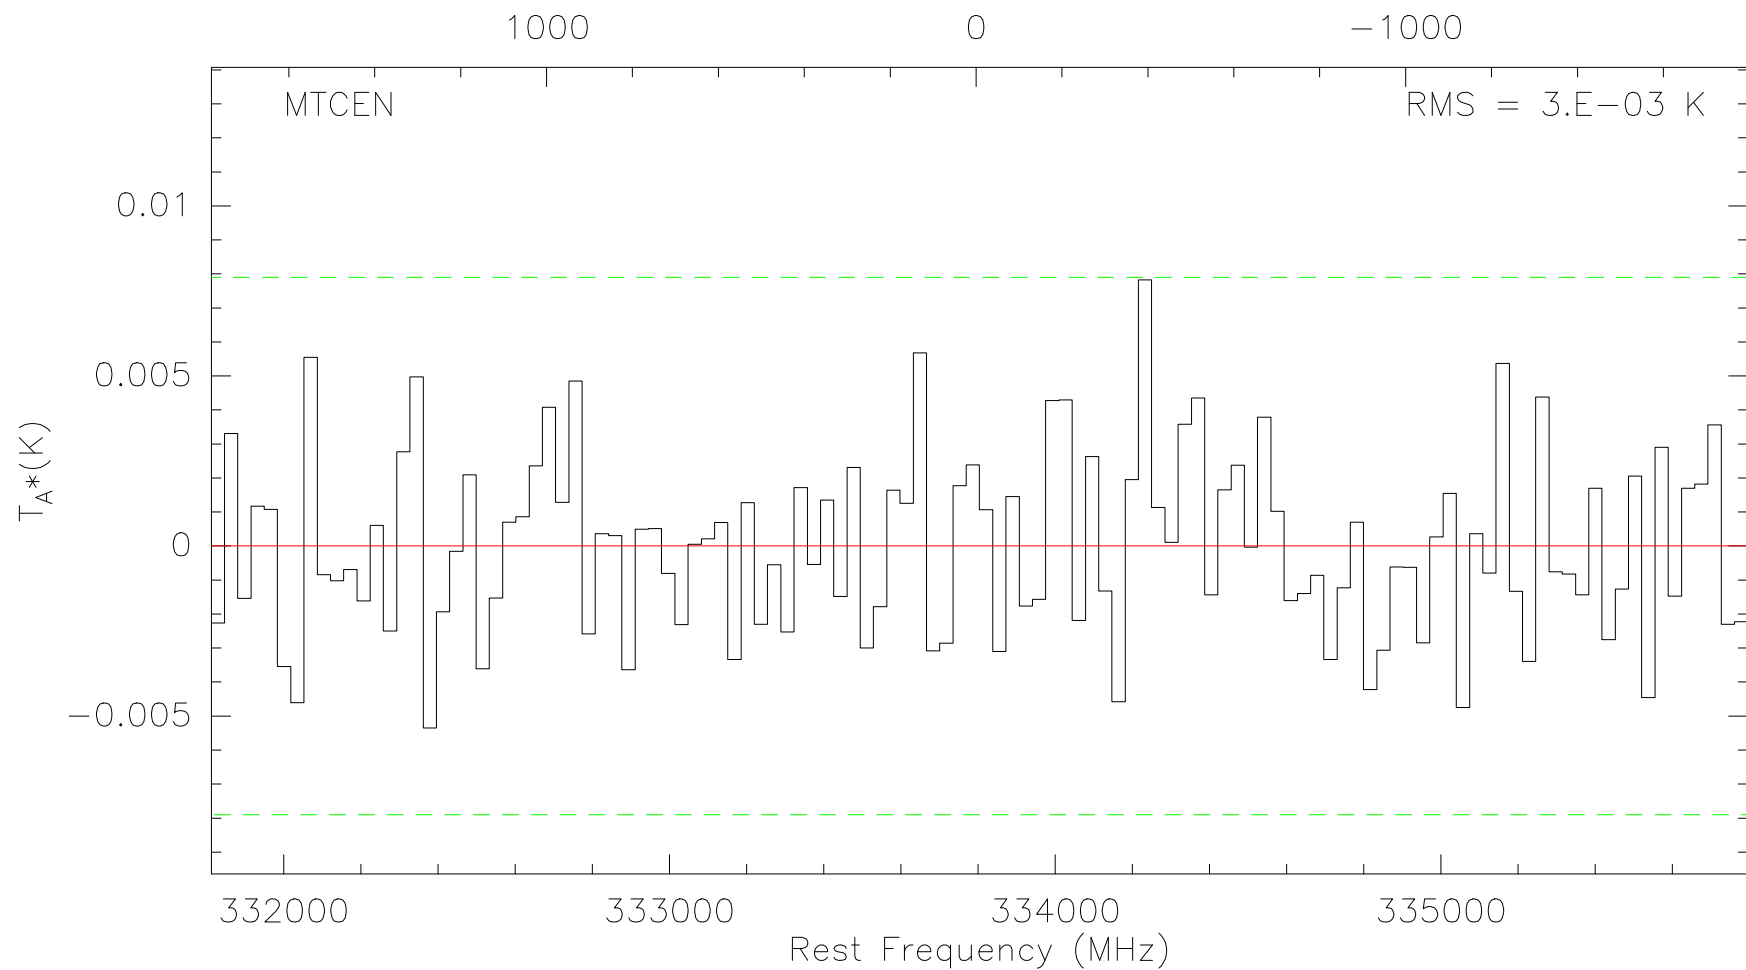

1;1 RSCAR CO(3-2) OSB AP-F301-XF0- 0:30-JUN-2016 R:07-AUG-2020  
RA: 11:08:06.63 DEC: -61:56:04.6 Eq 2000.0 Rad. 0.0° Offs: +0.3 -0.6  
Unknown tau: 0.257 Tsys: 260. Time: 19.8min El: 47.6  
N: 116 IO: 58.7548 V0: 0.000 Dv: 30.84 LSR  
FO: 333794.980 Df: -34.34 Fi: 345795.990

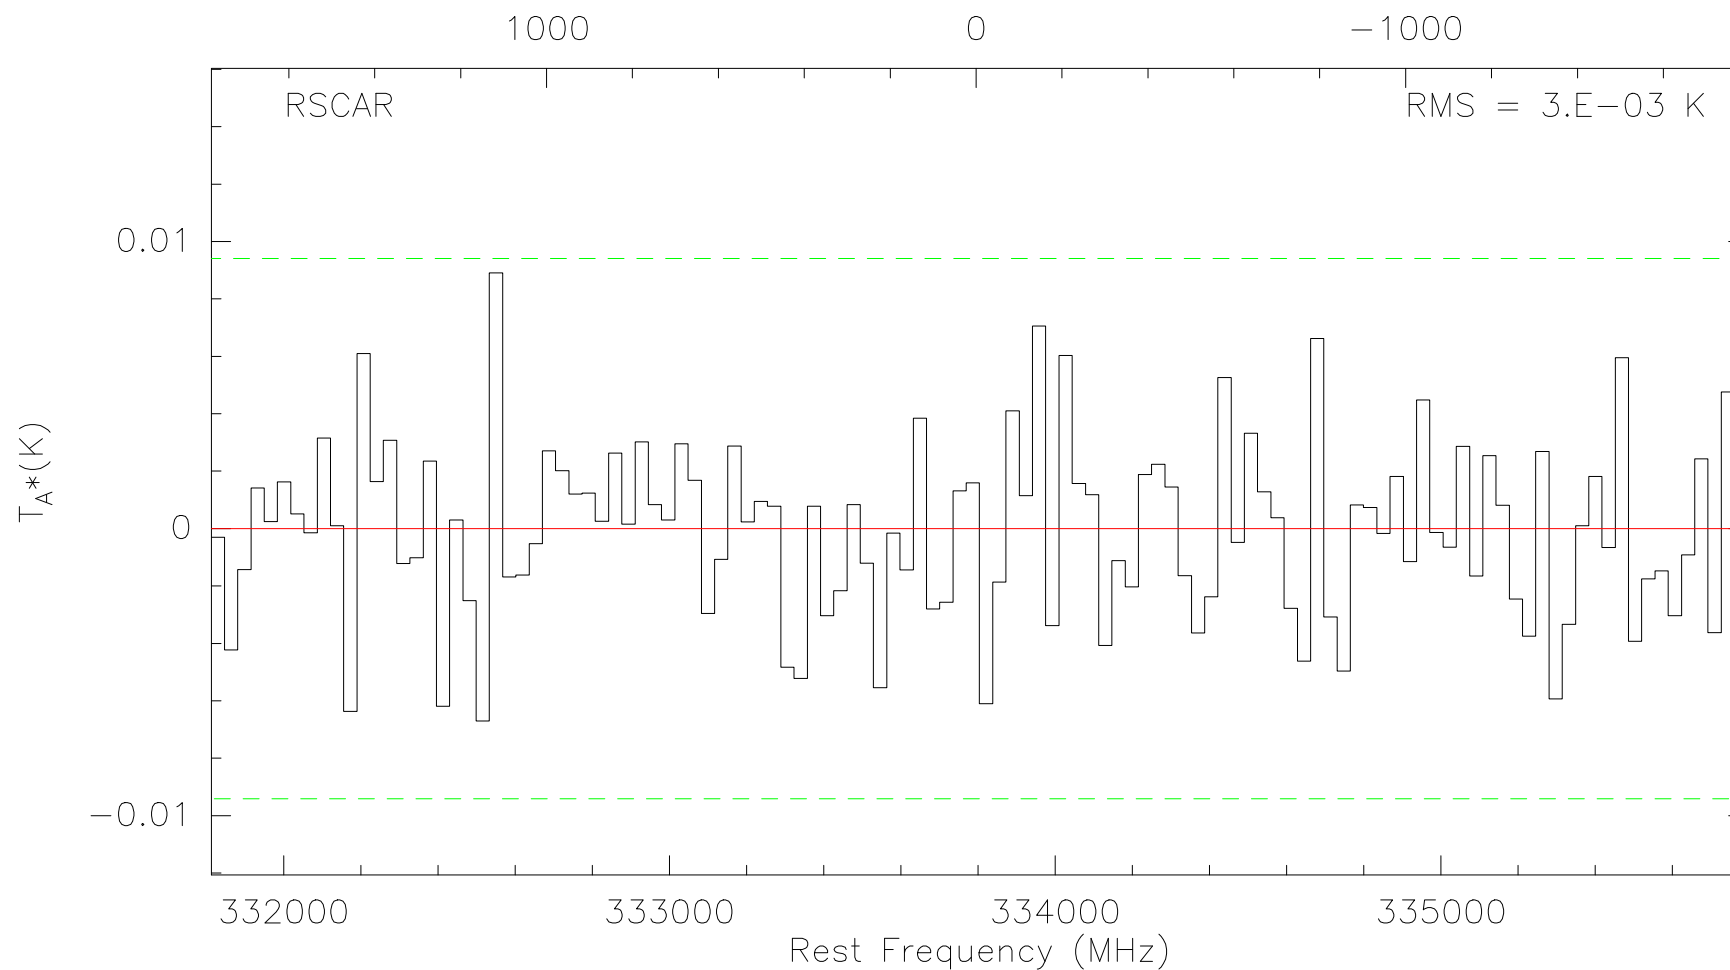

1;1 V1015SGR CO(3-2) OSB AP-F301-XF0- O:13-JUL-2016 R:07-AUG-2020  
RA: 18:09:02.00 DEC: -32:28:32.0 Eq 2000.0 Rad. 0.0° Offs: +0.3 -0.3  
Unknown tau: 0.254 Tsys: 271. Time: 19.8min El: 45.6  
N: 116 lO: 58.7542 V0: 0.000 Dv: 30.83 LSR  
FO: 333796.108 Df: -34.33 Fi: 345795.990

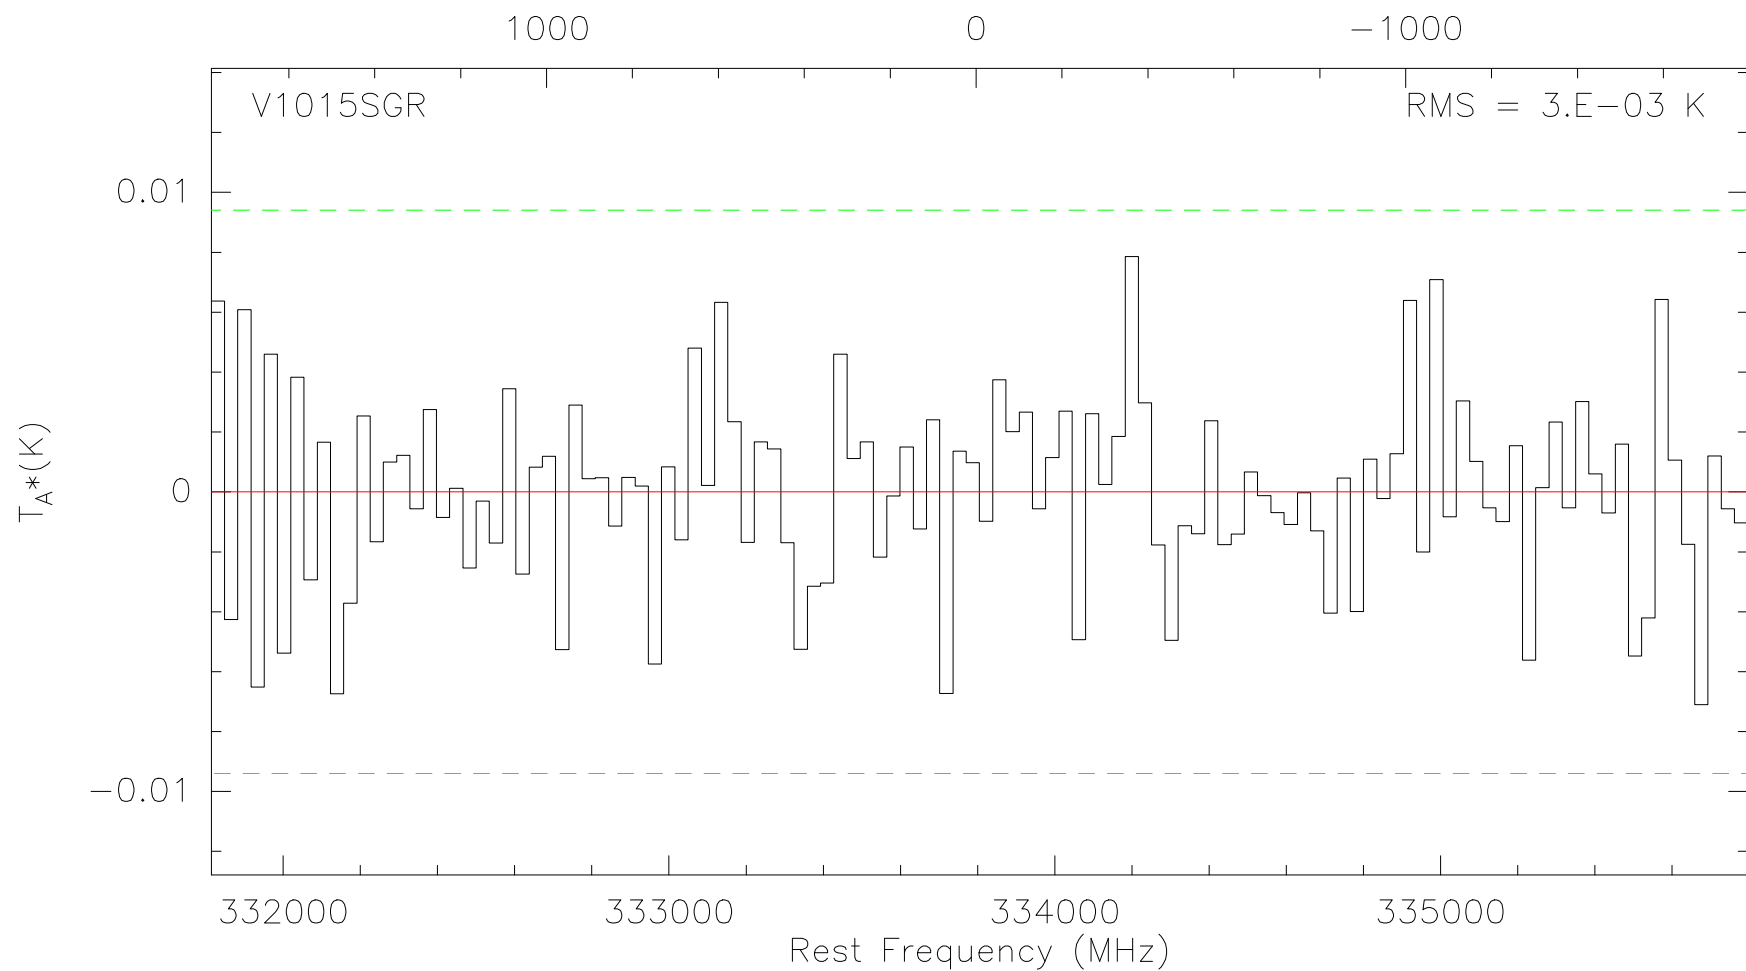

1;1 V1016SGR CO(3-2) OSB AP-F301-XF0- O:13-JUL-2016 R:07-AUG-2020  
RA: 18:19:57.63 DEC: -25:11:14.6 Eq 2000.0 Rad. 0.0° Offs: -0.2 -0.3  
Unknown tau: 0.181 Tsys: 241. Time: 9.9min El: 32.1  
N: 116 lO: 58.7548 V0: 0.000 Dv: 30.83 LSR  
FO: 333796.094 Df: -34.33 Fi: 345795.990

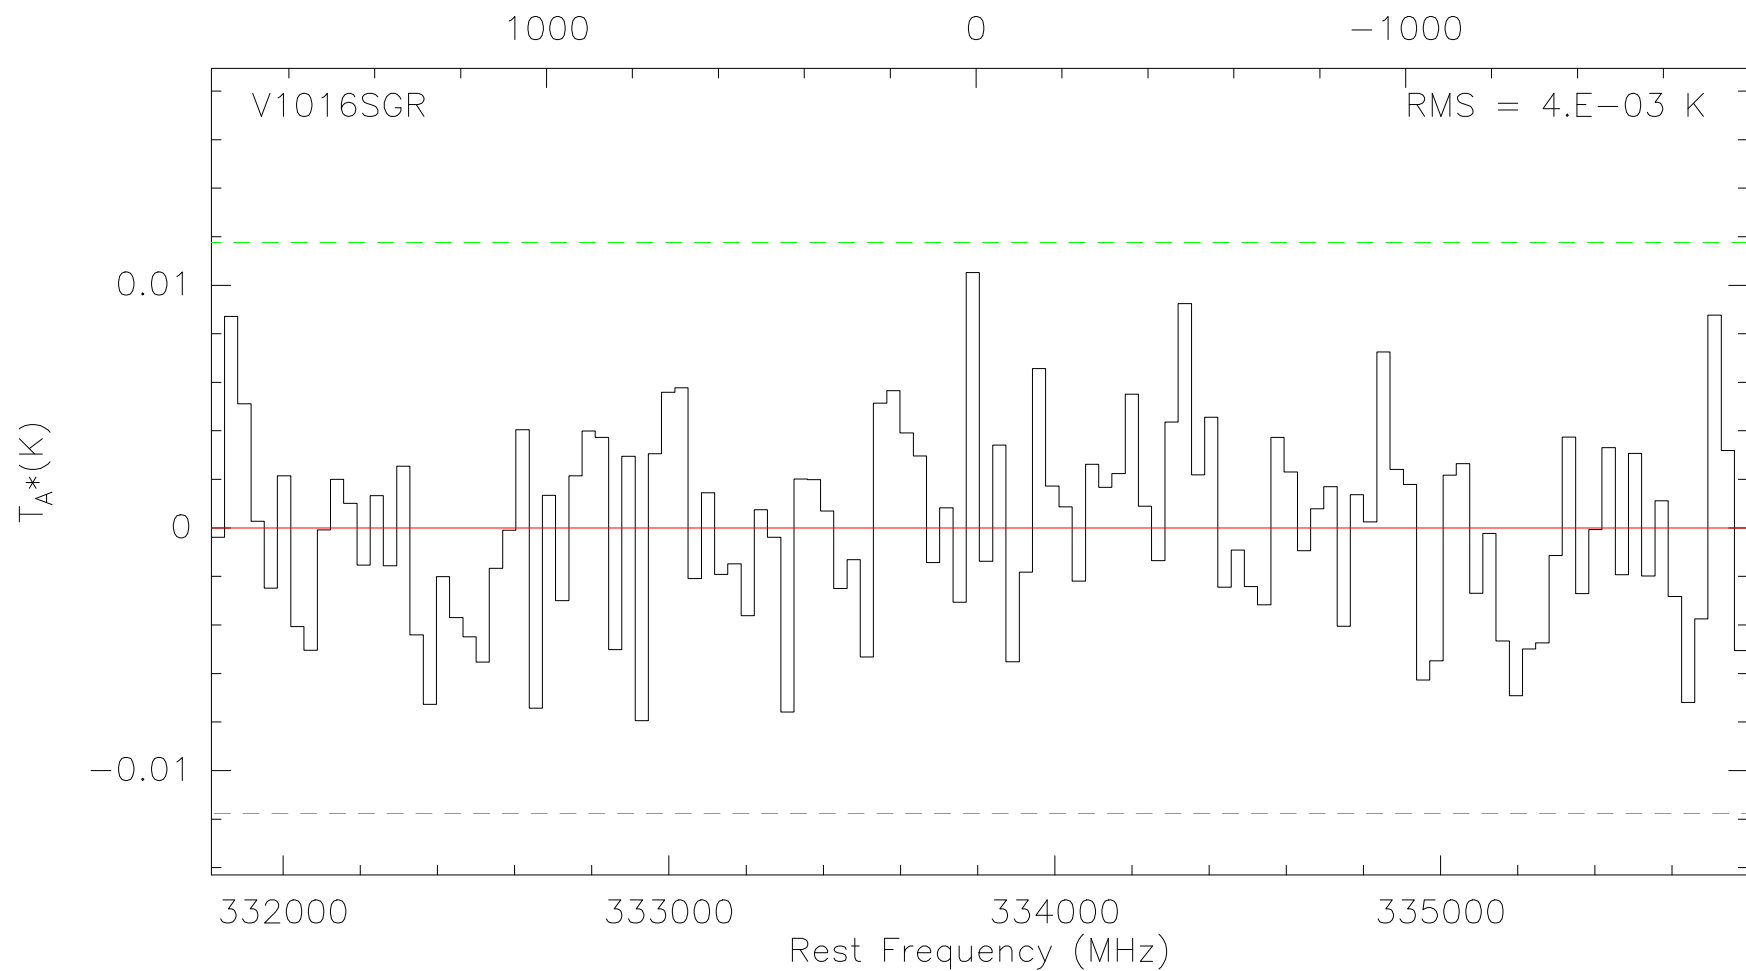

1;1 V1017SGR CO(3-2) OSB AP-F301-XF0- O:13-JUL-2016 R:07-AUG-2020  
RA: 18:32:04.47 DEC: -29:23:12.5 Eq 2000.0 Rad. 0.0° Offs: +0.4 -0.4  
Unknown tau: 0.258 Tsys: 210. Time: 14.9min El: 75.2  
N: 116 IO: 58.7548 V0: 0.000 Dv: 30.83 LSR  
FO: 333796.115 Df: -34.33 Fi: 345795.990

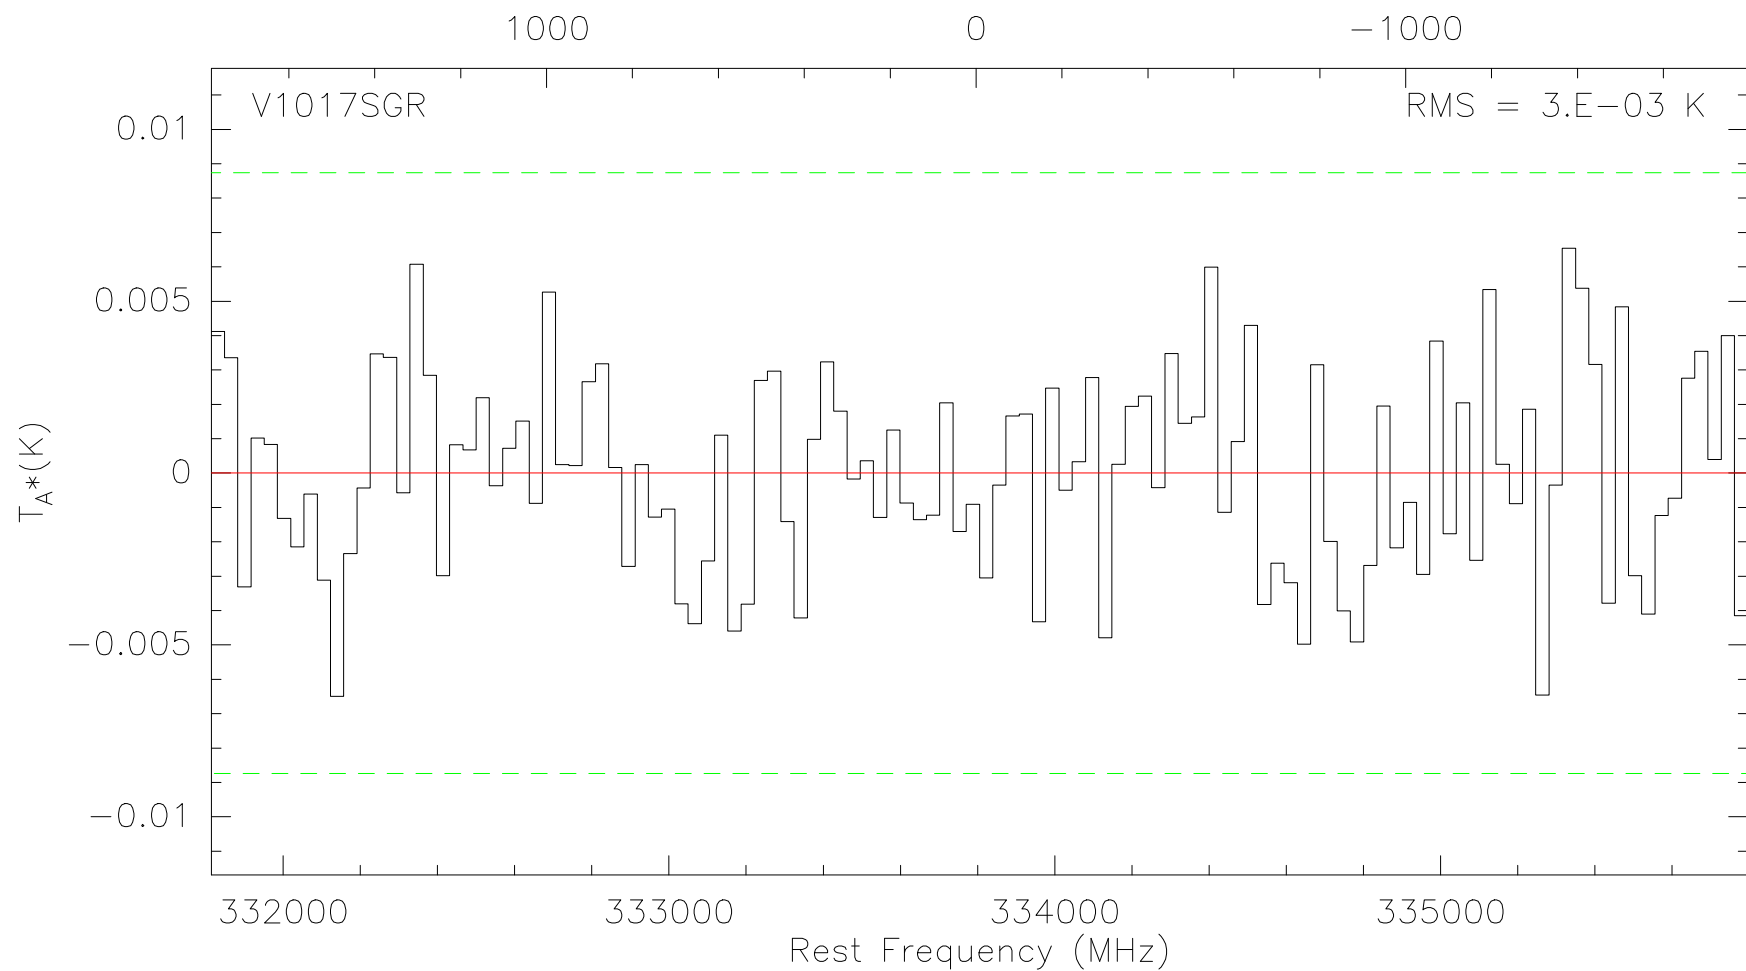

1;1 V1149SGR CO(3-2) OSB AP-F301-XF0- O:13-JUL-2016 R:07-AUG-2020  
RA: 18:18:30.40 DEC: -28:17:17.0 Eq 2000.0 Rad. 0.0° Offs: -0.2 -0.6  
Unknown tau: 0.202 Tsys: 194. Time: 9.9min El: 61.7  
N: 116 IO: 58.7548 V0: 0.000 Dv: 30.83 LSR  
F0: 333796.059 Df: -34.33 Fi: 345795.990

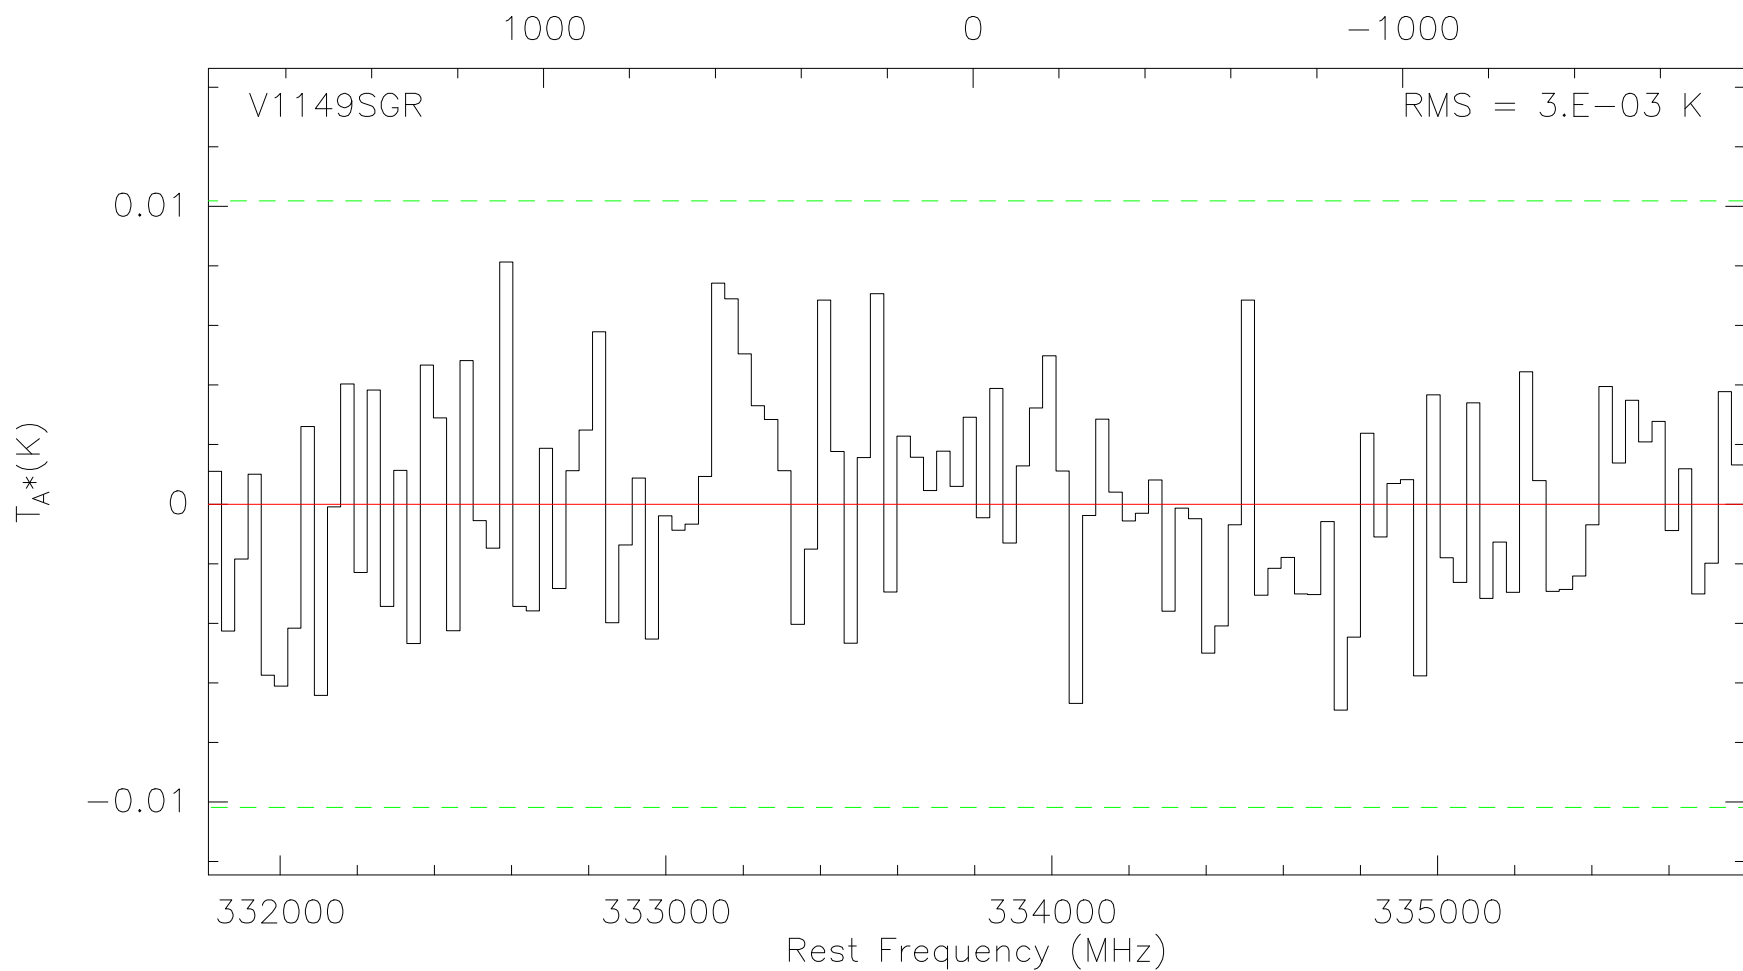

1;1 V1151SGR CO(3-2) OSB AP-F301-XF0- O:14-JUL-2016 R:07-AUG-2020  
RA: 18:25:23.75 DEC: -20:11:59.3 Eq 2000.0 Rad. 0.0° Offs: -0.2 -0.3  
Unknown tau: 0.194 Tsys: 283. Time: 9.9min El: 26.8  
N: 116 IO: 58.7548 V0: 0.000 Dv: 30.83 LSR  
FO: 333796.156 Df: -34.33 Fi: 345795.990

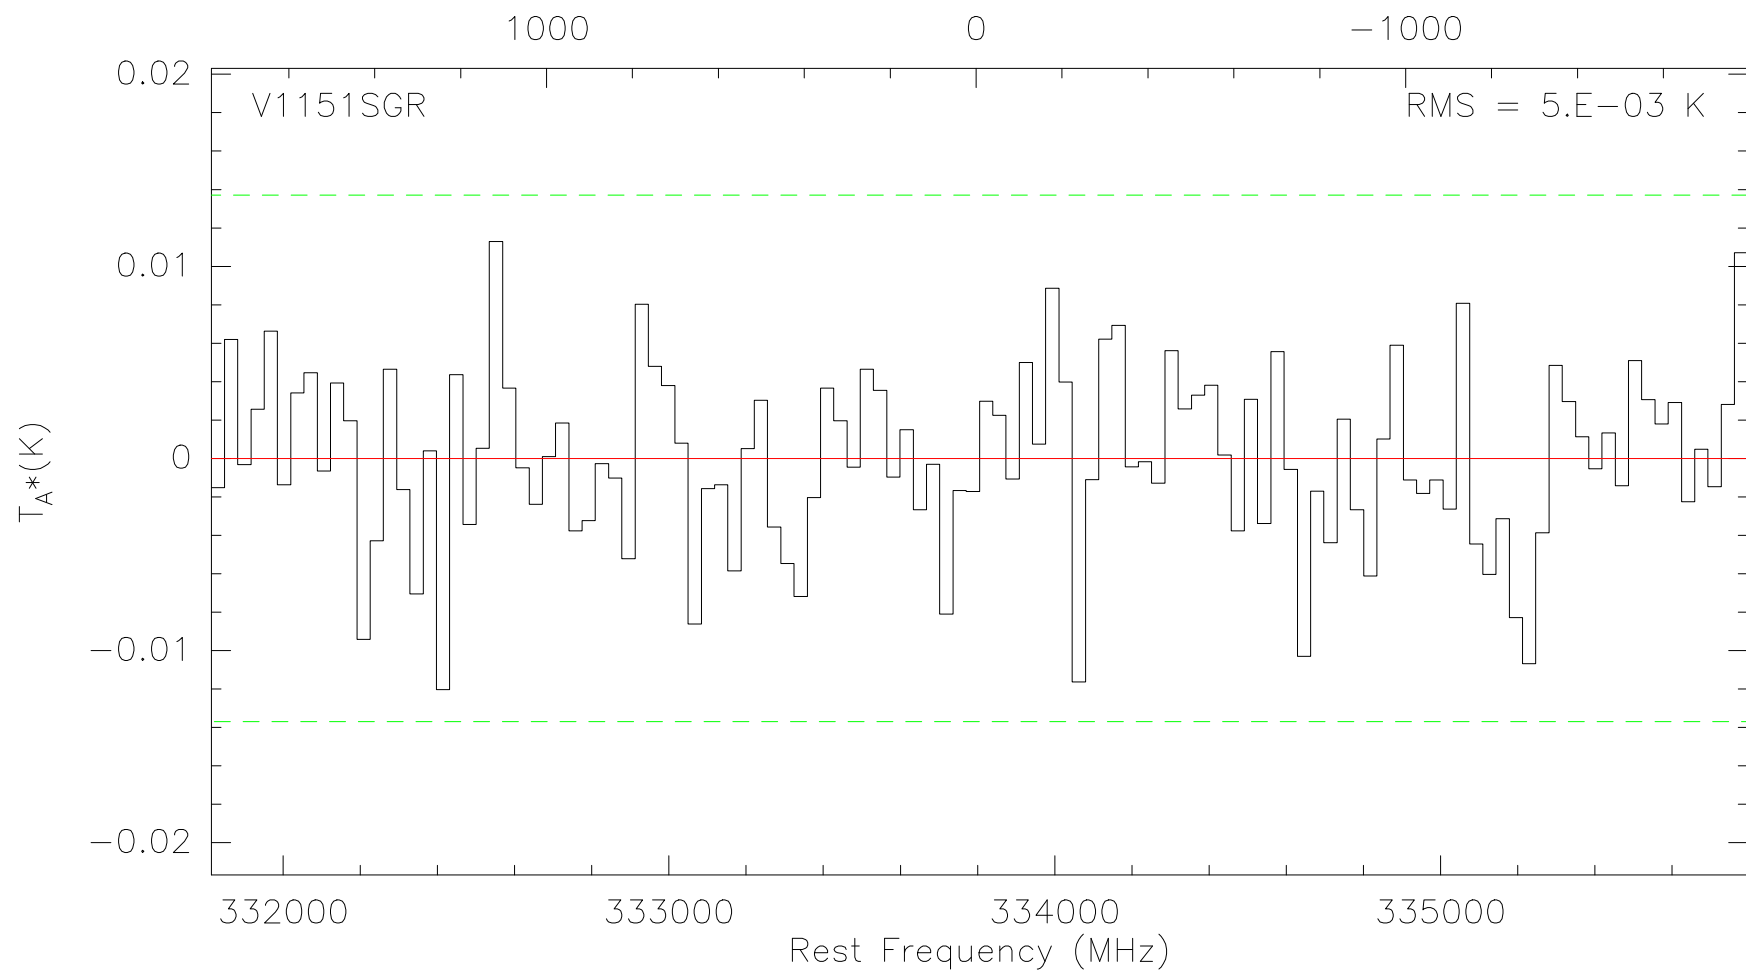

1;1 V1583SGR CO(3-2) OSB AP-F301-XF0- O:14-JUL-2016 R:07-AUG-2020  
RA: 18:15:26.30 DEC: -23:23:18.0 Eq 2000.0 Rad. 0.0° Offs: -0.2 -0.3  
Unknown tau: 0.202 Tsys: 269. Time: 9.9min El: 30.0  
N: 116 IO: 58.7548 V0: 0.000 Dv: 30.83 LSR  
FO: 333796.076 Df: -34.33 Fi: 345795.990

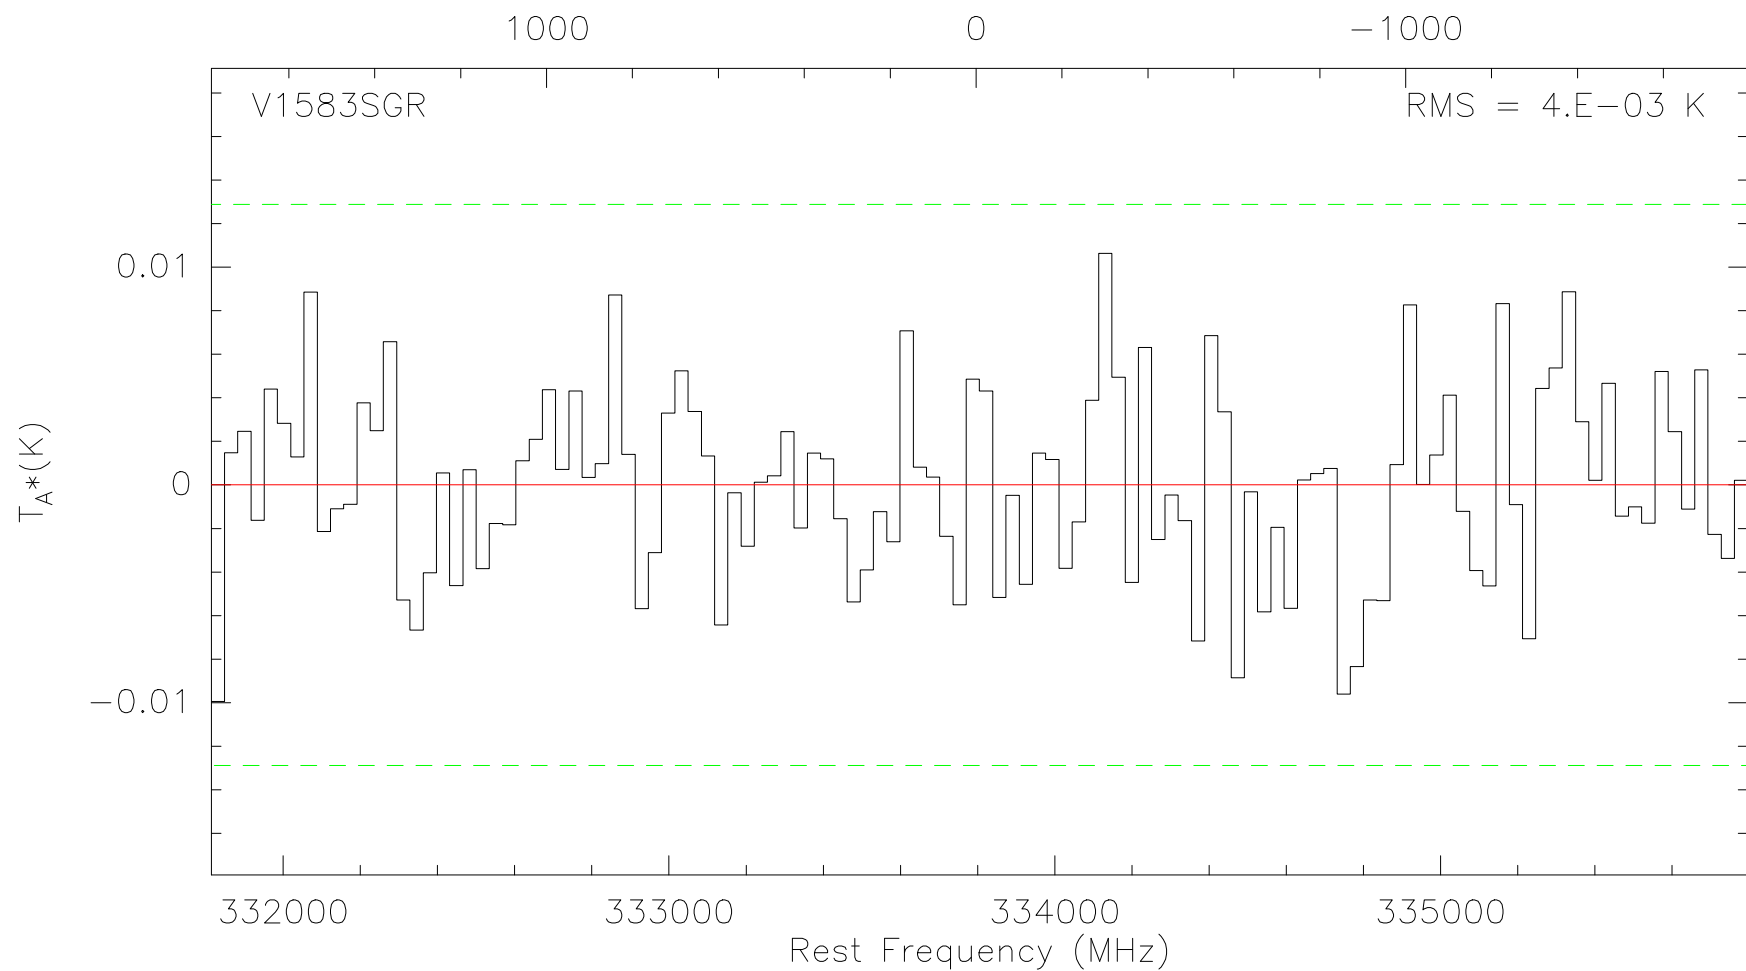

1;1 V363SGR CO(3-2) OSB AP-F301-XF0- 0:01-JUL-2016 R:07-AUG-2020  
RA: 19:11:16.30 DEC: -29:50:00.0 Eq 2000.0 Rad. 0.0° Offs: -0.2 -0.6  
Unknown tau: 0.418 Tsys: 391. Time: 19.9min El: 42.0  
N: 116 IO: 58.7548 V0: 0.000 Dv: 30.83 LSR  
FO: 333796.475 Df: -34.33 Fi: 345795.990

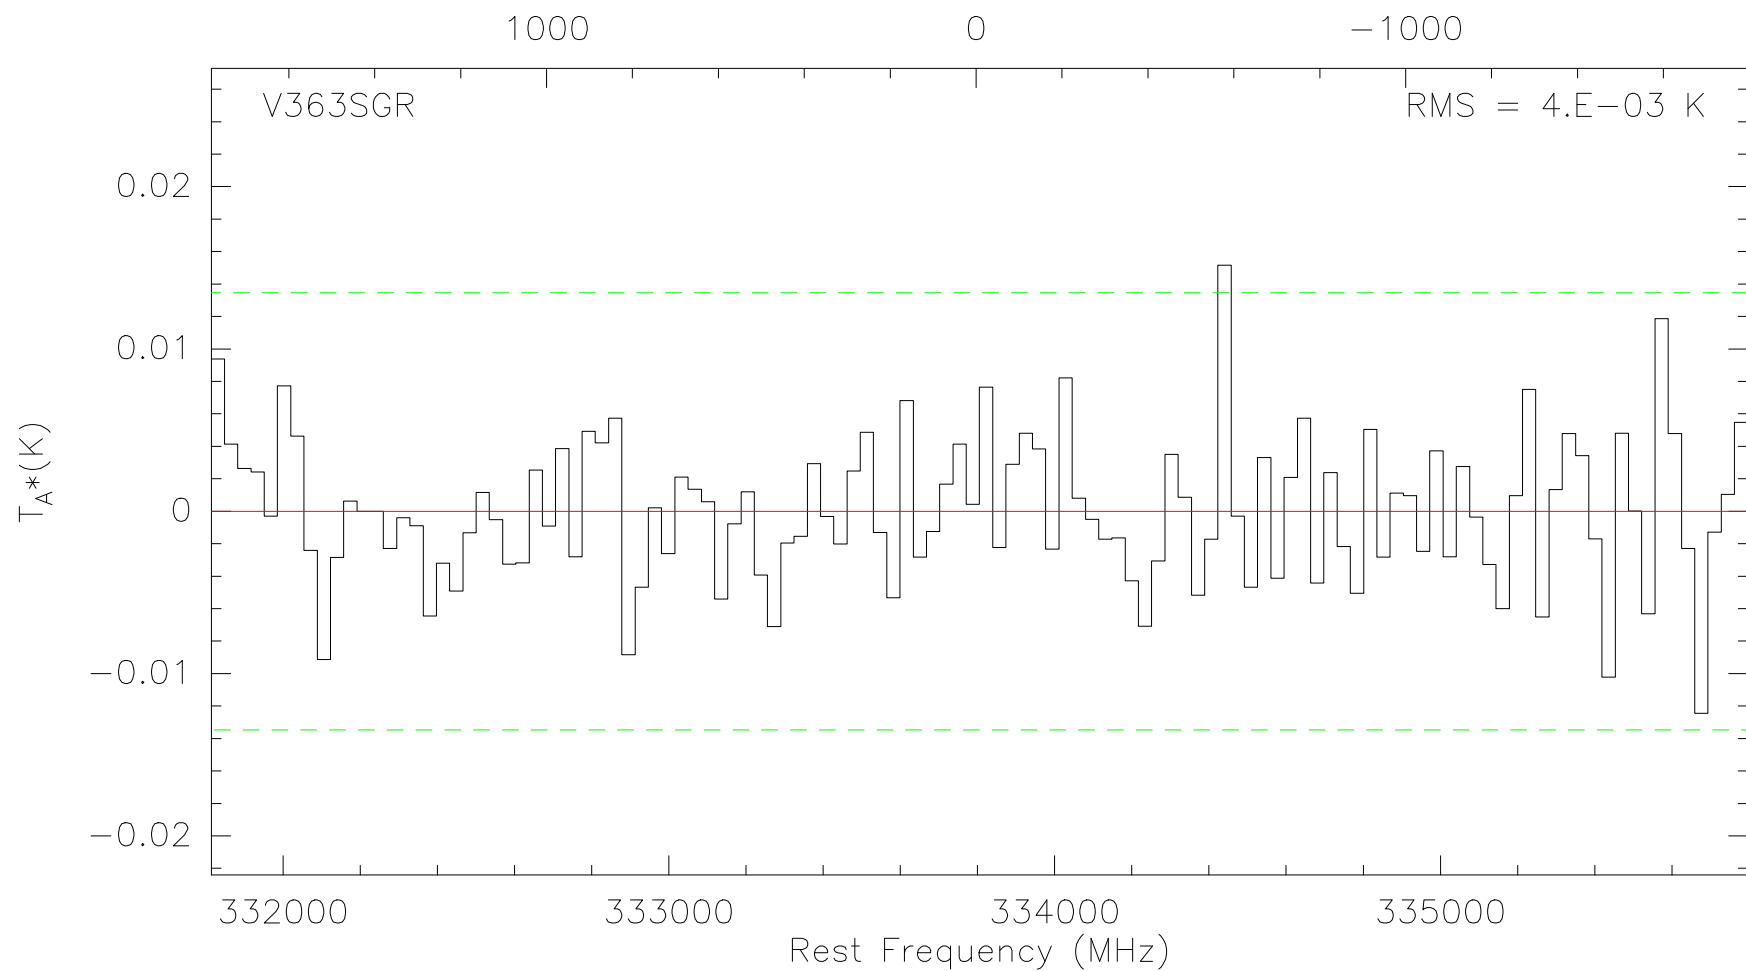

1;1 V365CAR CO(3-2) OSB AP-F301-XF0- 0:30-JUN-2016 R:07-AUG-2020  
RA: 11:03:16.77 DEC: -58:27:24.9 Eq 2000.0 Rad. 0.0° Offs: +0.3 -0.5  
Unknown tau: 0.251 Tsys: 249. Time: 19.8min El: 51.3  
N: 116 IO: 58.7548 V0: 0.000 Dv: 30.84 LSR  
FO: 333794.926 Df: -34.34 Fi: 345795.990

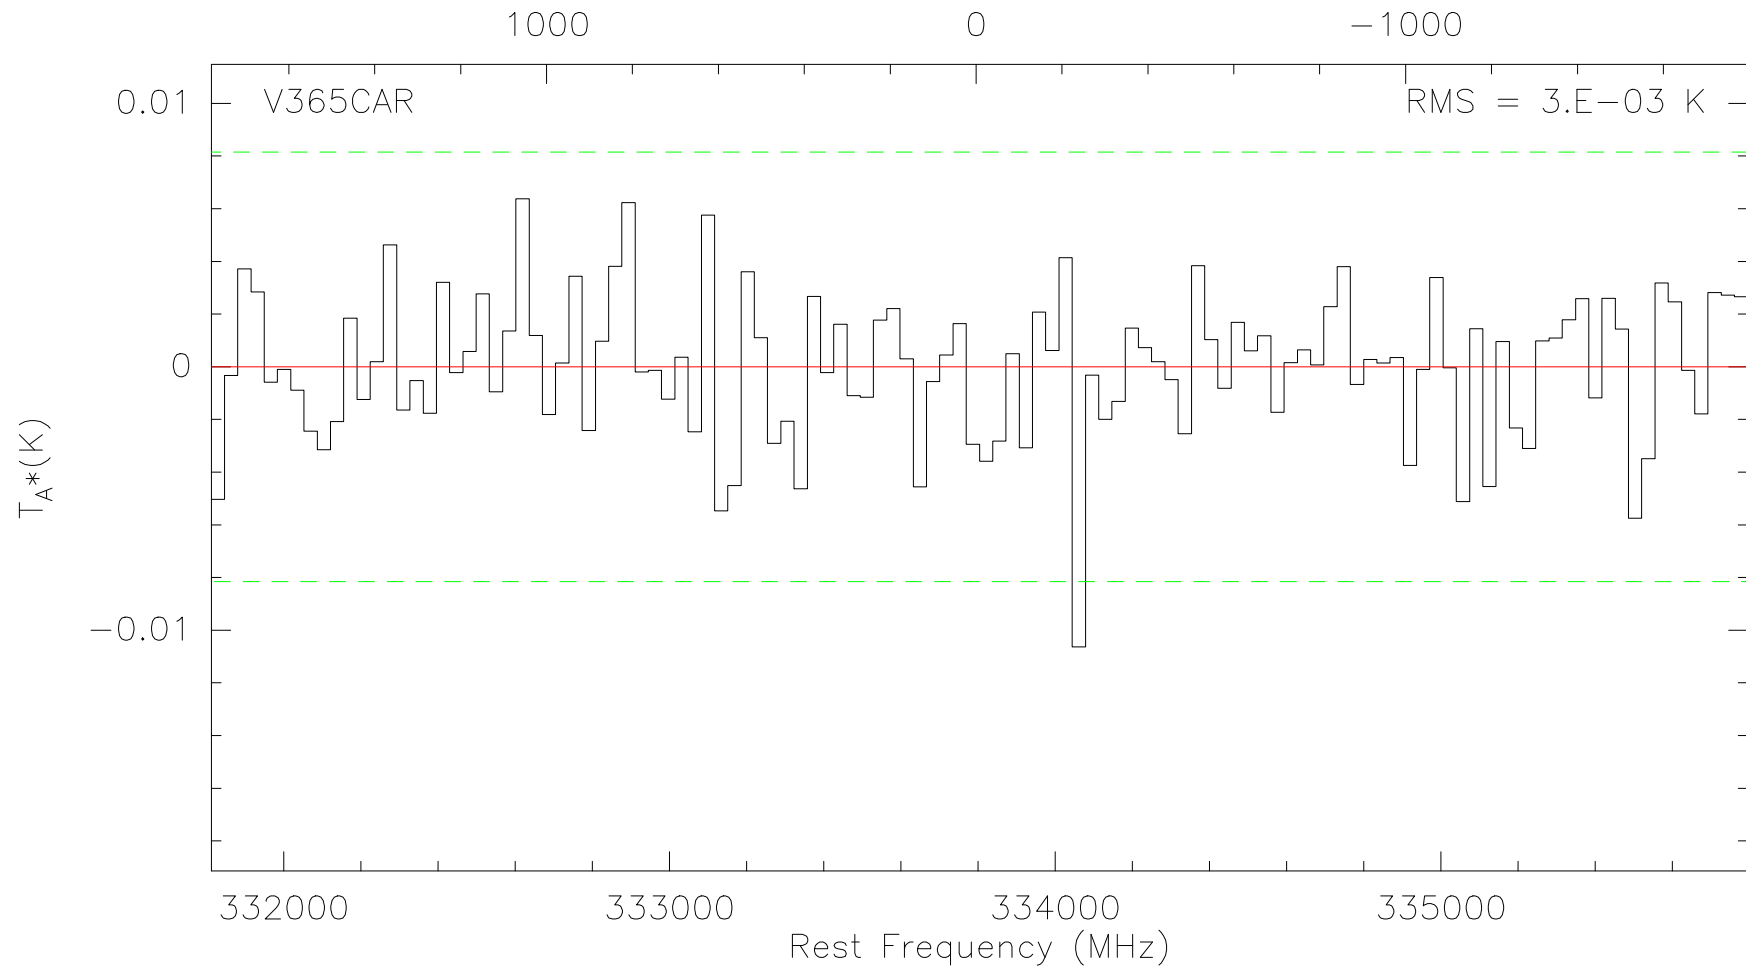

1;1 V382SCO CO(3-2) OSB AP-F301-XF0- 0:13-JUL-2016 R:07-AUG-2020  
RA: 17:51:56.13 DEC: -35:25:05.4 Eq 2000.0 Rad. 0.0° Offs: +0.1 -0.6  
Unknown tau: 0.205 Tsys: 187. Time: 9.9min El: 72.8  
N: 116 IO: 58.7548 V0: 0.000 Dv: 30.84 LSR  
F0: 333795.875 Df: -34.33 Fi: 345795.990

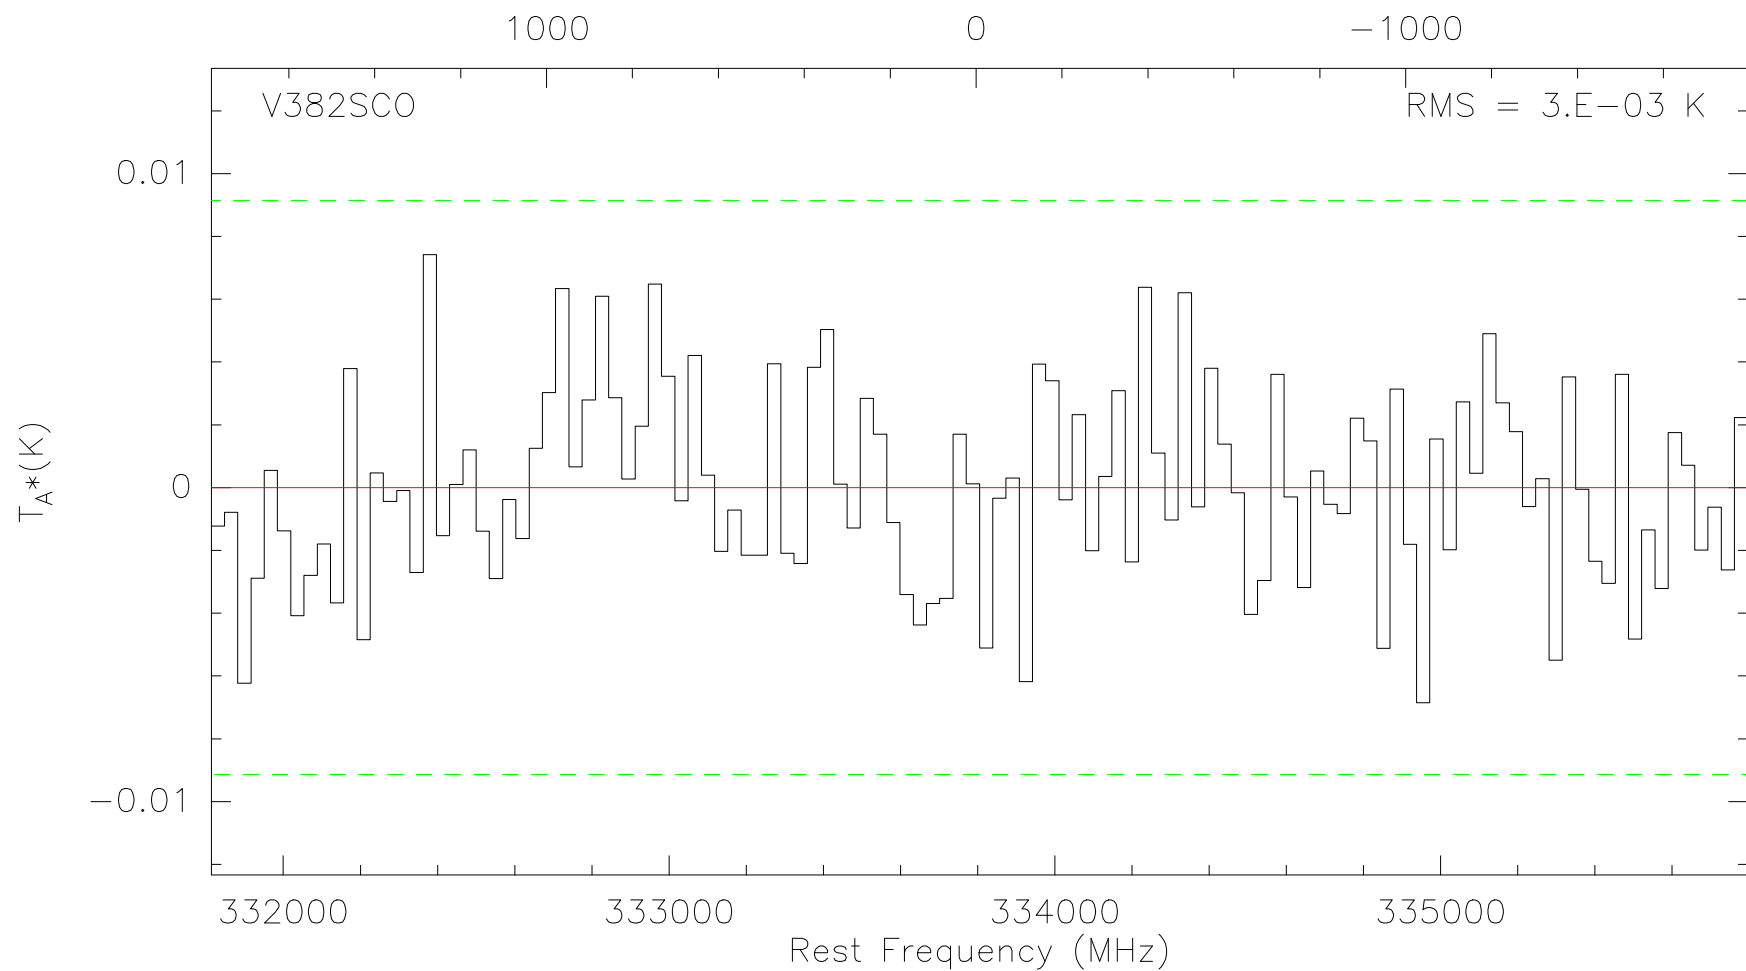

1;1 V384SCO CO(3-2) OSB AP-F301-XF0- 0:14-JUL-2016 R:07-AUG-2020  
RA: 18:01:43.15 DEC: -35:39:27.8 Eq 2000.0 Rad. 0.0° Offs: +0.3 -0.3  
Unknown tau: 0.296 Tsys: 270. Time: 9.9min El: 52.1  
N: 116 IO: 58.7548 V0: 0.000 Dv: 30.84 LSR  
FO: 333795.908 Df: -34.33 Fi: 345795.990

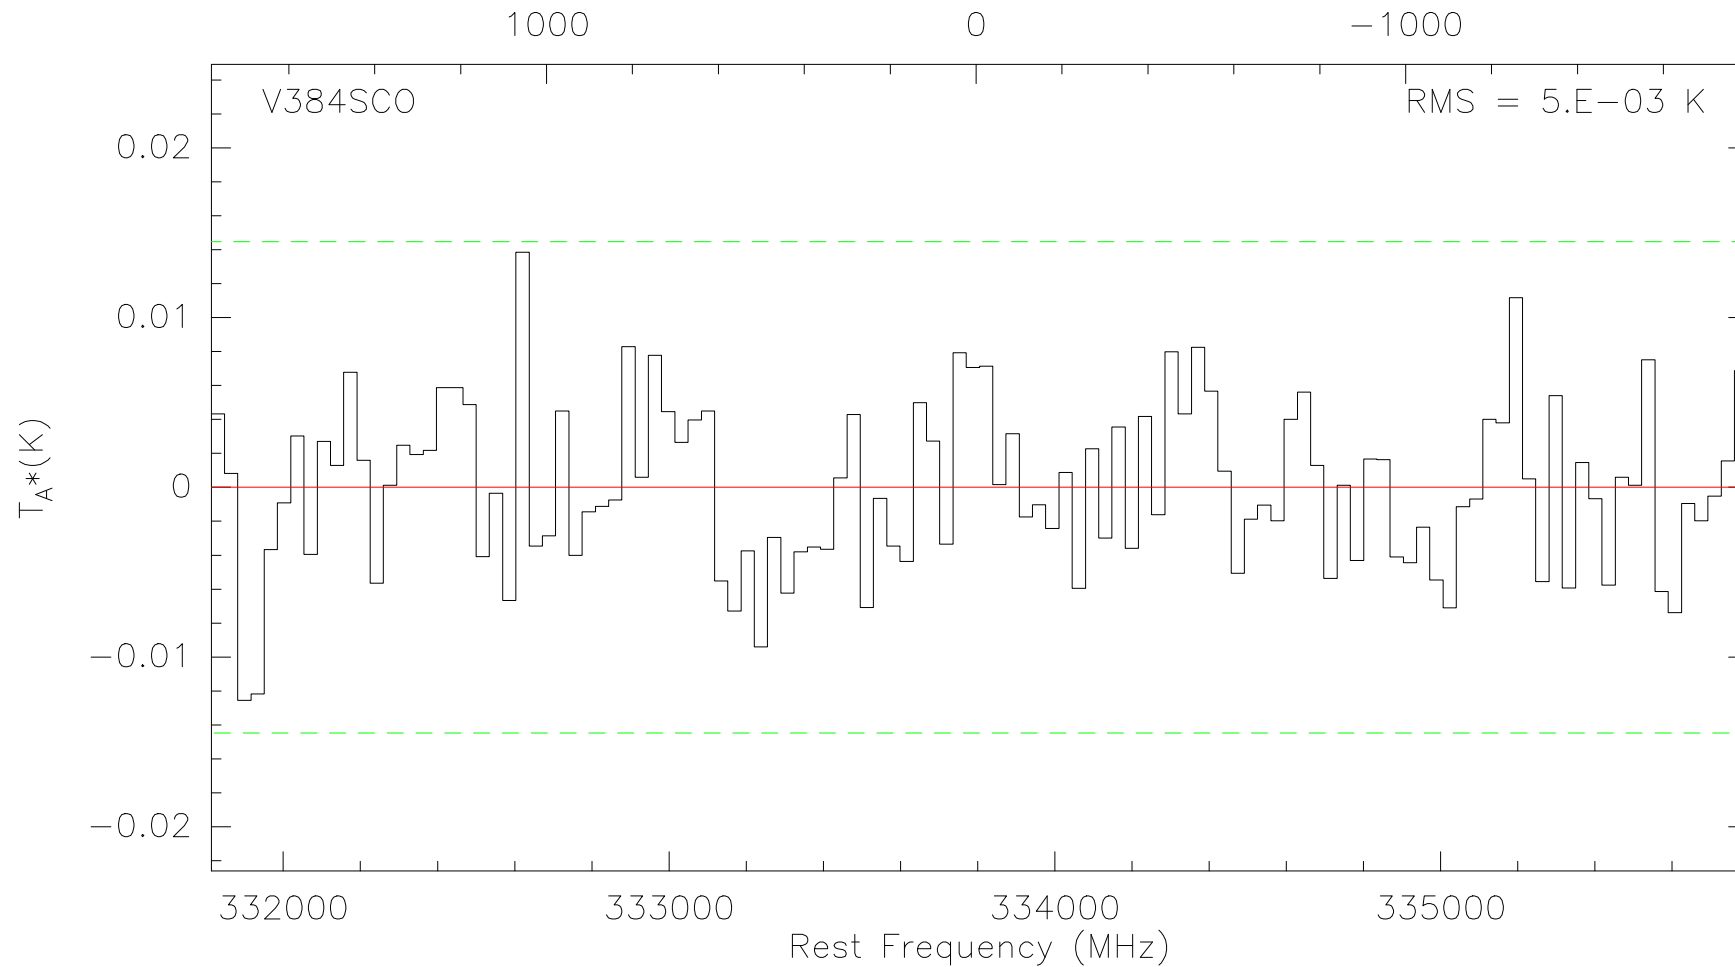

1;1 V522SGR CO(3-2) OSB AP-F301-XF0- 0:01-JUL-2016 R:07-AUG-2020  
RA: 18:48:00.47 DEC: -25:22:21.9 Eq 2000.0 Rad. 0.0° Offs: -0.2 -0.5  
Unknown tau: 0.407 Tsys: 461. Time: 19.8min El: 31.8  
N: 116 IO: 58.7548 V0: 0.000 Dv: 30.83 LSR  
FO: 333796.445 Df: -34.33 Fi: 345795.990

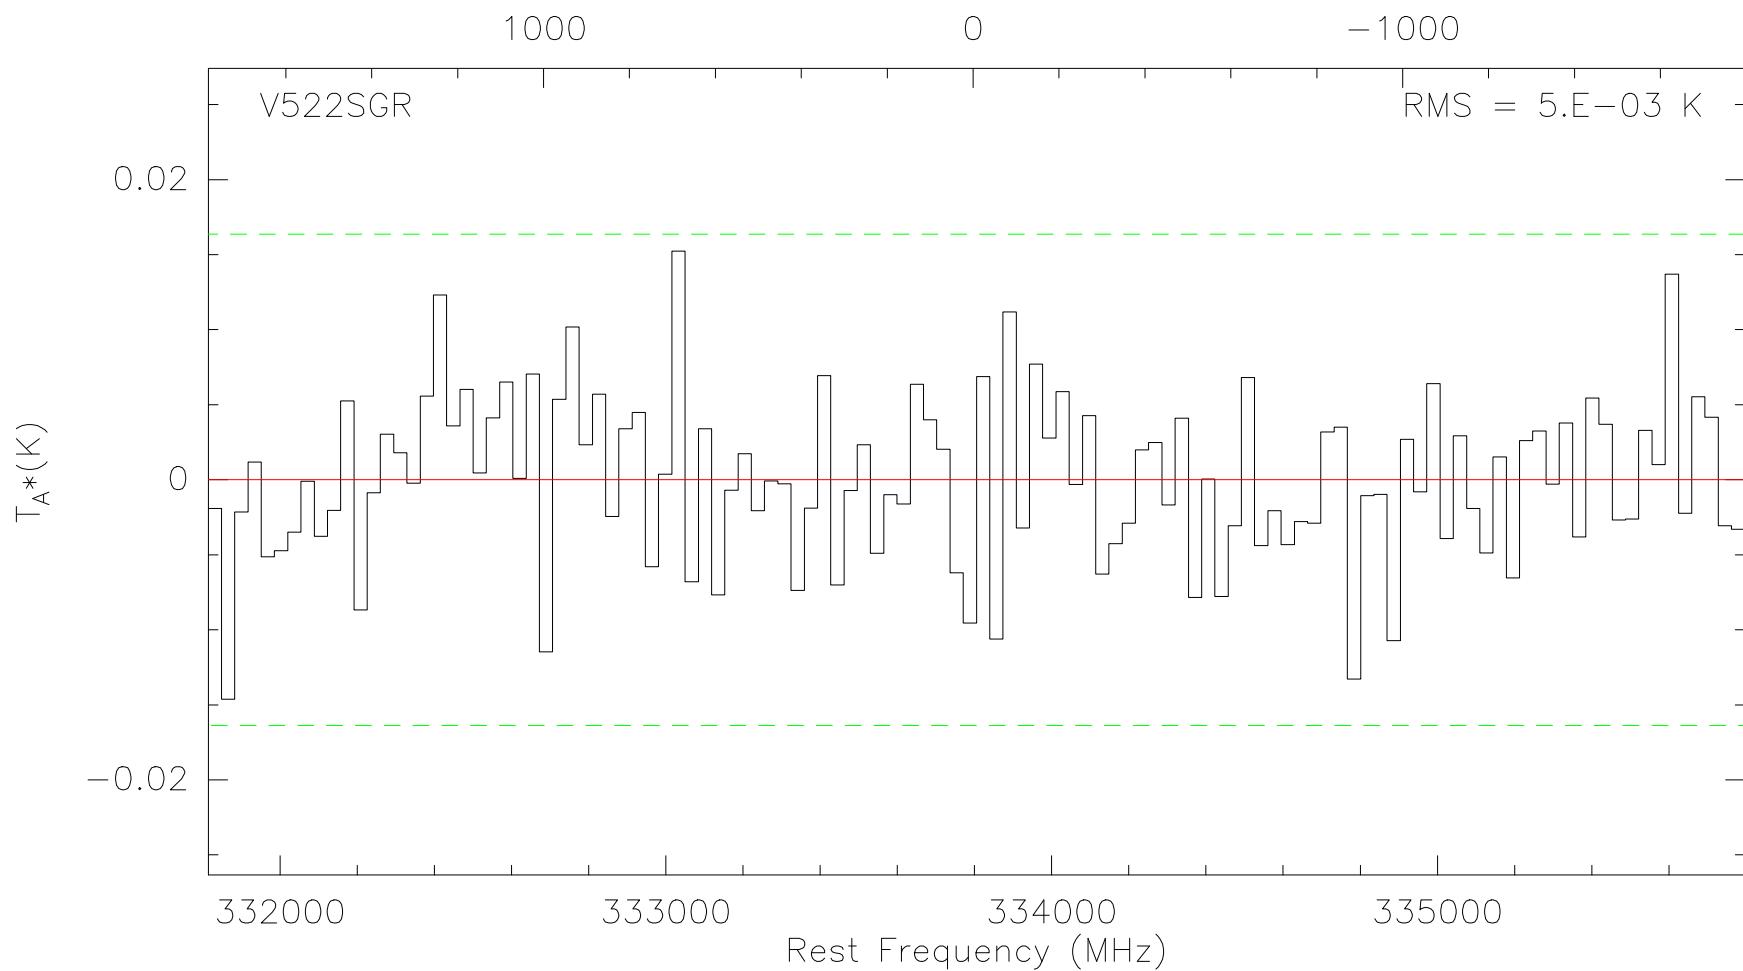

1;1 V5530PH CO(3-2) OSB AP-F301-XF0- 0:01-JUL-2016 R:07-AUG-2020  
RA: 17:42:53.50 DEC: -24:51:26.2 Eq 2000.0 Rad. 0.0° Offs: -0.4 -0.5  
Unknown tau: 0.418 Tsys: 425. Time: 9.9min El: 38.8  
N: 116 IO: 58.7548 V0: 0.000 Dv: 30.83 LSR  
FO: 333796.162 Df: -34.33 Fi: 345795.990

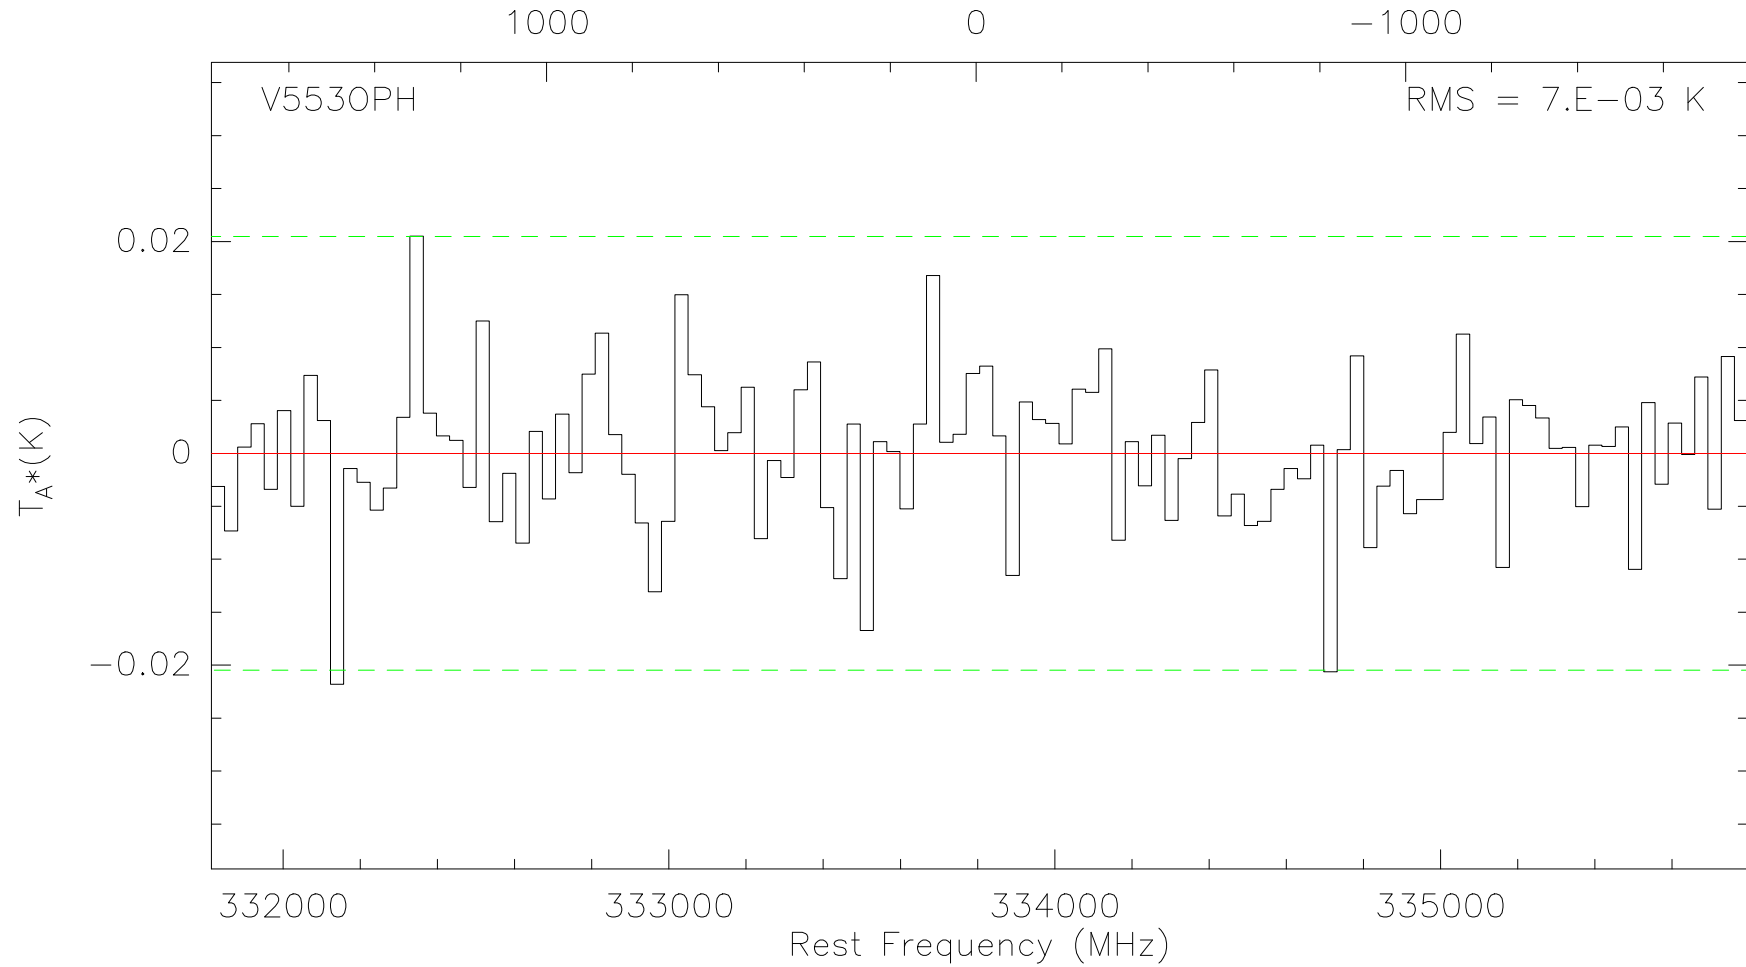

1;1 V696SCO CO(3-2) OSB AP-F301-XF0- O:13-JUL-2016 R:07-AUG-2020  
RA: 17:53:11.55 DEC: -35:50:14.4 Eq 2000.0 Rad. 0.0° Offs: +0.2 -0.6  
Unknown tau: 0.240 Tsys: 200. Time: 9.9min El: 77.1  
N: 116 IO: 58.7548 V0: 0.000 Dv: 30.84 LSR  
FO: 333795.879 Df: -34.33 Fi: 345795.990

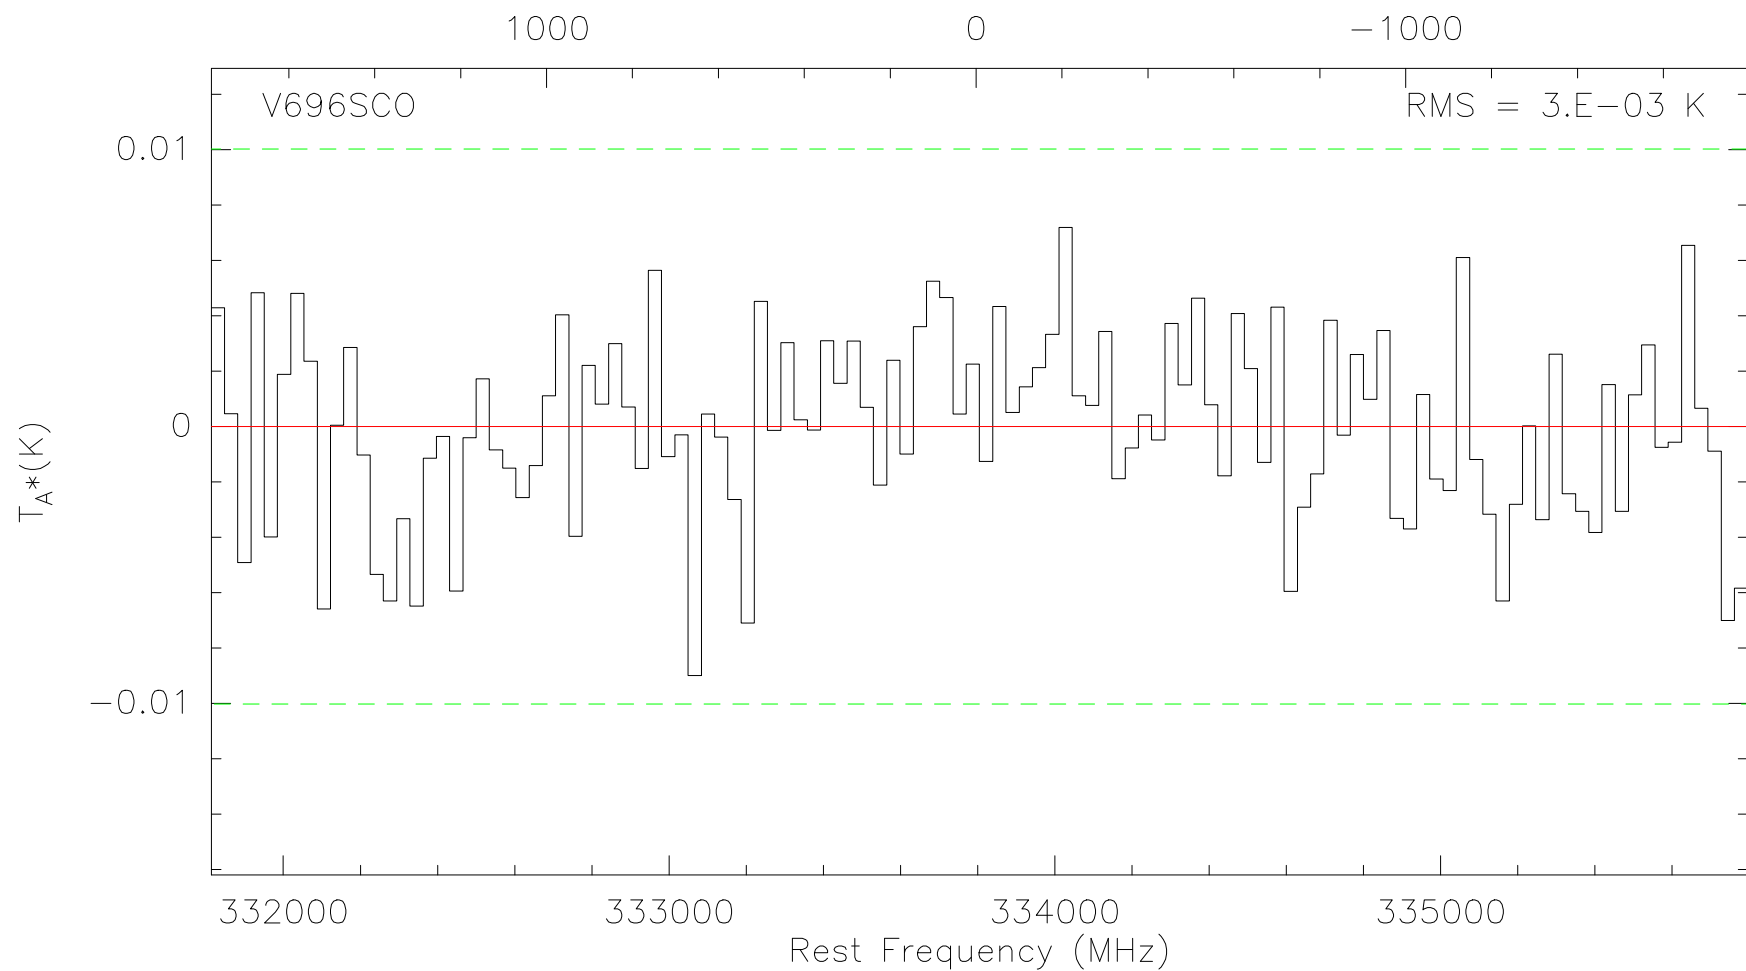

1;1 V697SCO CO(3-2) OSB AP-F301-XF0- O:13-JUL-2016 R:07-AUG-2020  
RA: 17:51:21.83 DEC: -37:24:55.2 Eq 2000.0 Rad. 0.0° Offs: -0.2 -0.5  
Unknown tau: 0.200 Tsys: 220. Time: 14.9min El: 43.3  
N: 116 IO: 58.7548 V0: 0.000 Dv: 30.84 LSR  
FO: 333795.842 Df: -34.33 Fi: 345795.990

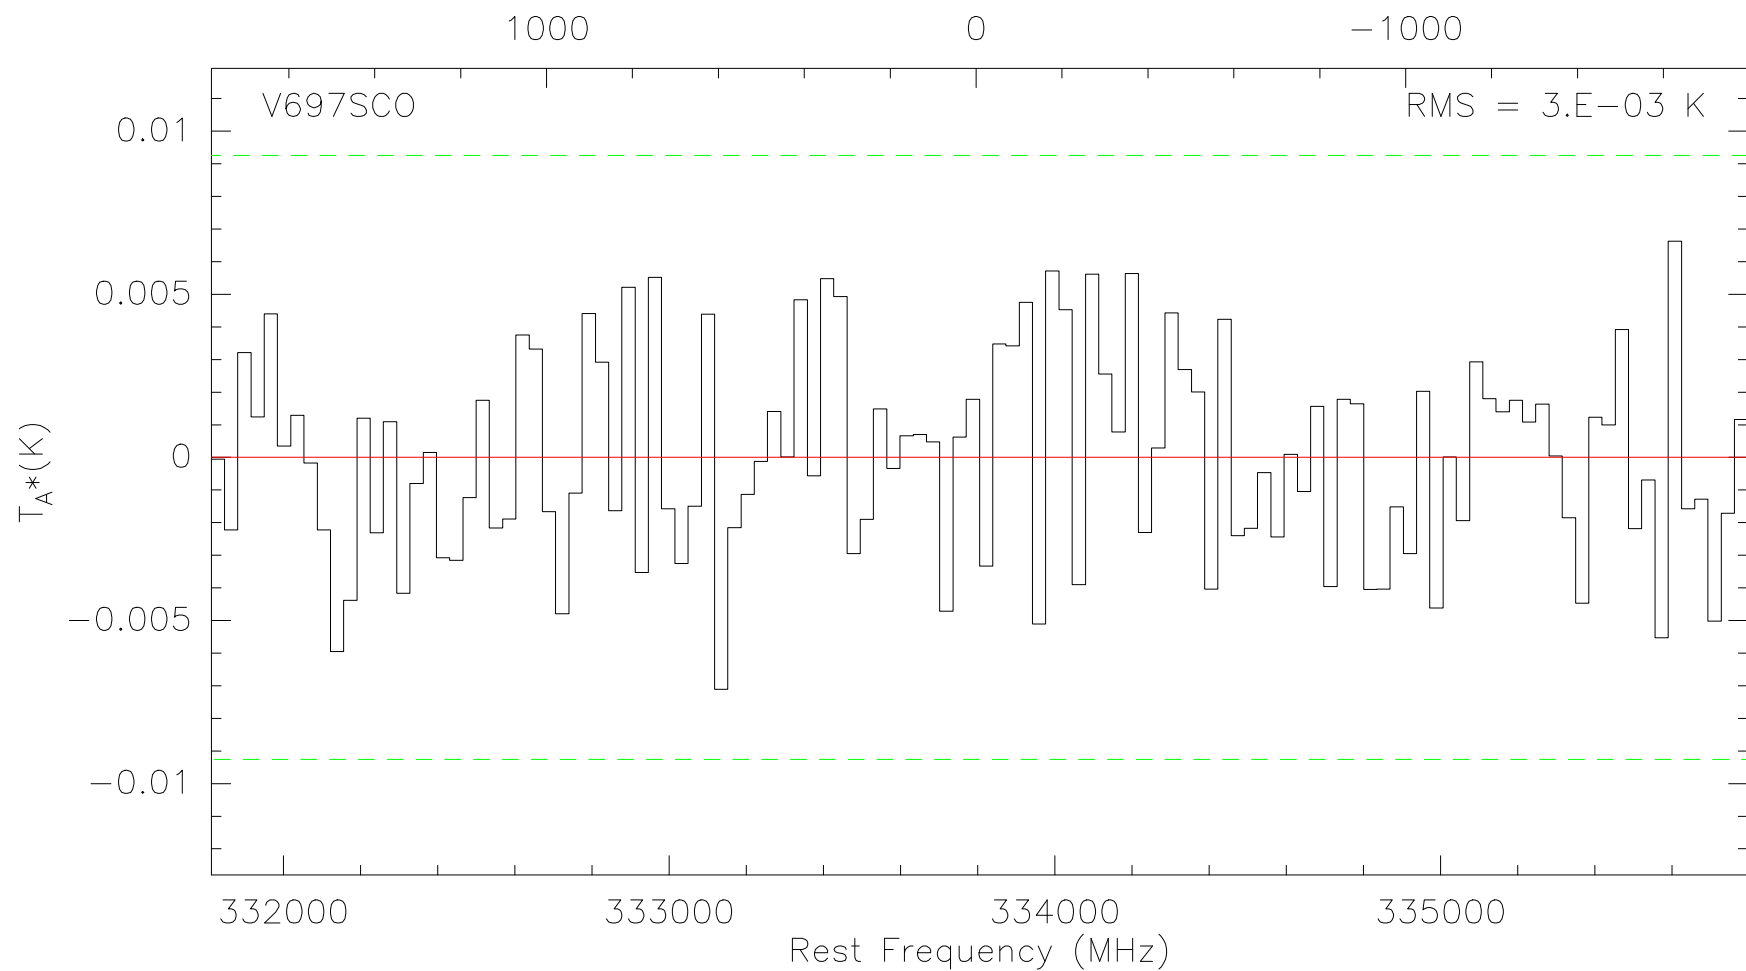

1;1 V707SCO CO(3-2) OSB AP-F301-XF0- 0:06-JUL-2016 R:07-AUG-2020  
RA: 17:48:26.38 DEC: -36:37:54.9 Eq 2000.0 Rad. 0.0° Offs: +0.3 -0.3  
Unknown tau: 0.259 Tsys: 286. Time: 9.9min El: 40.0  
N: 116 IO: 58.7548 V0: 0.000 Dv: 30.83 LSR  
FO: 333795.975 Df: -34.33 Fi: 345795.990

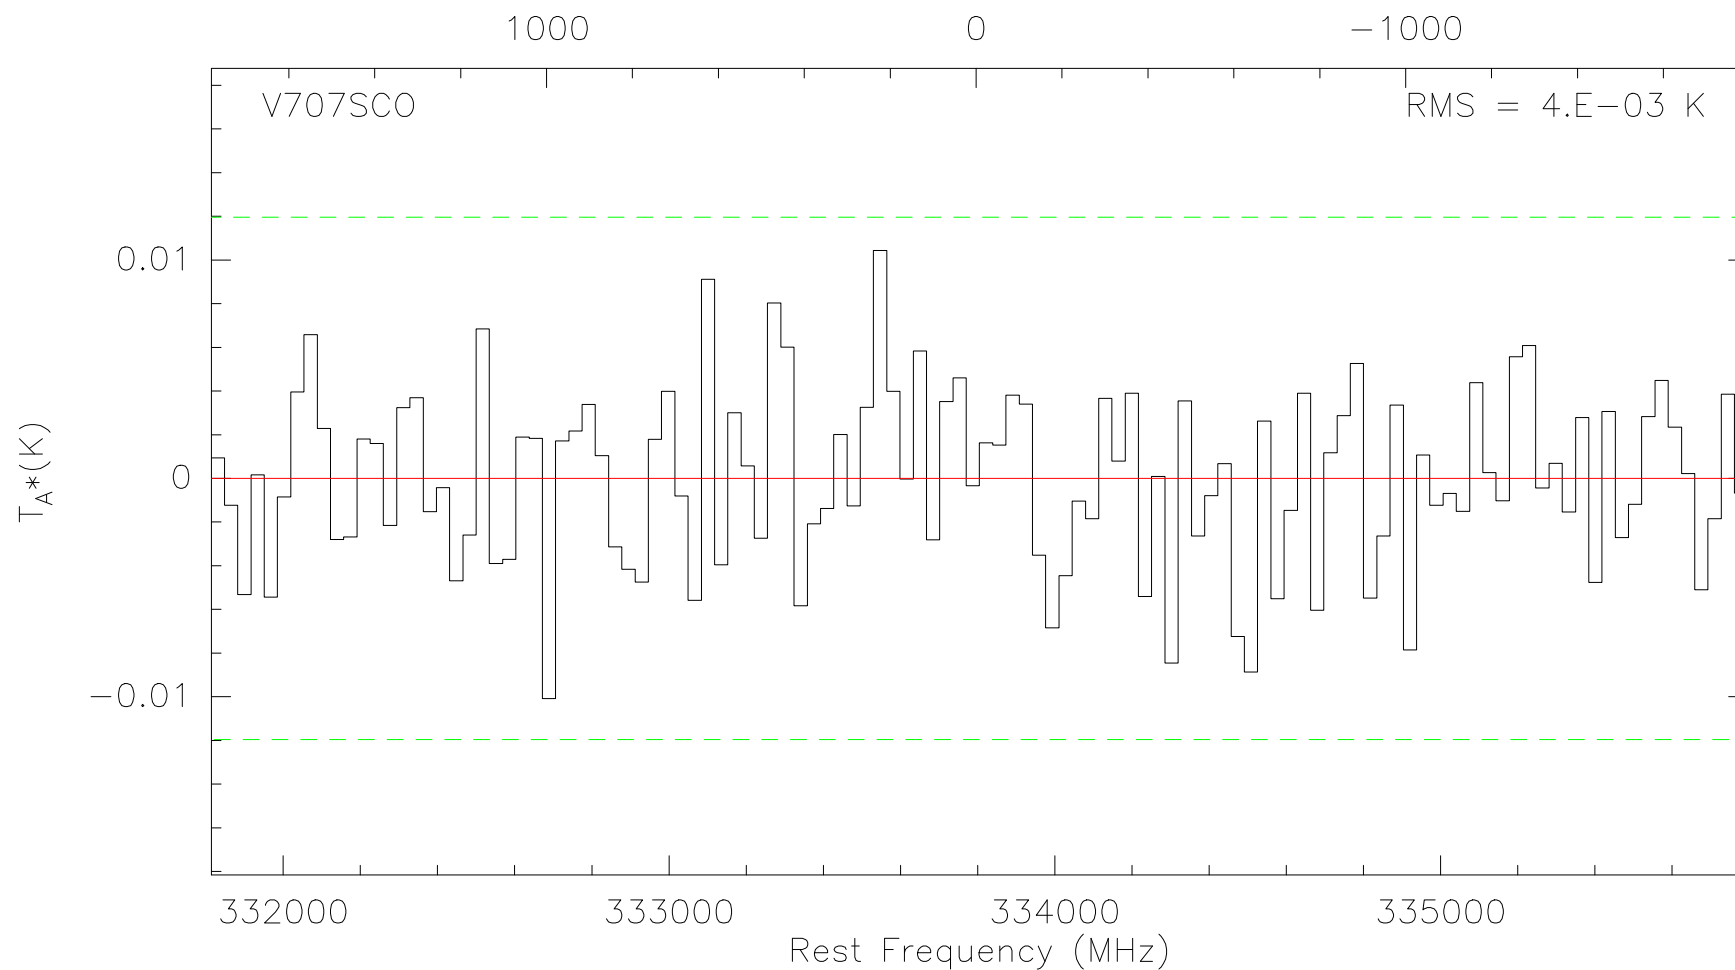

1;1 V711SCO CO(3-2) OSB AP-F301-XF0- O:14-JUL-2016 R:07-AUG-2020  
RA: 17:54:06.16 DEC: -34:21:15.5 Eq 2000.0 Rad. 0.0° Offs: +0.3 -0.3  
Unknown tau: 0.284 Tsys: 246. Time: 9.9min El: 58.0  
N: 116 IO: 58.7548 V0: 0.000 Dv: 30.84 LSR  
FO: 333795.891 Df: -34.33 Fi: 345795.990

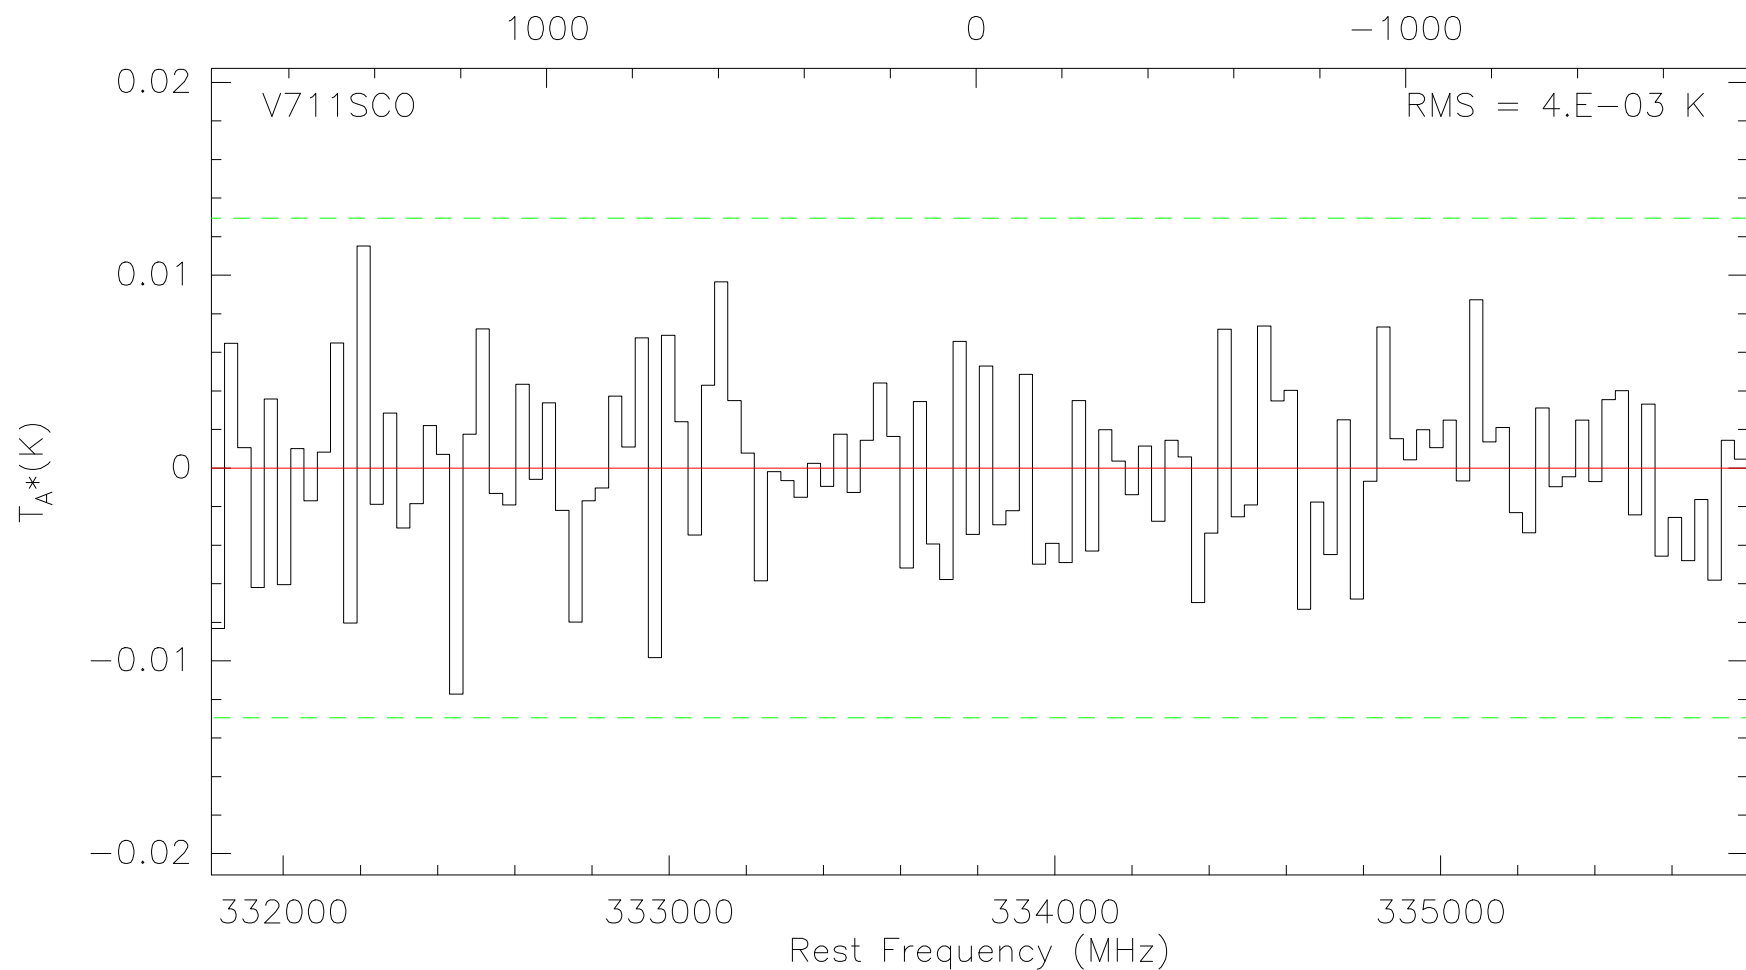

1;1 V729SCO CO(3-2) OSB AP-F301-XF0- 0:01-JUL-2016 R:07-AUG-2020  
RA: 17:22:02.66 DEC: -32:05:48.8 Eq 2000.0 Rad. 0.0° Offs: -0.2 -0.5  
Unknown tau: 0.400 Tsys: 503. Time: 14.9min El: 30.0  
N: 116 IO: 58.7548 V0: 0.000 Dv: 30.83 LSR  
FO: 333795.989 Df: -34.33 Fi: 345795.990

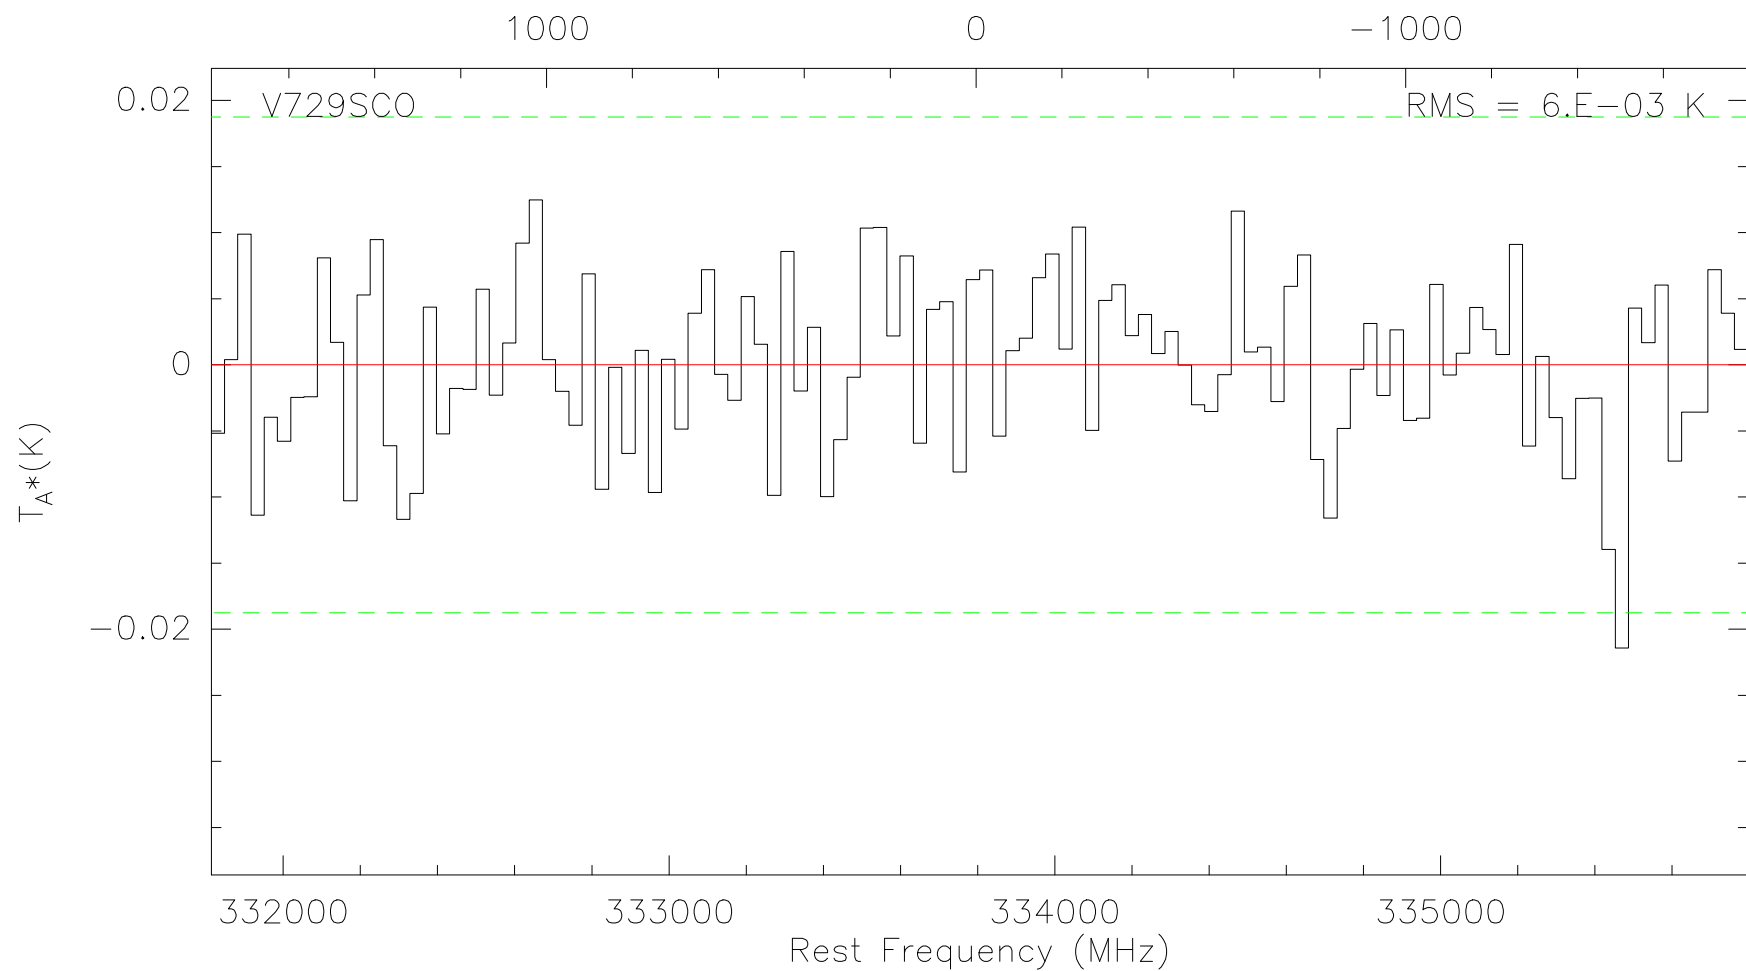

1;1 V732SGR CO(3-2) OSB AP-F301-XF0- 0:13-JUL-2016 R:07-AUG-2020  
RA: 17:56:07.51 DEC: -27:22:16.1 Eq 2000.0 Rad. 0.0° Offs: +0.2 -0.4  
Unknown tau: 0.255 Tsys: 213. Time: 9.9min El: 71.8  
N: 116 IO: 58.7548 V0: 0.000 Dv: 30.83 LSR  
FO: 333795.991 Df: -34.33 Fi: 345795.990

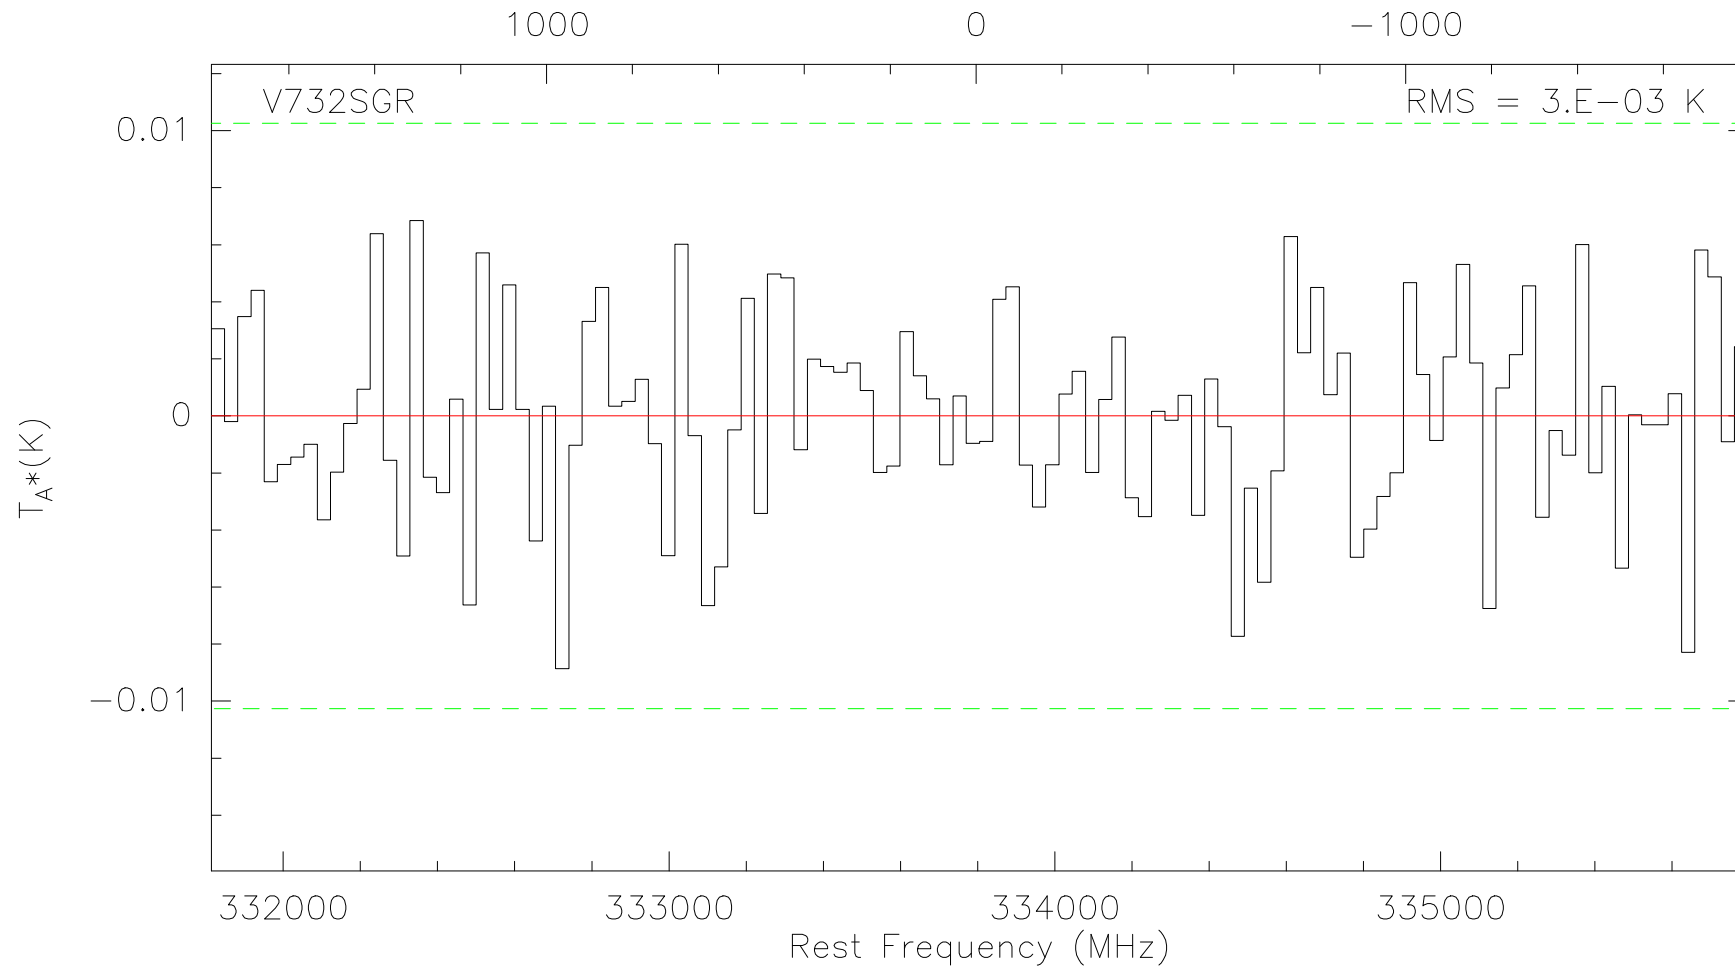

1;1 V733SCO CO(3-2) OSB AP-F301-XF0- 0:06-JUL-2016 R:07-AUG-2020  
RA: 17:39:42.88 DEC: -35:52:38.4 Eq 2000.0 Rad. 0.0° Offs: +0.3 -0.3  
Unknown tau: 0.245 Tsys: 288. Time: 9.9min El: 37.6  
N: 116 IO: 58.7548 V0: 0.000 Dv: 30.83 LSR  
FO: 333795.948 Df: -34.33 Fi: 345795.990

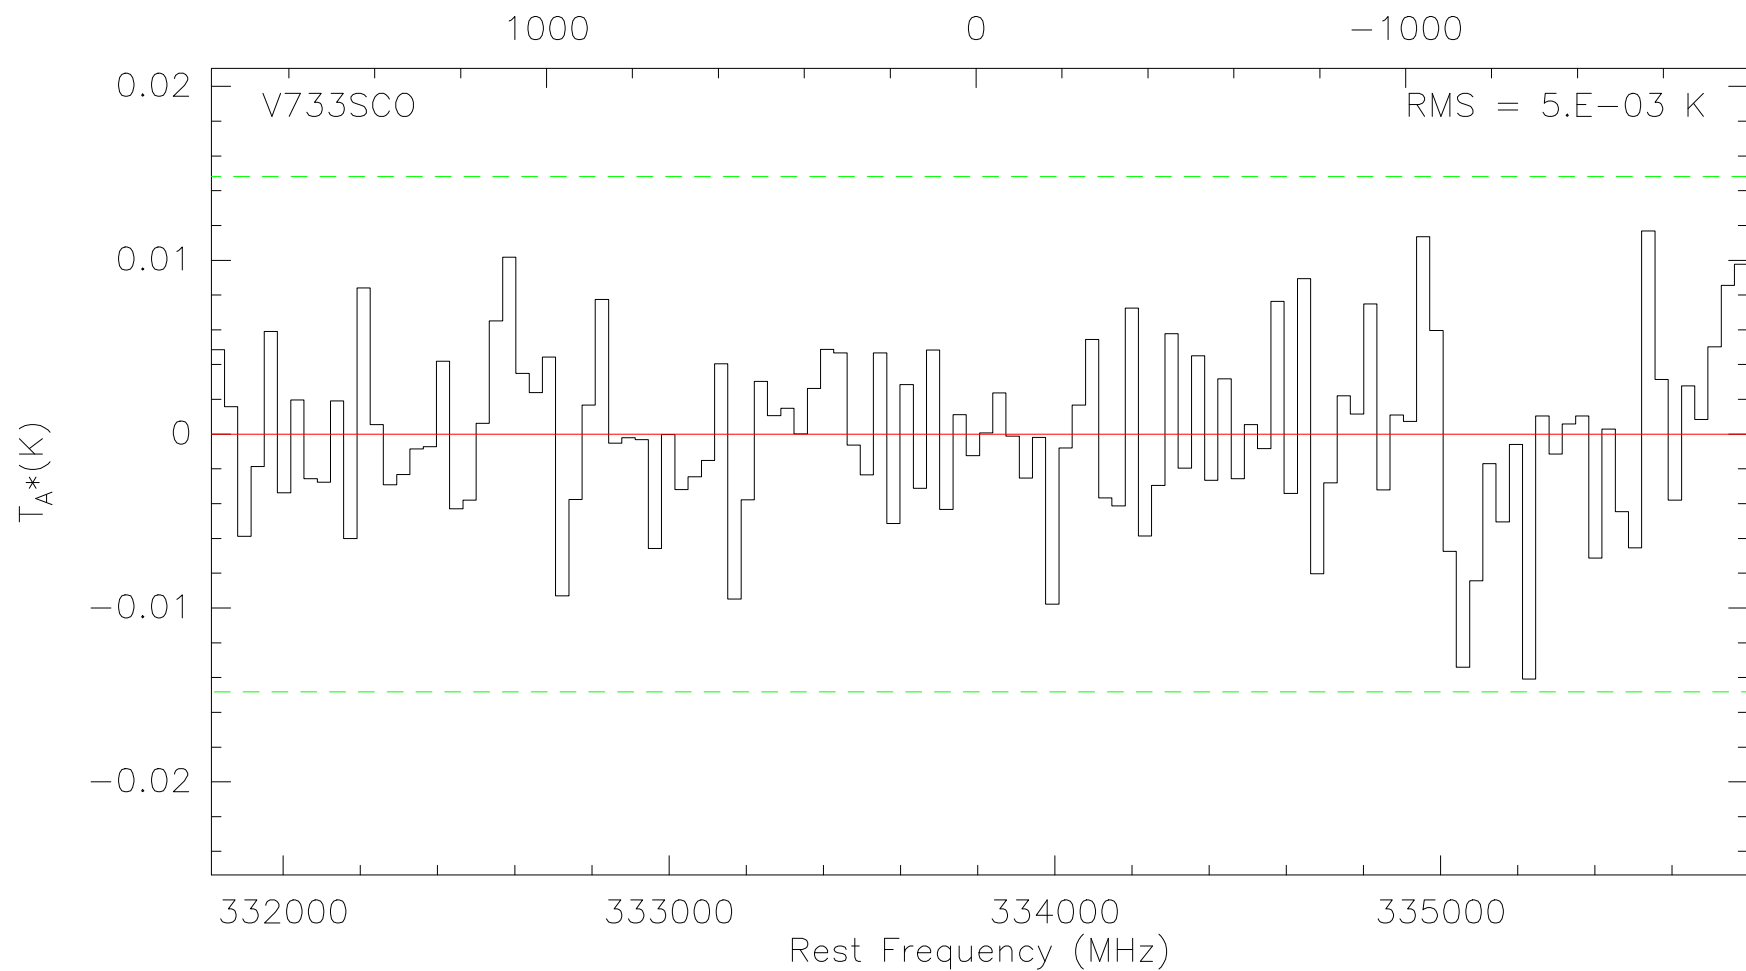

1;1 V737SGR CO(3-2) OSB AP-F301-XF0- 0:14-JUL-2016 R:07-AUG-2020  
RA: 18:07:08.66 DEC: -28:44:52.3 Eq 2000.0 Rad. 0.0° Offs: +0.2 -0.4  
Unknown tau: 0.270 Tsys: 224. Time: 9.9min El: 70.3  
N: 116 IO: 58.7548 V0: 0.000 Dv: 30.83 LSR  
FO: 333796.004 Df: -34.33 Fi: 345795.990

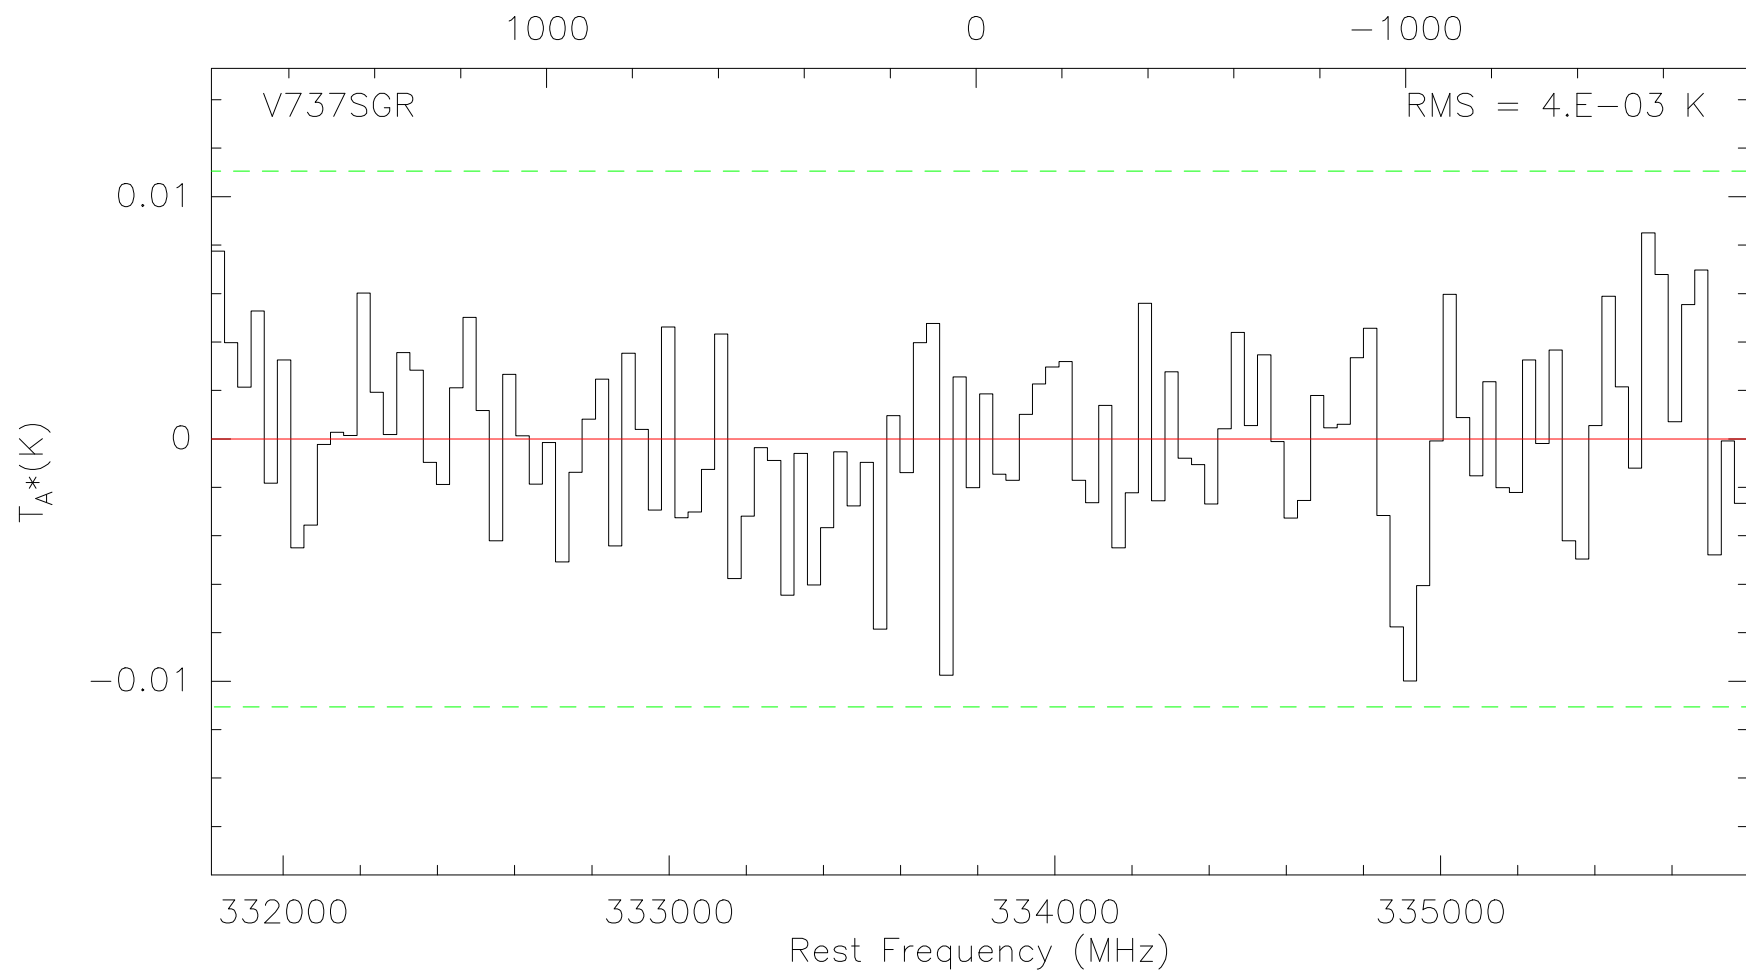

1;1 V745SCO CO(3-2) OSB AP-F301-XF0- O:13-JUL-2016 R:07-AUG-2020  
RA: 17:55:22.27 DEC: -33:14:58.5 Eq 2000.0 Rad. 0.0° Offs: +0.0 -0.7  
Unknown tau: 0.215 Tsys: 190. Time: 9.9min El: 77.6  
N: 116 IO: 58.7548 V0: 0.000 Dv: 30.84 LSR  
FO: 333795.914 Df: -34.33 Fi: 345795.990

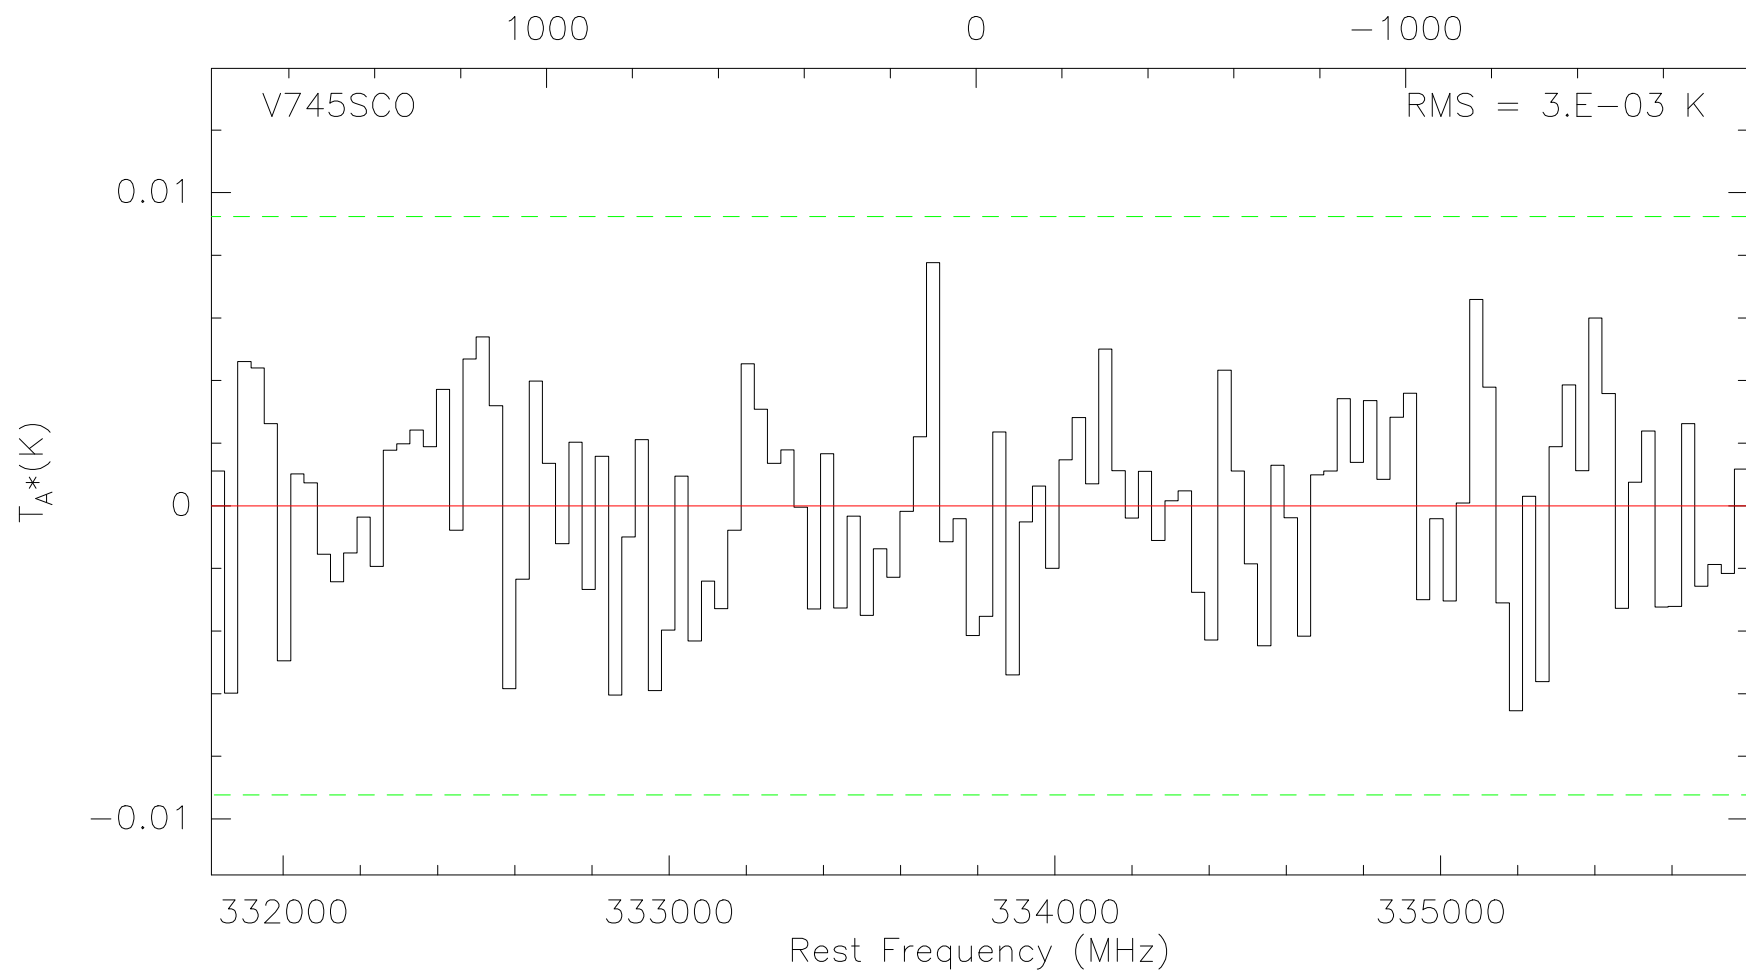

1;1 V787SGR CO(3-2) OSB AP-F301-XF0- 0:14-JUL-2016 R:07-AUG-2020  
RA: 18:00:02.20 DEC: -30:30:31.0 Eq 2000.0 Rad. 0.0° Offs: +0.2 -0.3  
Unknown tau: 0.291 Tsys: 243. Time: 9.9min El: 62.7  
N: 116 IO: 58.7548 V0: 0.000 Dv: 30.83 LSR  
FO: 333795.956 Df: -34.33 Fi: 345795.990

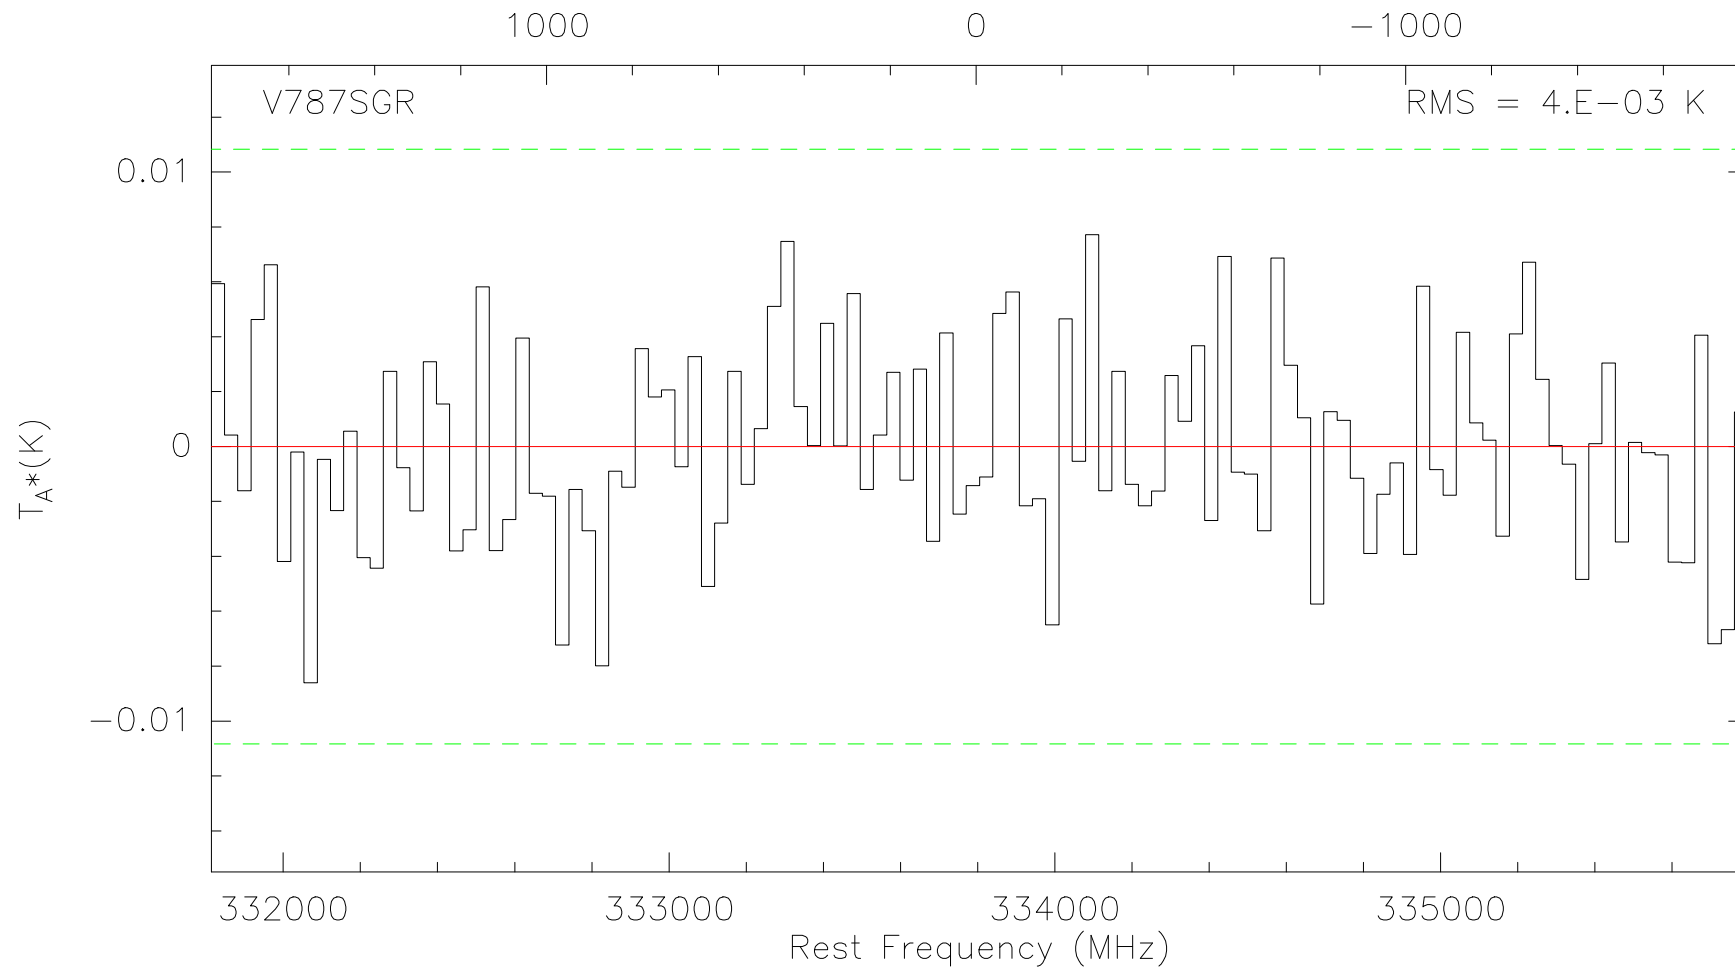

1;1 V7940PH CO(3-2) OSB AP-F301-XF0- 0:01-JUL-2016 R:07-AUG-2020  
RA: 17:38:49.25 DEC: -22:50:48.9 Eq 2000.0 Rad. 0.0° Offs: -0.2 -0.5  
Unknown tau: 0.404 Tsys: 394. Time: 9.9min El: 42.1  
N: 116 lO: 58.7548 V0: 0.000 Dv: 30.83 LSR  
FO: 333796.165 Df: -34.33 Fi: 345795.990

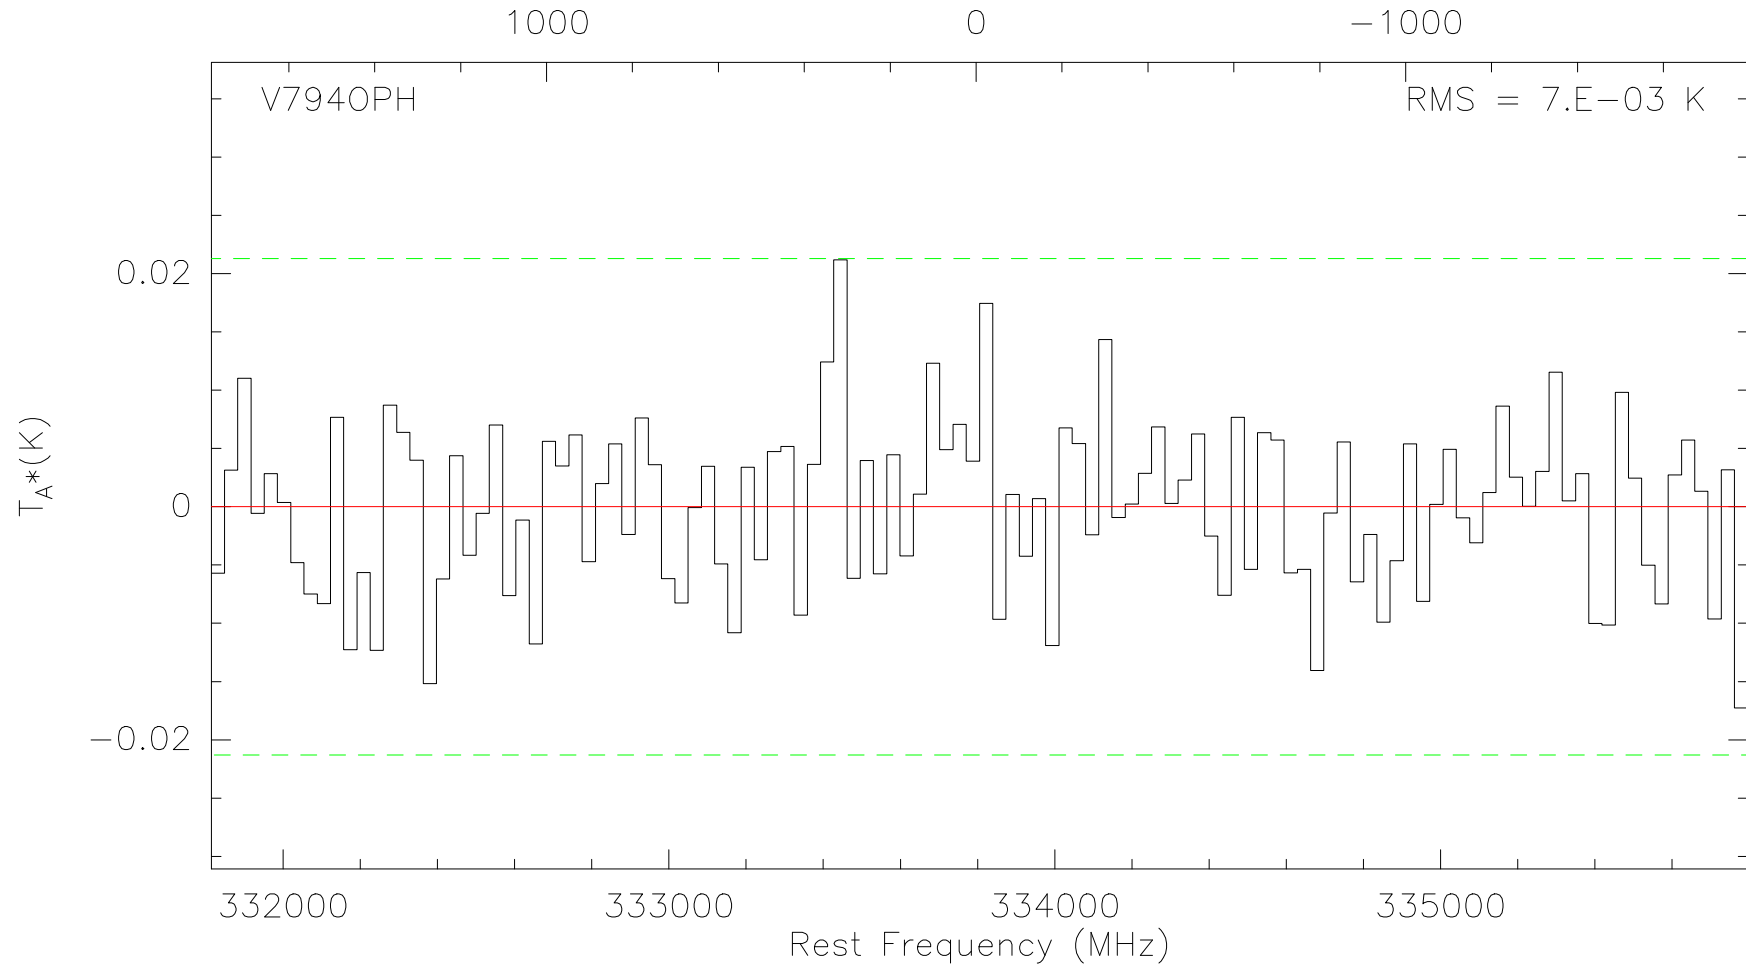

1;1 V909SGR CO(3-2) OSB AP-F301-XF0- 0:13-JUL-2016 R:07-AUG-2020  
RA: 18:25:52.30 DEC: -35:01:27.0 Eq 2000.0 Rad. 0.0° Offs: +0.2 -0.4  
Unknown tau: 0.254 Tsys: 217. Time: 9.9min El: 67.4  
N: 116 IO: 58.7548 V0: 0.000 Dv: 30.83 LSR  
FO: 333796.021 Df: -34.33 Fi: 345795.990

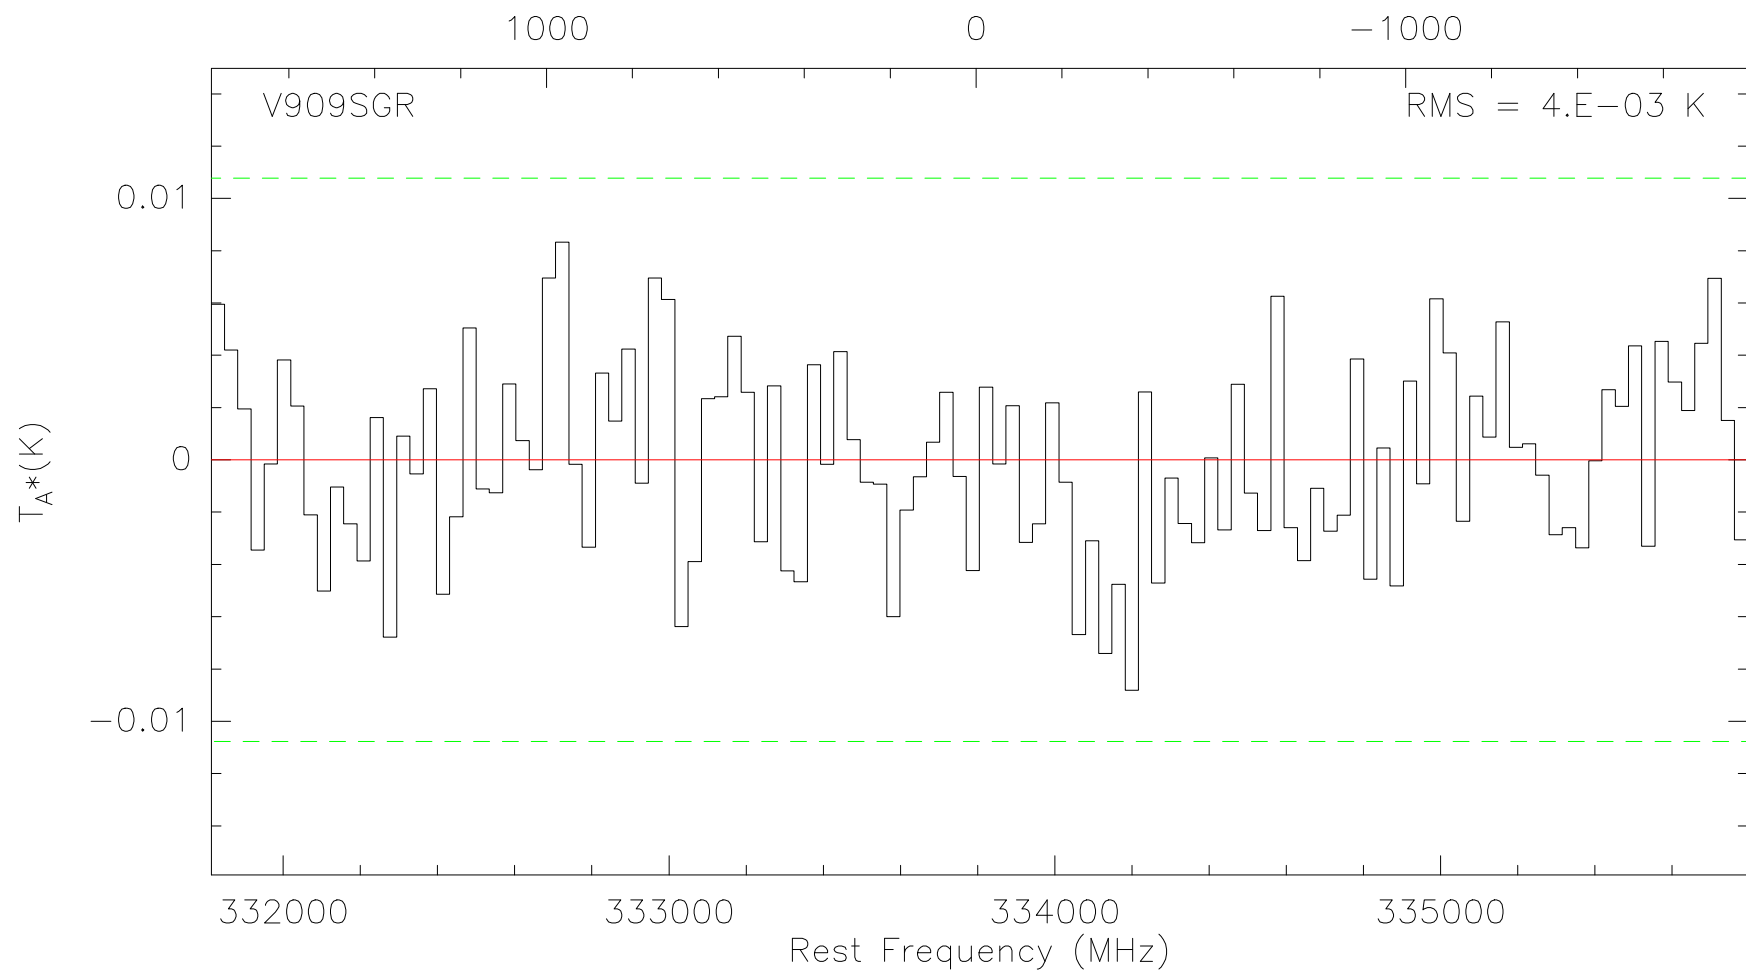

1;1 V941SGR CO(3-2) OSB AP-F301-XF0- 0:13-JUL-2016 R:07-AUG-2020  
RA: 18:34:43.46 DEC: -29:34:49.1 Eq 2000.0 Rad. 0.0° Offs: -0.2 -0.3  
Unknown tau: 0.173 Tsys: 263. Time: 9.9min El: 25.8  
N: 116 IO: 58.7548 V0: 0.000 Dv: 30.83 LSR  
FO: 333796.099 Df: -34.33 Fi: 345795.990

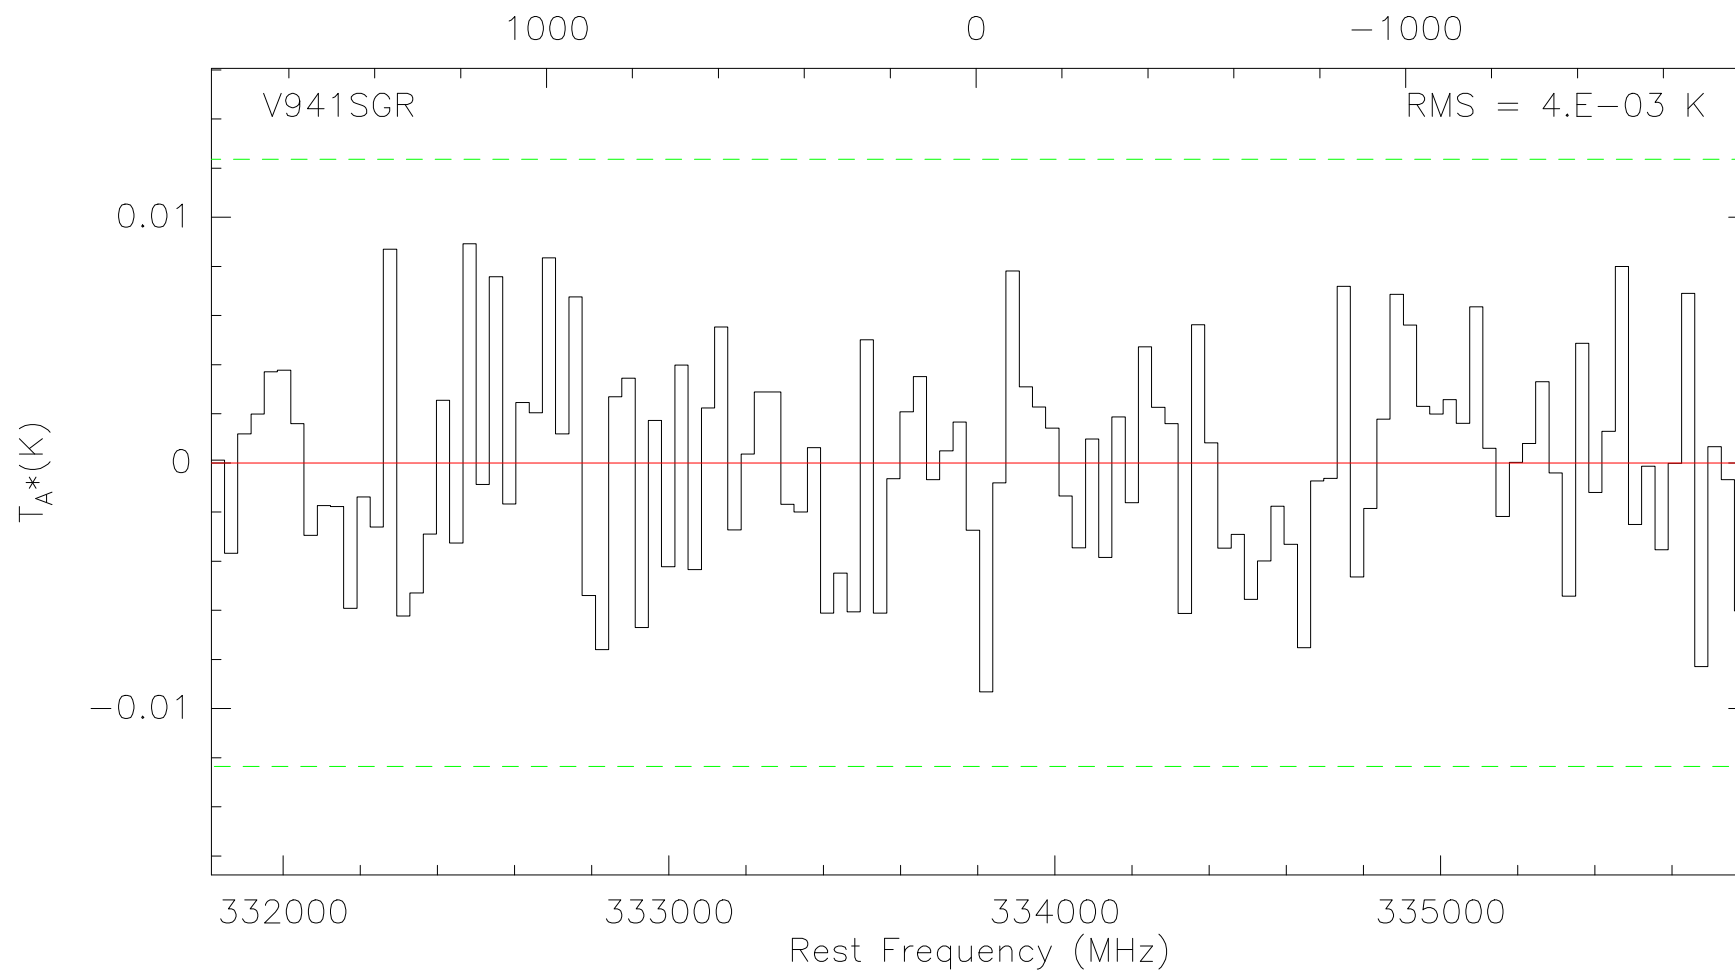

1;1 V999SGR CO(3-2) OSB AP-F301-XF0- 0:13-JUL-2016 R:07-AUG-2020  
RA: 18:00:05.59 DEC: -27:33:14.0 Eq 2000.0 Rad. 0.0° Offs: -0.2 -0.4  
Unknown tau: 0.195 Tsys: 225. Time: 9.9min El: 38.9  
N: 116 IO: 58.7548 V0: 0.000 Dv: 30.83 LSR  
FO: 333795.984 Df: -34.33 Fi: 345795.990

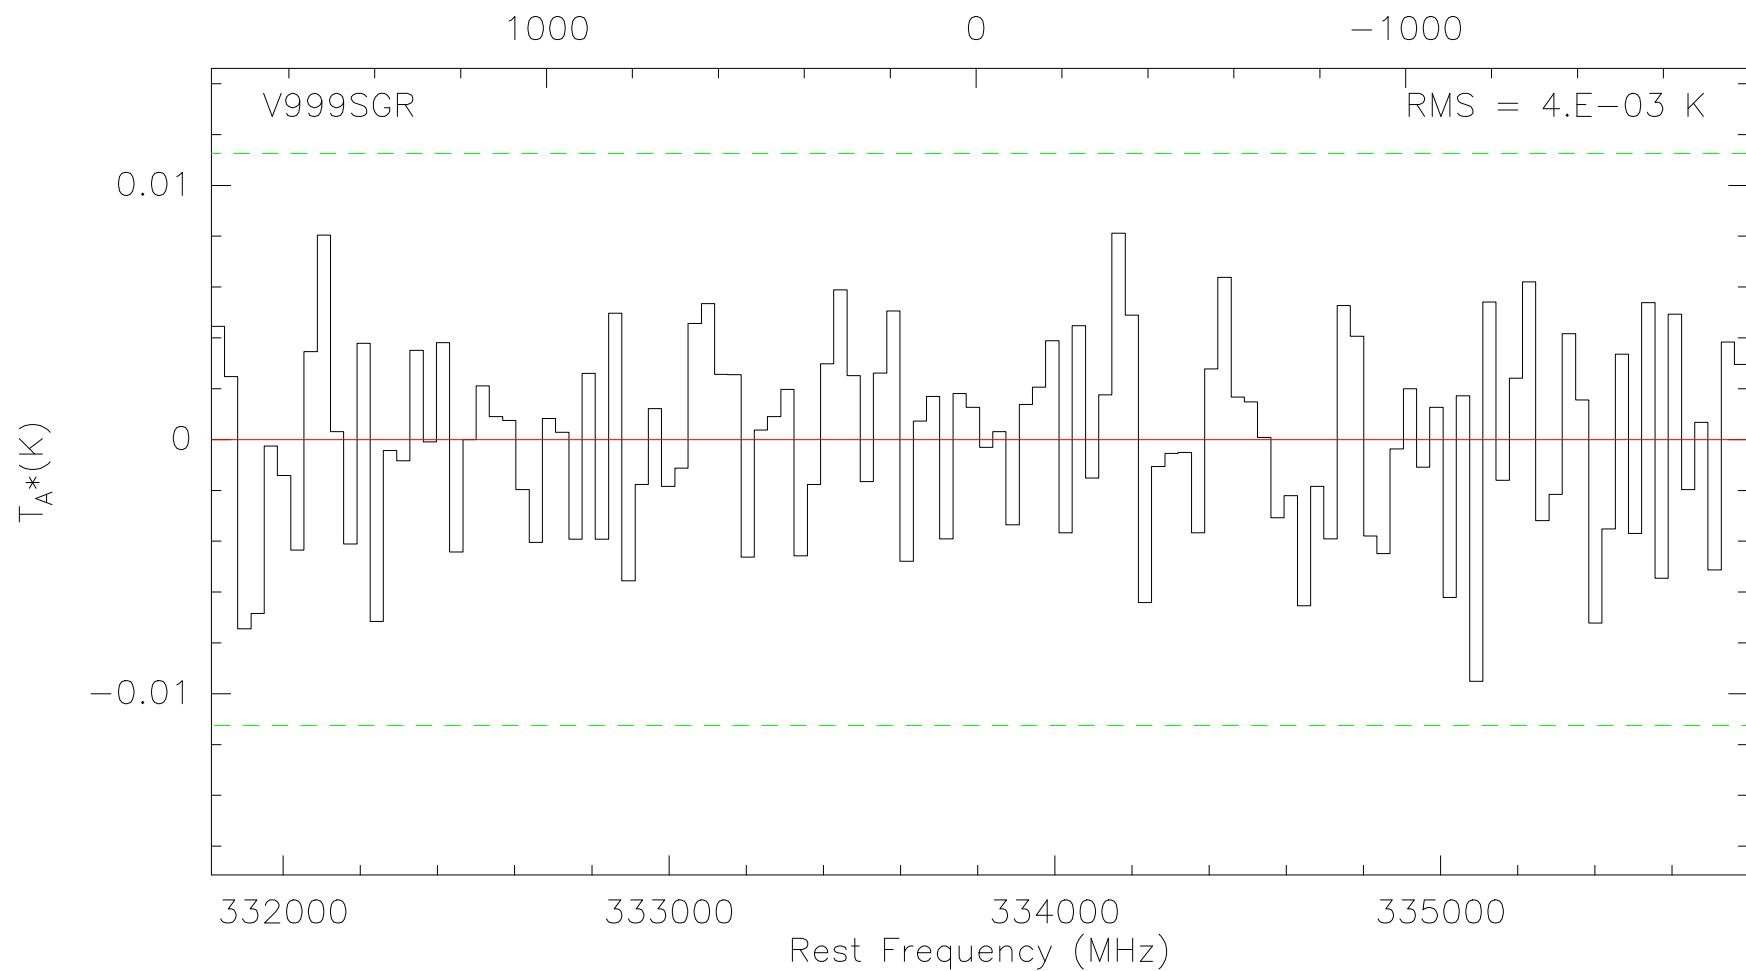

1;1 V1148-SGR CO(3-2) OSB AP-F301-XF0- O:03-JUN-2015 R:13-AUG-2020  
RA: 18:09:05.85 DEC: -25:59:08.0 Eq 2000.0 Rad. 0.0° Offs: +0.2 -0.4  
Unknown tau: 0.226 Tsys: 215. Time: 44.6min El: 48.5  
N: 116 IO: 58.7510 V0: 0.000 Dv: 30.83 LSR  
FO: 333797.613 Df: -34.33 Fi: 345795.990

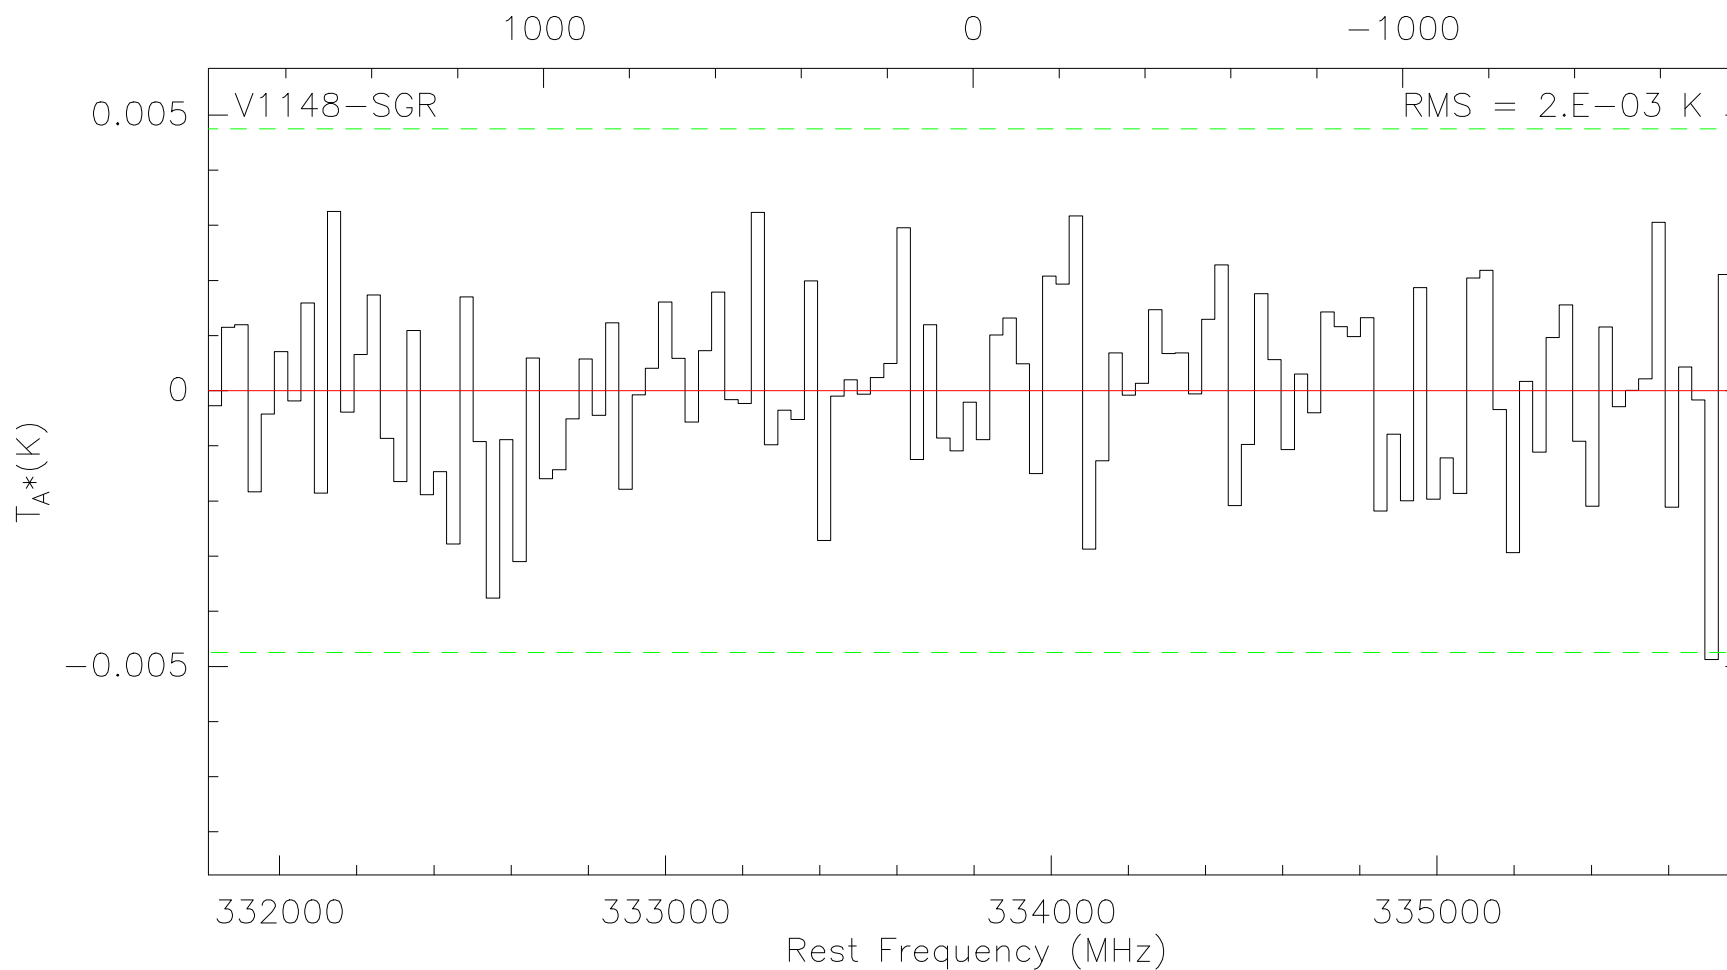

Supplement: Supplementary file 2 [file all_sm_CO32_OSB.pdf]
