# Supplementary material for: A search for cool molecular gas in GK Persei and other classical novae
Source: arXiv:2201.10332 source file (2022-01-25)

1;1 CN-VEL CO(4-3) AP-FL01-XF0- O:24-AUG-2014 R:12-AUG-2020  
RA: 11:02:38.57 DEC: -54:23:09.5 Eq 2000.0 Rad. 0.0° Offs: -0.1 -0.5  
Unknown tau: 0.694 Tsys: 711. Time: 23.4min El: 50.6  
N: 87 IO: 44.1918 V0: 0.000 Dv: -29.77 LSR  
FO: 461040.768 Df: 45.78 Fi: 473041.715

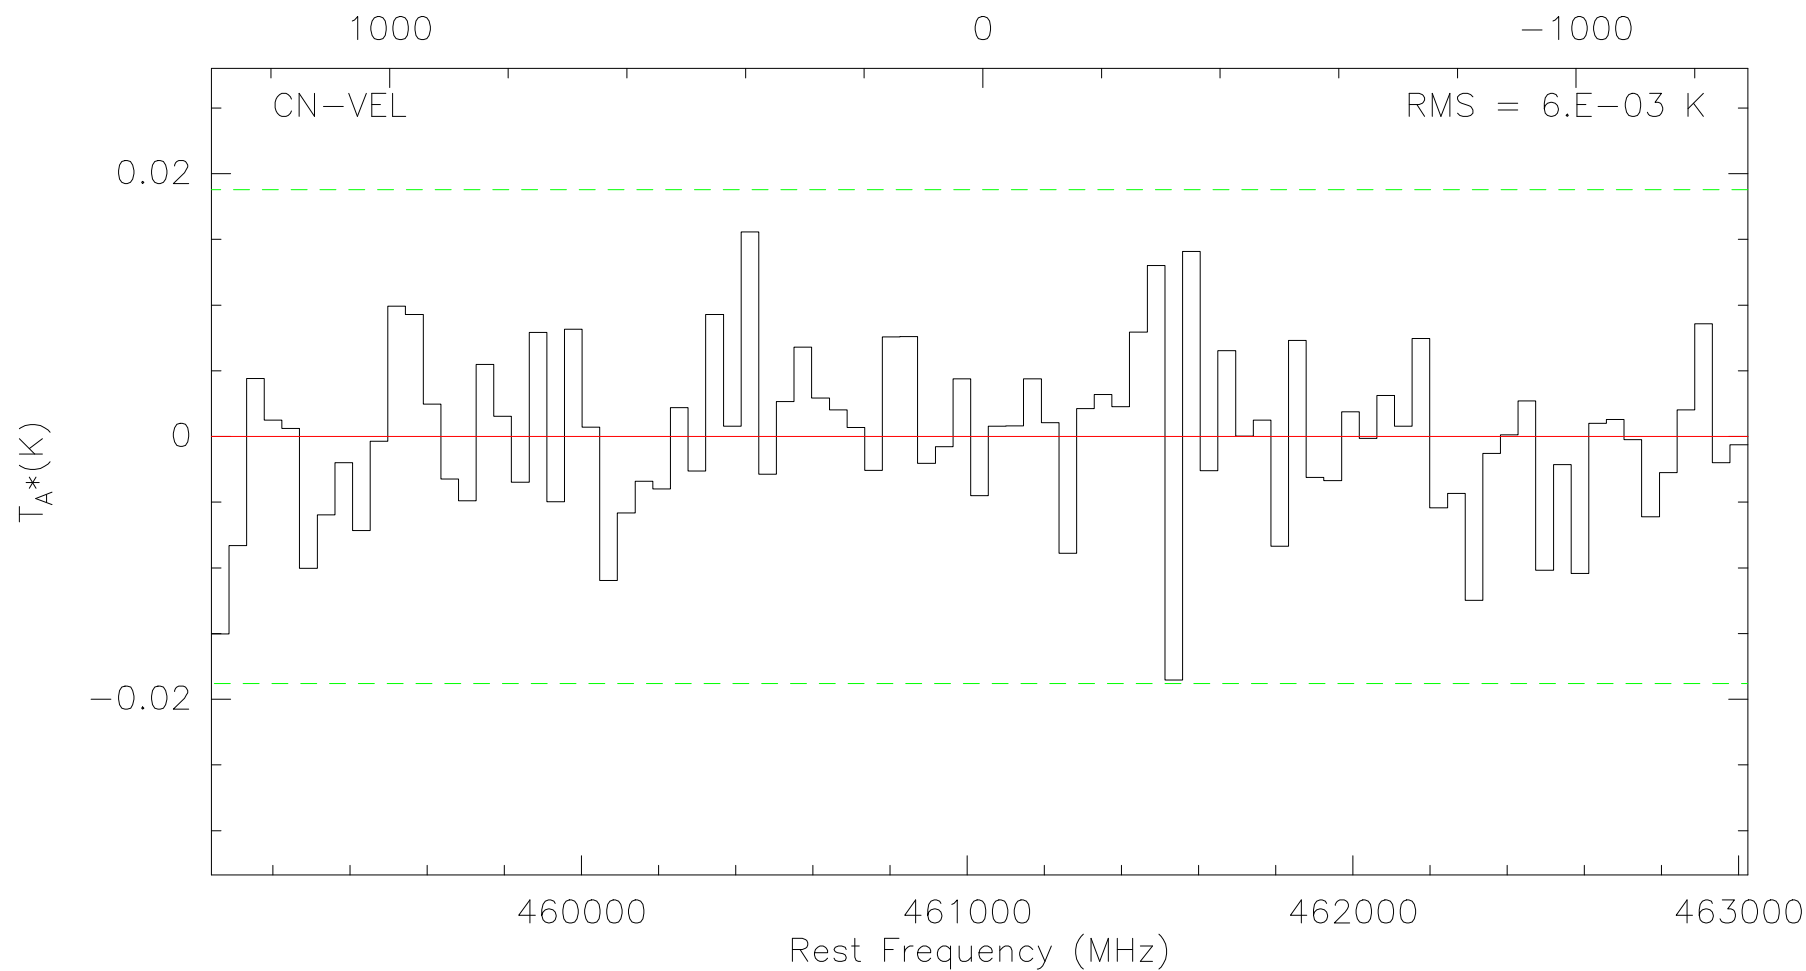

1;1 CQ-VEL CO(4-3) AP-FL01-XF0- O:26-AUG-2014 R:12-AUG-2020  
RA: 08:58:50.99 DEC: -53:20:17.8 Eq 2000.0 Rad. 0.0° Offs: +0.1 -0.5  
Unknown tau: 0.457 Tsys: 507. Time: 23.4min El: 58.6  
N: 87 IO: 44.1918 V0: 0.000 Dv: -29.77 LSR  
F0: 461040.768 Df: 45.78 Fi: 473041.532

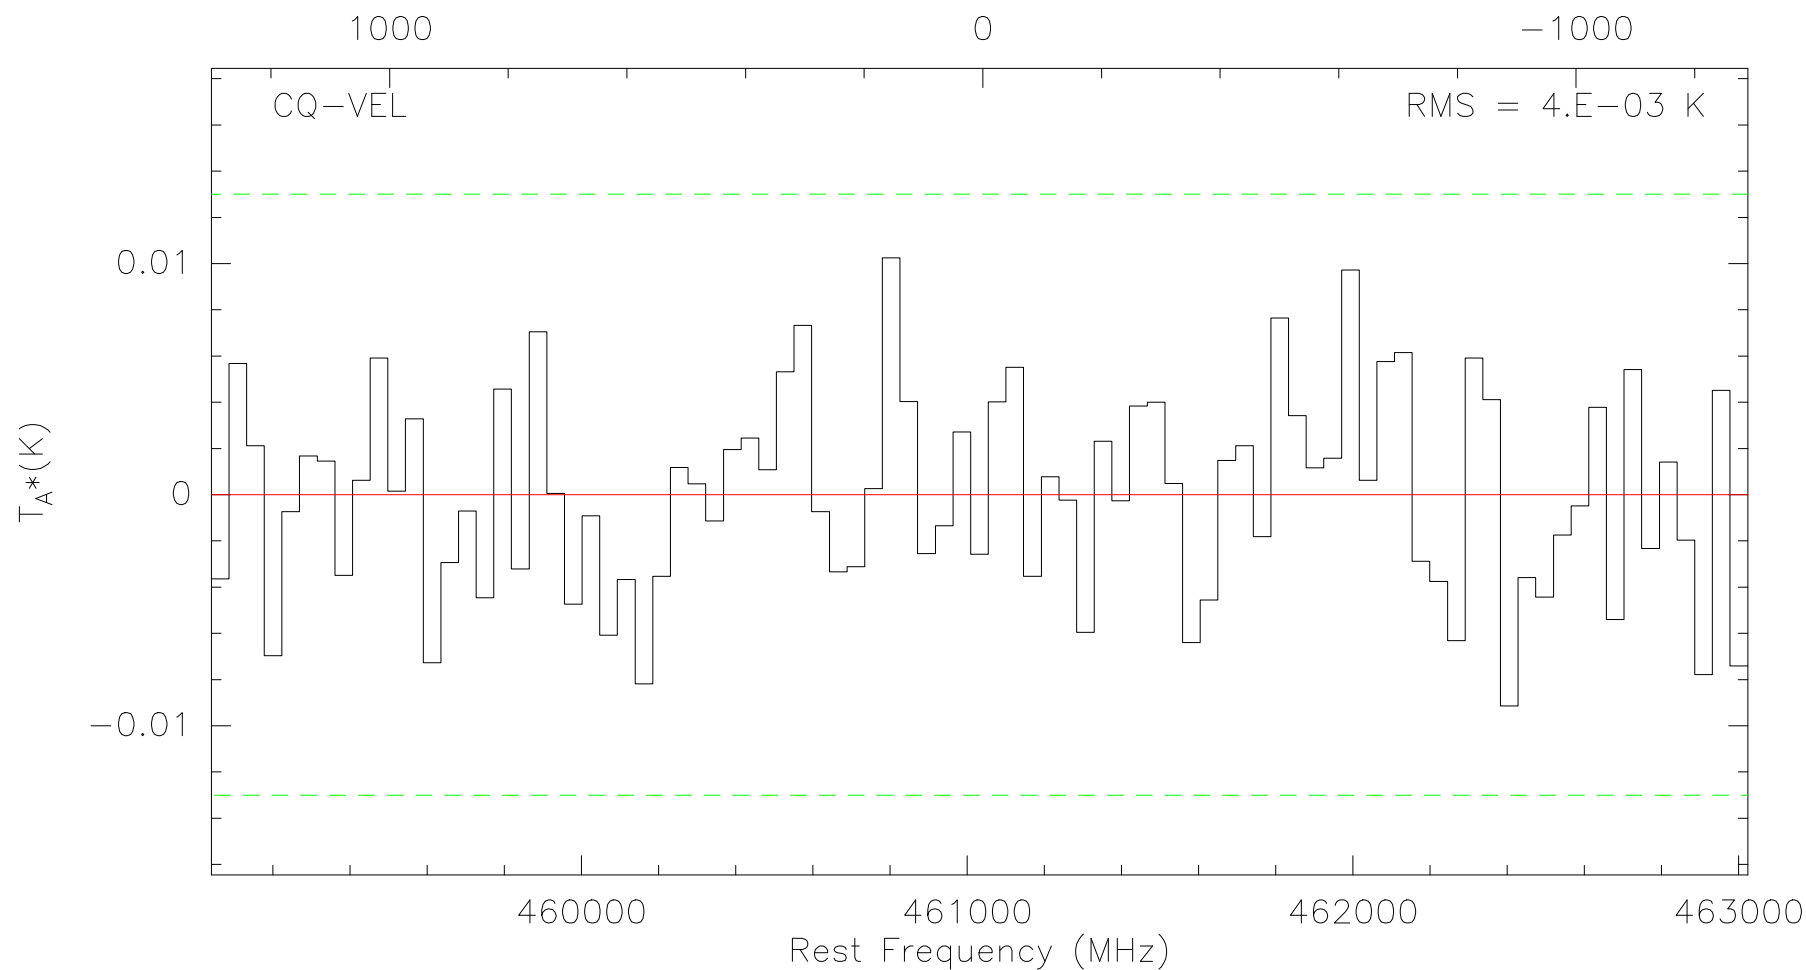

1;1 DY-PUP CO(4-3) AP-FL01-XF0- O:25-AUG-2014 R:12-AUG-2020

RA: 08:13:48.51 DEC: -26:33:56.5 Eq 2000.0 Rad. 0.0° Offs: +0.2 -0.2

Unknown tau: 0.425 Tsys: 407. Time: 23.5min El: 65.1

N: 87 IO: 44.1918 V0: 0.000 Dv: -29.77 LSR

F0: 461040.768 Df: 45.78 Fi: 473041.196

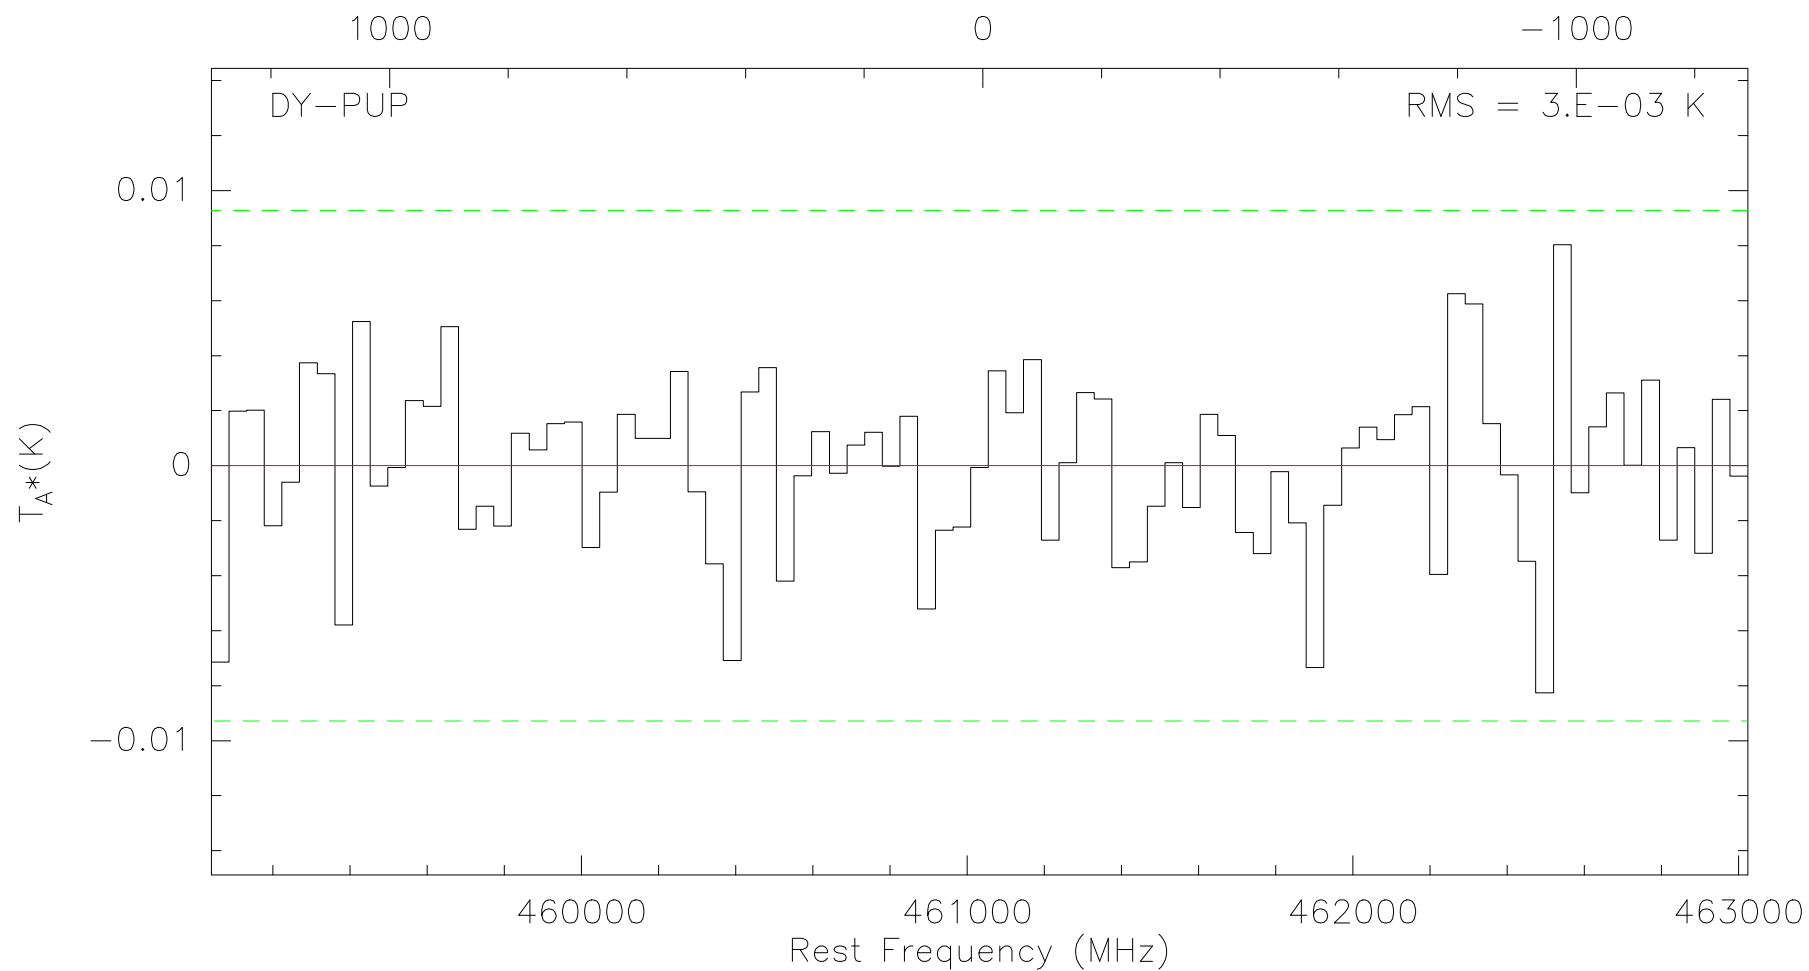

1;1 GU-MUS CO(4-3) AP-FL01-XF0- O:24-AUG-2014 R:12-AUG-2020

RA: 11:26:26.60 DEC: -68:40:32.3 Eq 2000.0 Rad. 0.0° Offs: -0.2 -0.4

Unknown tau: 0.620 Tsys: 989. Time: 23.3min El: 37.6

N: 87 IO: 44.1918 V0: 0.000 Dv: -29.77 LSR

F0: 461040.768 Df: 45.78 Fi: 473041.720

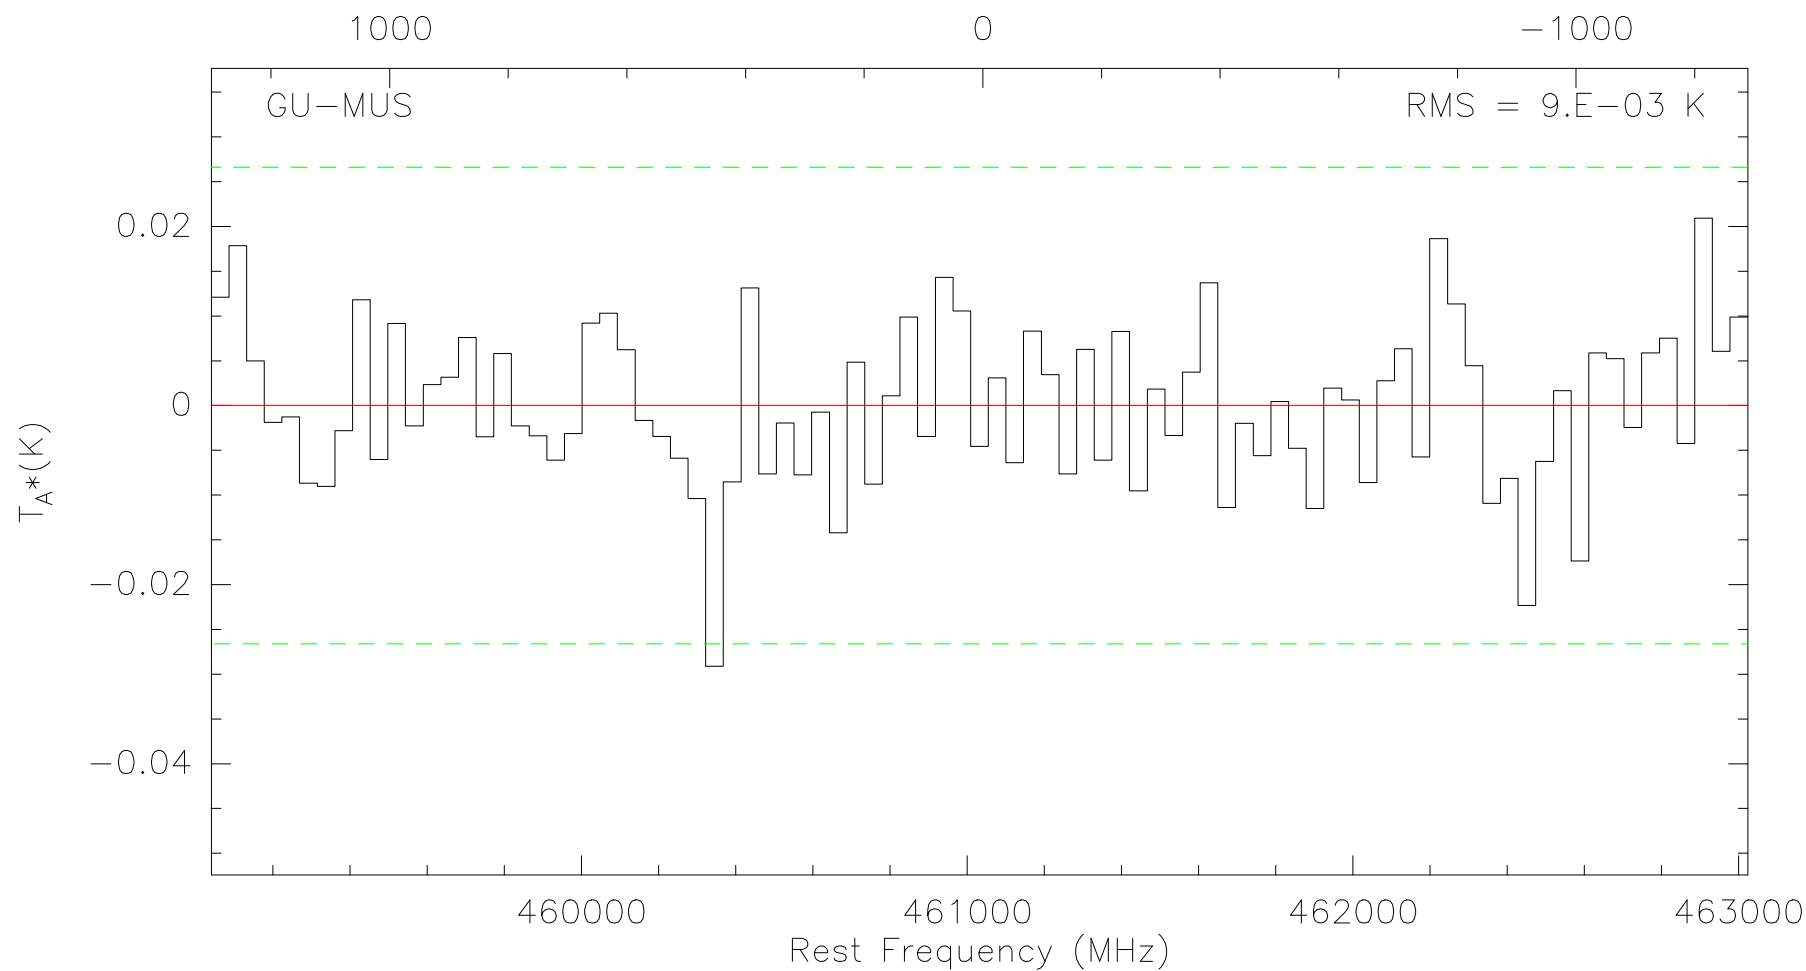

1;1 LZ-MUS CO(4-3) AP-FL01-XF0- O:24-AUG-2014 R:12-AUG-2020  
RA: 11:56:09.27 DEC: -65:34:20.1 Eq 2000.0 Rad. 0.0° Offs: -0.2 -0.4  
Unknown tau: 0.794 Tsys: 1274. Time: 23.4min El: 36.6  
N: 87 l0: 44.1918 v0: 0.000 Dv: -29.77 LSR  
F0: 461040.768 Df: 45.78 Fi: 473041.746

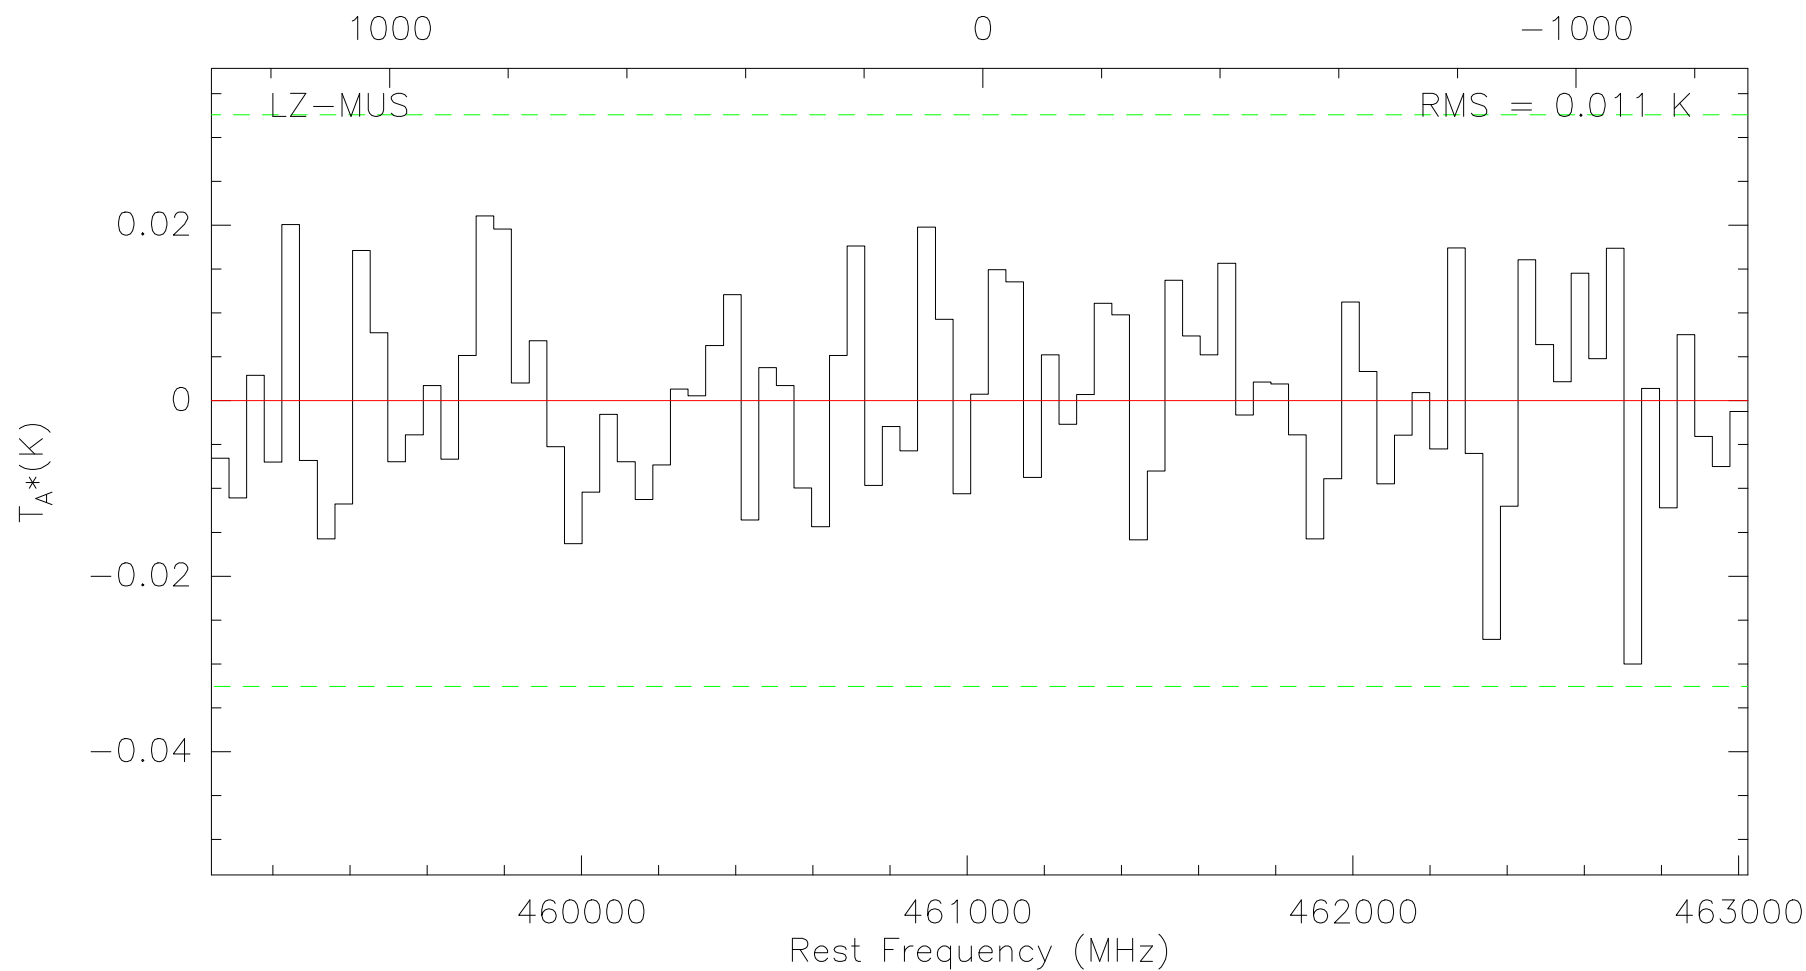

1;1 RR-PIC CO(4-3) AP-FL01-XF0- O:25-AUG-2014 R:12-AUG-2020  
RA: 06:35:36.06 DEC: -62:38:24.3 Eq 2000.0 Rad. 0.0° Offs: +0.3 -0.2  
Unknown tau: 0.449 Tsys: 536. Time: 23.3min El: 42.4  
N: 87 IO: 44.1918 V0: 0.000 Dv: -29.77 LSR  
FO: 461040.768 Df: 45.78 Fi: 473041.406

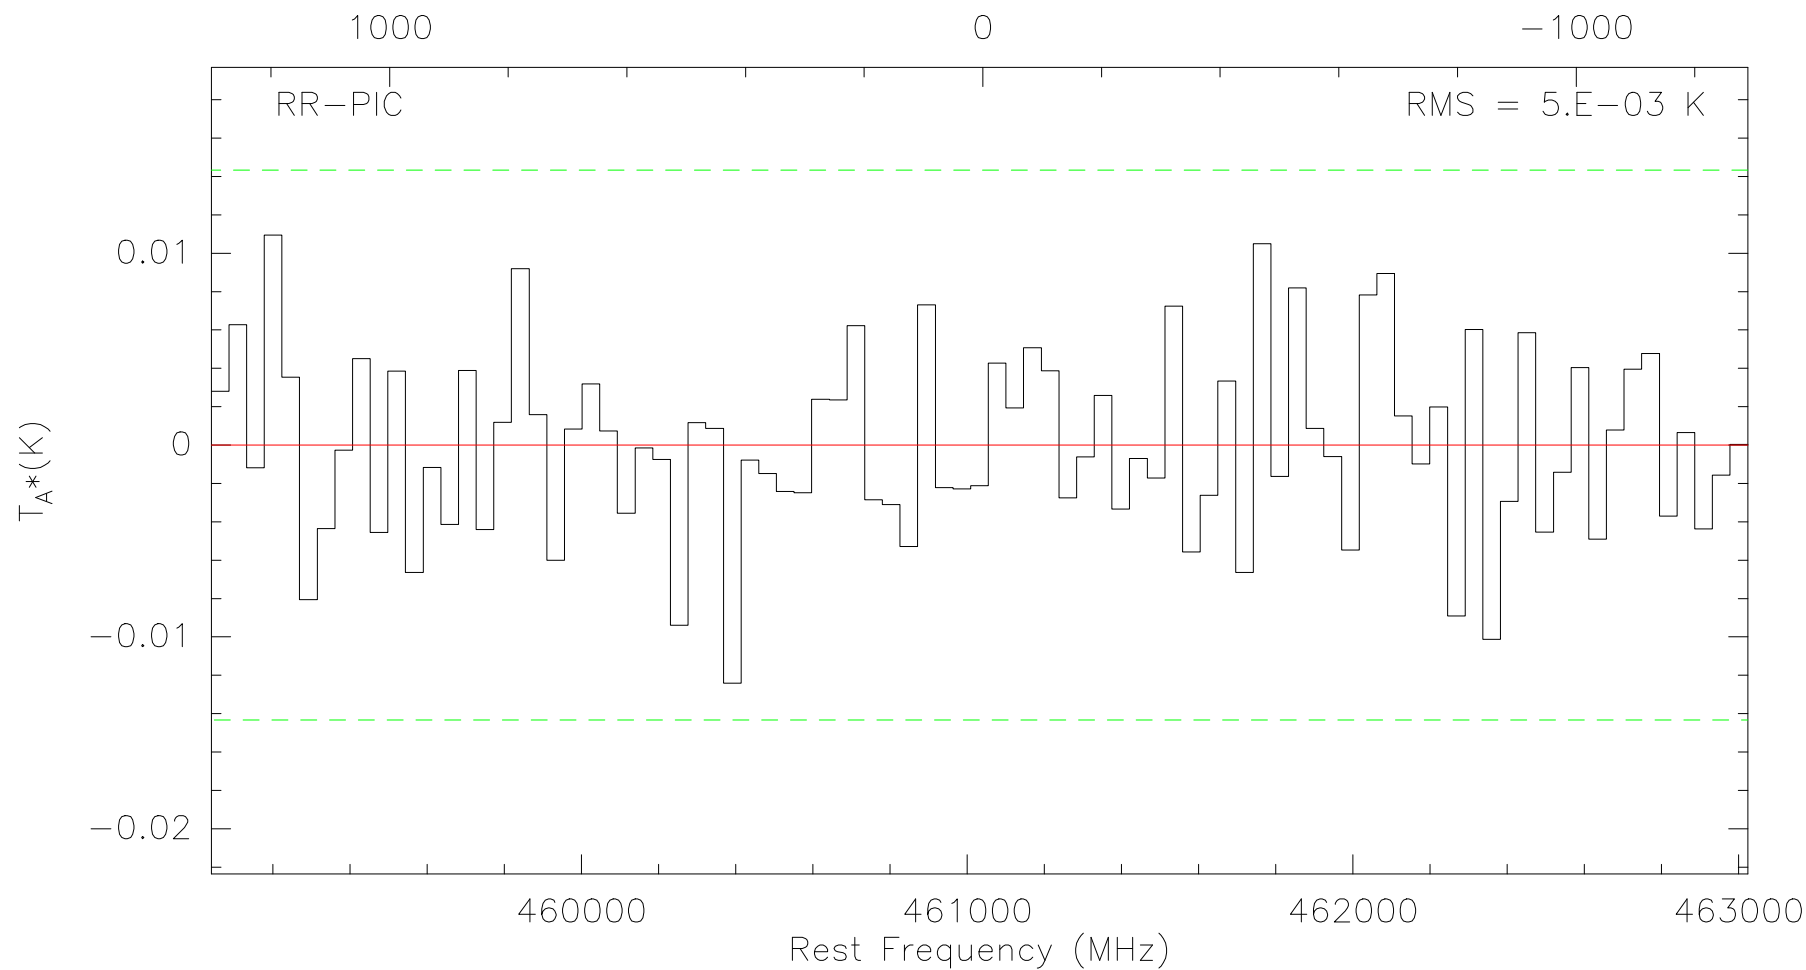

1;1 T-PYX CO(4-3) AP-FL01-XF0- O:24-AUG-2014 R:12-AUG-2020  
RA: 09:04:41.50 DEC: -32:22:47.5 Eq 2000.0 Rad. 0.0° Offs: -0.2 -0.5  
Unknown tau: 0.539 Tsys: 491. Time: 23.4min El: 66.0  
N: 87 IO: 44.1918 V0: 0.000 Dv: -29.77 LSR  
FO: 461040.768 Df: 45.78 Fi: 473041.401

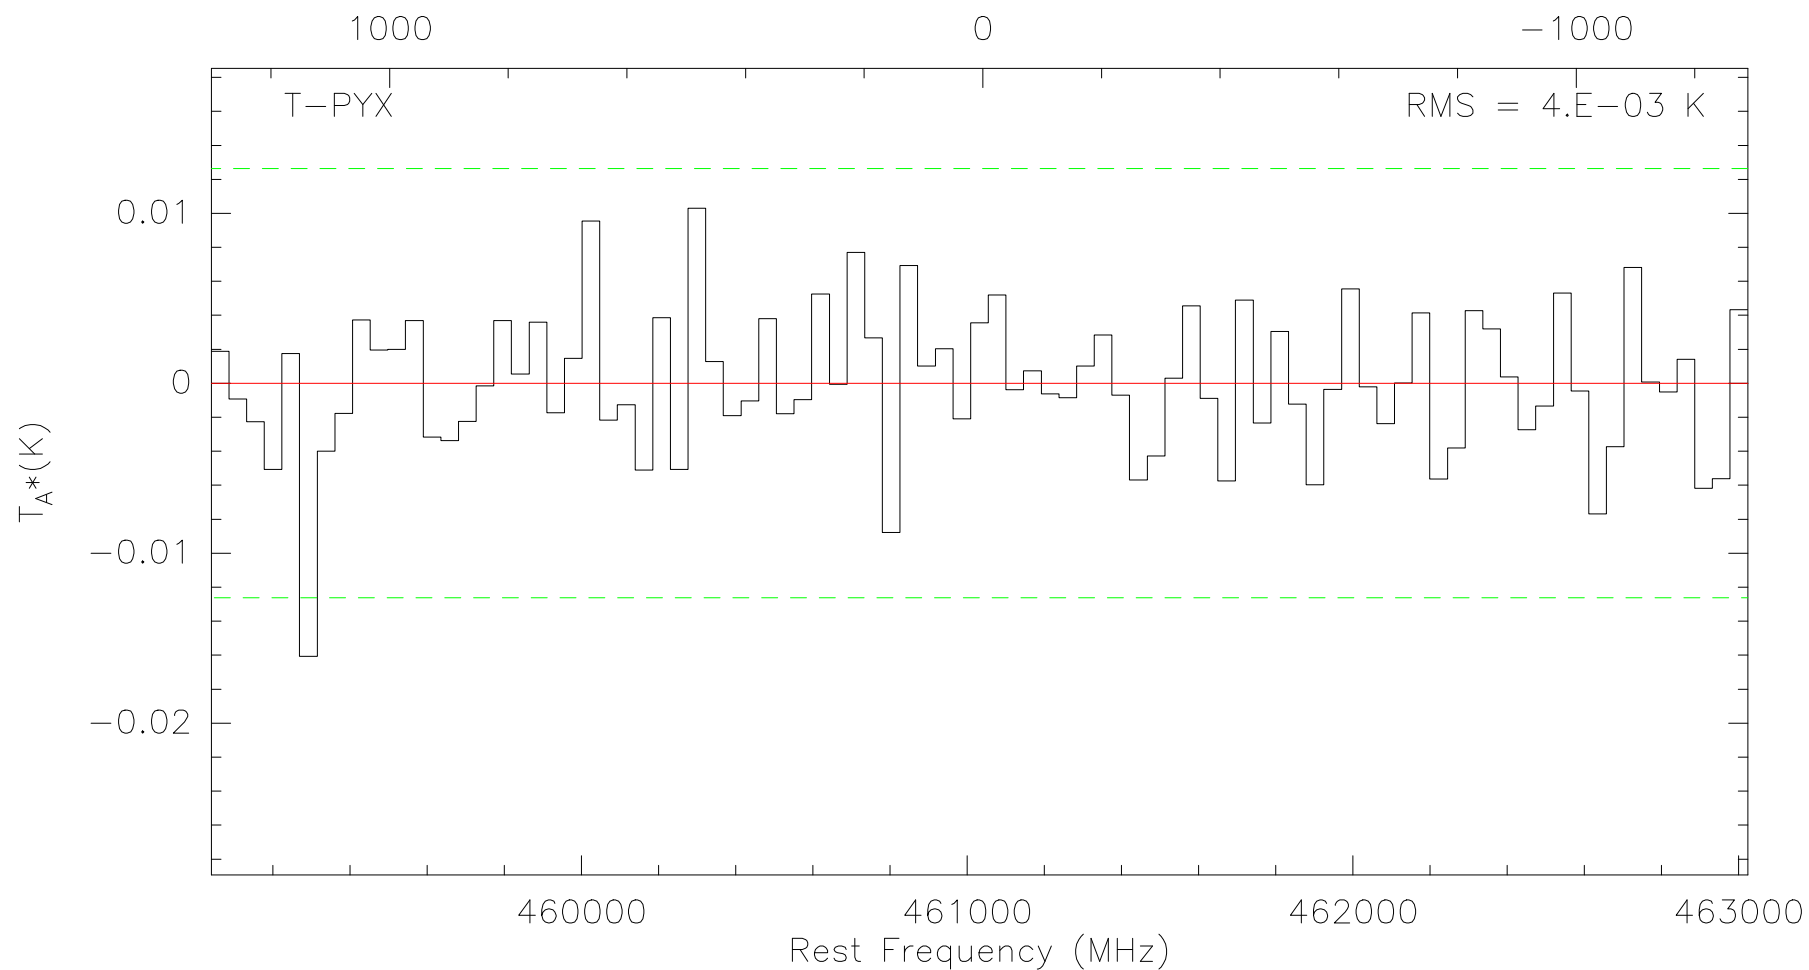

1;1 TV-CRV CO(4-3) AP-FL01-XF0- O:24-AUG-2014 R:12-AUG-2020  
RA: 12:20:24.15 DEC: -18:27:02.0 Eq 2000.0 Rad. 0.0° Offs: +0.2 -0.3  
Unknown tau: 0.486 Tsys: 525. Time: 23.3min El: 51.8  
N: 87 l0: 44.1918 V0: 0.000 Dv: -29.77 LSR  
F0: 461040.768 Df: 45.78 Fi: 473041.572

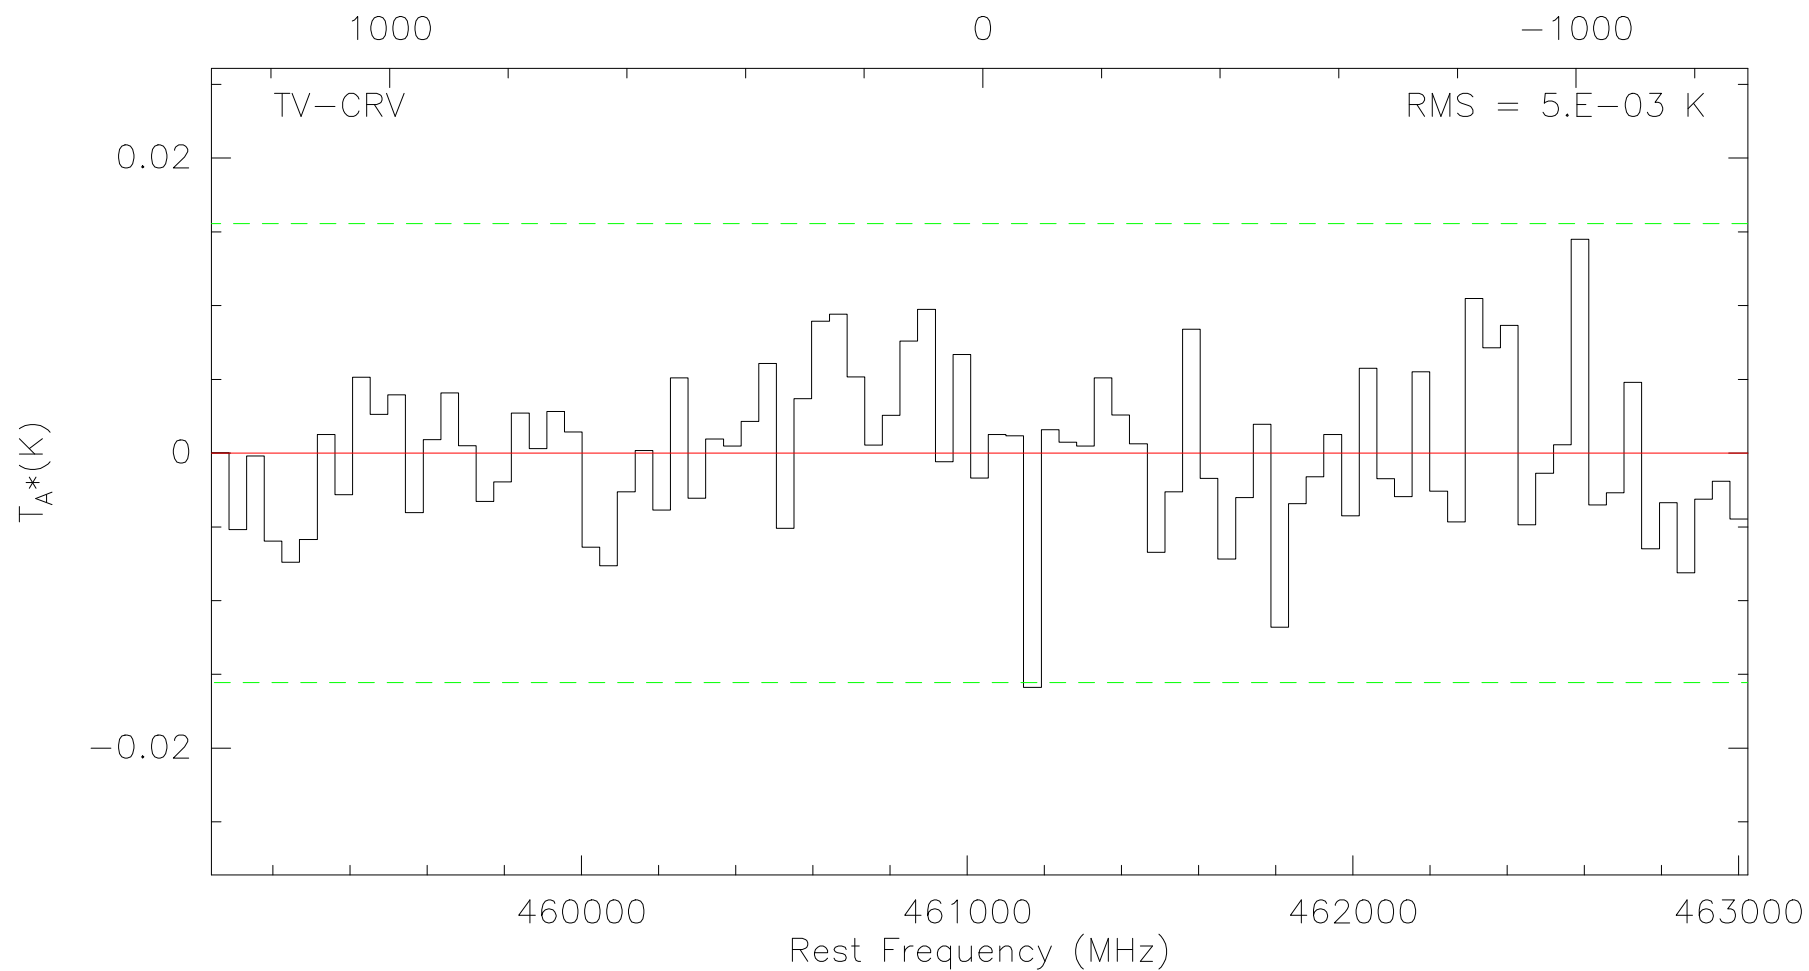

1;1 V1065-CEN CO(4-3) AP-FL01-XF0- 0:24-AUG-2014 R:12-AUG-2020  
RA: 11:43:10.33 DEC: -58:04:04.3 Eq 2000.0 Rad. 0.0° Offs: -0.4 -0.3  
Unknown tau: 0.817 Tsys: 1850. Time: 23.3min El: 30.0  
N: 87 IO: 44.1918 V0: 0.000 Dv: -29.77 LSR  
FO: 461040.768 Df: 45.78 Fi: 473041.755

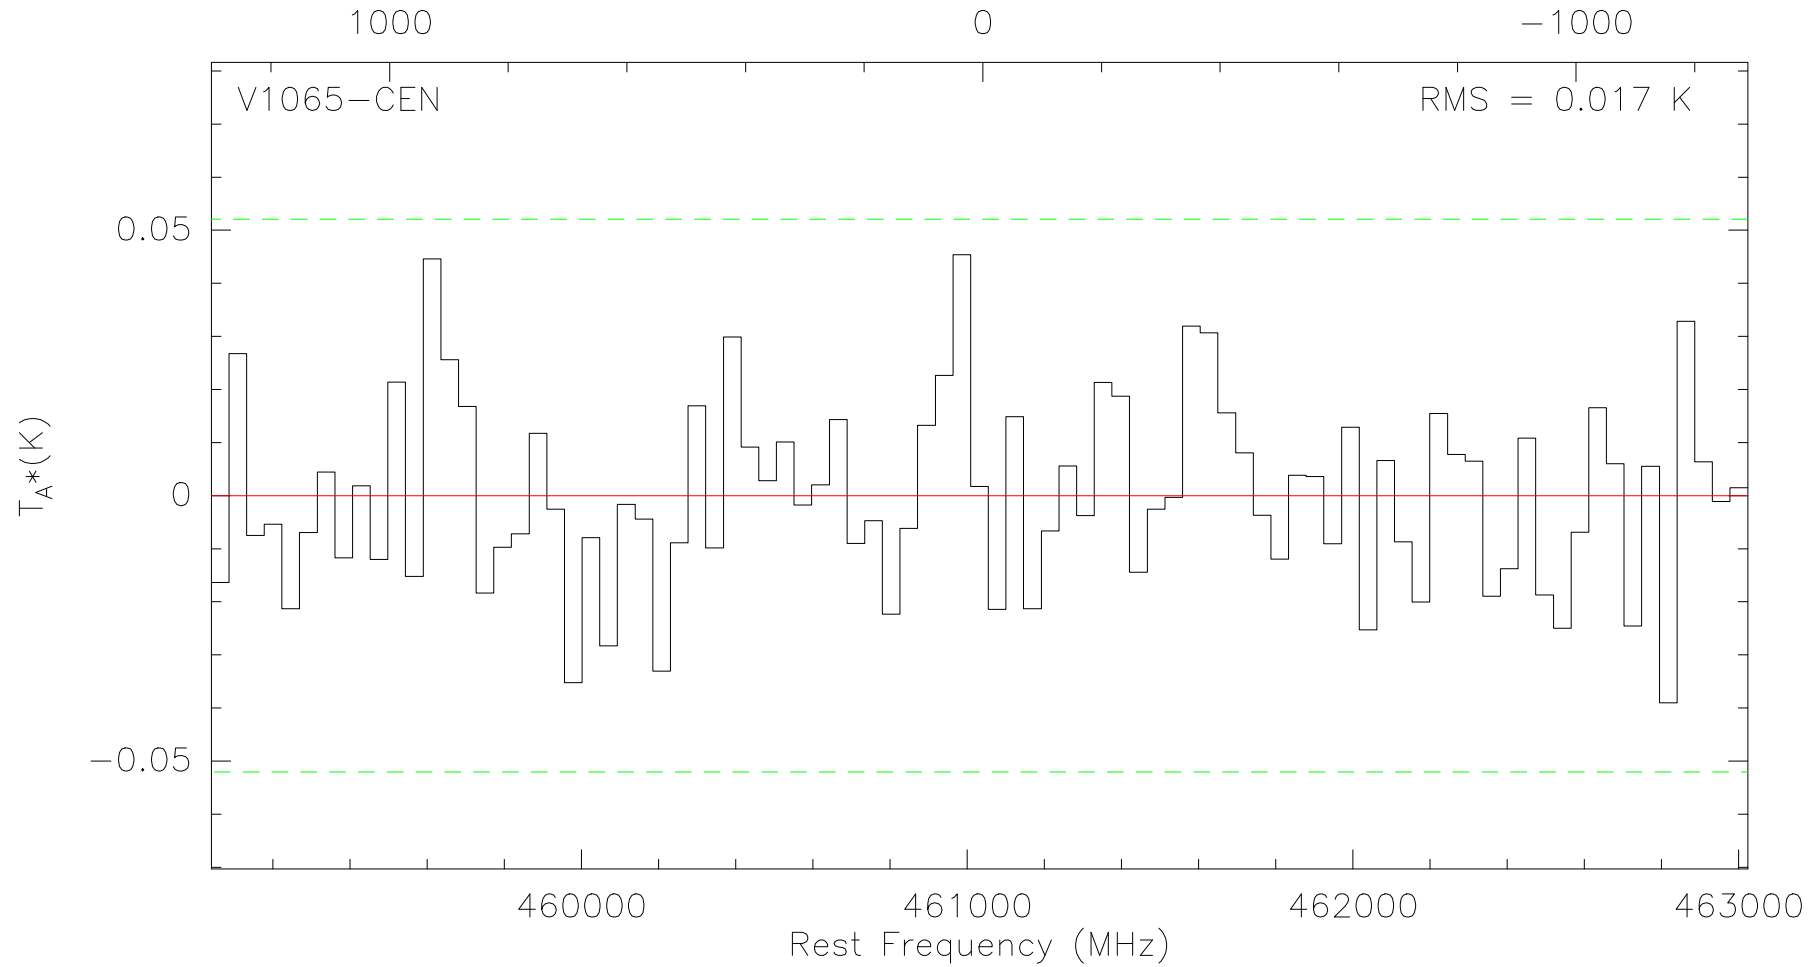

1;1 V351-CAR CO(4-3) AP-FL01-XF0- O:28-AUG-2014 R:12-AUG-2020  
RA: 10:45:19.14 DEC: -72:03:56.0 Eq 2000.0 Rad. 0.0° Offs: +0.2 -0.4  
Unknown tau: 0.739 Tsys: 1040. Time: 23.4min El: 40.8  
N: 87 IO: 44.1918 V0: 0.000 Dv: -29.77 LSR  
FO: 461040.768 Df: 45.78 Fi: 473041.671

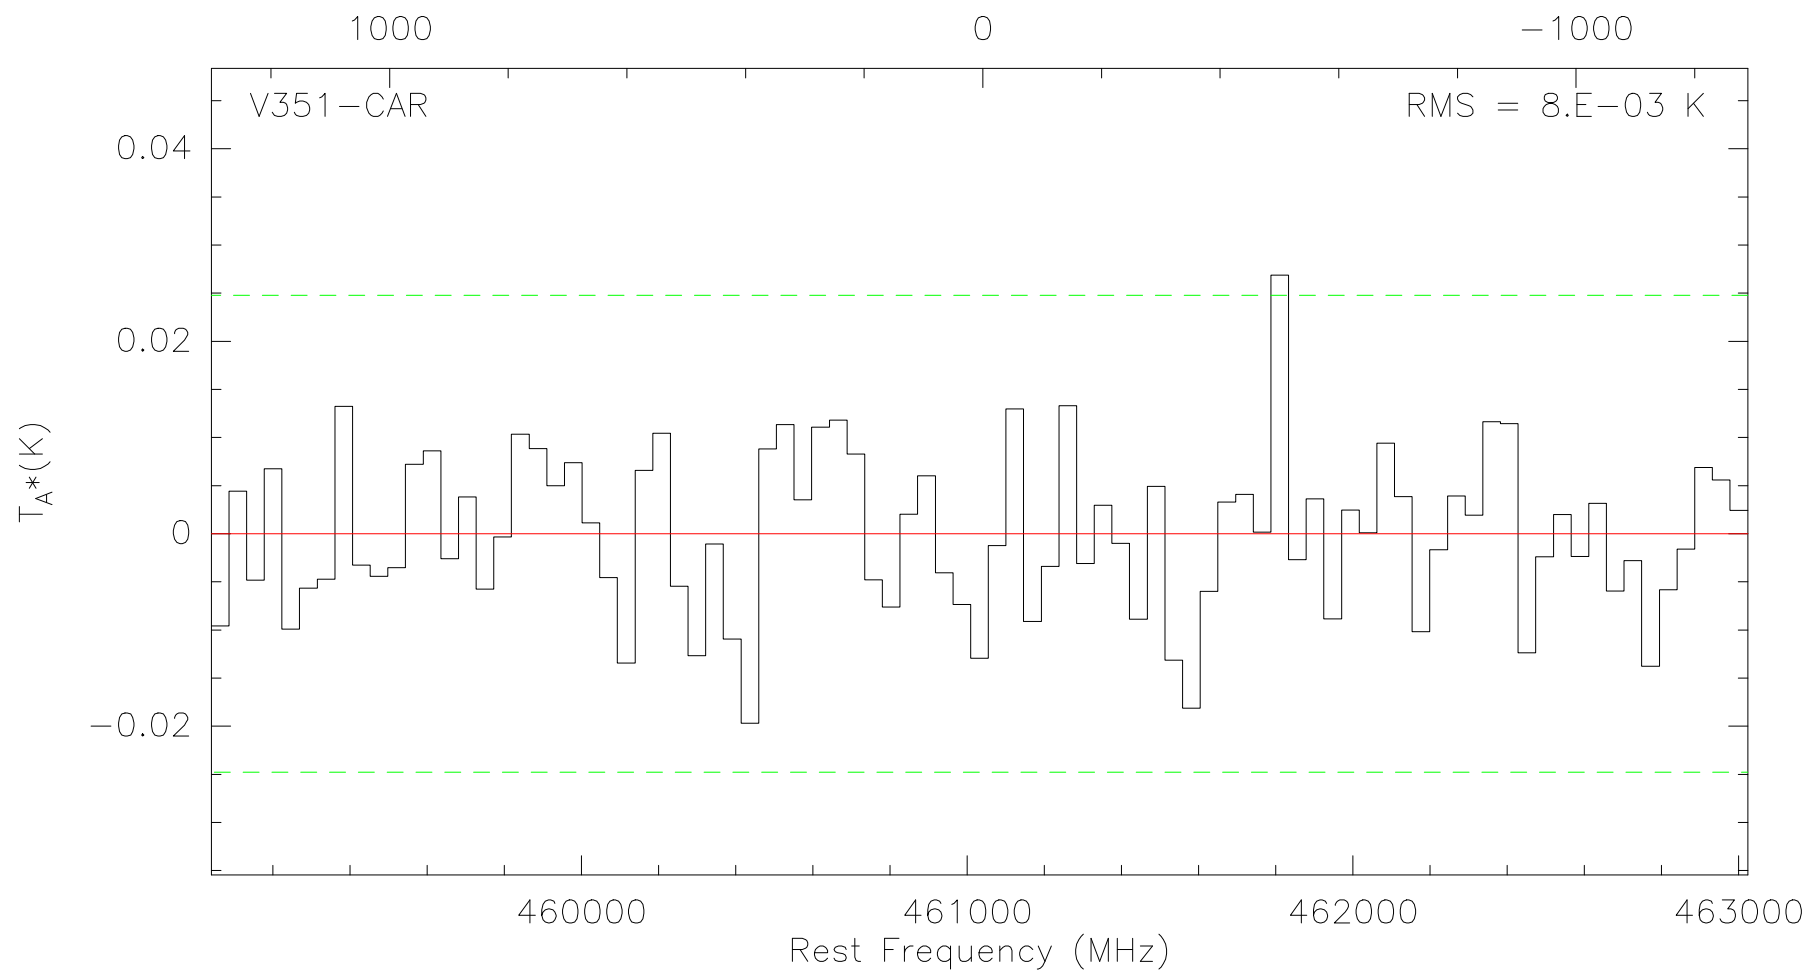

1;1 V359-CEN CO(4-3) AP-FL01-XF0- O:24-AUG-2014 R:12-AUG-2020  
RA: 11:58:15.33 DEC: -41:46:08.4 Eq 2000.0 Rad. 0.0° Offs: +0.2 -0.4  
Unknown tau: 0.525 Tsys: 497. Time: 23.4min El: 70.8  
N: 87 IO: 44.1918 V0: 0.000 Dv: -29.77 LSR  
FO: 461040.768 Df: 45.78 Fi: 473041.729

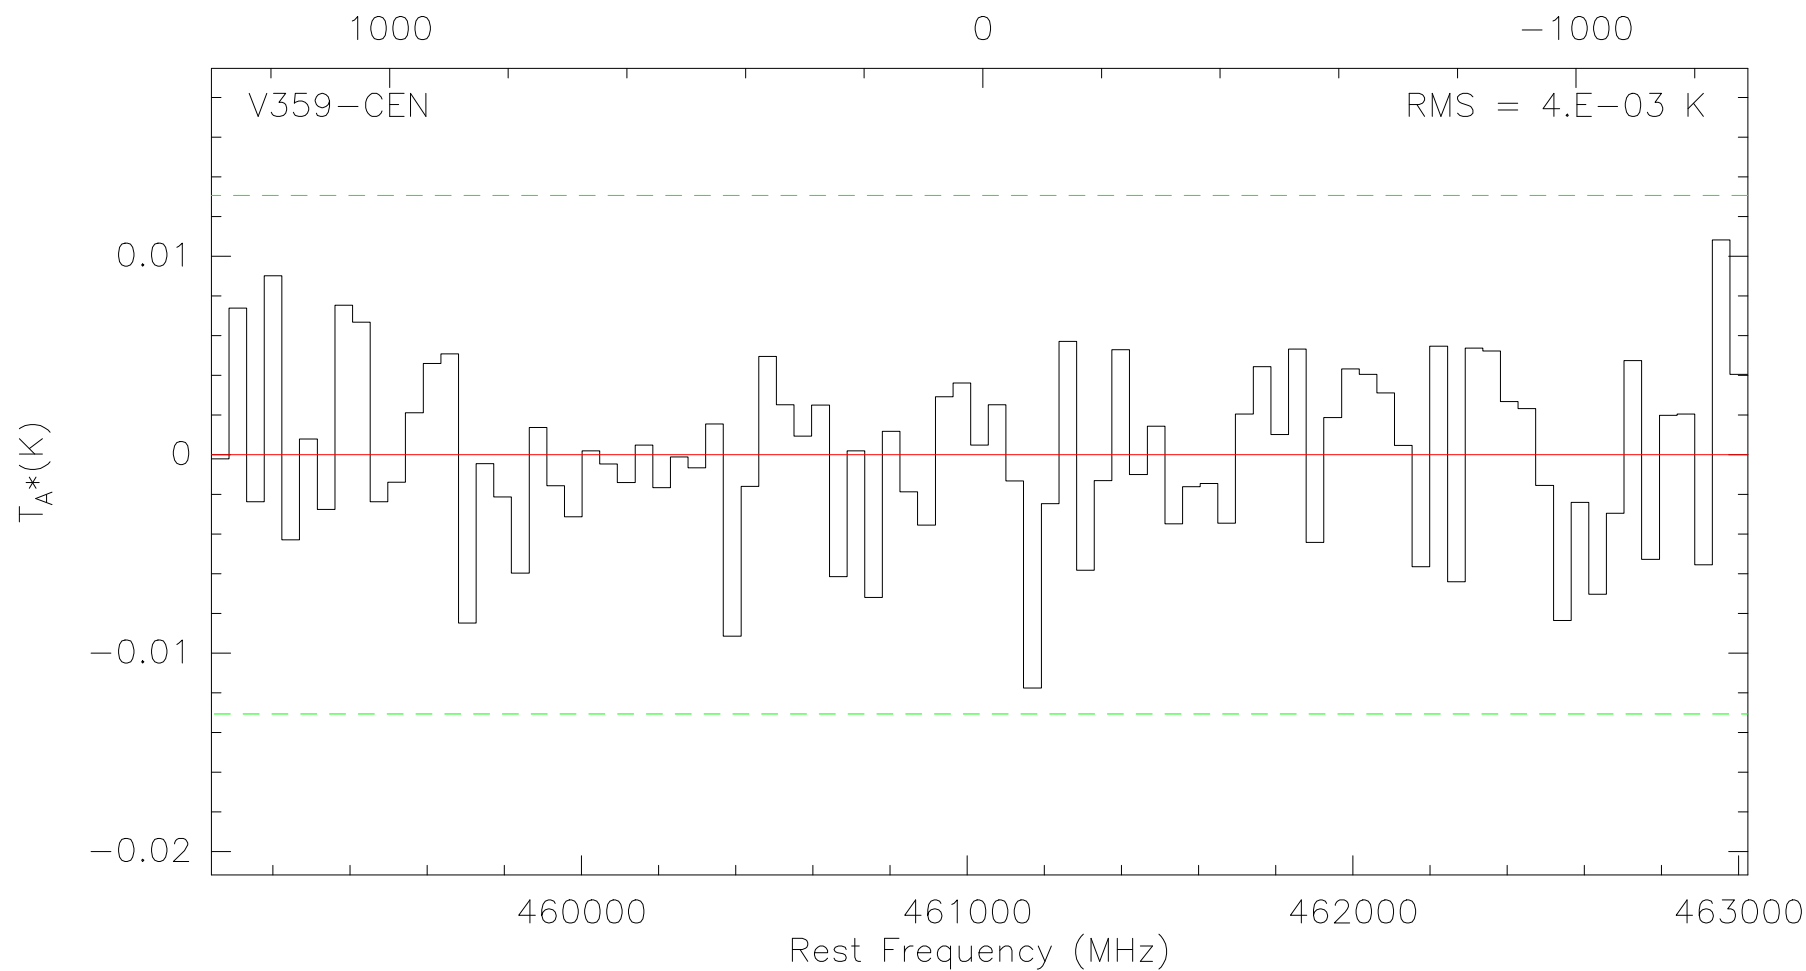

1;1 V382-VEL CO(4-3) AP-FL01-XF0- 0:08-SEP-2014 R:14-AUG-2020

RA: 10:44:48.39 DEC: -52:25:30.7 Eq 2000.0 Rad. 0.0° Offs: +0.3 -0.4

Unknown tau: 0.714 Tsys: 794. Time: 61.4min El: 57.9

N: 87 IO: 44.1918 V0: 0.000 Dv: -29.77 LSR

F0: 461040.768 Df: 45.78 Fi: 473041.649

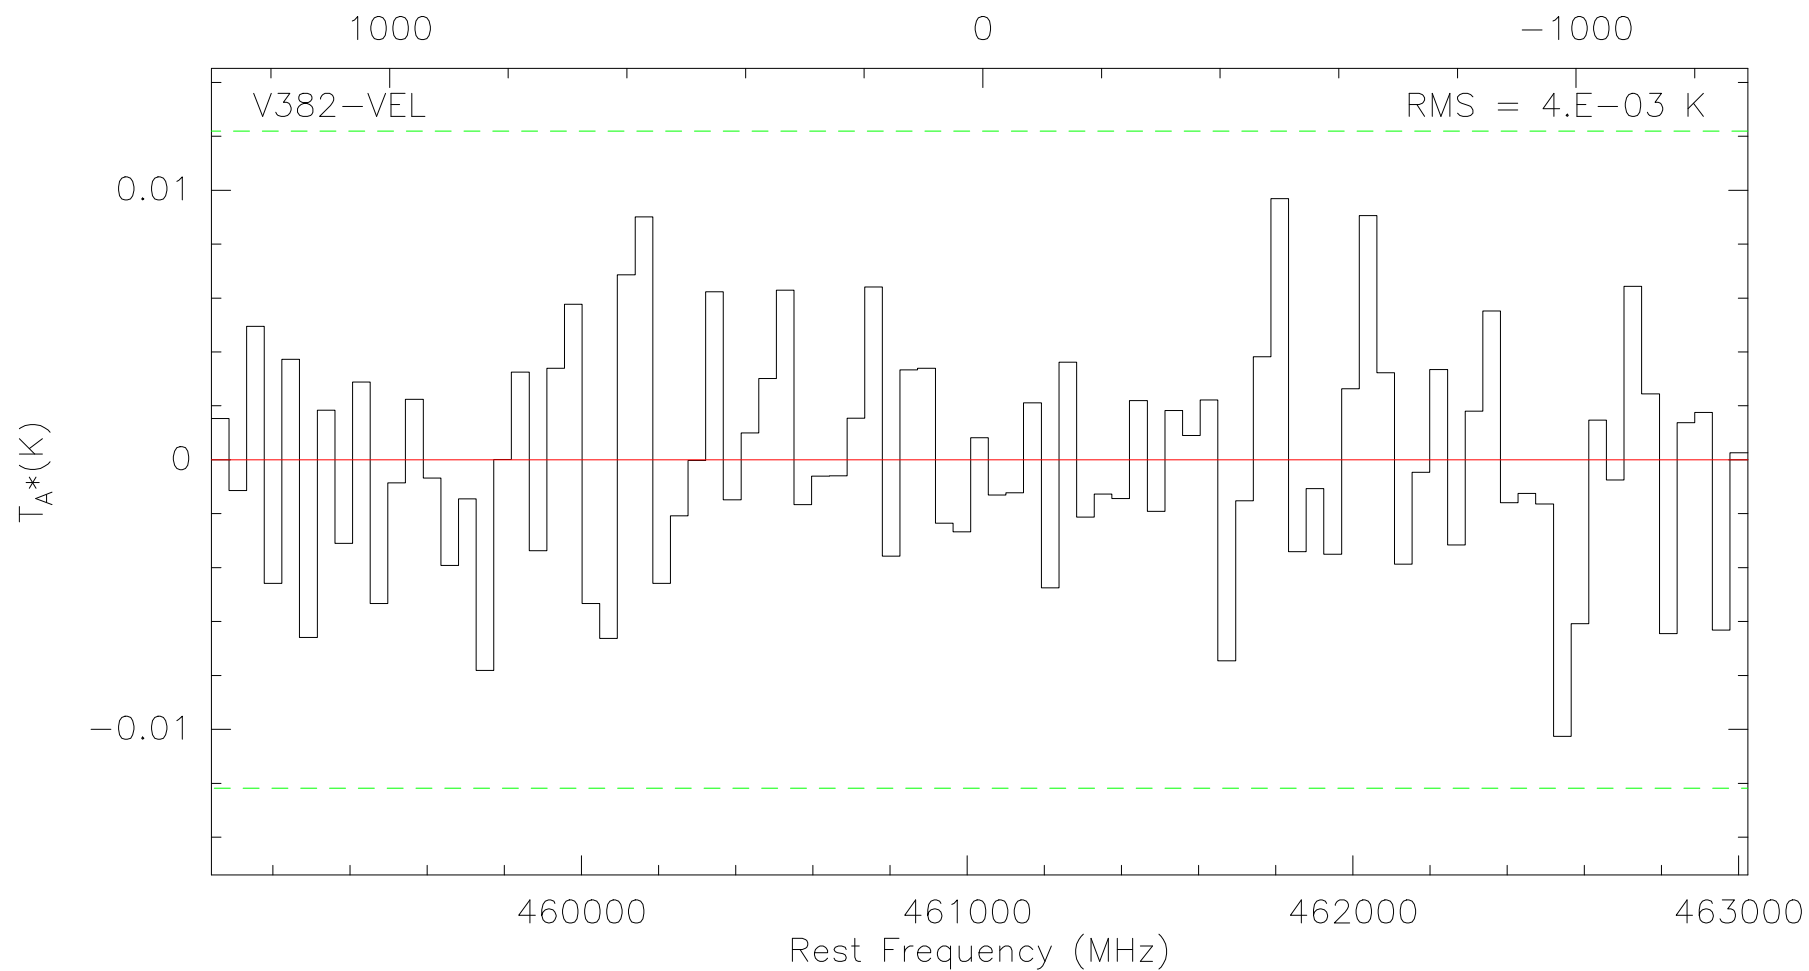

1;1 V598-PUP CO(4-3) AP-FL01-XF0- O:25-AUG-2014 R:12-AUG-2020  
RA: 07:05:42.50 DEC: -38:14:39.4 Eq 2000.0 Rad. 0.0° Offs: +0.2 -0.3  
Unknown tau: 0.431 Tsys: 428. Time: 23.4min El: 59.6  
N: 87 l0: 44.1918 V0: 0.000 Dv: -29.77 LSR  
F0: 461040.768 Df: 45.78 Fi: 473041.186

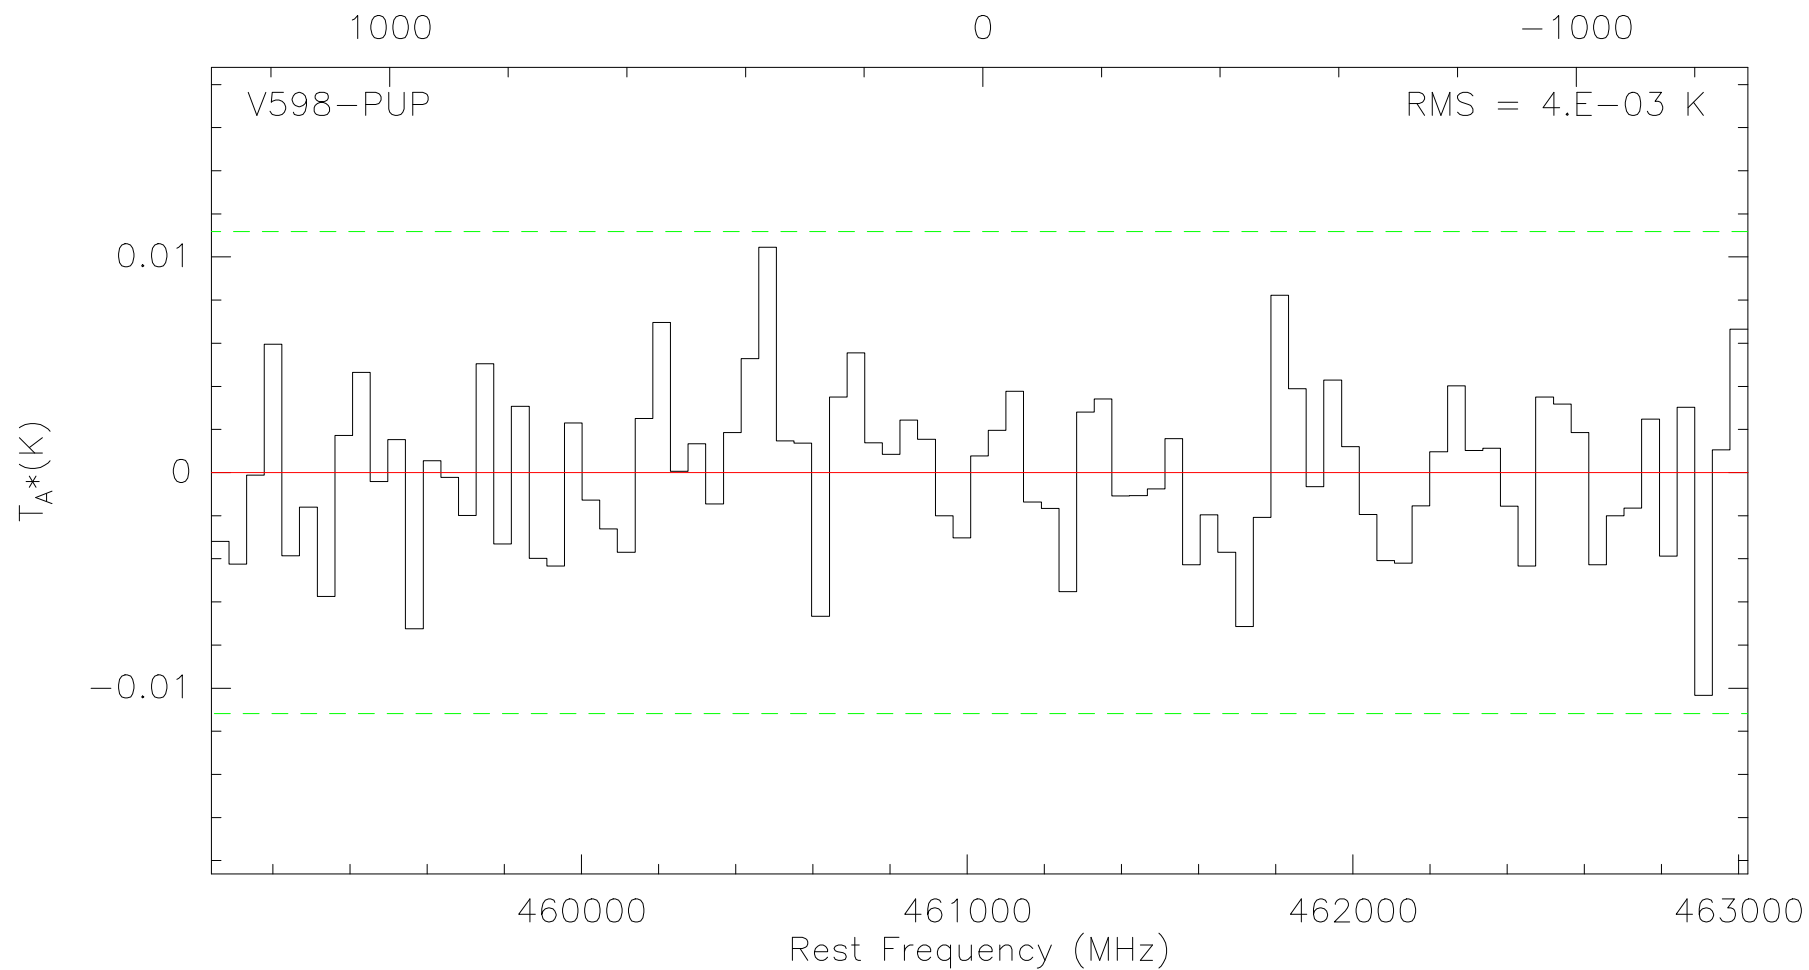

1;1 VX-FOR CO(4-3) AP-FL01-XF0- O:24-AUG-2014 R:12-AUG-2020  
RA: 03:26:45.71 DEC: -34:26:25.2 Eq 2000.0 Rad. 0.0° Offs: +0.2 -0.2  
Unknown tau: 0.782 Tsys: 764. Time: 23.3min El: 53.4  
N: 87 IO: 44.1918 V0: 0.000 Dv: -29.77 LSR  
FO: 461040.768 Df: 45.78 Fi: 473040.757

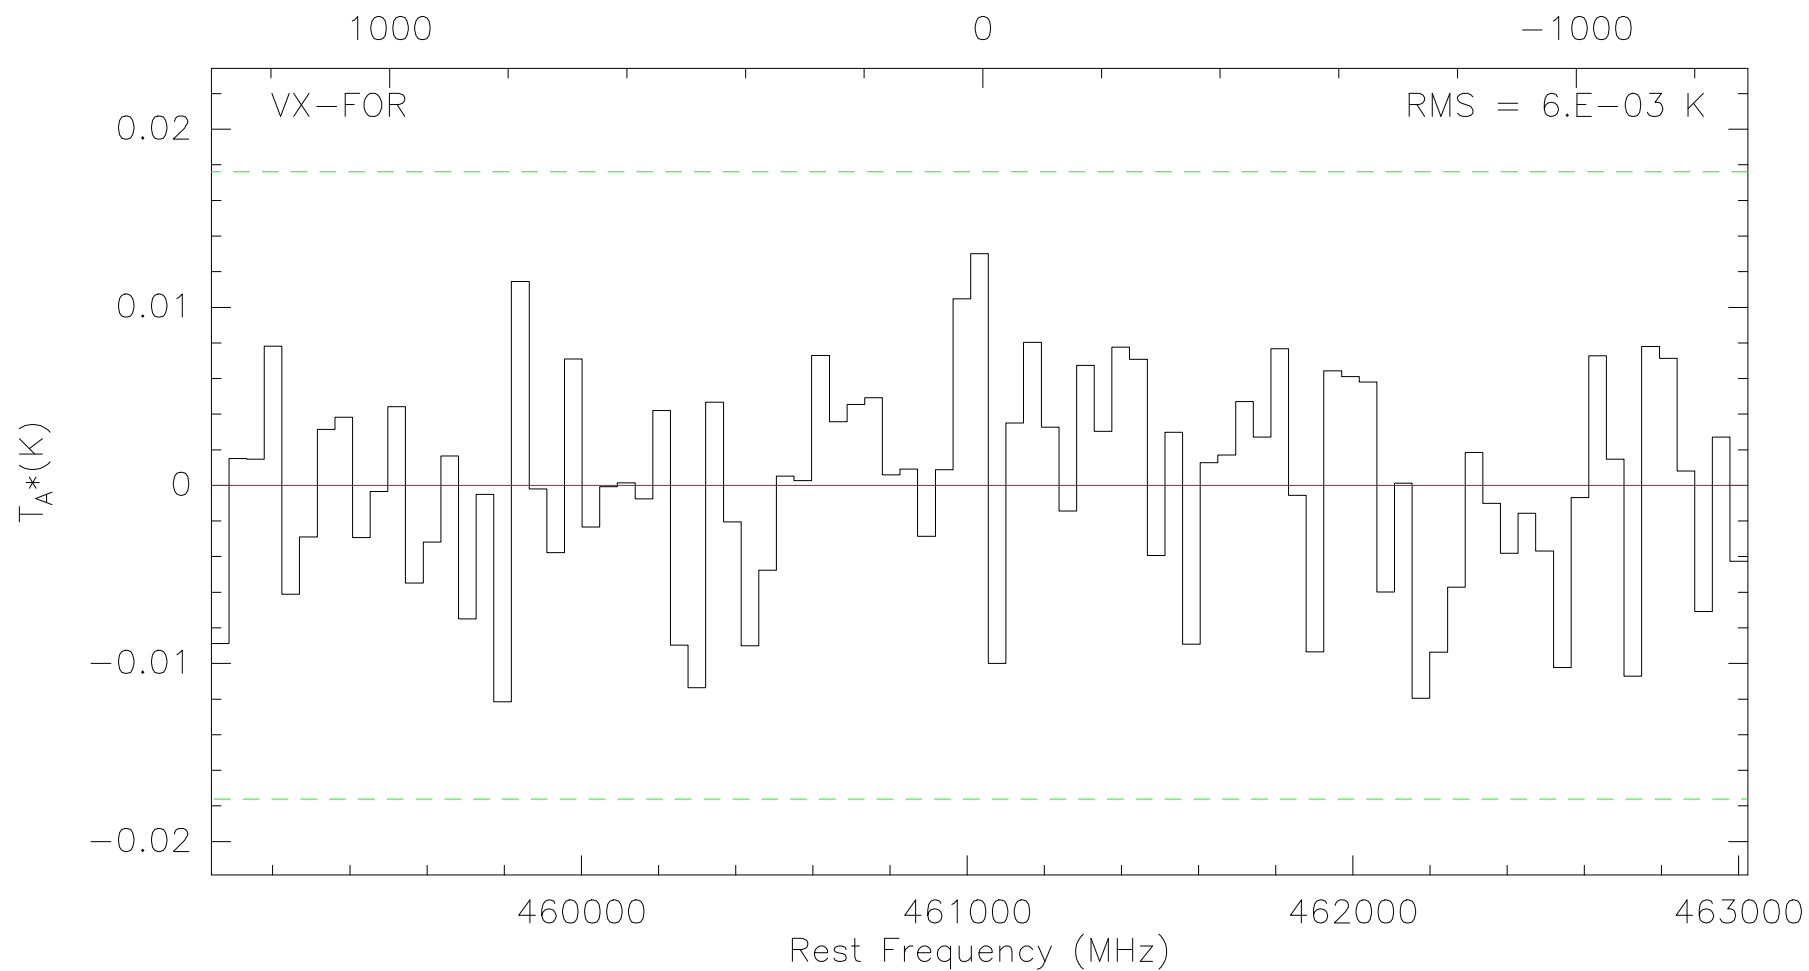

1;1 WX-CET CO(4-3) AP-FL01-XF0- O:24-AUG-2014 R:12-AUG-2020  
RA: 01:17:04.17 DEC: -17:56:23.0 Eq 2000.0 Rad. 0.0° Offs: -0.2 -0.3  
Unknown tau: 0.554 Tsys: 489. Time: 23.3min El: 67.5  
N: 87 l0: 44.1918 V0: 0.000 Dv: -29.77 LSR  
F0: 461040.768 Df: 45.78 Fi: 473040.428

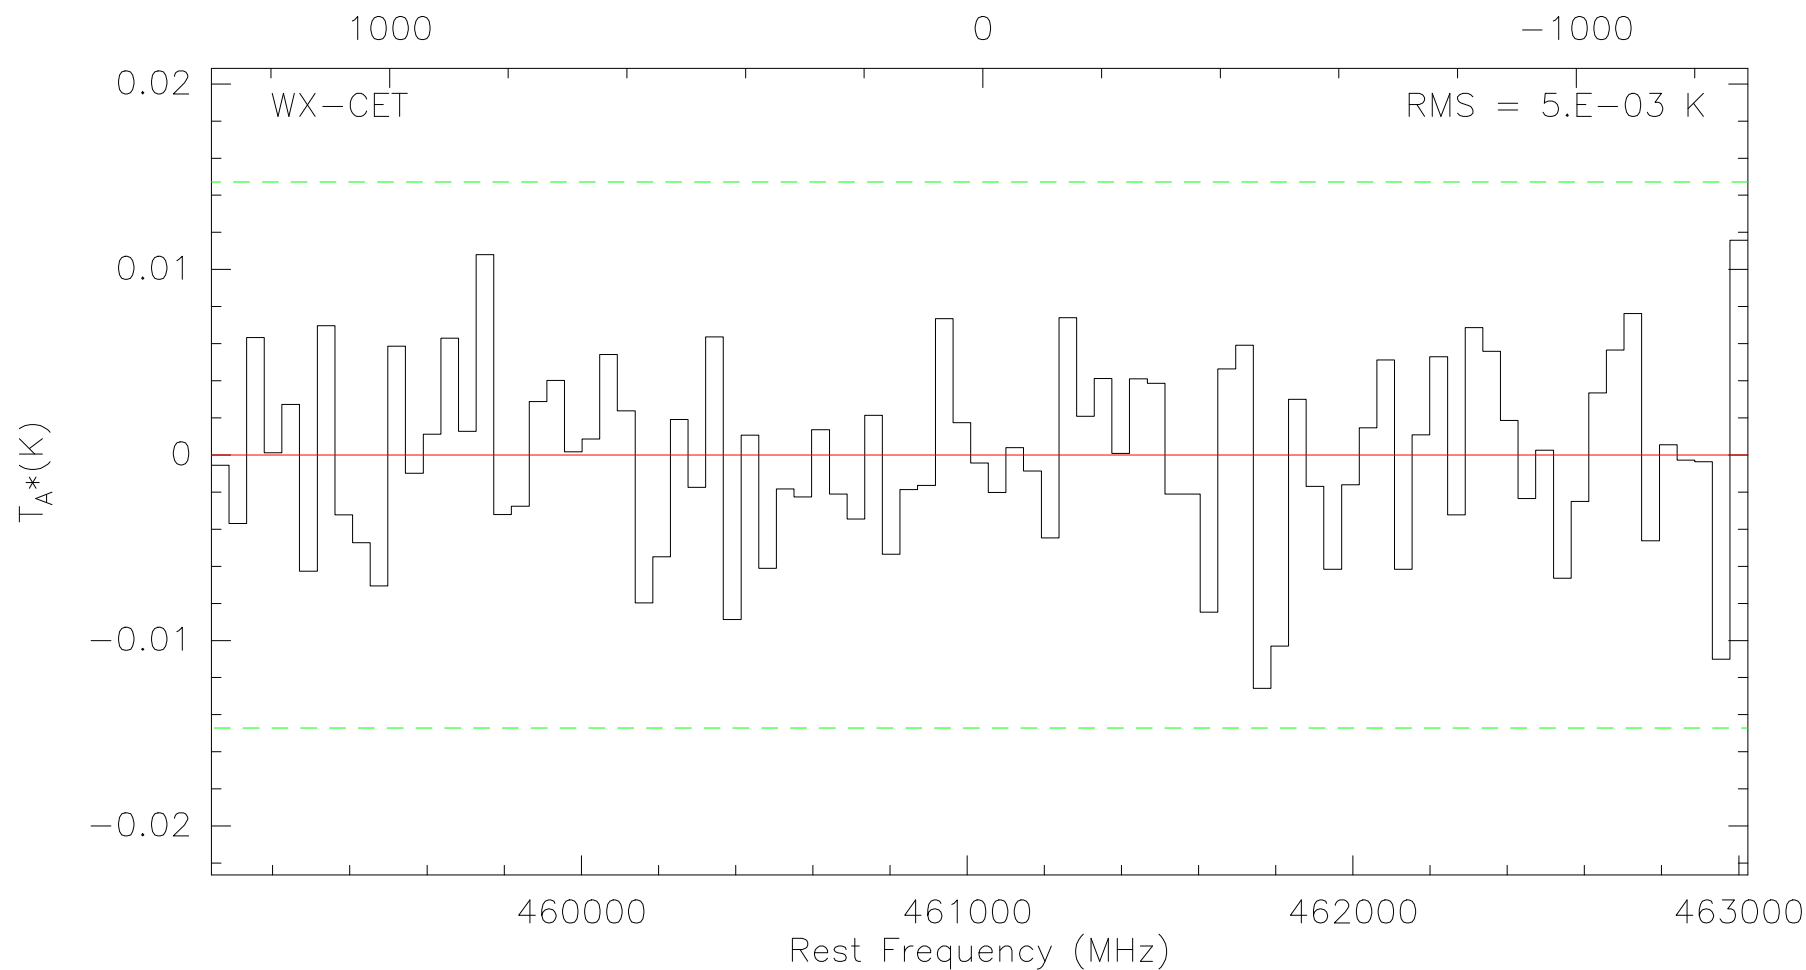

1;1 AICIR CO(4-3) AP-FL01-XF0- O:13-JUL-2016 R:07-AUG-2020  
RA: 14:49:31.29 DEC: -68:51:35.9 Eq 2000.0 Rad. 0.0° Offs: +0.5 -0.2  
Unknown tau: 0.735 Tsys: 1331. Time: 5.0min El: 33.7  
N: 87 IO: 44.1918 V0: 0.000 Dv: -29.77 LSR  
FO: 461040.768 Df: 45.78 Fi: 473041.520

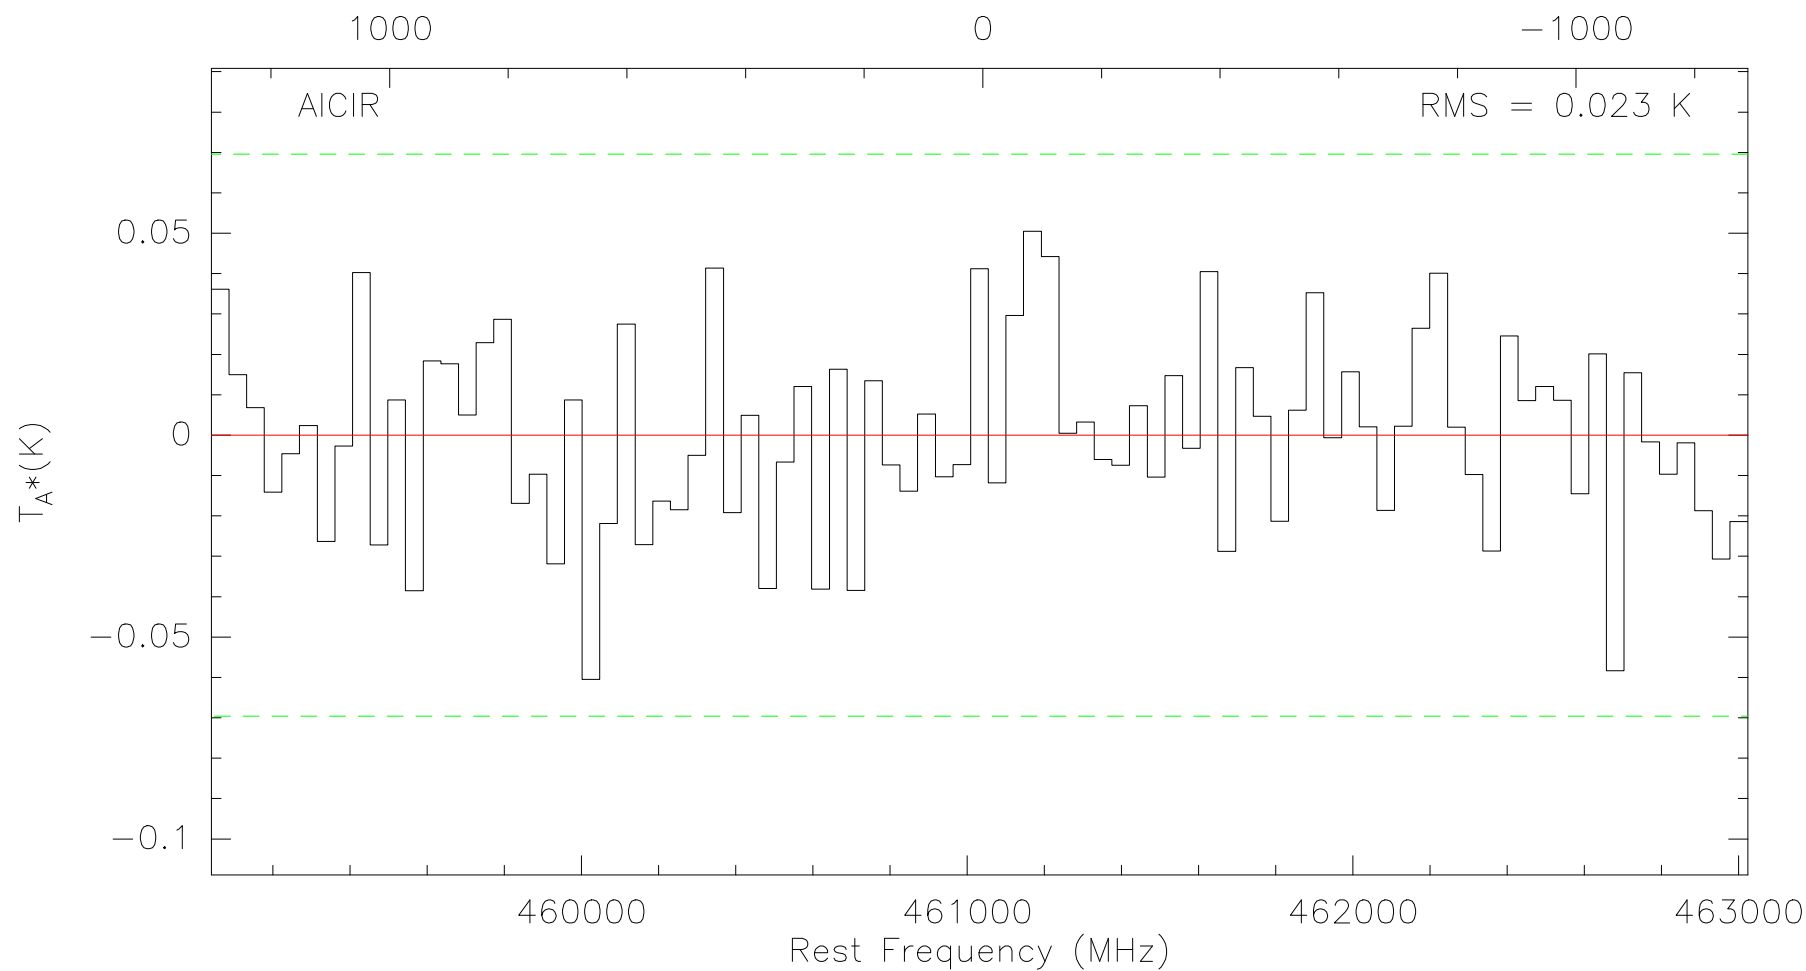

1;1 ATSGR CO(4-3) AP-FL01-XF0- 0:14-JUL-2016 R:07-AUG-2020  
RA: 18:03:30.87 DEC: -26:28:28.5 Eq 2000.0 Rad. 0.0° Offs: +0.1 -0.4  
Unknown tau: 0.778 Tsys: 709. Time: 9.9min El: 66.9  
N: 87 IO: 44.1918 V0: 0.000 Dv: -29.77 LSR  
FO: 461040.768 Df: 45.78 Fi: 473040.742

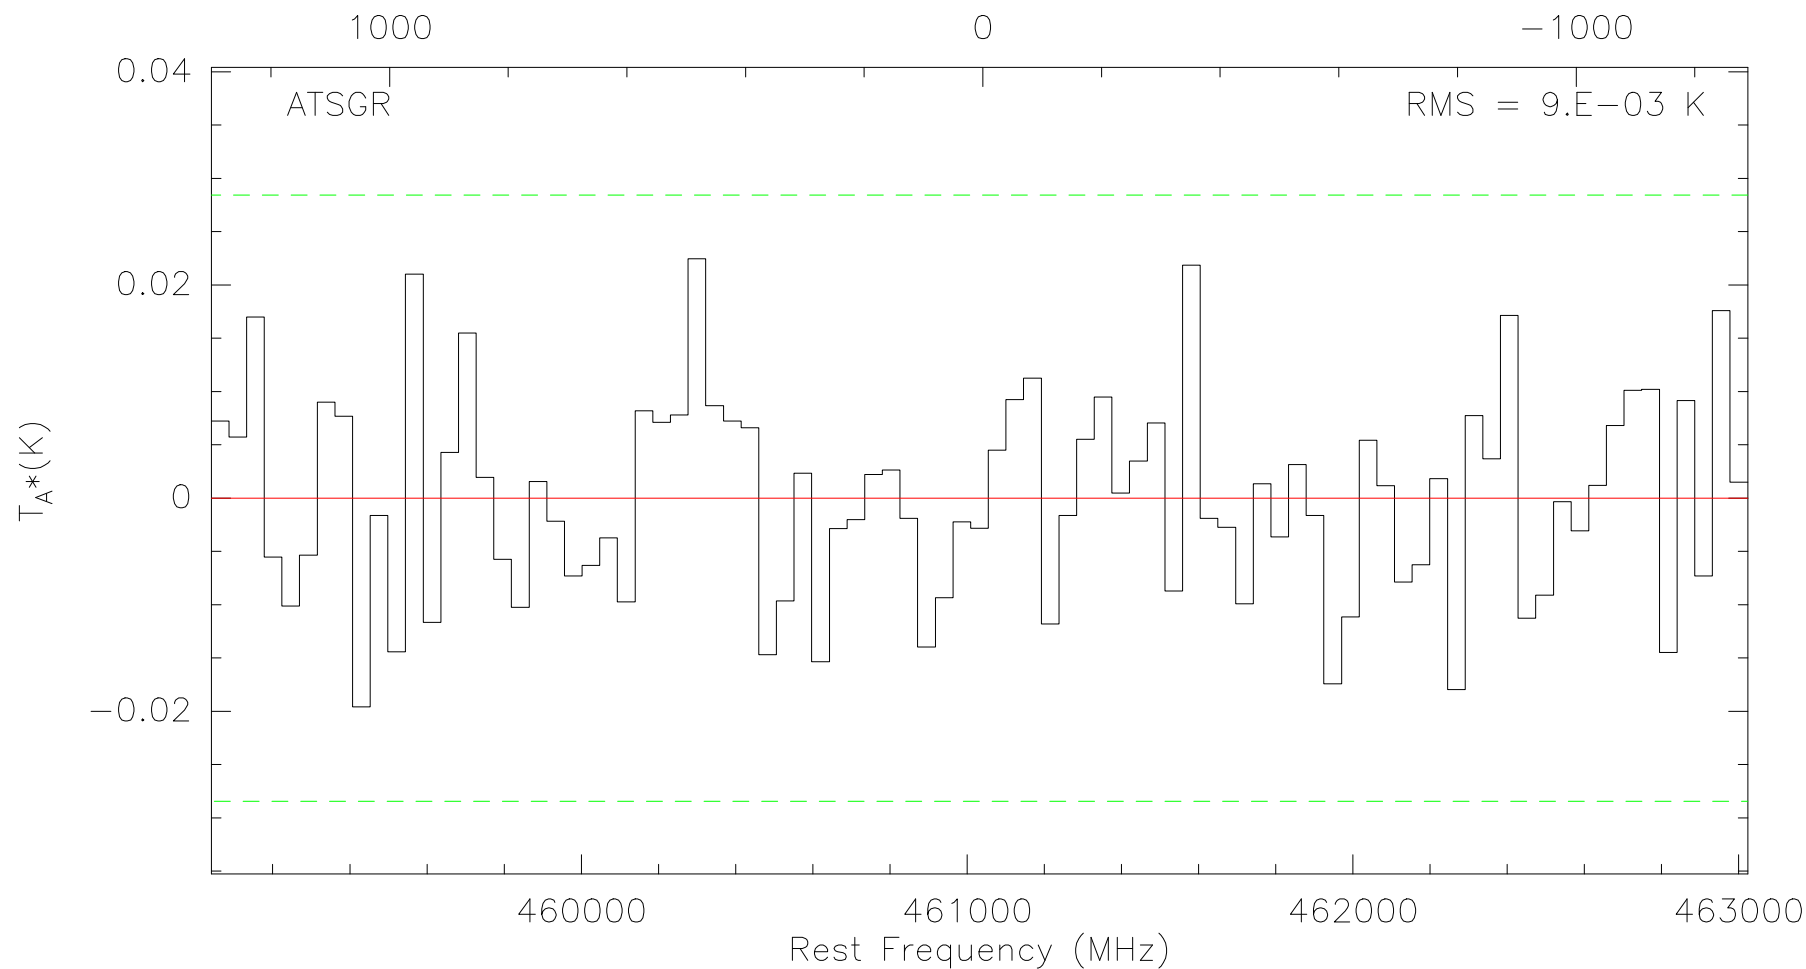

1;1 FMSGF CO(4-3) AP-FL01-XF0- O:13-JUL-2016 R:07-AUG-2020  
RA: 18:17:18.10 DEC: -23:38:27.0 Eq 2000.0 Rad. 0.0° Offs: -0.1 -0.4  
Unknown tau: 0.474 Tsys: 646. Time: 9.9min El: 35.9  
N: 87 IO: 44.1918 V0: 0.000 Dv: -29.77 LSR  
F0: 461040.768 Df: 45.78 Fi: 473040.657

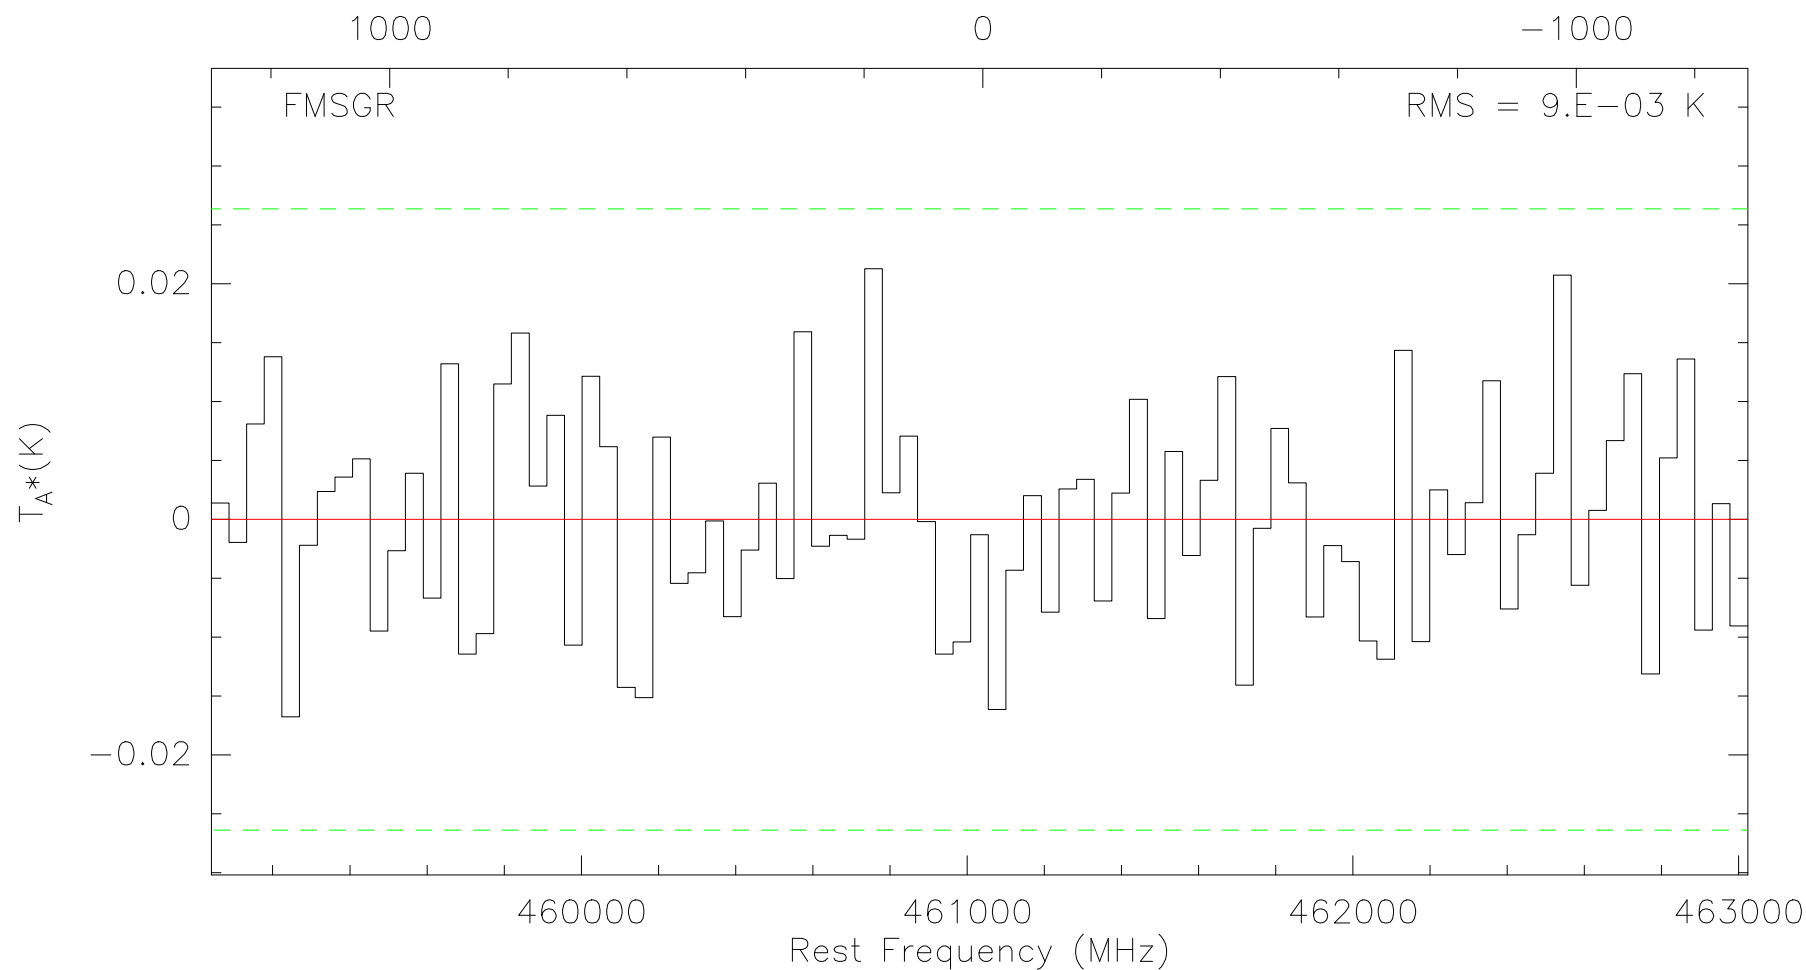

1;1 GRSR CO(4-3) AP-FL01-XF0- O:13-JUL-2016 R:07-AUG-2020  
RA: 18:22:58.50 DEC: -25:34:47.3 Eq 2000.0 Rad. 0.0° Offs: -0.1 -0.5  
Unknown tau: 0.517 Tsys: 489. Time: 9.9min El: 58.2  
N: 87 IO: 44.1918 V0: 0.000 Dv: -29.77 LSR  
FO: 461040.768 Df: 45.78 Fi: 473040.649

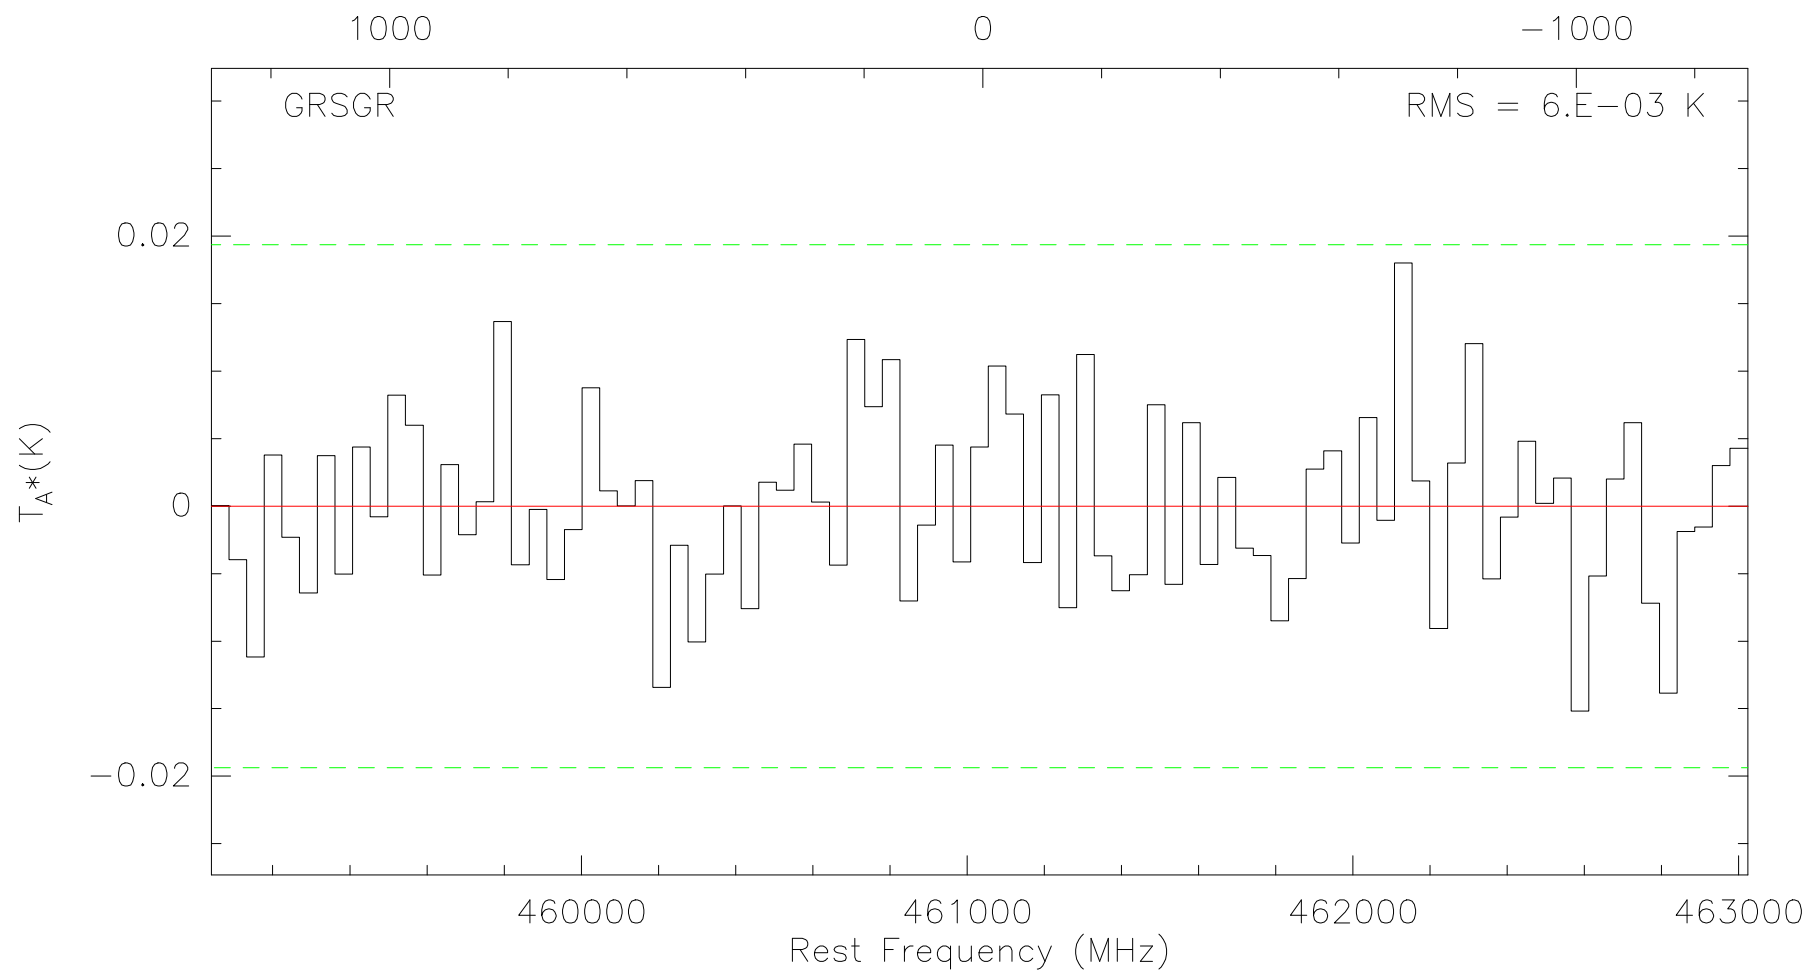

1;1 HSSGR CO(4-3) AP-FL01-XF0- O:13-JUL-2016 R:07-AUG-2020  
RA: 18:28:03.44 DEC: -21:34:24.7 Eq 2000.0 Rad. 0.0° Offs: -0.3 -0.3  
Unknown tau: 0.445 Tsys: 787. Time: 9.9min El: 27.0  
N: 87 IO: 44.1918 V0: 0.000 Dv: -29.77 LSR  
FO: 461040.768 Df: 45.78 Fi: 473040.588

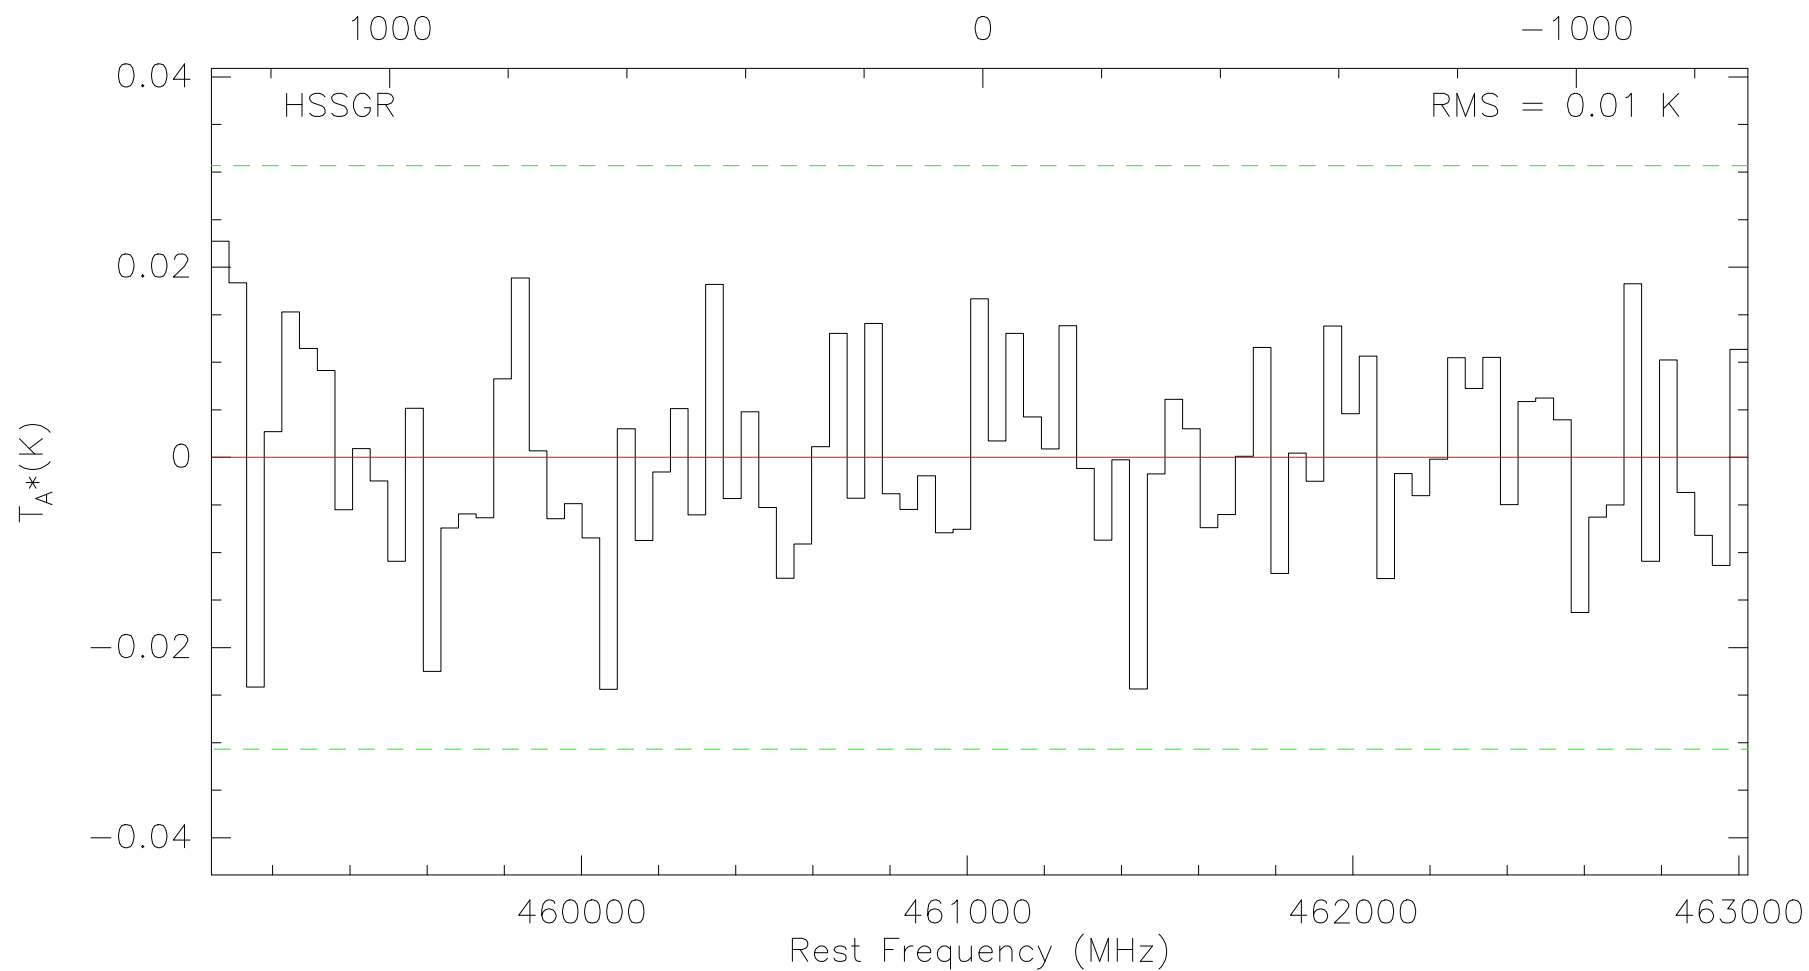

1;1 ILNOR CO(4-3) AP-FL01-XF0- 0:07-JUL-2016 R:07-AUG-2020  
RA: 15:29:23.18 DEC: -50:35:00.7 Eq 2000.0 Rad. 0.0° Offs: -0.2 -0.5  
Unknown tau: 0.761 Tsys: 827. Time: 9.9min El: 52.2  
N: 87 IO: 44.1918 V0: 0.000 Dv: -29.77 LSR  
FO: 461040.768 Df: 45.78 Fi: 473041.415

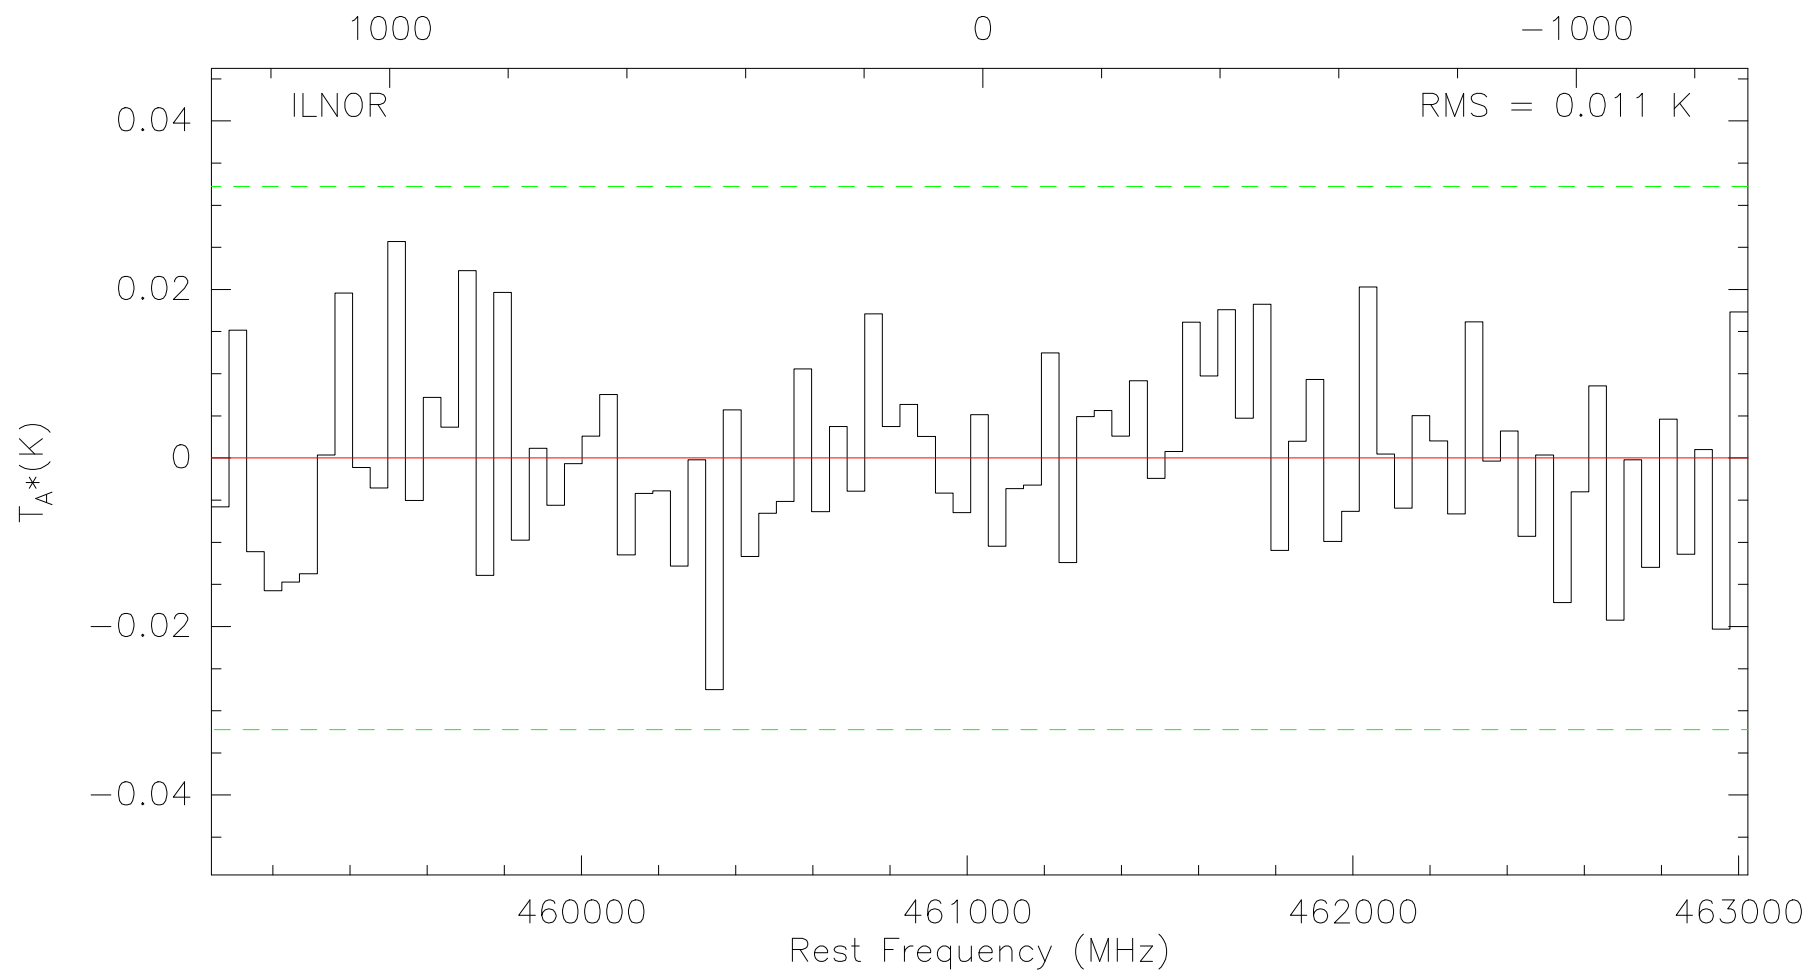

1;1 IMNOR CO(4-3) AP-FL01-XF0- 0:07-JUL-2016 R:07-AUG-2020  
RA: 15:39:26.46 DEC: -52:19:17.9 Eq 2000.0 Rad. 0.0° Offs: -0.2 -0.5  
Unknown tau: 0.752 Tsys: 767. Time: 9.9min El: 54.7  
N: 87 IO: 44.1918 V0: 0.000 Dv: -29.77 LSR  
FO: 461040.768 Df: 45.78 Fi: 473041.384

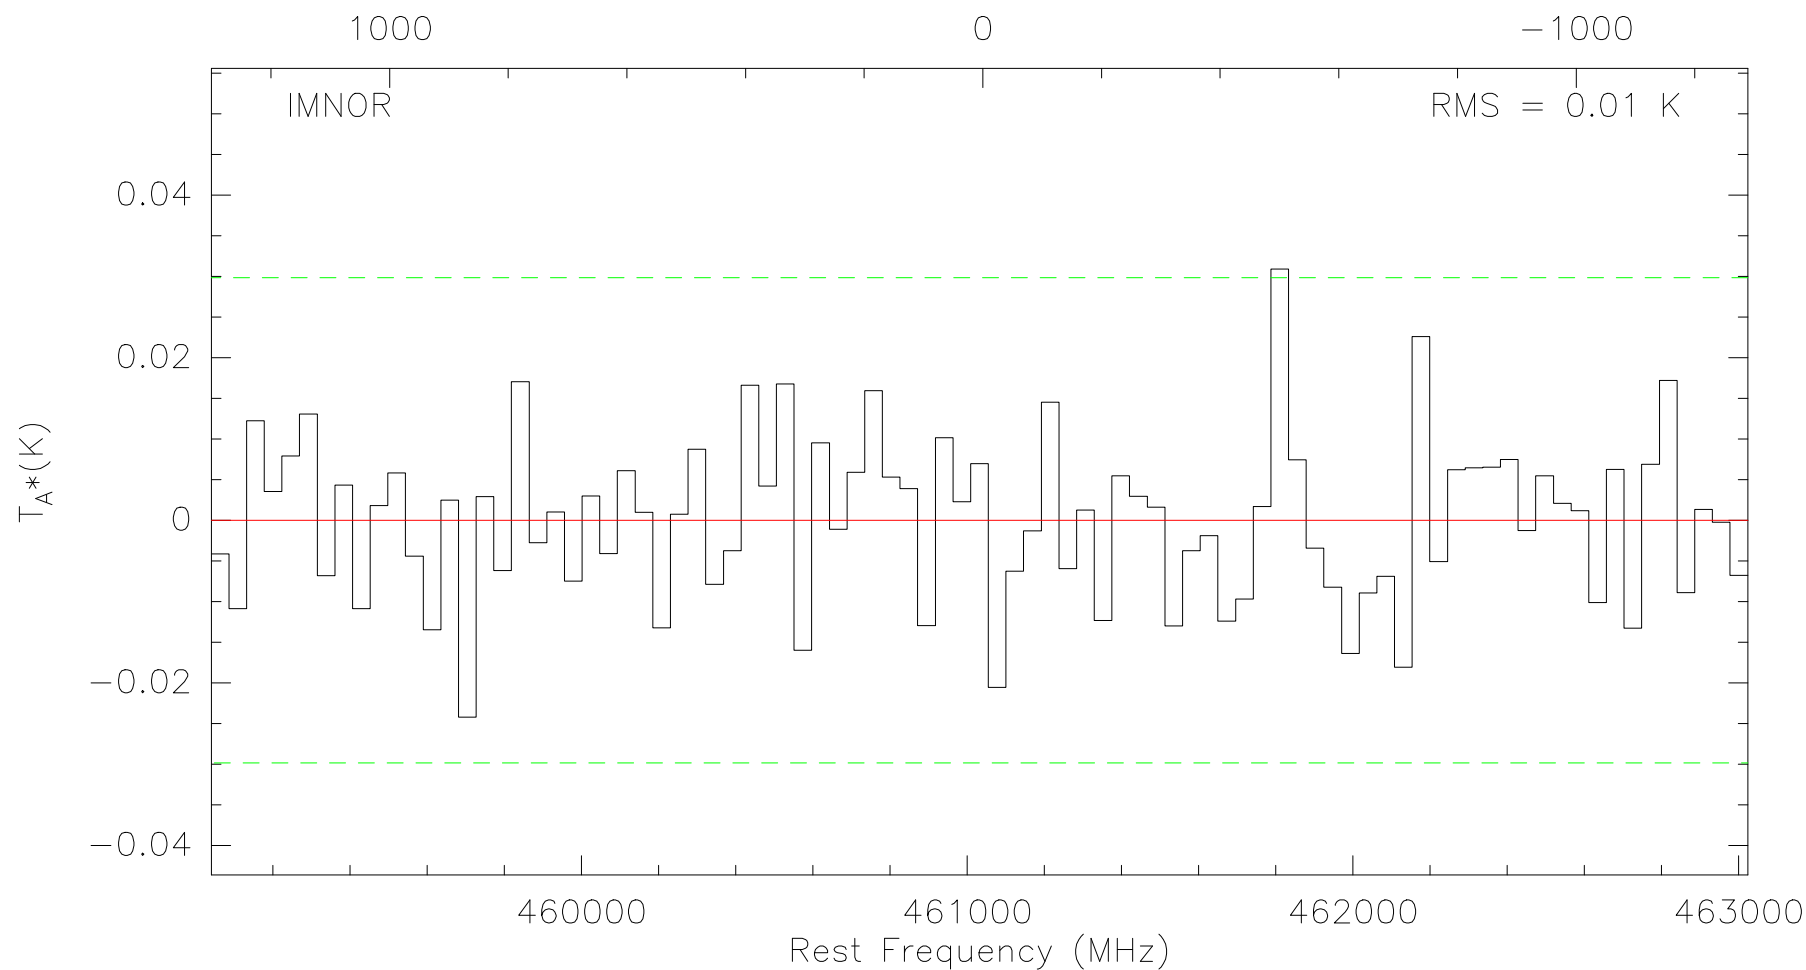

1;1 MTCEN CO(4-3) AP-FL01-XF0- O:01-JUL-2016 R:07-AUG-2020  
RA: 11:44:00.80 DEC: -60:33:39.5 Eq 2000.0 Rad. 0.0° Offs: +0.3 -0.5  
Unknown tau: 0.693 Tsys: 991. Time: 24.8min El: 46.2  
N: 87 IO: 44.1918 V0: 0.000 Dv: -29.77 LSR  
FO: 461040.768 Df: 45.78 Fi: 473041.772

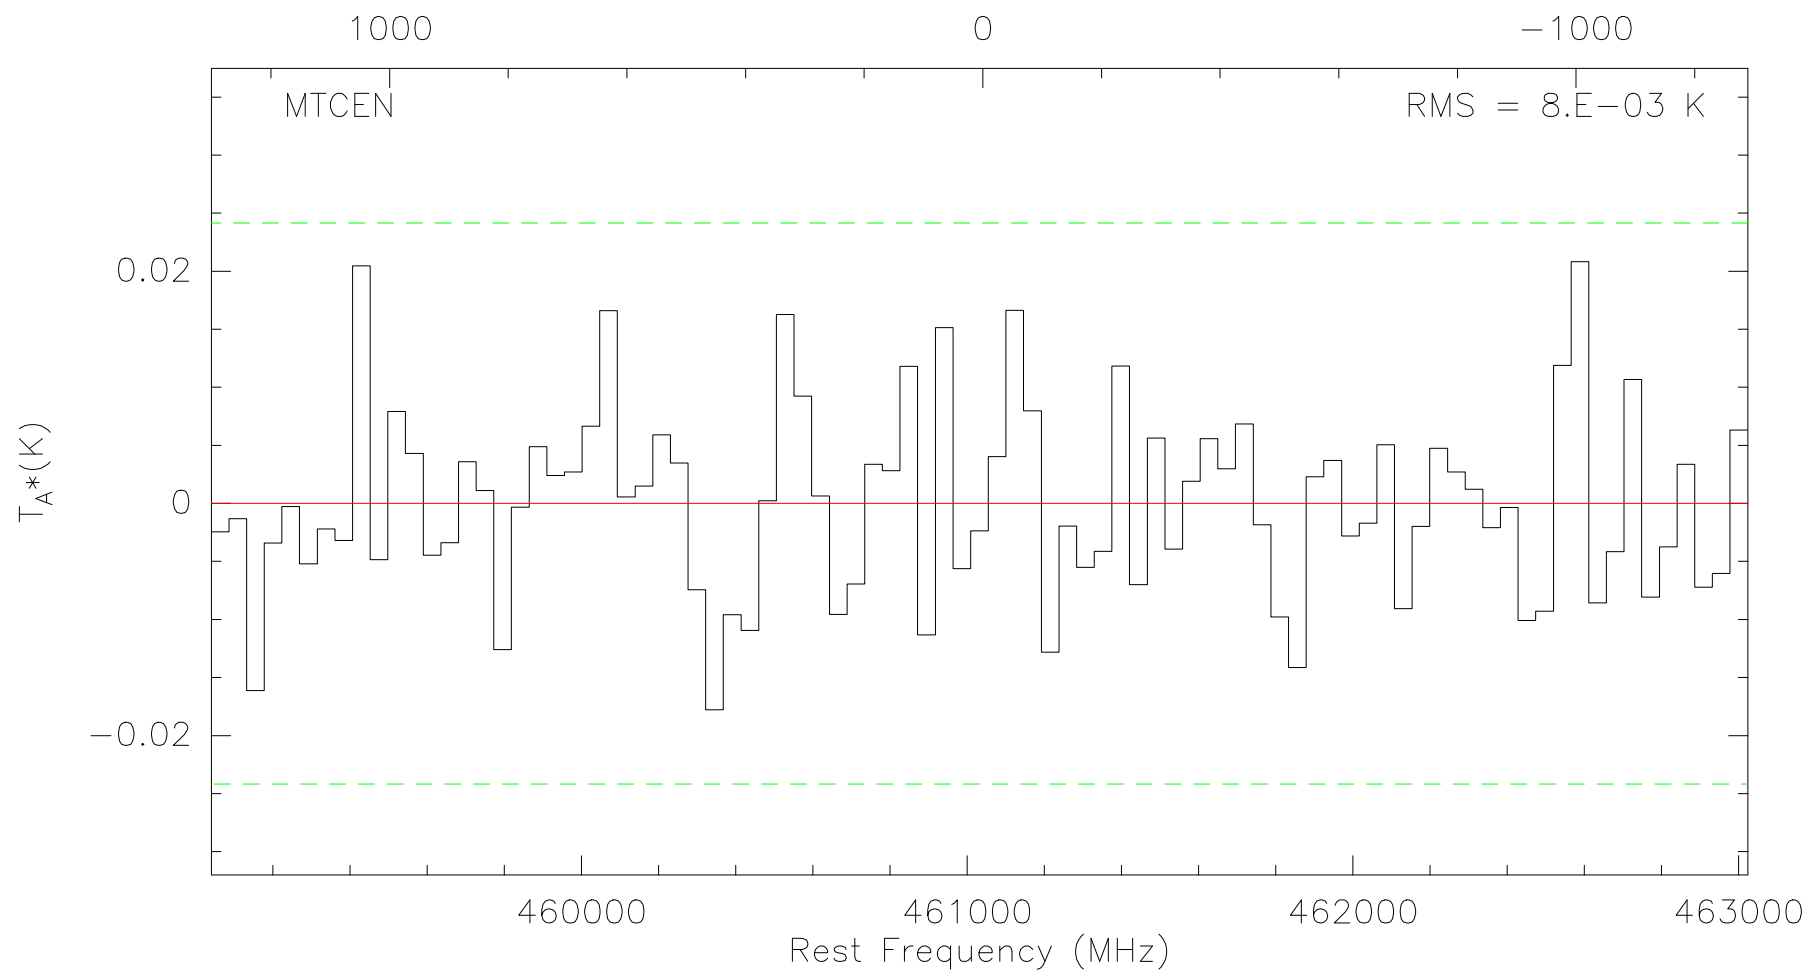

1;1 RSCAR CO(4-3) AP-FL01-XF0- O:30-JUN-2016 R:07-AUG-2020  
RA: 11:08:06.63 DEC: -61:56:04.6 Eq 2000.0 Rad. 0.0° Offs: +0.3 -0.6  
Unknown tau: 0.697 Tsys: 861. Time: 19.8min El: 47.6  
N: 87 IO: 44.1918 V0: 0.000 Dv: -29.77 LSR  
FO: 461040.768 Df: 45.78 Fi: 473041.778

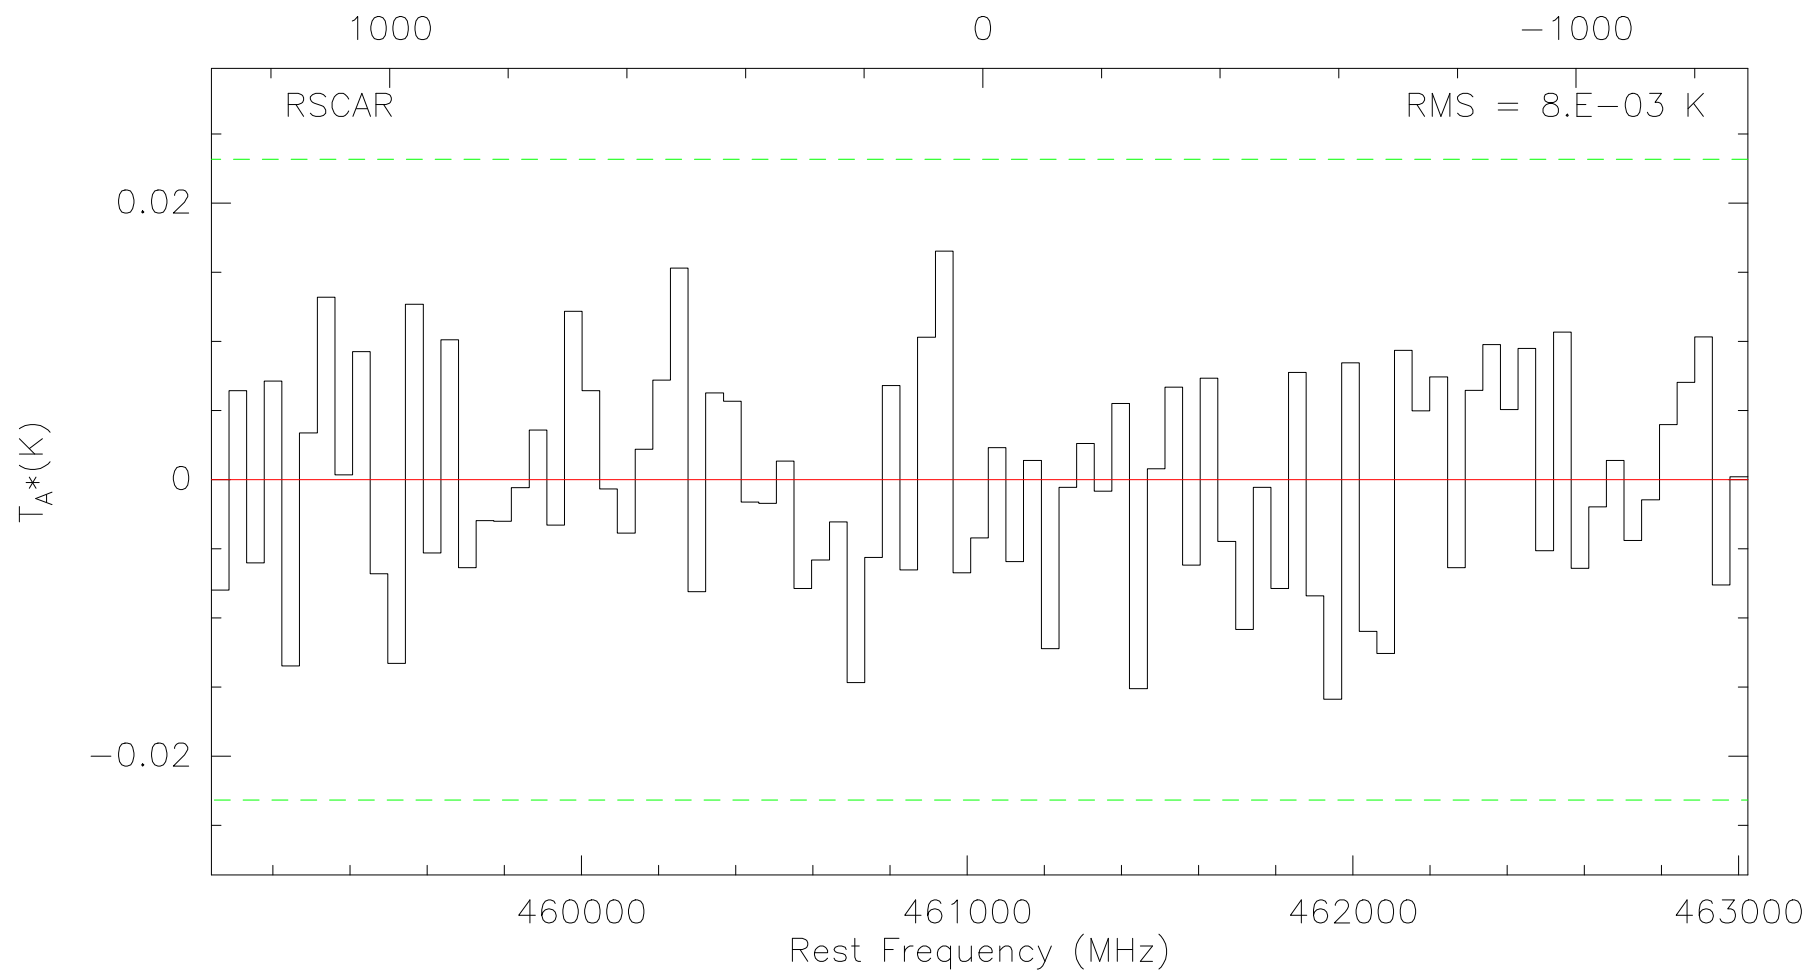

1;1 V1015SGR CO(4-3) AP-FL01-XF0- O:13-JUL-2016 R:07-AUG-2020

RA: 18:09:02.00 DEC: -32:28:32.0 Eq 2000.0 Rad. 0.0° Offs: +0.3 -0.3

Unknown tau: 0.717 Tsys: 966. Time: 19.8min El: 45.6

N: 87 l0: 44.1918 V0: 0.000 Dv: -29.77 LSR

F0: 461040.768 Df: 45.78 Fi: 473040.651

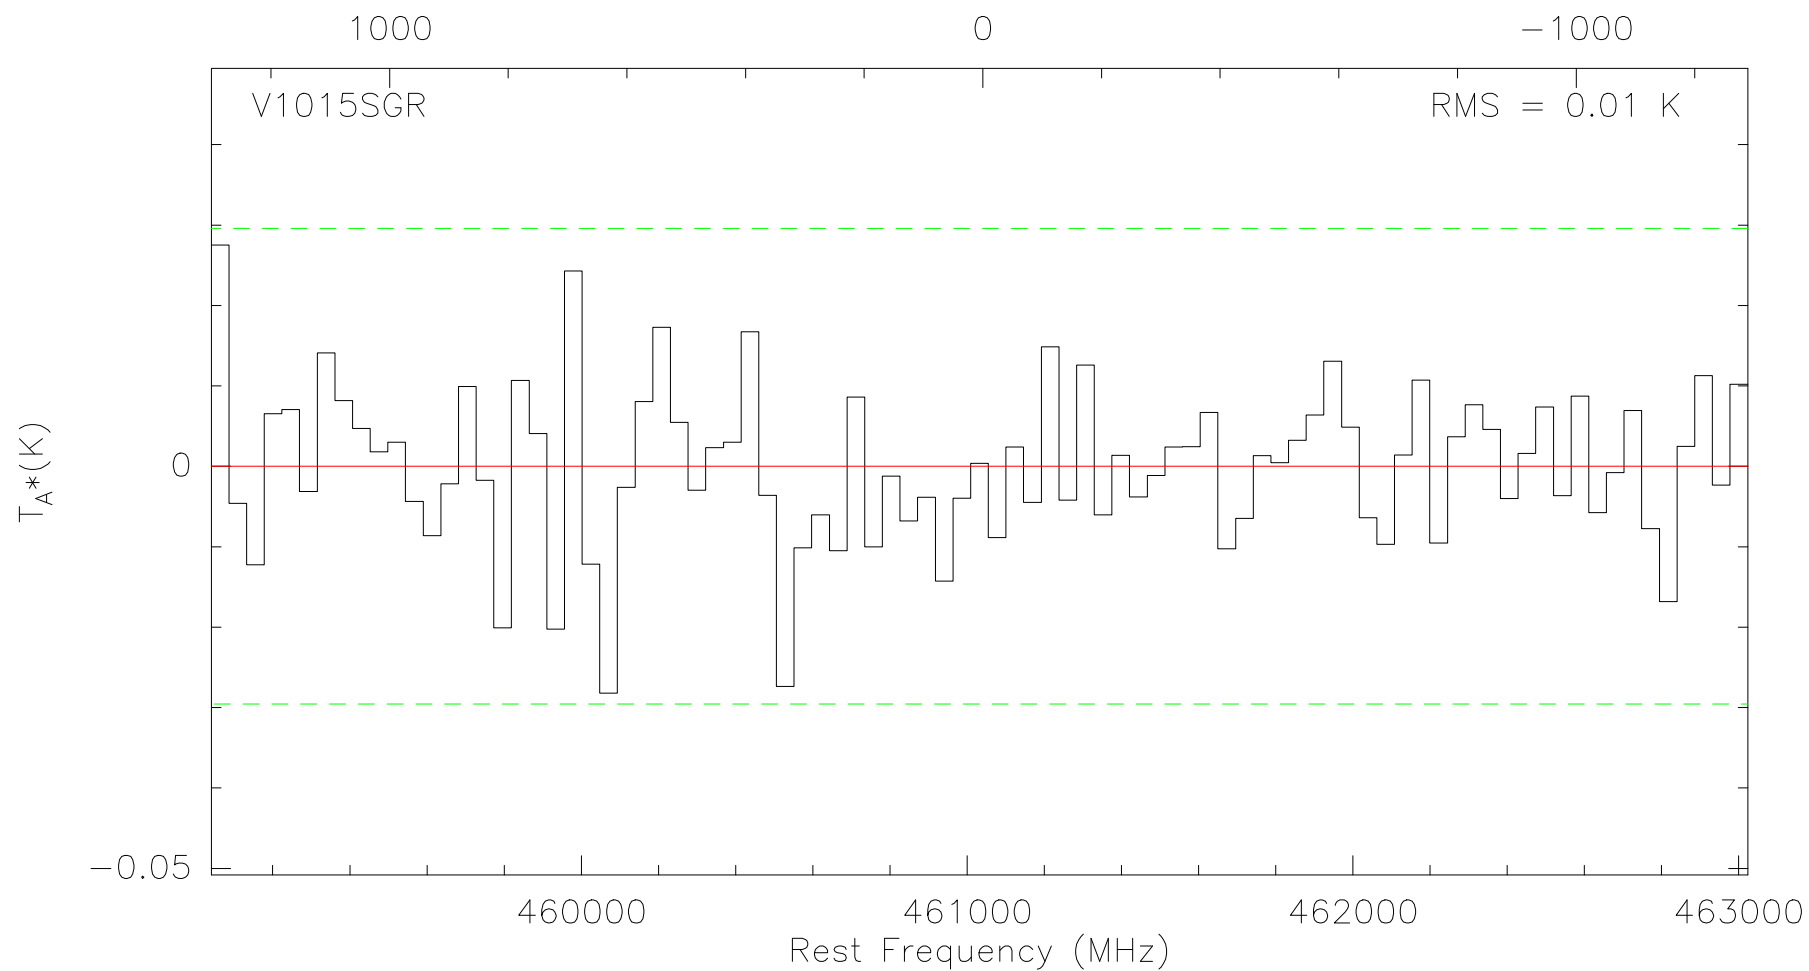

1;1 V1016SGR CO(4-3) AP-FL01-XF0- O:13-JUL-2016 R:07-AUG-2020  
RA: 18:19:57.63 DEC: -25:11:14.6 Eq 2000.0 Rad. 0.0° Offs: -0.2 -0.3  
Unknown tau: 0.459 Tsys: 695. Time: 9.9min El: 32.1  
N: 87 IO: 44.1918 V0: 0.000 Dv: -29.77 LSR  
FO: 461040.768 Df: 45.78 Fi: 473040.664

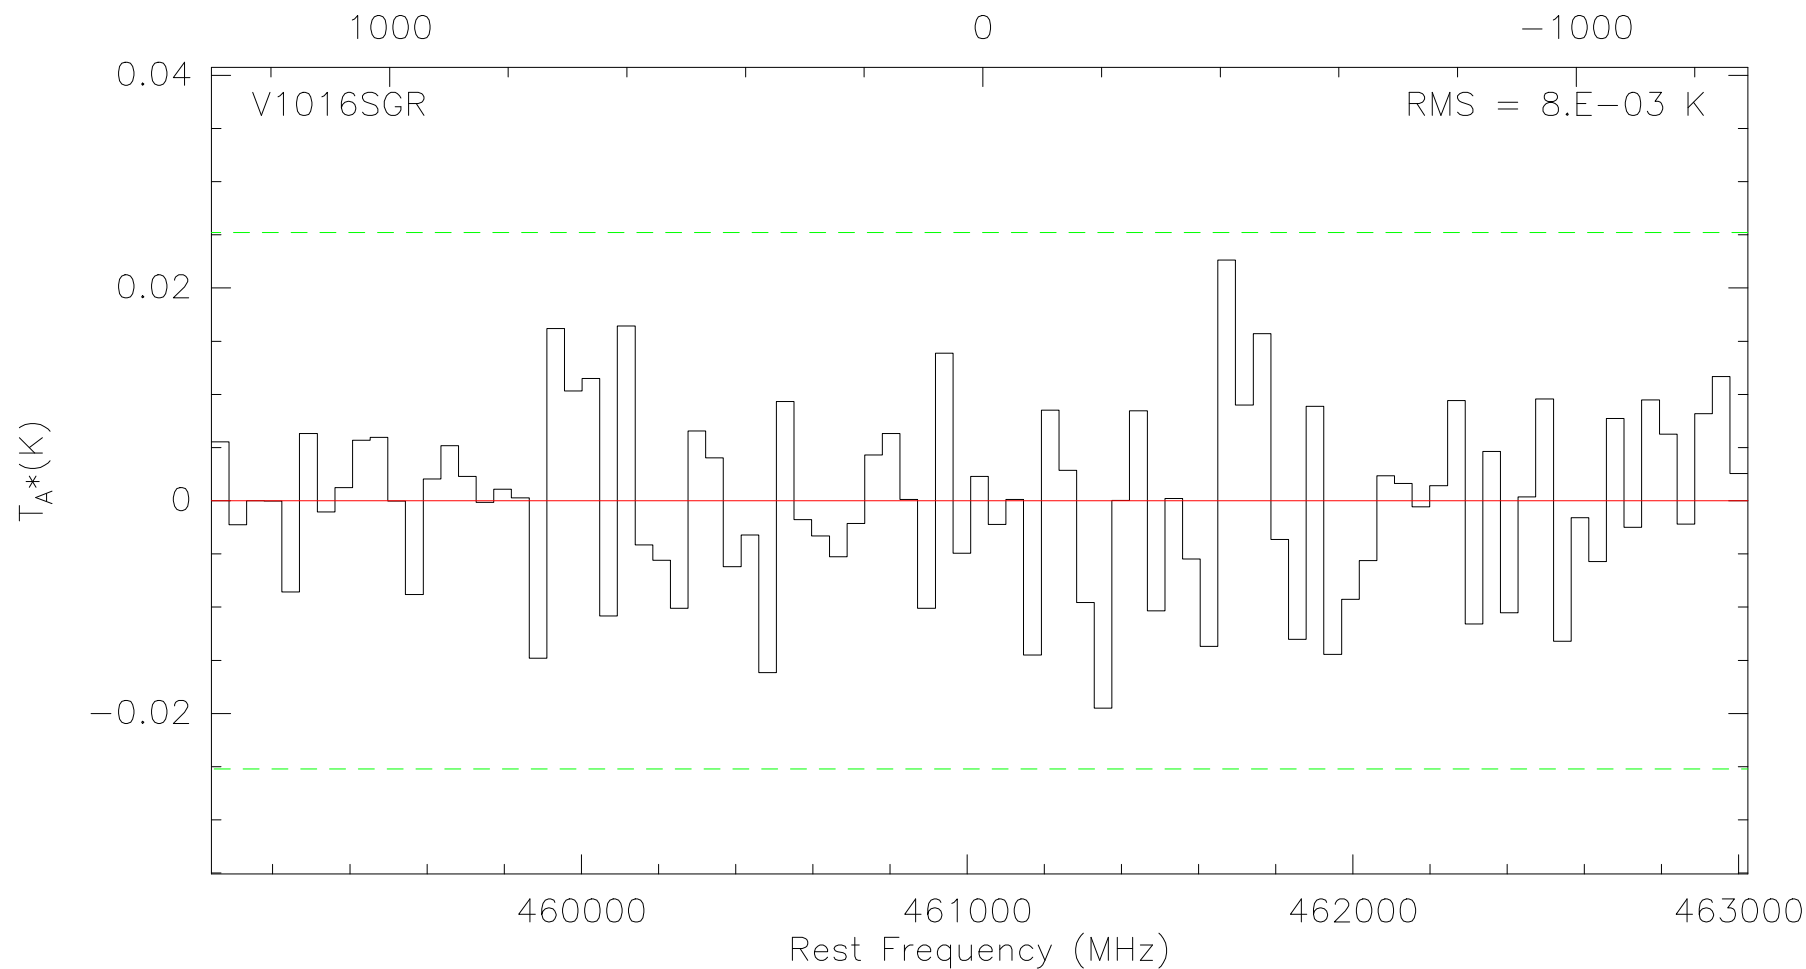

1;1 V1017SGR CO(4-3) AP-FL01-XF0- O:13-JUL-2016 R:07-AUG-2020  
RA: 18:32:04.47 DEC: -29:23:12.5 Eq 2000.0 Rad. 0.0° Offs: +0.4 -0.4  
Unknown tau: 0.710 Tsys: 580. Time: 14.9min El: 75.2  
N: 87 IO: 44.1918 V0: 0.000 Dv: -29.77 LSR  
F0: 461040.768 Df: 45.78 Fi: 473040.643

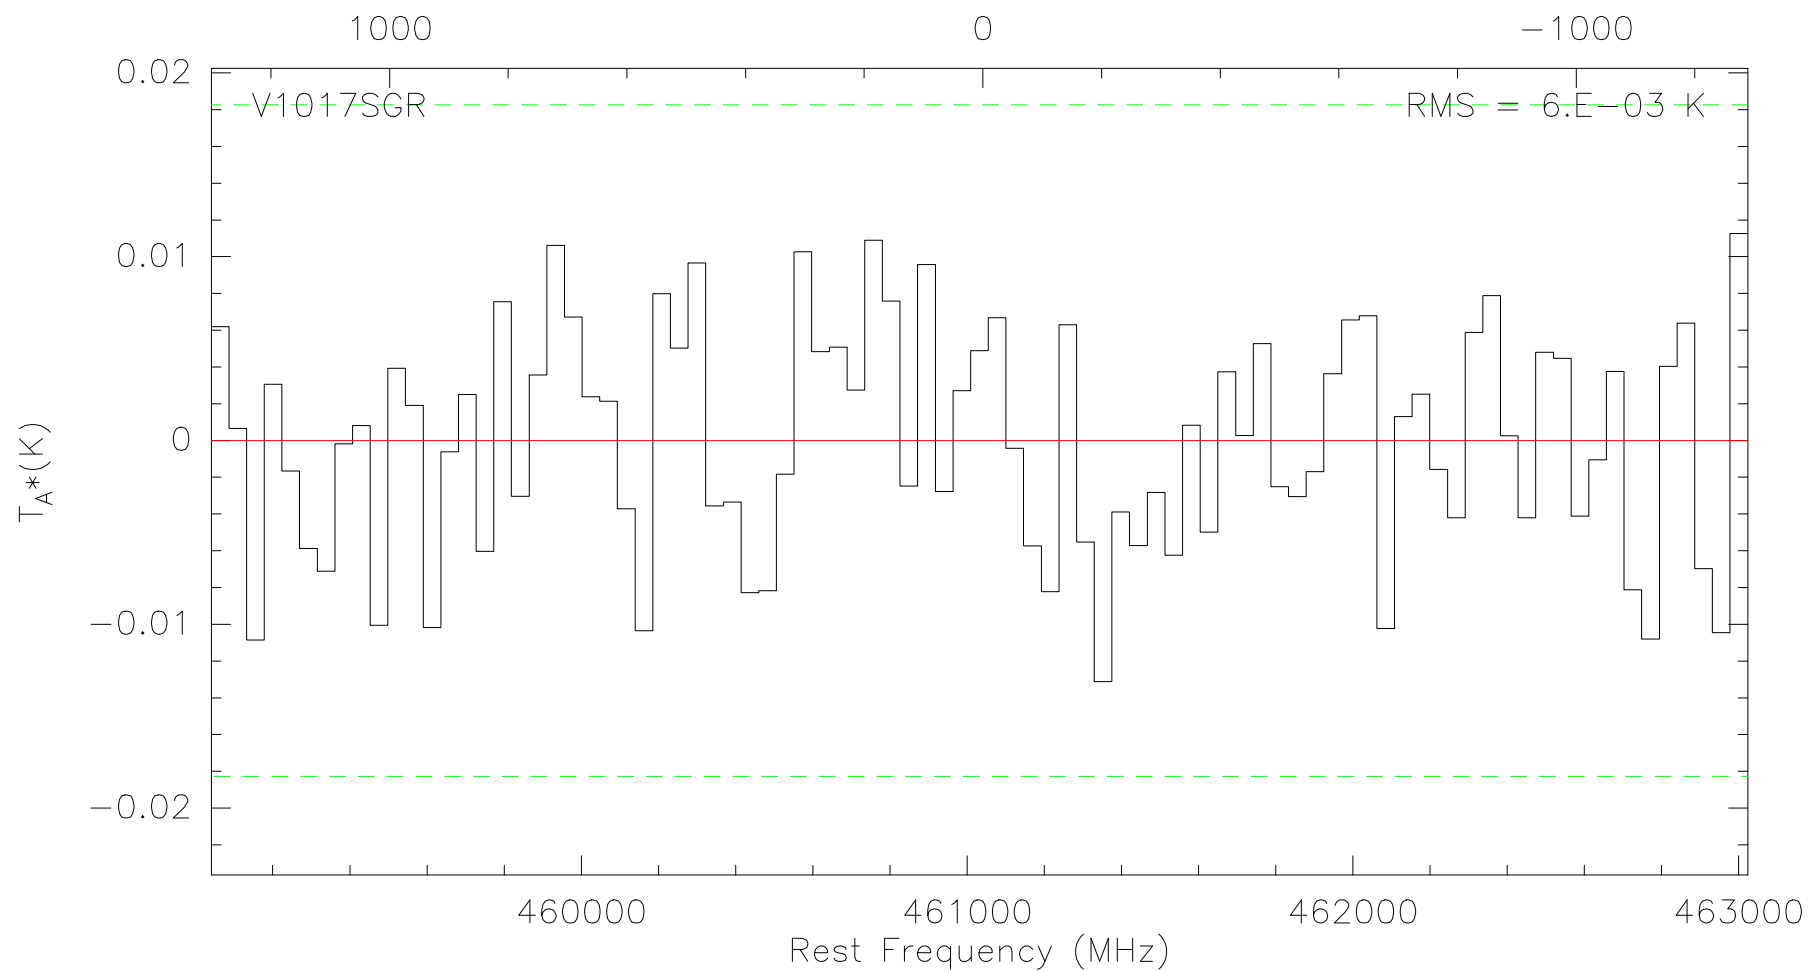

1;1 V1149SGR CO(4-3) AP-FL01-XF0- O:13-JUL-2016 R:07-AUG-2020  
RA: 18:18:30.40 DEC: -28:17:17.0 Eq 2000.0 Rad. 0.0° Offs: -0.2 -0.6  
Unknown tau: 0.494 Tsys: 466. Time: 9.9min El: 61.7  
N: 87 IO: 44.1918 V0: 0.000 Dv: -29.77 LSR  
FO: 461040.768 Df: 45.78 Fi: 473040.699

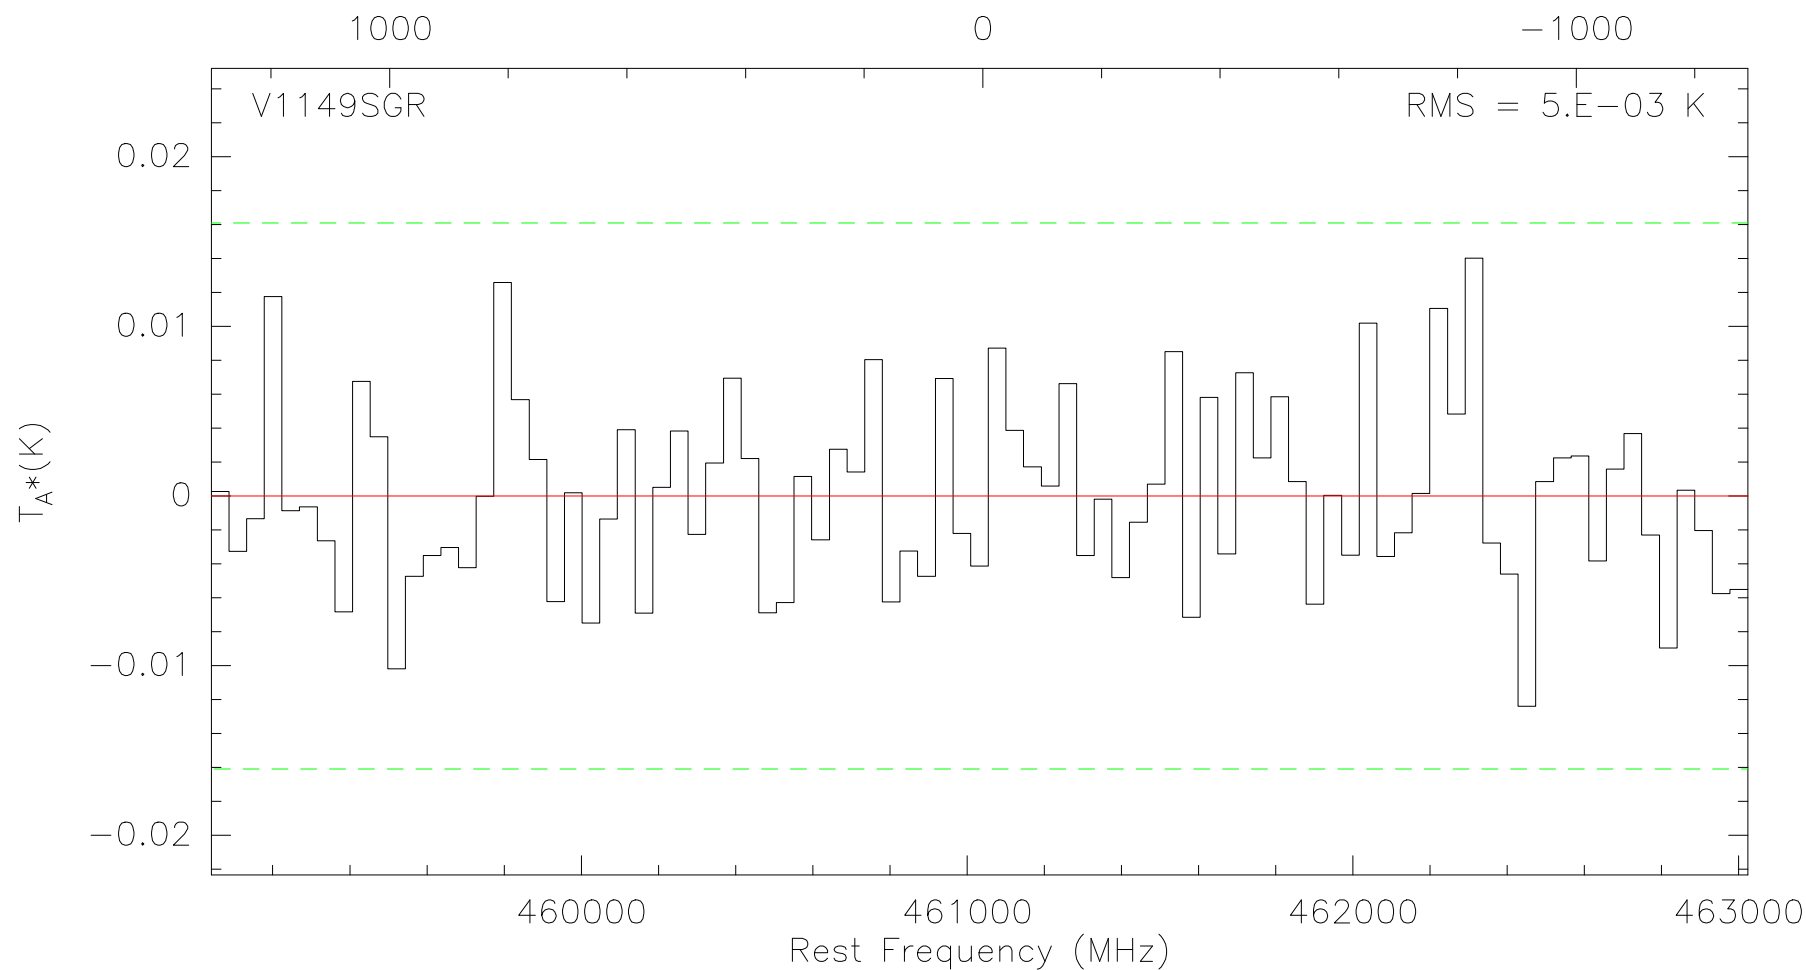

1;1 V1151SGR CO(4-3) AP-FL01-XF0- O:14-JUL-2016 R:07-AUG-2020  
RA: 18:25:23.75 DEC: -20:11:59.3 Eq 2000.0 Rad. 0.0° Offs: -0.2 -0.3  
Unknown tau: 0.524 Tsys: 984. Time: 9.9min El: 26.8  
N: 87 IO: 44.1918 V0: 0.000 Dv: -29.77 LSR  
F0: 461040.768 Df: 45.78 Fi: 473040.602

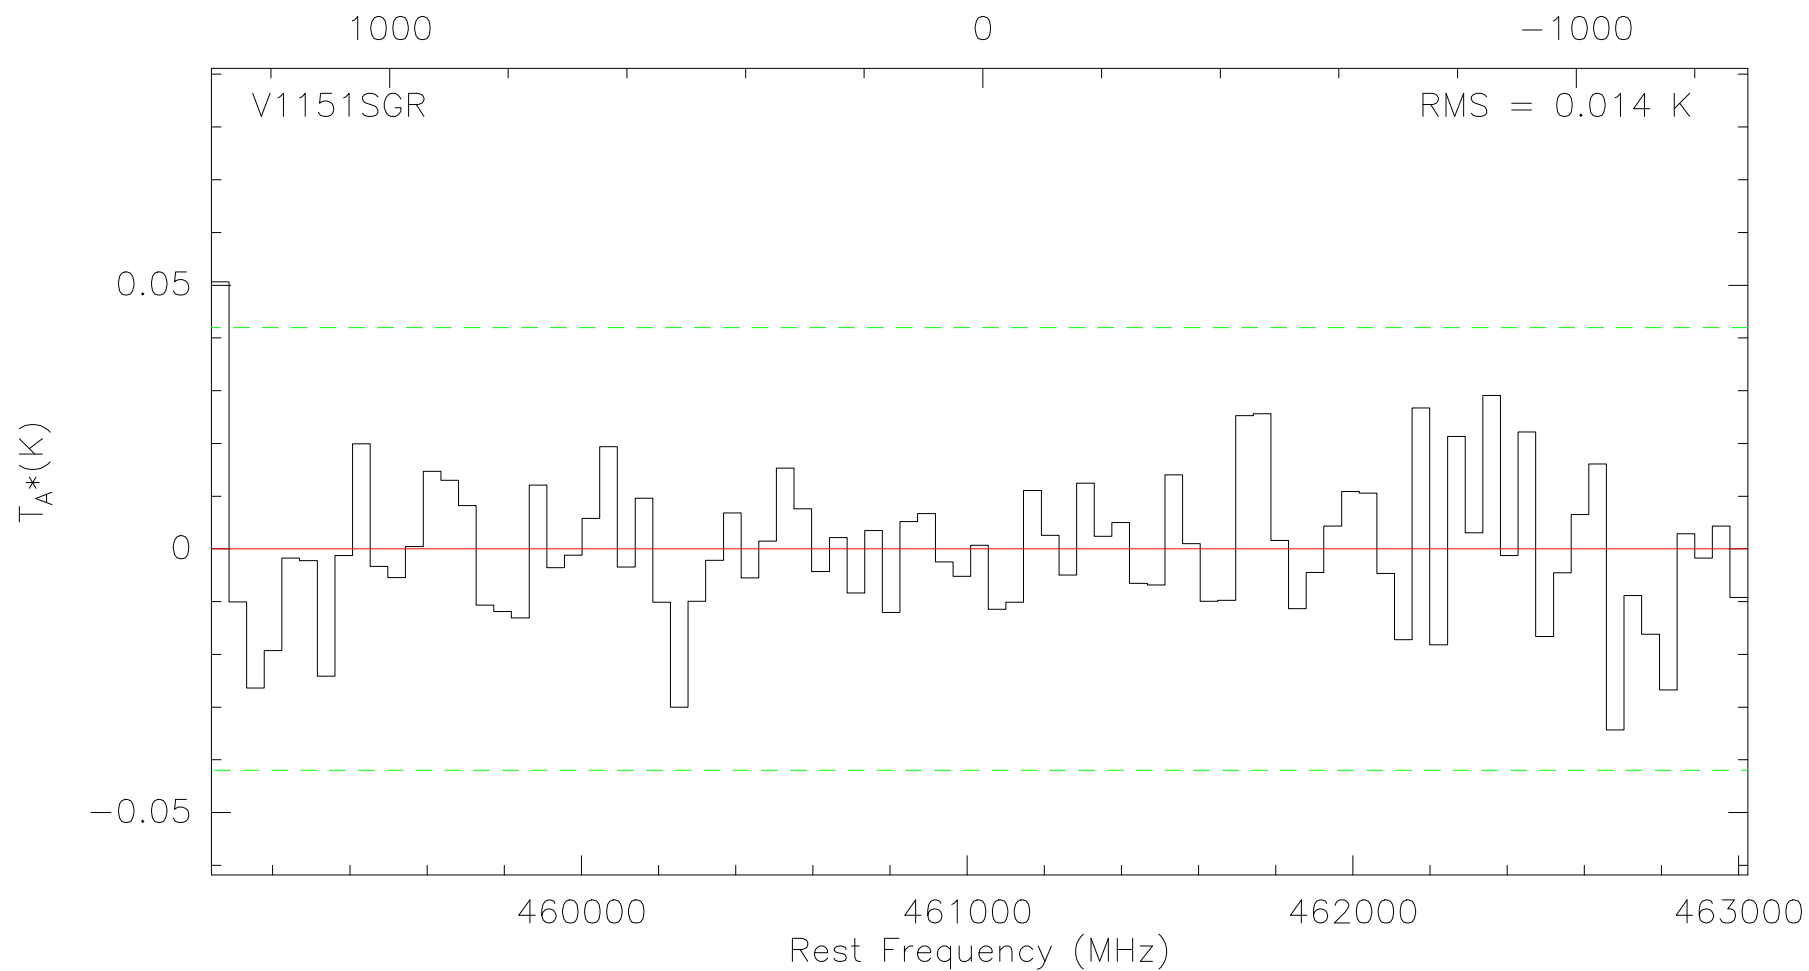

1;1 V1583SGR CO(4-3) AP-FL01-XF0- O:14-JUL-2016 R:07-AUG-2020  
RA: 18:15:26.30 DEC: -23:23:18.0 Eq 2000.0 Rad. 0.0° Offs: -0.2 -0.3  
Unknown tau: 0.545 Tsys: 897. Time: 9.9min El: 30.0  
N: 87 IO: 44.1918 V0: 0.000 Dv: -29.77 LSR  
FO: 461040.768 Df: 45.78 Fi: 473040.682

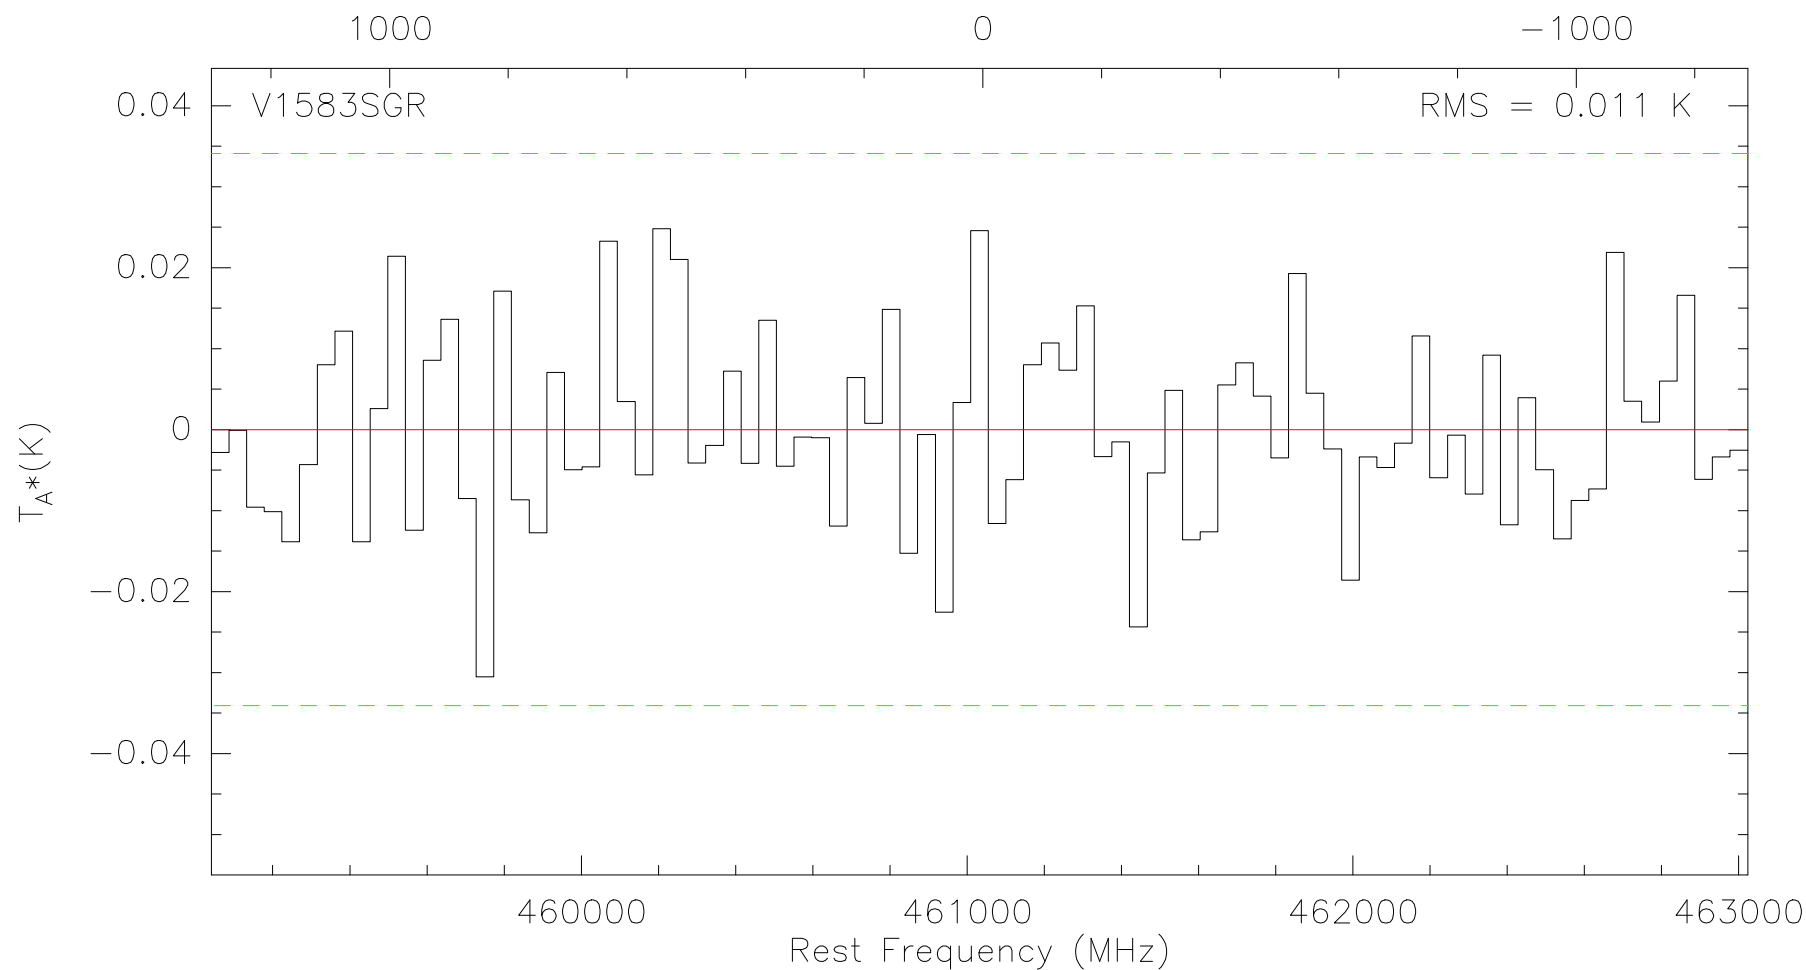

1;1 V363SGR CO(4-3) AP-FL01-XF0- O:01-JUL-2016 R:07-AUG-2020  
RA: 19:11:16.30 DEC: -29:50:00.0 Eq 2000.0 Rad. 0.0° Offs: -0.2 -0.6  
Unknown tau: 1.284 Tsys: 2222. Time: 19.9min El: 42.0  
N: 87 IO: 44.1918 V0: 0.000 Dv: -29.76 LSR  
FO: 461040.768 Df: 45.77 Fi: 473040.283

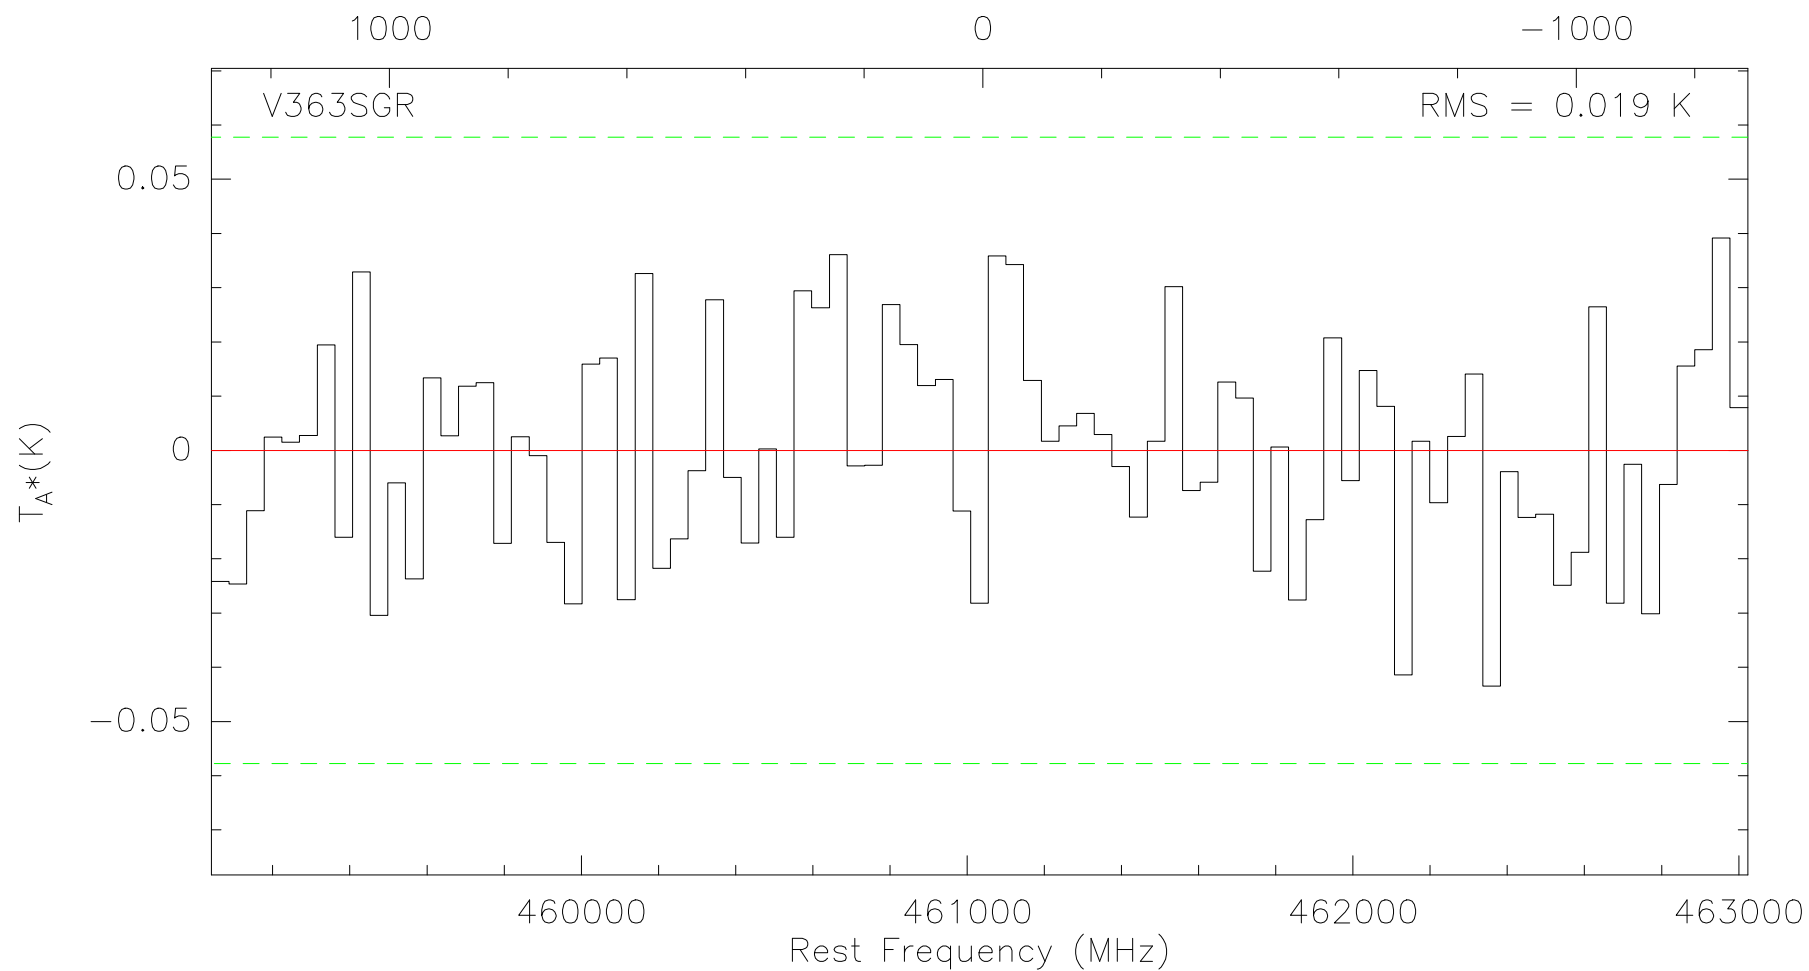

1;1 V365CAR CO(4-3) AP-FL01-XF0- O:30-JUN-2016 R:07-AUG-2020  
RA: 11:03:16.77 DEC: -58:27:24.9 Eq 2000.0 Rad. 0.0° Offs: +0.3 -0.5  
Unknown tau: 0.679 Tsys: 801. Time: 19.8min El: 51.3  
N: 87 IO: 44.1918 V0: 0.000 Dv: -29.77 LSR  
FO: 461040.768 Df: 45.78 Fi: 473041.832

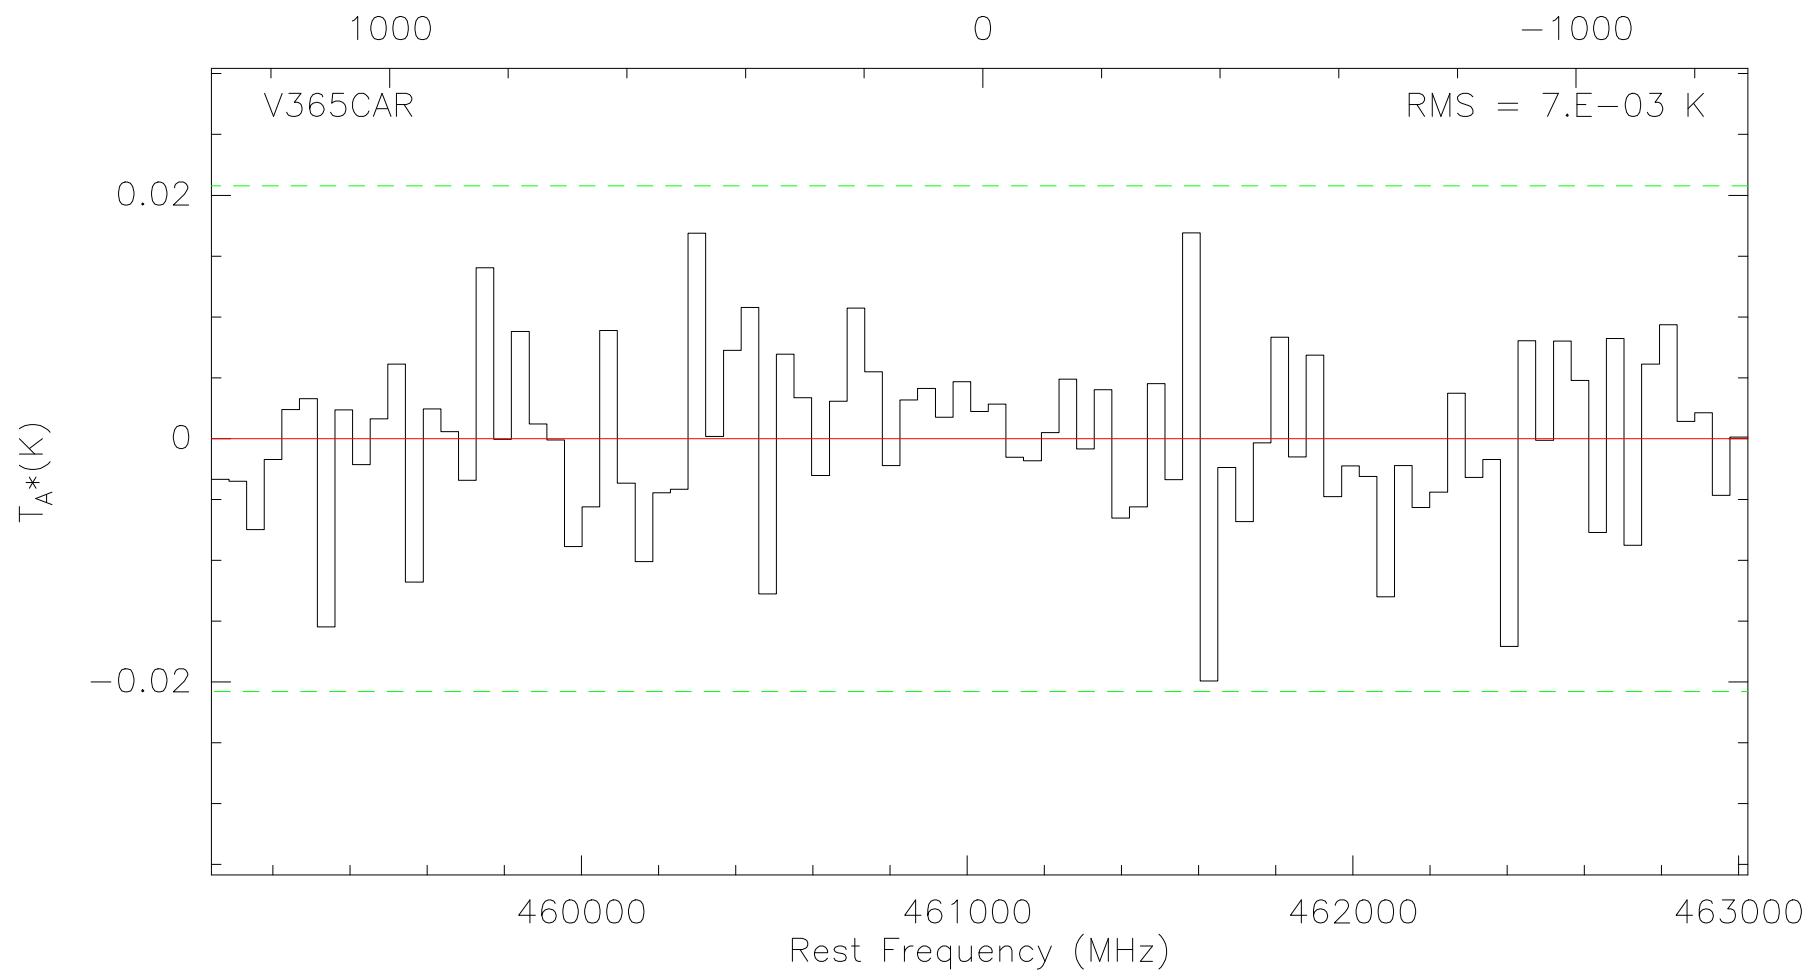

1;1 V382SCO CO(4-3) AP-FL01-XF0- O:13-JUL-2016 R:07-AUG-2020  
RA: 17:51:56.13 DEC: -35:25:05.4 Eq 2000.0 Rad. 0.0° Offs: +0.1 -0.6  
Unknown tau: 0.508 Tsys: 445. Time: 9.9min El: 72.8  
N: 87 l0: 44.1918 V0: 0.000 Dv: -29.77 LSR  
F0: 461040.768 Df: 45.78 Fi: 473040.883

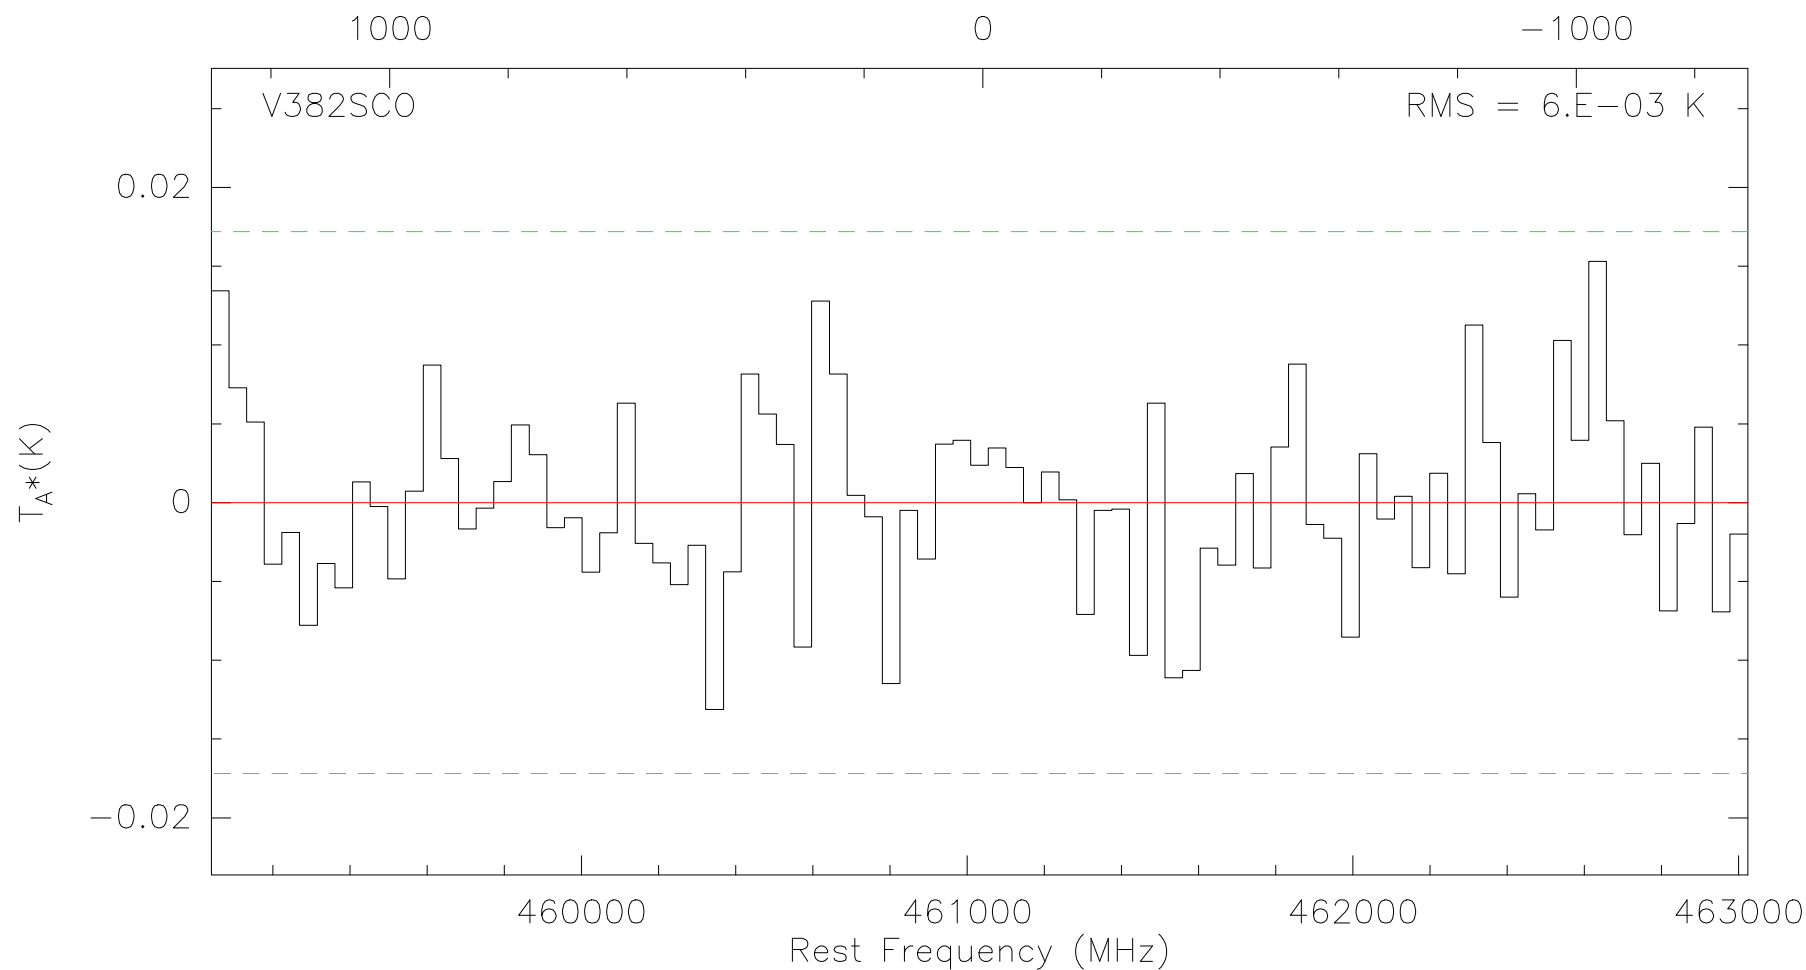

1;1 V384SCO CO(4-3) AP-FL01-XF0- O:14-JUL-2016 R:07-AUG-2020  
RA: 18:01:43.15 DEC: -35:39:27.8 Eq 2000.0 Rad. 0.0° Offs: +0.3 -0.3  
Unknown tau: 0.849 Tsys: 985. Time: 9.9min El: 52.1  
N: 87 IO: 44.1918 V0: 0.000 Dv: -29.77 LSR  
F0: 461040.768 Df: 45.78 Fi: 473040.850

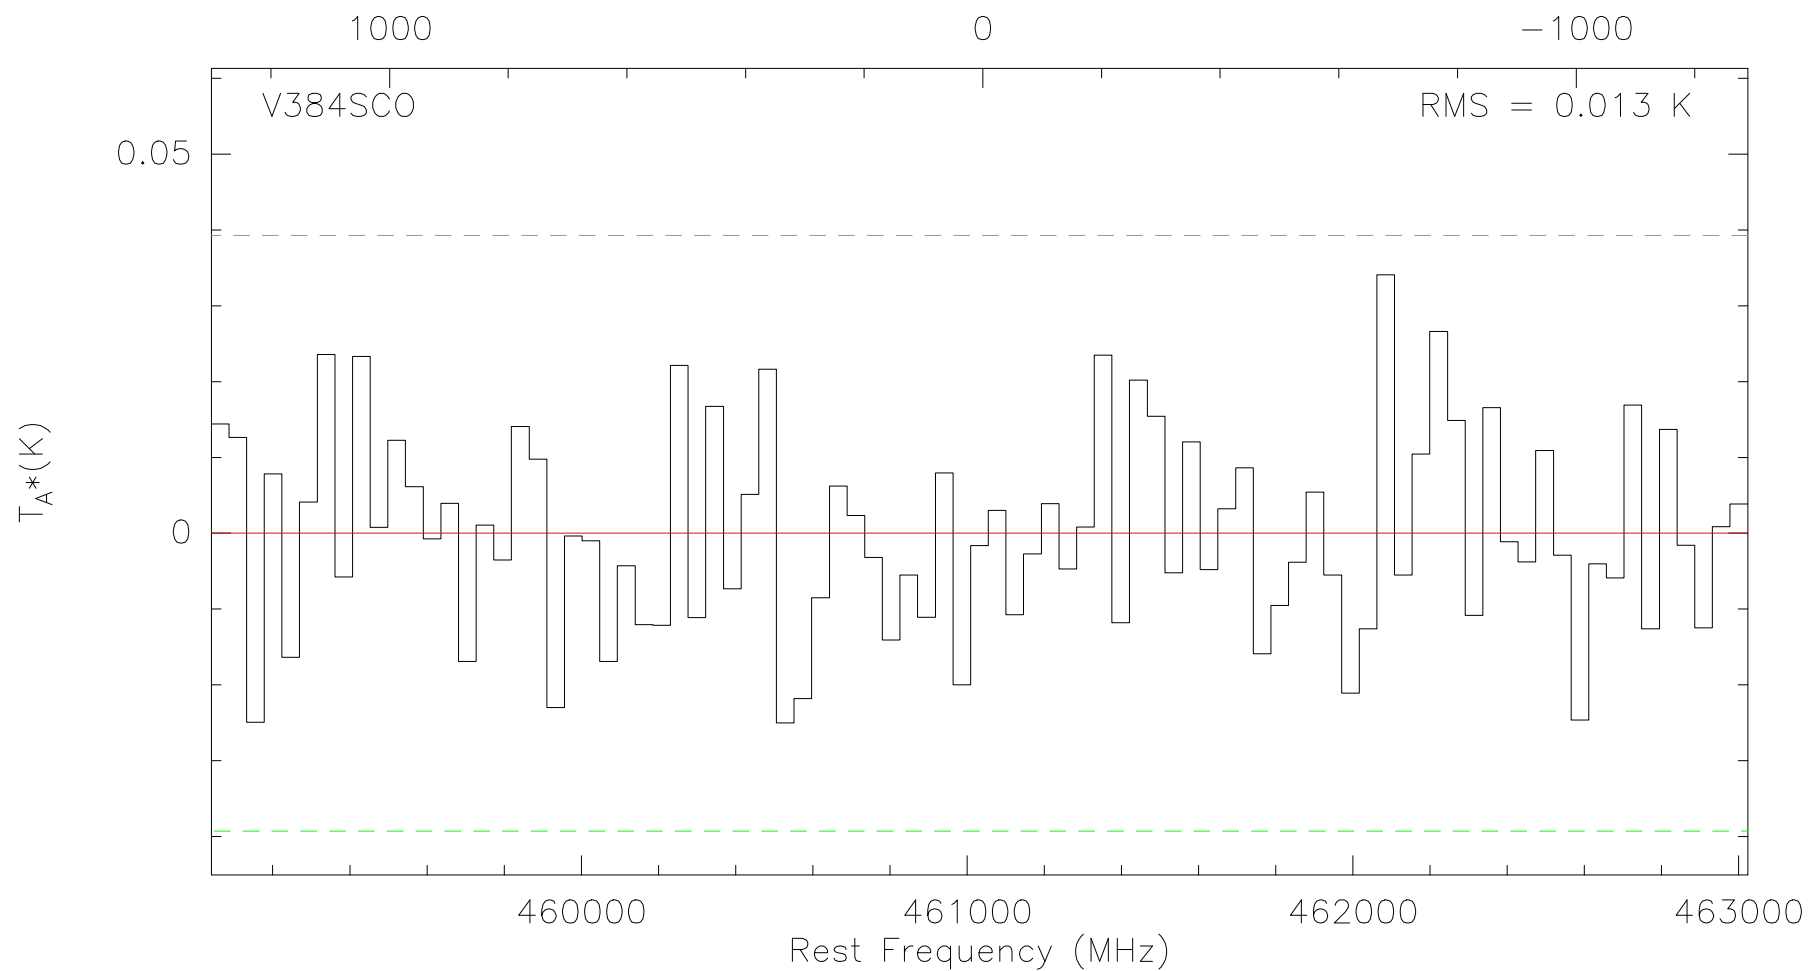

1;1 V522SGR CO(4-3) AP-FL01-XF0- O:01-JUL-2016 R:07-AUG-2020  
RA: 18:48:00.47 DEC: -25:22:21.9 Eq 2000.0 Rad. 0.0° Offs: -0.2 -0.5  
Unknown tau: 1.247 Tsys: 3066. Time: 19.8min El: 31.8  
N: 87 IO: 44.1918 V0: 0.000 Dv: -29.77 LSR  
F0: 461040.768 Df: 45.77 Fi: 473040.313

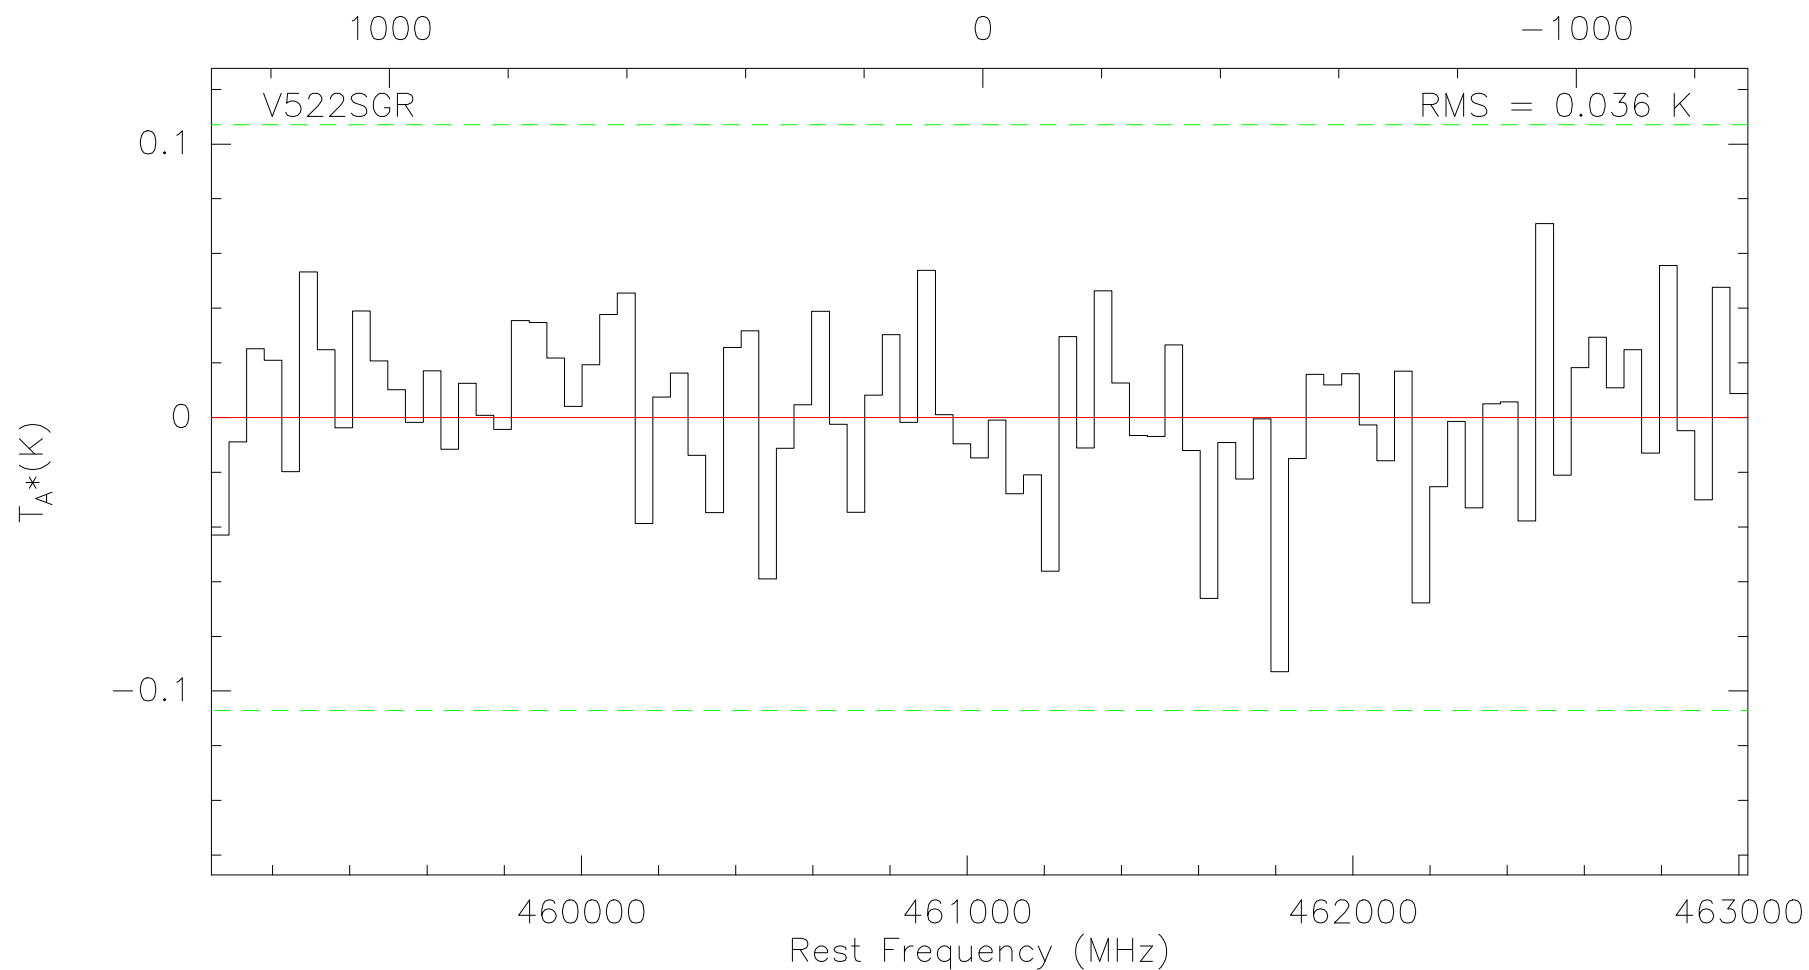

1;1 V5530PH CO(4-3) AP-FL01-XF0- 0:01-JUL-2016 R:07-AUG-2020  
RA: 17:42:53.50 DEC: -24:51:26.2 Eq 2000.0 Rad. 0.0° Offs: -0.4 -0.5  
Unknown tau: 1.291 Tsys: 2625. Time: 9.9min El: 38.8  
N: 87 IO: 44.1918 V0: 0.000 Dv: -29.77 LSR  
FO: 461040.768 Df: 45.78 Fi: 473040.596

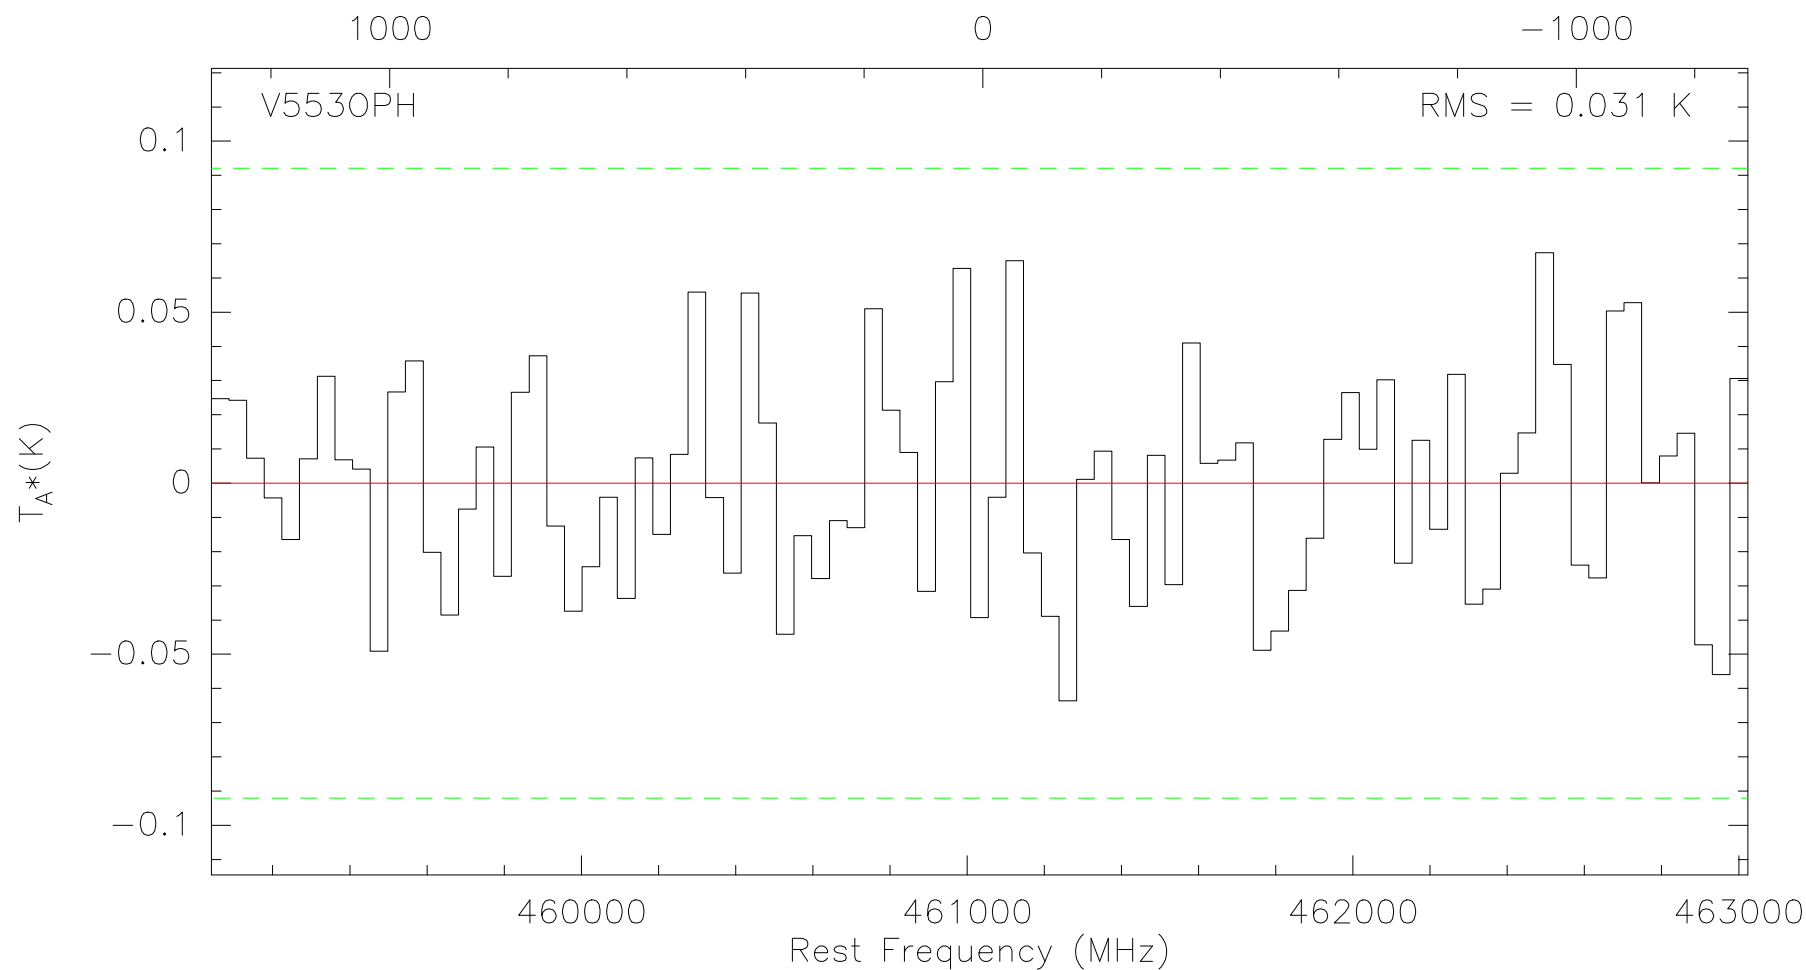

1;1 V696SCO CO(4-3) AP-FL01-XF0- O:13-JUL-2016 R:07-AUG-2020  
RA: 17:53:11.55 DEC: -35:50:14.4 Eq 2000.0 Rad. 0.0° Offs: +0.2 -0.6  
Unknown tau: 0.625 Tsys: 513. Time: 9.9min El: 77.1  
N: 87 IO: 44.1918 V0: 0.000 Dv: -29.77 LSR  
F0: 461040.768 Df: 45.78 Fi: 473040.879

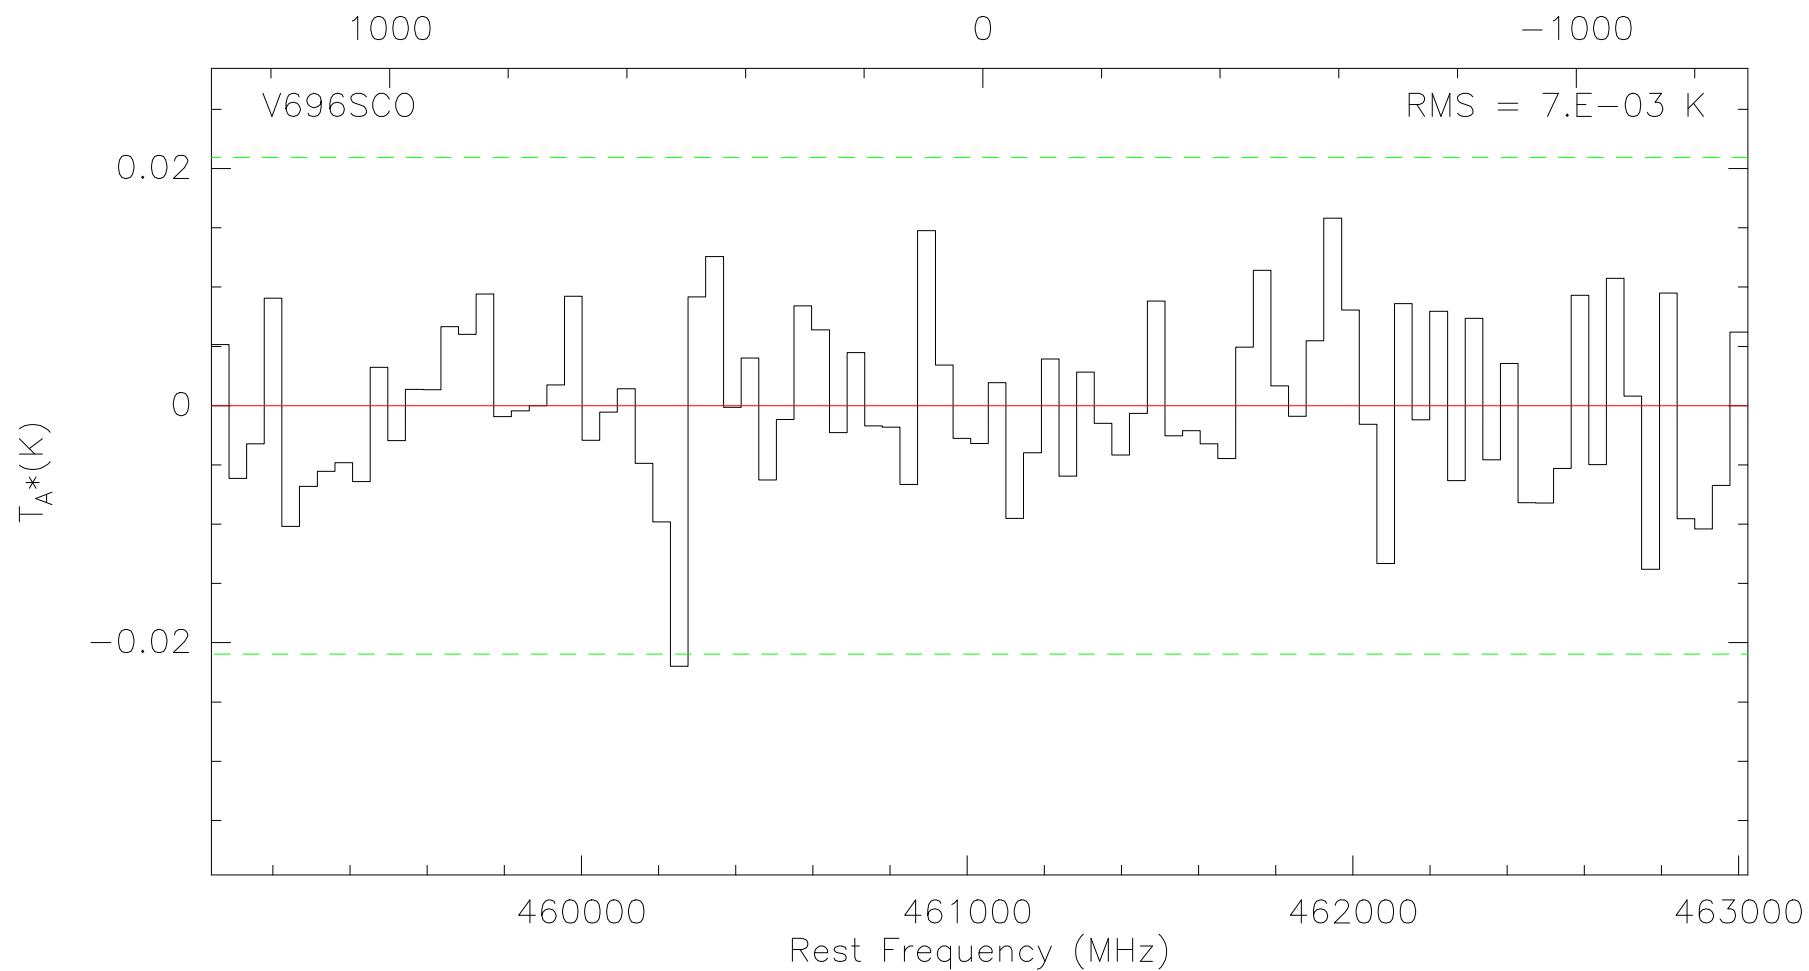

1;1 V697SCO CO(4-3) AP-FL01-XF0- O:13-JUL-2016 R:07-AUG-2020  
RA: 17:51:21.83 DEC: -37:24:55.2 Eq 2000.0 Rad. 0.0° Offs: -0.2 -0.5  
Unknown tau: 0.493 Tsys: 584. Time: 14.9min El: 43.3  
N: 87 IO: 44.1918 V0: 0.000 Dv: -29.77 LSR  
FO: 461040.768 Df: 45.78 Fi: 473040.916

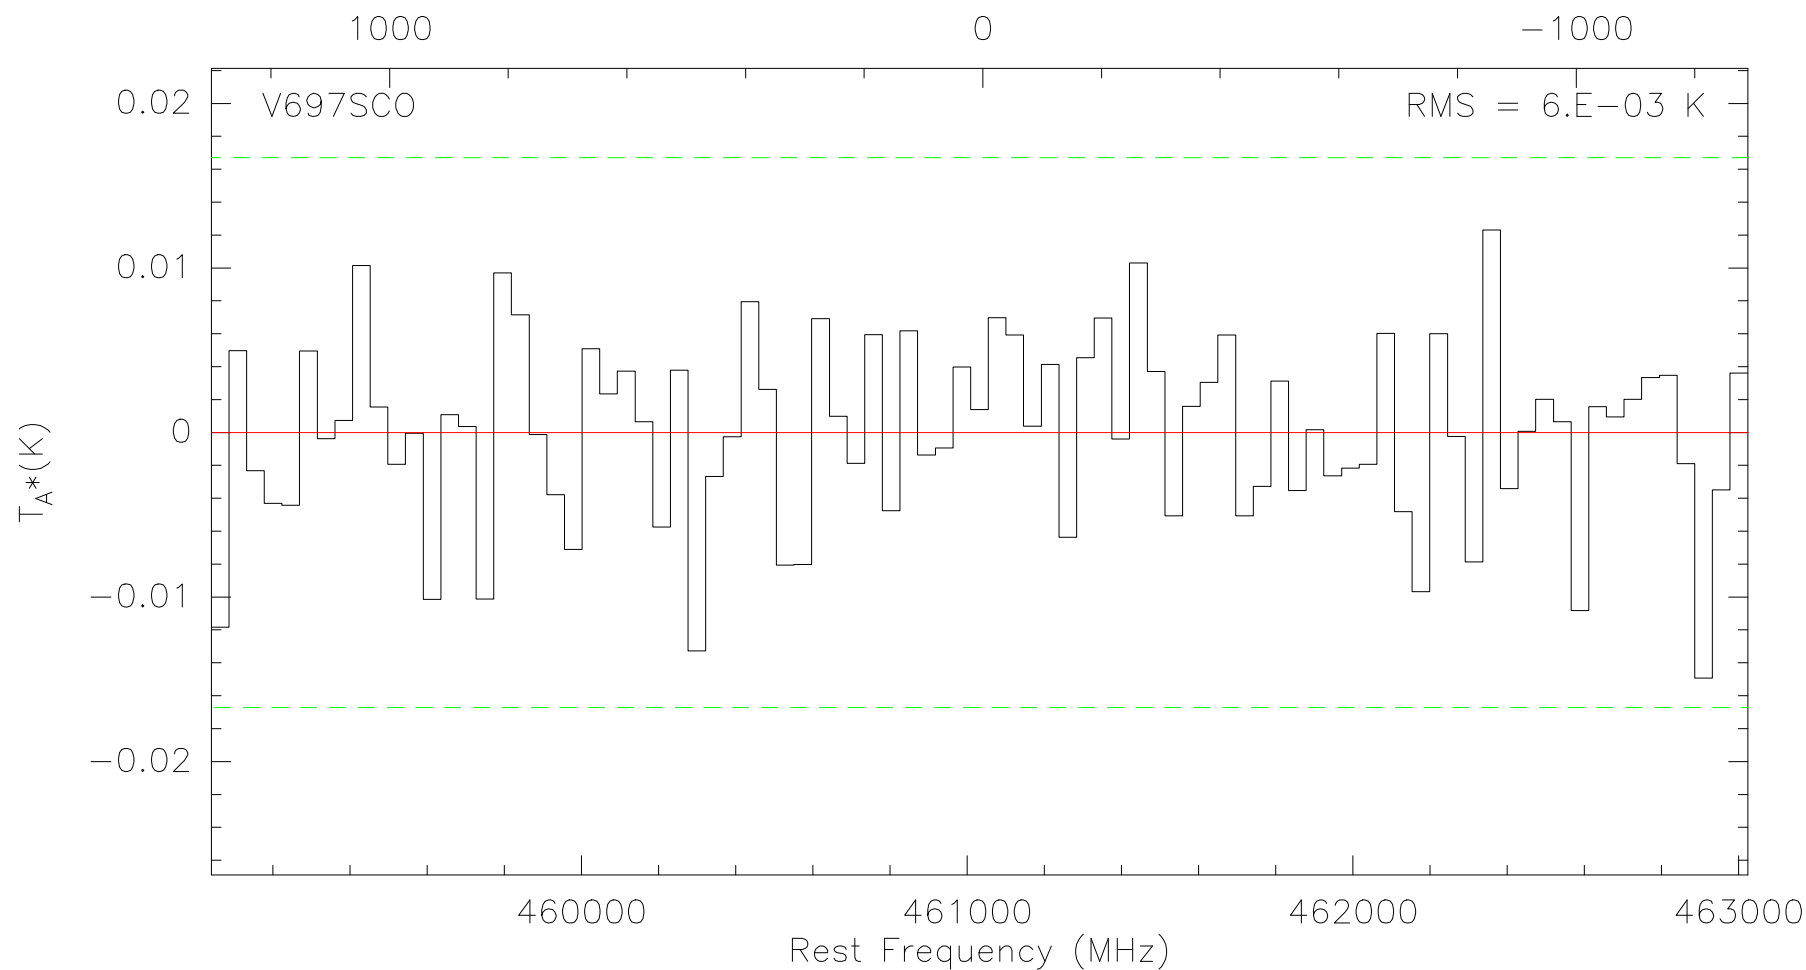

1;1 V707SCO CO(4-3) AP-FL01-XF0- 0:06-JUL-2016 R:07-AUG-2020

RA: 17:48:26.38 DEC: -36:37:54.9 Eq 2000.0 Rad. 0.0° Offs: +0.3 -0.3

Unknown tau: 0.734 Tsys: 1073. Time: 9.9min El: 40.0

N: 87 l0: 44.1918 V0: 0.000 Dv: -29.77 LSR

F0: 461040.768 Df: 45.78 Fi: 473040.784

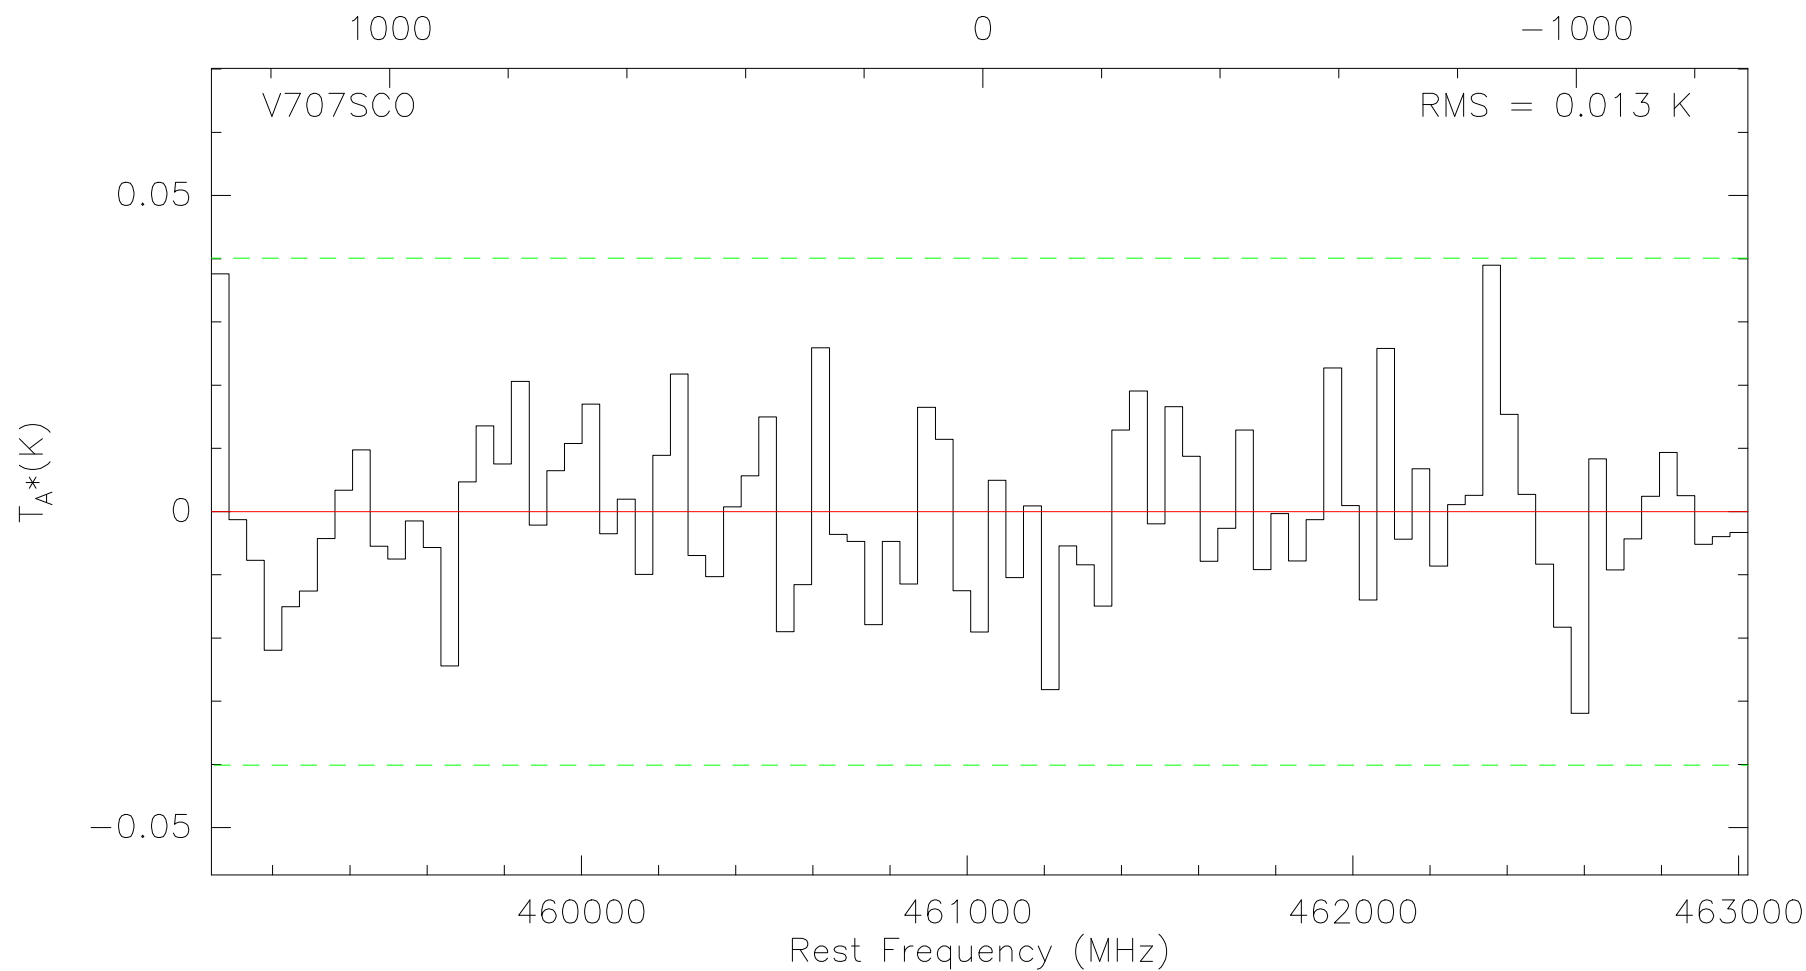

1;1 V711SCO CO(4-3) AP-FL01-XF0- O:14-JUL-2016 R:07-AUG-2020  
RA: 17:54:06.16 DEC: -34:21:15.5 Eq 2000.0 Rad. 0.0° Offs: +0.3 -0.3  
Unknown tau: 0.797 Tsys: 812. Time: 9.9min El: 58.0  
N: 87 IO: 44.1918 V0: 0.000 Dv: -29.77 LSR  
FO: 461040.768 Df: 45.78 Fi: 473040.867

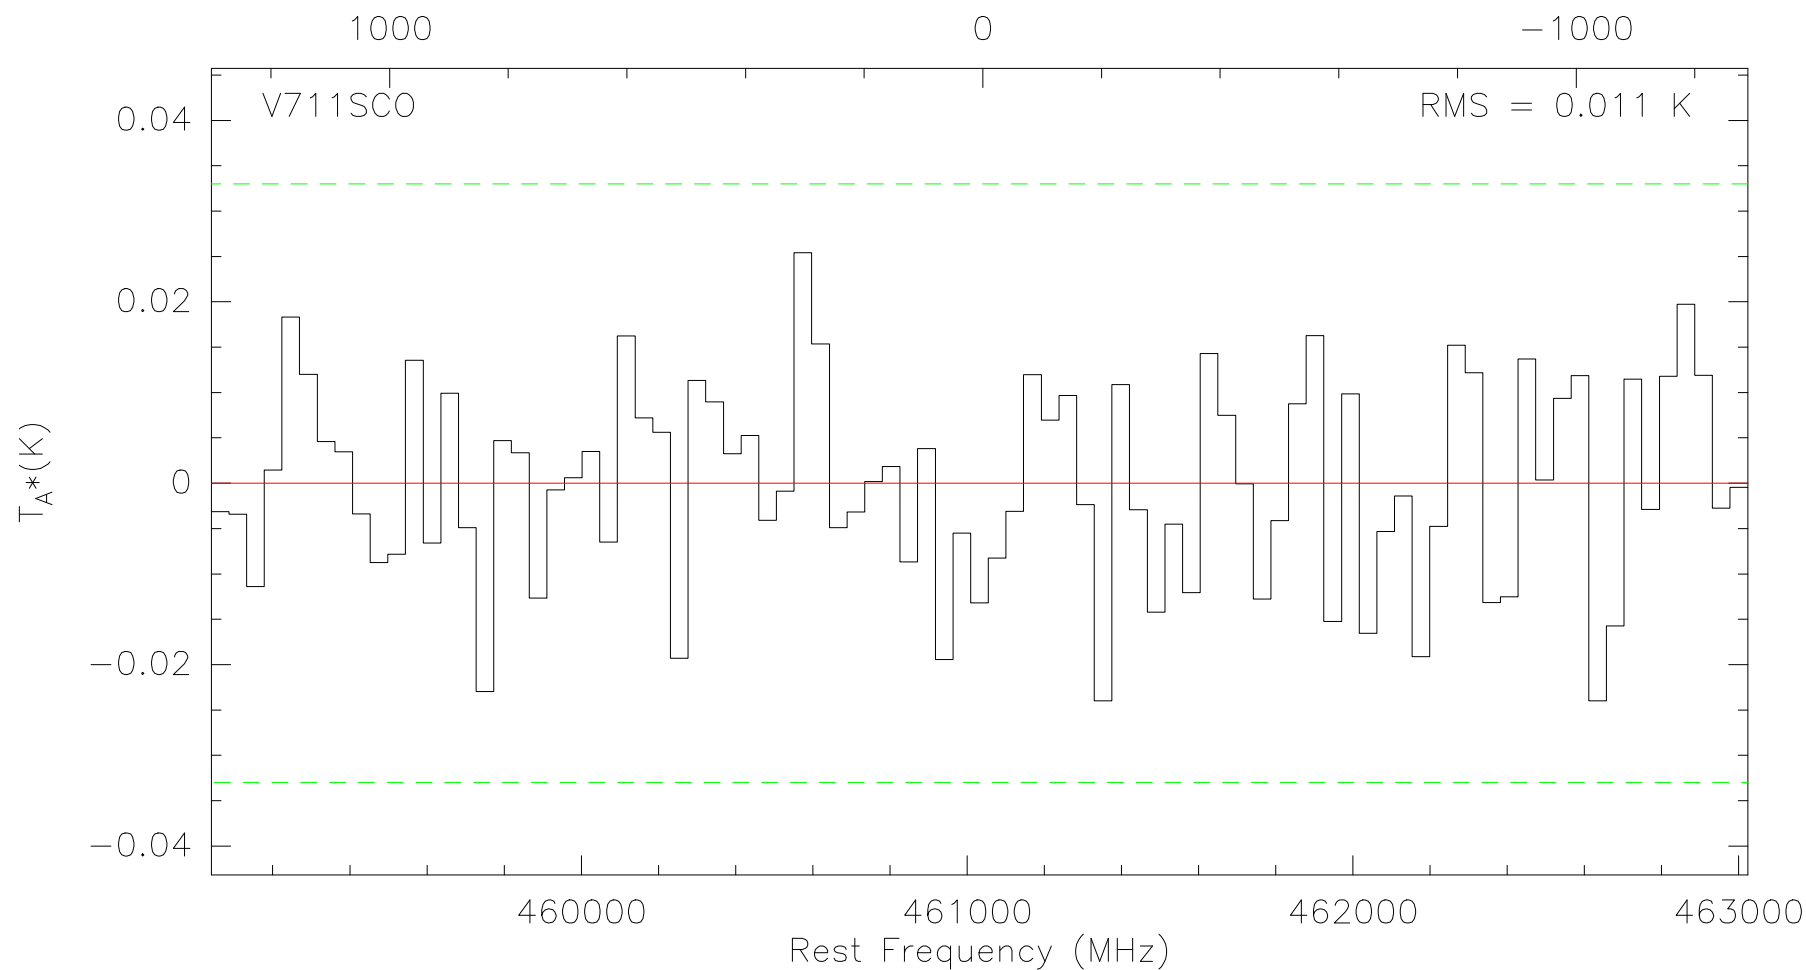

1;1 V729SCO CO(4-3) AP-FL01-XF0- 0:01-JUL-2016 R:07-AUG-2020  
RA: 17:22:02.66 DEC: -32:05:48.8 Eq 2000.0 Rad. 0.0° Offs: -0.2 -0.5  
Unknown tau: 1.225 Tsys: 3625. Time: 14.9min El: 30.0  
N: 87 IO: 44.1918 V0: 0.000 Dv: -29.77 LSR  
FO: 461040.768 Df: 45.78 Fi: 473040.769

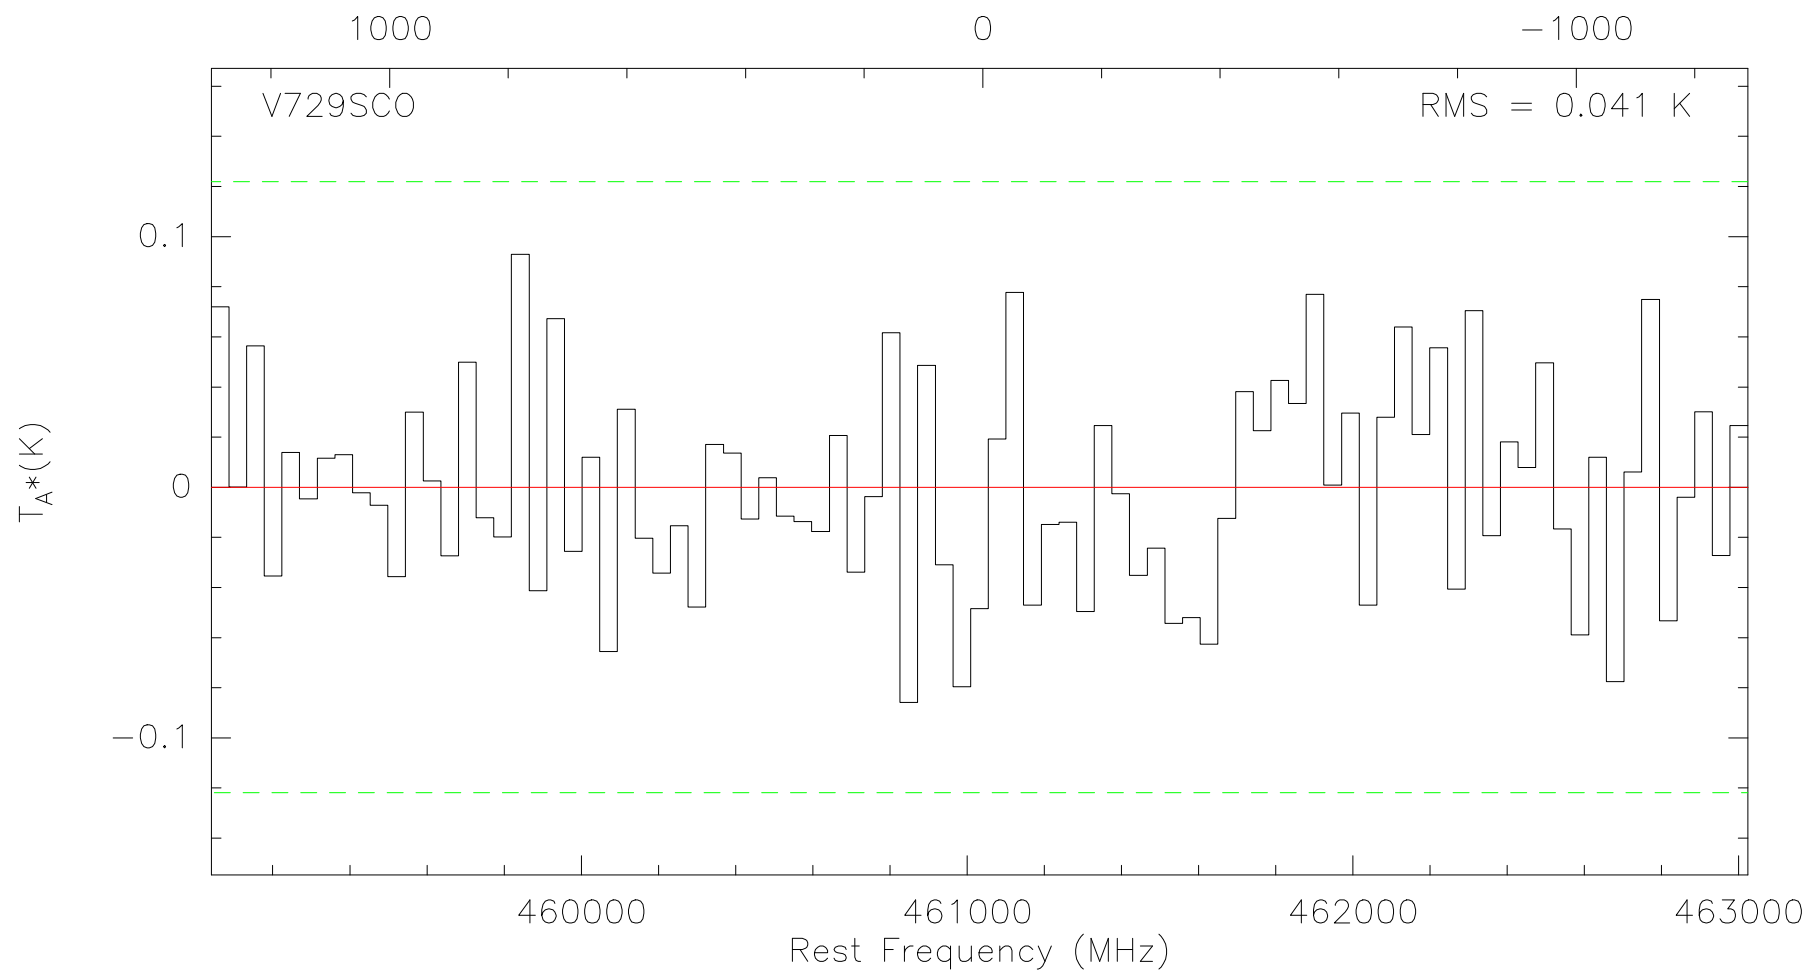

1;1 V732SGR CO(4-3) AP-FL01-XF0- O:13-JUL-2016 R:07-AUG-2020  
RA: 17:56:07.51 DEC: -27:22:16.1 Eq 2000.0 Rad. 0.0° Offs: +0.2 -0.4  
Unknown tau: 0.689 Tsys: 597. Time: 9.9min El: 71.8  
N: 87 lO: 44.1918 V0: 0.000 Dv: -29.77 LSR  
F0: 461040.768 Df: 45.78 Fi: 473040.767

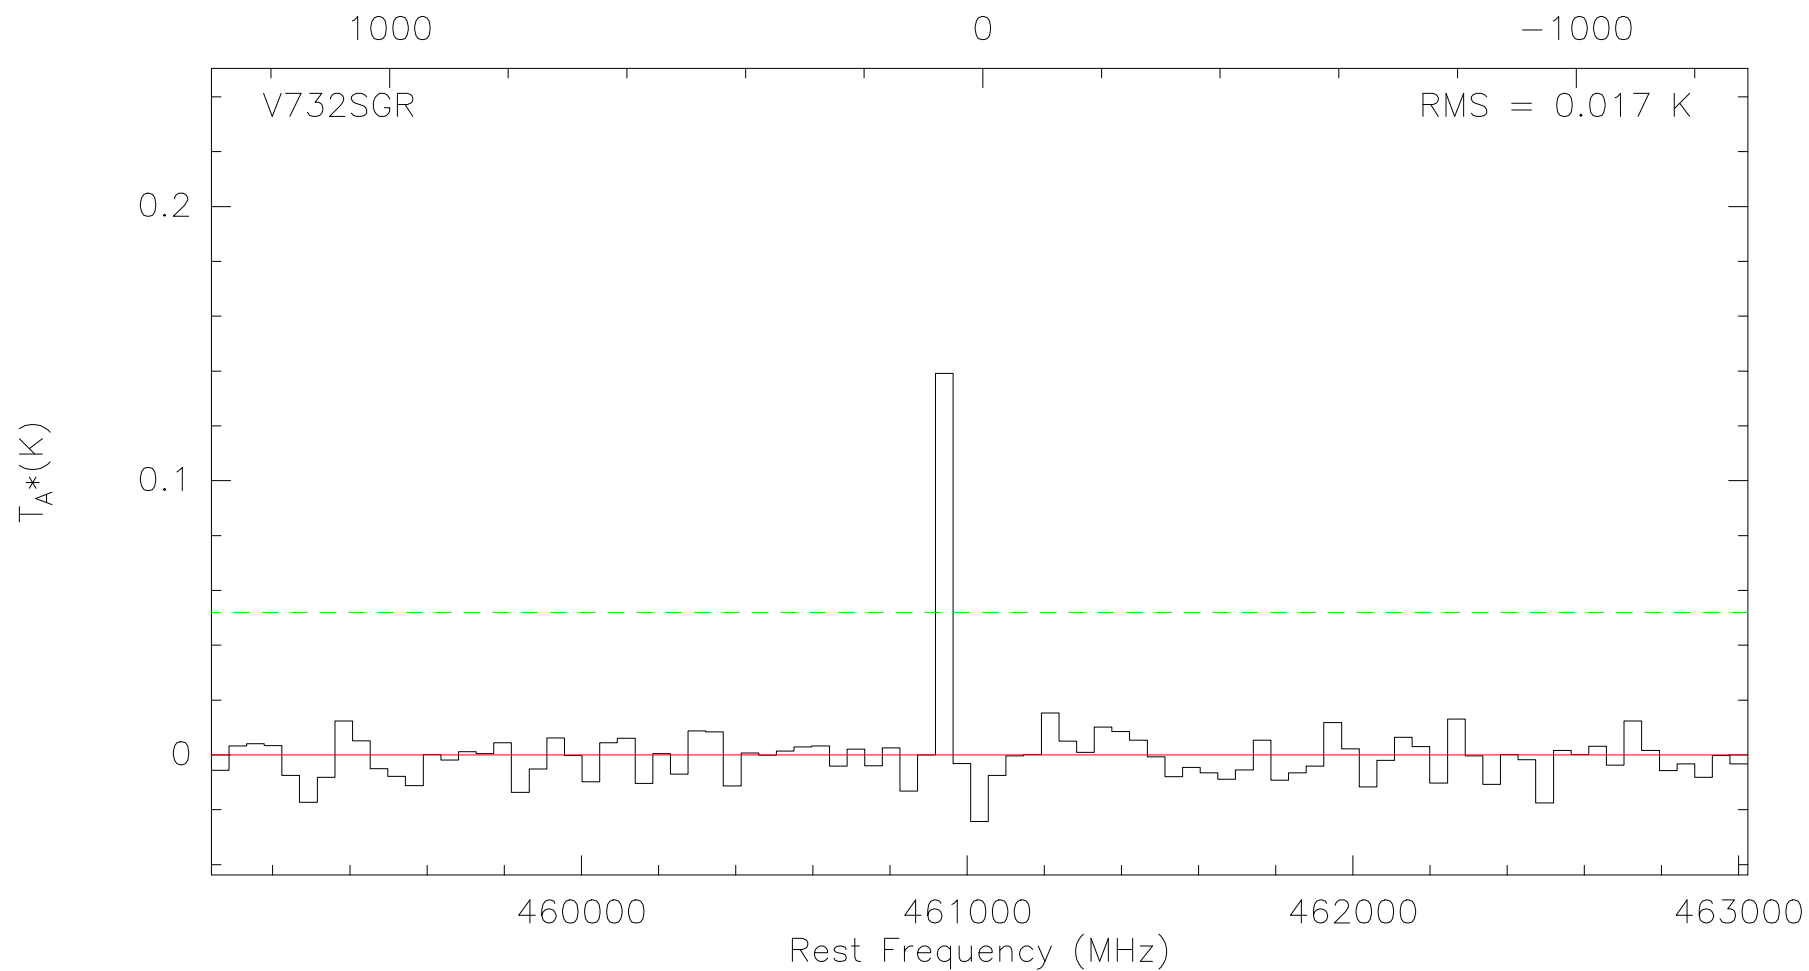

1;1 V733SCO CO(4-3) AP-FL01-XF0- 0:06-JUL-2016 R:07-AUG-2020

RA: 17:39:42.88 DEC: -35:52:38.4 Eq 2000.0 Rad. 0.0° Offs: +0.3 -0.3

Unknown tau: 0.691 Tsys: 1079. Time: 9.9min El: 37.6

N: 87 IO: 44.1918 V0: 0.000 Dv: -29.77 LSR

F0: 461040.768 Df: 45.78 Fi: 473040.811

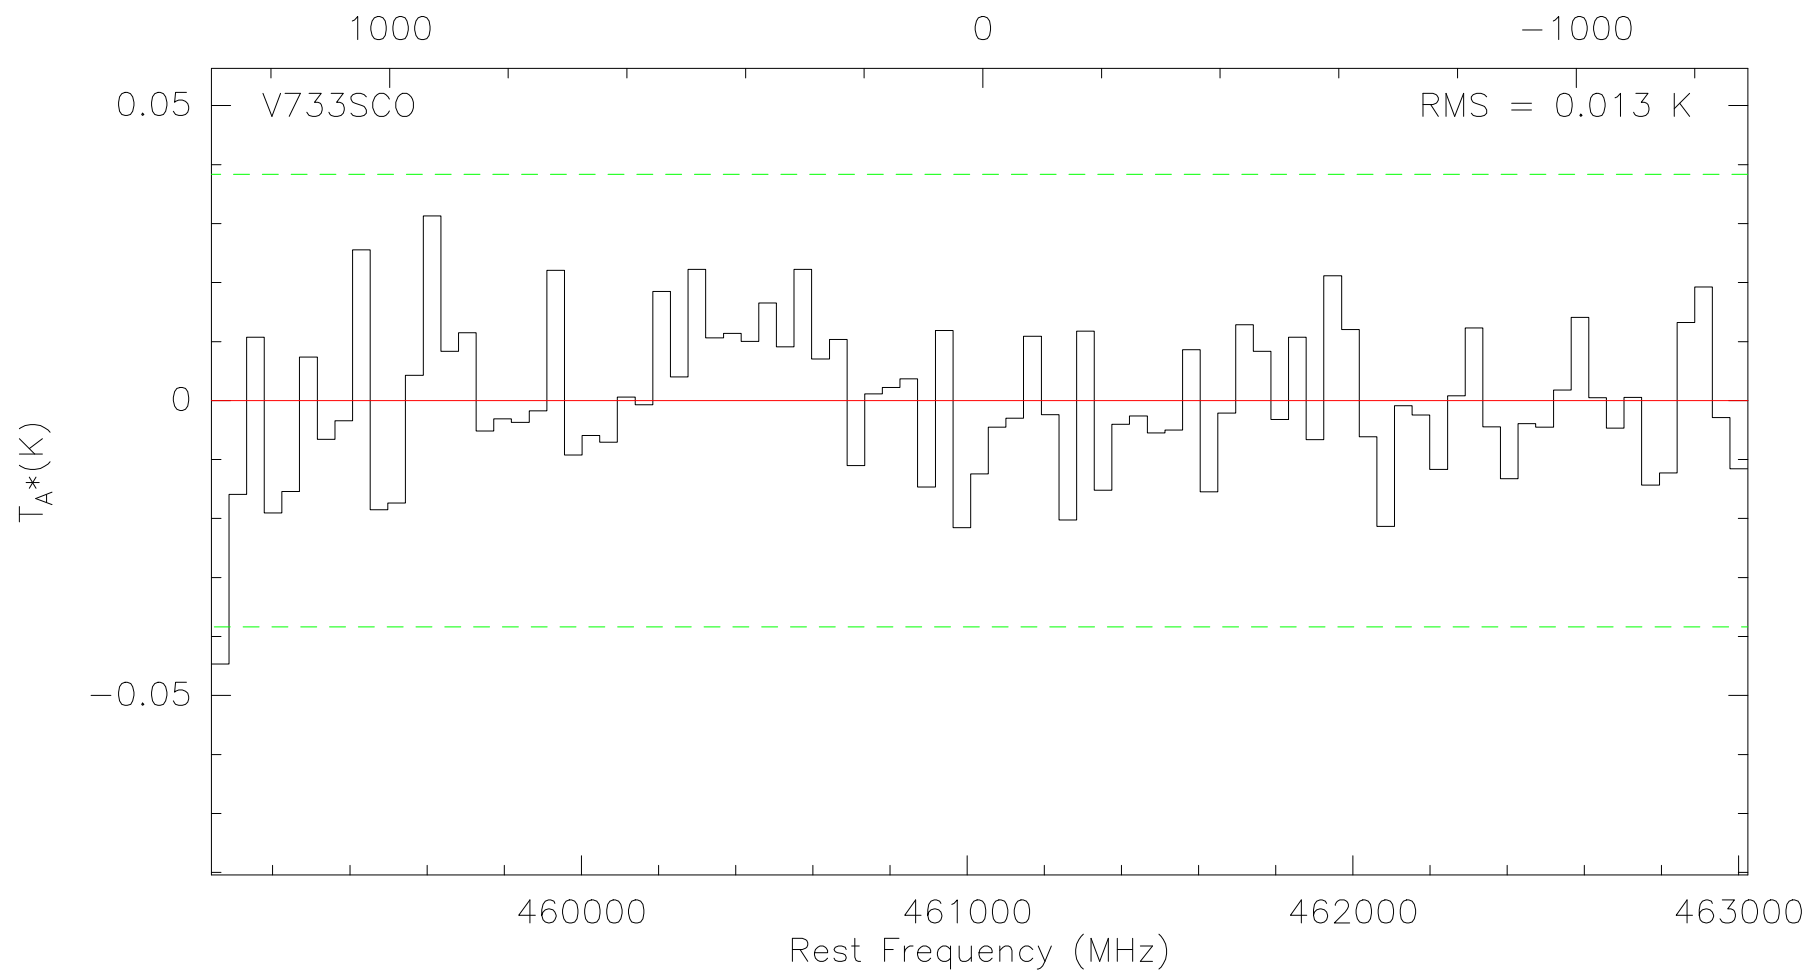

1;1 V737SGR CO(4-3) AP-FL01-XF0- O:14-JUL-2016 R:07-AUG-2020

RA: 18:07:08.66 DEC: -28:44:52.3 Eq 2000.0 Rad. 0.0° Offs: +0.2 -0.4

Unknown tau: 0.741 Tsys: 676. Time: 9.9min El: 70.3

N: 87 IO: 44.1918 V0: 0.000 Dv: -29.77 LSR

F0: 461040.768 Df: 45.78 Fi: 473040.755

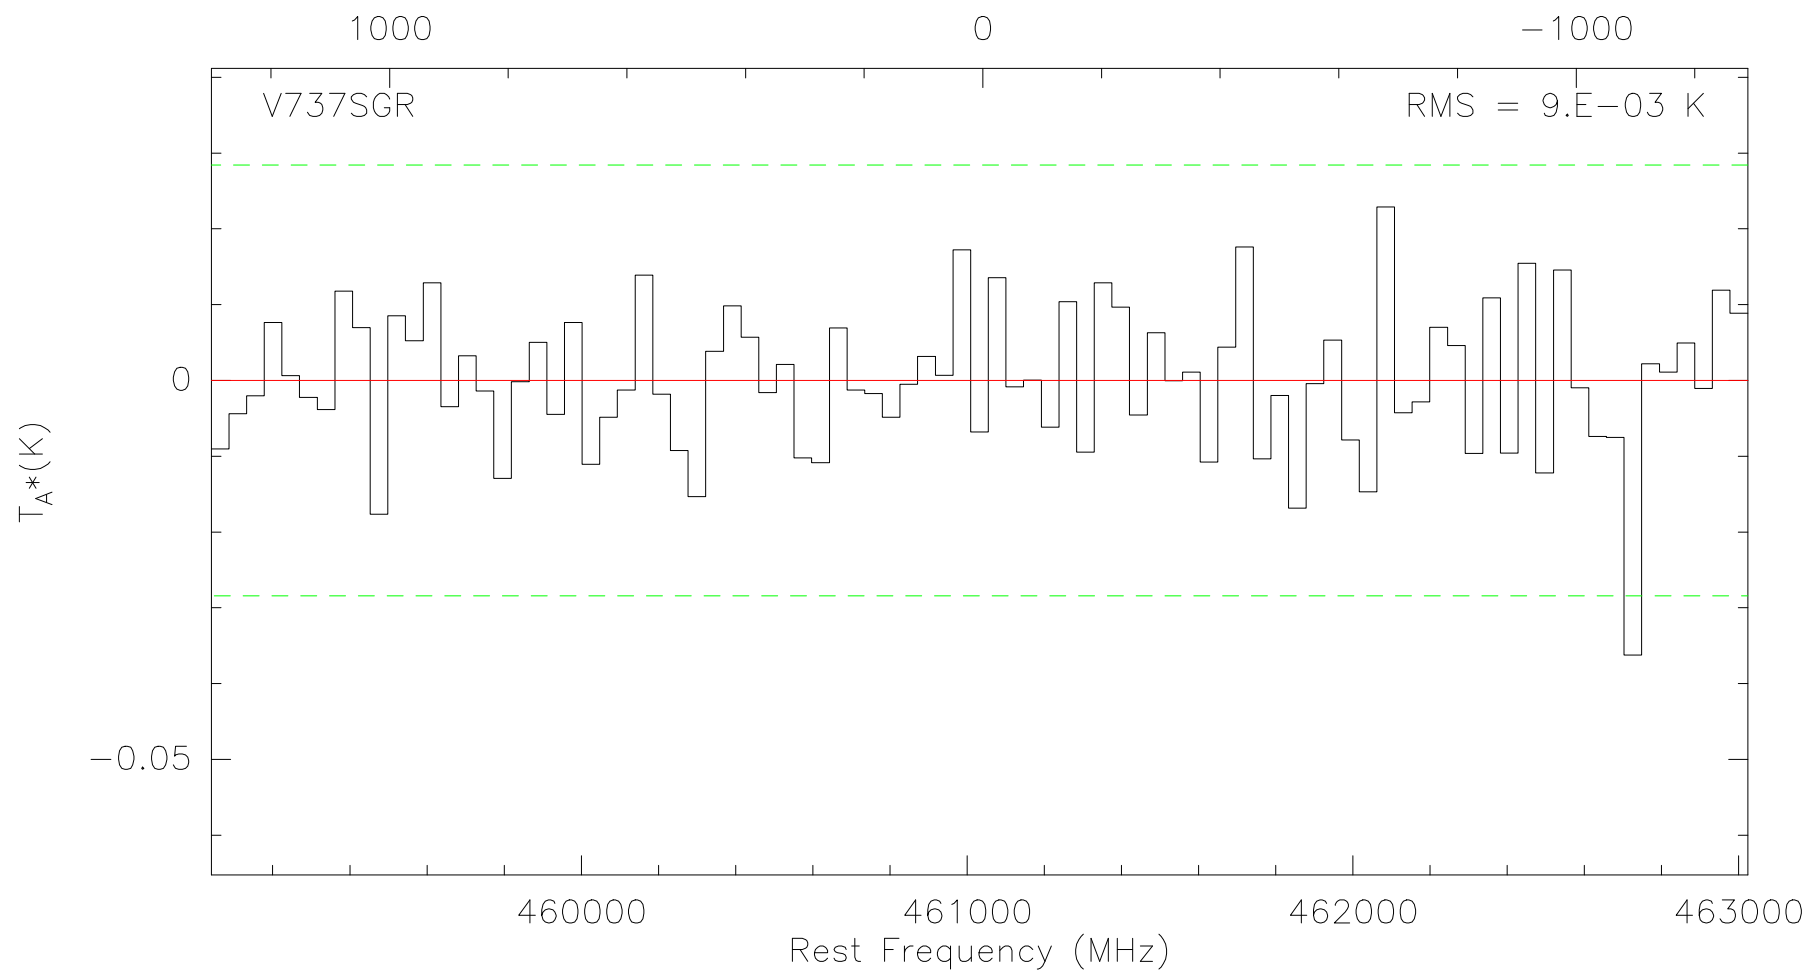

1;1 V745SCO CO(4-3) AP-FL01-XF0- O:13-JUL-2016 R:07-AUG-2020  
RA: 17:55:22.27 DEC: -33:14:58.5 Eq 2000.0 Rad. 0.0° Offs: +0.0 -0.7  
Unknown tau: 0.551 Tsys: 462. Time: 9.9min El: 77.6  
N: 87 IO: 44.1918 V0: 0.000 Dv: -29.77 LSR  
FO: 461040.768 Df: 45.78 Fi: 473040.844

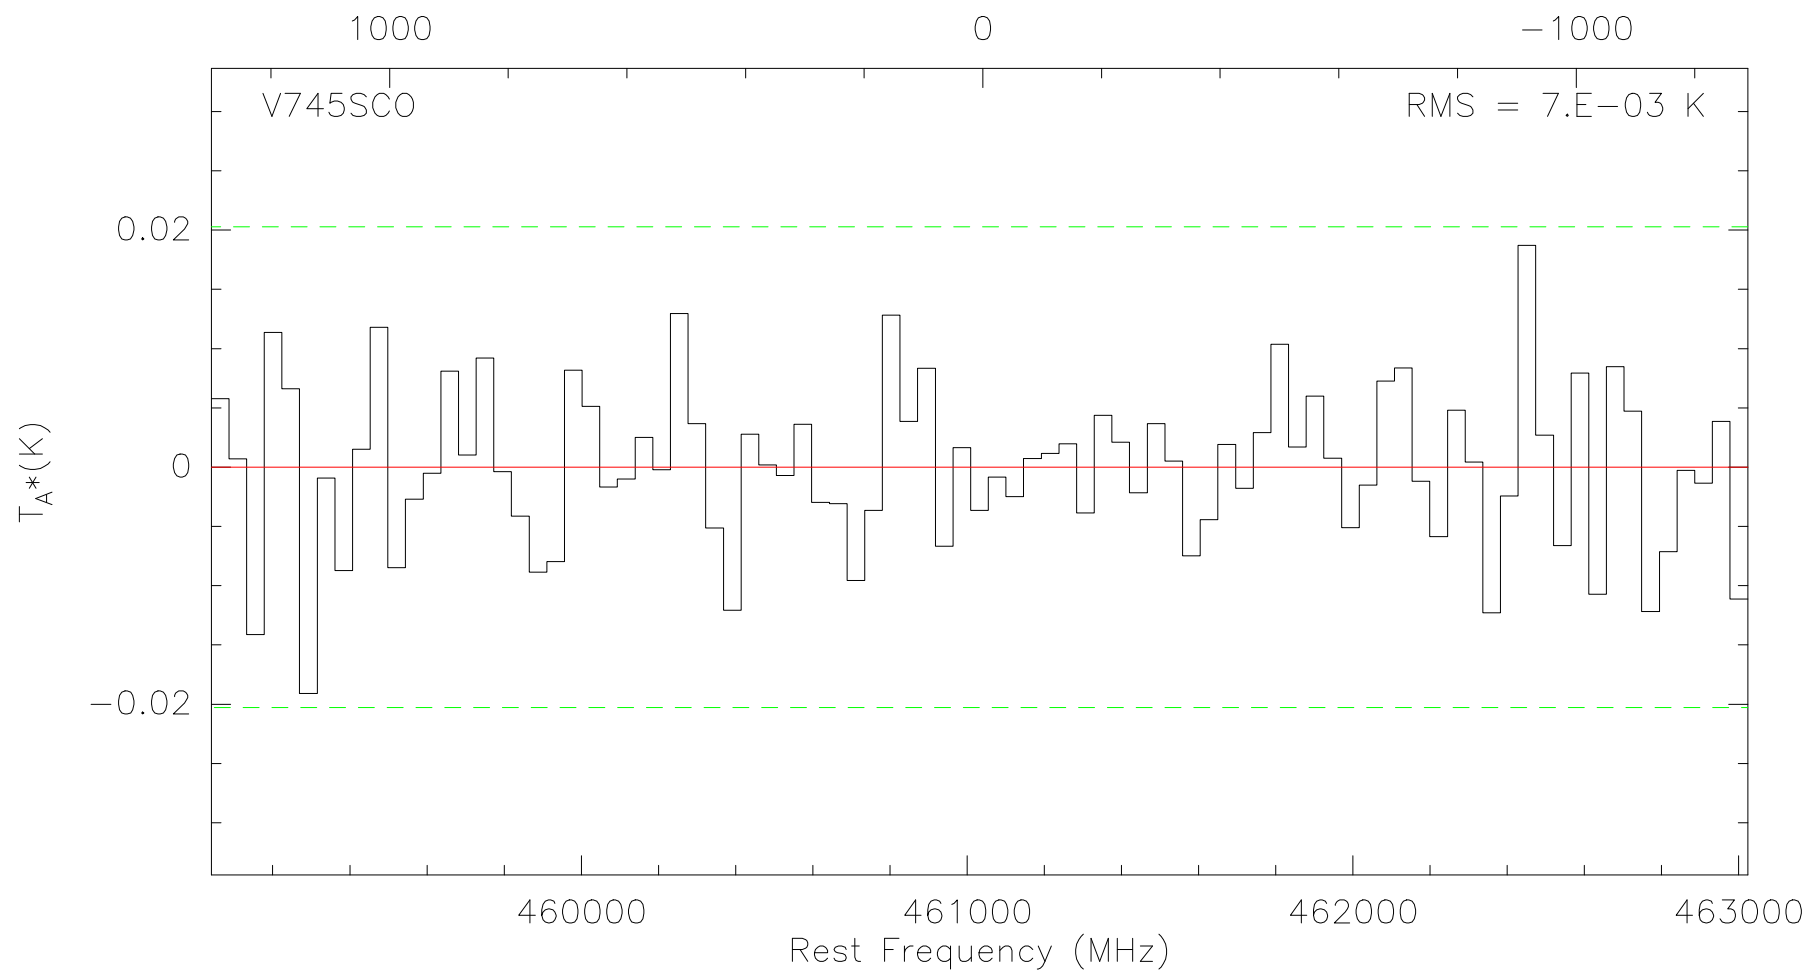

1;1 V787SGR CO(4-3) AP-FL01-XF0- O:14-JUL-2016 R:07-AUG-2020  
RA: 18:00:02.20 DEC: -30:30:31.0 Eq 2000.0 Rad. 0.0° Offs: +0.2 -0.3  
Unknown tau: 0.826 Tsys: 795. Time: 9.9min El: 62.7  
N: 87 l0: 44.1918 V0: 0.000 Dv: -29.77 LSR  
F0: 461040.768 Df: 45.78 Fi: 473040.802

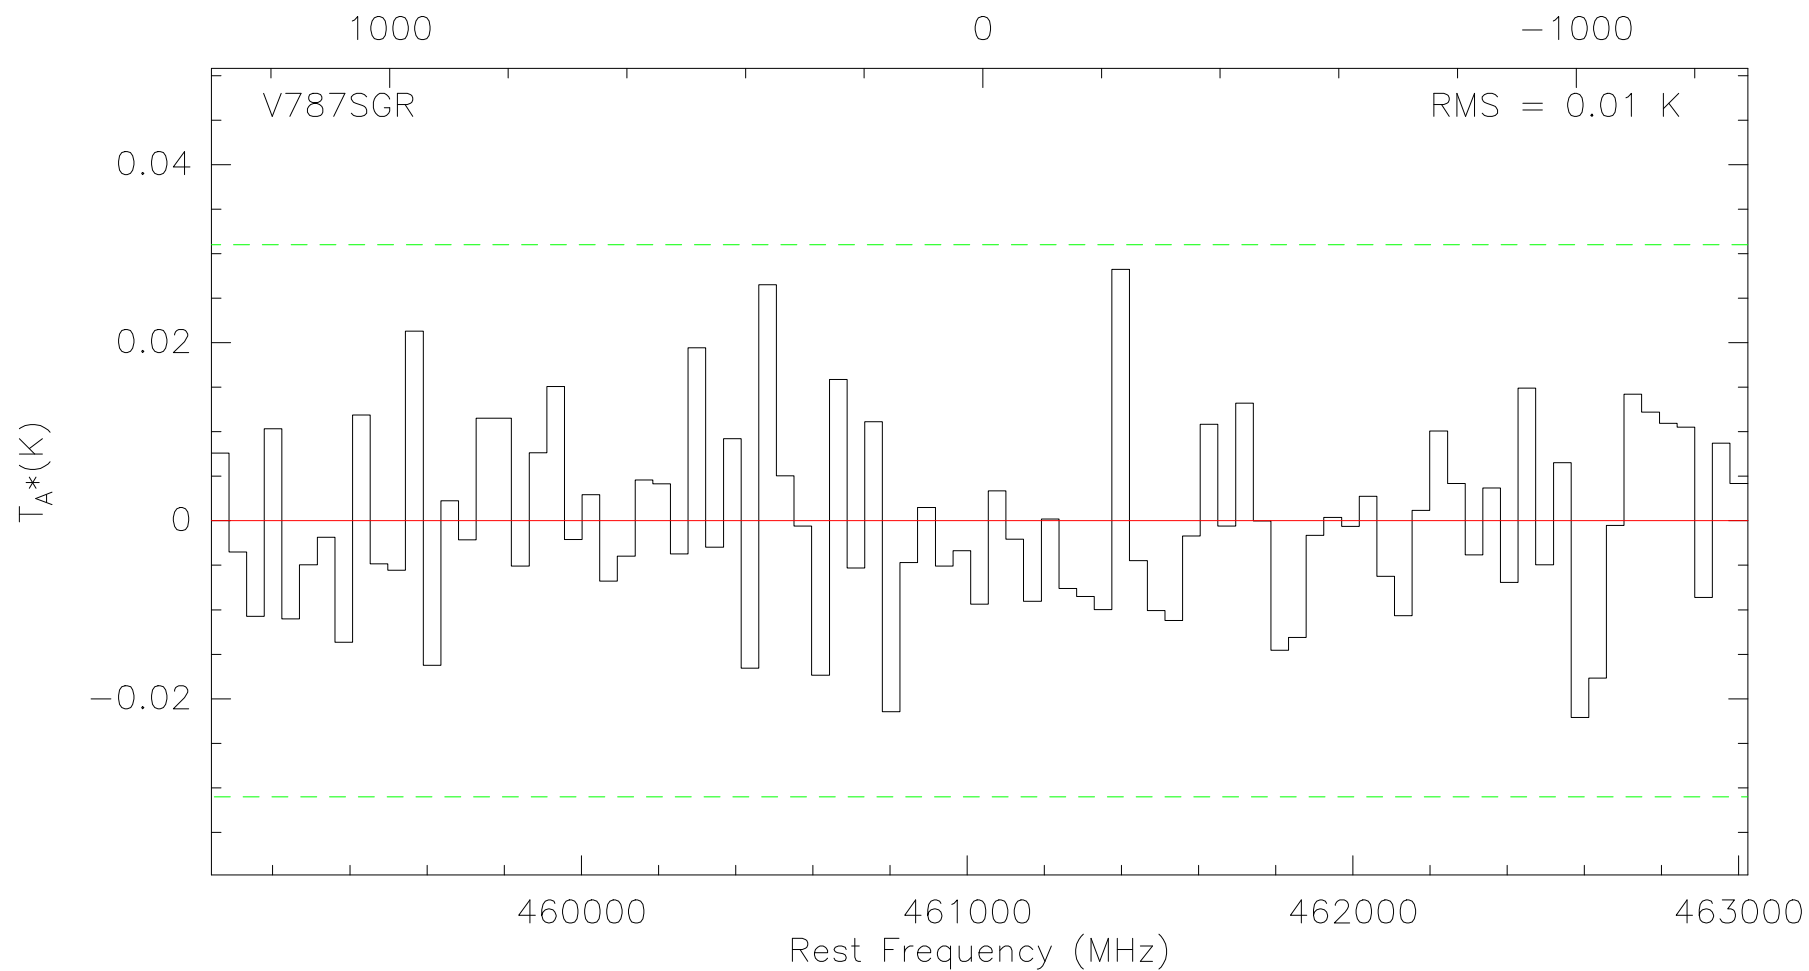

1;1 V7940PH CO(4-3) AP-FL01-XF0- O:01-JUL-2016 R:07-AUG-2020  
RA: 17:38:49.25 DEC: -22:50:48.9 Eq 2000.0 Rad. 0.0° Offs: -0.2 -0.5  
Unknown tau: 1.242 Tsys: 2262. Time: 9.9min El: 42.1  
N: 87 IO: 44.1918 V0: 0.000 Dv: -29.77 LSR  
FO: 461040.768 Df: 45.78 Fi: 473040.593

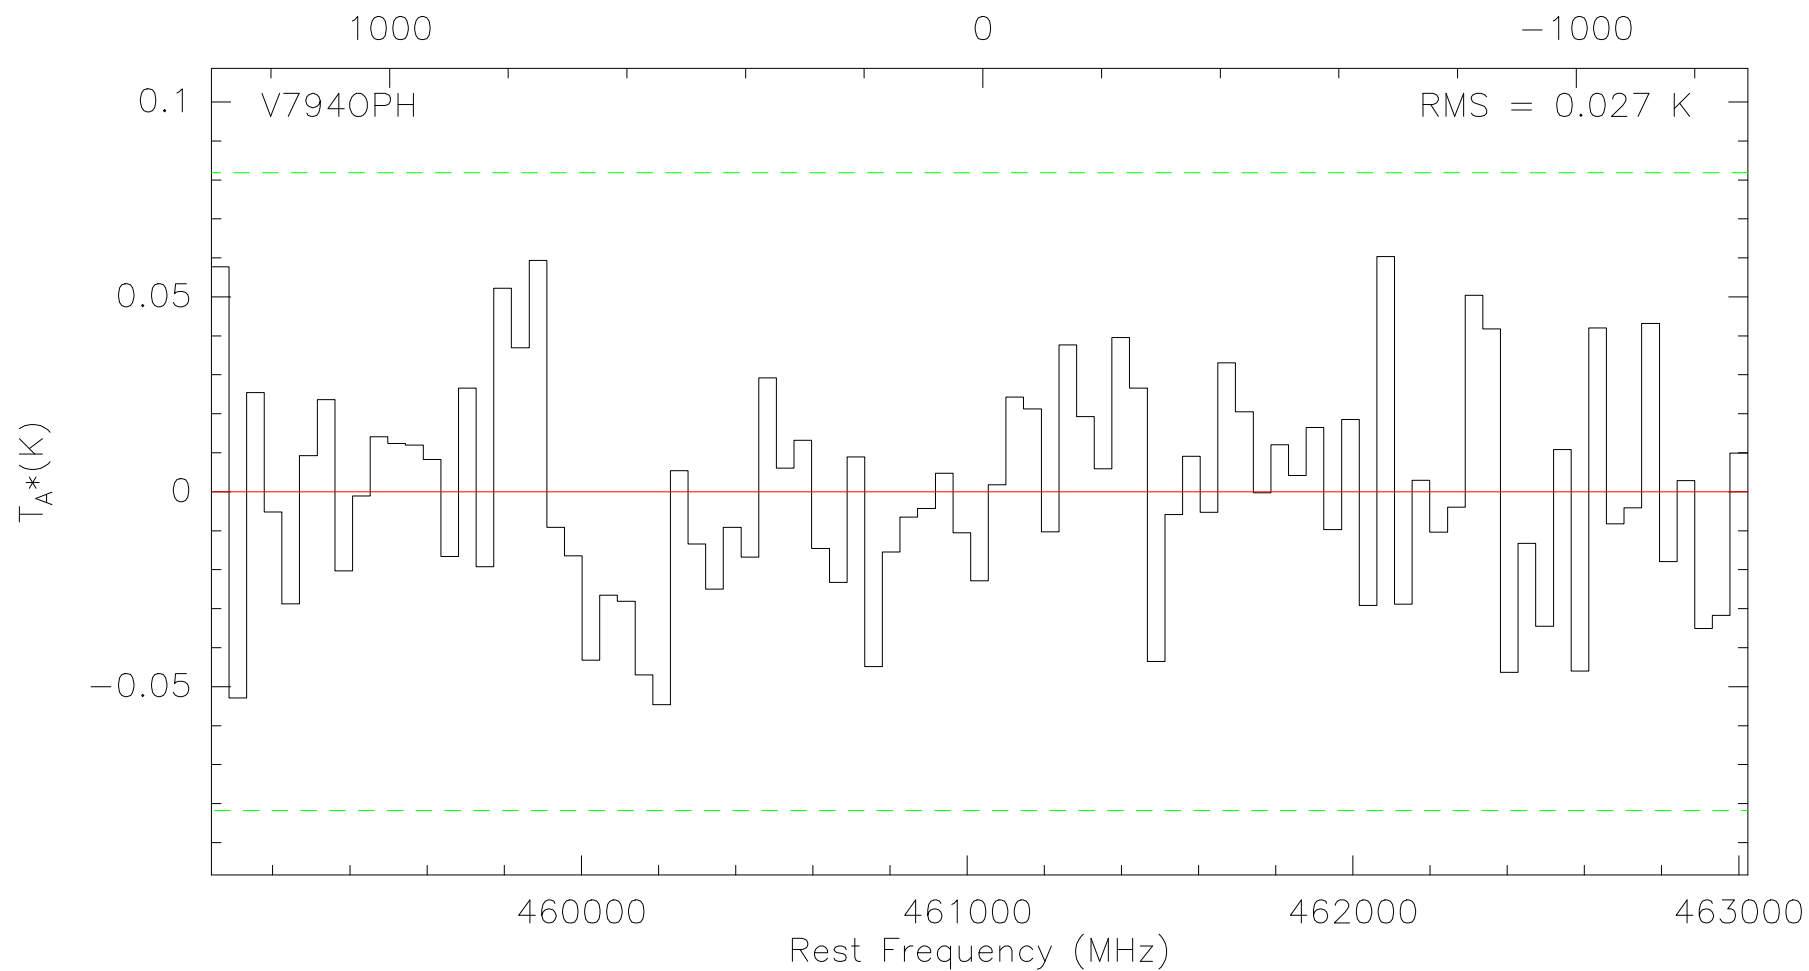

1;1 V909SGR CO(4-3) AP-FL01-XF0- O:13-JUL-2016 R:07-AUG-2020  
RA: 18:25:52.30 DEC: -35:01:27.0 Eq 2000.0 Rad. 0.0° Offs: +0.2 -0.4  
Unknown tau: 0.685 Tsys: 617. Time: 9.9min El: 67.4  
N: 87 IO: 44.1918 V0: 0.000 Dv: -29.77 LSR  
FO: 461040.768 Df: 45.78 Fi: 473040.737

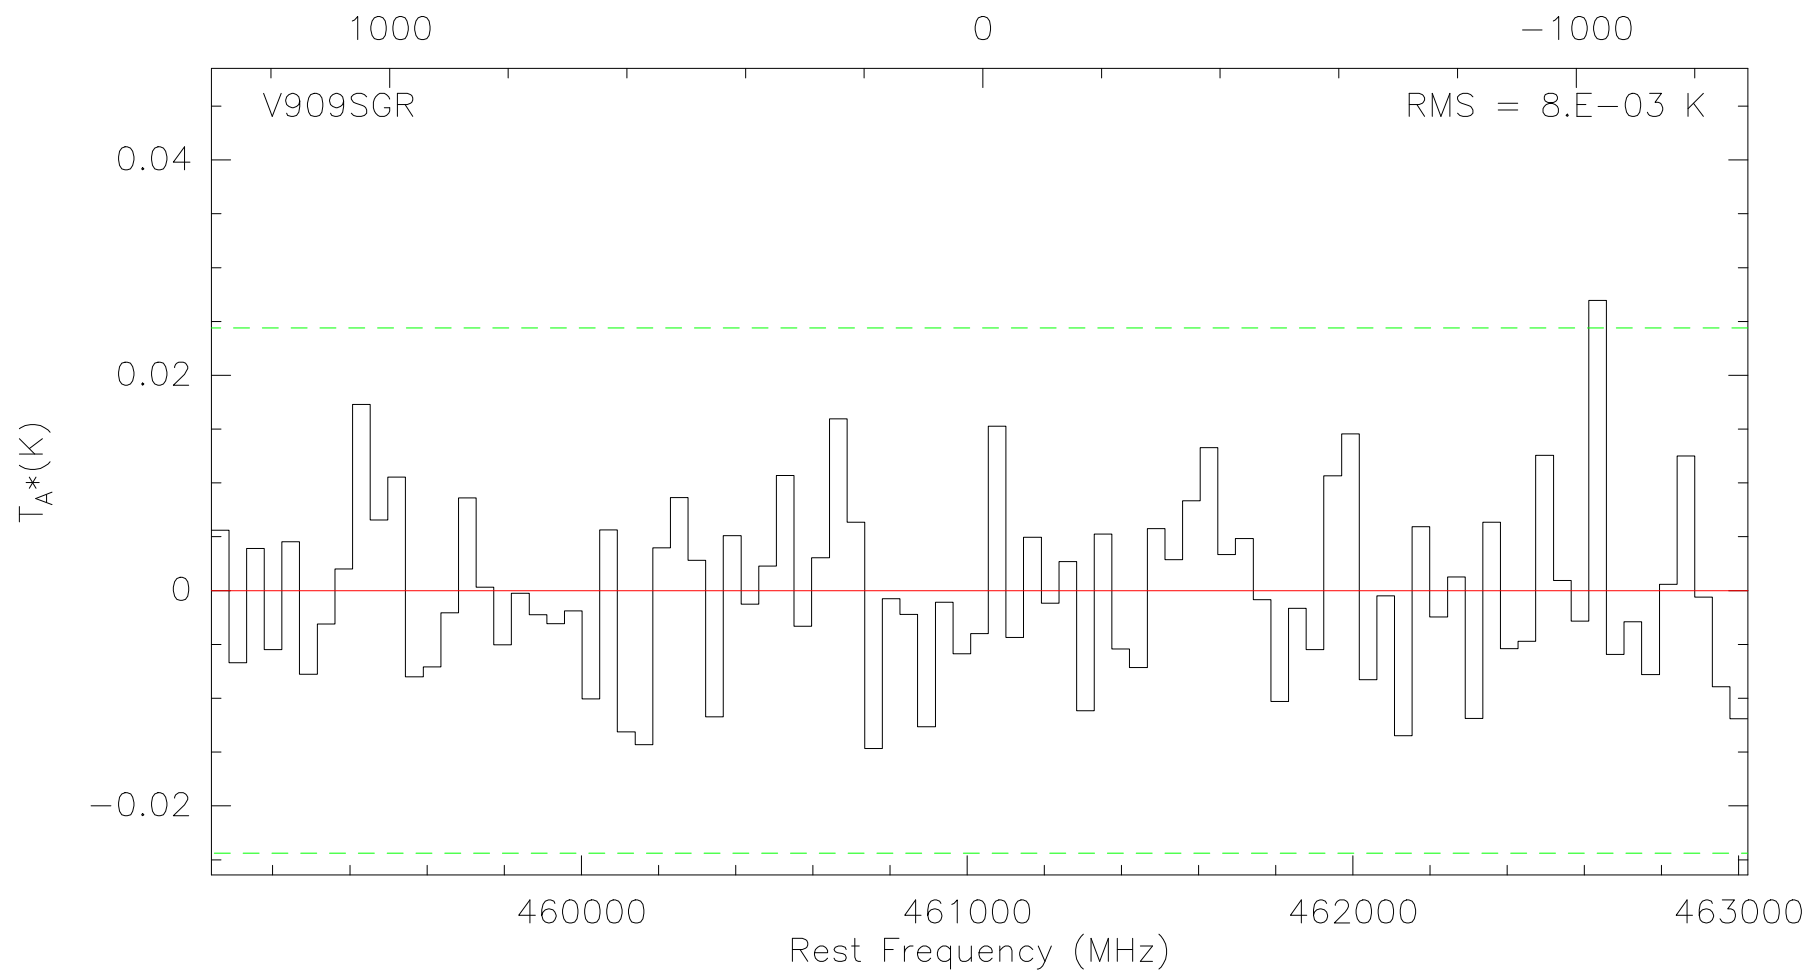

1;1 V941SGR CO(4-3) AP-FL01-XF0- O:13-JUL-2016 R:07-AUG-2020  
RA: 18:34:43.46 DEC: -29:34:49.1 Eq 2000.0 Rad. 0.0° Offs: -0.2 -0.3  
Unknown tau: 0.440 Tsys: 820. Time: 9.9min El: 25.8  
N: 87 IO: 44.1918 V0: 0.000 Dv: -29.77 LSR  
FO: 461040.768 Df: 45.78 Fi: 473040.659

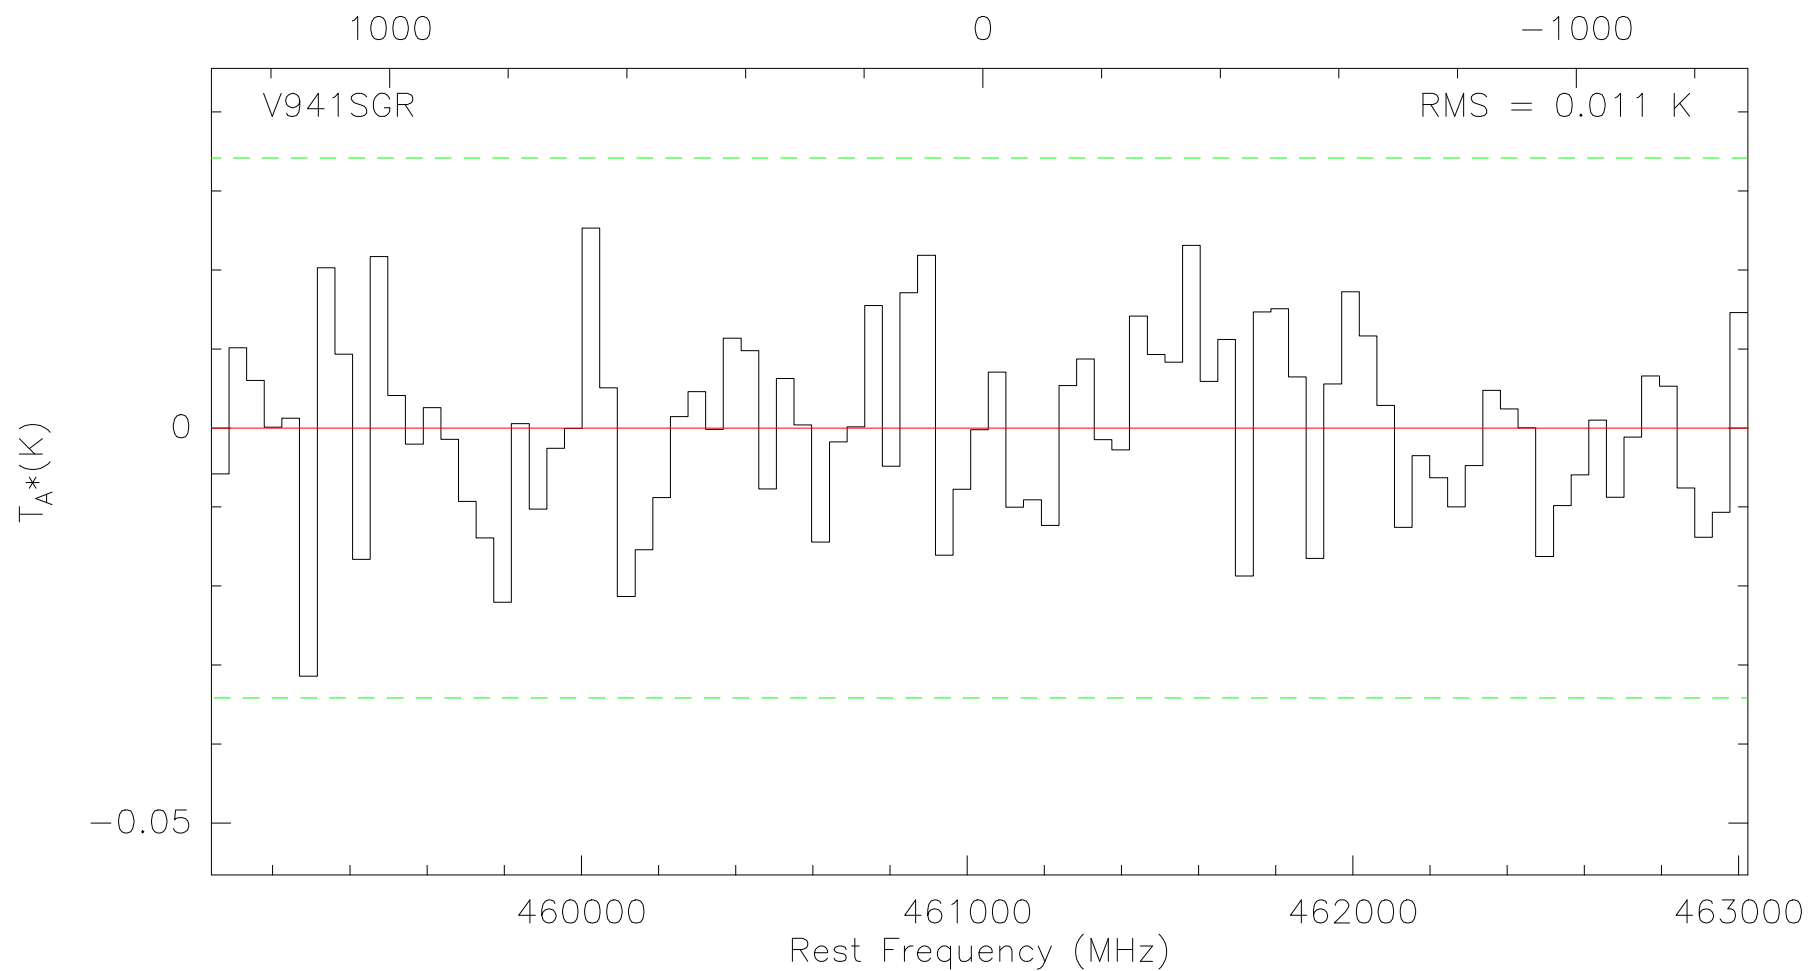

1;1 V999SGR CO(4-3) AP-FL01-XF0- O:13-JUL-2016 R:07-AUG-2020  
RA: 18:00:05.59 DEC: -27:33:14.0 Eq 2000.0 Rad. 0.0° Offs: -0.2 -0.4  
Unknown tau: 0.494 Tsys: 616. Time: 9.9min El: 38.9  
N: 87 IO: 44.1918 V0: 0.000 Dv: -29.77 LSR  
FO: 461040.768 Df: 45.78 Fi: 473040.775

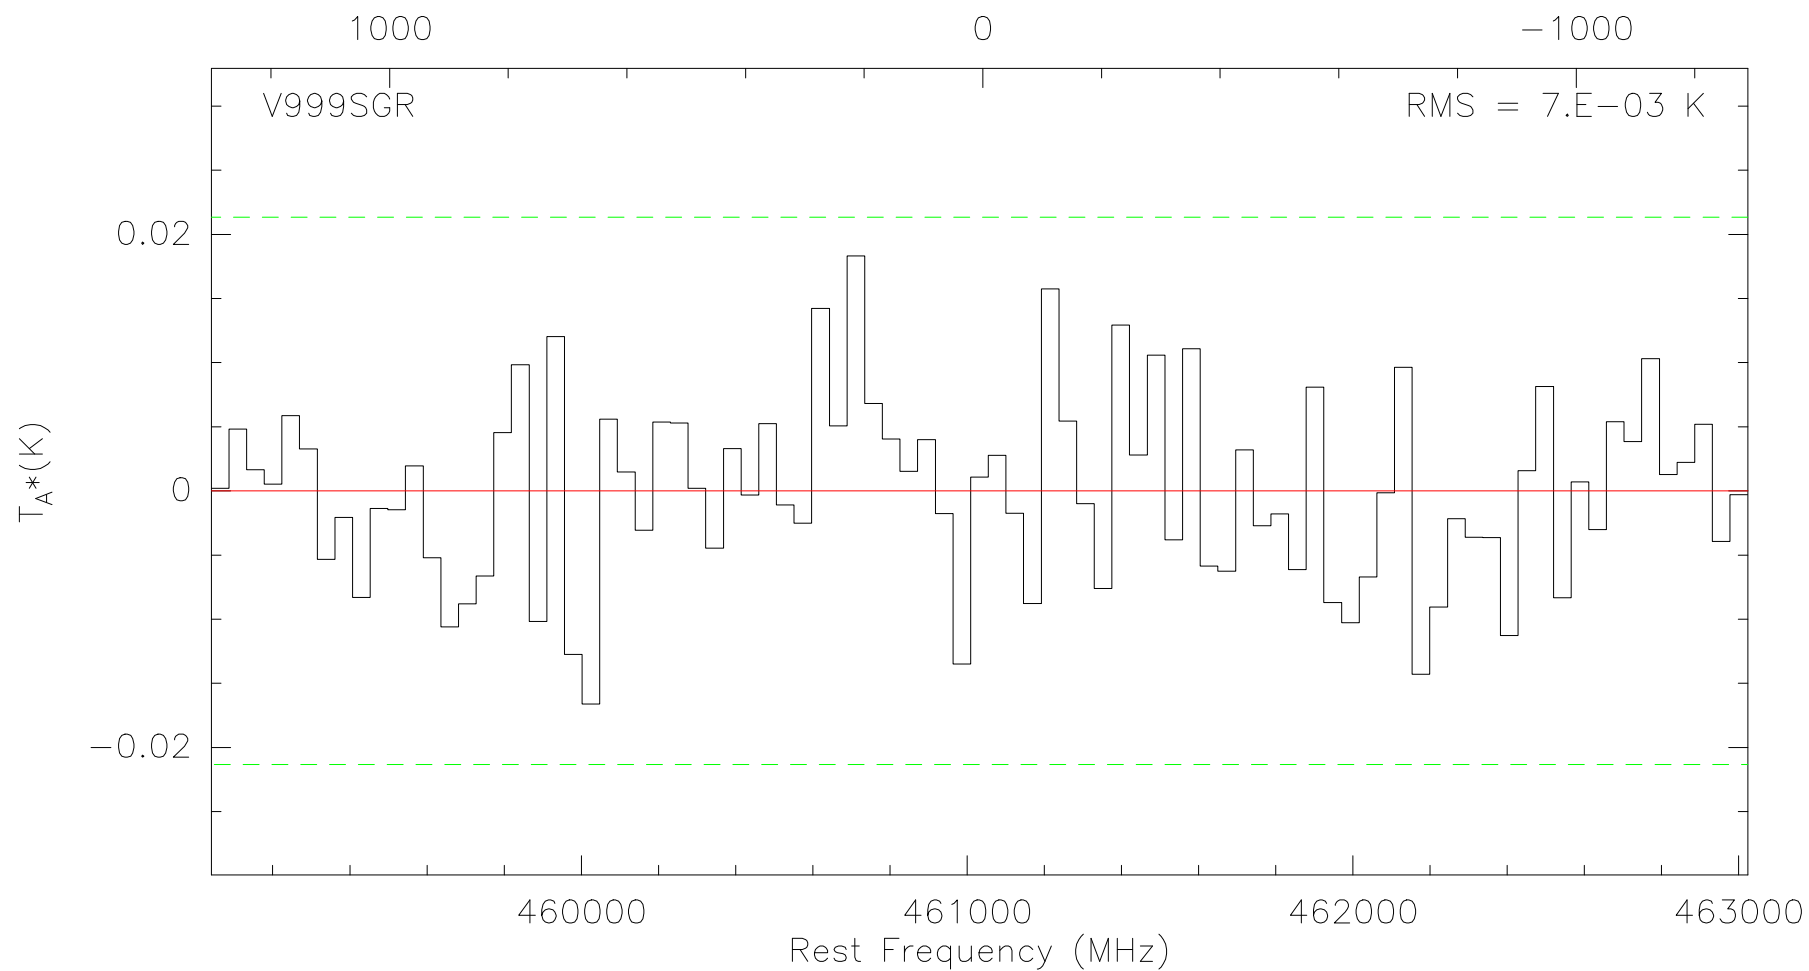

1;1 V1148-SGR CO(4-3) AP-FL01-XF0- 0:03-JUN-2015 R:13-AUG-2020

RA: 18:09:05.85 DEC: -25:59:08.0 Eq 2000.0 Rad. 0.0° Offs: +0.2 -0.4

Unknown tau: 0.649 Tsys: 463. Time: 44.6min El: 48.5

N: 87 l0: 44.1918 V0: 0.000 Dv: -29.76 LSR

F0: 461040.768 Df: 45.77 Fi: 473039.145

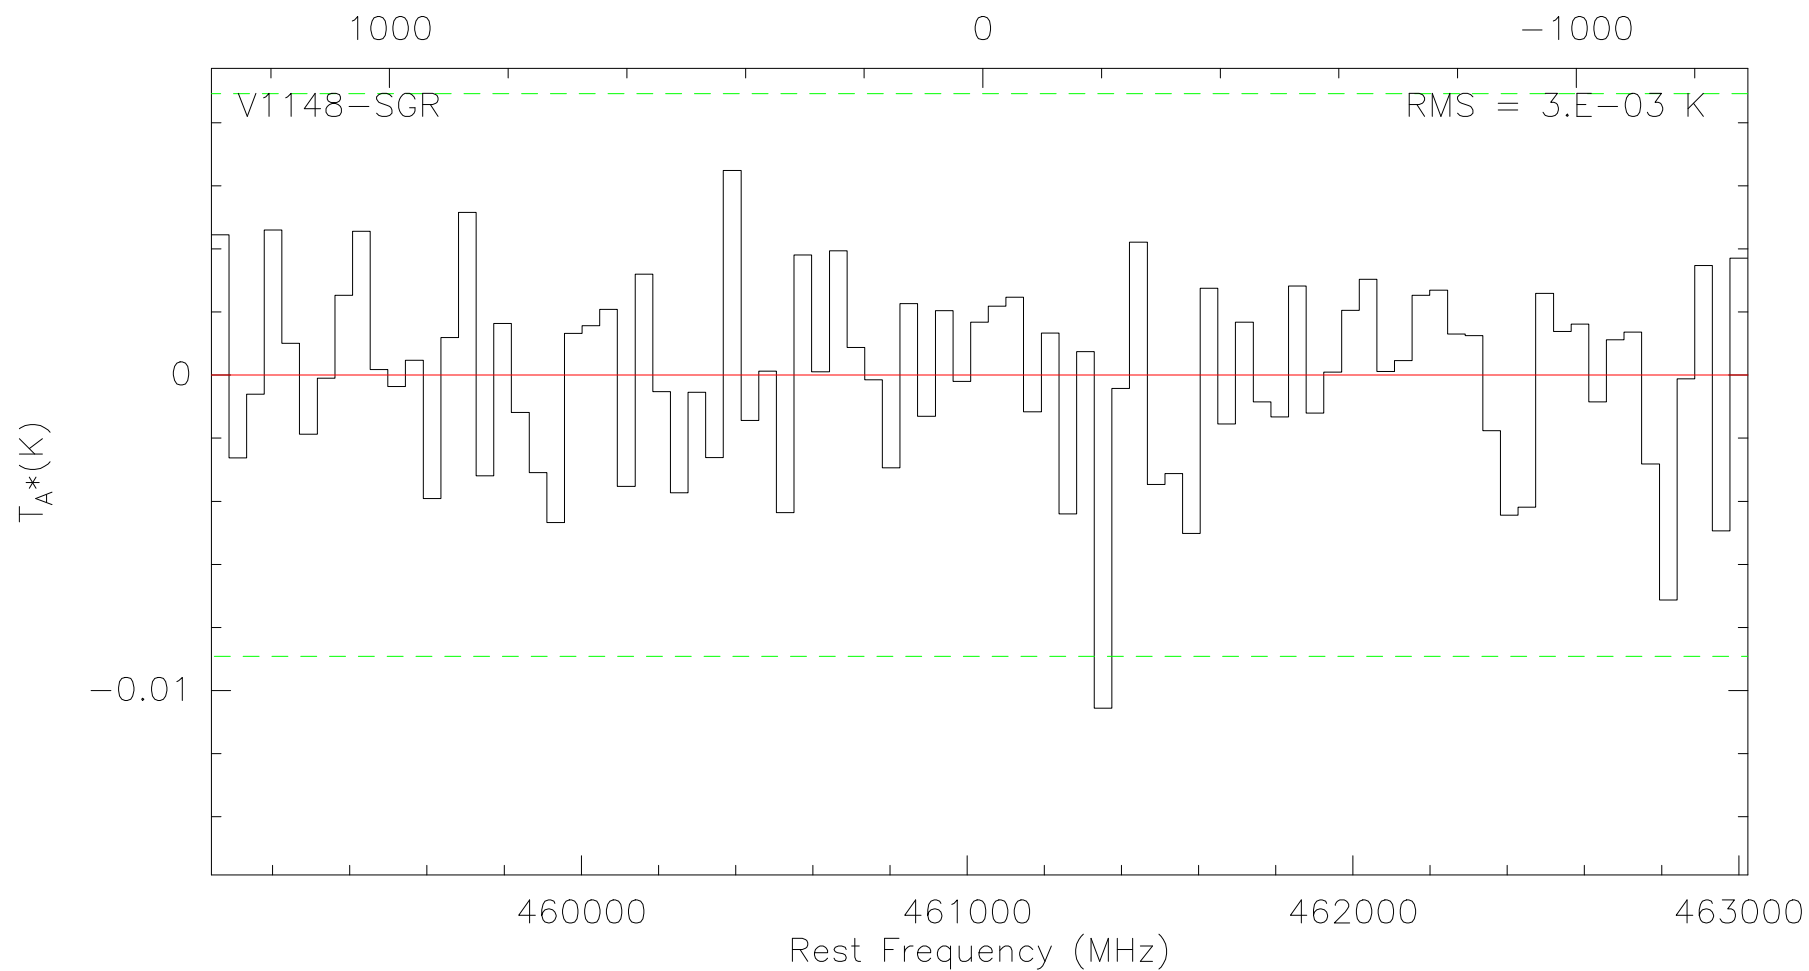

Supplement: Supplementary file 3 [file all_sm_CO43.pdf]
