# Supplementary material for: A search for cool molecular gas in GK Persei and other classical novae
Source: arXiv:2201.10332 source file (2022-01-25)

1;1 CN-VEL CO(4-3) OSB AP-FL02-XF0- 0:24-AUG-2014 R:12-AUG-2020  
RA: 11:02:38.57 DEC: -54:23:09.5 Eq 2000.0 Rad. 0.0° Offs: -0.1 -0.5  
Unknown tau: 1.808 Tsys: 2460. Time: 23.4min El: 50.6  
N: 87 l0: 44.1919 V0: 0.000 Dv: 29.01 LSR  
FO: 473041.715 Df: -45.78 Fi: 461040.768

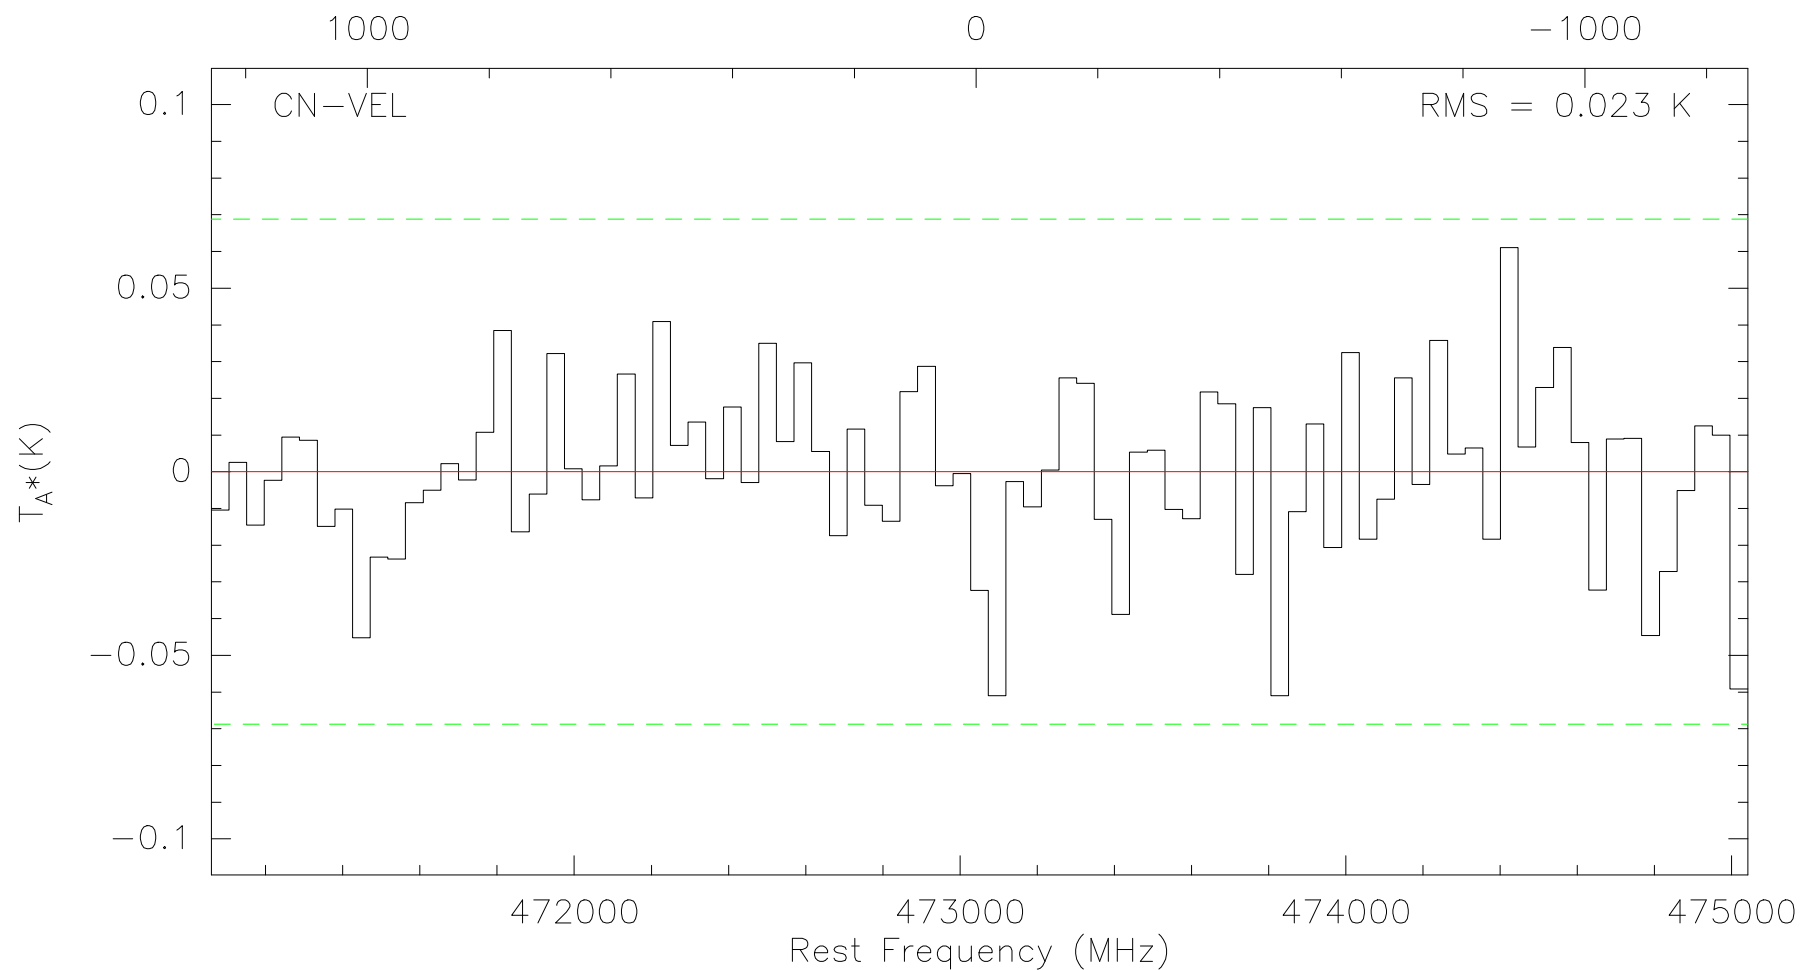

1;1 CQ-VEL CO(4-3) OSB AP-FL02-XF0- 0:26-AUG-2014 R:12-AUG-2020  
RA: 08:58:50.99 DEC: -53:20:17.8 Eq 2000.0 Rad. 0.0° Offs: +0.1 -0.5  
Unknown tau: 1.379 Tsys: 1509. Time: 23.4min El: 58.6  
N: 87 l0: 44.1919 V0: 0.000 Dv: 29.01 LSR  
FO: 473041.532 Df: -45.78 Fi: 461040.768

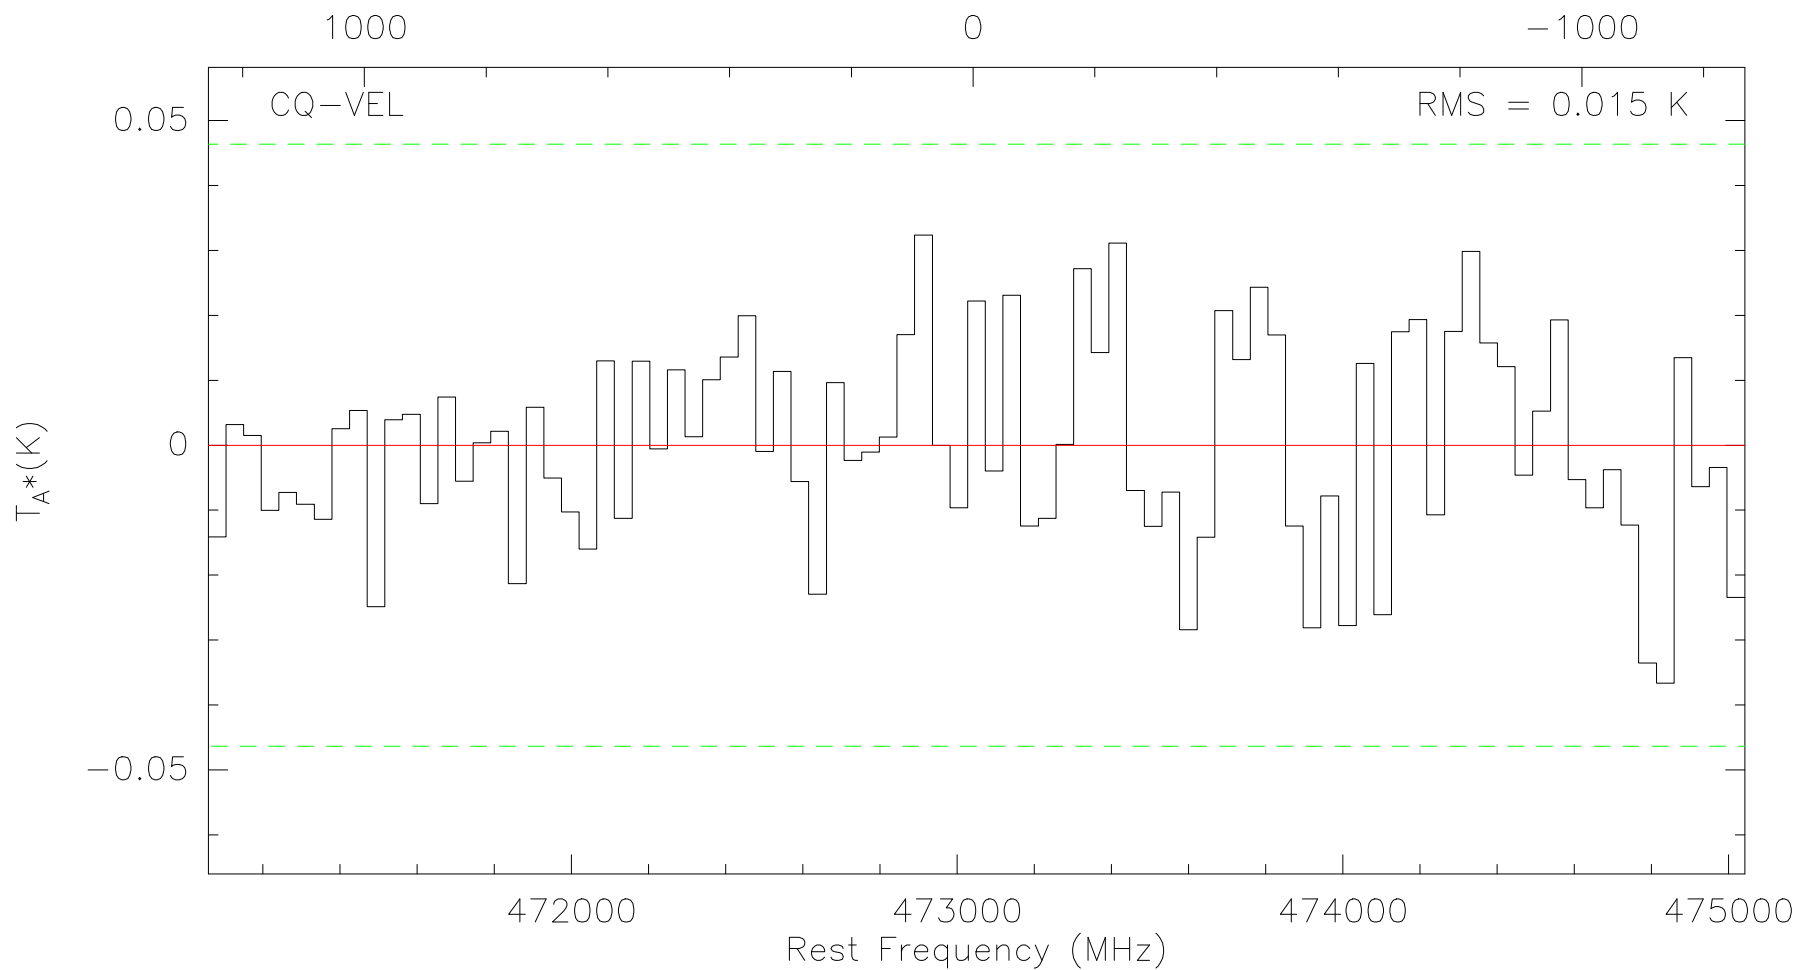

1;1 DY-PUP CO(4-3) OSB AP-FL02-XF0- 0:25-AUG-2014 R:12-AUG-2020  
RA: 08:13:48.51 DEC: -26:33:56.5 Eq 2000.0 Rad. 0.0° Offs: +0.2 -0.2  
Unknown tau: 1.337 Tsys: 1084. Time: 23.5min El: 65.1  
N: 87 l0: 44.1919 V0: 0.000 Dv: 29.01 LSR  
F0: 473041.196 Df: -45.78 Fi: 461040.768

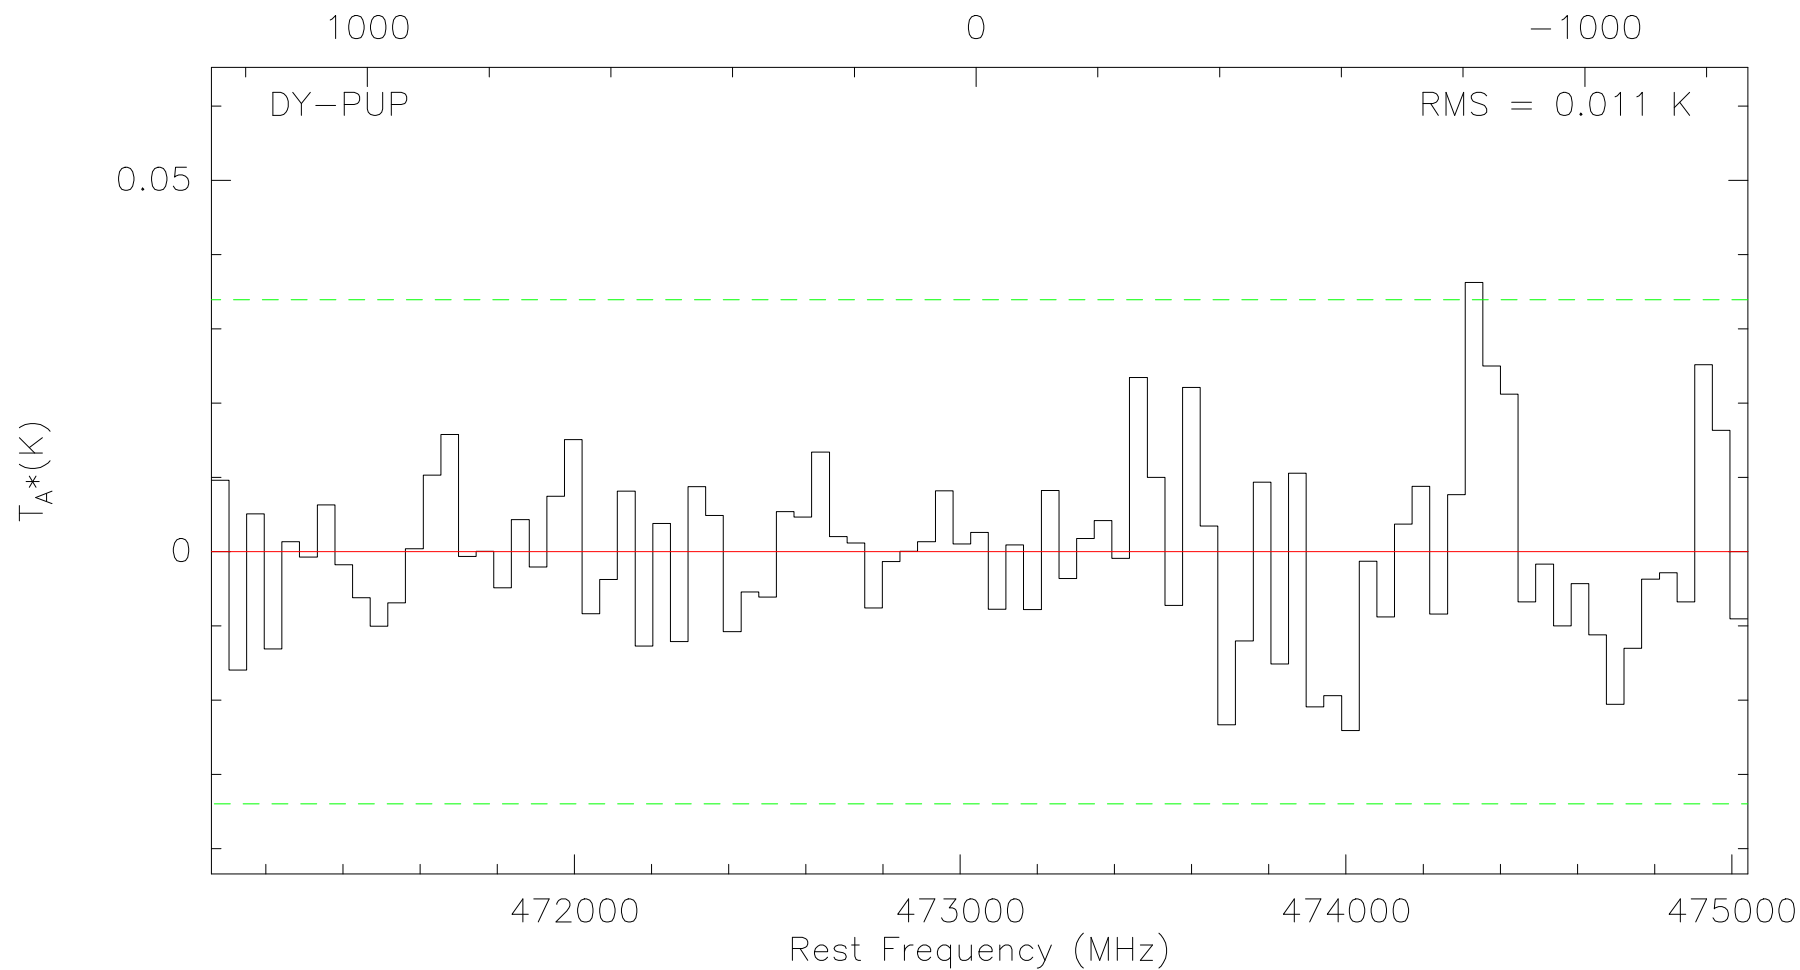

1;1 GU-MUS CO(4-3) OSB AP-FL02-XF0- O:24-AUG-2014 R:12-AUG-2020  
RA: 11:26:26.60 DEC: -68:40:32.3 Eq 2000.0 Rad. 0.0° Offs: -0.2 -0.4  
Unknown tau: 1.572 Tsys: 3778. Time: 23.3min El: 37.6  
N: 87 l0: 44.1919 V0: 0.000 Dv: 29.01 LSR  
FO: 473041.720 Df: -45.78 Fi: 461040.768

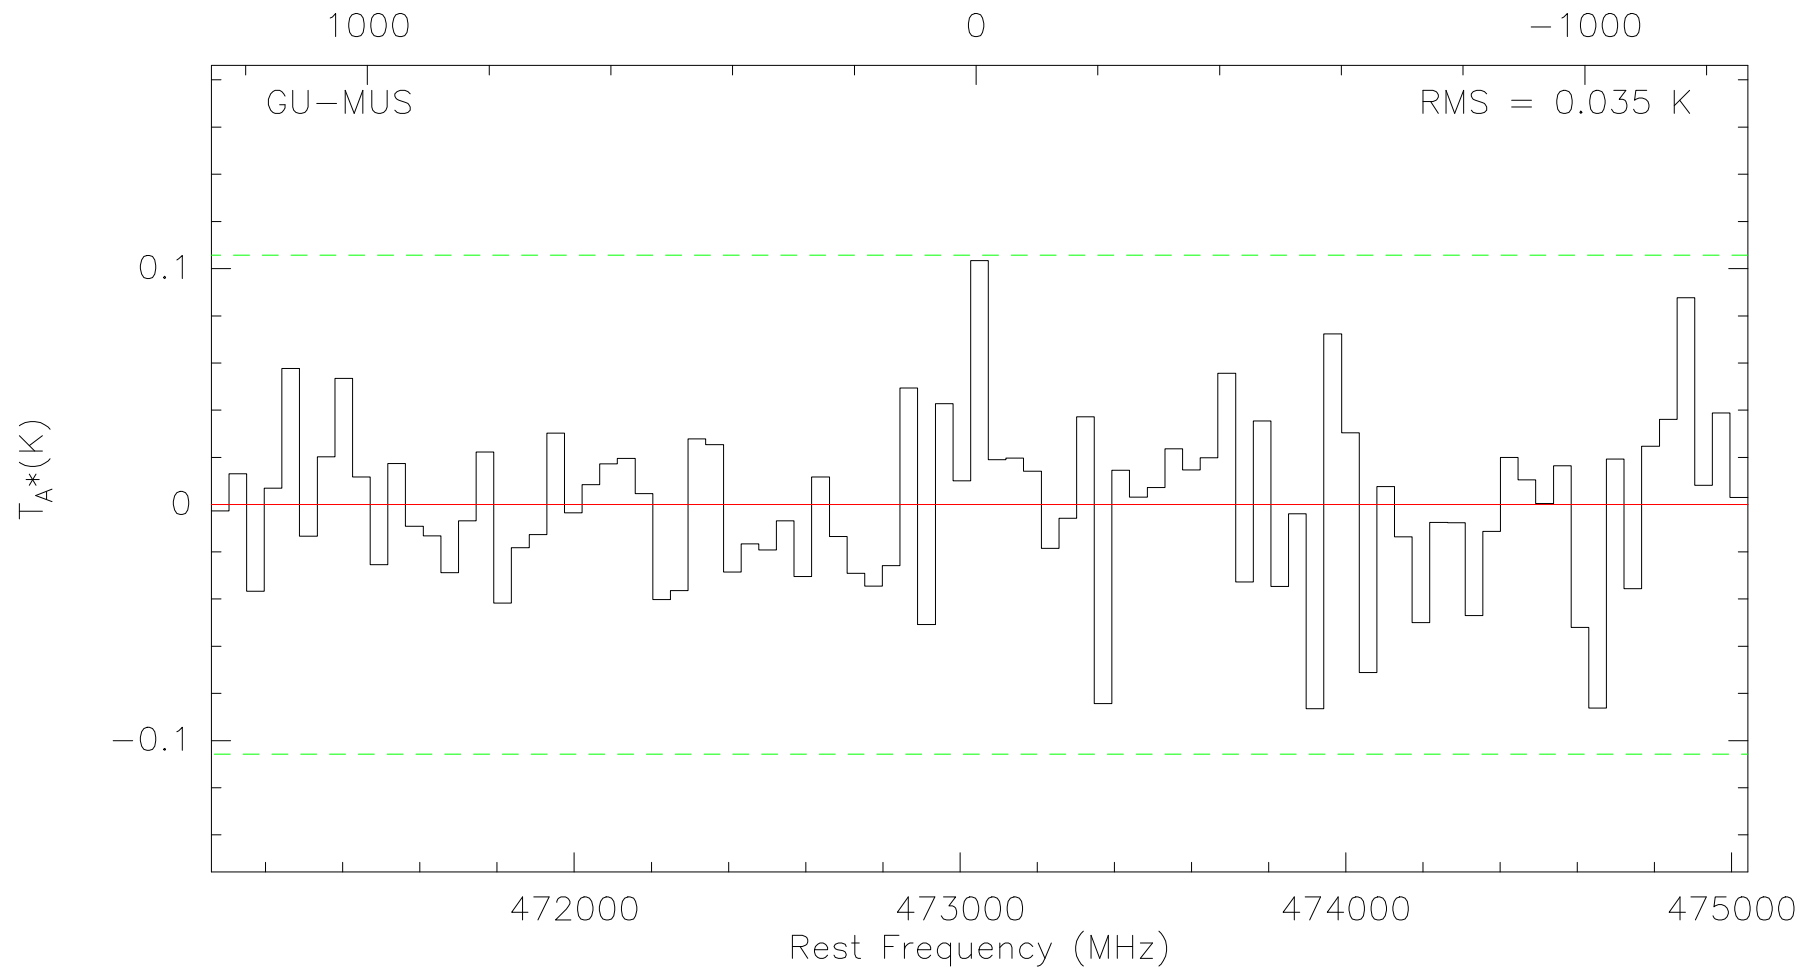

1;1 LZ-MUS CO(4-3) OSB AP-FL02-XF0- O:24-AUG-2014 R:12-AUG-2020  
RA: 11:56:09.27 DEC: -65:34:20.1 Eq 2000.0 Rad. 0.0° Offs: -0.2 -0.4  
Unknown tau: 1.756 Tsys: 5005. Time: 23.4min El: 36.6  
N: 87 l0: 44.1919 V0: 0.000 Dv: 29.01 LSR  
F0: 473041.746 Df: -45.78 Fi: 461040.768

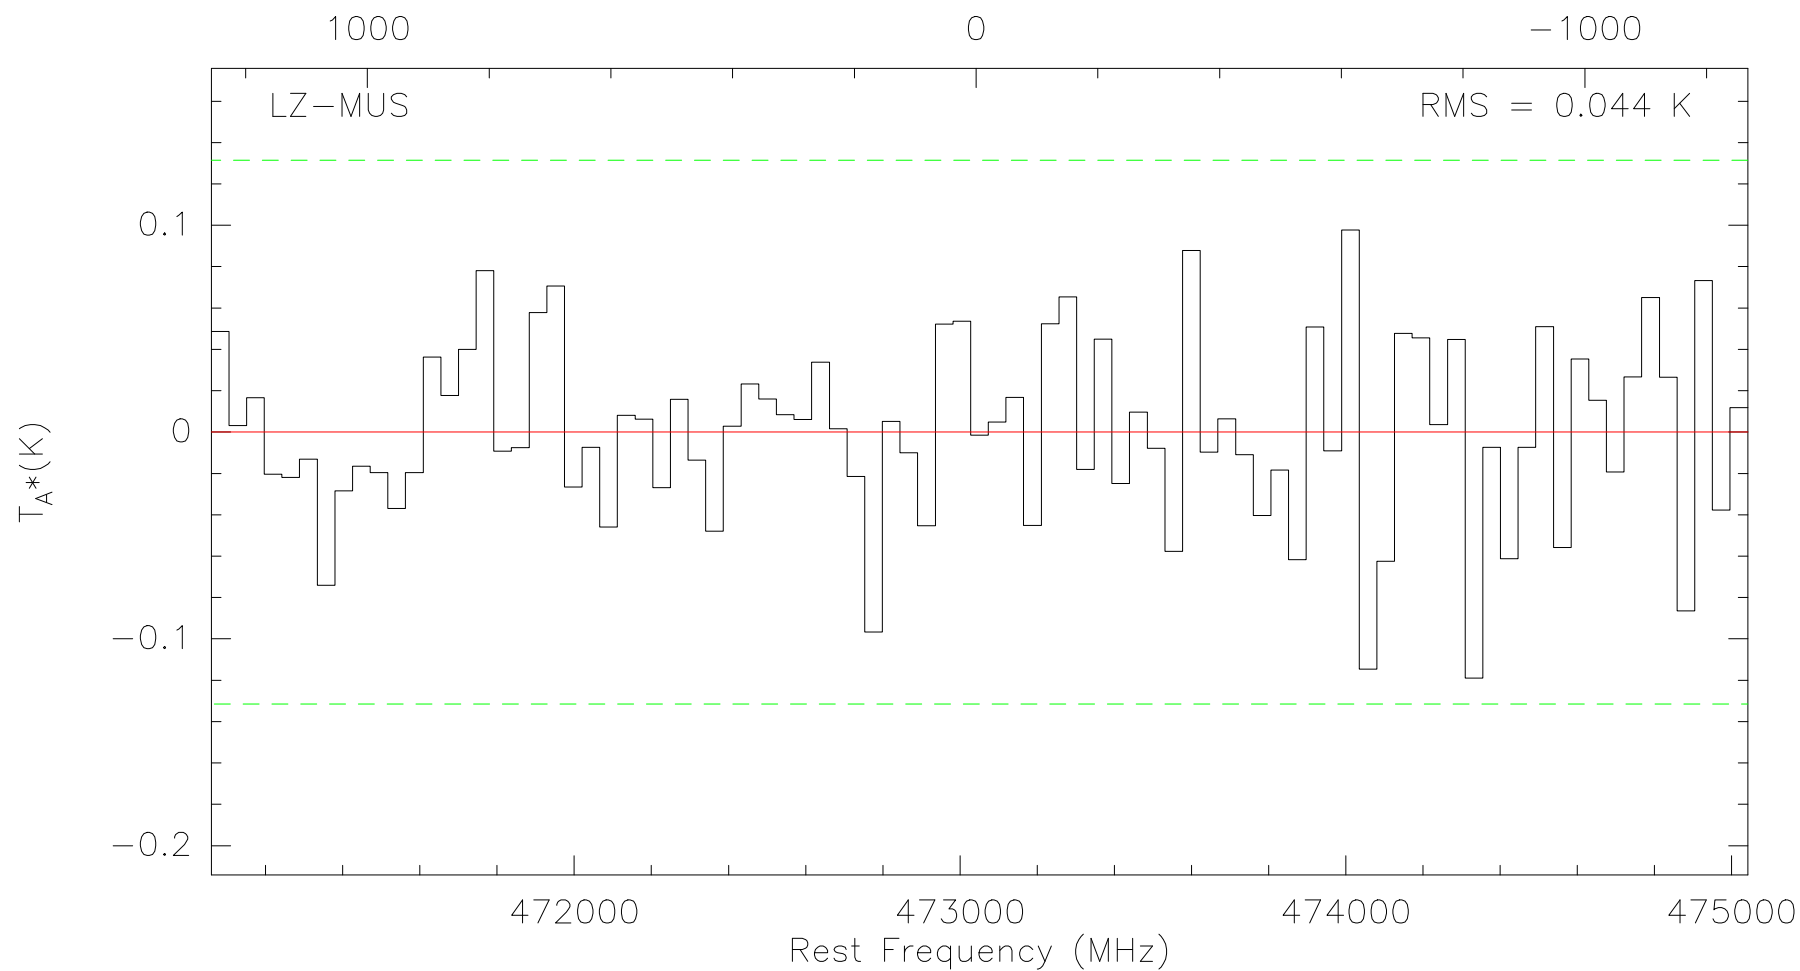

1;1 RR-PIC CO(4-3) OSB AP-FL02-XF0- 0:25-AUG-2014 R:12-AUG-2020  
RA: 06:35:36.06 DEC: -62:38:24.3 Eq 2000.0 Rad. 0.0° Offs: +0.3 -0.2  
Unknown tau: 1.321 Tsys: 1734. Time: 23.3min El: 42.4  
N: 87 l0: 44.1919 V0: 0.000 Dv: 29.01 LSR  
F0: 473041.406 Df: -45.78 Fi: 461040.768

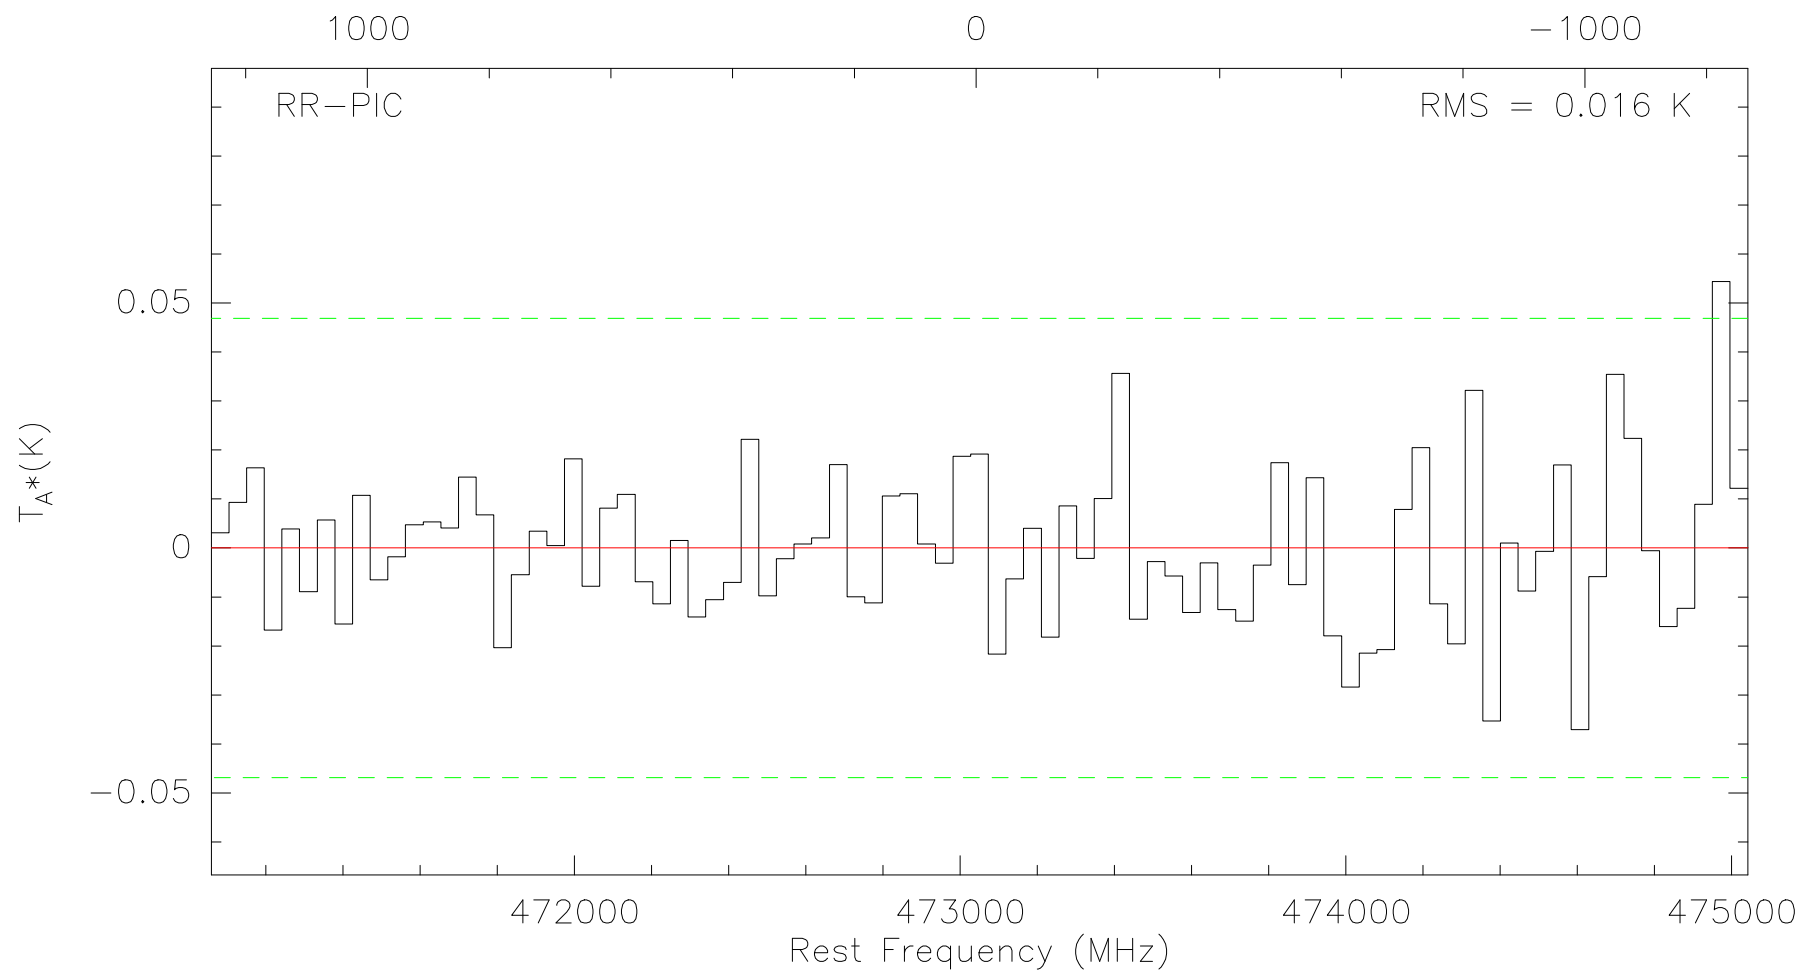

1;1 T-PYX CO(4-3) OSB AP-FL02-XF0- O:24-AUG-2014 R:12-AUG-2020  
RA: 09:04:41.50 DEC: -32:22:47.5 Eq 2000.0 Rad. 0.0° Offs: -0.2 -0.5  
Unknown tau: 1.591 Tsys: 1437. Time: 23.4min El: 66.0  
N: 87 l0: 44.1919 V0: 0.000 Dv: 29.01 LSR  
FO: 473041.401 Df: -45.78 Fi: 461040.768

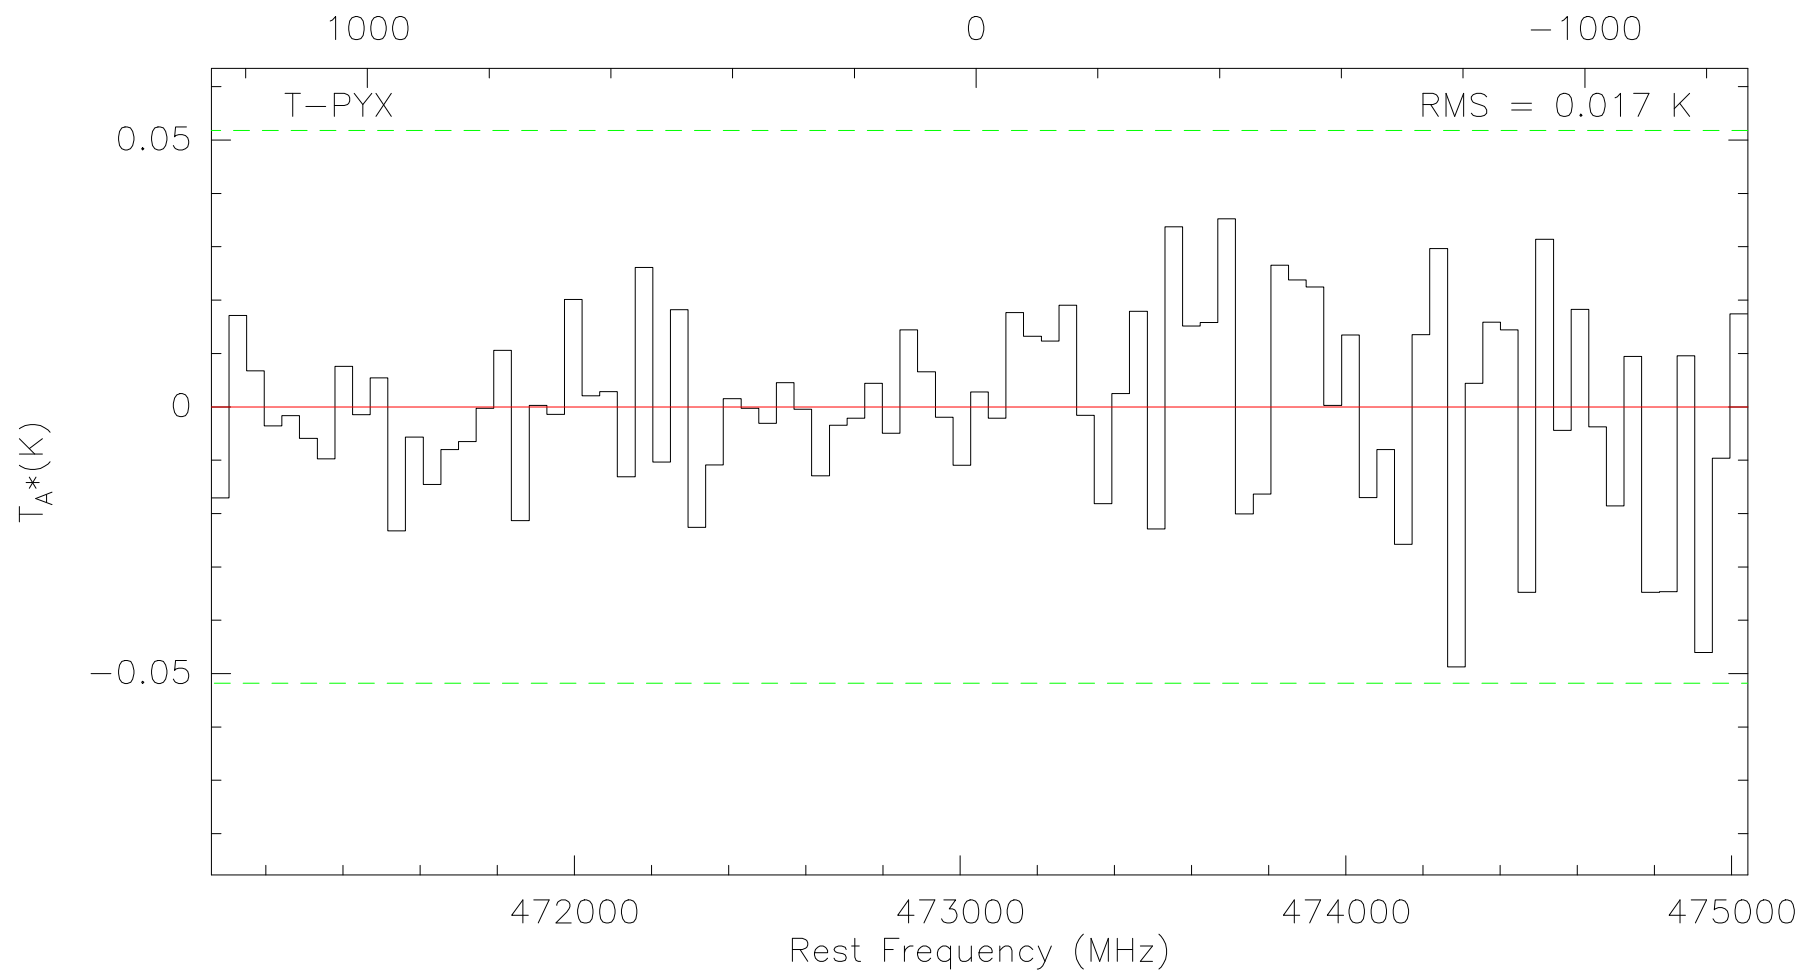

1;1 TV-CRV CO(4-3) OSB AP-FL02-XF0- O:24-AUG-2014 R:12-AUG-2020  
RA: 12:20:24.15 DEC: -18:27:02.0 Eq 2000.0 Rad. 0.0° Offs: +0.2 -0.3  
Unknown tau: 1.377 Tsys: 1585. Time: 23.3min El: 51.8  
N: 87 l0: 44.1919 V0: 0.000 Dv: 29.01 LSR  
F0: 473041.572 Df: -45.78 Fi: 461040.768

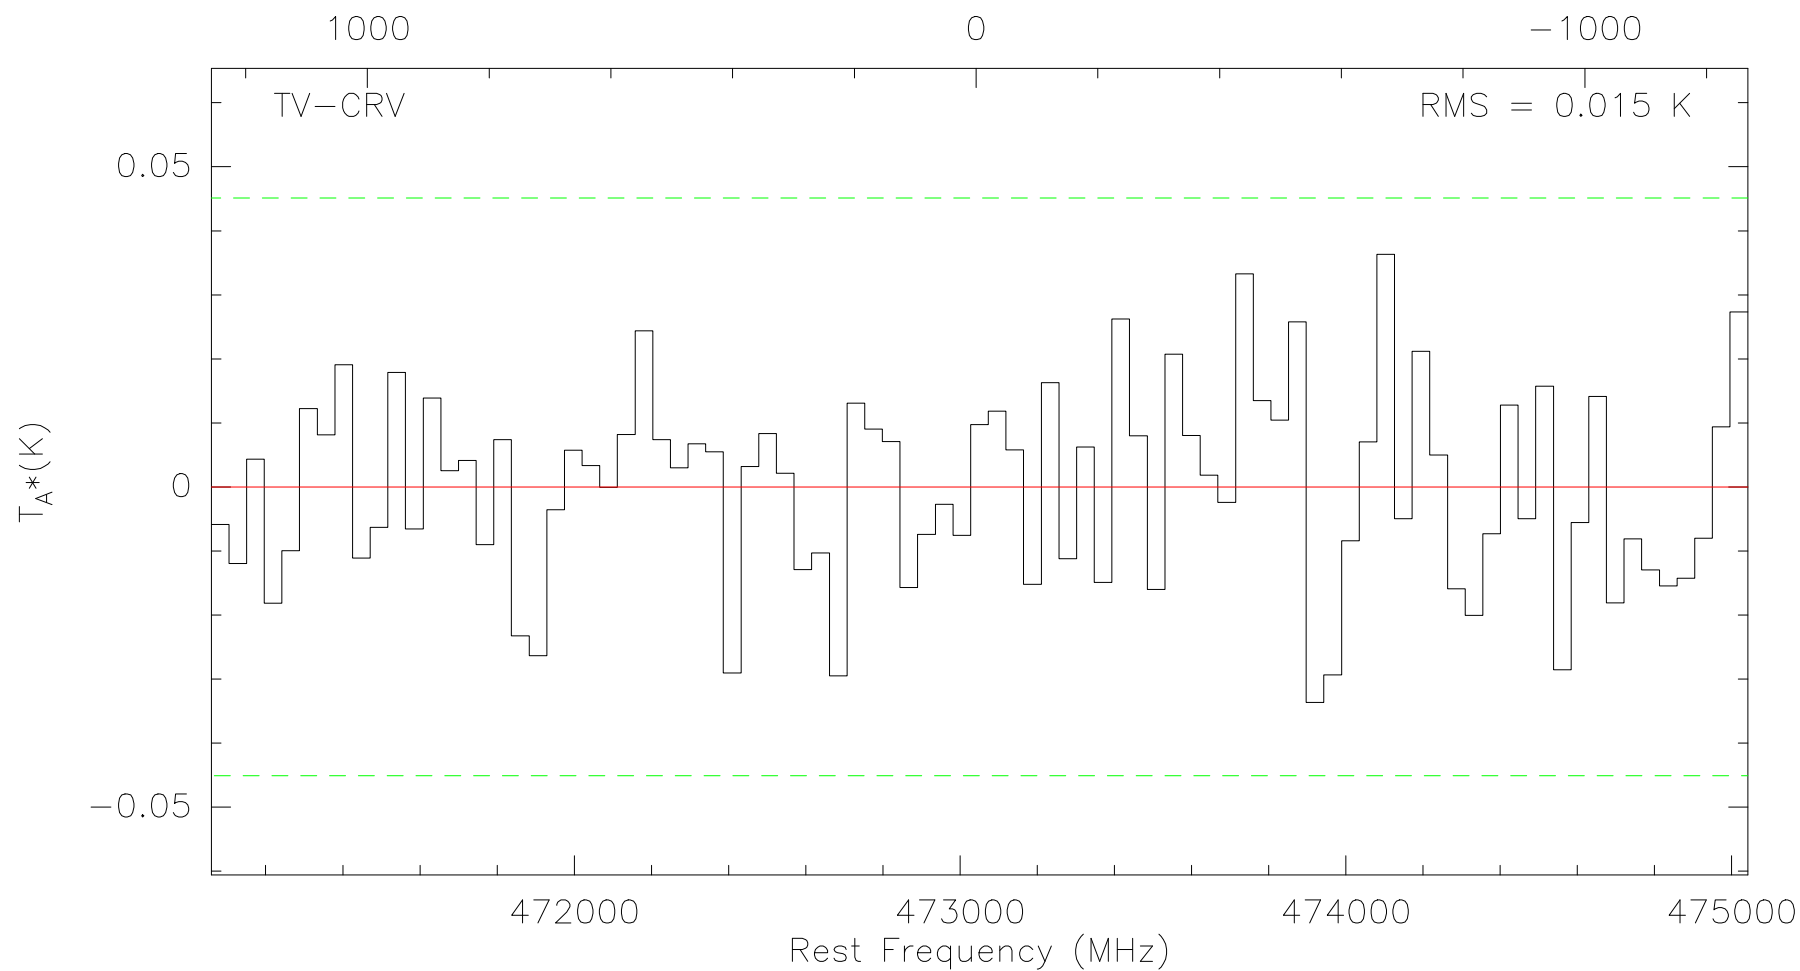

1;1 V1065-CEN CO(4-3) OSB AP-FL02-XF0- O:24-AUG-2014 R:12-AUG-2020  
RA: 11:43:10.33 DEC: -58:04:04.3 Eq 2000.0 Rad. 0.0° Offs: -0.4 -0.3  
Unknown tau: 1.628 Tsys: 6869. Time: 23.3min El: 30.0  
N: 87 l0: 44.1918 V0: 0.000 Dv: 29.01 LSR  
F0: 473041.755 Df: -45.78 Fi: 461040.768

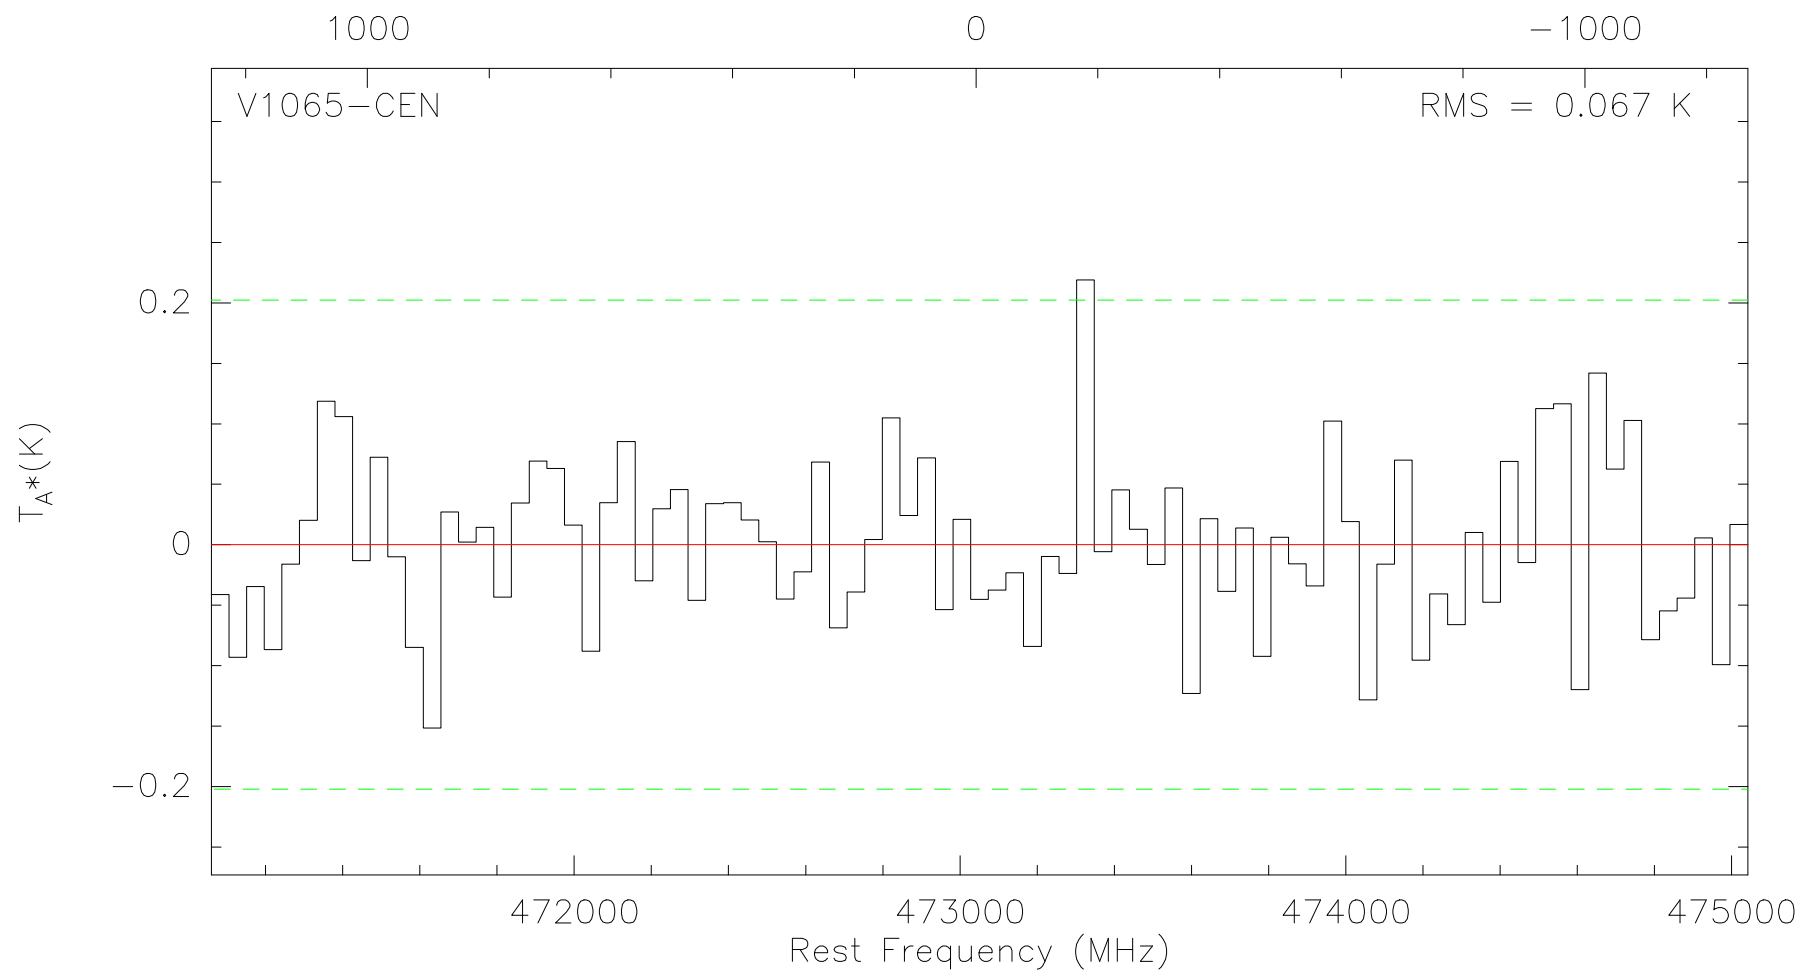

1;1 V351-CAR CO(4-3) OSB AP-FL02-XF0- 0:28-AUG-2014 R:12-AUG-2020

RA: 10:45:19.14 DEC: -72:03:56.0 Eq 2000.0 Rad. 0.0° Offs: +0.2 -0.4

Unknown tau: 1.743 Tsys: 4017. Time: 23.4min El: 40.8

N: 87 l0: 44.1919 V0: 0.000 Dv: 29.01 LSR

F0: 473041.671 Df: -45.78 Fi: 461040.768

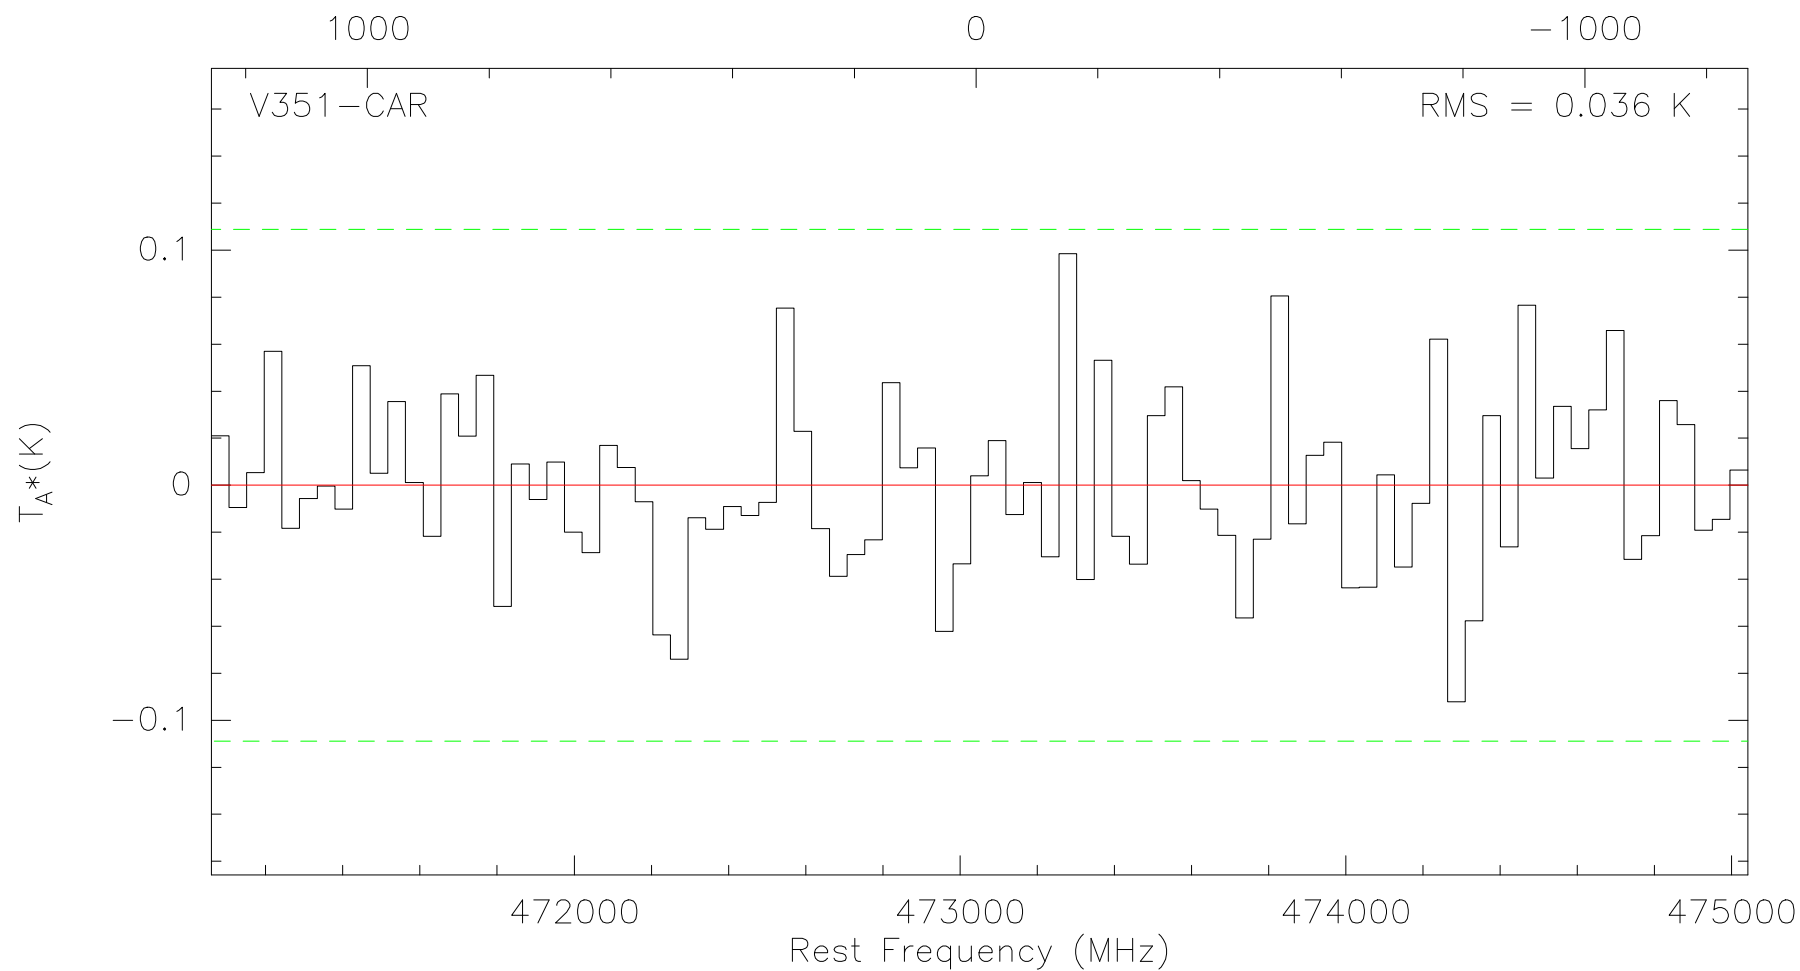

1;1 V359-CEN CO(4-3) OSB AP-FL02-XF0- 0:24-AUG-2014 R:12-AUG-2020  
RA: 11:58:15.33 DEC: -41:46:08.4 Eq 2000.0 Rad. 0.0° Offs: +0.2 -0.4  
Unknown tau: 1.528 Tsys: 1433. Time: 23.4min El: 70.8  
N: 87 l0: 44.1919 V0: 0.000 Dv: 29.01 LSR  
FO: 473041.729 Df: -45.78 Fi: 461040.768

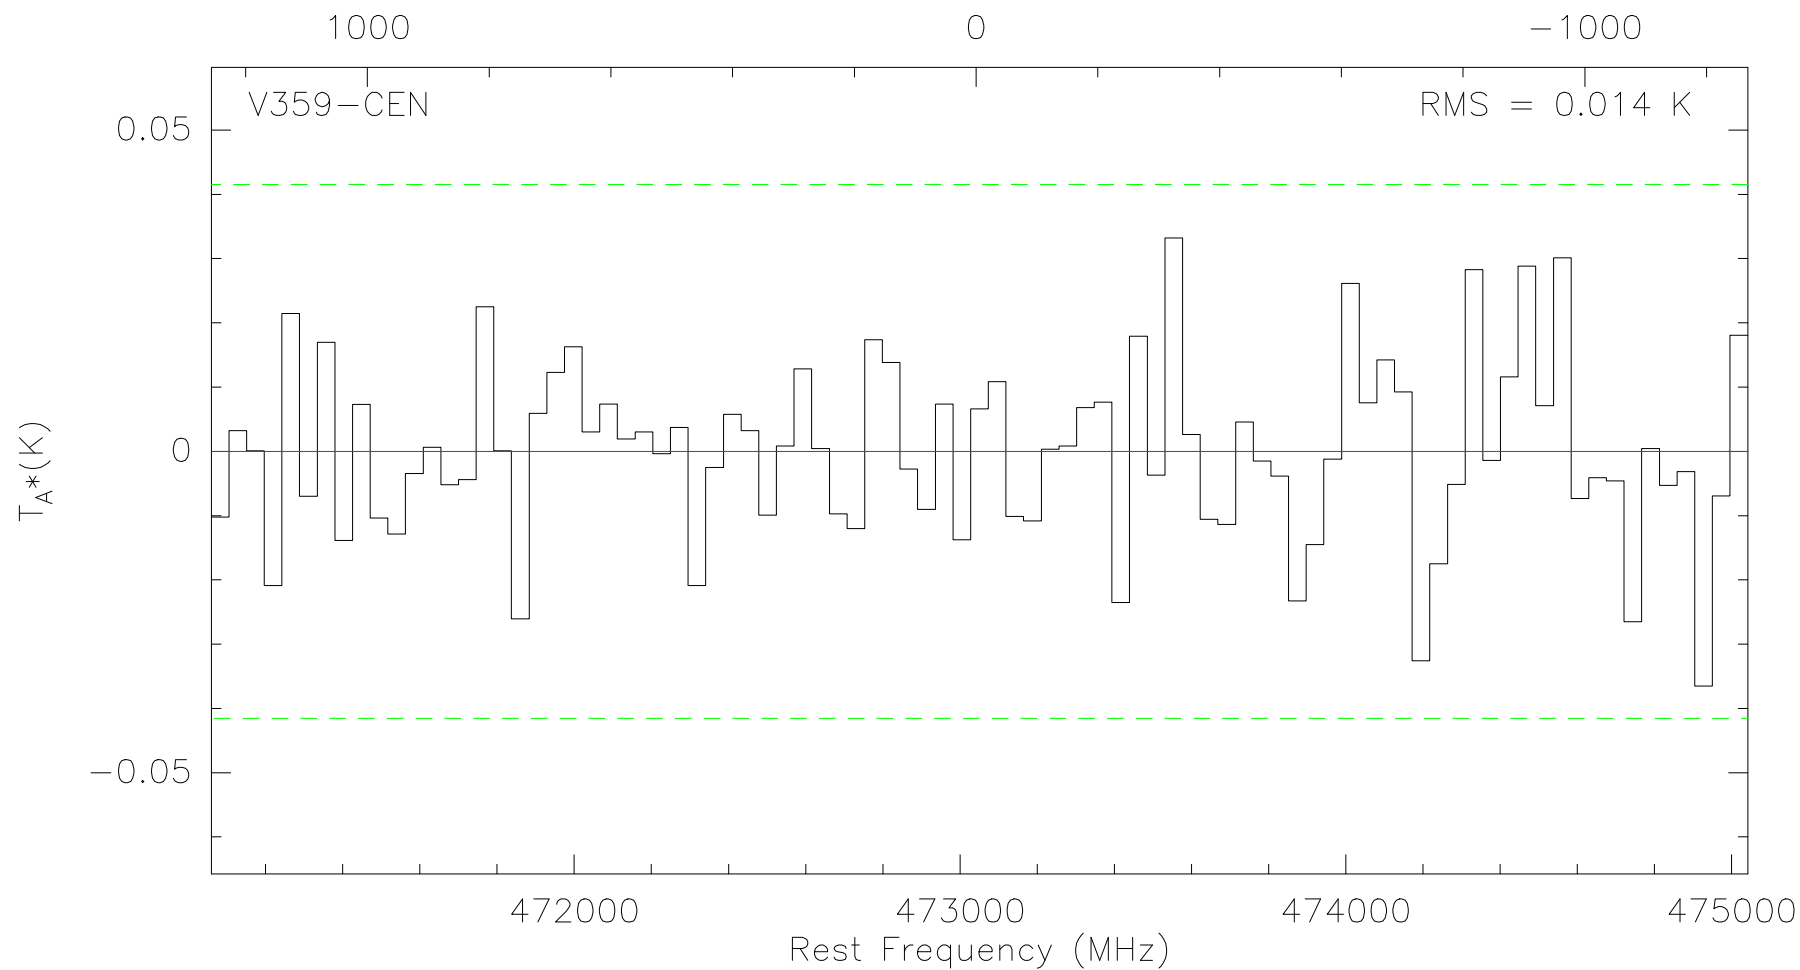

1;1 V382-VEL CO(4-3) OSB AP-FL02-XF0- 0:28-AUG-2014 R:12-AUG-2020

RA: 10:44:48.39 DEC: -52:25:30.7 Eq 2000.0 Rad. 0.0° Offs: +0.3 -0.4

Unknown tau: 1.877 Tsys: 2664. Time: 23.4min El: 58.5

N: 87 l0: 44.1919 V0: 0.000 Dv: 29.01 LSR

F0: 473041.649 Df: -45.78 Fi: 461040.768

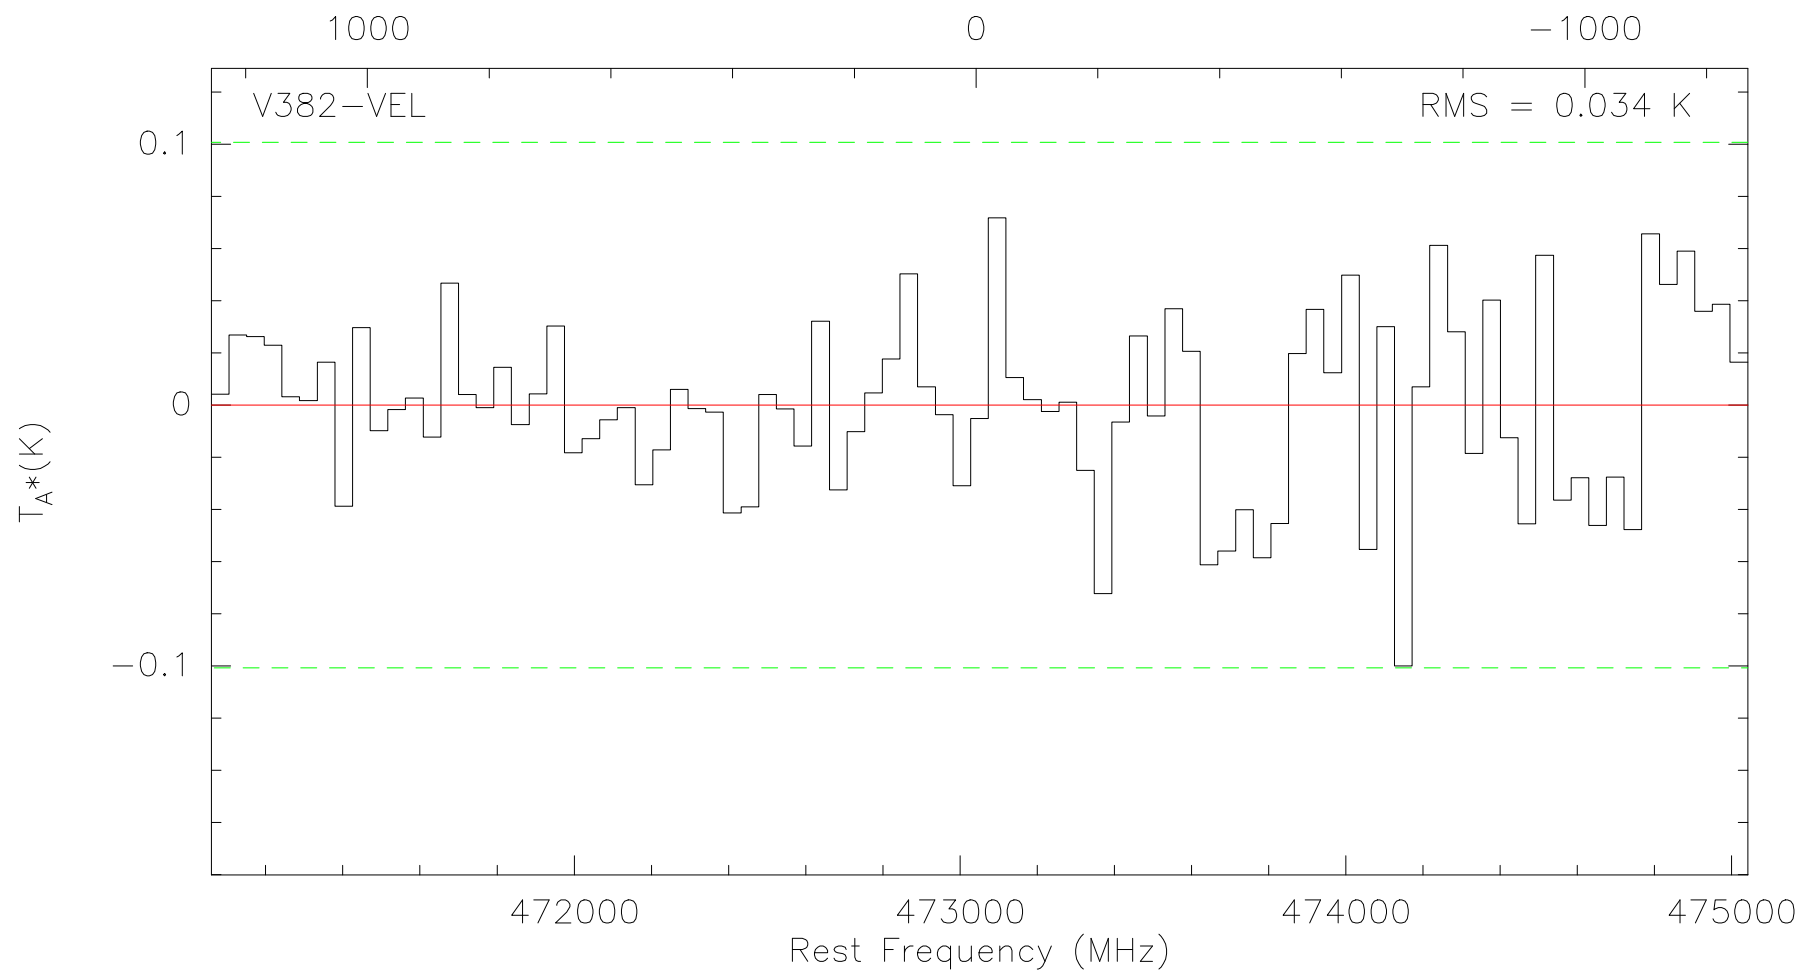

1;1 V598-PUP CO(4-3) OSB AP-FL02-XF0- 0:25-AUG-2014 R:12-AUG-2020  
RA: 07:05:42.50 DEC: -38:14:39.4 Eq 2000.0 Rad. 0.0° Offs: +0.2 -0.3  
Unknown tau: 1.351 Tsys: 1195. Time: 23.4min El: 59.6  
N: 87 l0: 44.1919 V0: 0.000 Dv: 29.01 LSR  
F0: 473041.186 Df: -45.78 Fi: 461040.768

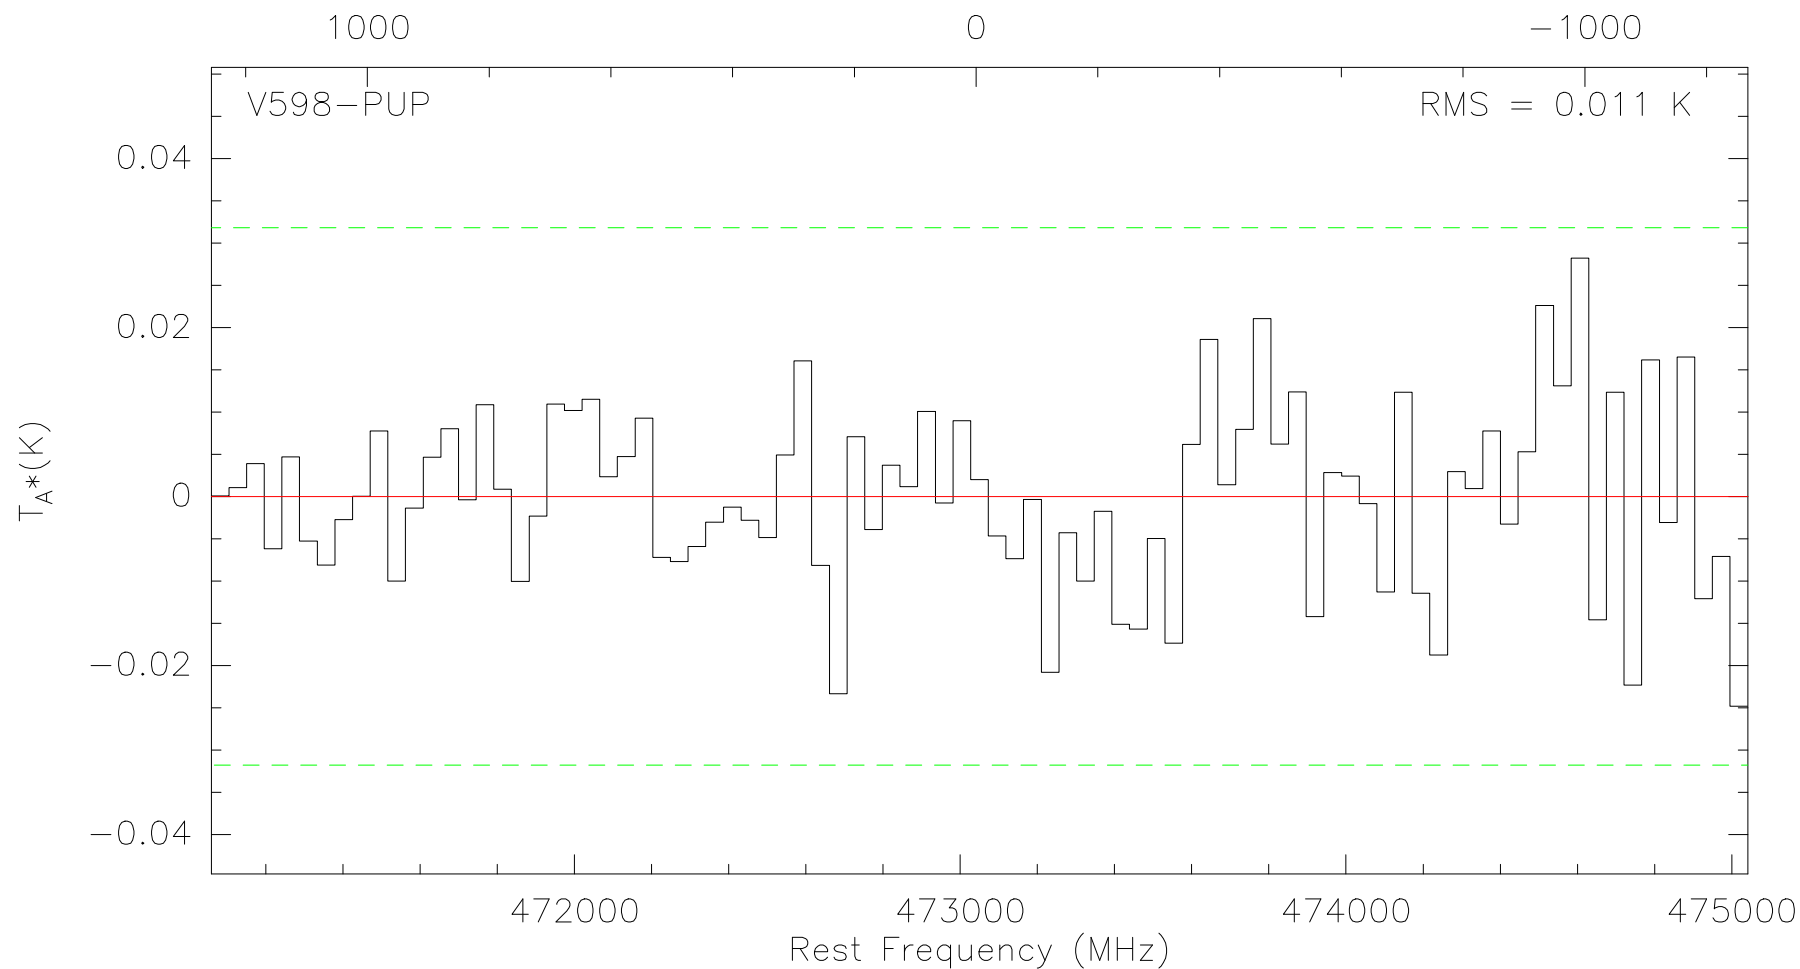

1;1 VX-FOR CO(4-3) OSB AP-FL02-XF0- O:24-AUG-2014 R:12-AUG-2020  
RA: 03:26:45.71 DEC: -34:26:25.2 Eq 2000.0 Rad. 0.0° Offs: +0.2 -0.2  
Unknown tau: 1.965 Tsys: 2805. Time: 23.3min El: 53.4  
N: 87 l0: 44.1919 V0: 0.000 Dv: 29.01 LSR  
F0: 473040.757 Df: -45.78 Fi: 461040.768

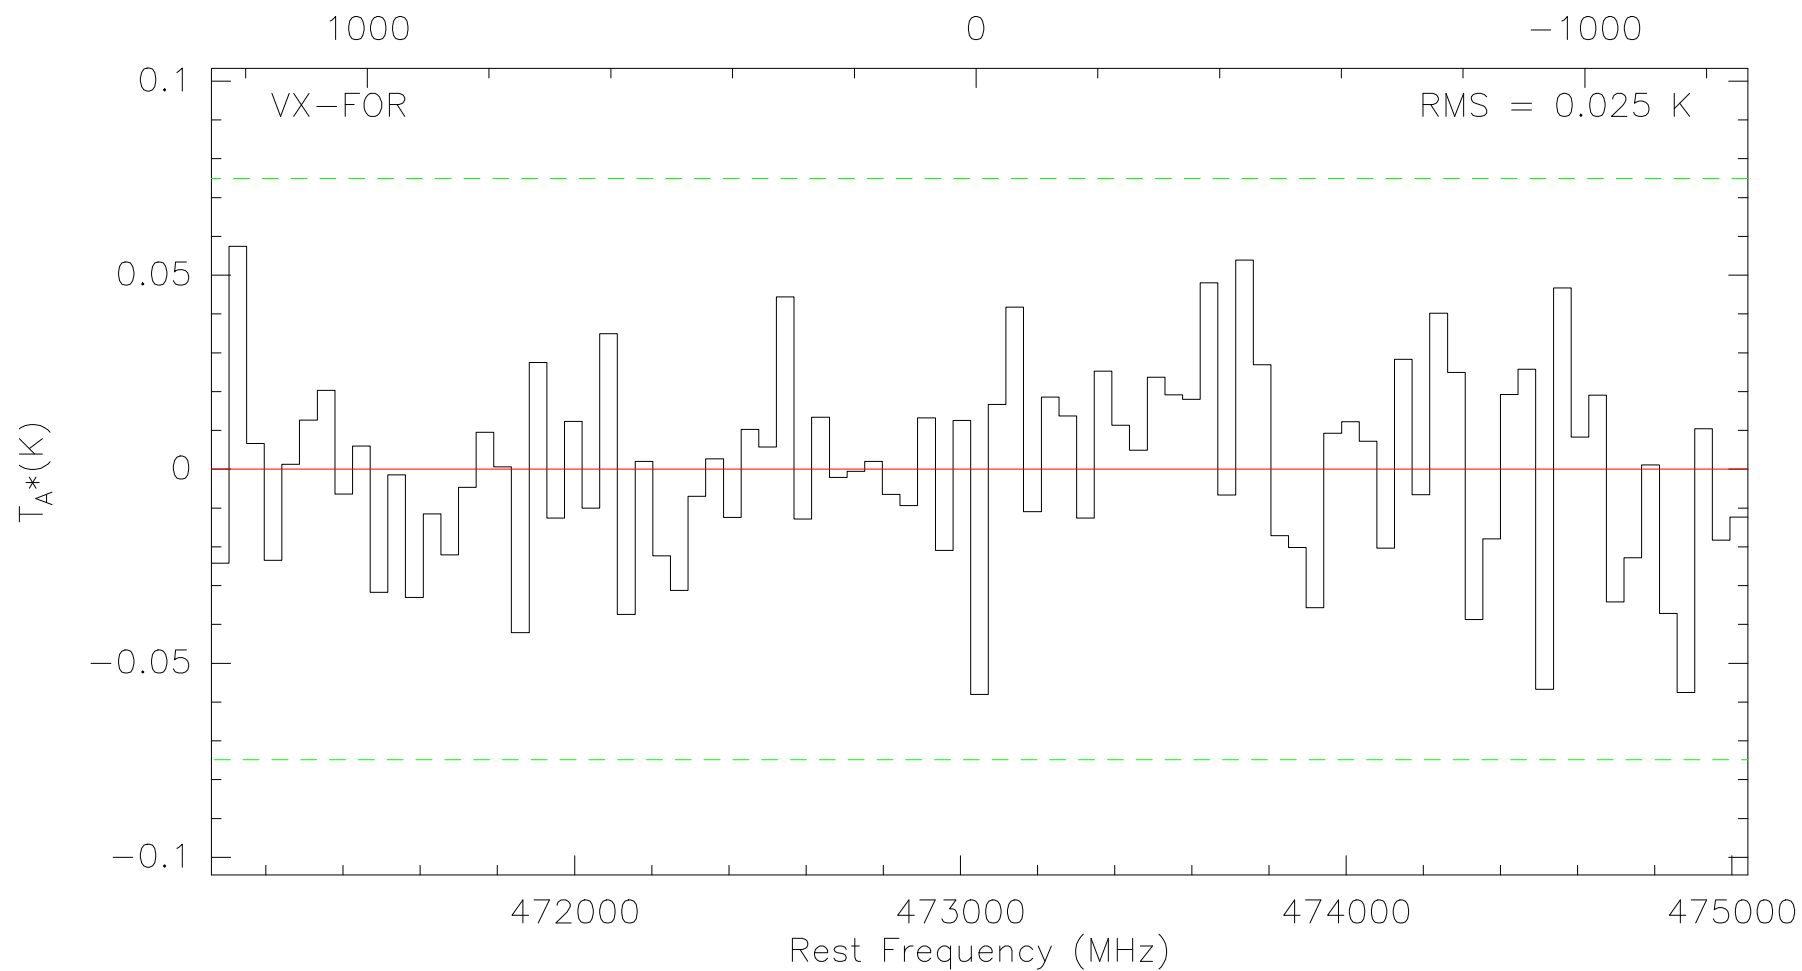

1;1 WX-CET CO(4-3) OSB AP-FL02-XF0- O:24-AUG-2014 R:12-AUG-2020  
RA: 01:17:04.17 DEC: -17:56:23.0 Eq 2000.0 Rad. 0.0° Offs: -0.2 -0.3  
Unknown tau: 1.622 Tsys: 1417. Time: 23.3min El: 67.5  
N: 87 l0: 44.1919 V0: 0.000 Dv: 29.01 LSR  
FO: 473040.428 Df: -45.78 Fi: 461040.768

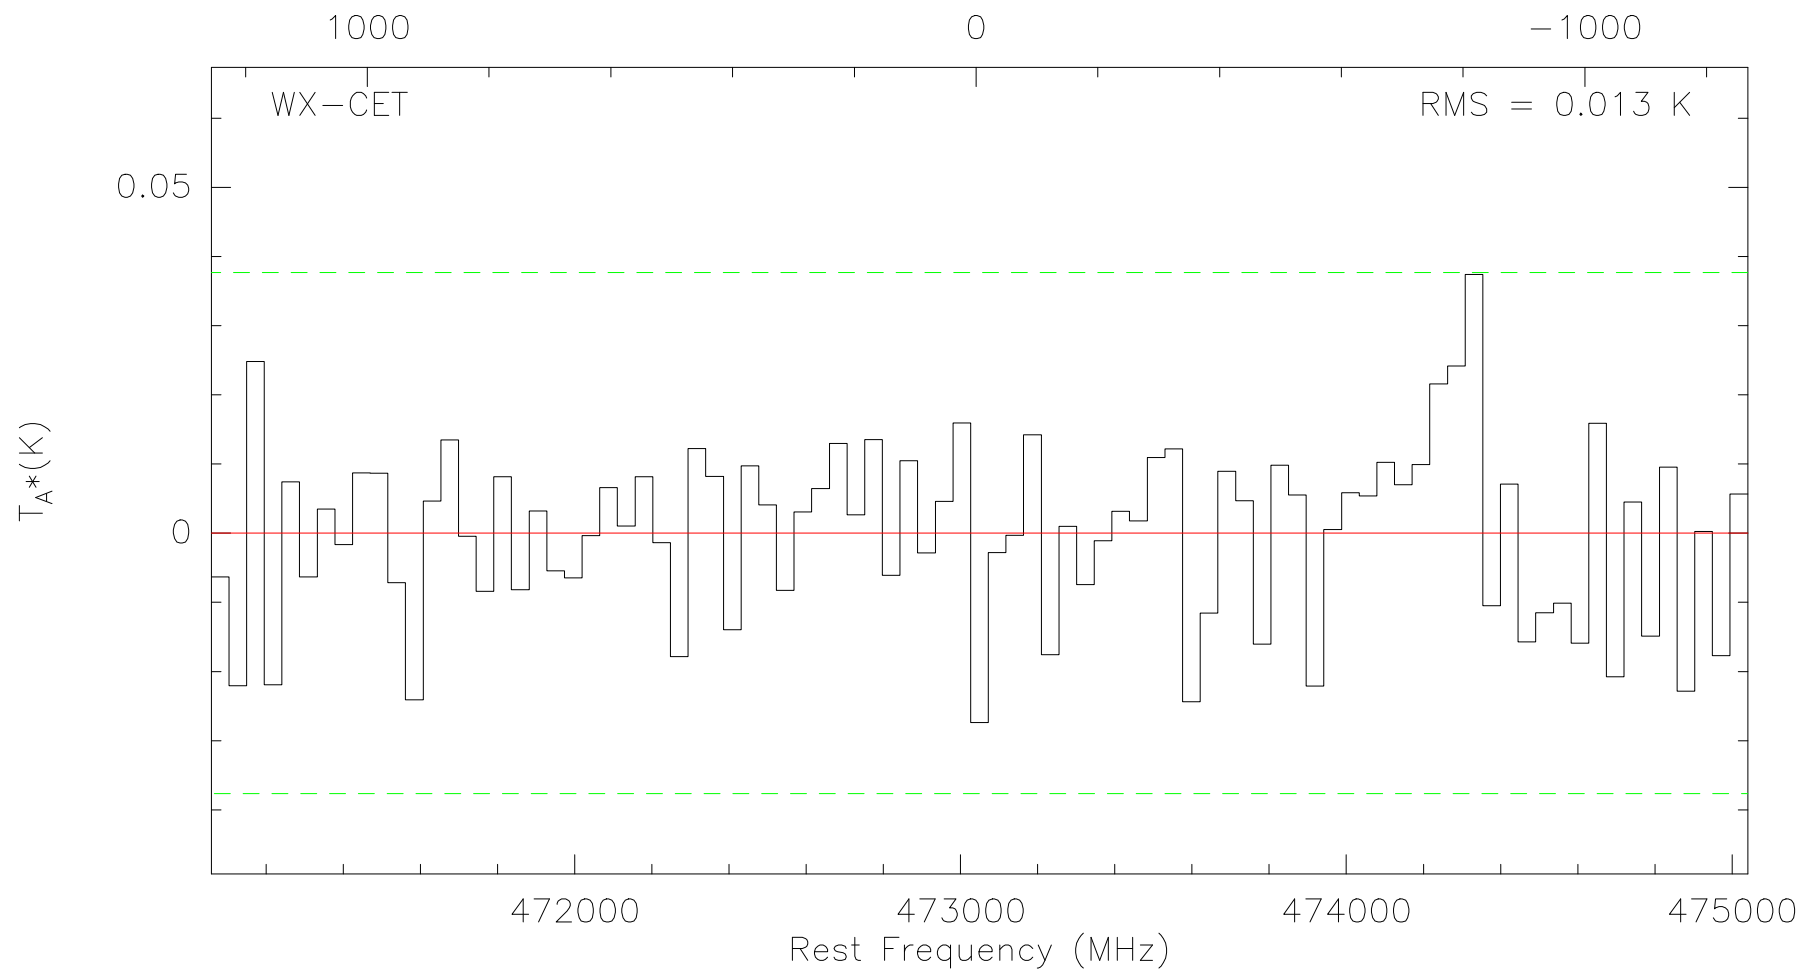

1;1 AICIR CO(4-3) OSB AP-FL02-XF0- 0:13-JUL-2016 R:07-AUG-2020  
RA: 14:49:31.29 DEC: -68:51:35.9 Eq 2000.0 Rad. 0.0° Offs: +0.5 -0.2  
Unknown tau: 1.701 Tsys: 4975. Time: 5.0min El: 33.7  
N: 87 l0: 44.1918 V0: 0.000 Dv: 29.01 LSR  
F0: 473041.520 Df: -45.78 Fi: 461040.768

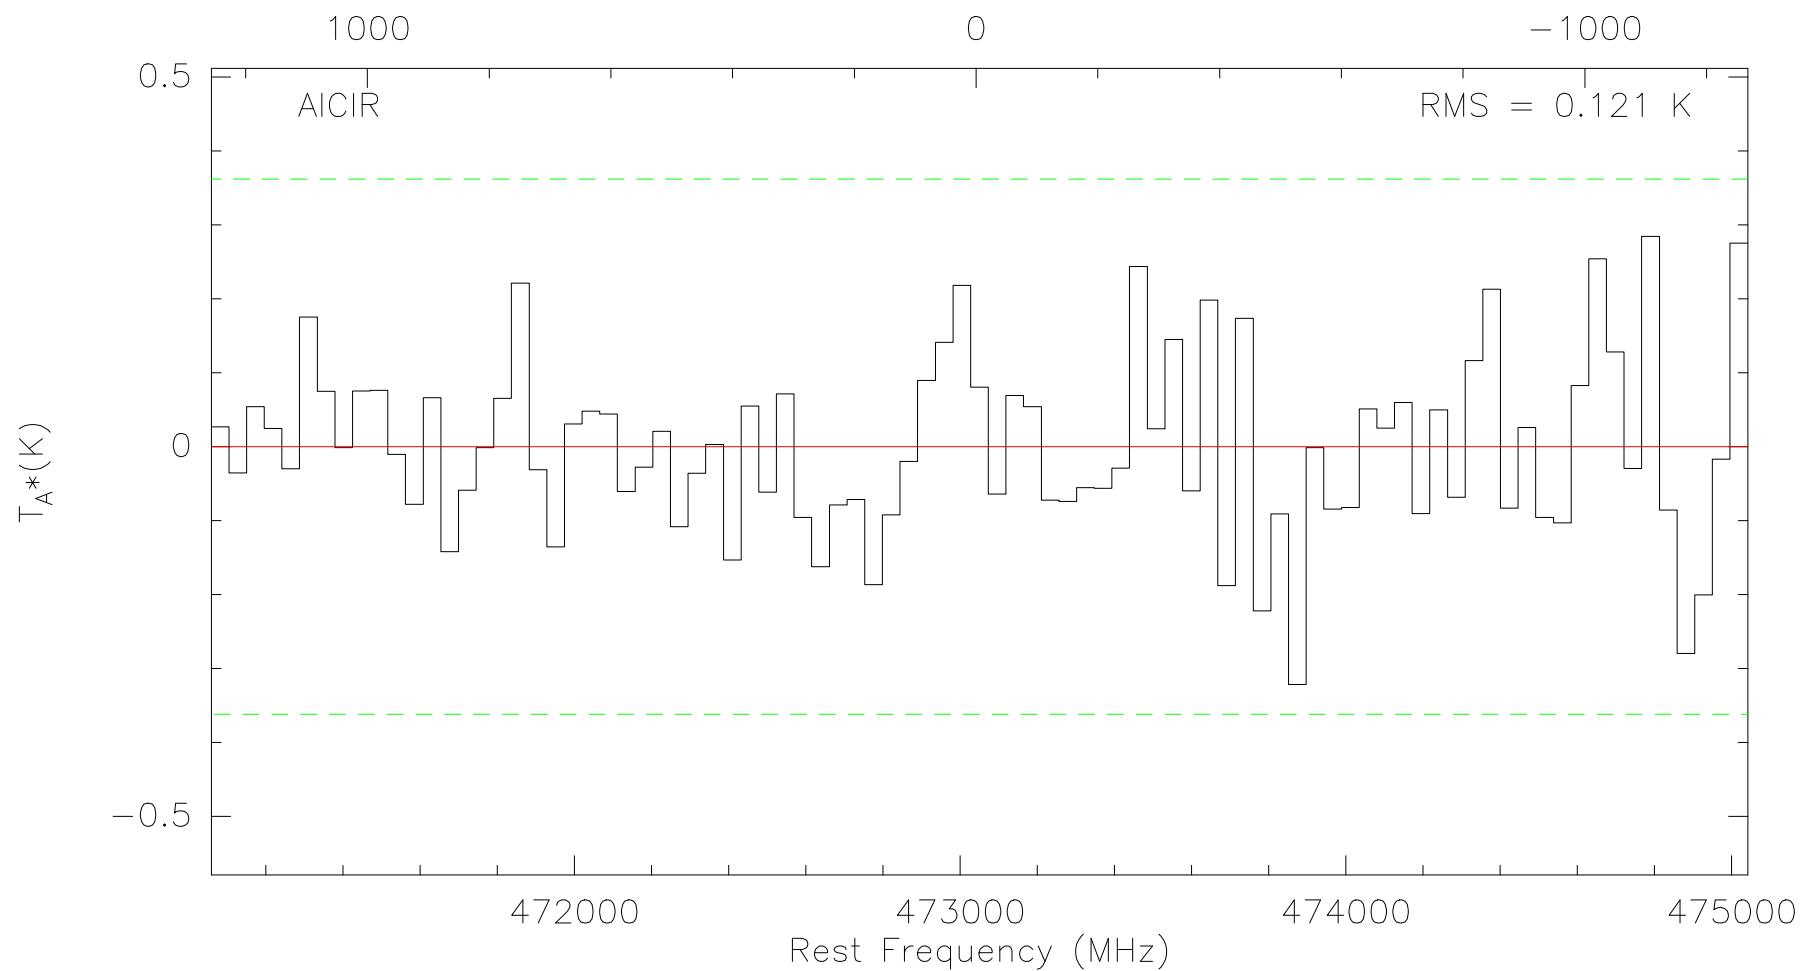

1;1 ATSGR CO(4-3) OSB AP-FL02-XF0- O:14-JUL-2016 R:07-AUG-2020  
RA: 18:03:30.87 DEC: -26:28:28.5 Eq 2000.0 Rad. 0.0° Offs: +0.1 -0.4  
Unknown tau: 2.168 Tsys: 2268. Time: 9.9min El: 66.9  
N: 87 l0: 44.1918 V0: 0.000 Dv: 29.01 LSR  
FO: 473040.742 Df: -45.78 Fi: 461040.768

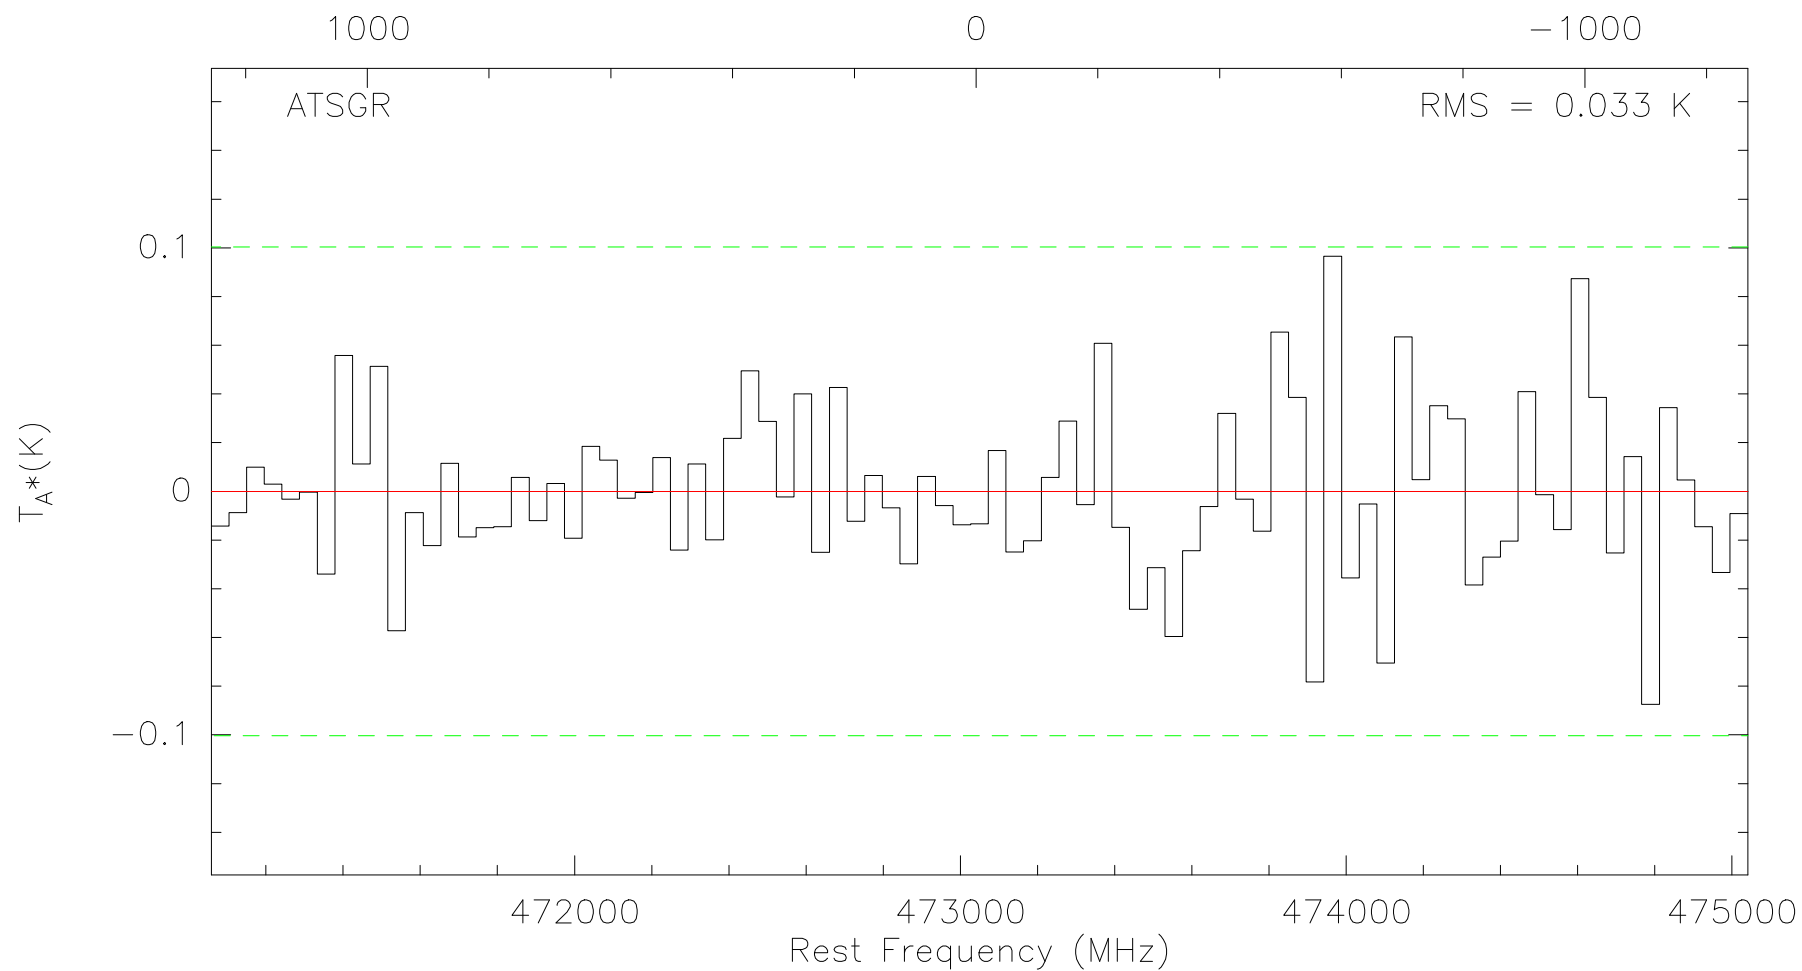

1;1 FMSGR CO(4-3) OSB AP-FL02-XF0- O:13-JUL-2016 R:07-AUG-2020  
RA: 18:17:18.10 DEC: -23:38:27.0 Eq 2000.0 Rad. 0.0° Offs: -0.1 -0.4  
Unknown tau: 1.353 Tsys: 1969. Time: 9.9min El: 35.9  
N: 87 l0: 44.1918 V0: 0.000 Dv: 29.01 LSR  
FO: 473040.657 Df: -45.78 Fi: 461040.768

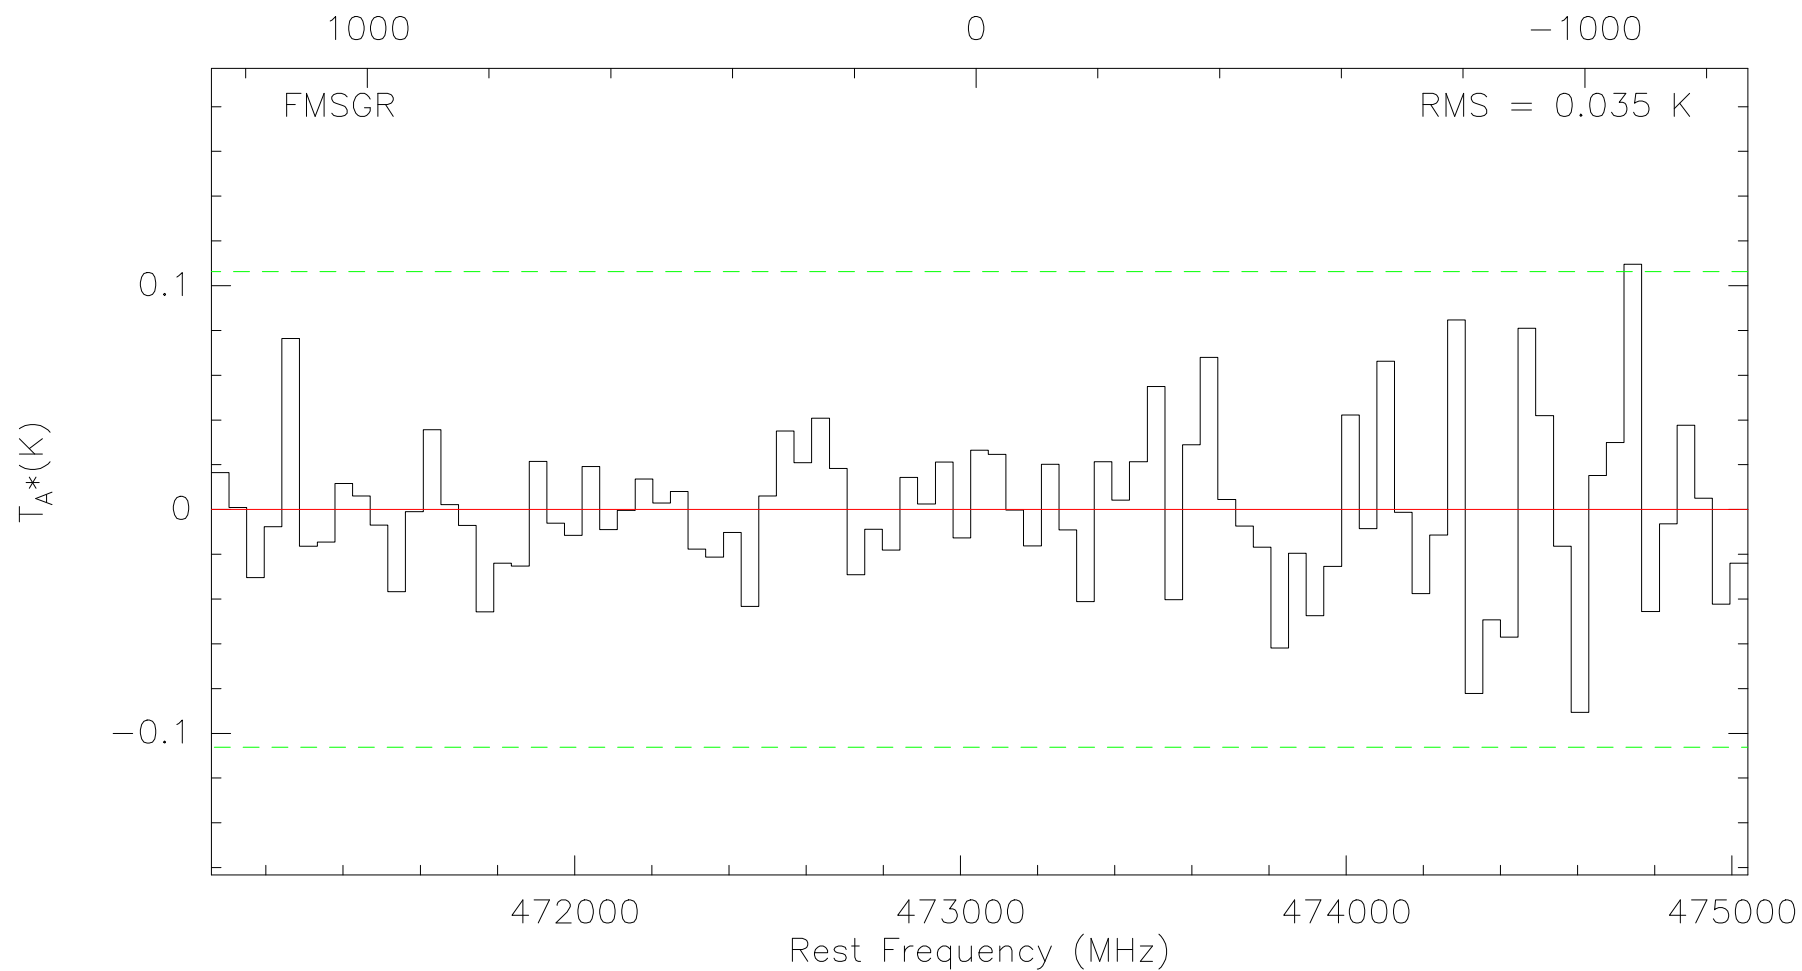

1;1 GRSGR CO(4-3) OSB AP-FL02-XF0- 0:13-JUL-2016 R:07-AUG-2020  
RA: 18:22:58.50 DEC: -25:34:47.3 Eq 2000.0 Rad. 0.0° Offs: -0.1 -0.5  
Unknown tau: 1.509 Tsys: 1246. Time: 9.9min El: 58.2  
N: 87 l0: 44.1918 V0: 0.000 Dv: 29.01 LSR  
F0: 473040.649 Df: -45.78 Fi: 461040.768

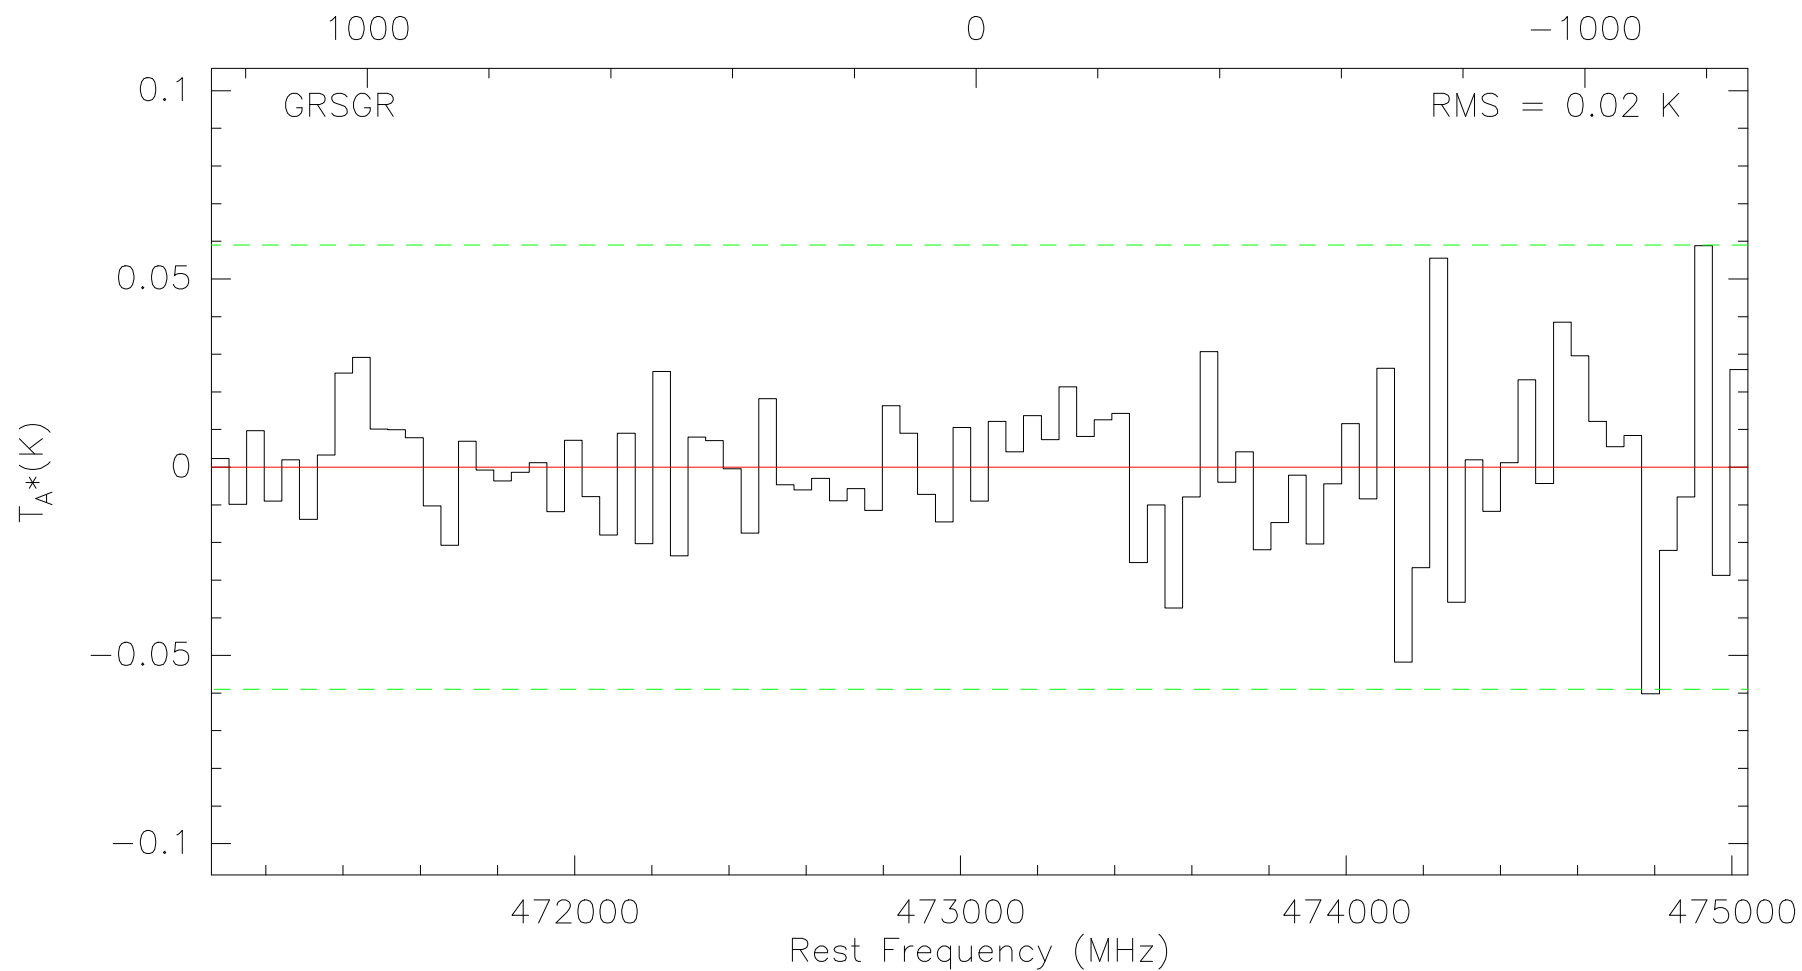

1;1 HSSGR CO(4-3) OSB AP-FL02-XF0- O:13-JUL-2016 R:07-AUG-2020  
RA: 18:28:03.44 DEC: -21:34:24.7 Eq 2000.0 Rad. 0.0° Offs: -0.3 -0.3  
Unknown tau: 1.226 Tsys: 2644. Time: 9.9min El: 27.0  
N: 87 l0: 44.1918 V0: 0.000 Dv: 29.01 LSR  
FO: 473040.588 Df: -45.78 Fi: 461040.768

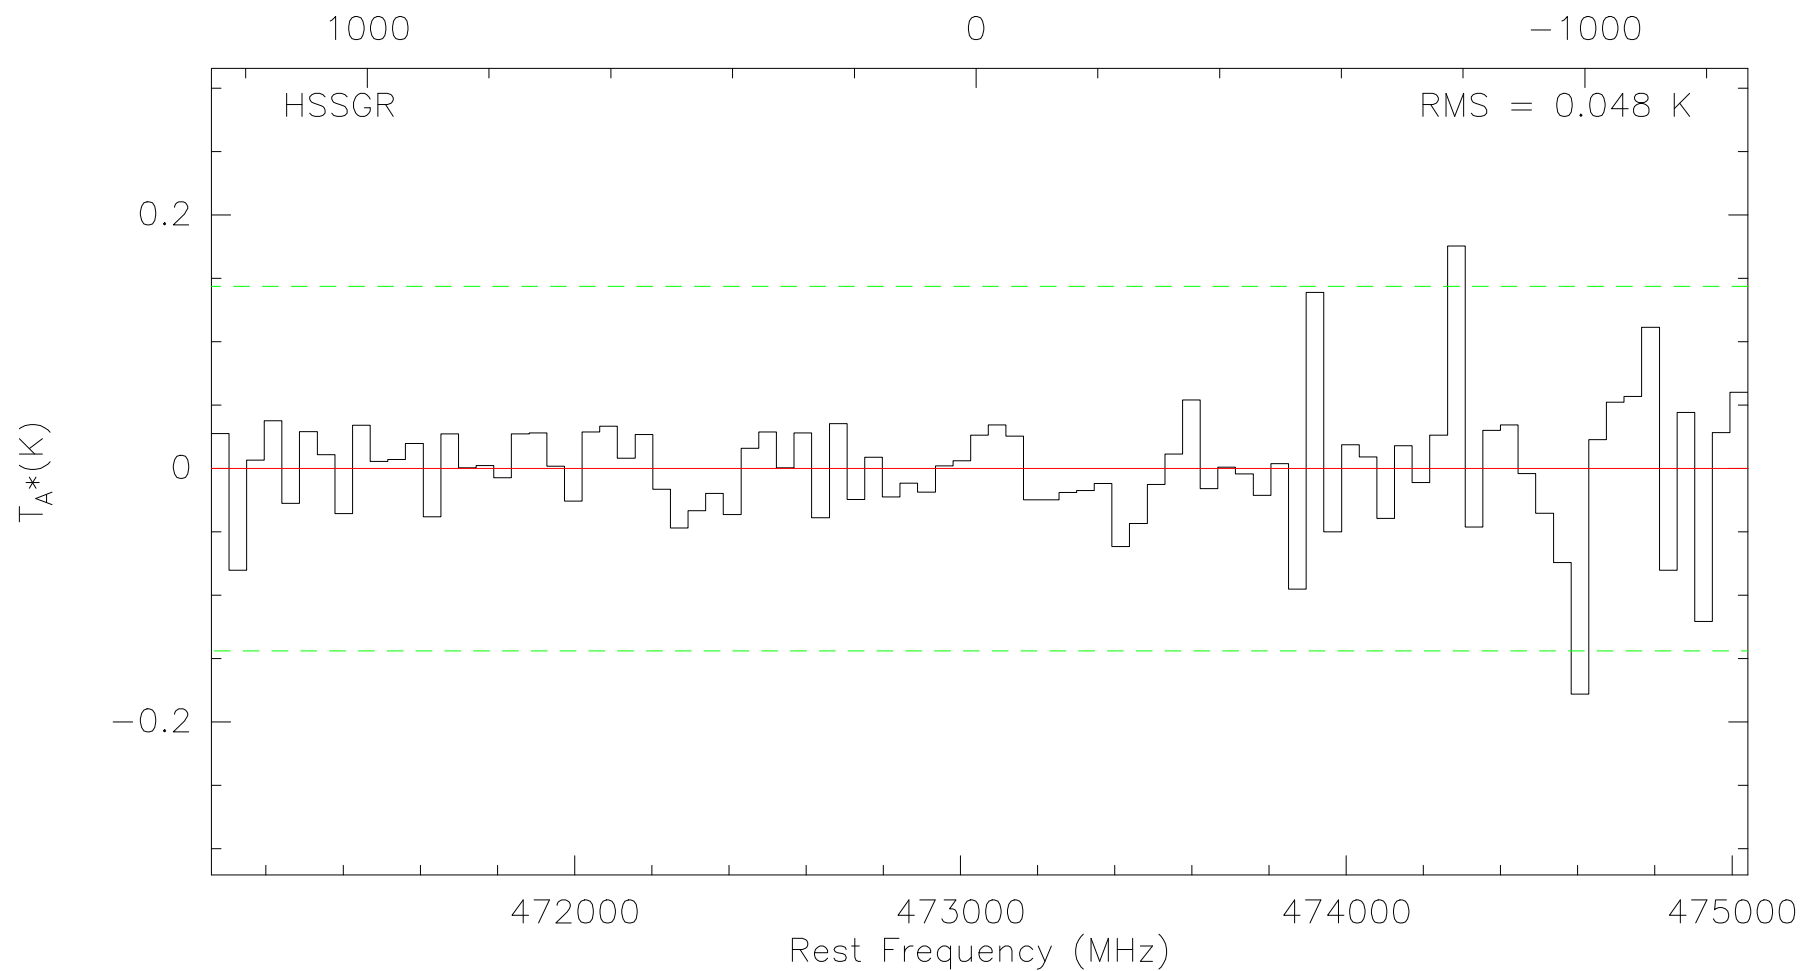

1;1 ILNOR CO(4-3) OSB AP-FL02-XF0- 0:07-JUL-2016 R:07-AUG-2020  
RA: 15:29:23.18 DEC: -50:35:00.7 Eq 2000.0 Rad. 0.0° Offs: -0.2 -0.5  
Unknown tau: 2.112 Tsys: 2947. Time: 9.9min El: 52.2  
N: 87 l0: 44.1918 V0: 0.000 Dv: 29.01 LSR  
F0: 473041.415 Df: -45.78 Fi: 461040.768

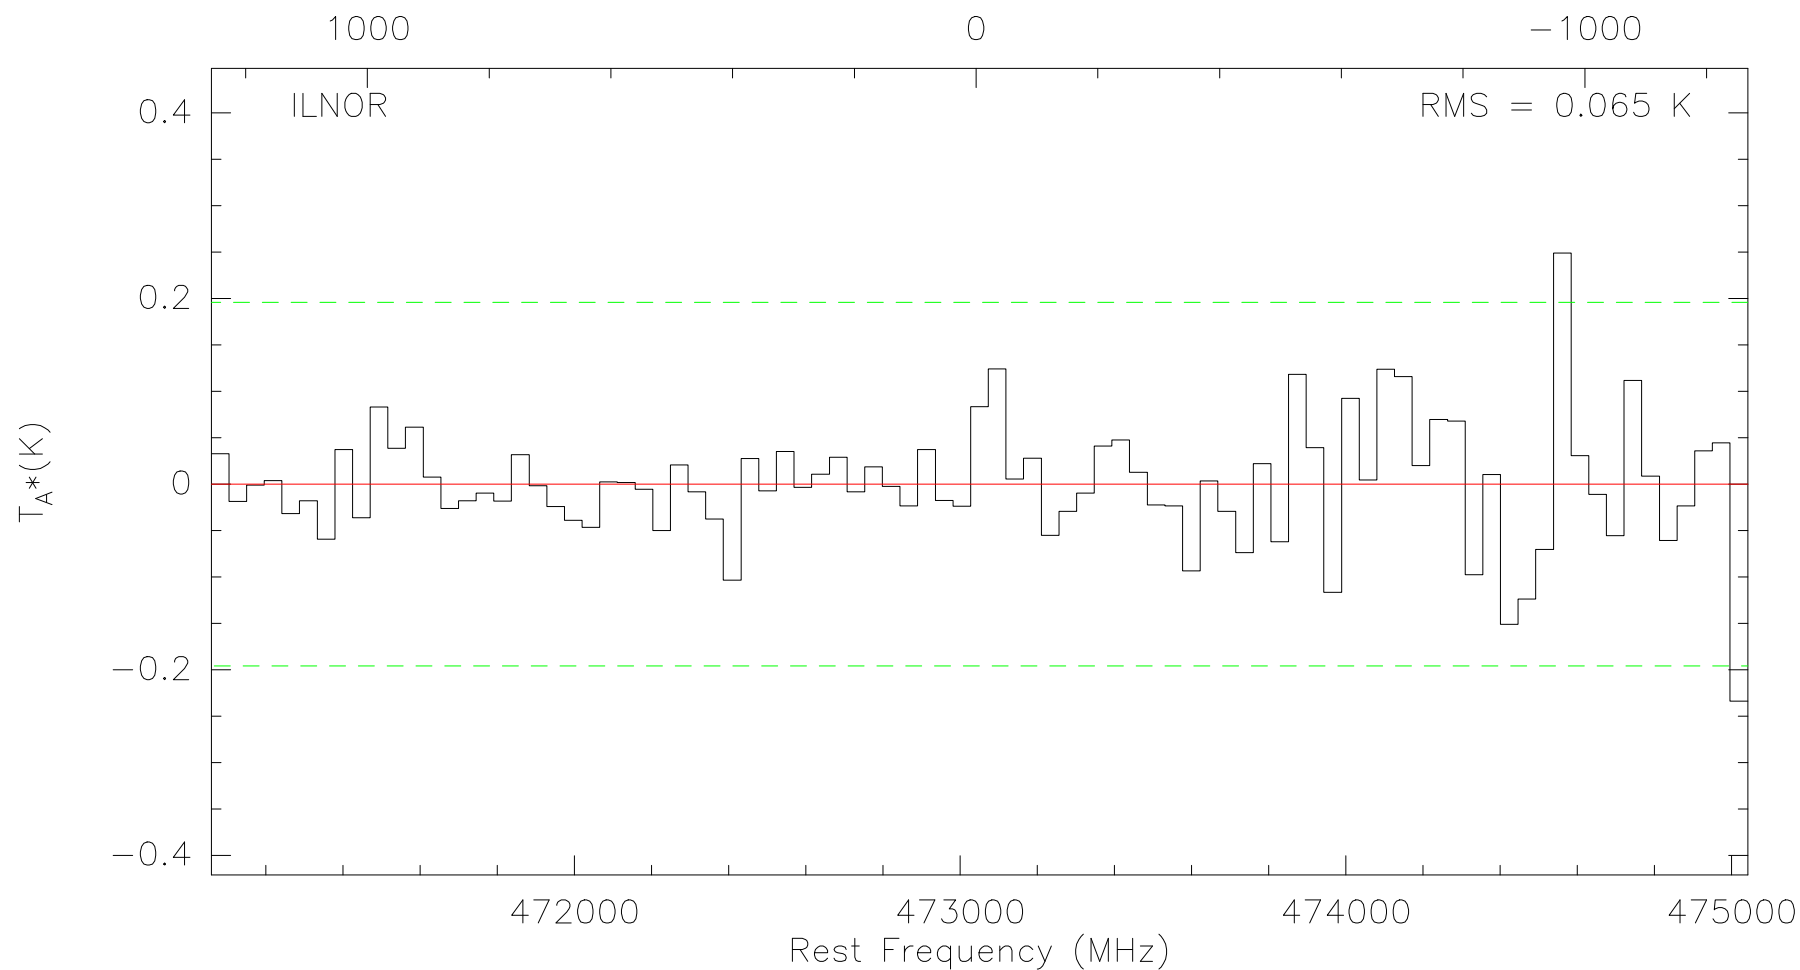

1;1 IMNOR CO(4-3) OSB AP-FL02-XF0- 0:07-JUL-2016 R:07-AUG-2020  
RA: 15:39:26.46 DEC: -52:19:17.9 Eq 2000.0 Rad. 0.0° Offs: -0.2 -0.5  
Unknown tau: 2.118 Tsys: 2631. Time: 9.9min El: 54.7  
N: 87 l0: 44.1918 V0: 0.000 Dv: 29.01 LSR  
F0: 473041.384 Df: -45.78 Fi: 461040.768

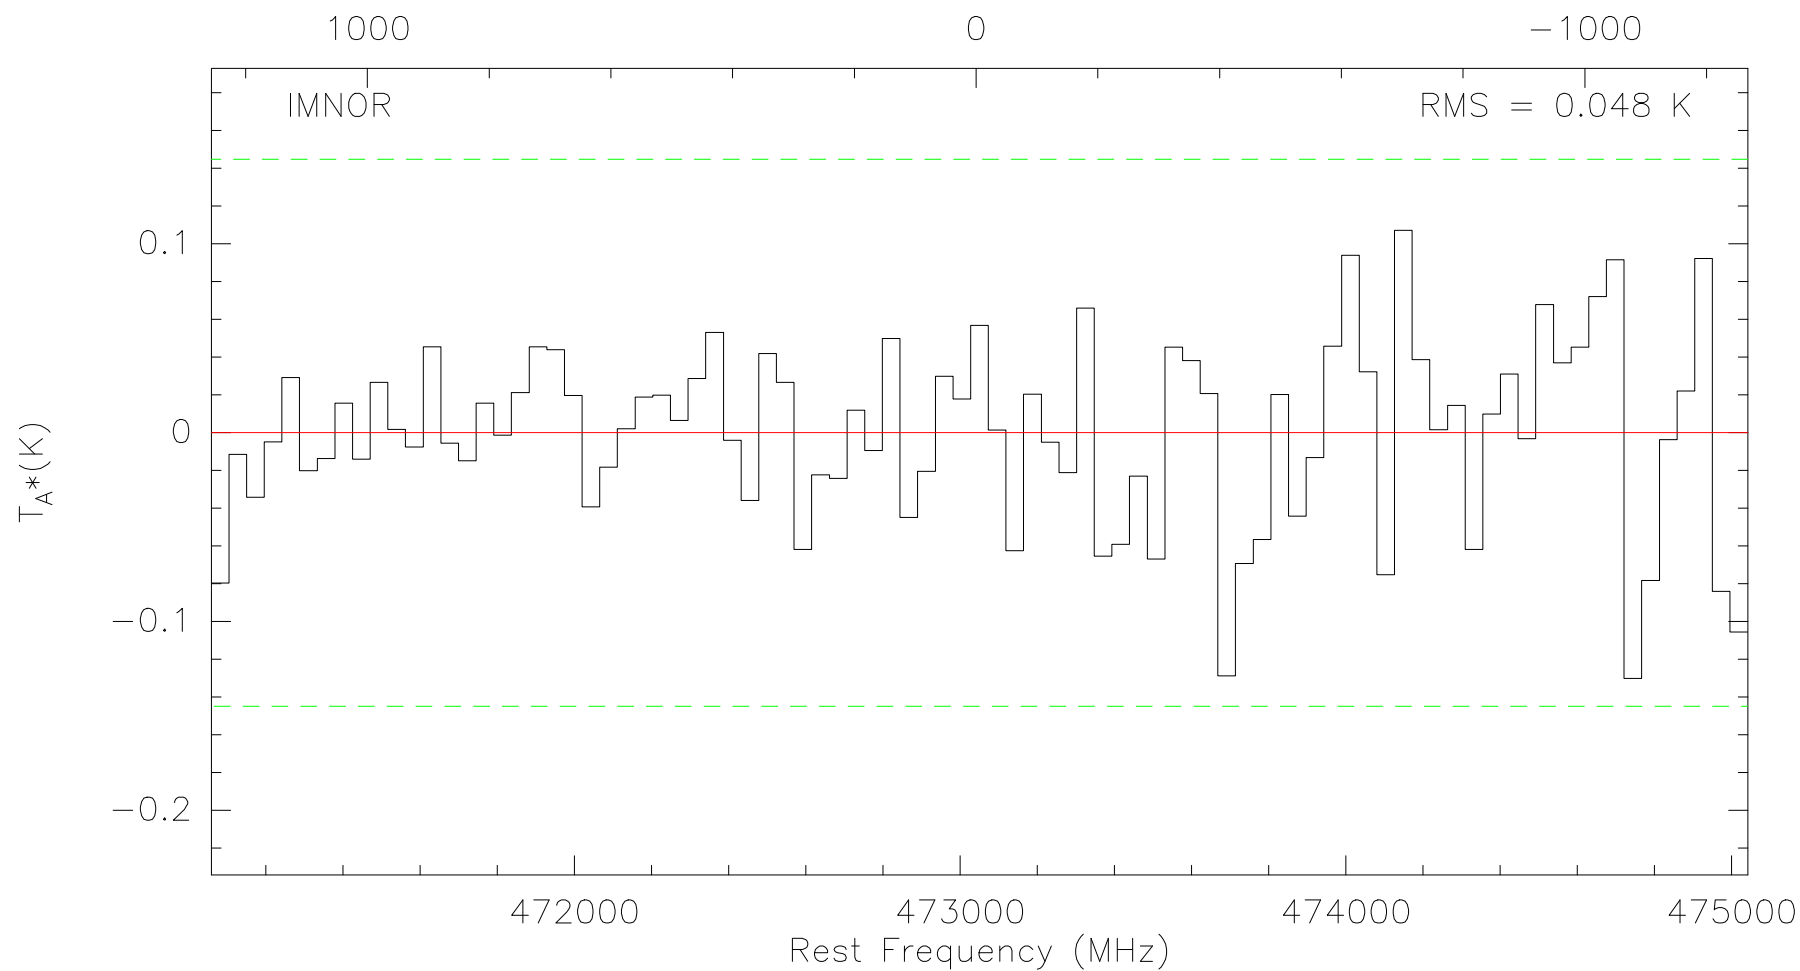

1;1 MTCEN CO(4-3) OSB AP-FL02-XF0- 0:01-JUL-2016 R:07-AUG-2020  
RA: 11:44:00.80 DEC: -60:33:39.5 Eq 2000.0 Rad. 0.0° Offs: +0.3 -0.5  
Unknown tau: 1.891 Tsys: 3562. Time: 24.8min El: 46.2  
N: 87 l0: 44.1920 V0: 0.000 Dv: 29.01 LSR  
FO: 473041.772 Df: -45.78 Fi: 461040.768

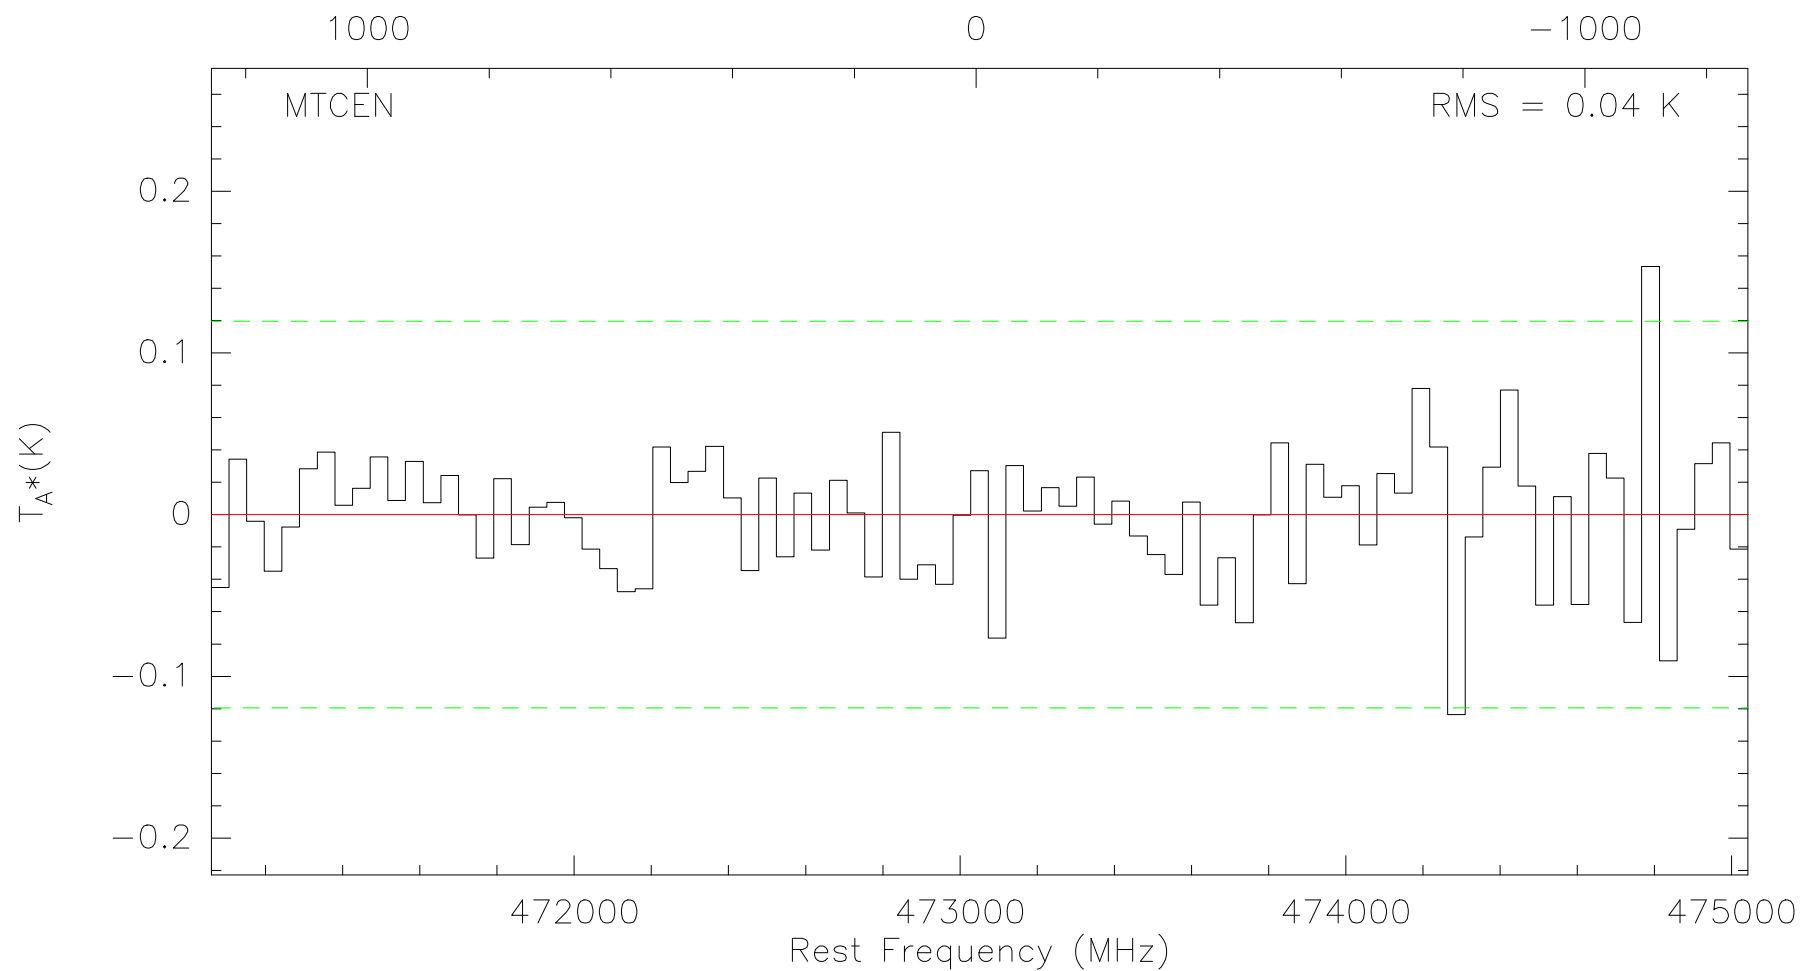

1;1 RSCAR CO(4-3) OSB AP-FL02-XF0- 0:30-JUN-2016 R:07-AUG-2020  
RA: 11:08:06.63 DEC: -61:56:04.6 Eq 2000.0 Rad. 0.0° Offs: +0.3 -0.6  
Unknown tau: 1.888 Tsys: 2936. Time: 19.8min El: 47.6  
N: 87 l0: 44.1919 V0: 0.000 Dv: 29.01 LSR  
F0: 473041.778 Df: -45.78 Fi: 461040.768

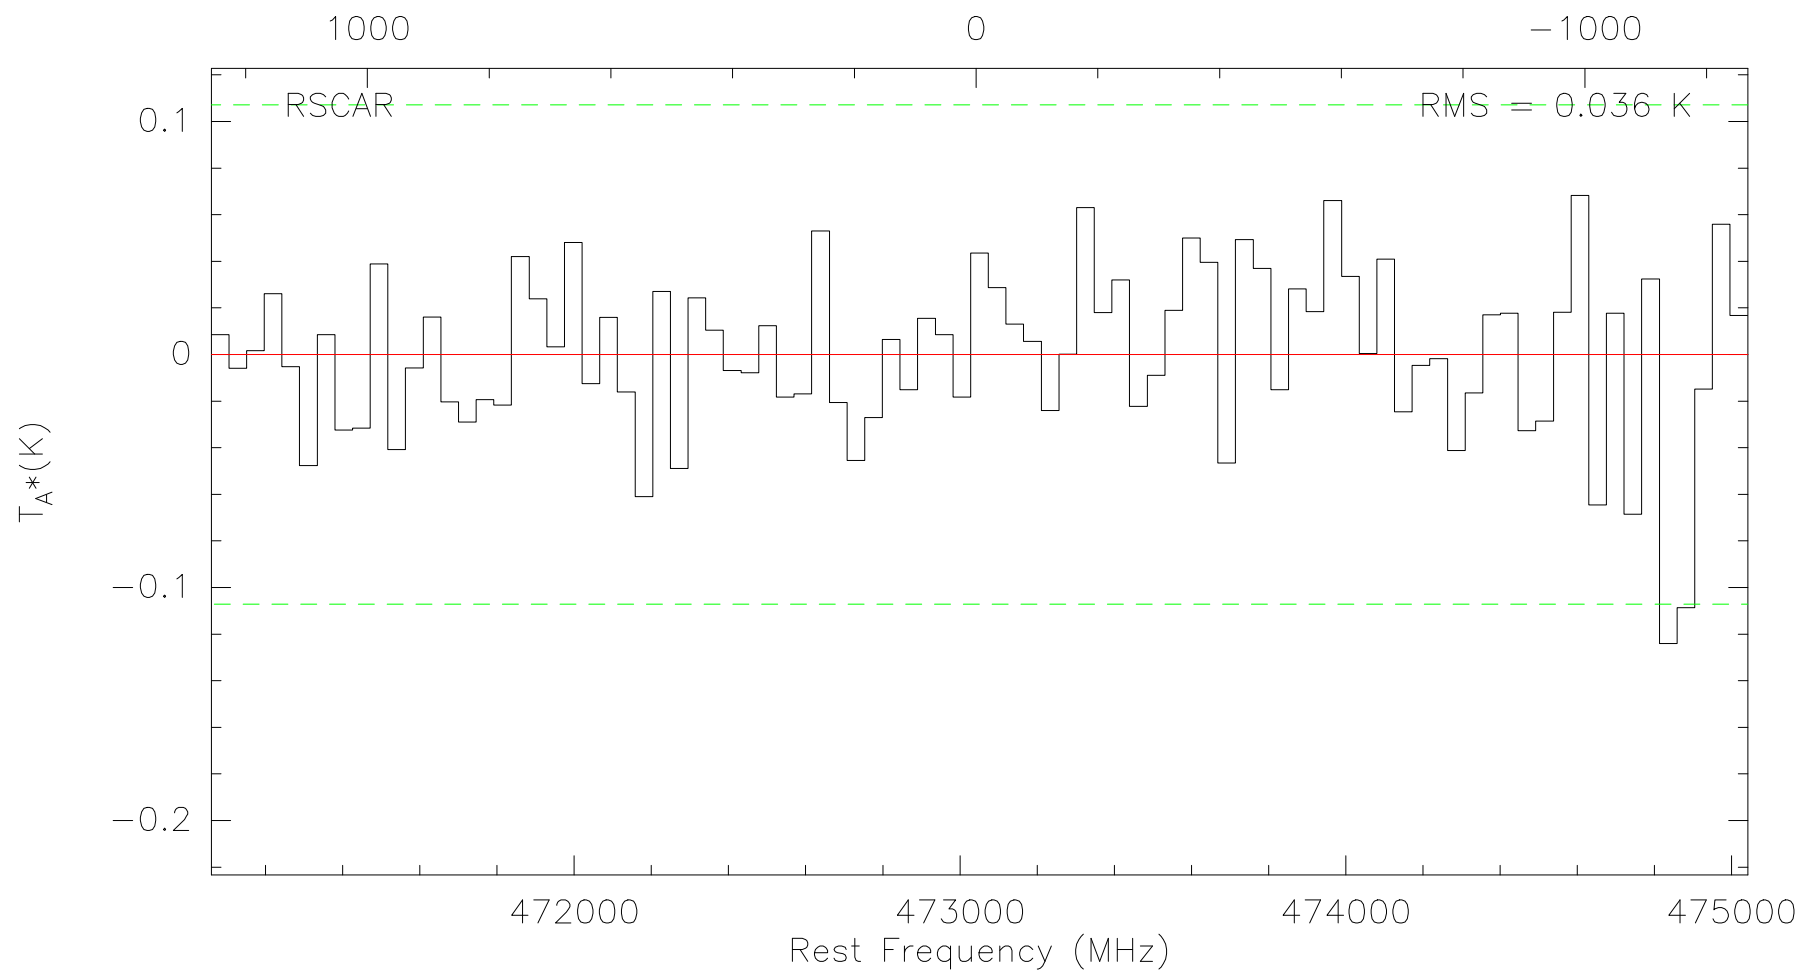

1;1 V1015SGR CO(4-3) OSB AP-FL02-XF0- 0:13-JUL-2016 R:07-AUG-2020  
RA: 18:09:02.00 DEC: -32:28:32.0 Eq 2000.0 Rad. 0.0° Offs: +0.3 -0.3  
Unknown tau: 1.840 Tsys: 3543. Time: 19.8min El: 45.6  
N: 87 l0: 44.1944 V0: 0.000 Dv: 29.01 LSR  
F0: 473040.651 Df: -45.78 Fi: 461040.768

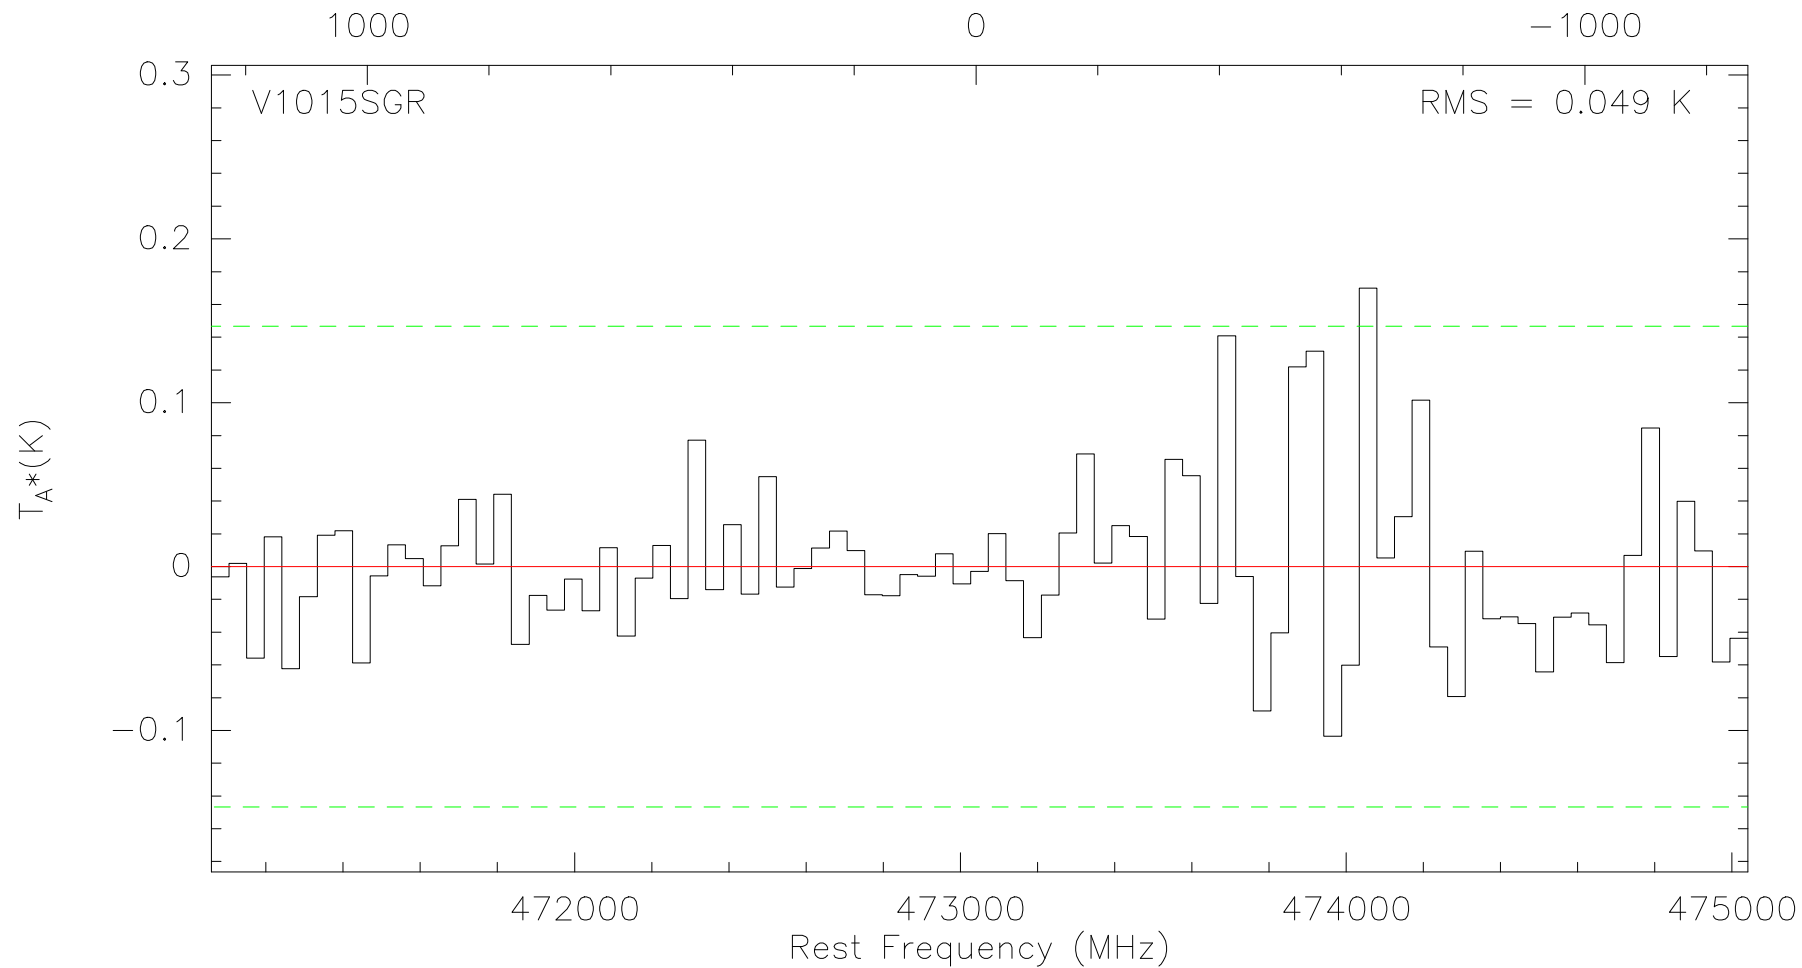

1;1 V1016SGR CO(4-3) OSB AP-FL02-XF0- 0:13-JUL-2016 R:07-AUG-2020  
RA: 18:19:57.63 DEC: -25:11:14.6 Eq 2000.0 Rad. 0.0° Offs: -0.2 -0.3  
Unknown tau: 1.312 Tsys: 2216. Time: 9.9min El: 32.1  
N: 87 l0: 44.1918 V0: 0.000 Dv: 29.01 LSR  
FO: 473040.664 Df: -45.78 Fi: 461040.768

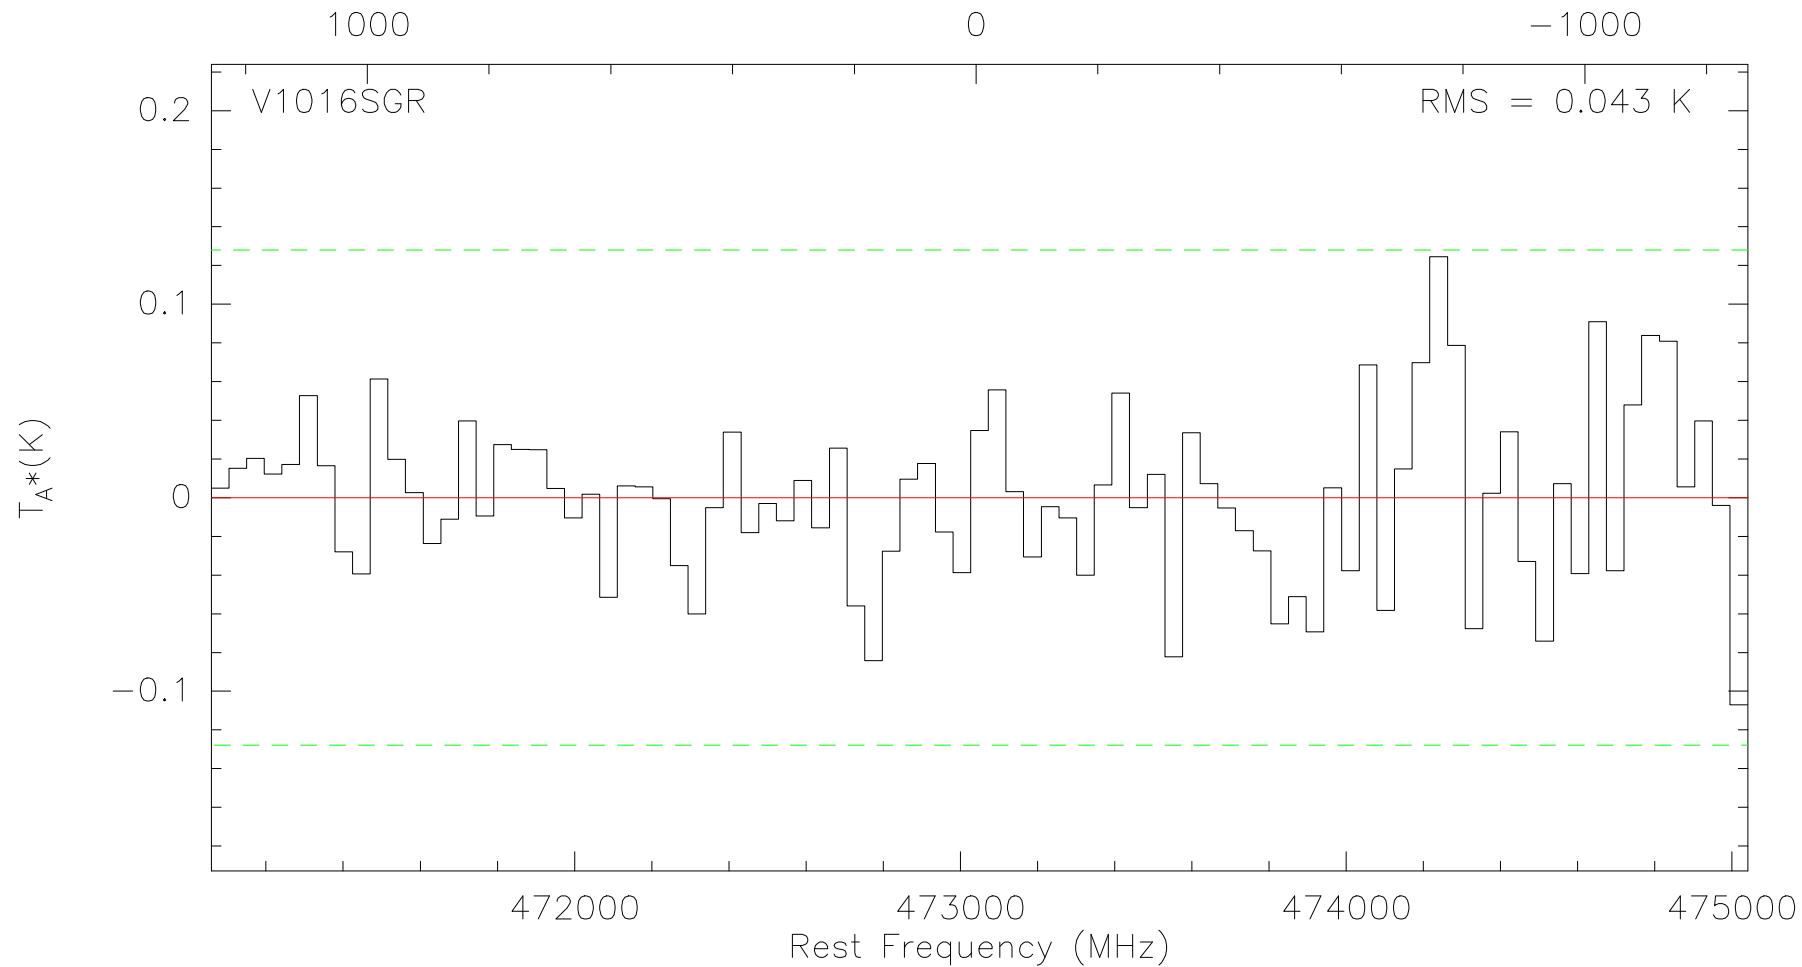

1;1 V1017SGR CO(4-3) OSB AP-FL02-XF0- 0:13-JUL-2016 R:07-AUG-2020  
RA: 18:32:04.47 DEC: -29:23:12.5 Eq 2000.0 Rad. 0.0° Offs: +0.4 -0.4  
Unknown tau: 2.015 Tsys: 1636. Time: 14.9min El: 75.2  
N: 87 l0: 44.1919 V0: 0.000 Dv: 29.01 LSR  
F0: 473040.643 Df: -45.78 Fi: 461040.768

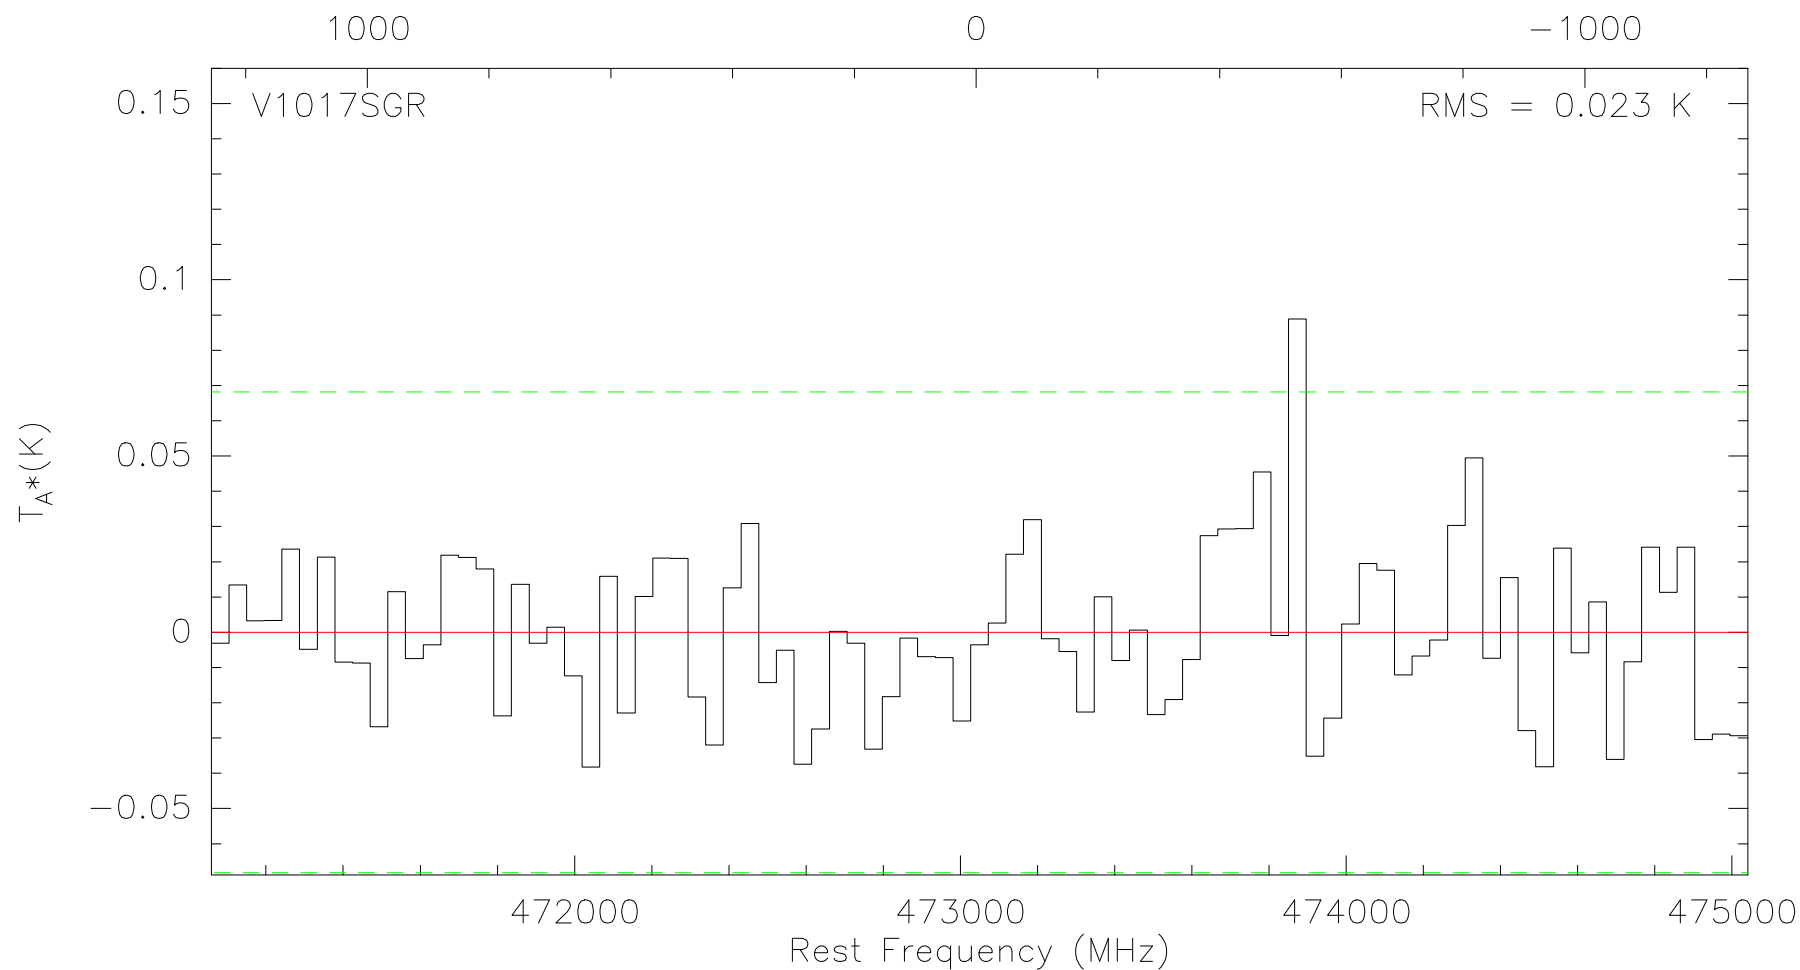

1;1 V1149SGR CO(4-3) OSB AP-FL02-XF0- 0:13-JUL-2016 R:07-AUG-2020  
RA: 18:18:30.40 DEC: -28:17:17.0 Eq 2000.0 Rad. 0.0° Offs: -0.2 -0.6  
Unknown tau: 1.437 Tsys: 1153. Time: 9.9min El: 61.7  
N: 87 l0: 44.1918 V0: 0.000 Dv: 29.01 LSR  
FO: 473040.699 Df: -45.78 Fi: 461040.768

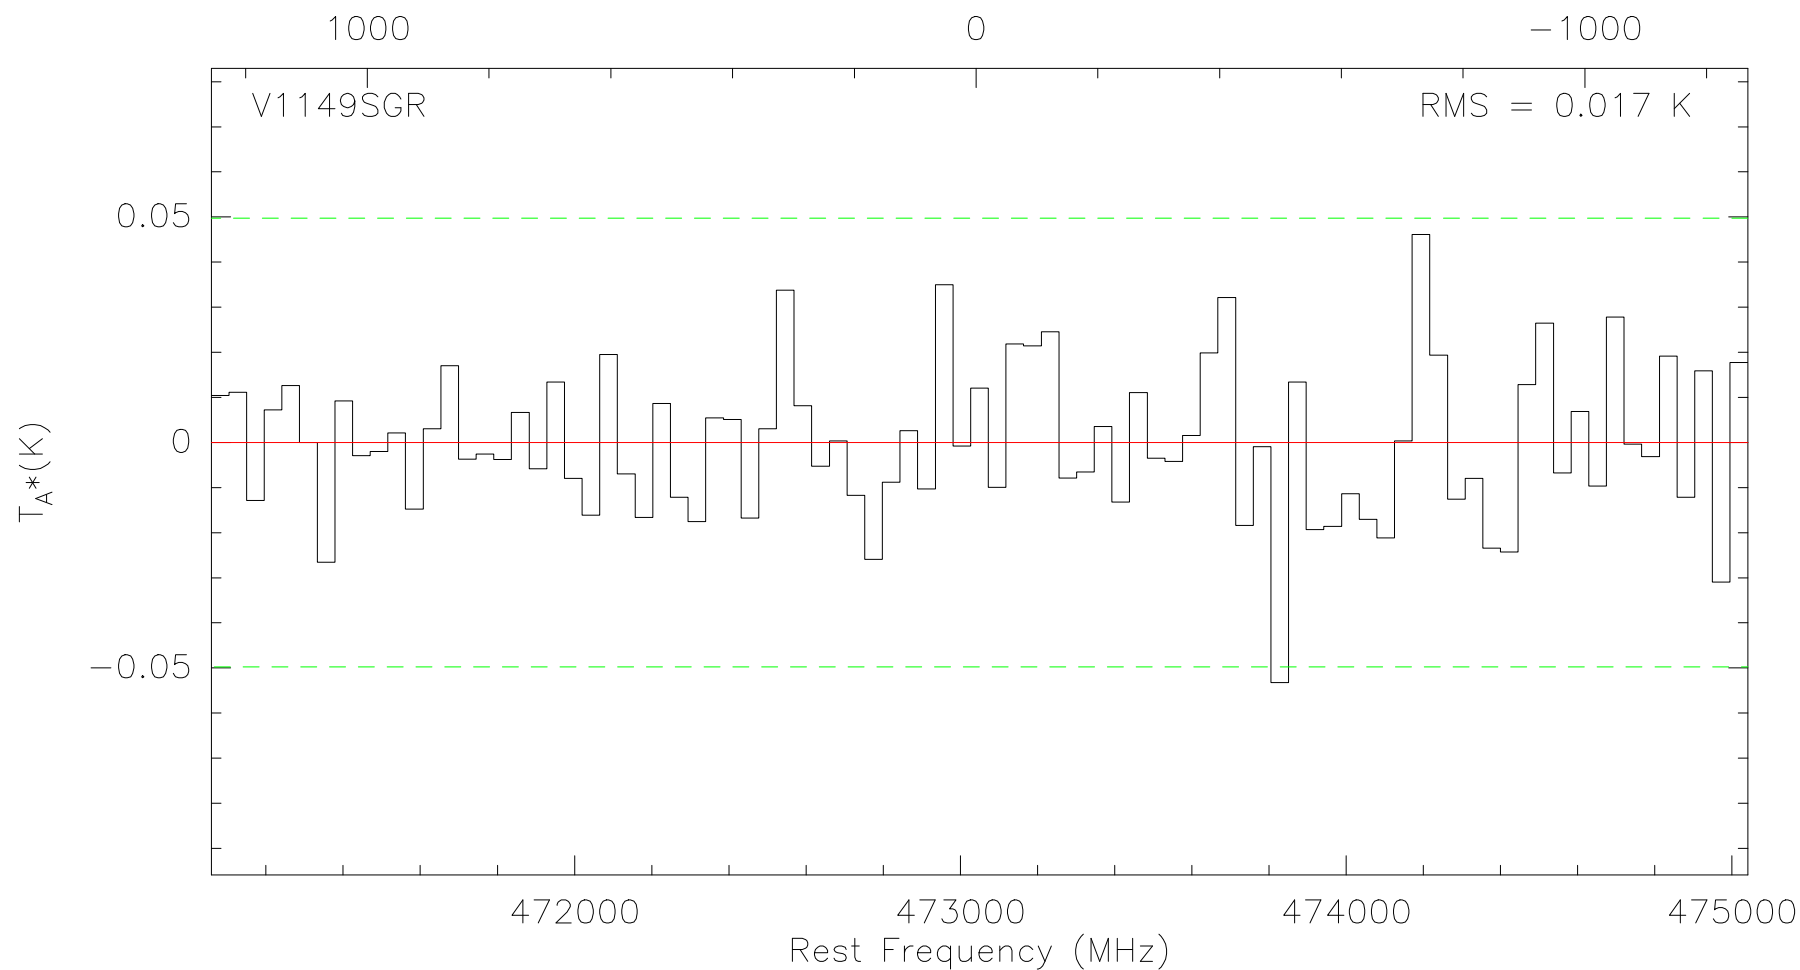

1;1 V1151SGR CO(4-3) OSB AP-FL02-XF0- 0:14-JUL-2016 R:07-AUG-2020  
RA: 18:25:23.75 DEC: -20:11:59.3 Eq 2000.0 Rad. 0.0° Offs: -0.2 -0.3  
Unknown tau: 1.383 Tsys: 3629. Time: 9.9min El: 26.8  
N: 87 l0: 44.1918 V0: 0.000 Dv: 29.01 LSR  
F0: 473040.602 Df: -45.78 Fi: 461040.768

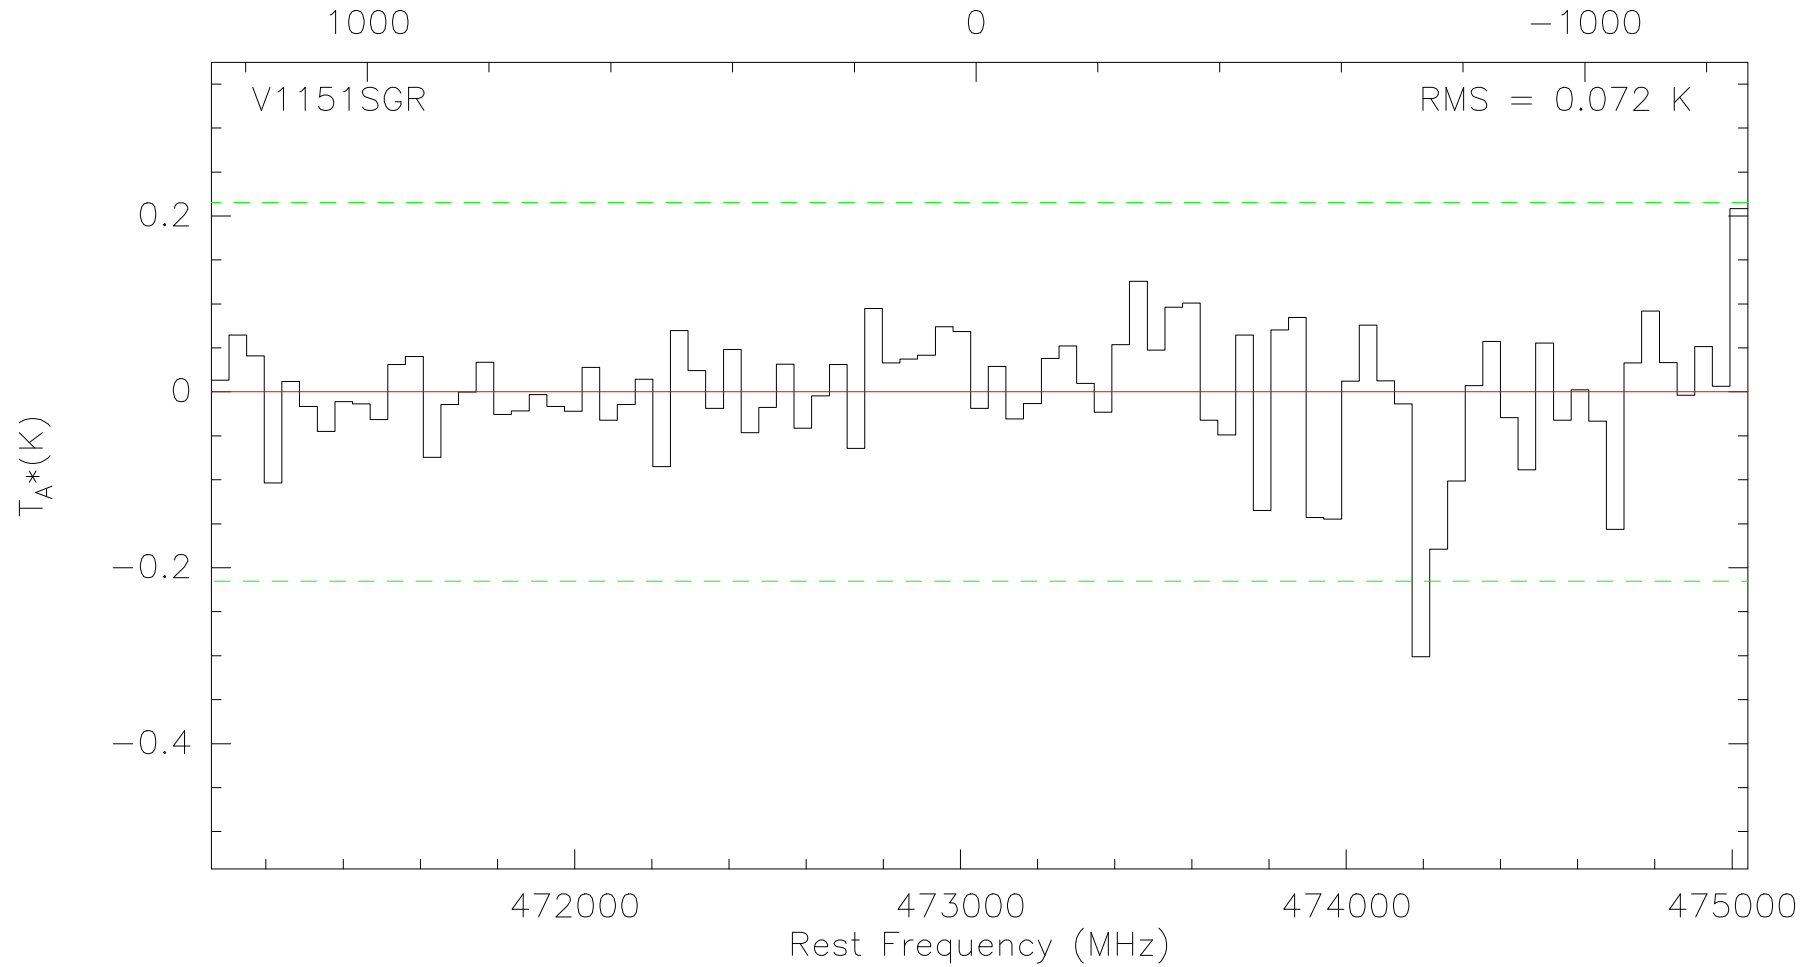

1;1 V1583SGR CO(4-3) OSB AP-FL02-XF0- 0:14-JUL-2016 R:07-AUG-2020  
RA: 18:15:26.30 DEC: -23:23:18.0 Eq 2000.0 Rad. 0.0° Offs: -0.2 -0.3  
Unknown tau: 1.502 Tsys: 3272. Time: 9.9min El: 30.0  
N: 87 l0: 44.1918 V0: 0.000 Dv: 29.01 LSR  
F0: 473040.682 Df: -45.78 Fi: 461040.768

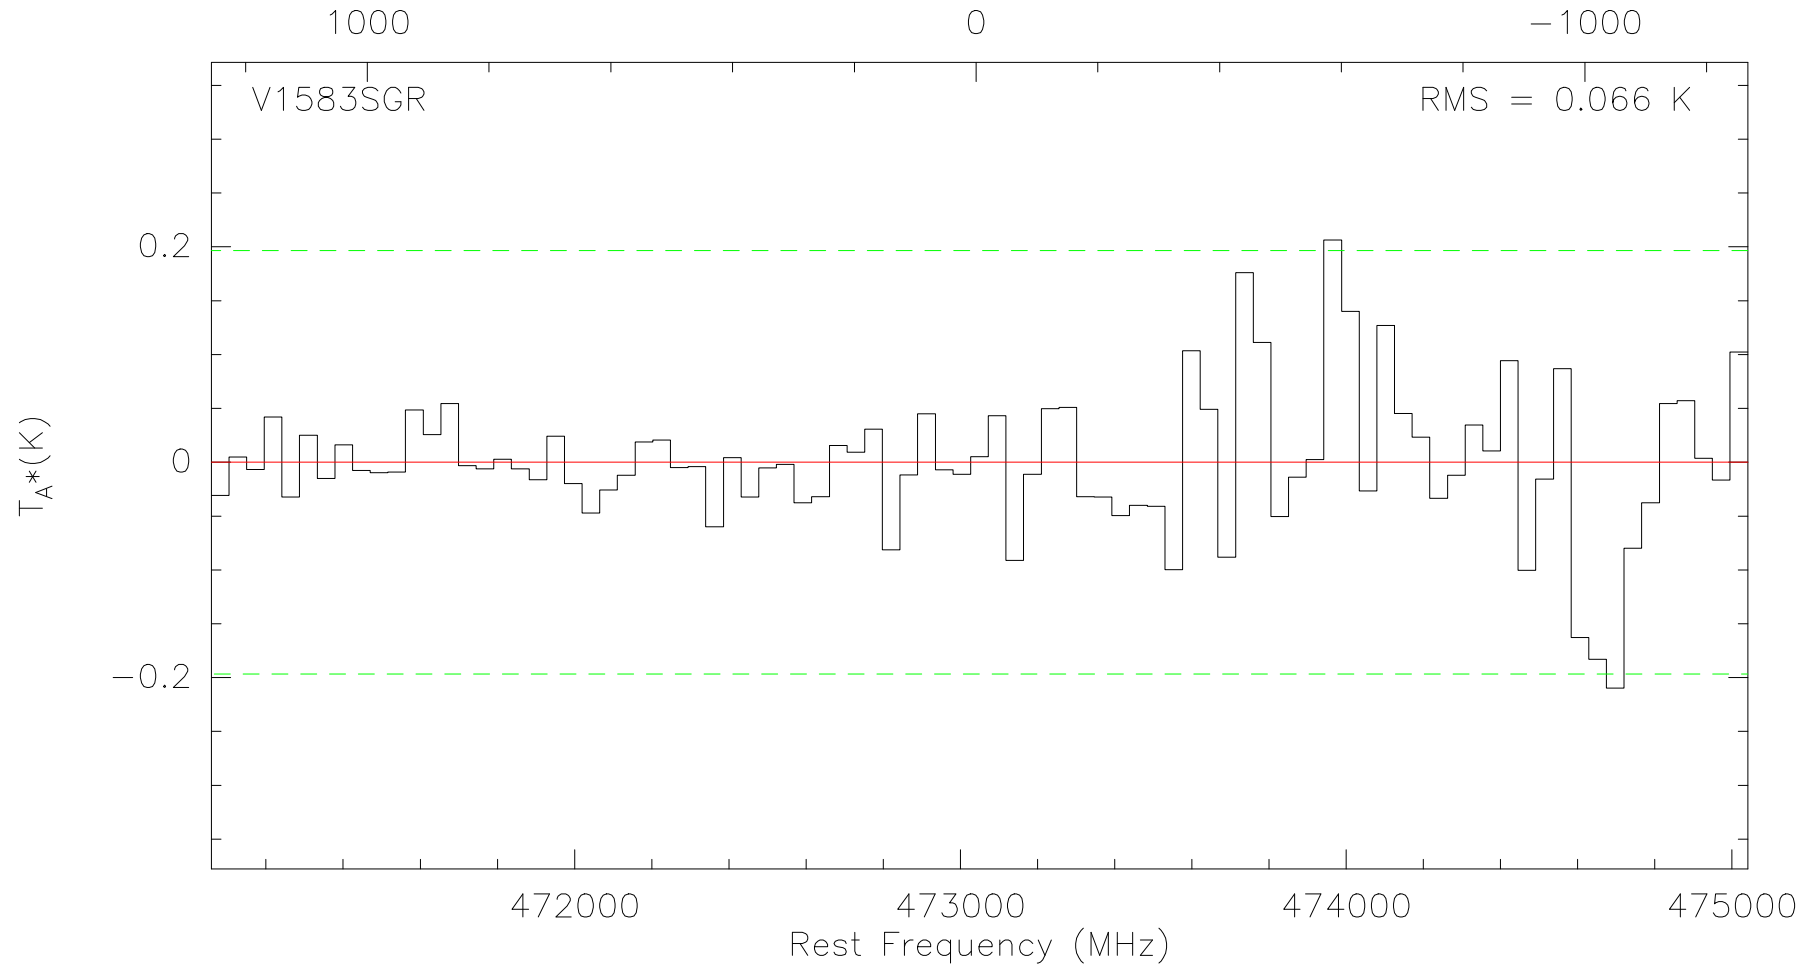

1;1 V363SGR CO(4-3) OSB AP-FL02-XF0- 0:01-JUL-2016 R:07-AUG-2020  
RA: 19:11:16.30 DEC: -29:50:00.0 Eq 2000.0 Rad. 0.0° Offs: -0.2 -0.6  
Unknown tau: 2.733 Tsys: 9152. Time: 19.9min El: 42.0  
N: 87 l0: 44.1919 V0: 0.000 Dv: 29.01 LSR  
FO: 473040.283 Df: -45.77 Fi: 461040.768

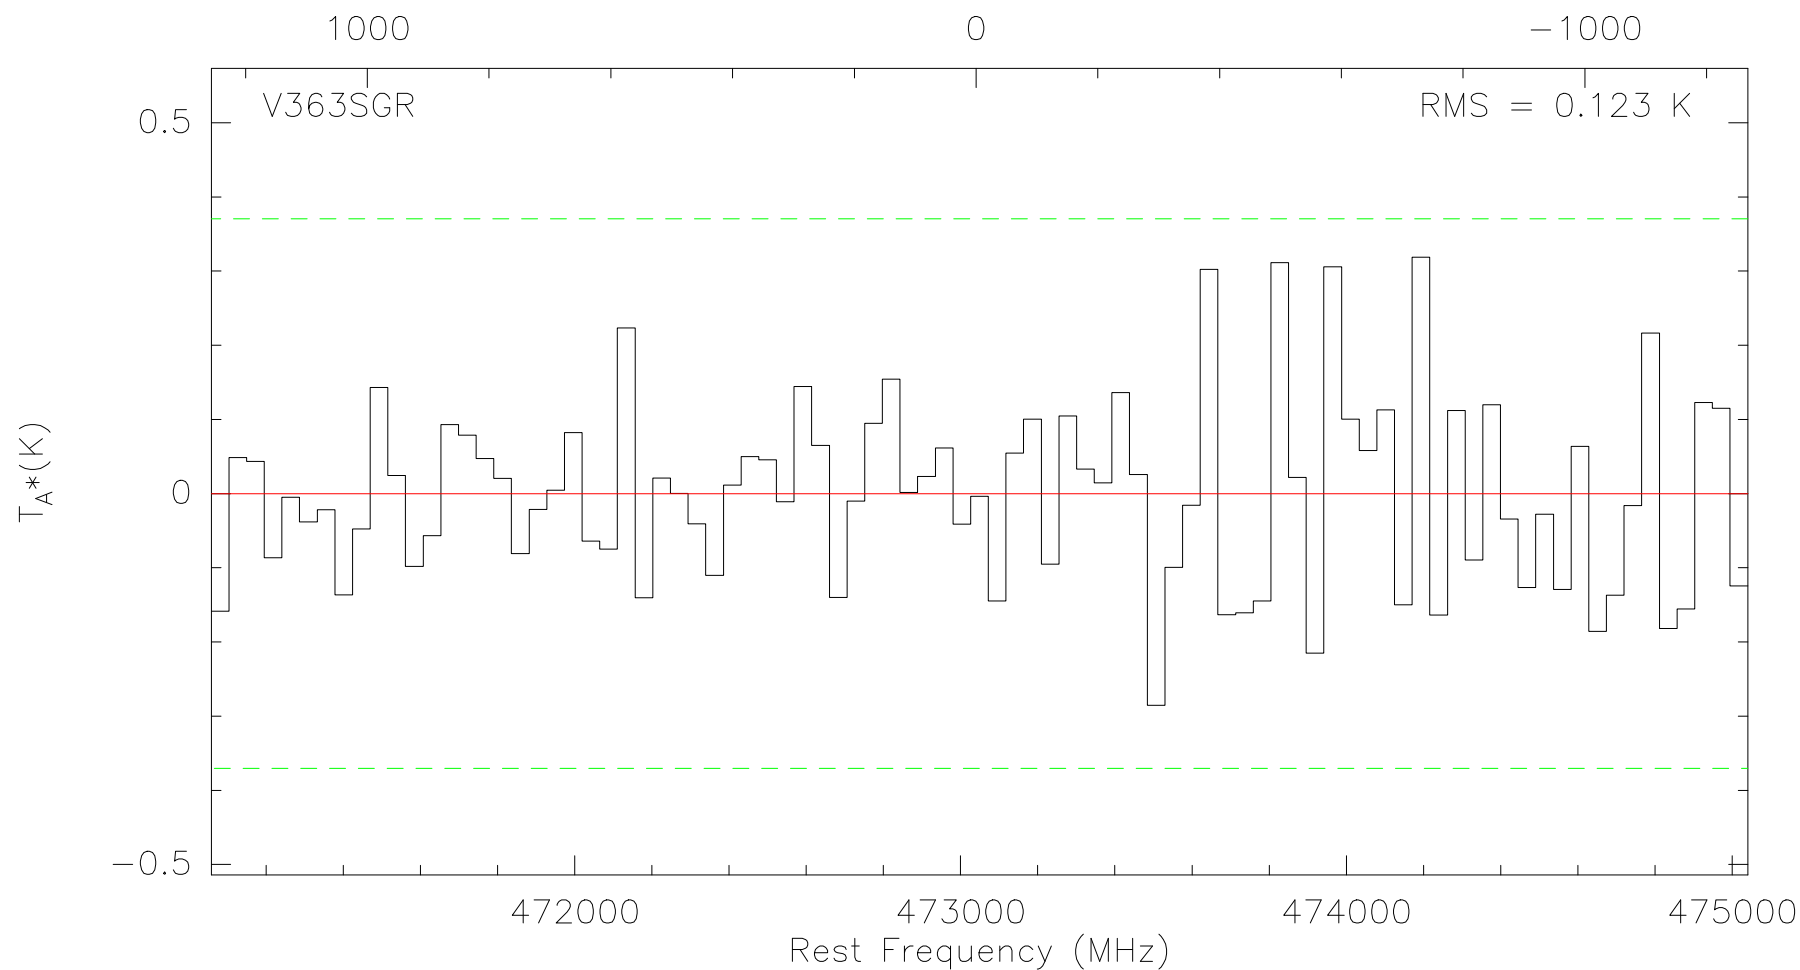

1;1 V365CAR CO(4-3) OSB AP-FL02-XF0- 0:30-JUN-2016 R:07-AUG-2020  
RA: 11:03:16.77 DEC: -58:27:24.9 Eq 2000.0 Rad. 0.0° Offs: +0.3 -0.5  
Unknown tau: 1.877 Tsys: 2662. Time: 19.8min El: 51.3  
N: 87 l0: 44.1920 V0: 0.000 Dv: 29.01 LSR  
F0: 473041.832 Df: -45.78 Fi: 461040.768

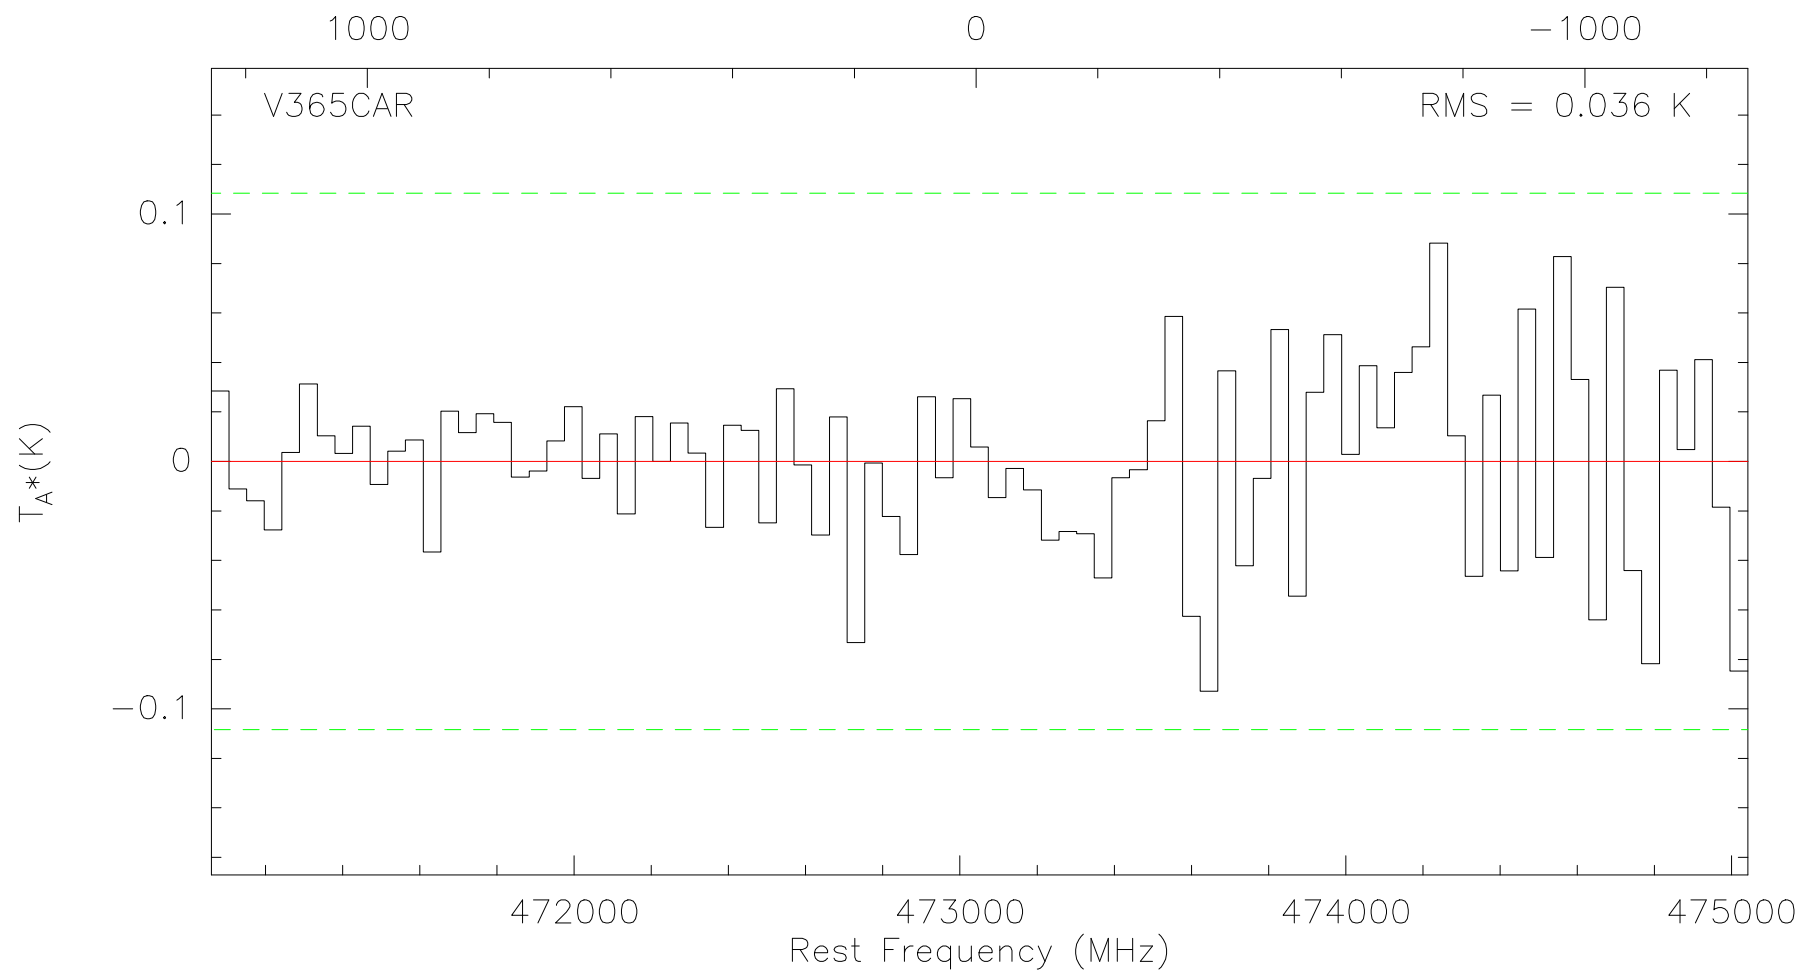

1;1 V382SCO CO(4-3) OSB AP-FL02-XF0- 0:13-JUL-2016 R:07-AUG-2020  
RA: 17:51:56.13 DEC: -35:25:05.4 Eq 2000.0 Rad. 0.0° Offs: +0.1 -0.6  
Unknown tau: 1.492 Tsys: 1082. Time: 9.9min El: 72.8  
N: 87 l0: 44.1918 V0: 0.000 Dv: 29.01 LSR  
F0: 473040.883 Df: -45.78 Fi: 461040.768

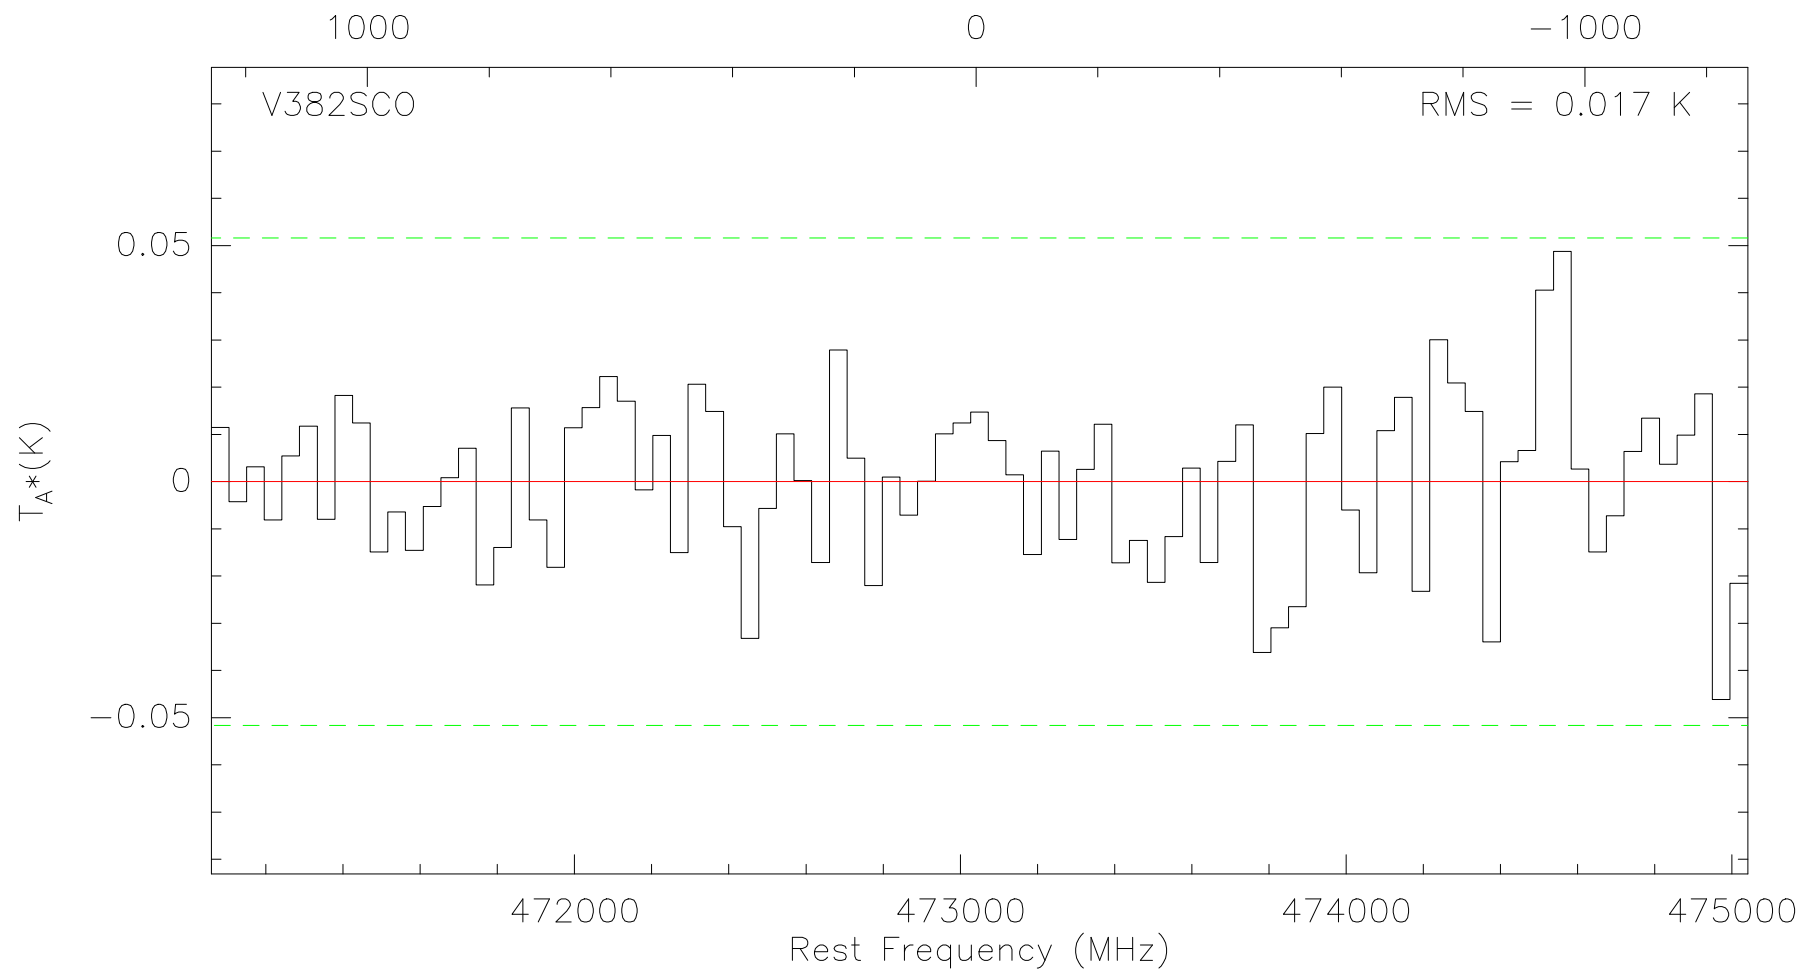

1;1 V384SCO CO(4-3) OSB AP-FL02-XF0- 0:14-JUL-2016 R:07-AUG-2020  
RA: 18:01:43.15 DEC: -35:39:27.8 Eq 2000.0 Rad. 0.0° Offs: +0.3 -0.3  
Unknown tau: 2.221 Tsys: 3655. Time: 9.9min El: 52.1  
N: 87 l0: 44.1918 V0: 0.000 Dv: 29.01 LSR  
FO: 473040.850 Df: -45.78 Fi: 461040.768

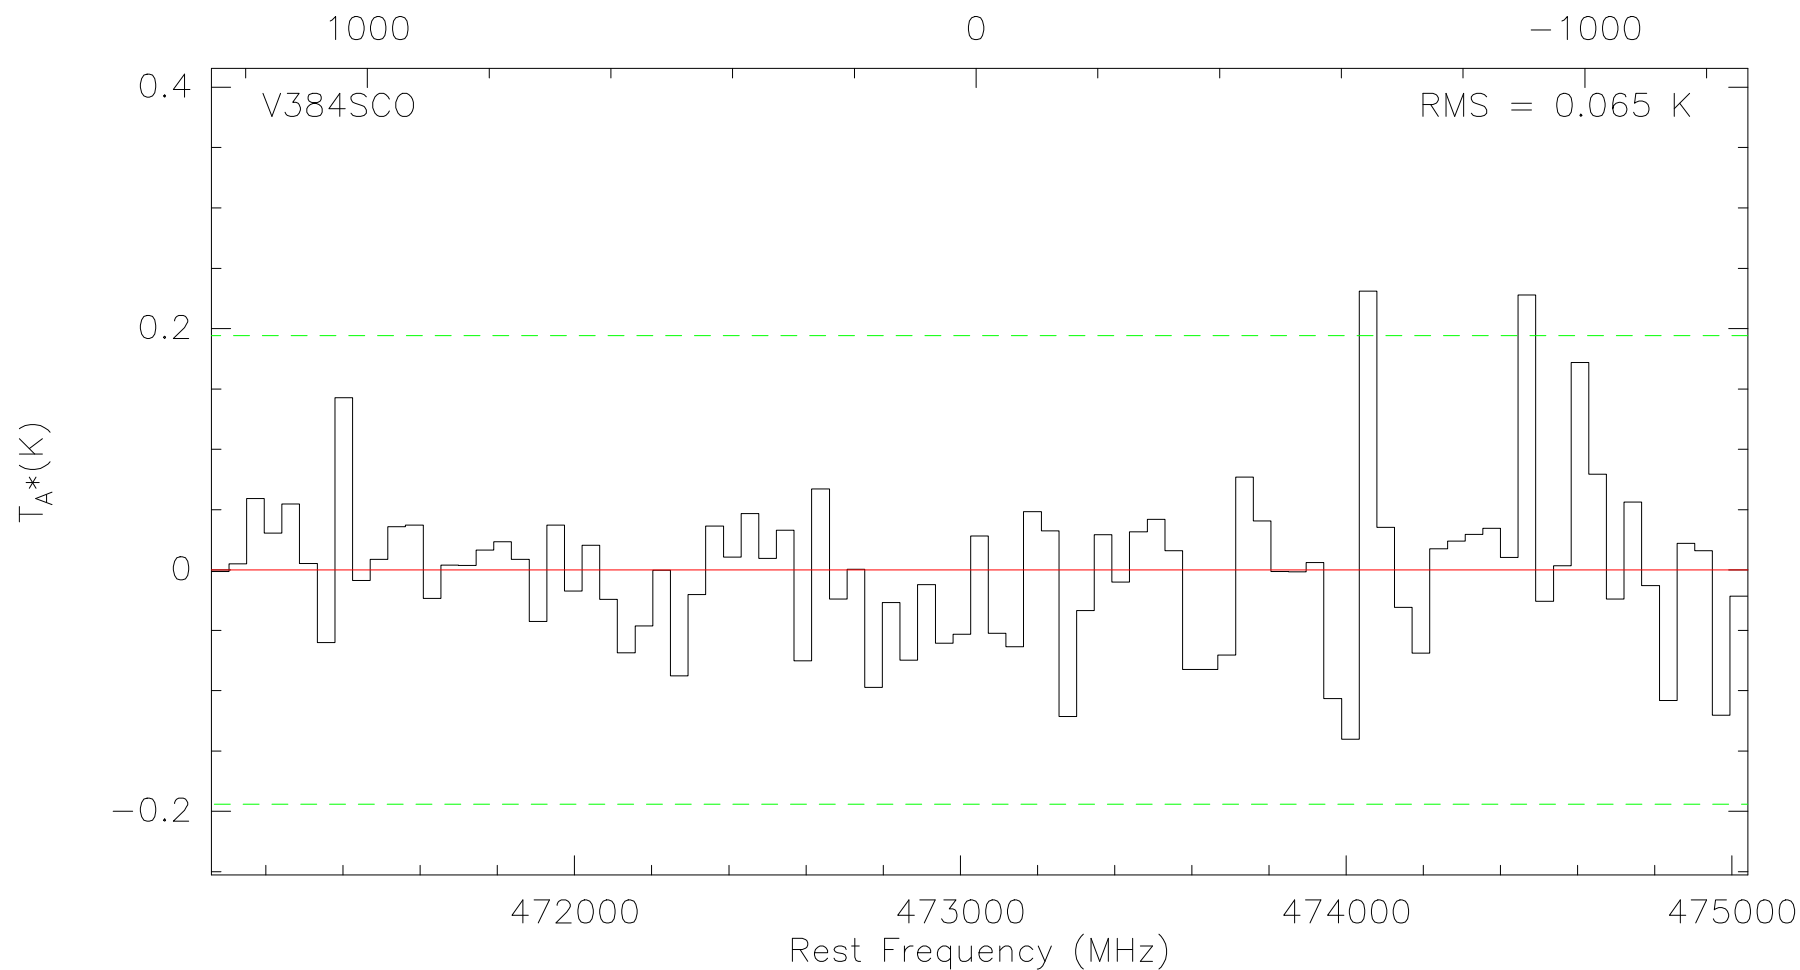

1;1 V522SGR CO(4-3) OSB AP-FL02-XF0- 0:01-JUL-2016 R:07-AUG-2020  
RA: 18:48:00.47 DEC: -25:22:21.9 Eq 2000.0 Rad. 0.0° Offs: -0.2 -0.5  
Unknown tau: 2.420 Tsys: 11343. Time: 19.8min El: 31.8  
N: 87 l0: 44.1919 V0: 0.000 Dv: 29.01 LSR  
F0: 473040.313 Df: -45.77 Fi: 461040.768

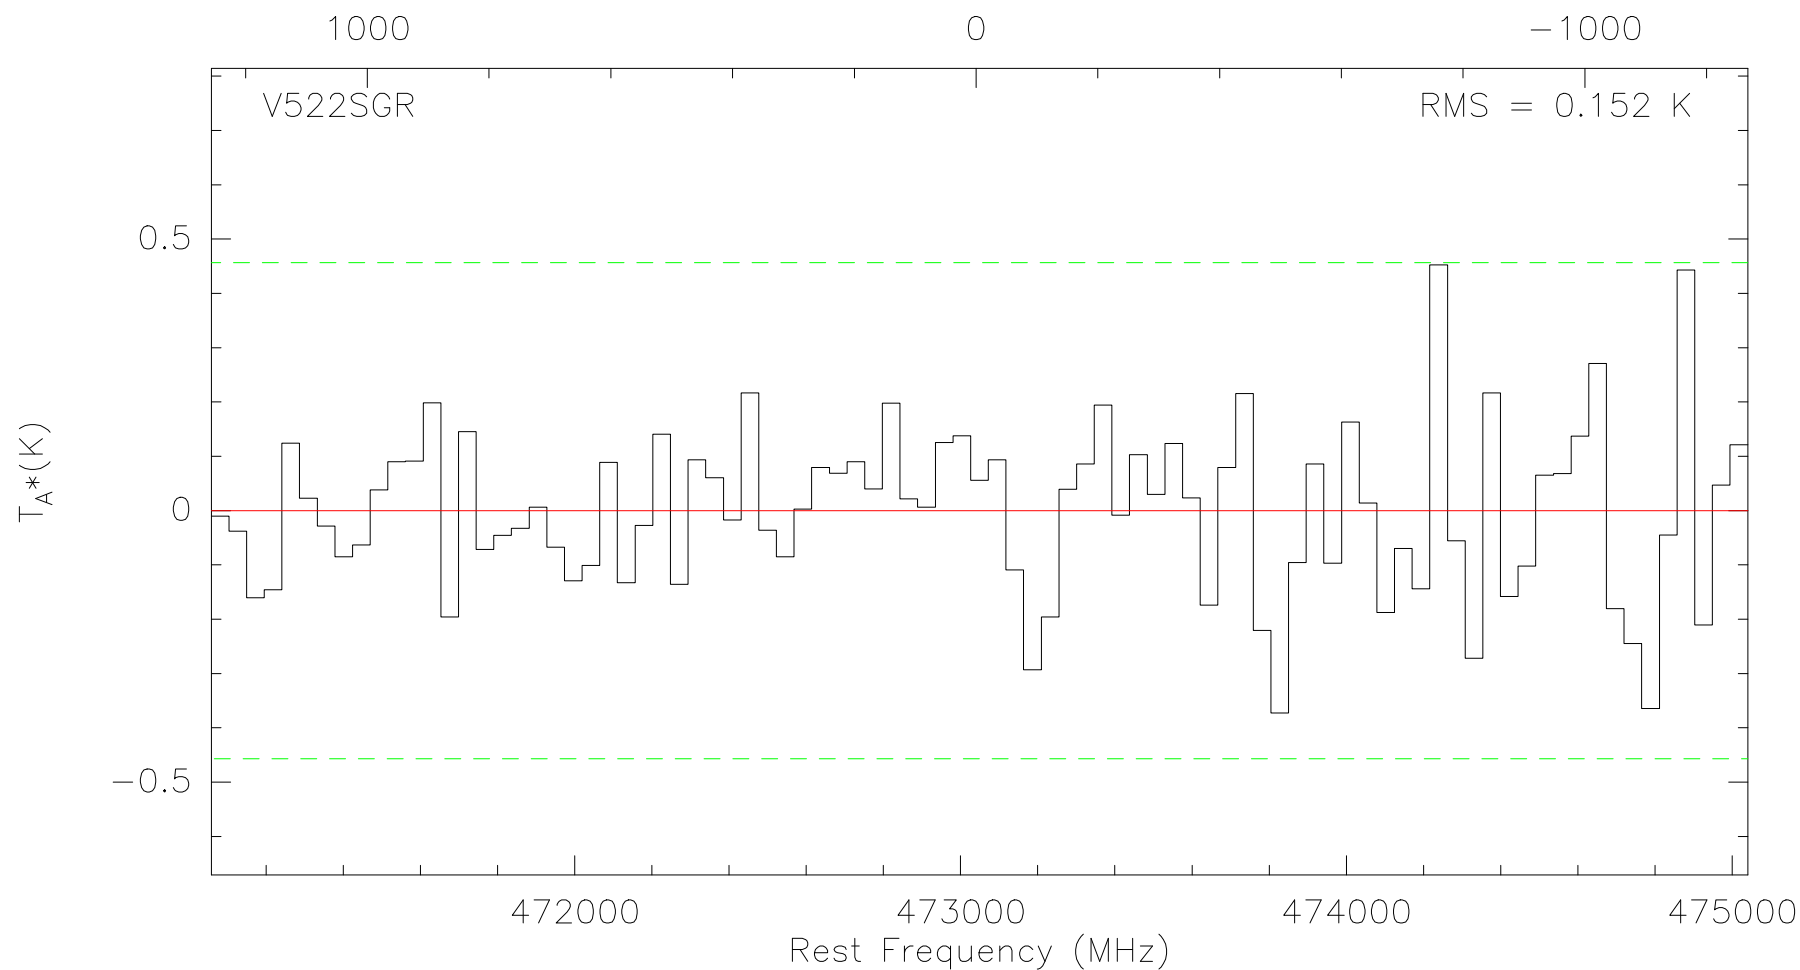

1;1 V5530PH CO(4-3) OSB AP-FL02-XF0- 0:01-JUL-2016 R:07-AUG-2020  
RA: 17:42:53.50 DEC: -24:51:26.2 Eq 2000.0 Rad. 0.0° Offs: -0.4 -0.5  
Unknown tau: 2.577 Tsys: 10566. Time: 9.9min El: 38.8  
N: 87 l0: 44.1918 V0: 0.000 Dv: 29.01 LSR  
F0: 473040.596 Df: -45.78 Fi: 461040.768

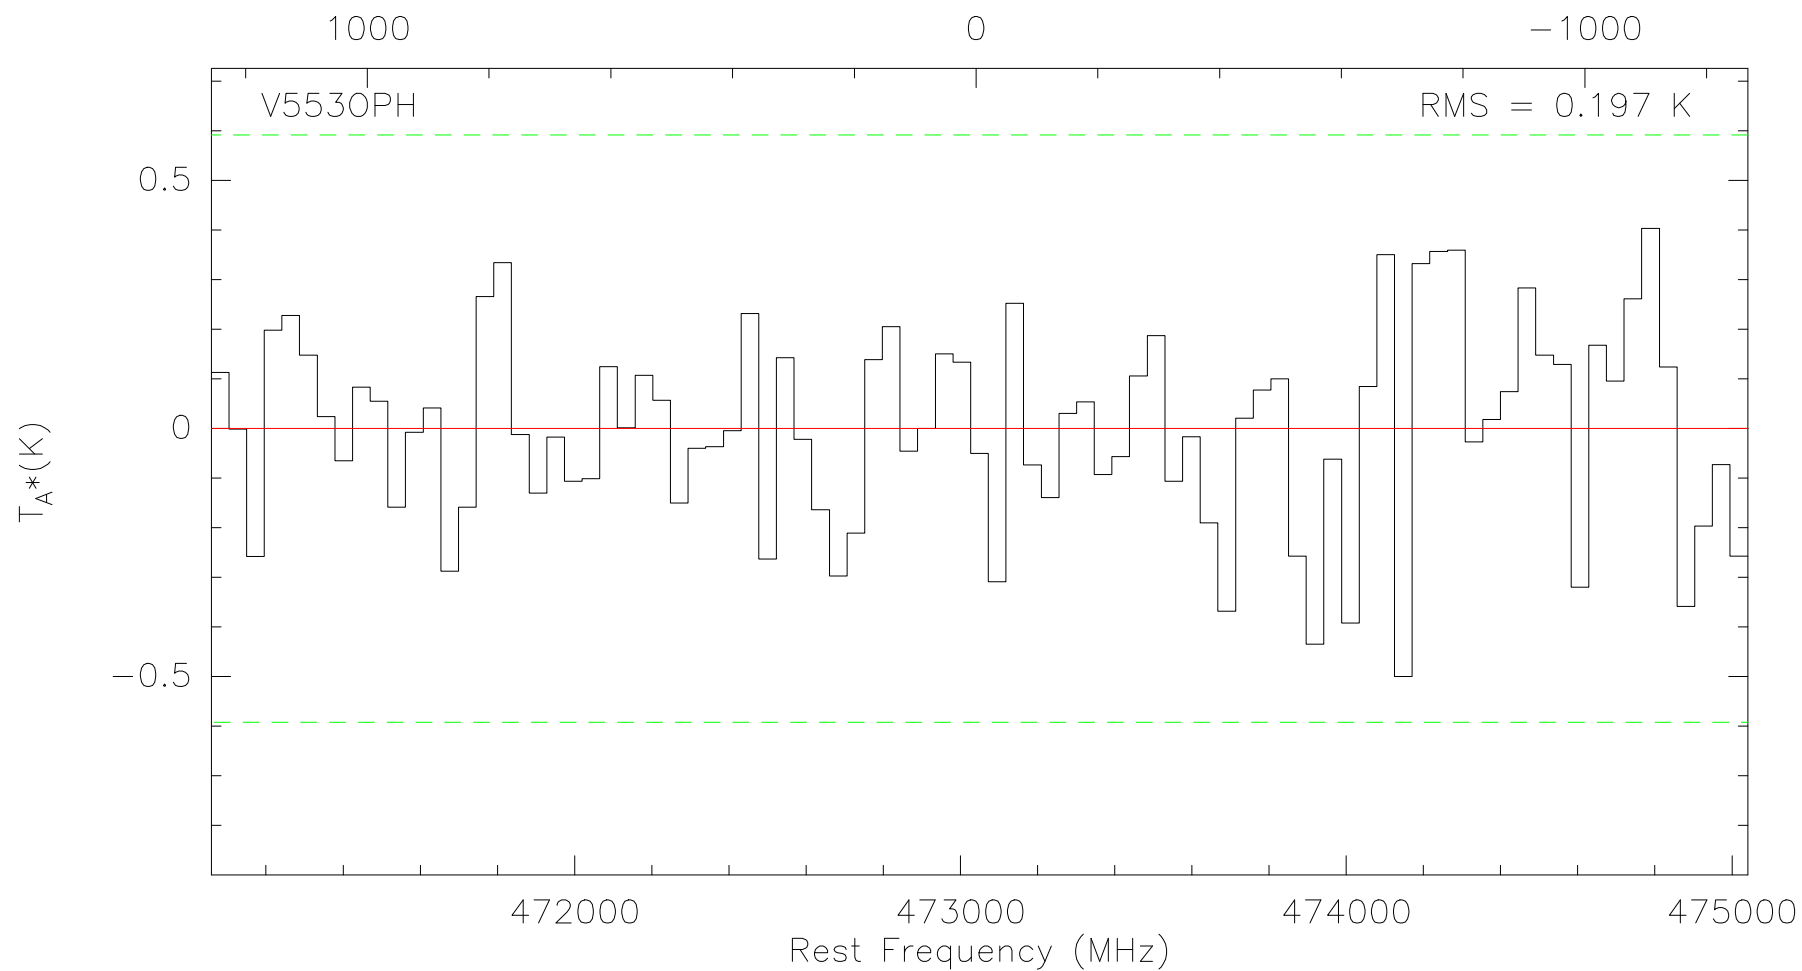

1;1 V696SCO CO(4-3) OSB AP-FL02-XF0- 0:13-JUL-2016 R:07-AUG-2020  
RA: 17:53:11.55 DEC: -35:50:14.4 Eq 2000.0 Rad. 0.0° Offs: +0.2 -0.6  
Unknown tau: 1.807 Tsys: 1369. Time: 9.9min El: 77.1  
N: 87 l0: 44.1918 V0: 0.000 Dv: 29.01 LSR  
F0: 473040.879 Df: -45.78 Fi: 461040.768

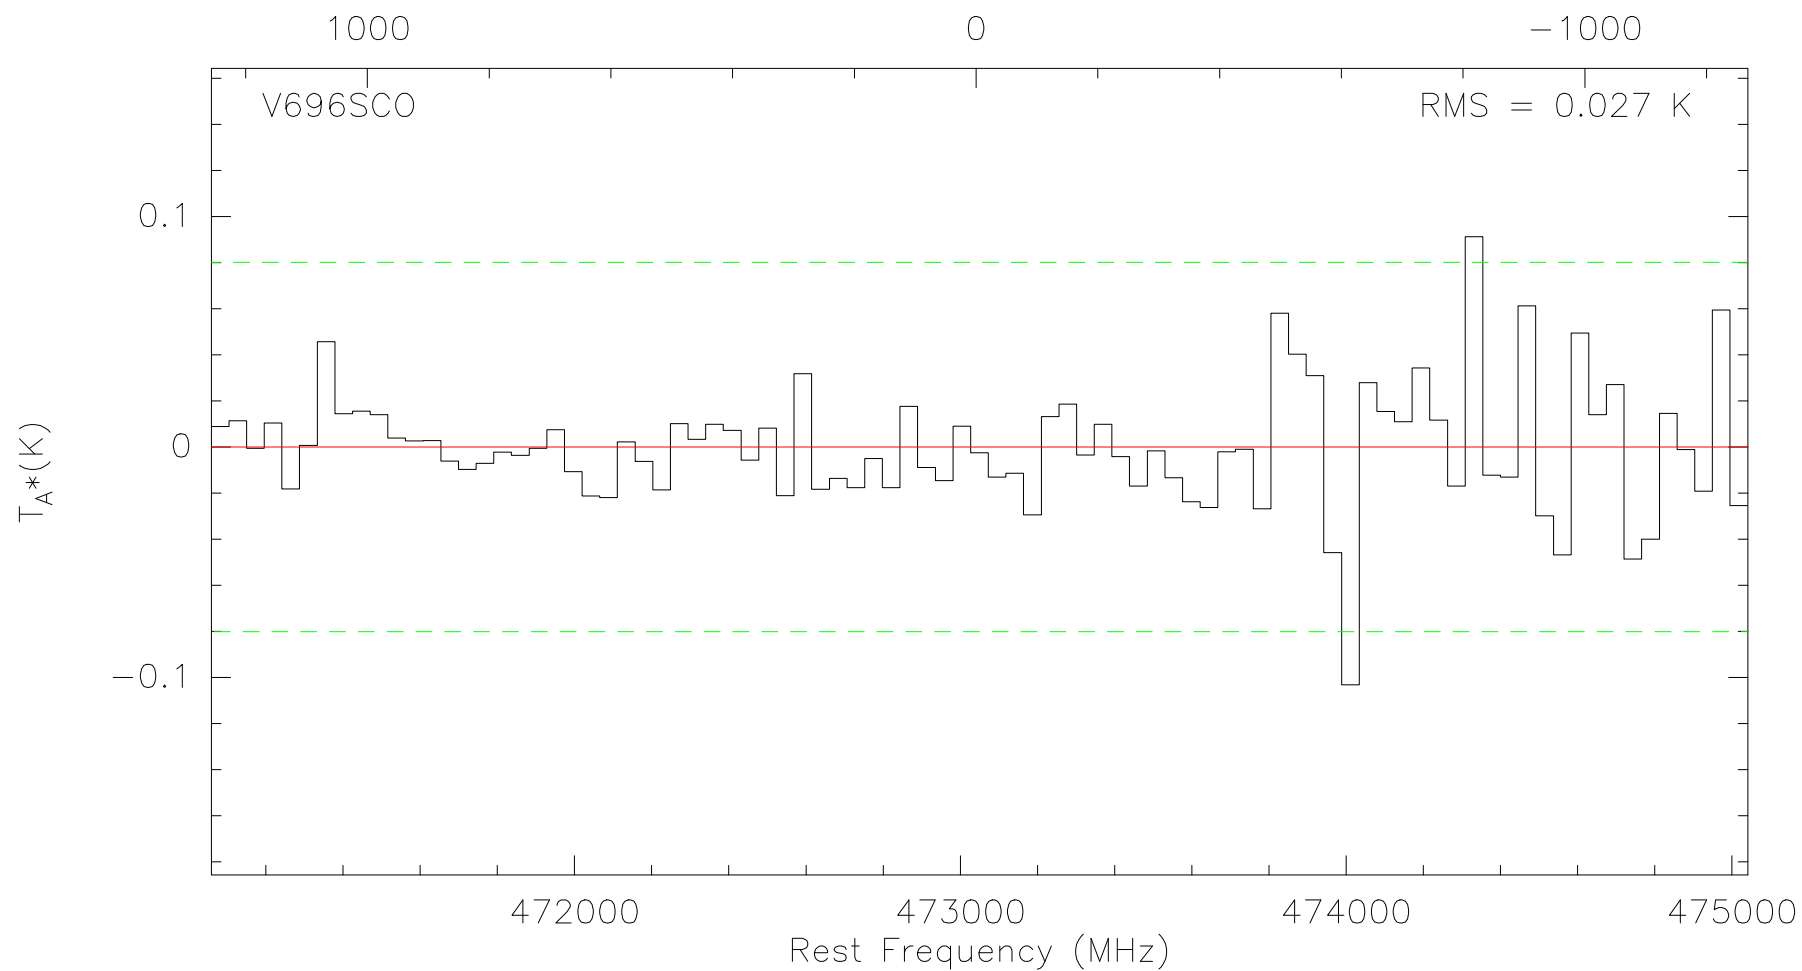

1;1 V697SCO CO(4-3) OSB AP-FL02-XF0- 0:13-JUL-2016 R:07-AUG-2020  
RA: 17:51:21.83 DEC: -37:24:55.2 Eq 2000.0 Rad. 0.0° Offs: -0.2 -0.5  
Unknown tau: 1.435 Tsys: 1696. Time: 14.9min El: 43.3  
N: 87 l0: 44.1919 V0: 0.000 Dv: 29.01 LSR  
F0: 473040.916 Df: -45.78 Fi: 461040.768

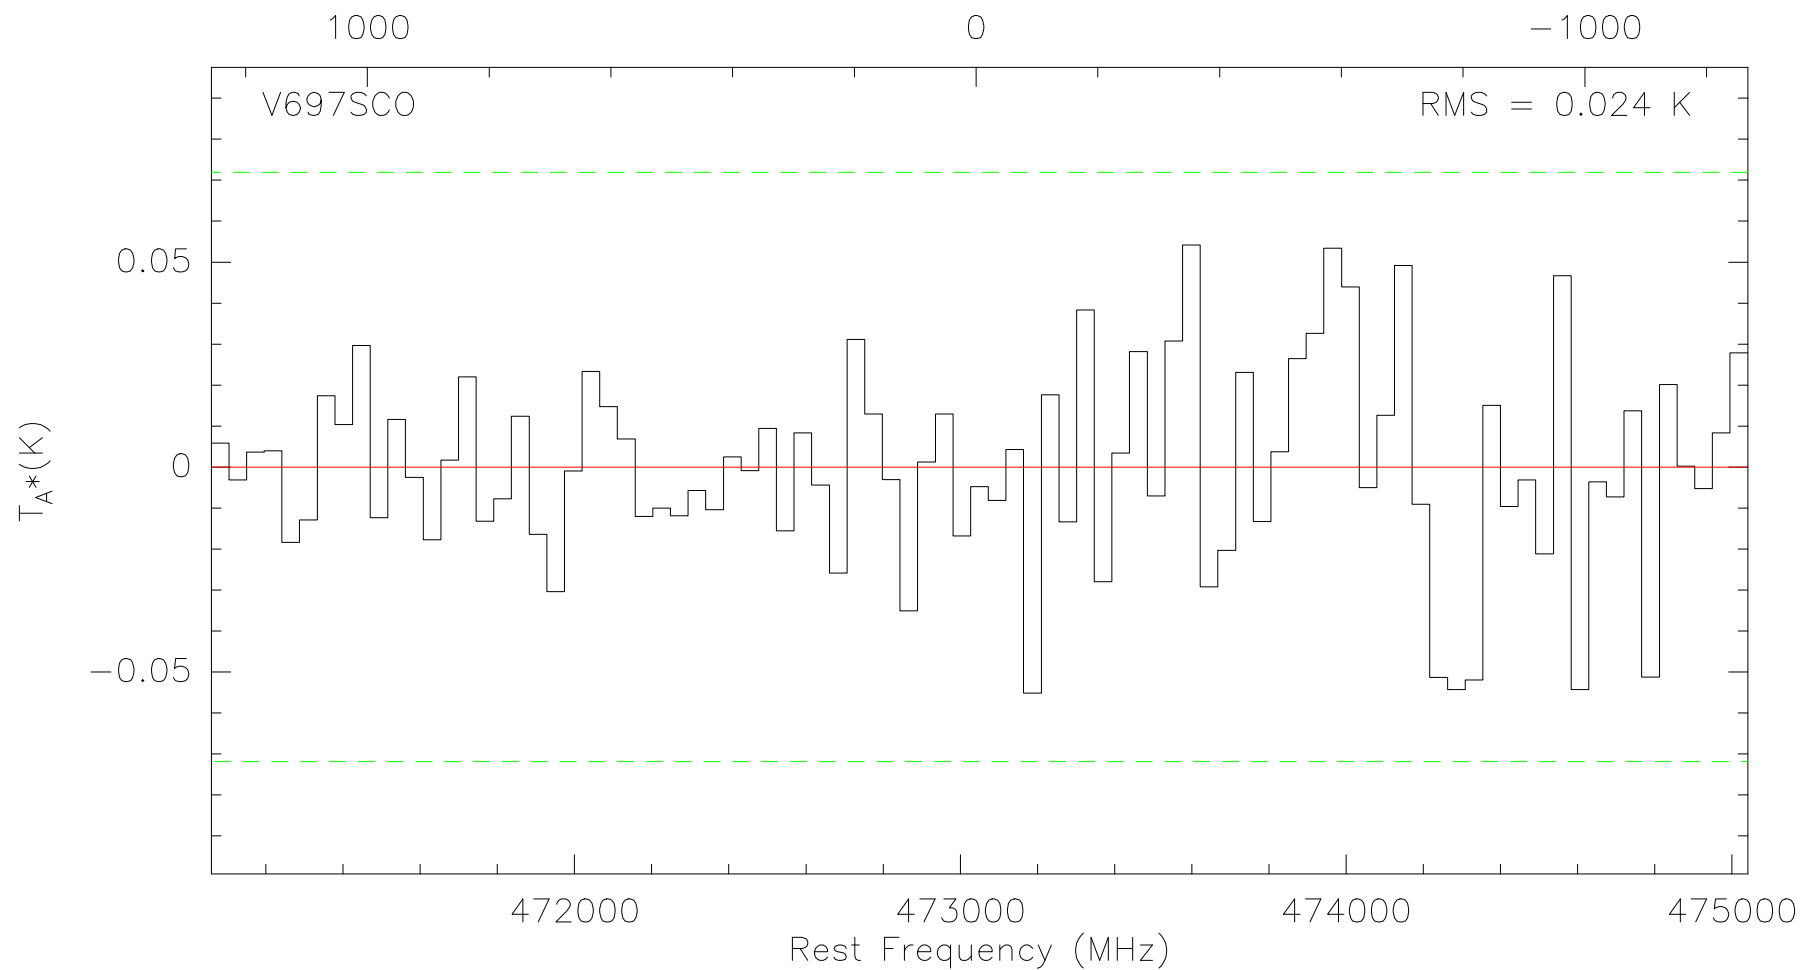

1;1 V707SCO CO(4-3) OSB AP-FL02-XF0- 0:06-JUL-2016 R:07-AUG-2020  
RA: 17:48:26.38 DEC: -36:37:54.9 Eq 2000.0 Rad. 0.0° Offs: +0.3 -0.3  
Unknown tau: 1.878 Tsys: 4159. Time: 9.9min El: 40.0  
N: 87 l0: 44.1918 V0: 0.000 Dv: 29.01 LSR  
F0: 473040.784 Df: -45.78 Fi: 461040.768

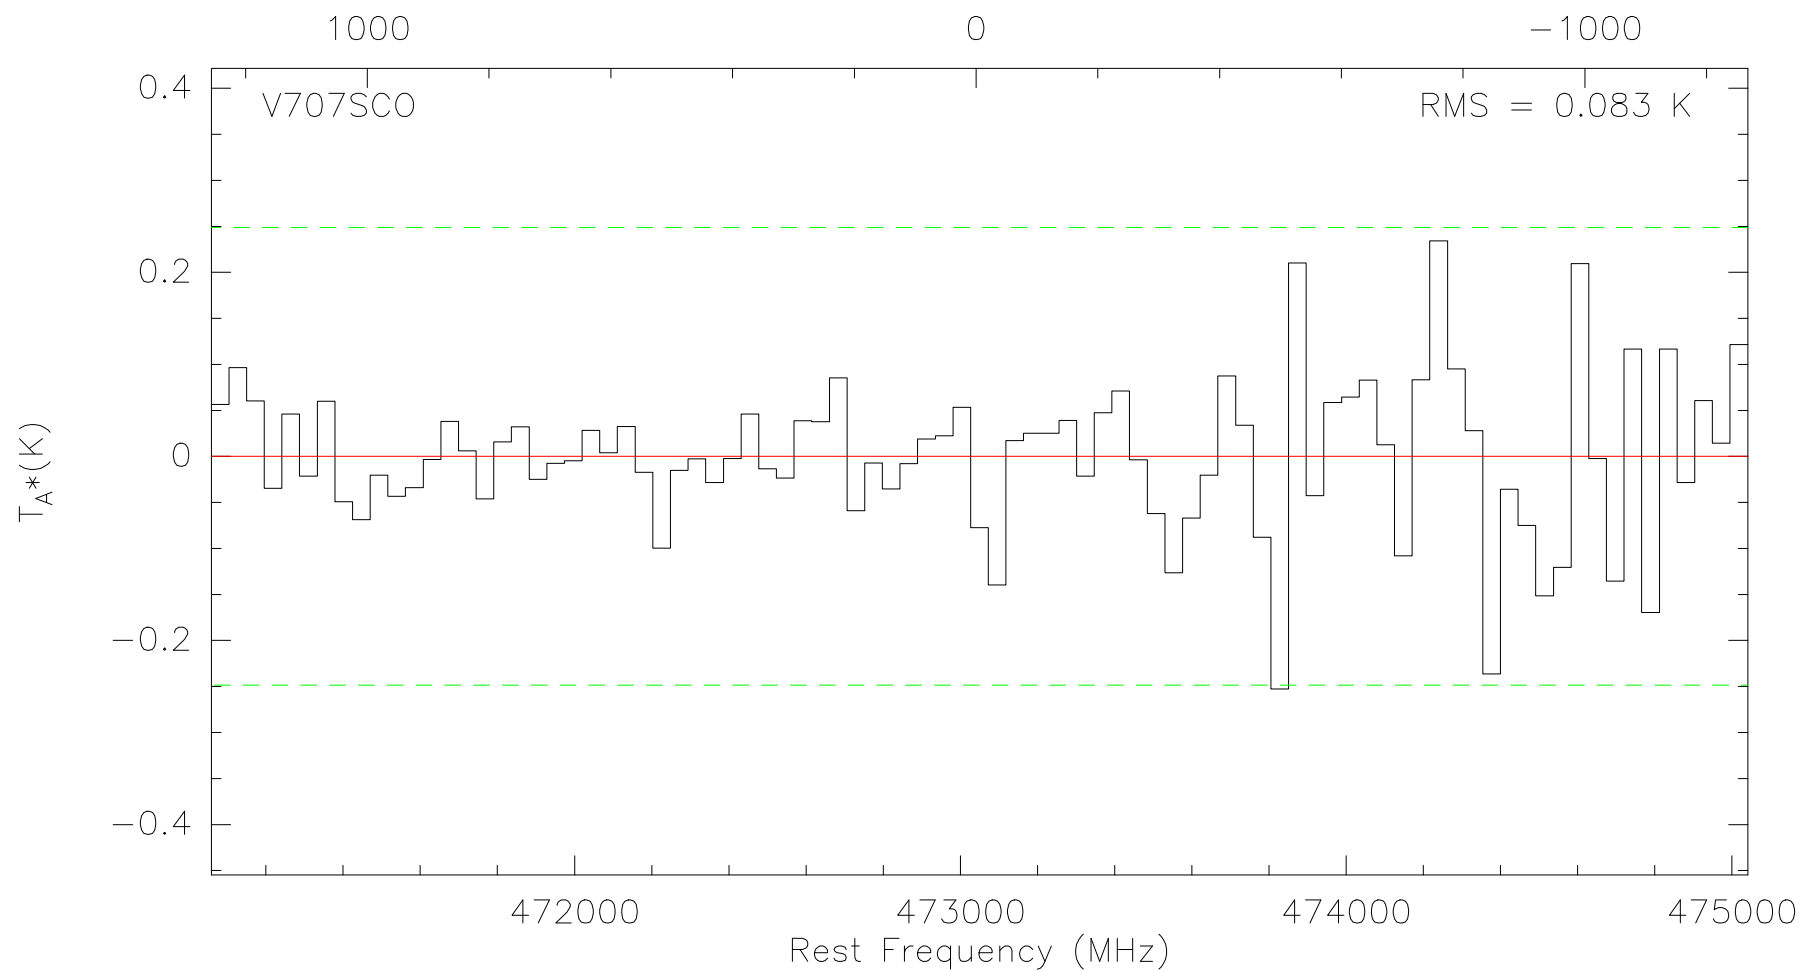

1;1 V711SCO CO(4-3) OSB AP-FL02-XF0- 0:14-JUL-2016 R:07-AUG-2020  
RA: 17:54:06.16 DEC: -34:21:15.5 Eq 2000.0 Rad. 0.0° Offs: +0.3 -0.3  
Unknown tau: 2.196 Tsys: 2835. Time: 9.9min El: 58.0  
N: 87 l0: 44.1918 V0: 0.000 Dv: 29.01 LSR  
F0: 473040.867 Df: -45.78 Fi: 461040.768

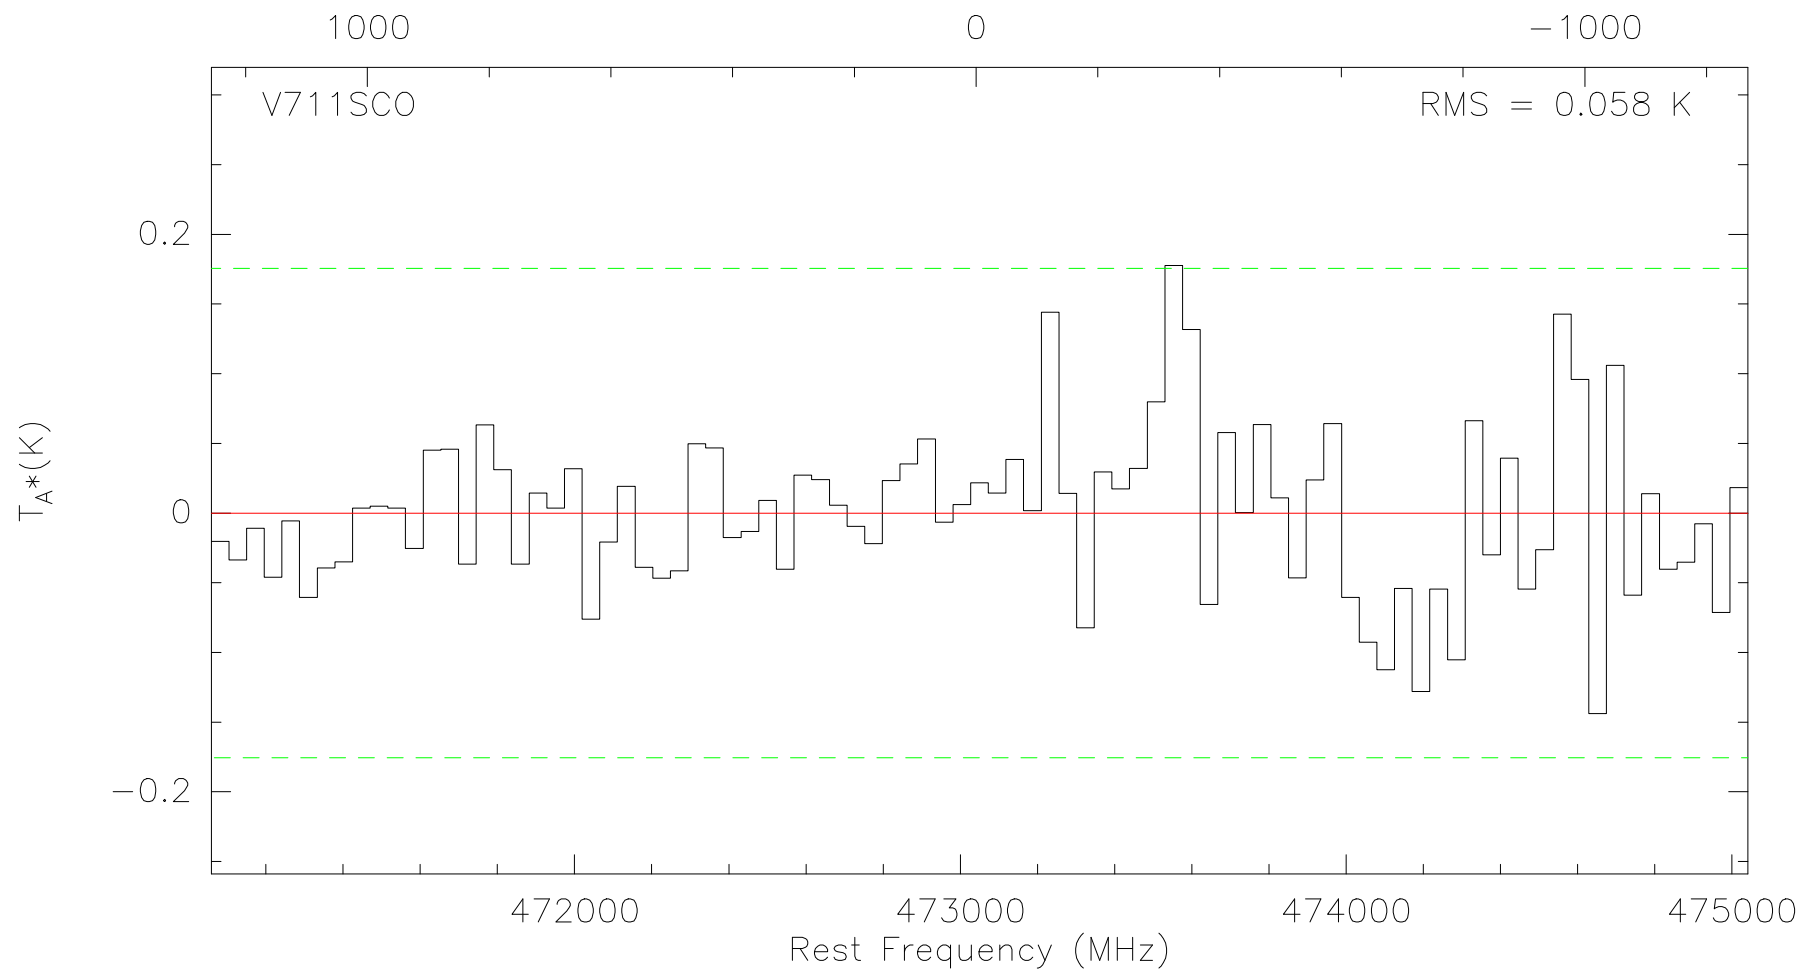

1;1 V729SCO CO(4-3) OSB AP-FL02-XF0- 0:01-JUL-2016 R:07-AUG-2020  
RA: 17:22:02.66 DEC: -32:05:48.8 Eq 2000.0 Rad. 0.0° Offs: -0.2 -0.5  
Unknown tau: 2.242 Tsys: 12721. Time: 14.9min El: 30.0  
N: 87 l0: 44.1918 V0: 0.000 Dv: 29.01 LSR  
F0: 473040.769 Df: -45.78 Fi: 461040.768

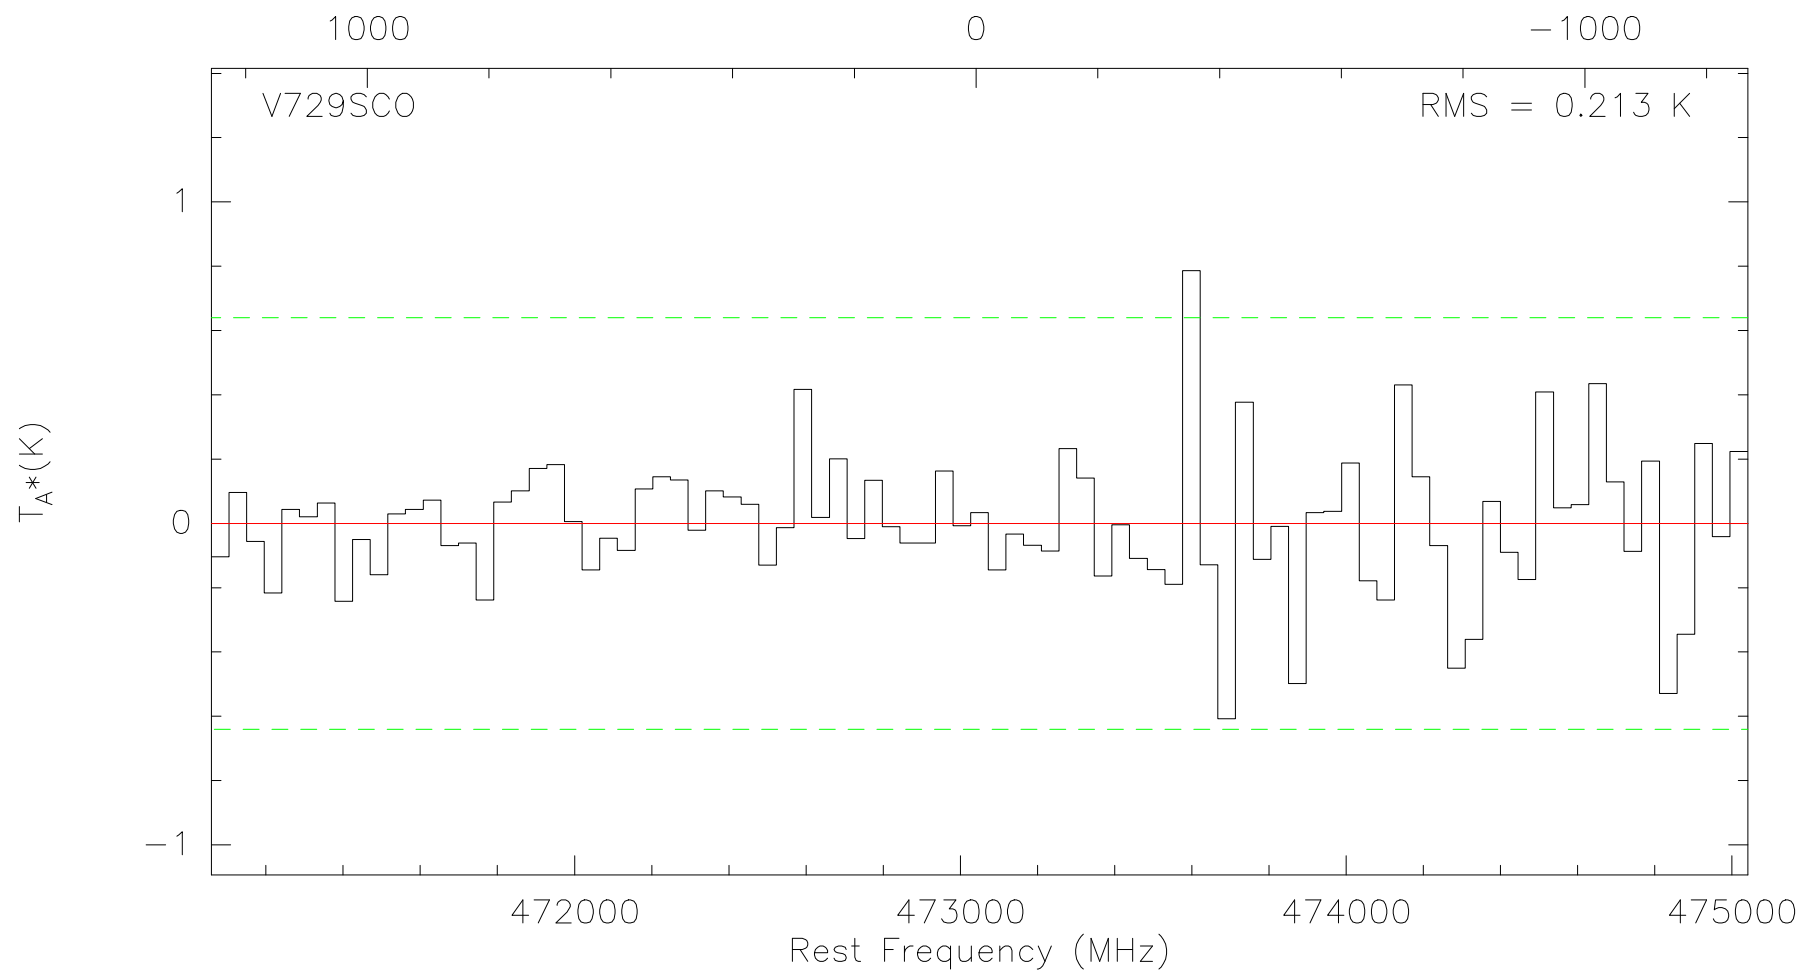

1;1 V732SGR CO(4-3) OSB AP-FL02-XF0- 0:13-JUL-2016 R:07-AUG-2020  
RA: 17:56:07.51 DEC: -27:22:16.1 Eq 2000.0 Rad. 0.0° Offs: +0.2 -0.4  
Unknown tau: 1.979 Tsys: 1747. Time: 9.9min El: 71.8  
N: 87 l0: 44.1918 V0: 0.000 Dv: 29.01 LSR  
F0: 473040.767 Df: -45.78 Fi: 461040.768

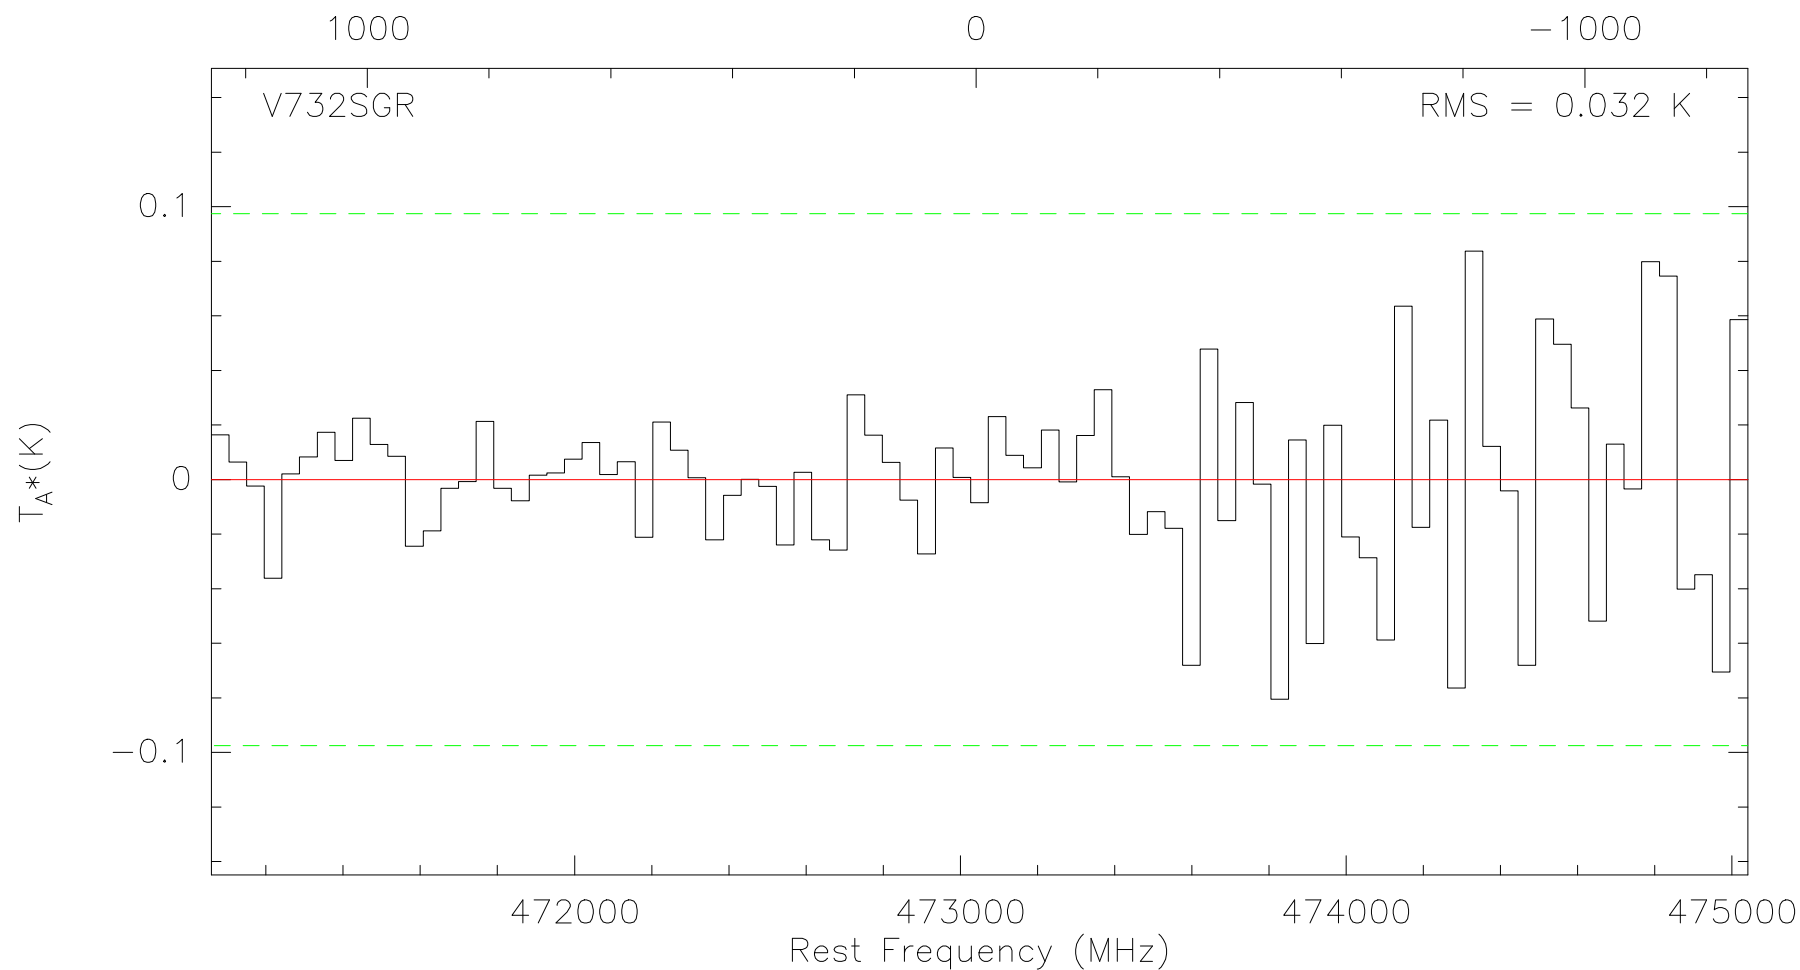

1;1 V733SCO CO(4-3) OSB AP-FL02-XF0- 0:06-JUL-2016 R:07-AUG-2020  
RA: 17:39:42.88 DEC: -35:52:38.4 Eq 2000.0 Rad. 0.0° Offs: +0.3 -0.3  
Unknown tau: 1.763 Tsys: 4182. Time: 9.9min El: 37.6  
N: 87 l0: 44.1918 V0: 0.000 Dv: 29.01 LSR  
F0: 473040.811 Df: -45.78 Fi: 461040.768

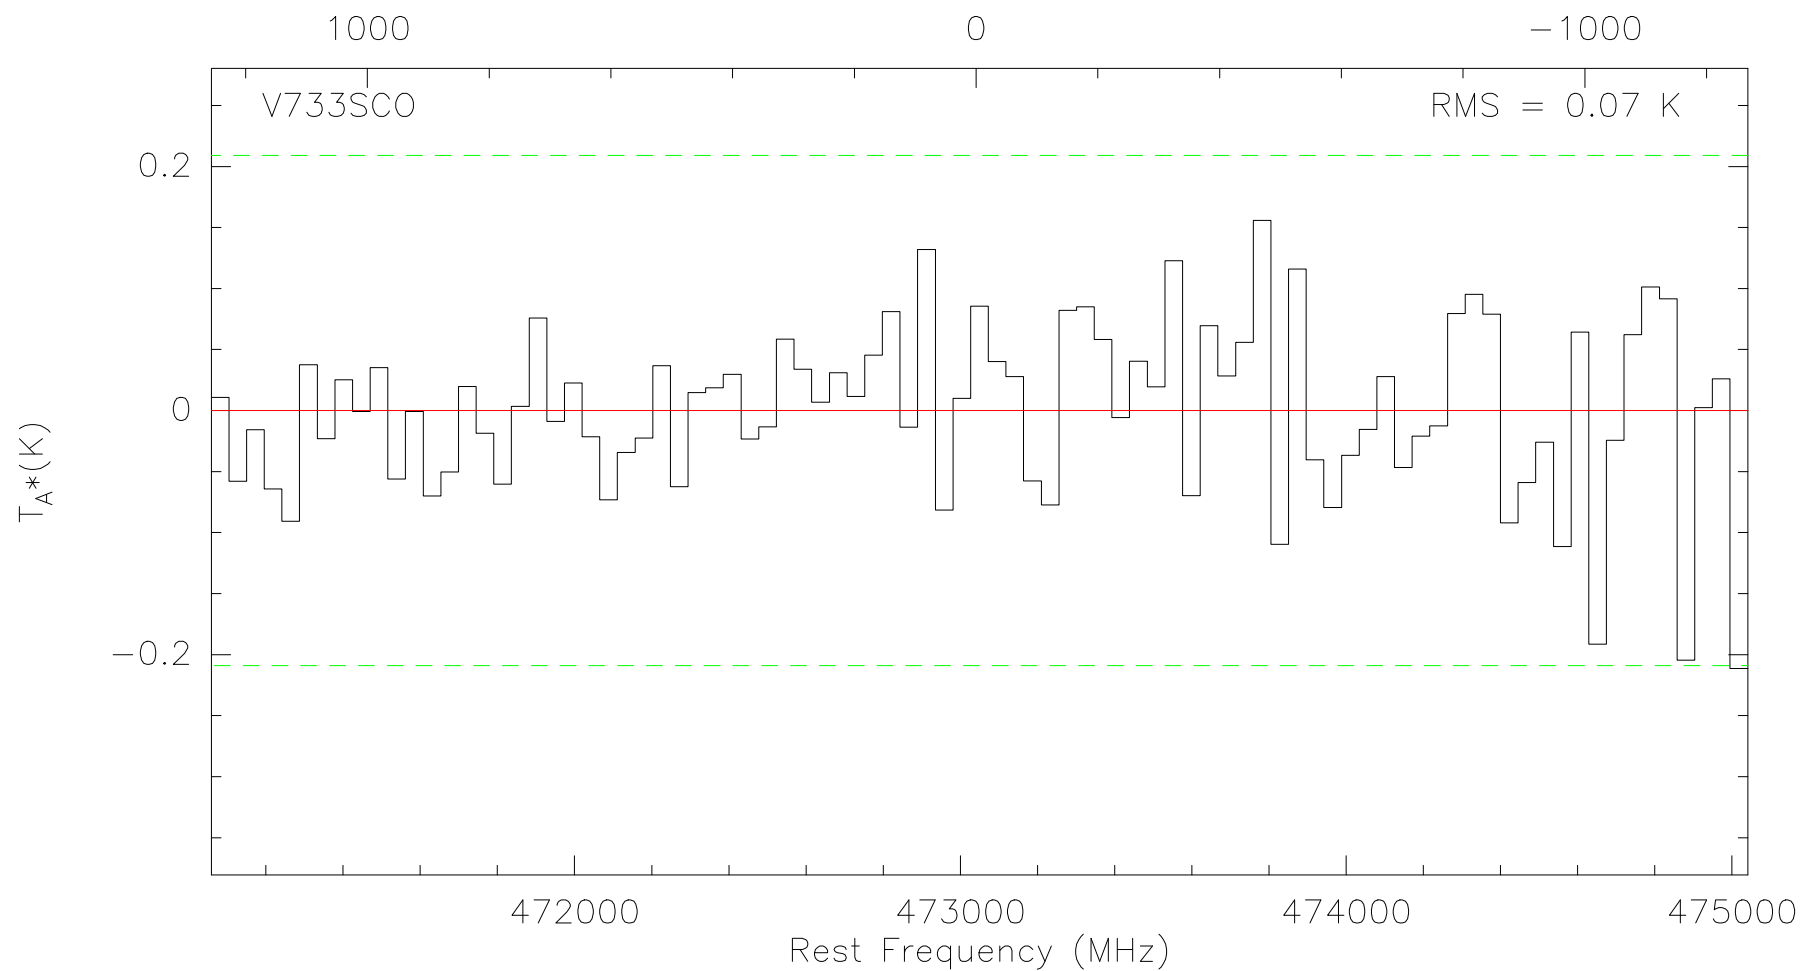

1;1 V737SGR CO(4-3) OSB AP-FL02-XF0- O:14-JUL-2016 R:07-AUG-2020  
RA: 18:07:08.66 DEC: -28:44:52.3 Eq 2000.0 Rad. 0.0° Offs: +0.2 -0.4  
Unknown tau: 2.115 Tsys: 2116. Time: 9.9min El: 70.3  
N: 87 l0: 44.1918 V0: 0.000 Dv: 29.01 LSR  
F0: 473040.755 Df: -45.78 Fi: 461040.768

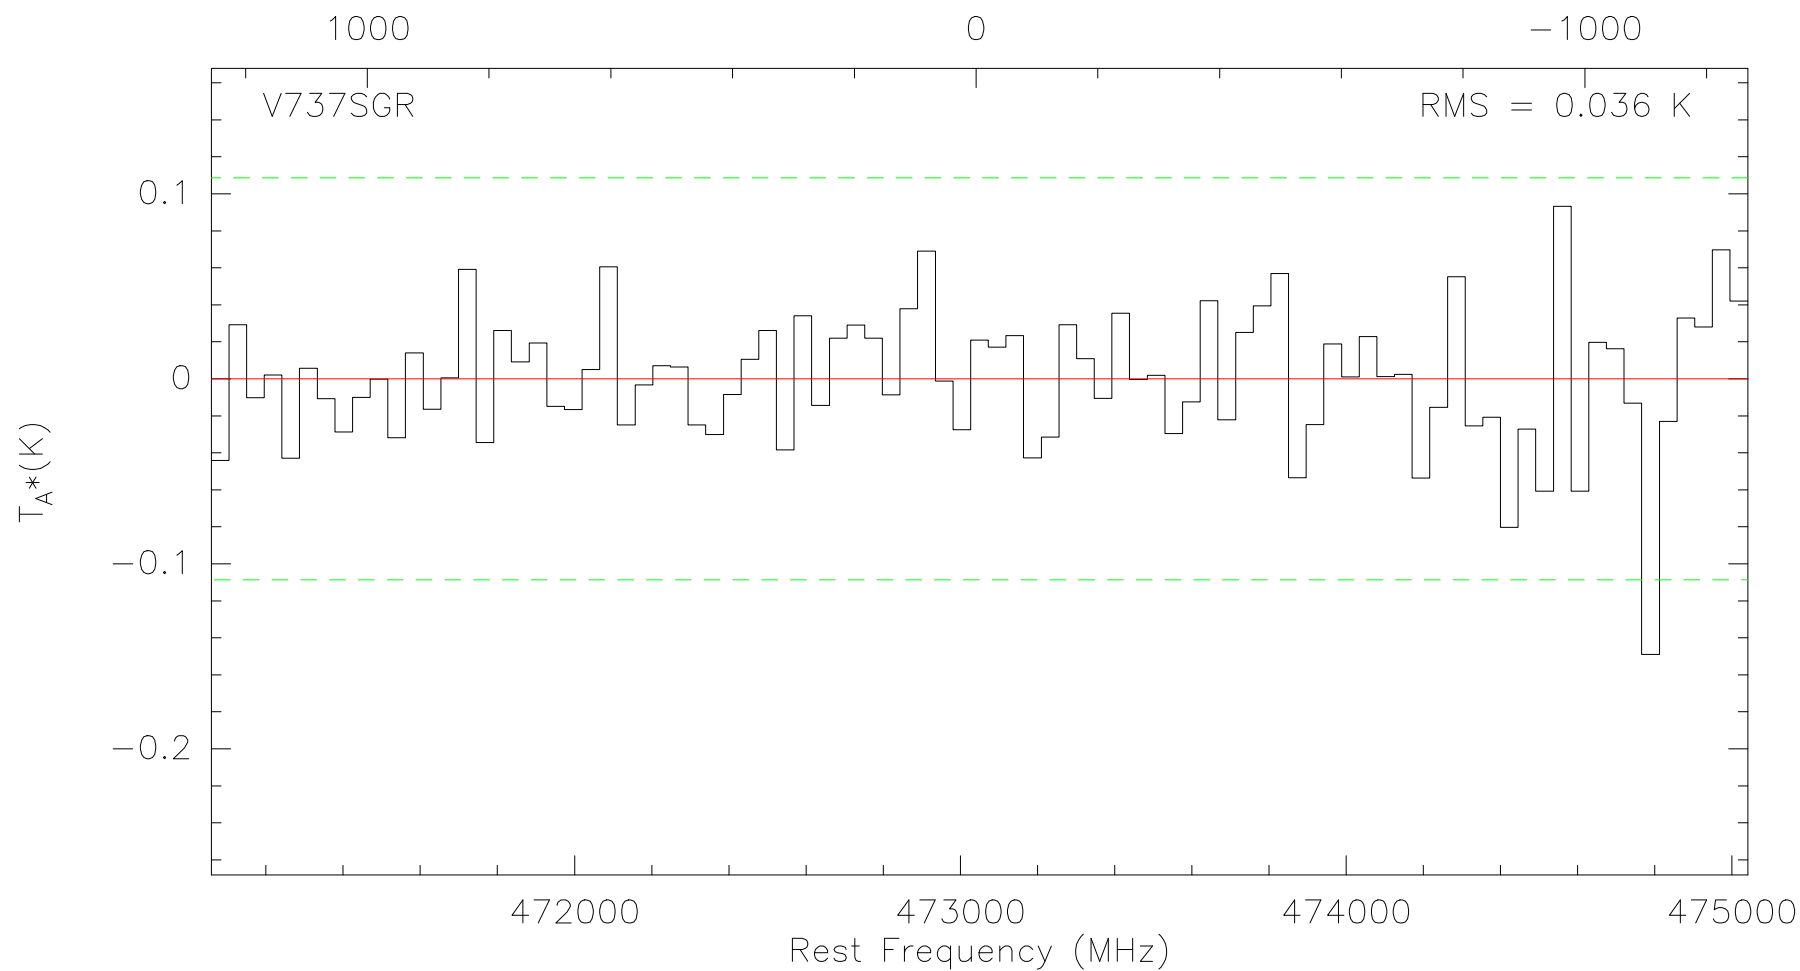

1;1 V745SCO CO(4-3) OSB AP-FL02-XF0- 0:13-JUL-2016 R:07-AUG-2020  
RA: 17:55:22.27 DEC: -33:14:58.5 Eq 2000.0 Rad. 0.0° Offs: +0.0 -0.7  
Unknown tau: 1.610 Tsys: 1156. Time: 9.9min El: 77.6  
N: 87 l0: 44.1918 V0: 0.000 Dv: 29.01 LSR  
F0: 473040.844 Df: -45.78 Fi: 461040.768

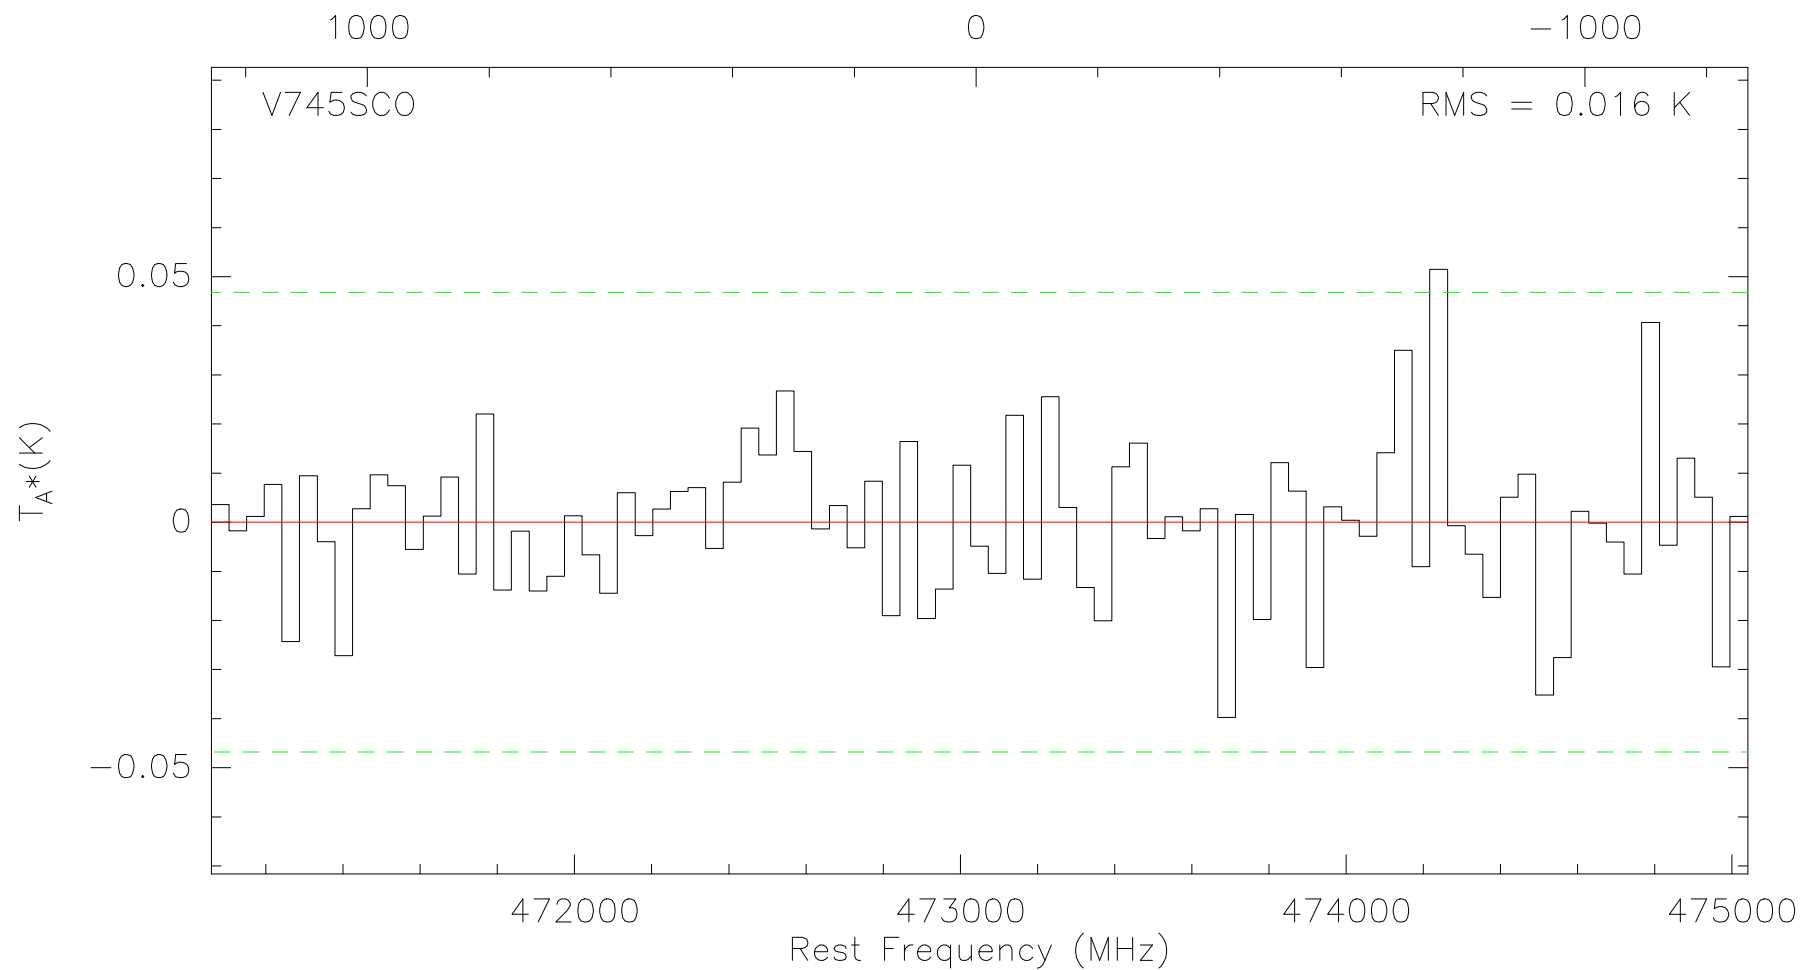

1;1 V787SGR CO(4-3) OSB AP-FL02-XF0- 0:14-JUL-2016 R:07-AUG-2020  
RA: 18:00:02.20 DEC: -30:30:31.0 Eq 2000.0 Rad. 0.0° Offs: +0.2 -0.3  
Unknown tau: 2.266 Tsys: 2716. Time: 9.9min El: 62.7  
N: 87 l0: 44.1918 V0: 0.000 Dv: 29.01 LSR  
FO: 473040.802 Df: -45.78 Fi: 461040.768

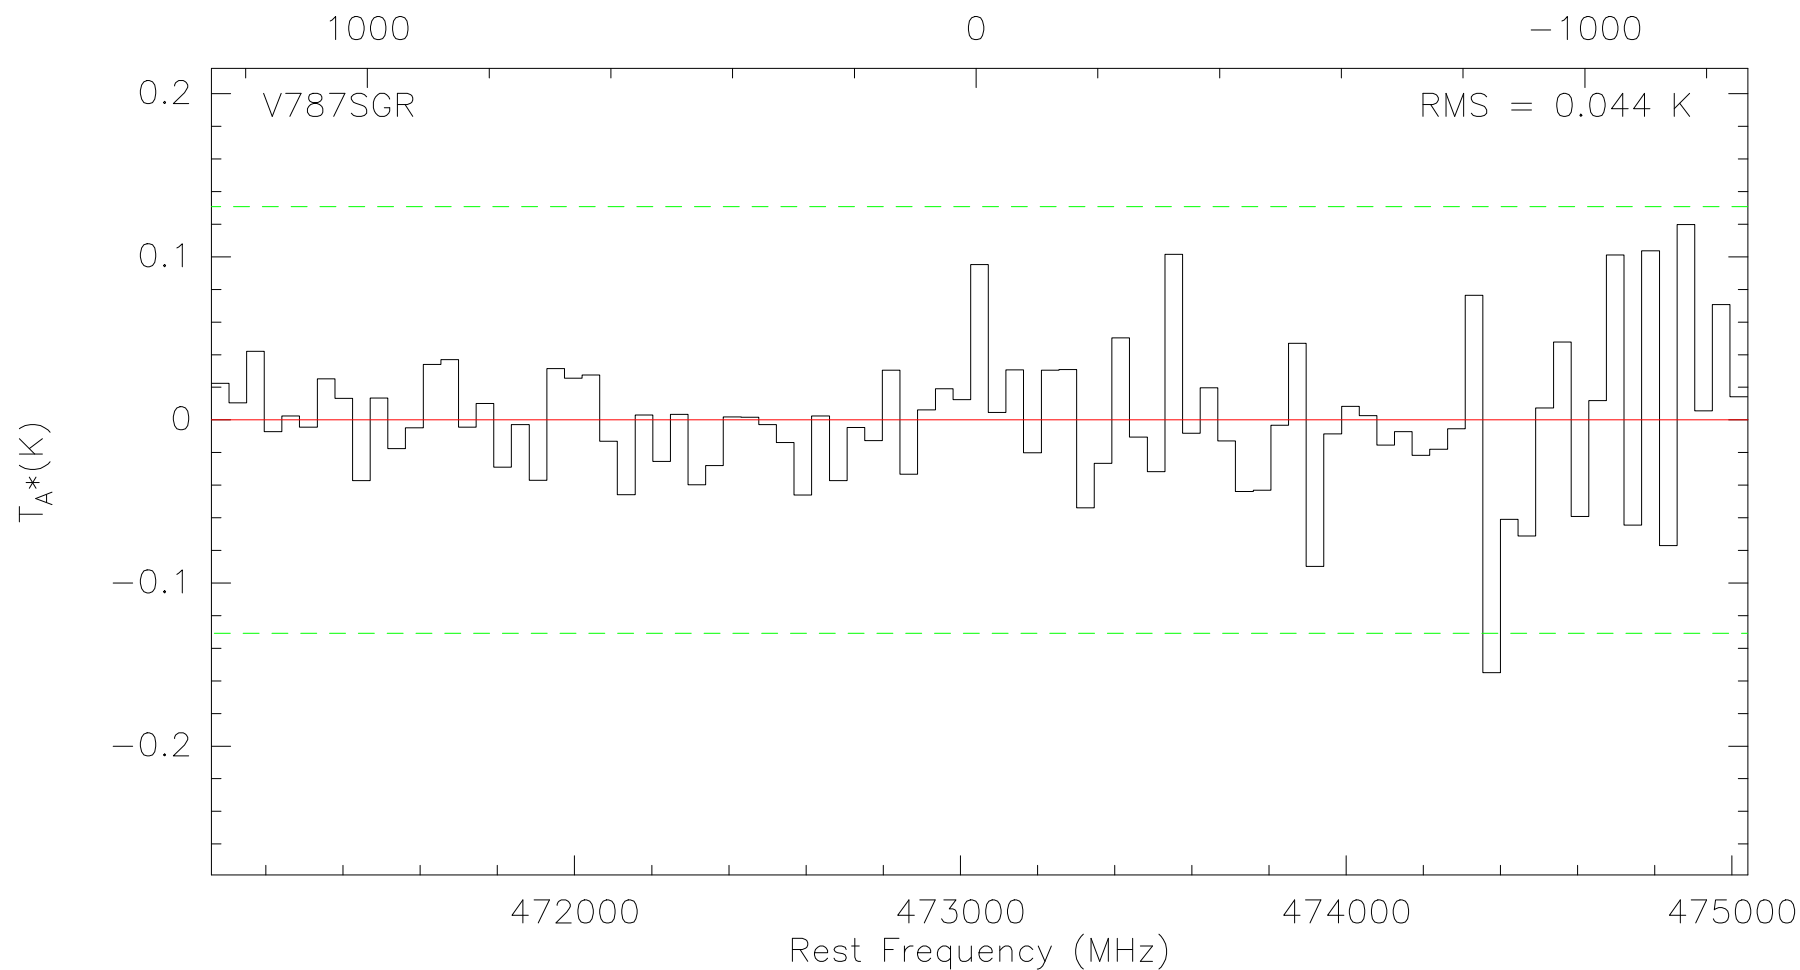

1;1 V7940PH CO(4-3) OSB AP-FL02-XF0- 0:01-JUL-2016 R:07-AUG-2020  
RA: 17:38:49.25 DEC: -22:50:48.9 Eq 2000.0 Rad. 0.0° Offs: -0.2 -0.5  
Unknown tau: 2.642 Tsys: 9661. Time: 9.9min El: 42.1  
N: 87 l0: 44.1918 V0: 0.000 Dv: 29.01 LSR  
F0: 473040.593 Df: -45.78 Fi: 461040.768

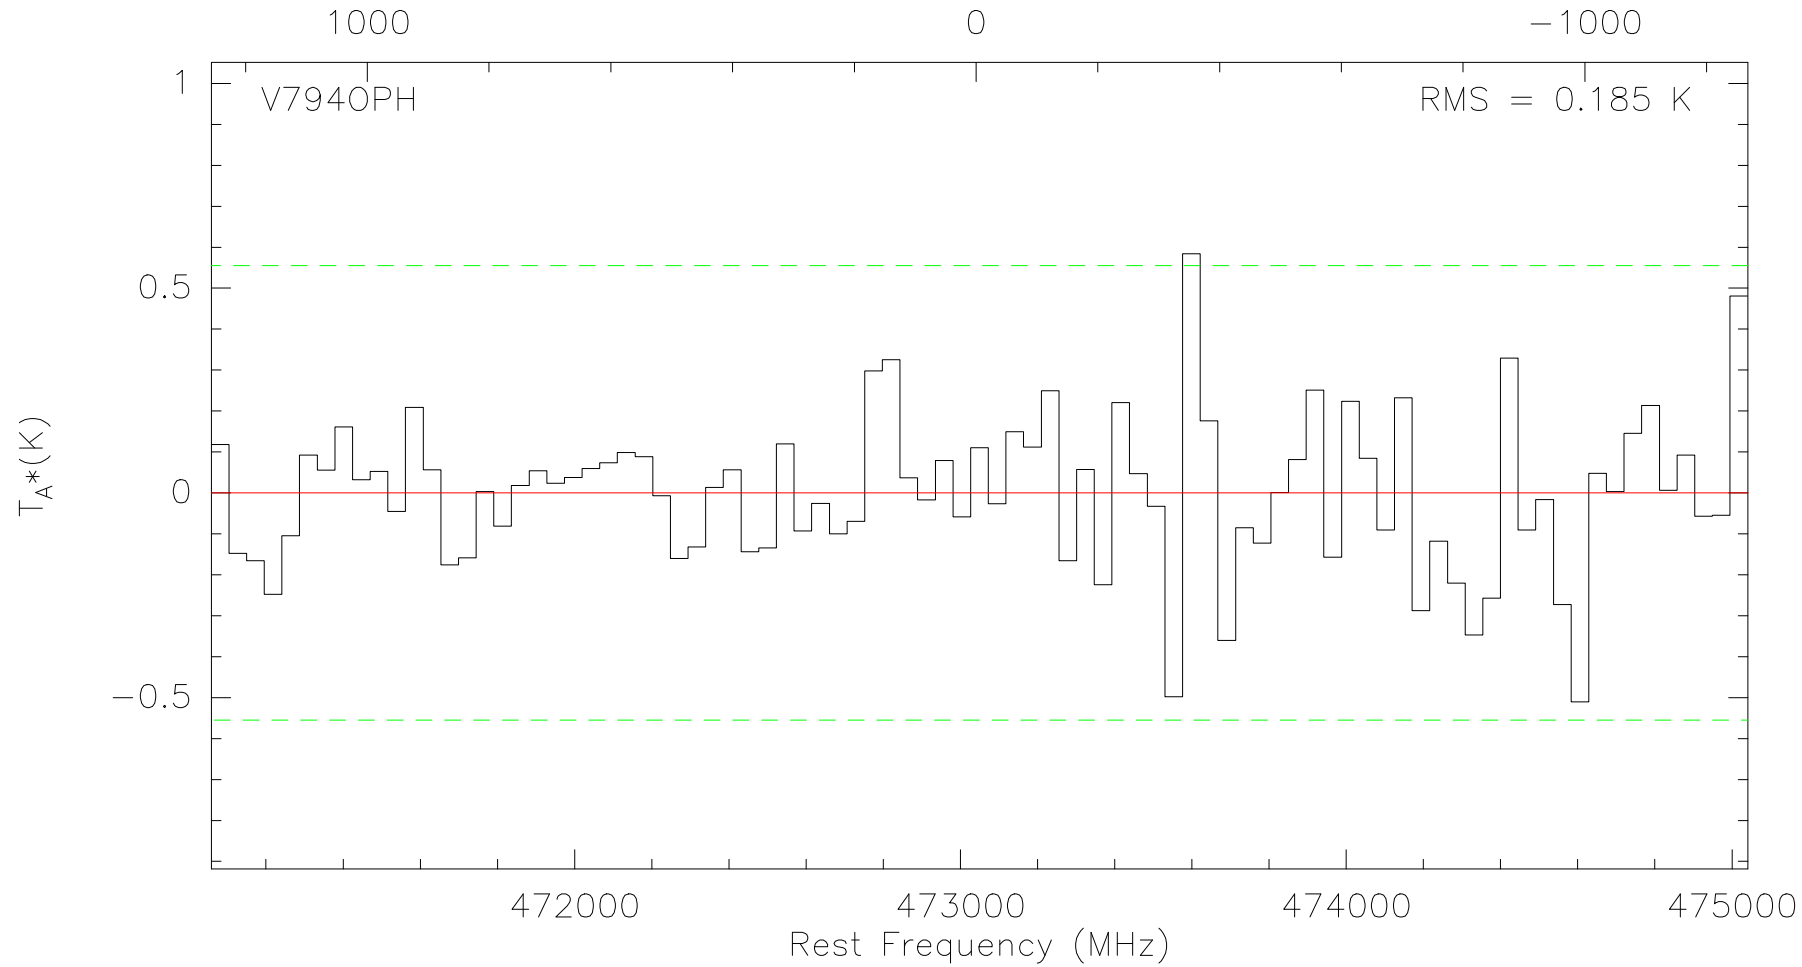

1;1 V909SGR CO(4-3) OSB AP-FL02-XF0- 0:13-JUL-2016 R:07-AUG-2020  
RA: 18:25:52.30 DEC: -35:01:27.0 Eq 2000.0 Rad. 0.0° Offs: +0.2 -0.4  
Unknown tau: 1.939 Tsys: 1826. Time: 9.9min El: 67.4  
N: 87 l0: 44.1918 V0: 0.000 Dv: 29.01 LSR  
F0: 473040.737 Df: -45.78 Fi: 461040.768

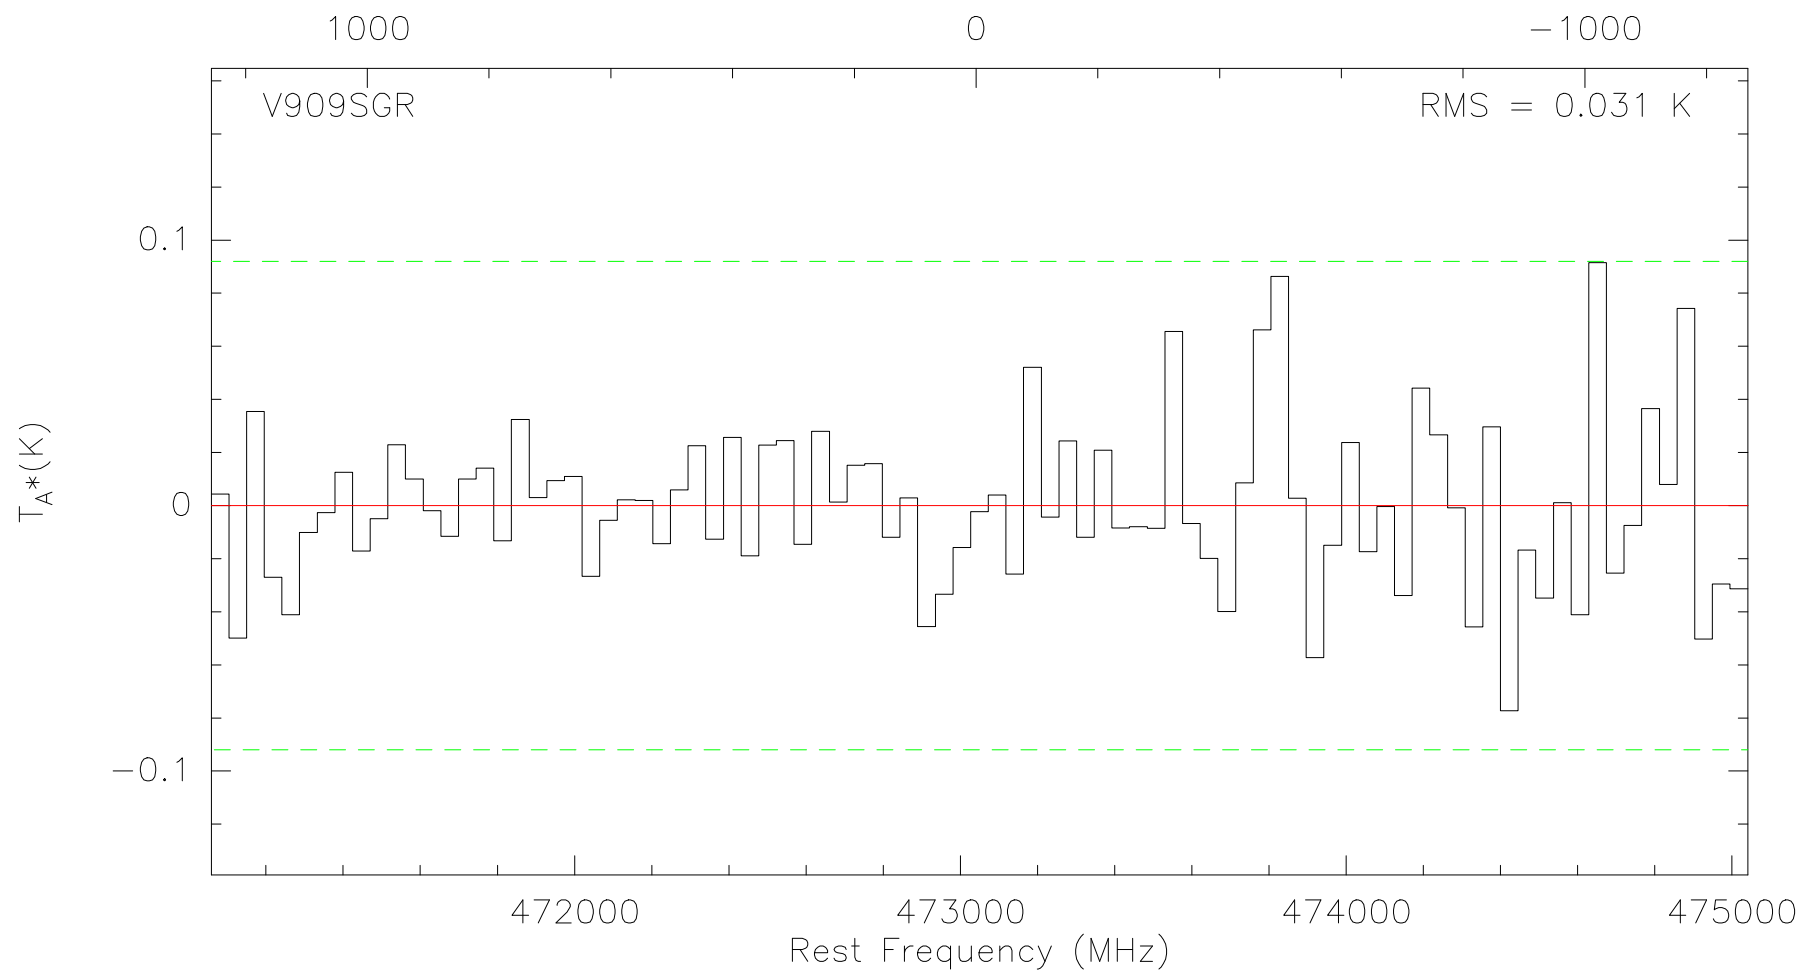

1;1 V941SGR CO(4-3) OSB AP-FL02-XF0- 0:13-JUL-2016 R:07-AUG-2020

RA: 18:34:43.46 DEC: -29:34:49.1 Eq 2000.0 Rad. 0.0° Offs: -0.2 -0.3

Unknown tau: 1.208 Tsys: 2817. Time: 9.9min El: 25.8

N: 87 l0: 44.1918 V0: 0.000 Dv: 29.01 LSR

F0: 473040.659 Df: -45.78 Fi: 461040.768

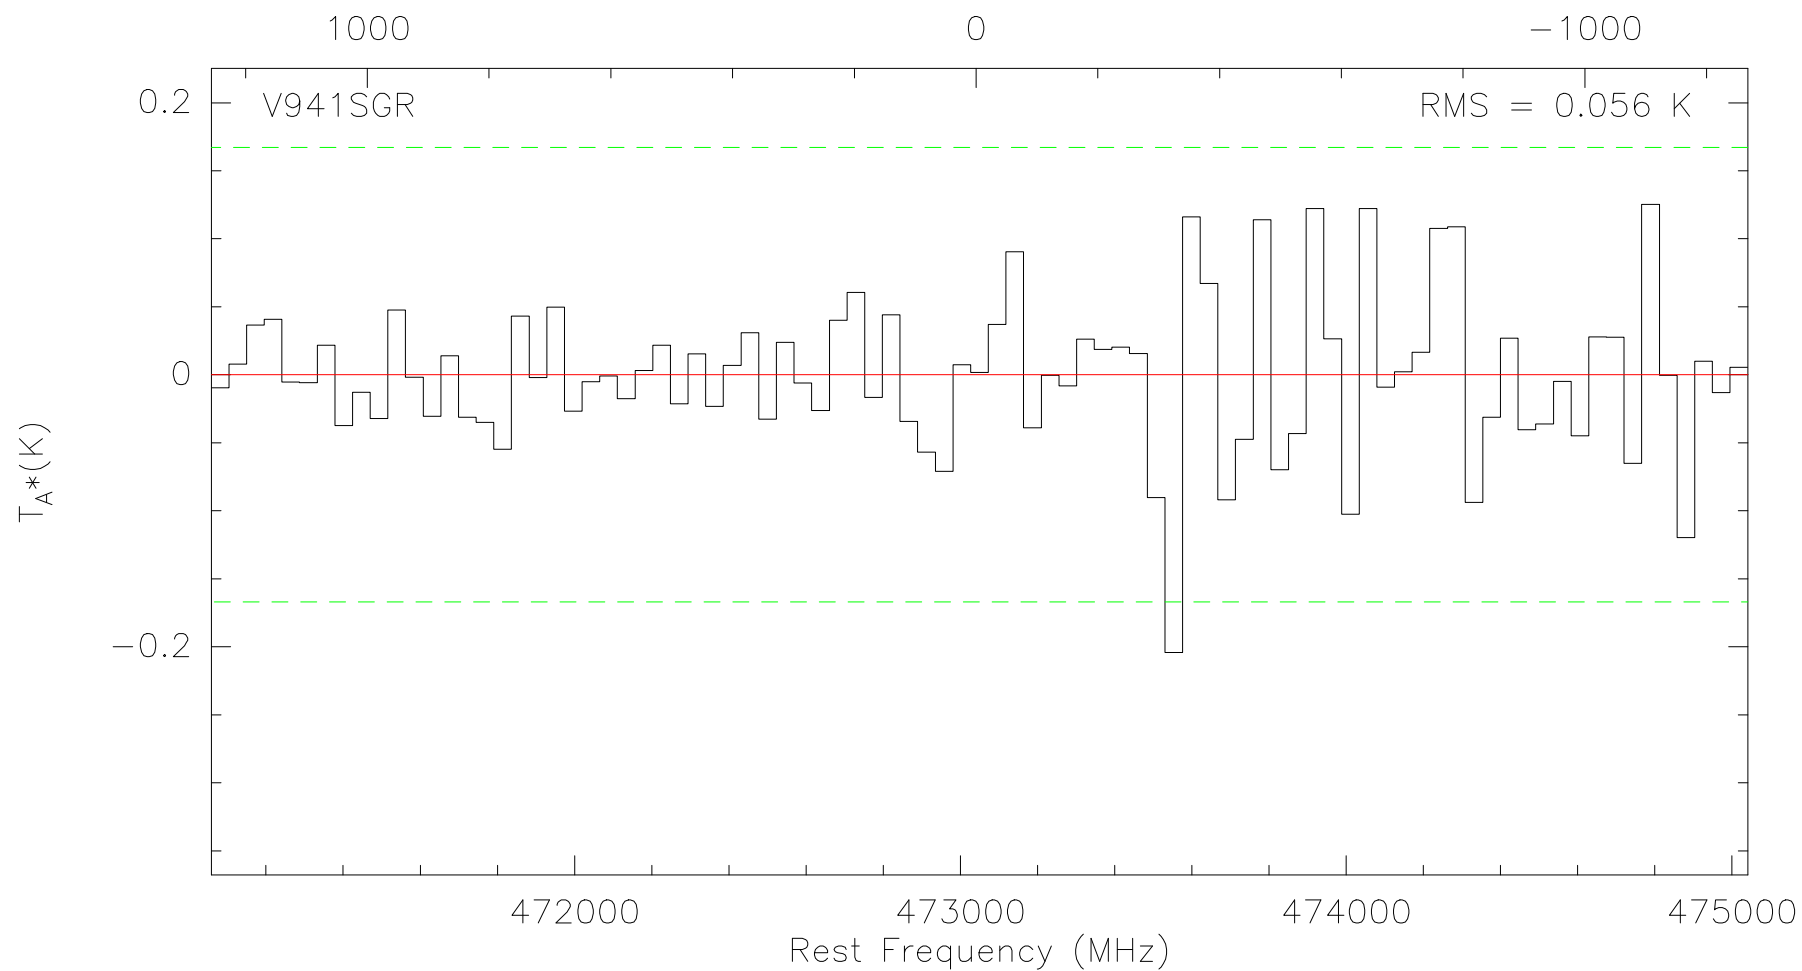

1;1 V999SGR CO(4-3) OSB AP-FL02-XF0- 0:13-JUL-2016 R:07-AUG-2020  
RA: 18:00:05.59 DEC: -27:33:14.0 Eq 2000.0 Rad. 0.0° Offs: -0.2 -0.4  
Unknown tau: 1.416 Tsys: 1833. Time: 9.9min El: 38.9  
N: 87 l0: 44.1918 V0: 0.000 Dv: 29.01 LSR  
F0: 473040.775 Df: -45.78 Fi: 461040.768

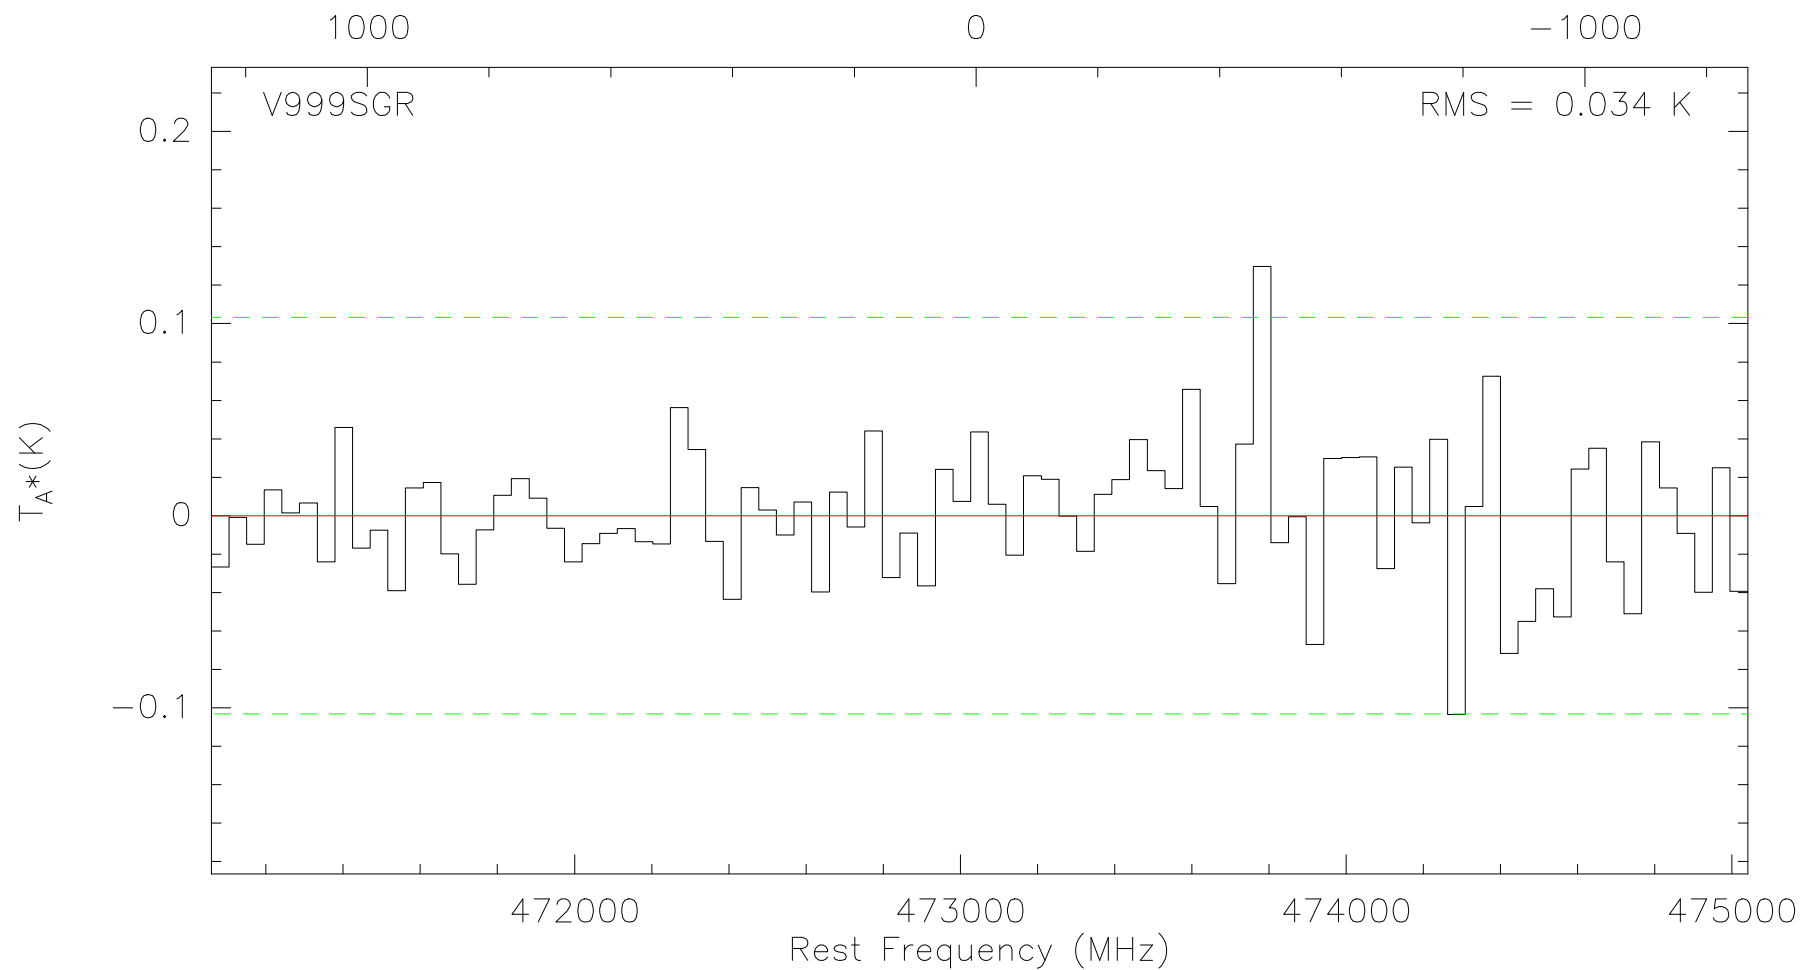

1;1 V1148-SGR CO(4-3) OSB AP-FL02-XF0- O:03-JUN-2015 R:13-AUG-2020

RA: 18:09:05.85 DEC: -25:59:08.0 Eq 2000.0 Rad. 0.0° Offs: +0.2 -0.4

Unknown tau: 1.807 Tsys: 1163. Time: 44.6min El: 48.5

N: 87 l0: 44.2089 V0: 0.000 Dv: 29.01 LSR

F0: 473039.145 Df: -45.77 Fi: 461040.768

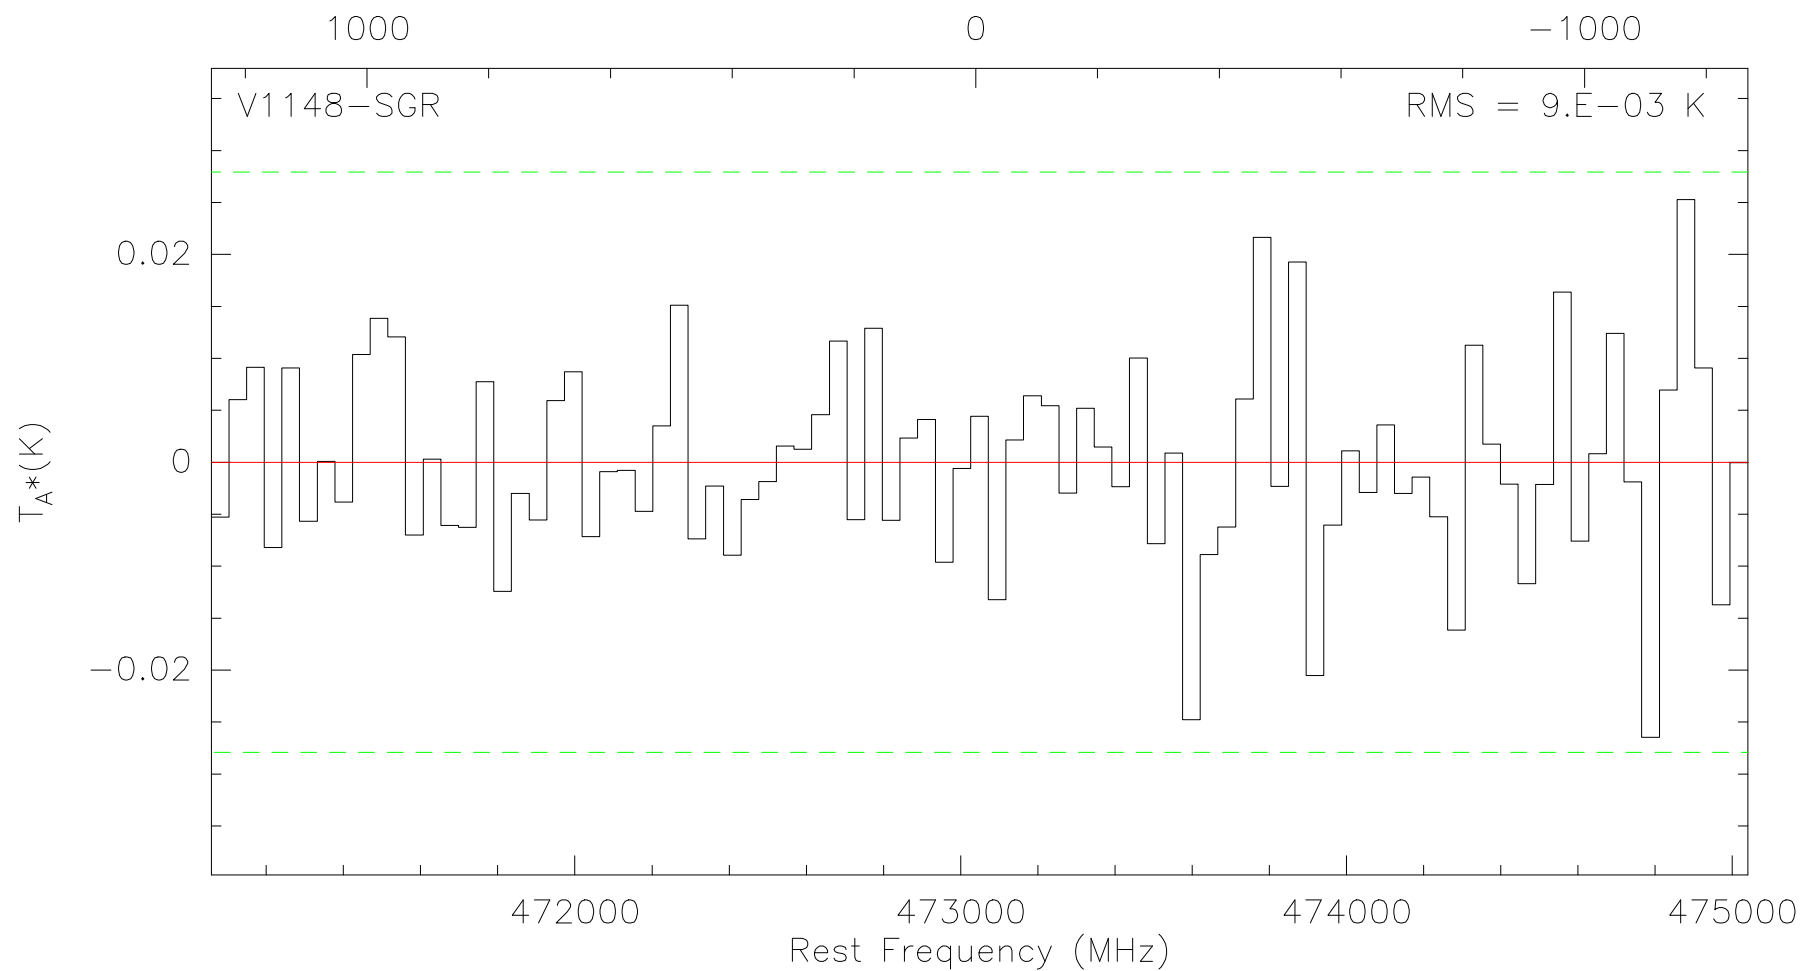

Supplement: Supplementary file 4 [file all_sm_CO43_OSB.pdf]
